# Supplementary material for: Understanding Structural Representation in Foundation Models for Polymers
Source: arXiv:2512.11881 source file (2026-09-18)
Supplement: Supplementary file 1 [file supplementary_information.tex]

\documentclass[pdflatex,sn-nature]{sn-jnl}% Style for submissions to Nature Portfolio journals

%%%% Standard Packages
%%<additional latex packages if required can be included here>
\usepackage{graphicx}%
\graphicspath{{./}{./egc/}{./egb/}{./ei/}{./eps/}{./eea/}{./nc/}{./xc/}{./acs_ami_tg/}{./eat/}{./netl_co2/}{./netl_n2/}{./netl_ch4/}{./netl_co2_ch4/}{./netl_co2_n2/}}
\usepackage{multirow}%
\usepackage{amsmath,amssymb,amsfonts}%
\usepackage{amsthm}%
\usepackage{mathrsfs}%
\usepackage[title]{appendix}%
\usepackage{xcolor}%
\usepackage{textcomp}%
\usepackage{manyfoot}%
\usepackage{booktabs}%
\usepackage{algorithm}%
\usepackage{algorithmicx}%
\usepackage{algpseudocode}%
\usepackage{listings}%
\usepackage{titlesec}
\usepackage{titletoc}

\begin{document}

\title[Understanding Structural Representation in Foundation Models for Polymers]{Understanding Structural Representation in Foundation Models for Polymers}

\author*[1]{\fnm{Nathaniel H.} \sur{Park}}\email{npark@us.ibm.com}

\author[2]{\fnm{Eduardo} \sur{Soares}}\email{eduardo.soares@ibm.com}

\author[2]{\fnm{Victor} \sur{Shirasuna}}\email{vshirasuna@ibm.com}

\author[1]{\fnm{Tiffany J.} \sur{Callahan}}\email{tiffany.callahan@ibm.com}

\author[1]{\fnm{Sara} \sur{Capponi}}\email{sara.capponi@ibm.com}

\author[2]{\fnm{Emilio Vital} \sur{Brazil}}\email{evital@br.ibm.com}

\affil*[1]{\orgname{IBM Research Almaden}, \orgaddress{\street{650 Harry Rd.}, \city{San Jose}, \postcode{95120}, \state{CA}, \country{United States of America}}}

\affil[2]{\orgname{IBM Research Brazil}, \orgaddress{\street{Street}, \city{Rio de Janeiro}, \postcode{10587}, \state{RJ}, \country{Brazil}}}

\maketitle

\tableofcontents

\newpage

\section{Supplemental Methods}

\subsection{Representation Experiments}\label{rep_exp_section}

\paragraph{Atom Replacement Methods}As noted in the main text, we utilized three different approaches to transform the CPG representation into other SMILES strings, including PSMILES. The transformation was performed from benchmark data which had been converted into the CPG representation as opposed to the original data in order to ensure identical sequences of tokens for each entity were maintained. During conversion to the CPG notation, the SMILES strings had been canonicalized using RDKit, which resulted in new ordering in the SMILES strings as compared to the original data. The three replacement methods are:

\begin{itemize}
    \item \textit{All} – which replaces all characters including the brackets.
    \item \textit{Bracket} – which replaces all characters inside the brackets.
    \item \textit{Star} – which replaces only the asterisk character.
\end{itemize}

Following substitution, a separate copy of the converted dataset was canonicalized again for comparison, as some atom substitutions resulted in different canonical atom orders than the original.

\paragraph{Replacement Atoms}Below is a list of all the replacement atoms, which substitution methods were used, and whether a separate, re-canonicalized dataset was also created.

\begin{table}[hbtp]
\caption{Replacement Atoms for Input Representations}\label{atomtab}
\begin{tabular}{ccc}
\toprule
Atom & Methods & Canonicalization\\
\midrule
\textbf{*} & \textit{All}\footnotemark[1], \textit{Star} & Yes\\
\textbf{*} & \textit{Bracket}\footnotemark[1] & No\footnotemark[2] \\
\textbf{H} & \textit{Bracket} & Yes\footnotemark[3] \\
\textbf{C} & \textit{All}, \textit{Bracket}, \textit{Star} & Yes\\
\textbf{c} & \textit{All}, \textit{Bracket} & No\\
\textbf{N} & \textit{All}, \textit{Bracket} & Yes\\
\textbf{n} & \textit{All} & No\\
\textbf{n\textsuperscript{+}} & \textit{Bracket} & No\\
\textbf{O} & \textit{All}, \textit{Bracket} & Yes\\
\textbf{S} & \textit{All}, \textit{Bracket} & Yes\\
\textbf{P} & \textit{All}, \textit{Bracket} & Yes\\
\textbf{B} & \textit{All}, \textit{Bracket} & Yes\\
\textbf{Cl} & \textit{All}, \textit{Bracket} & Yes\\
\textbf{F} & \textit{All}, \textit{Bracket} & Yes\\
\textbf{Ne} & \textit{Bracket} & No\\
\textbf{Si} & \textit{Bracket} & Yes\\
\textbf{Na} & \textit{Bracket} & Yes\\
\textbf{Mg} & \textit{Bracket} & Yes\\
\textbf{Ti\textsuperscript{2+}} & \textit{Bracket} & Yes\\
\textbf{Au} & \textit{Bracket} & Yes\\
\textbf{Te} & \textit{Bracket} & Yes\\
\textbf{At} & \textit{Bracket} & Yes\\
\textbf{\textsuperscript{201}Bi} & \textit{Bracket} & Yes\\
\botrule
\end{tabular}
\footnotetext[1]{These replacement methods on the using the asterisk will afford the corresponding PSMILES representation}
\footnotetext[2]{Canonicalization of the asterisk inside a bracket removes the bracket, giving an equivalent representation as the \textit{all} method}
\footnotetext[3]{Canonicaliztion of SMILES with the [H] token, removes the token entirely as hydrogen atoms are implicit in SMILES.}
\end{table}

\pagebreak

\section{Supplemental Figures}

\subsection{Polymer Representation}

\begin{figure}[H]
\centering
\includegraphics[width=1\textwidth]{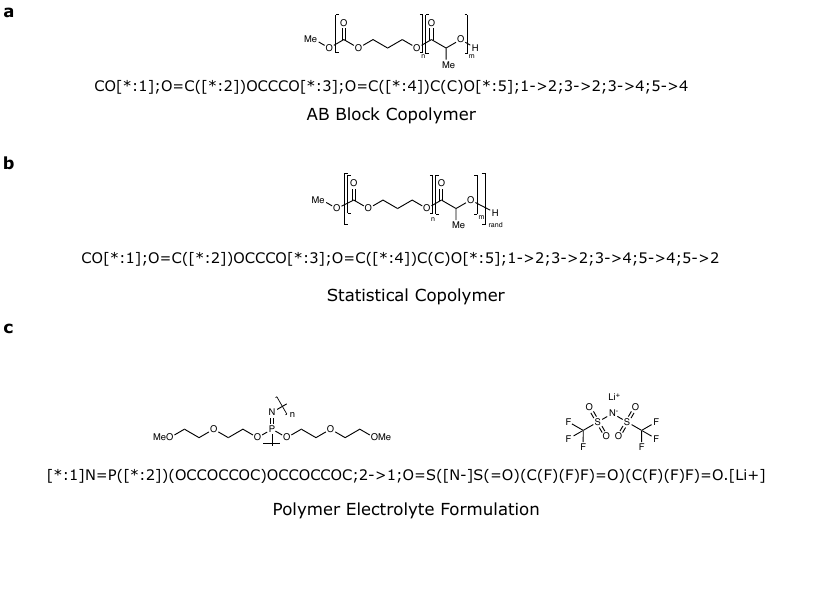}
\caption{Examples polymer structures and their corresponding CPG representation.~\textbf{a}. Example of AB block copolymer represented using the CPG notation.~\textbf{b}. Example of statistical copolymer containing identical components as \textbf{a}. Differentiation in the CPG representation is in the labeled edge connections.~\textbf{c}. Example of a polymer electrolyte formulation containing a small-molecule lithium salt component.}\label{rep_fig_si}
\end{figure}

\subsection{Pre-Training Data}\label{secA1}

\begin{figure}[H]
\centering
\includegraphics[width=1\textwidth]{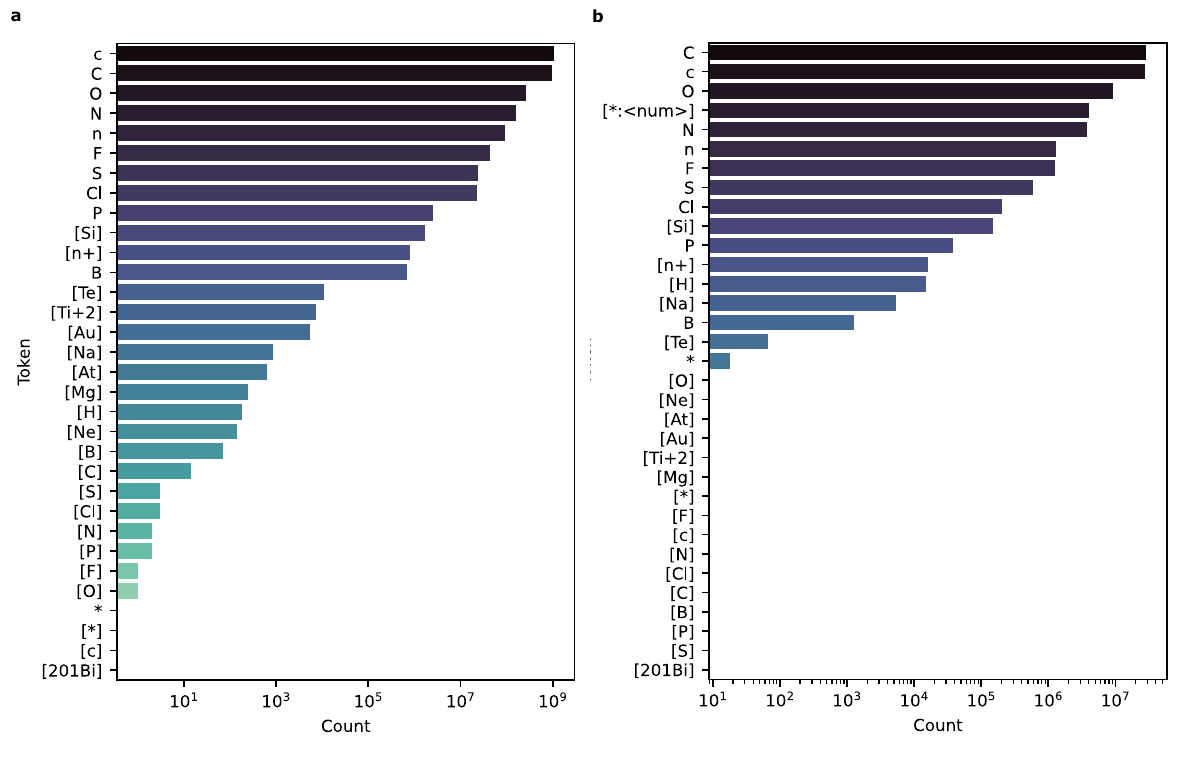}
\caption{Plots of token counts in the pre-training for the substituted tokens and asterisk containing tokens from Supplementary Table~\ref{atomtab}.~\textbf{a}. Token counts from SMI-TED pre-training data.~\textbf{b}. Token counts from further pre-traing data used for SMI-TED-POLYMER.~The token [*:\textless{num}\textgreater{}] indicates the total for all numbered asterisk points e.g. ([*:1], [*:2], etc.).}\label{pretrain_tokens}
\end{figure}

\subsection{Error Analysis}
\subsubsection{Latent Embedding Distance}

Below are the remaining plots of the R\textsuperscript{2} from linear regression between the predicted property value of each candidate in the hold-out test set and the average true value from its top five nearest neighbors in the training set as a function of the model used not included in the main manuscript. As in the main text, fine-tuned models are labeled by their respective base model followed by the representation with which it was fine-tuned with and the associated loss for the checkpoint. All losses for fine-tuned models are RMSE unless indicated otherwise. Circular markers indicate individual data points of each representation system evaluated. Markers are colored according to their representation group, with CM = CPG representation, Elemental = indicates non-asterisk atom substitutions, RT = randomized token selection, RC = randomly shuffled CPG representation, and RF = randomly shuffled SMILES string with randomly selected replacement atoms.

\begin{figure}[H]
\centering
\includegraphics[width=1\textwidth]{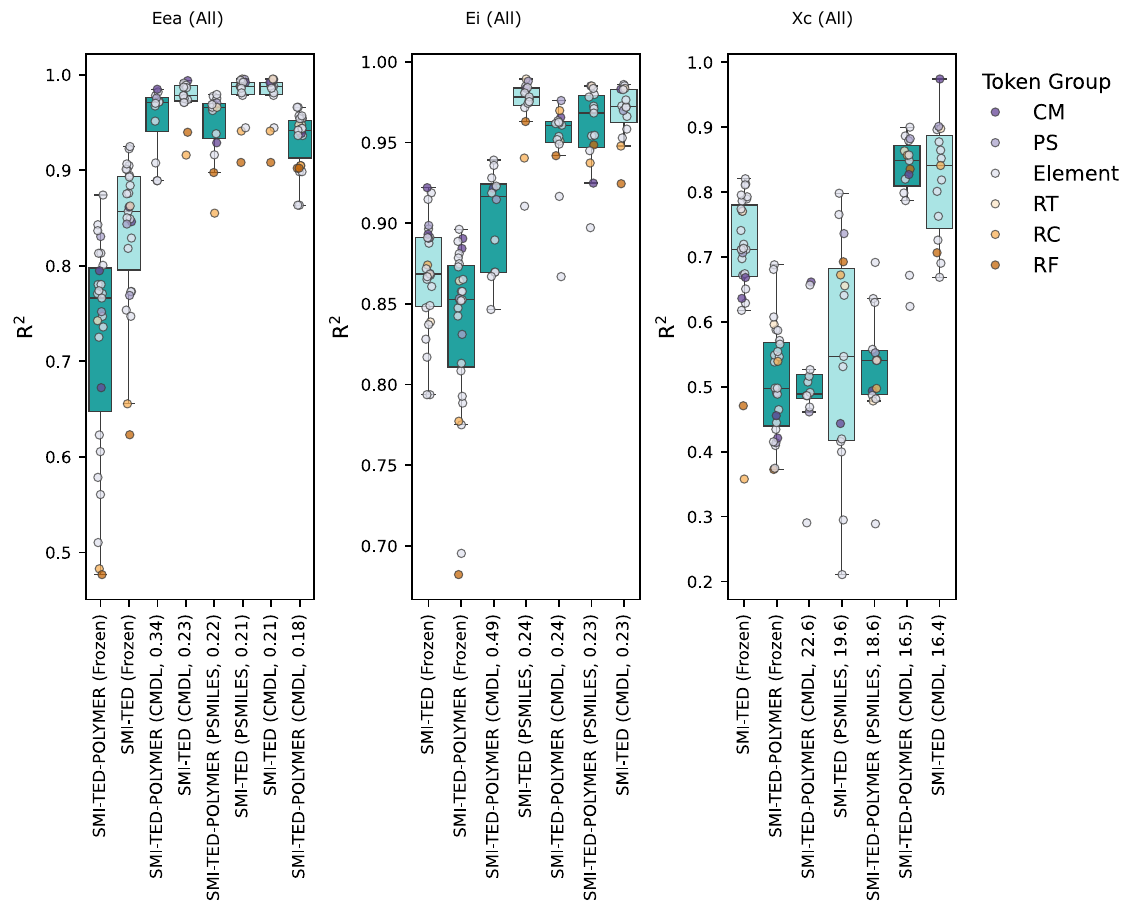}
\caption{Plots of R\textsuperscript{2} value distributions for the benchmark datasets \textit{E\textsubscript{ea}}, \textit{E\textsubscript{i}}, and \textit{X\textsubscript{c}} using the \textit{all} substitution strategy.}\label{knn_rsq_all}
\end{figure}

\begin{figure}[H]
\centering
\includegraphics[width=1\textwidth]{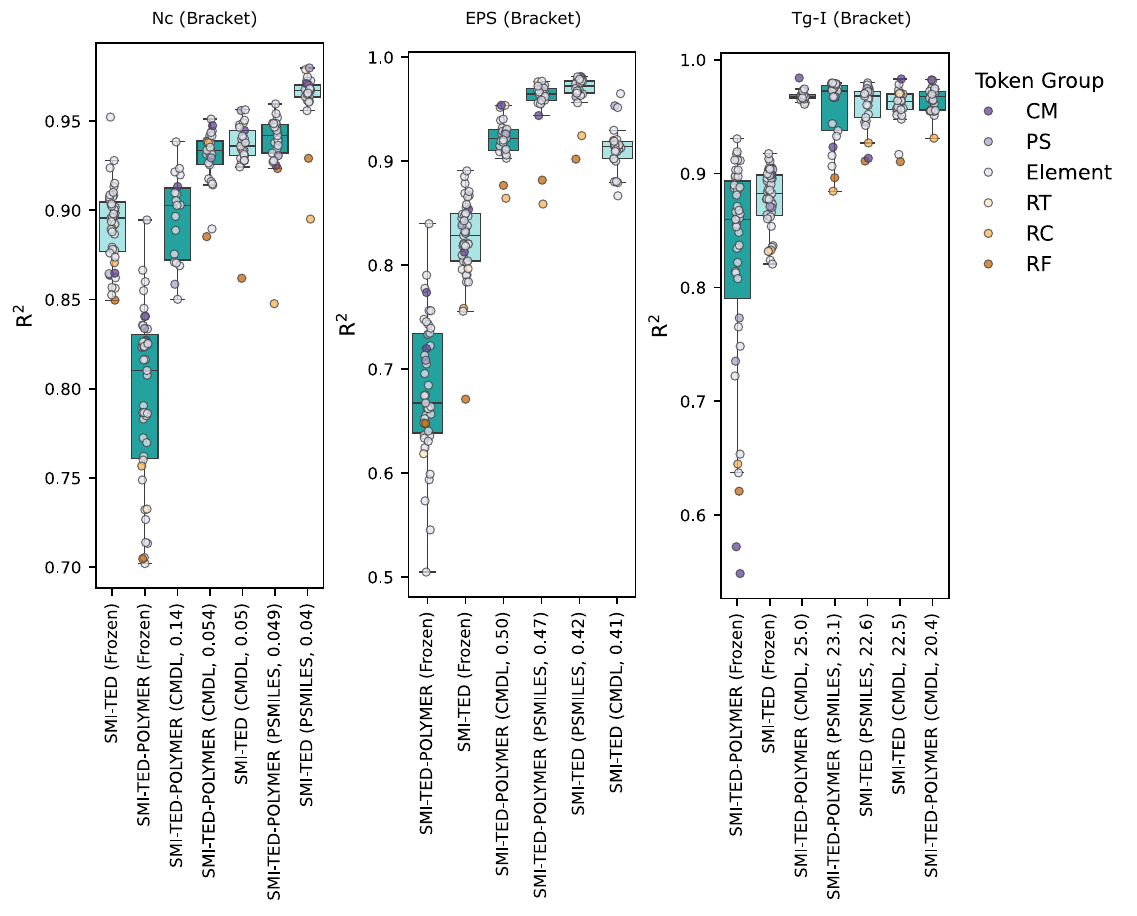}
\caption{Plots of R\textsuperscript{2} value distributions for the benchmark datasets \textit{N\textsubscript{c}}, \textit{EPS}, and \textit{Tg-I} using the \textit{bracket} substitution strategy.}\label{knn_rsq_si}
\end{figure}

\begin{figure}[H]
\centering
\includegraphics[width=1\textwidth]{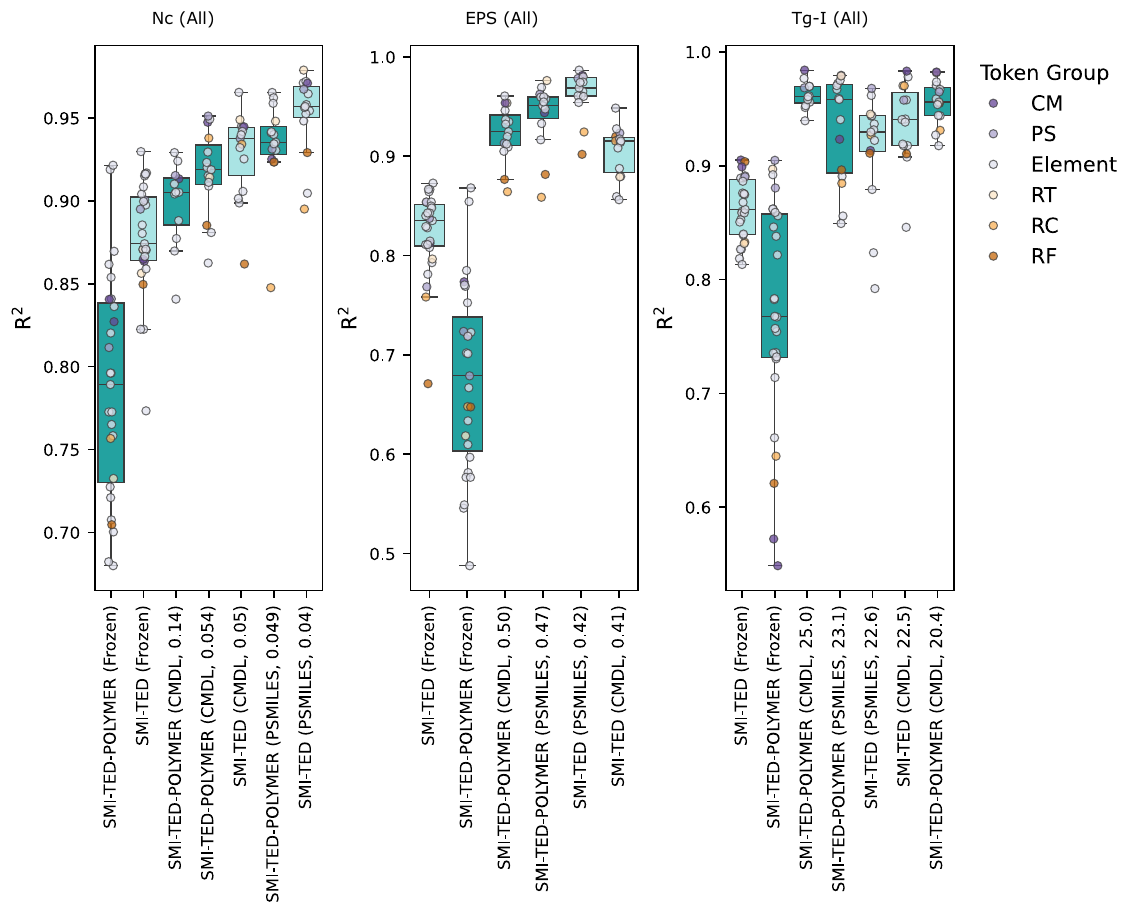}
\caption{Plots of R\textsuperscript{2} value distributions for the benchmark datasets \textit{N\textsubscript{c}}, \textit{EPS}, and \textit{Tg-I} using the \textit{all} substitution strategy.}\label{knn_rsq_si_2_all}
\end{figure}

\begin{figure}[H]
\centering
\includegraphics[width=1\textwidth]{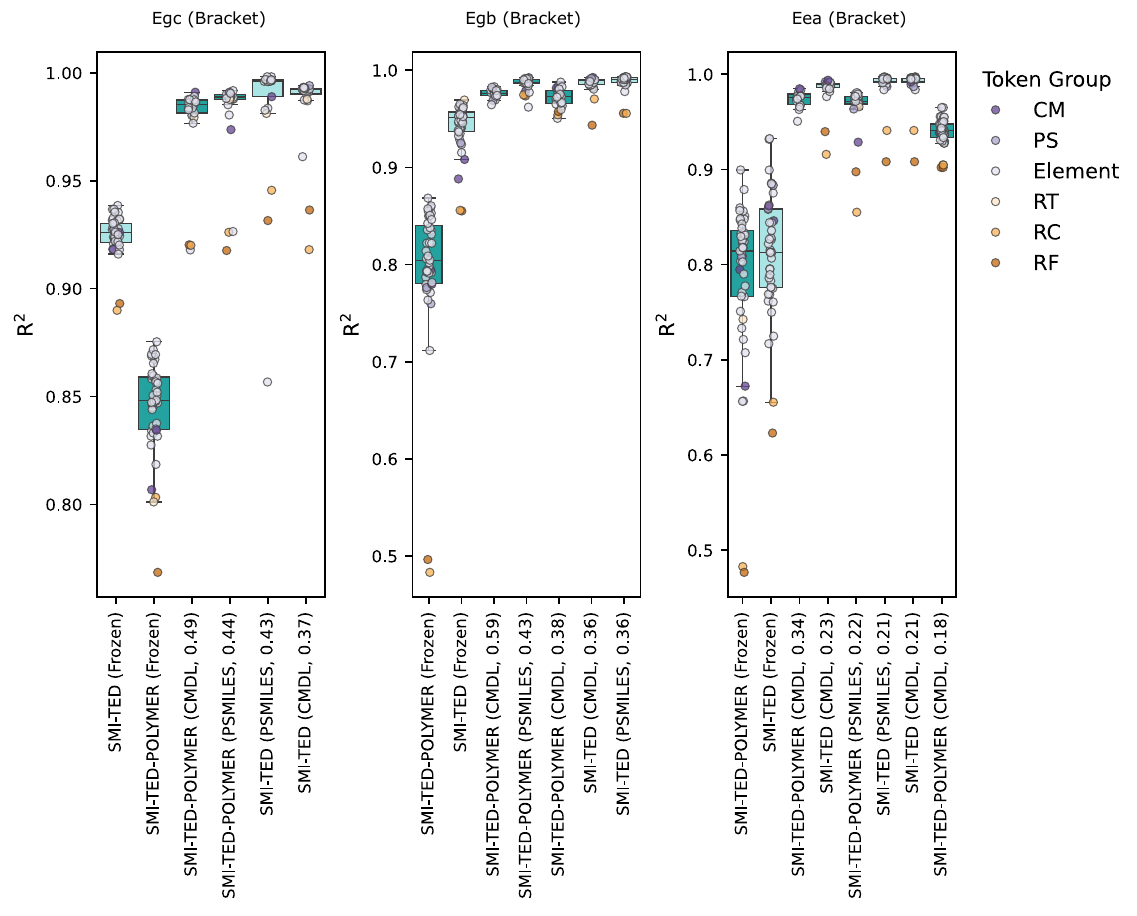}
\caption{Plots of R\textsuperscript{2} value distributions for the benchmark datasets \textit{E\textsubscript{gc}}, \textit{E\textsubscript{gb}}, and \textit{E\textsubscript{ea}} using the \textit{bracket} substitution strategy.}\label{knn_rsq_si_2}
\end{figure}

\begin{figure}[H]
\centering
\includegraphics[width=1\textwidth]{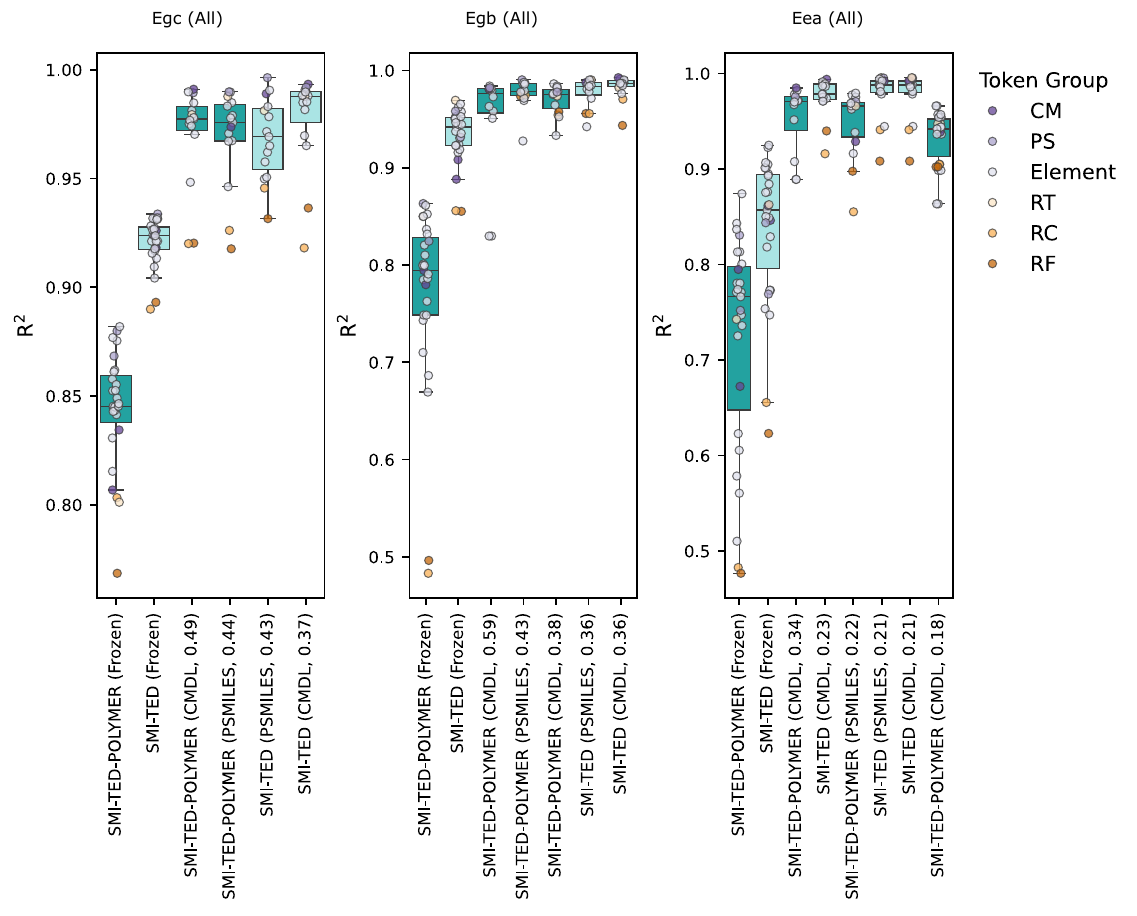}
\caption{Plots of R\textsuperscript{2} value distributions for the benchmark datasets \textit{E\textsubscript{gc}}, \textit{E\textsubscript{gb}}, and \textit{E\textsubscript{ea}} using the \textit{all} substitution strategy.}\label{knn_rsq_si_all}
\end{figure}

\subsubsection{Fingerprint Similarity}

Below are the plots of the R\textsuperscript{2} from linear regression between the predicted property value of each candidate in the hold-out test set and the average true value from its top five nearest neighbors based on fingerprint chemical similarity in the training set as a function of the model used. Not all representations could be used to compute viable chemical fingerprints using the RDKit package. Substituted representations that resulted in an invalid SMILES or any of the randomly shuffled forms were not included in this analysis. Chemical similarity was computed using Dice similarity as reported previously. Fine-tuned models are labeled by their respective base model followed by the representation with which it was fine-tuned with and the associated loss for the checkpoint. All losses for fine-tuned models are RMSE unless indicated otherwise.

\begin{figure}[H]
\centering
\includegraphics[width=1\textwidth]{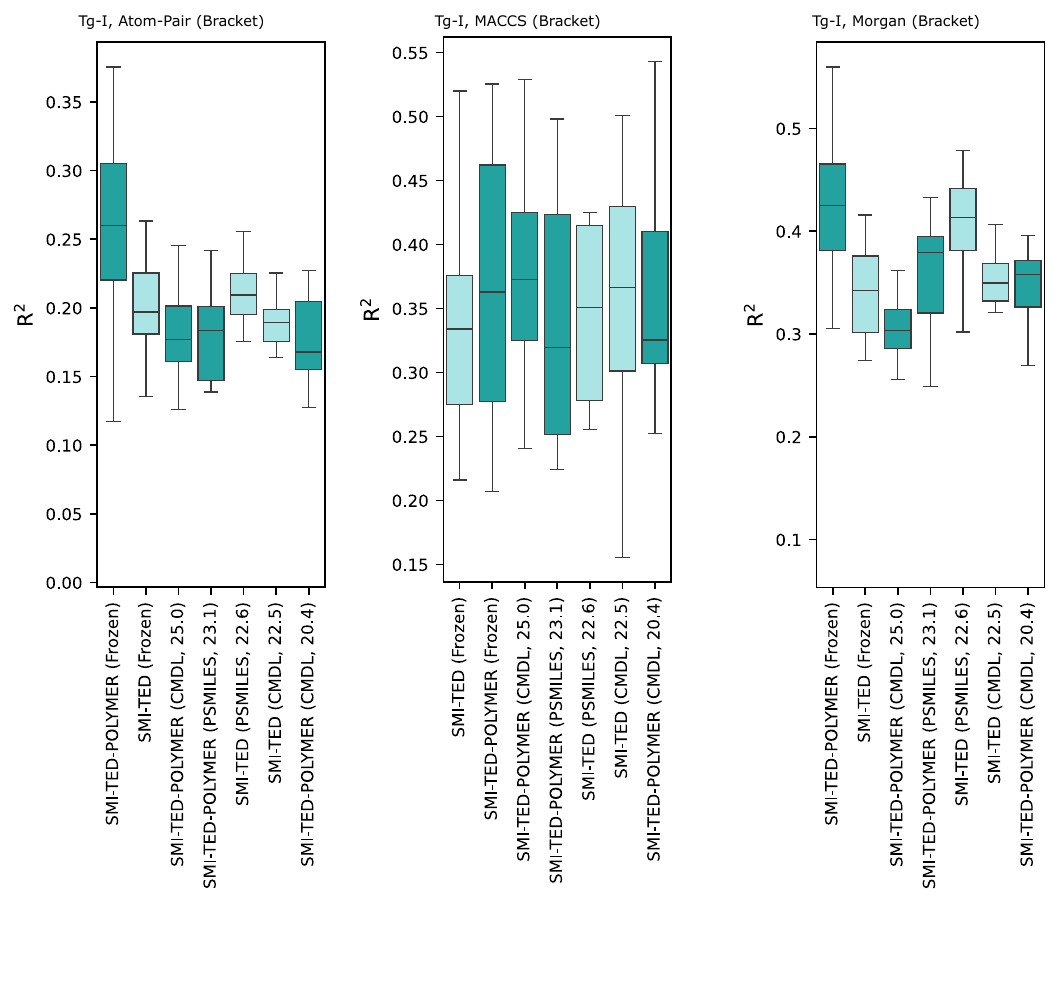}
\caption{Plots of fingerprint R\textsuperscript{2} value distributions for the T\textsubscript{g}-I benchmark dataset using the \textit{bracket} substitution strategy.}\label{acs_ami_knn_fp}
\end{figure}

\begin{figure}[H]
\centering
\includegraphics[width=1\textwidth]{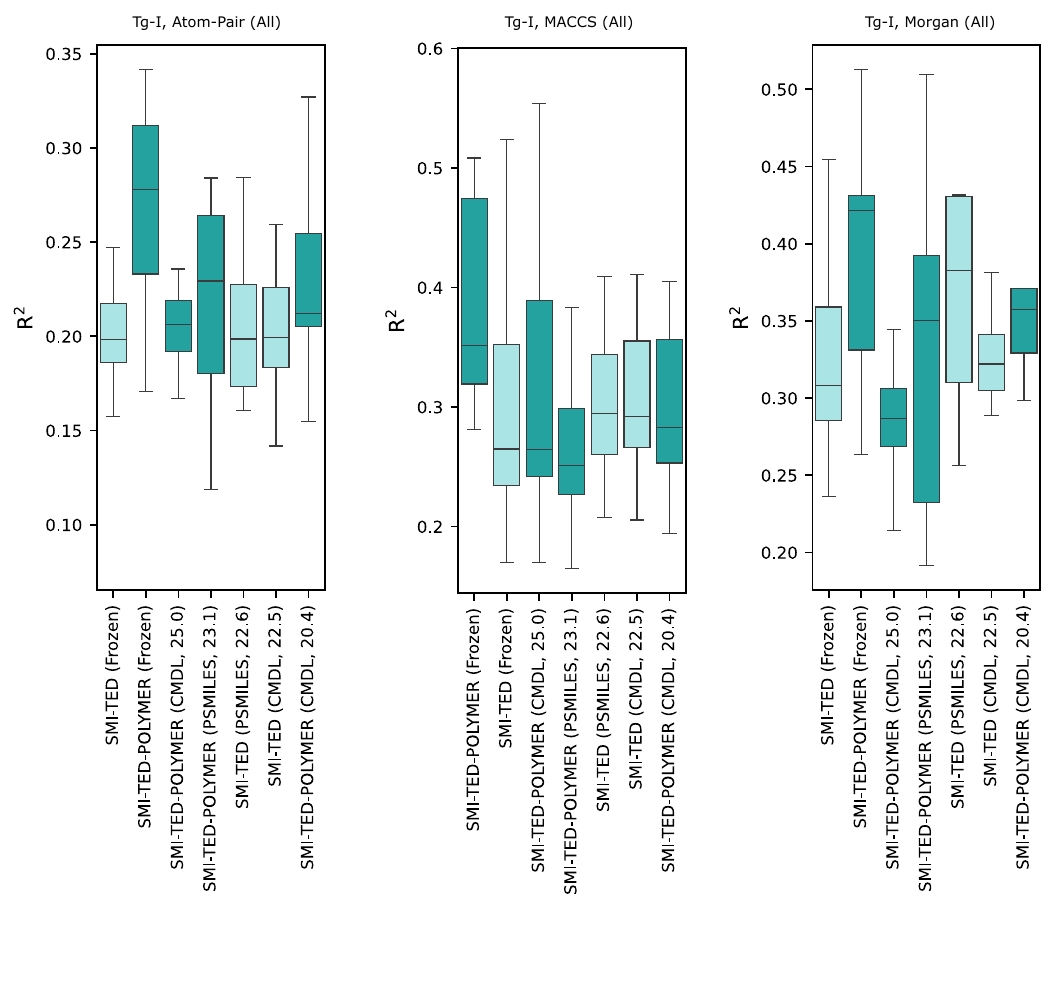}
\caption{Plots of fingerprint R\textsuperscript{2} value distributions for the T\textsubscript{g}-I benchmark dataset using the \textit{all} substitution strategy.}\label{acs_ami_knn_fp_all}
\end{figure}

\begin{figure}[H]
\centering
\includegraphics[width=1\textwidth]{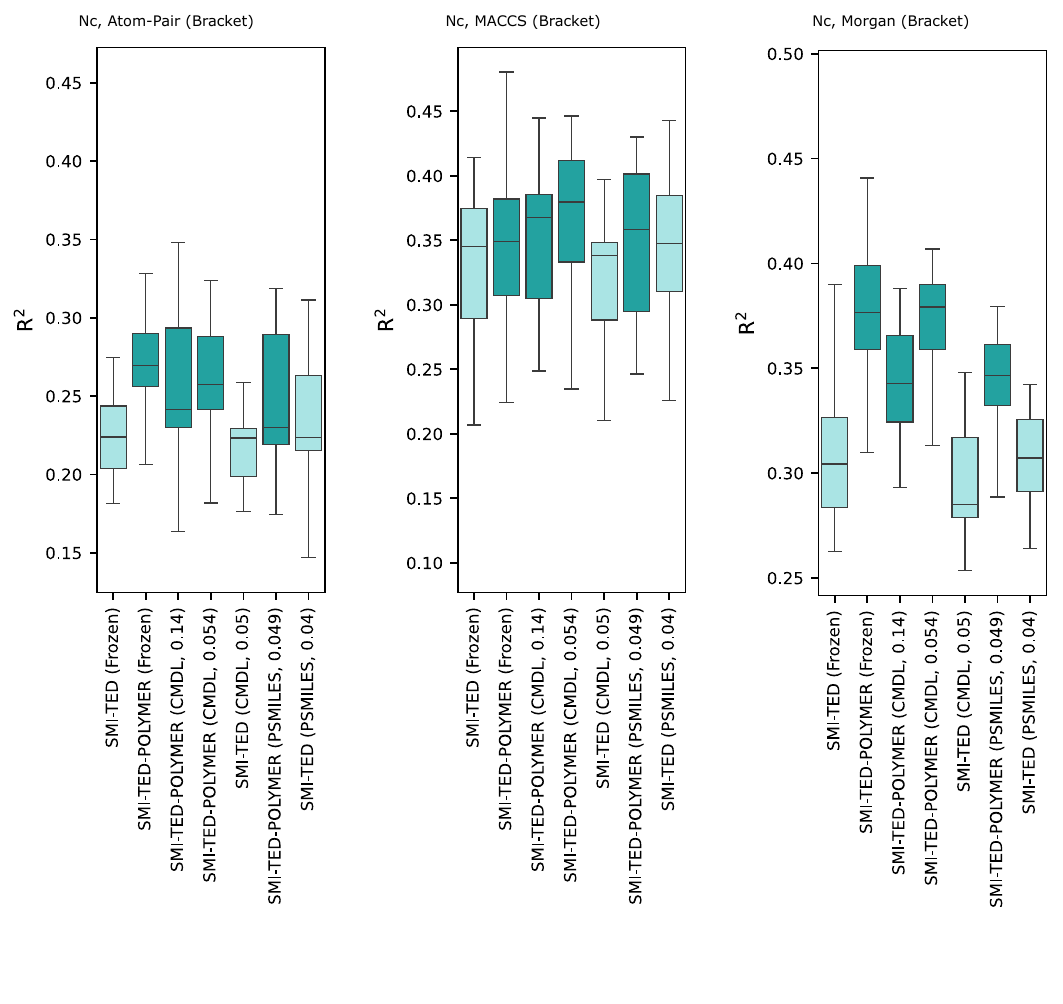}
\caption{Plots of fingerprint R\textsuperscript{2} value distributions for the N\textsubscript{c} benchmark dataset using the \textit{bracket} substitution strategy.}\label{nc_ami_knn_fp_bracket}
\end{figure}

\begin{figure}[H]
\centering
\includegraphics[width=1\textwidth]{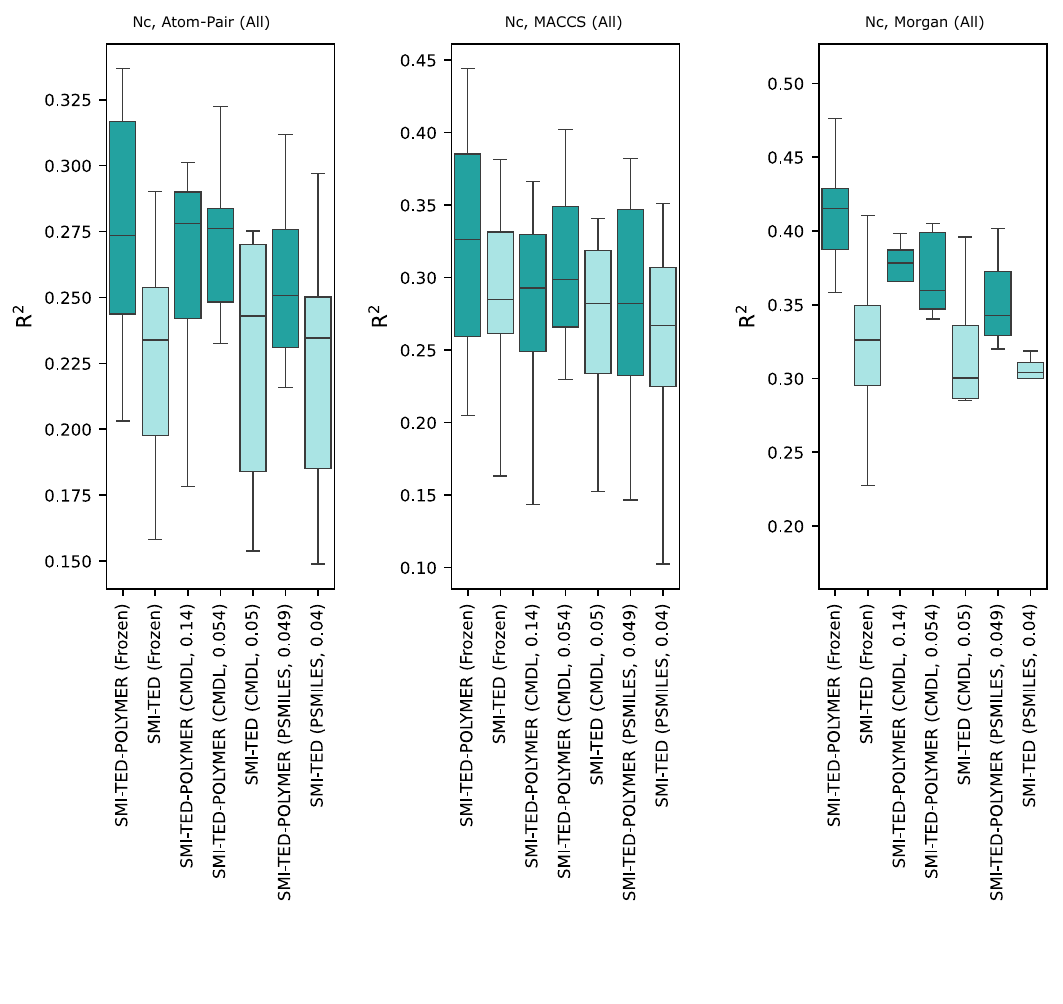}
\caption{Plots of fingerprint R\textsuperscript{2} value distributions for the N\textsubscript{c} benchmark dataset using the \textit{all} substitution strategy.}\label{nc_ami_knn_fp_all}
\end{figure}

\begin{figure}[H]
\centering
\includegraphics[width=1\textwidth]{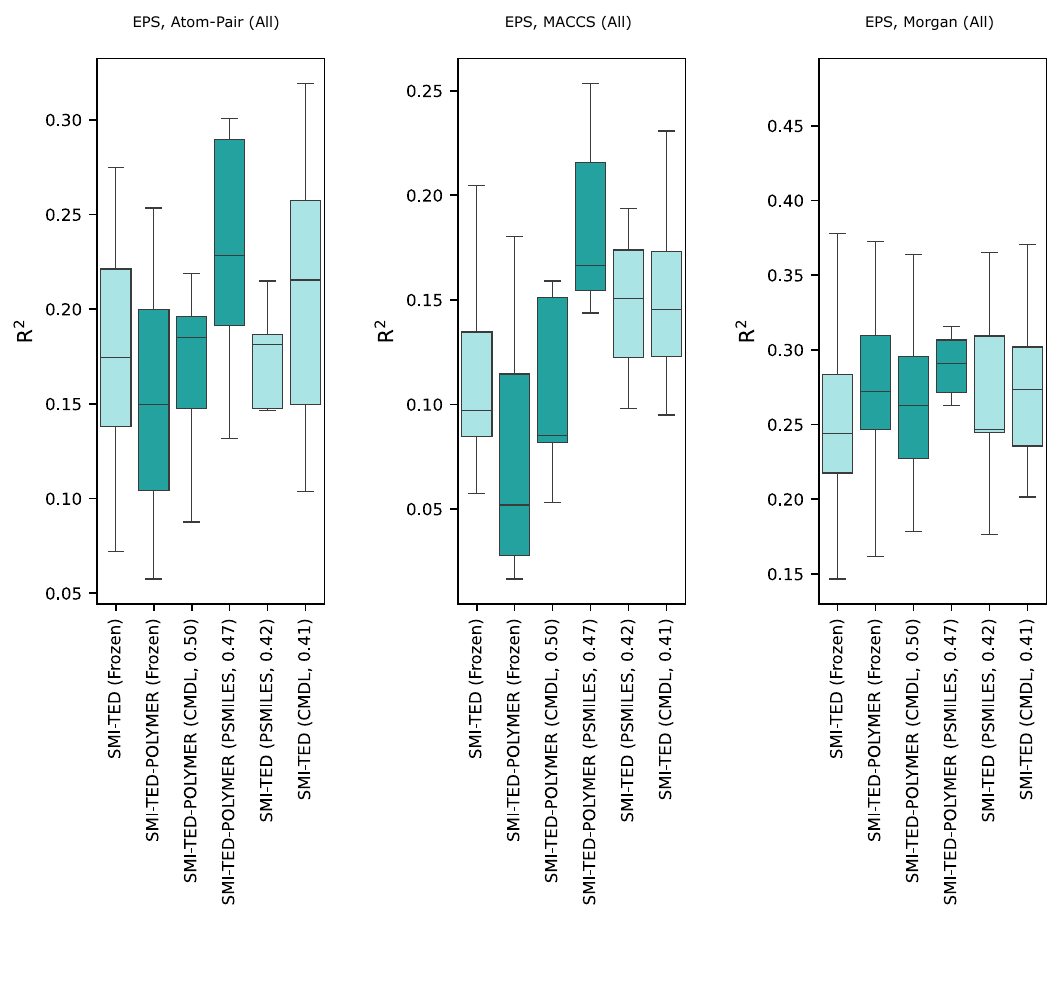}
\caption{Plots of fingerprint R\textsuperscript{2} value distributions for the EPS benchmark dataset using the \textit{all} substitution strategy.}\label{eps_knn_fp_all}
\end{figure}

\begin{figure}[H]
\centering
\includegraphics[width=1\textwidth]{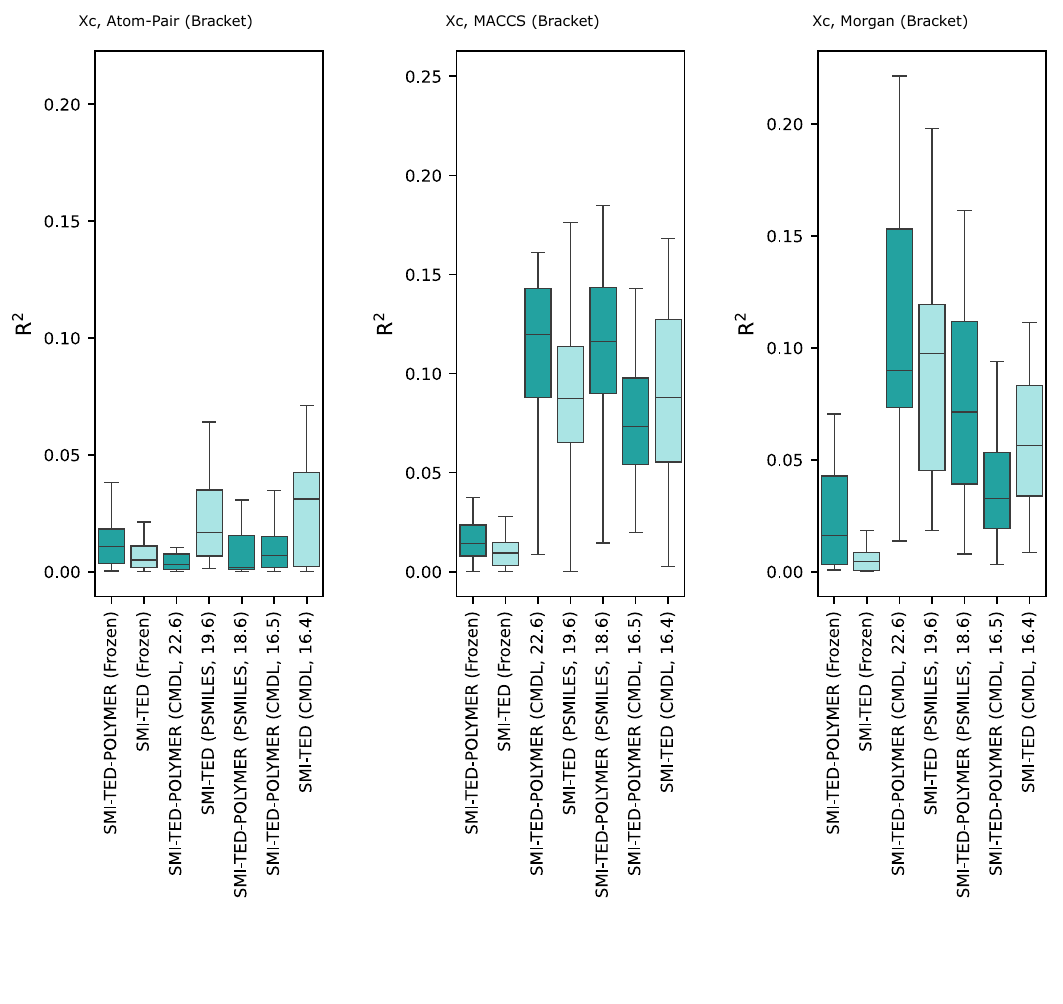}
\caption{Plots of fingerprint R\textsuperscript{2} value distributions for the X\textsubscript{c} benchmark dataset using the \textit{bracket} substitution strategy.}\label{xc_knn_fp_bracket}
\end{figure}

\begin{figure}[H]
\centering
\includegraphics[width=1\textwidth]{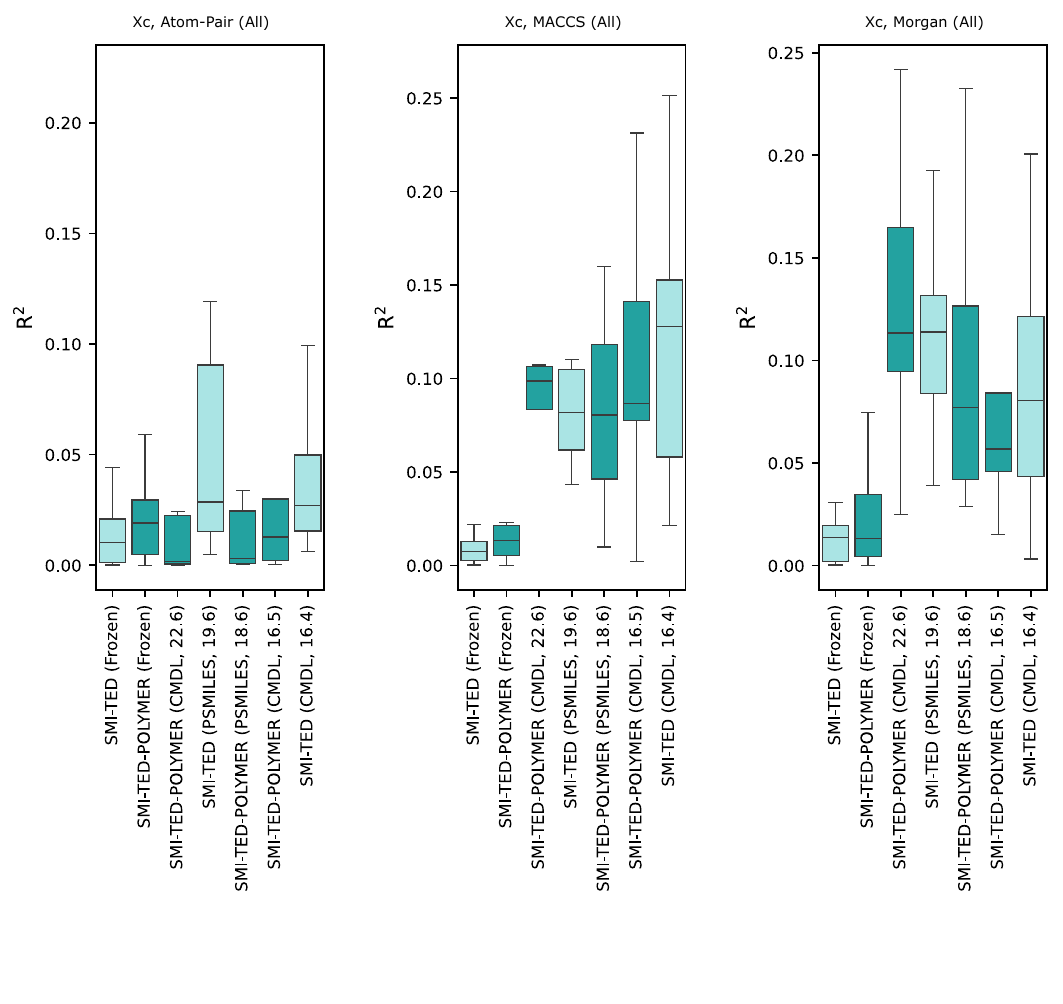}
\caption{Plots of fingerprint R\textsuperscript{2} value distributions for the X\textsubscript{c} benchmark dataset using the \textit{all} substitution strategy.}\label{xc_knn_fp_all}
\end{figure}

\begin{figure}[H]
\centering
\includegraphics[width=1\textwidth]{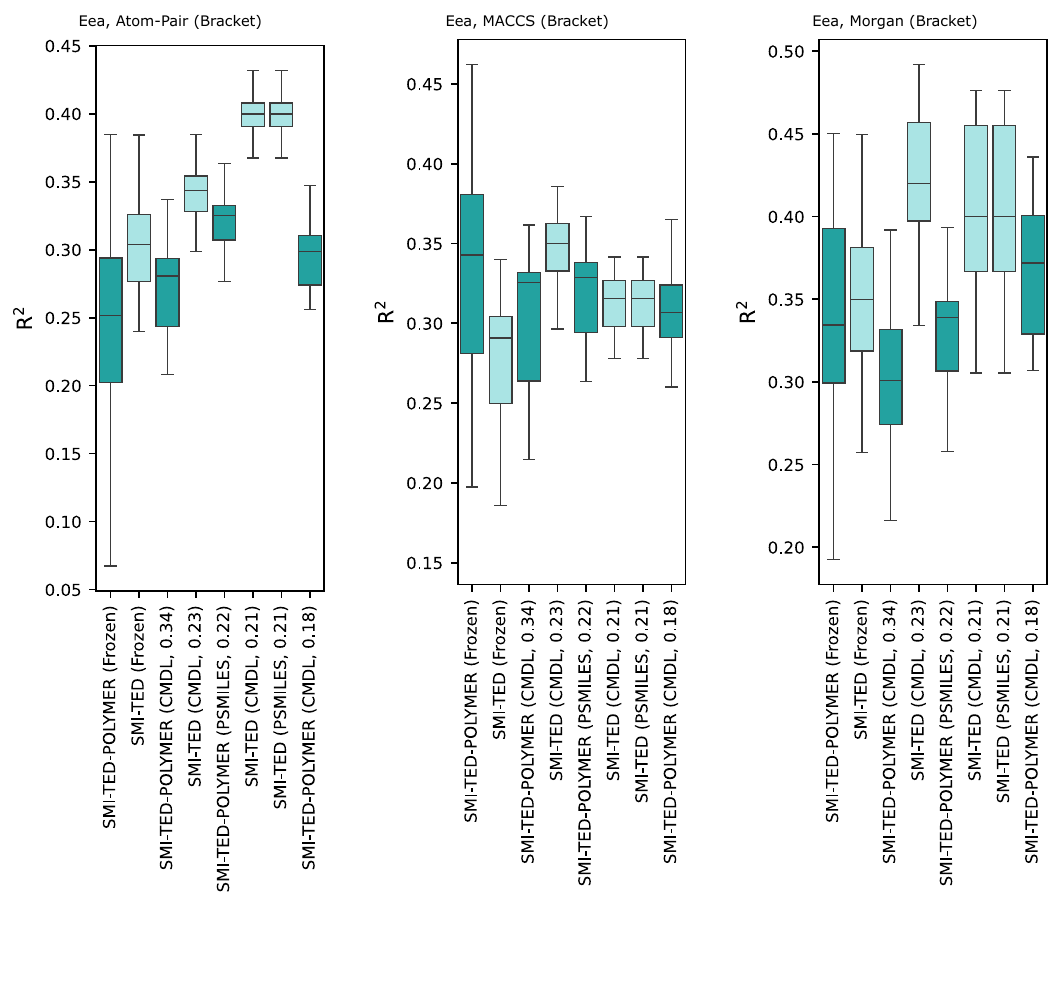}
\caption{Plots of fingerprint R\textsuperscript{2} value distributions for the E\textsubscript{ea} benchmark dataset using the \textit{bracket} substitution strategy.}\label{eea_knn_fp_bracket}
\end{figure}

\begin{figure}[H]
\centering
\includegraphics[width=1\textwidth]{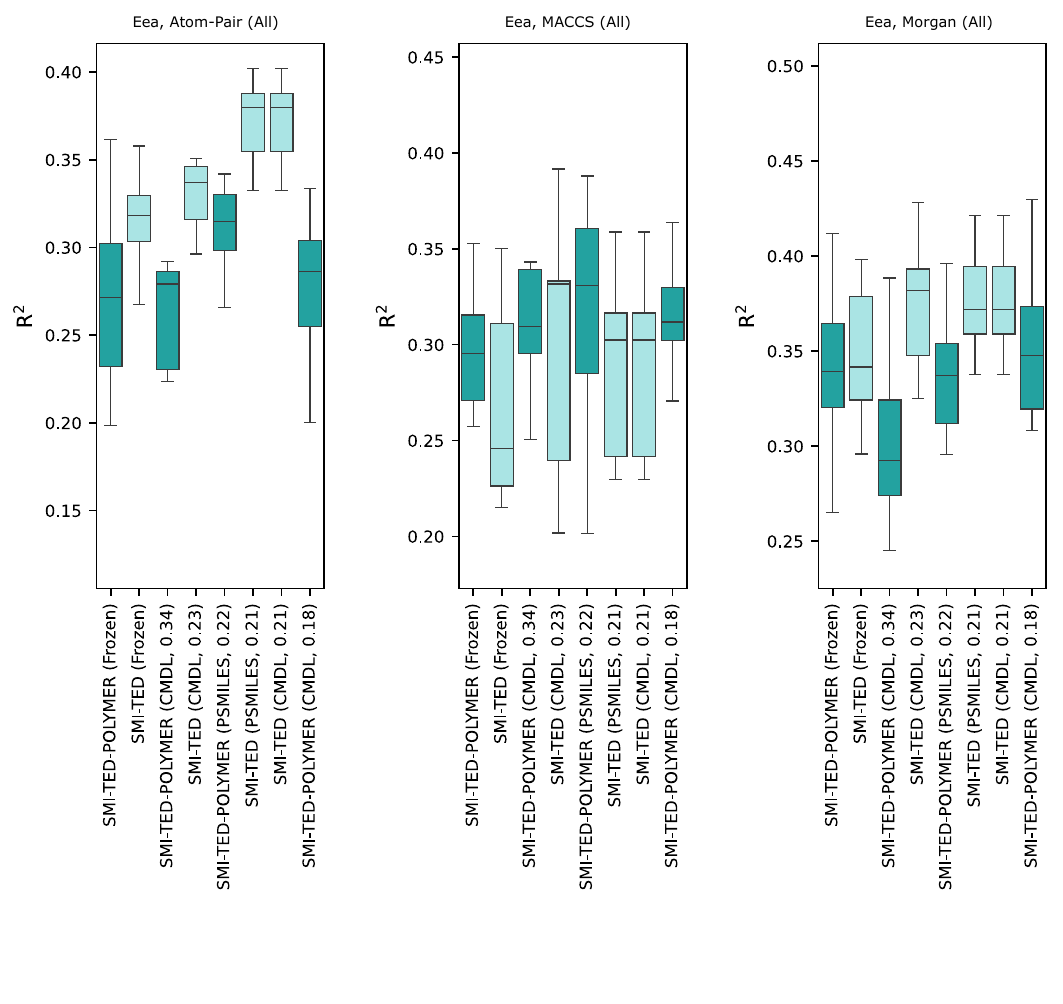}
\caption{Plots of fingerprint R\textsuperscript{2} value distributions for the E\textsubscript{ea} benchmark dataset using the \textit{all} substitution strategy.}\label{eea_knn_fp_all}
\end{figure}

\begin{figure}[H]
\centering
\includegraphics[width=1\textwidth]{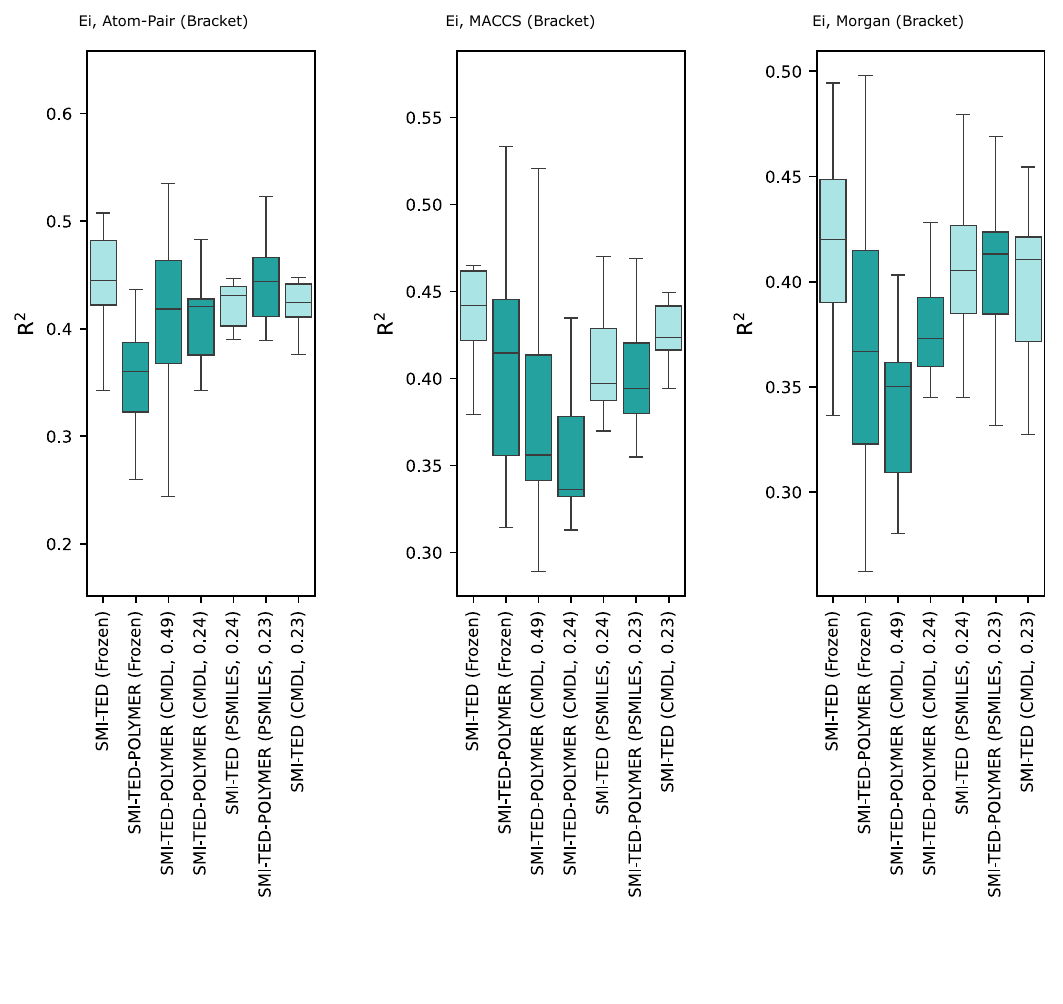}
\caption{Plots of fingerprint R\textsuperscript{2} value distributions for the E\textsubscript{i} benchmark dataset using the \textit{bracket} substitution strategy.}\label{ei_knn_fp_bracket}
\end{figure}

\begin{figure}[H]
\centering
\includegraphics[width=1\textwidth]{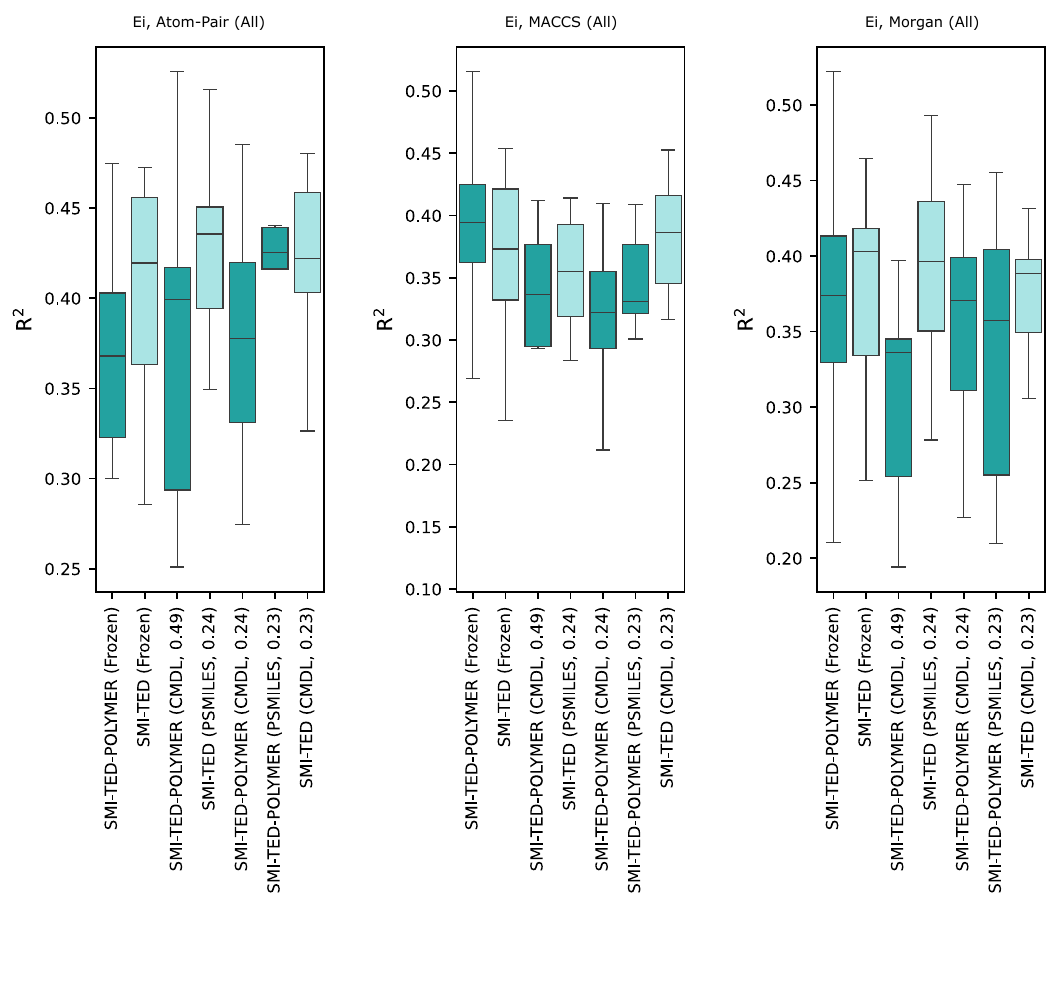}
\caption{Plots of fingerprint R\textsuperscript{2} value distributions for the E\textsubscript{i} benchmark dataset using the \textit{all} substitution strategy.}\label{ei_knn_fp_all}
\end{figure}

\begin{figure}[H]
\centering
\includegraphics[width=1\textwidth]{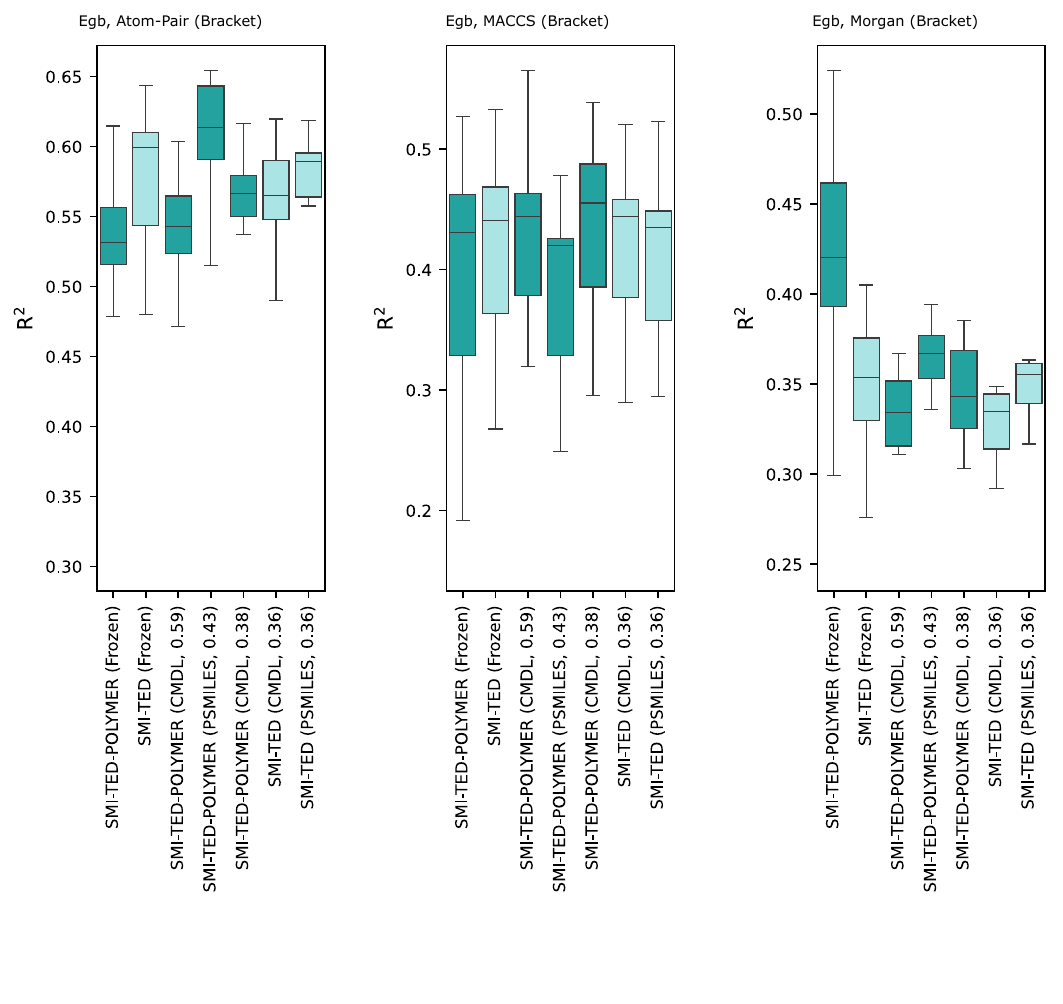}
\caption{Plots of fingerprint R\textsuperscript{2} value distributions for the E\textsubscript{gb} benchmark dataset using the \textit{bracket} substitution strategy.}\label{egb_knn_fp_bracket}
\end{figure}

\begin{figure}[H]
\centering
\includegraphics[width=1\textwidth]{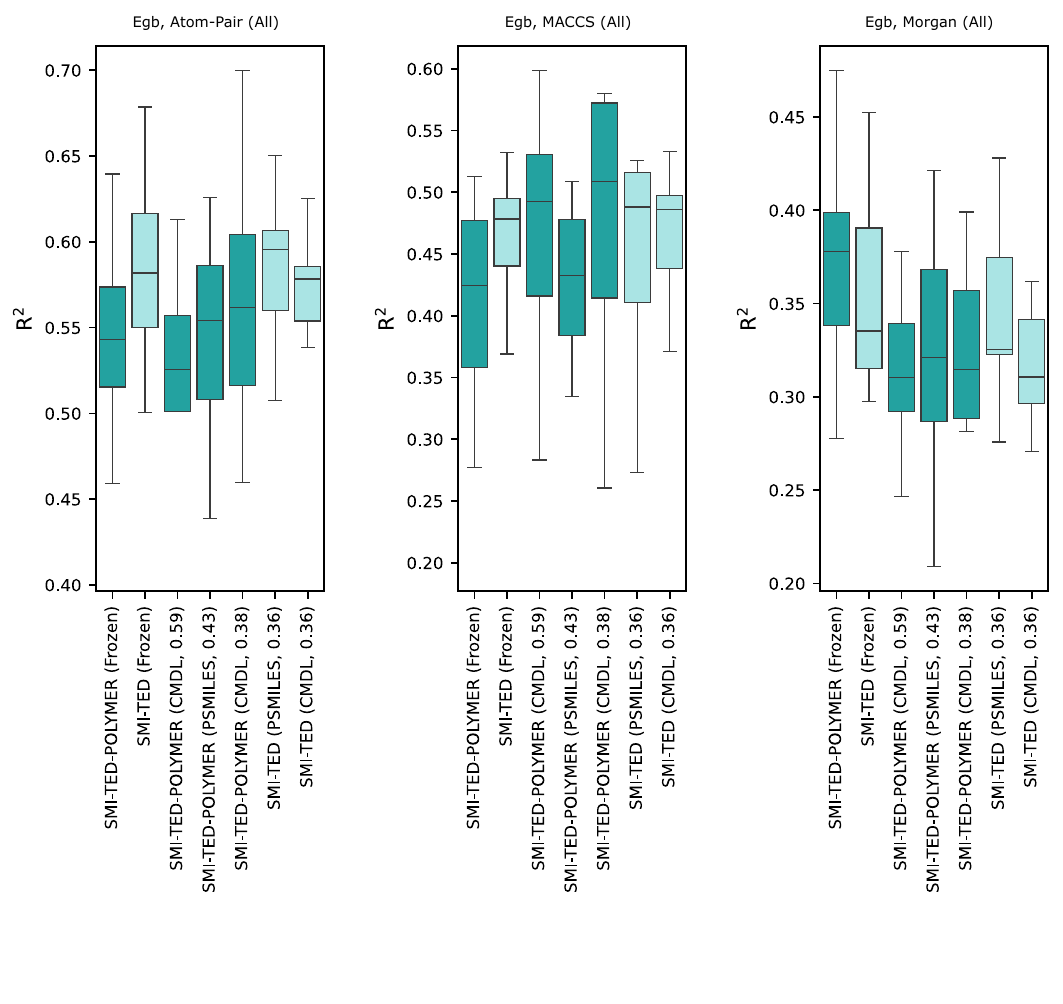}
\caption{Plots of fingerprint R\textsuperscript{2} value distributions for the E\textsubscript{gb} benchmark dataset using the \textit{all} substitution strategy.}\label{egb_knn_fp_all}
\end{figure}

\begin{figure}[H]
\centering
\includegraphics[width=1\textwidth]{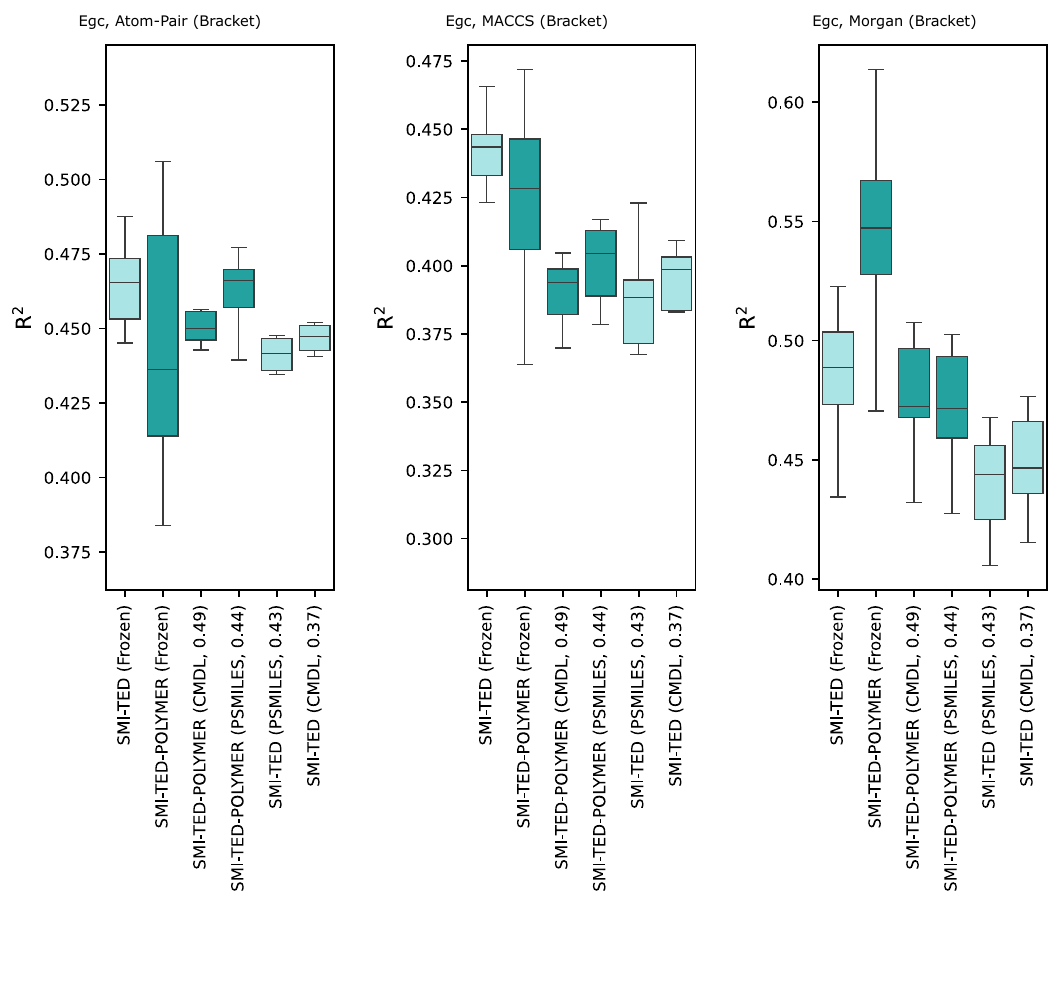}
\caption{Plots of fingerprint R\textsuperscript{2} value distributions for the E\textsubscript{gc} benchmark dataset using the \textit{bracket} substitution strategy.}\label{egc_knn_fp_bracket}
\end{figure}

\begin{figure}[H]
\centering
\includegraphics[width=1\textwidth]{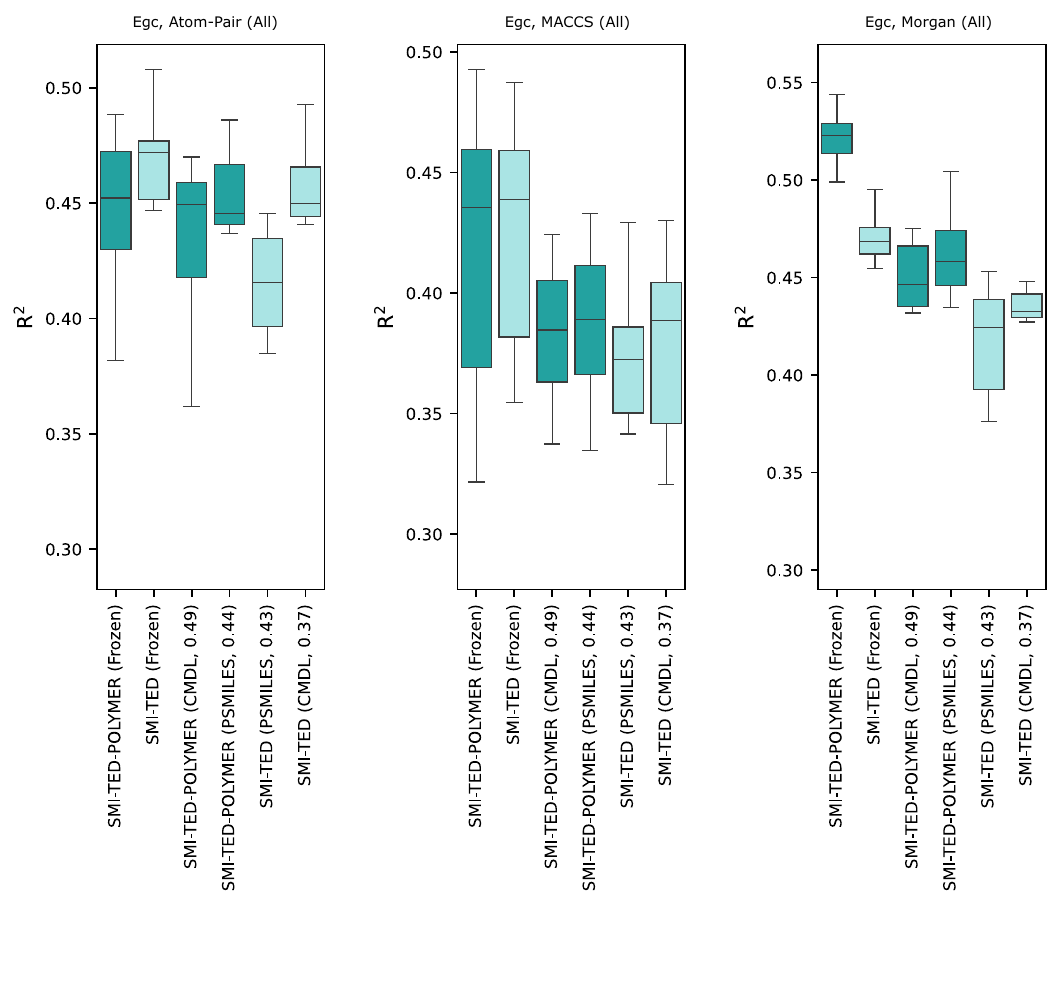}
\caption{Plots of fingerprint R\textsuperscript{2} value distributions for the E\textsubscript{gc} benchmark dataset using the \textit{all} substitution strategy.}\label{egc_knn_fp_all}
\end{figure}

\begin{figure}[H]
\centering
\includegraphics[width=1\textwidth]{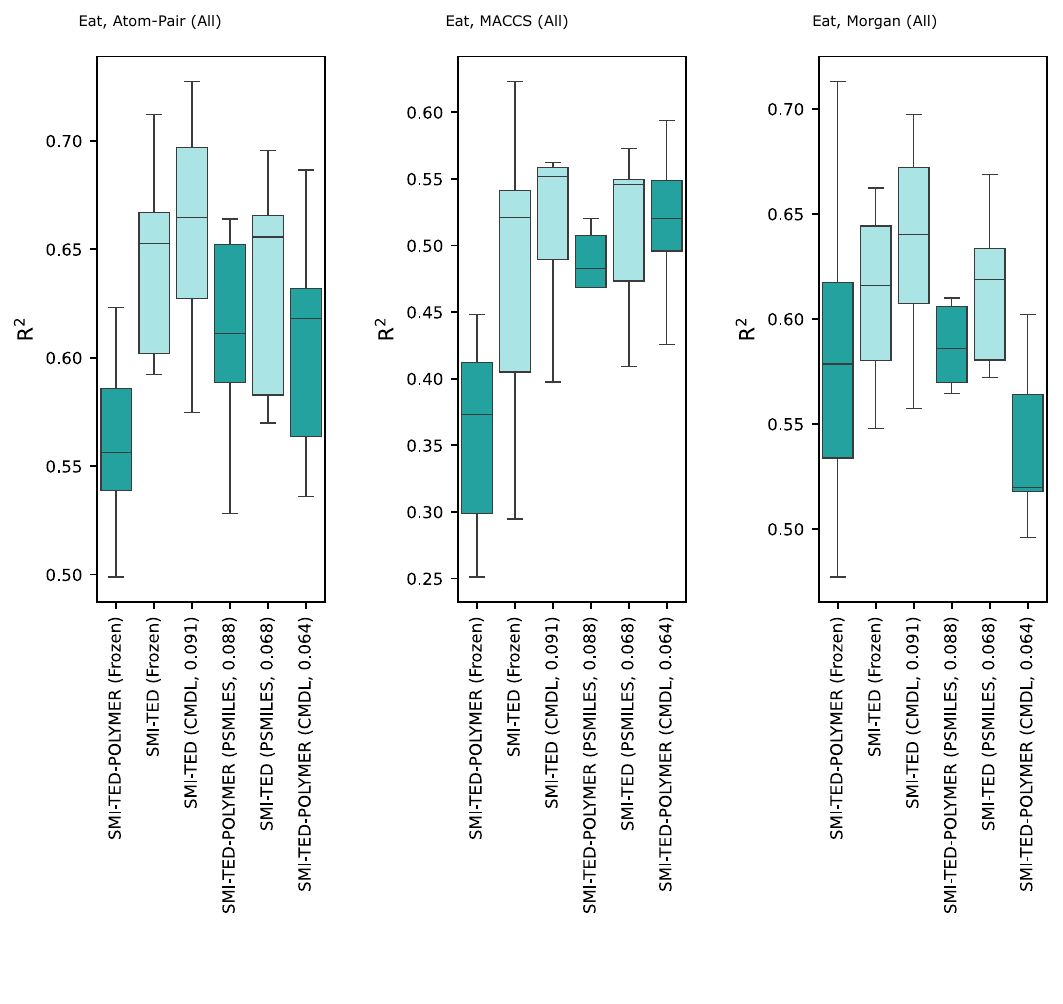}
\caption{Plots of fingerprint R\textsuperscript{2} value distributions for the E\textsubscript{at} benchmark dataset using the \textit{all} substitution strategy.}\label{eat_knn_fp_all}
\end{figure}

\begin{figure}[H]
\centering
\includegraphics[width=1\textwidth]{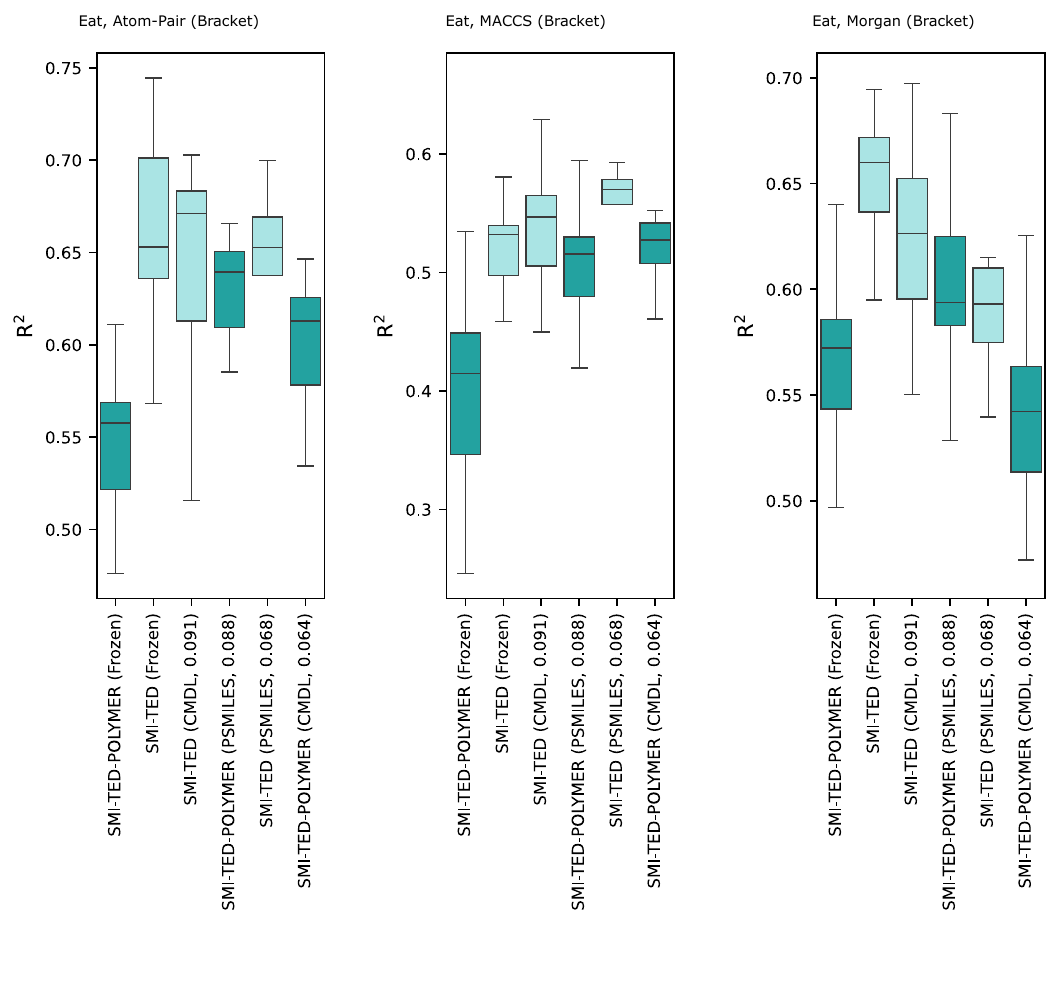}
\caption{Plots of fingerprint R\textsuperscript{2} value distributions for the E\textsubscript{at} benchmark dataset using the \textit{bracket} substitution strategy.}\label{eat_knn_fp_bracket}
\end{figure}

\begin{figure}[H]
\centering
\includegraphics[width=1\textwidth]{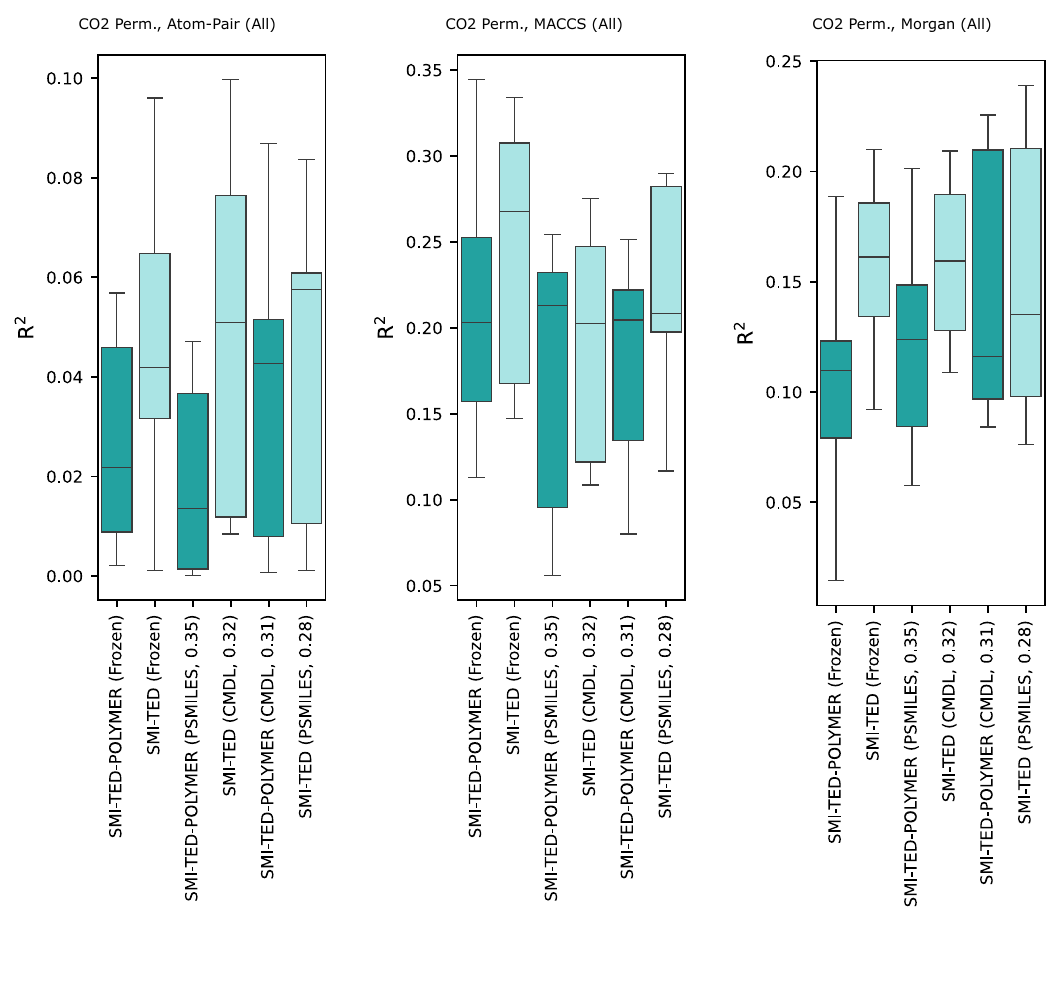}
\caption{Plots of fingerprint R\textsuperscript{2} value distributions for the CO\textsubscript{2} permeability benchmark dataset using the \textit{all} substitution strategy.}\label{netl_co2_knn_fp_all}
\end{figure}

\begin{figure}[H]
\centering
\includegraphics[width=1\textwidth]{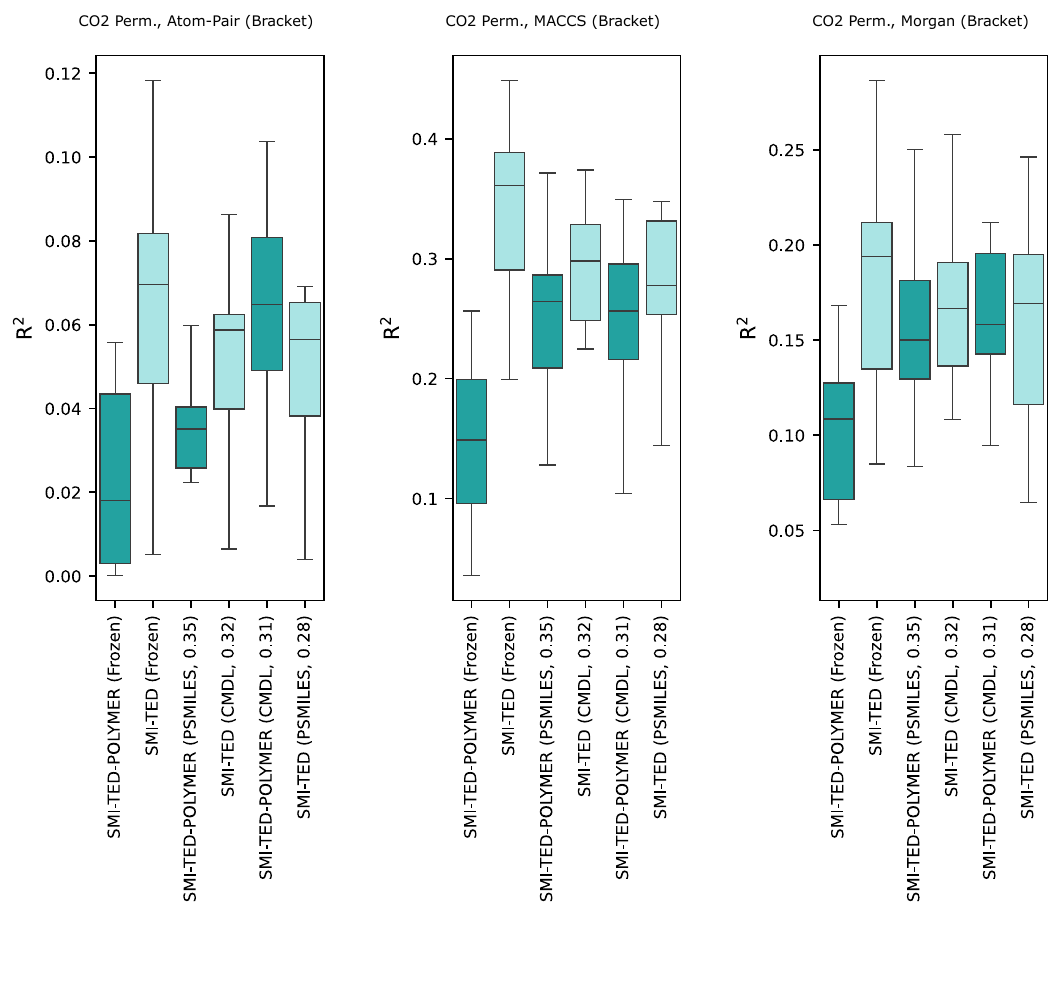}
\caption{Plots of fingerprint R\textsuperscript{2} value distributions for the CO\textsubscript{2} permeability benchmark dataset using the \textit{bracket} substitution strategy.}\label{netl_co2_knn_fp_bracket}
\end{figure}

\begin{figure}[H]
\centering
\includegraphics[width=1\textwidth]{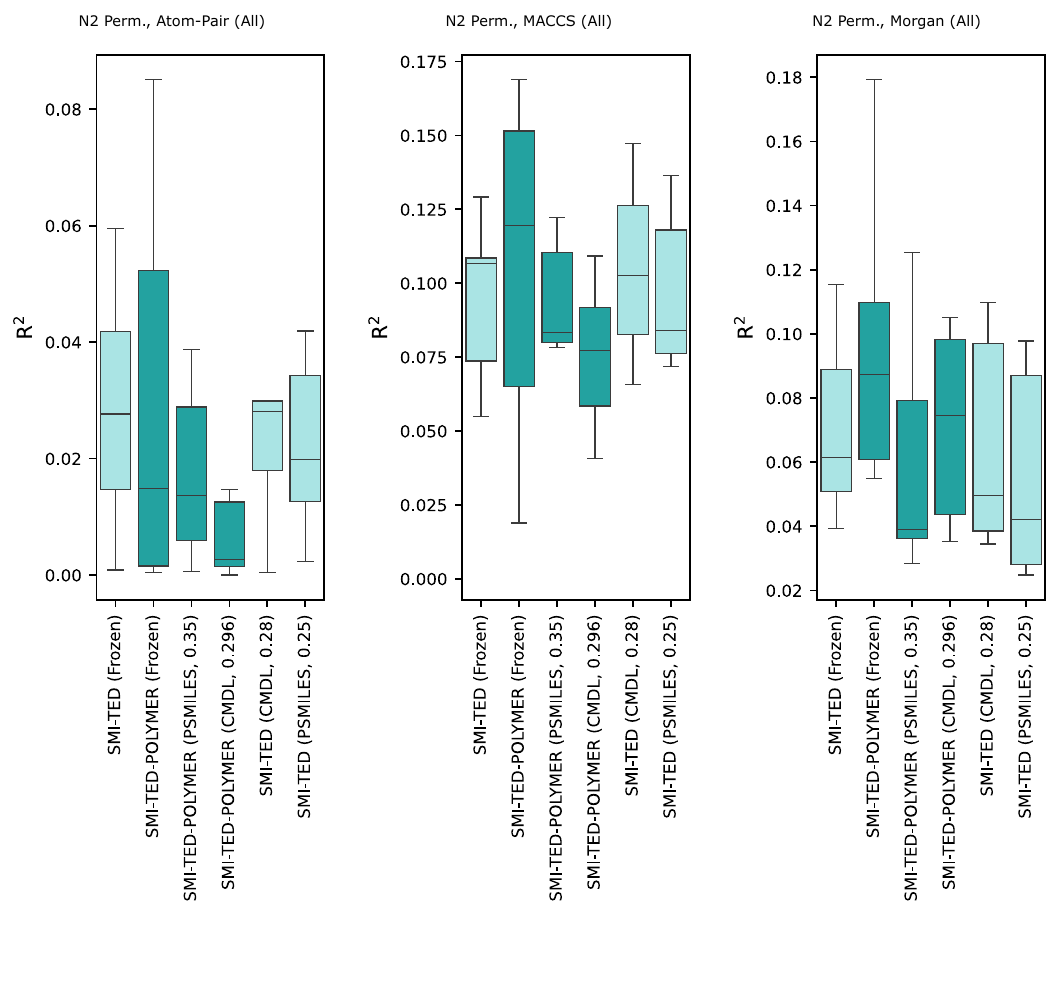}
\caption{Plots of fingerprint R\textsuperscript{2} value distributions for the N\textsubscript{2} permeability benchmark dataset using the \textit{all} substitution strategy.}\label{netl_n2_knn_fp_all}
\end{figure}

\begin{figure}[H]
\centering
\includegraphics[width=1\textwidth]{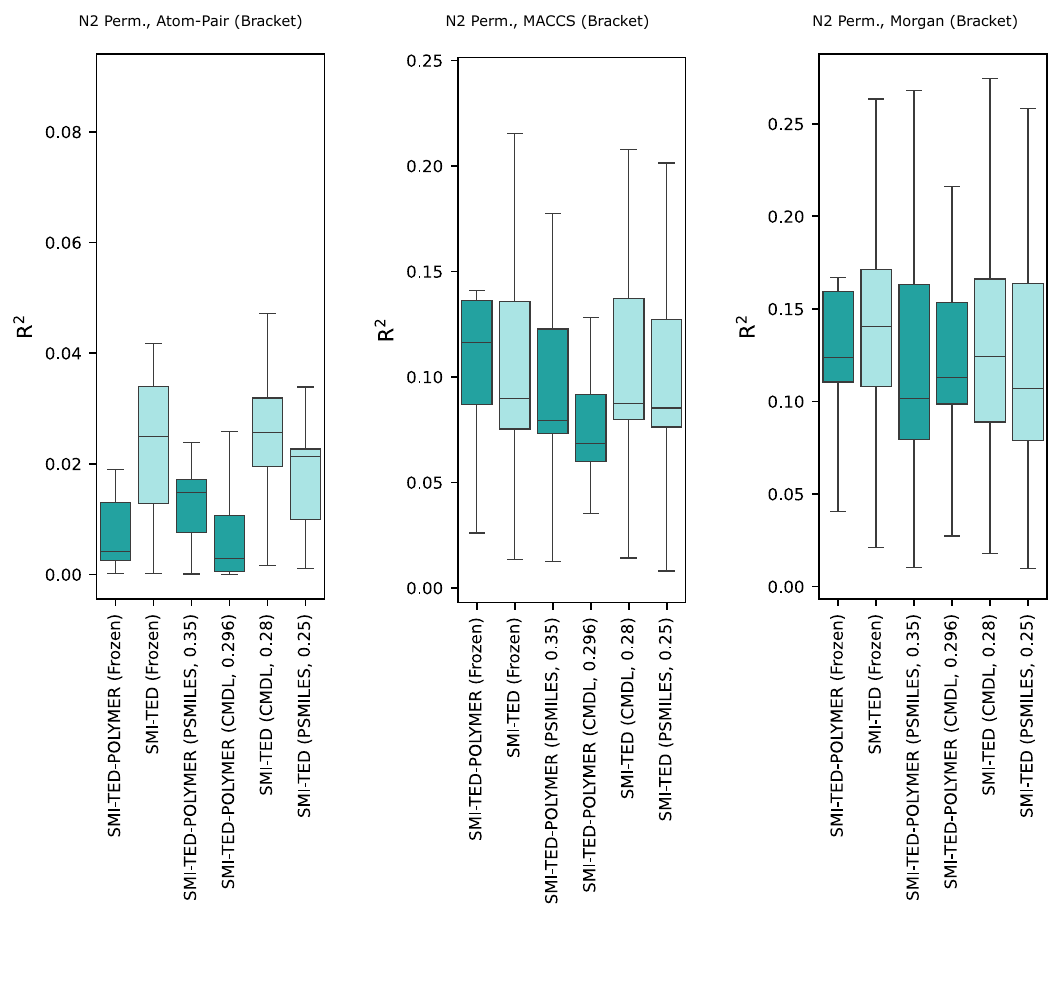}
\caption{Plots of fingerprint R\textsuperscript{2} value distributions for the N\textsubscript{2} permeability benchmark dataset using the \textit{bracket} substitution strategy.}\label{netl_n2_knn_fp_bracket}
\end{figure}

\begin{figure}[H]
\centering
\includegraphics[width=1\textwidth]{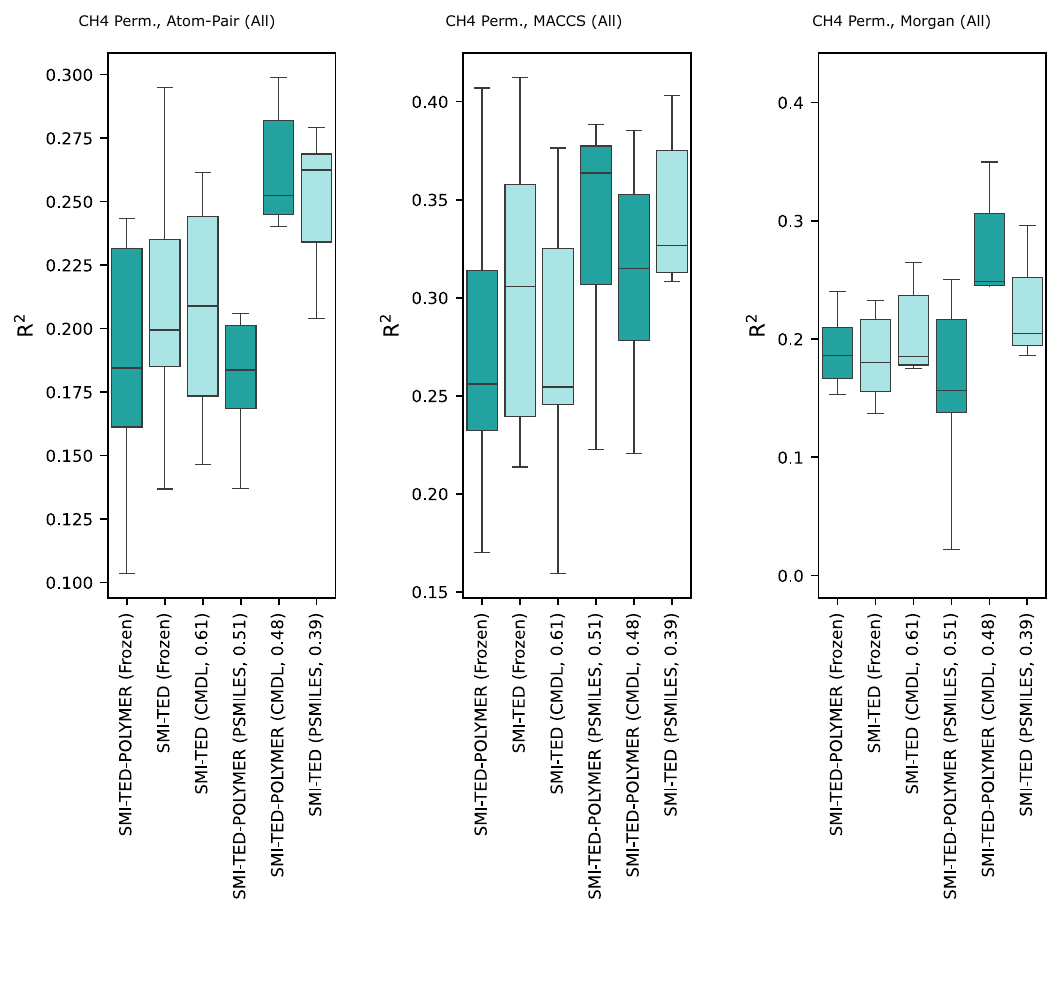}
\caption{Plots of fingerprint R\textsuperscript{2} value distributions for the CH\textsubscript{4} permeability benchmark dataset using the \textit{all} substitution strategy.}\label{netl_ch4_knn_fp_all}
\end{figure}

\begin{figure}[H]
\centering
\includegraphics[width=1\textwidth]{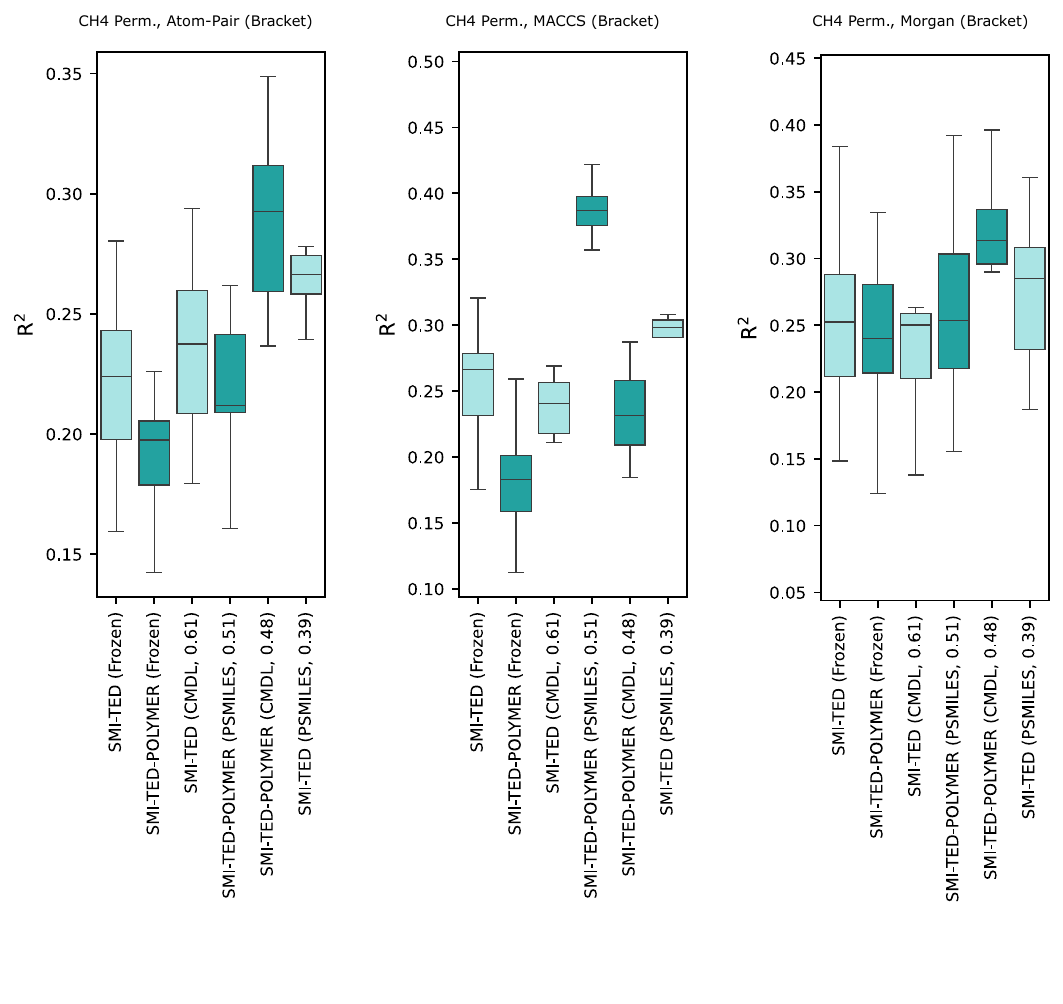}
\caption{Plots of fingerprint R\textsuperscript{2} value distributions for the CH\textsubscript{4} permeability benchmark dataset using the \textit{bracket} substitution strategy.}\label{netl_ch4_knn_fp_bracket}
\end{figure}

\begin{figure}[H]
\centering
\includegraphics[width=1\textwidth]{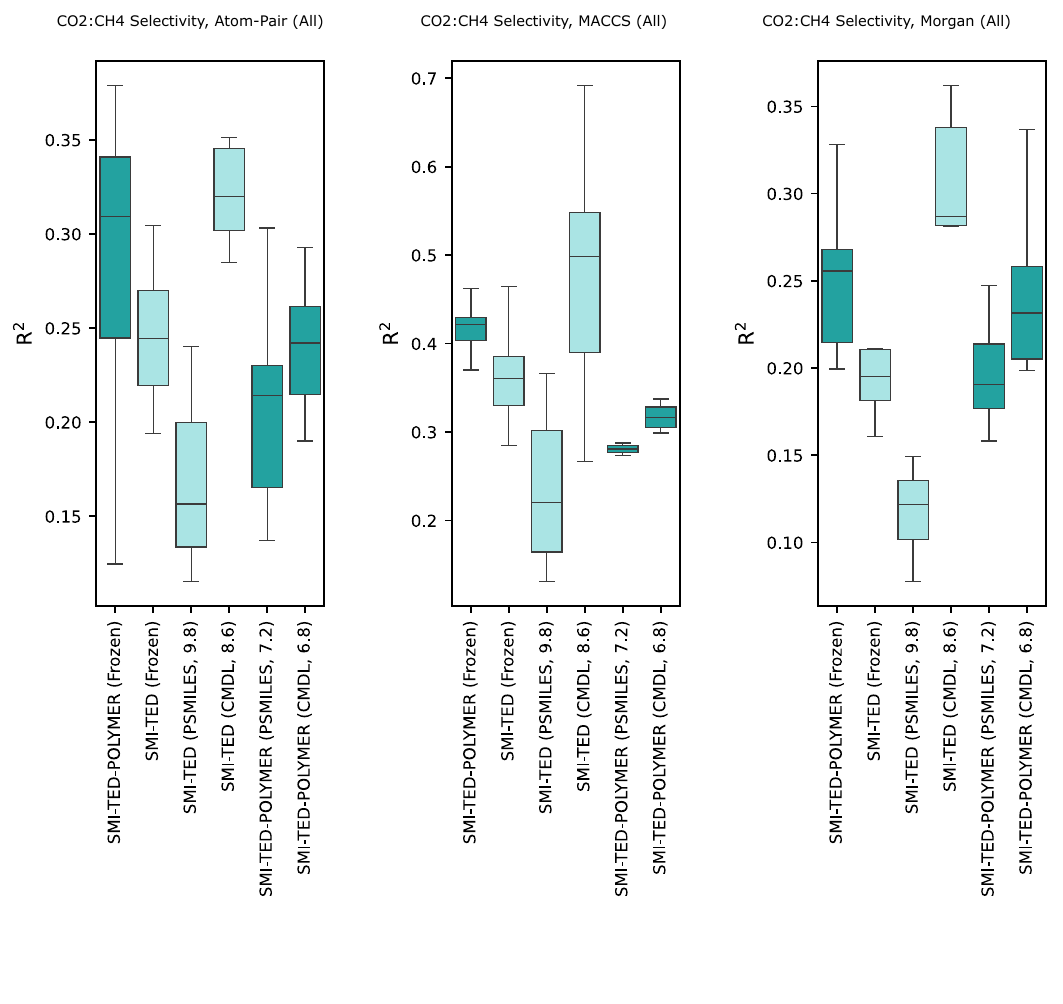}
\caption{Plots of fingerprint R\textsuperscript{2} value distributions for the CO\textsubscript{2}:CH\textsubscript{4} selectivity benchmark dataset using the \textit{all} substitution strategy.}\label{netl_co2_ch4_knn_fp_all}
\end{figure}

\begin{figure}[H]
\centering
\includegraphics[width=1\textwidth]{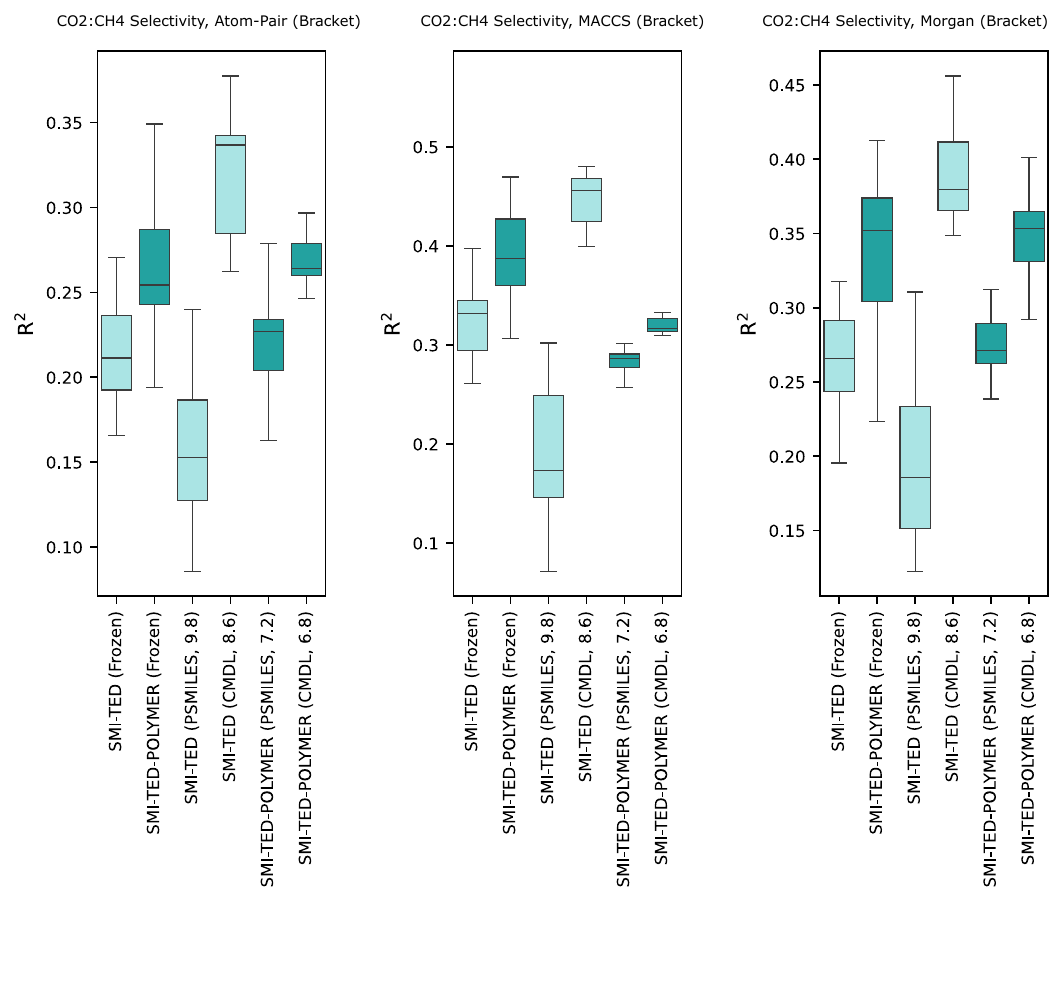}
\caption{Plots of fingerprint R\textsuperscript{2} value distributions for the CO\textsubscript{2}:CH\textsubscript{4} selectivity benchmark dataset using the \textit{bracket} substitution strategy.}\label{netl_co2_ch4_knn_fp_bracket}
\end{figure}

\begin{figure}[H]
\centering
\includegraphics[width=1\textwidth]{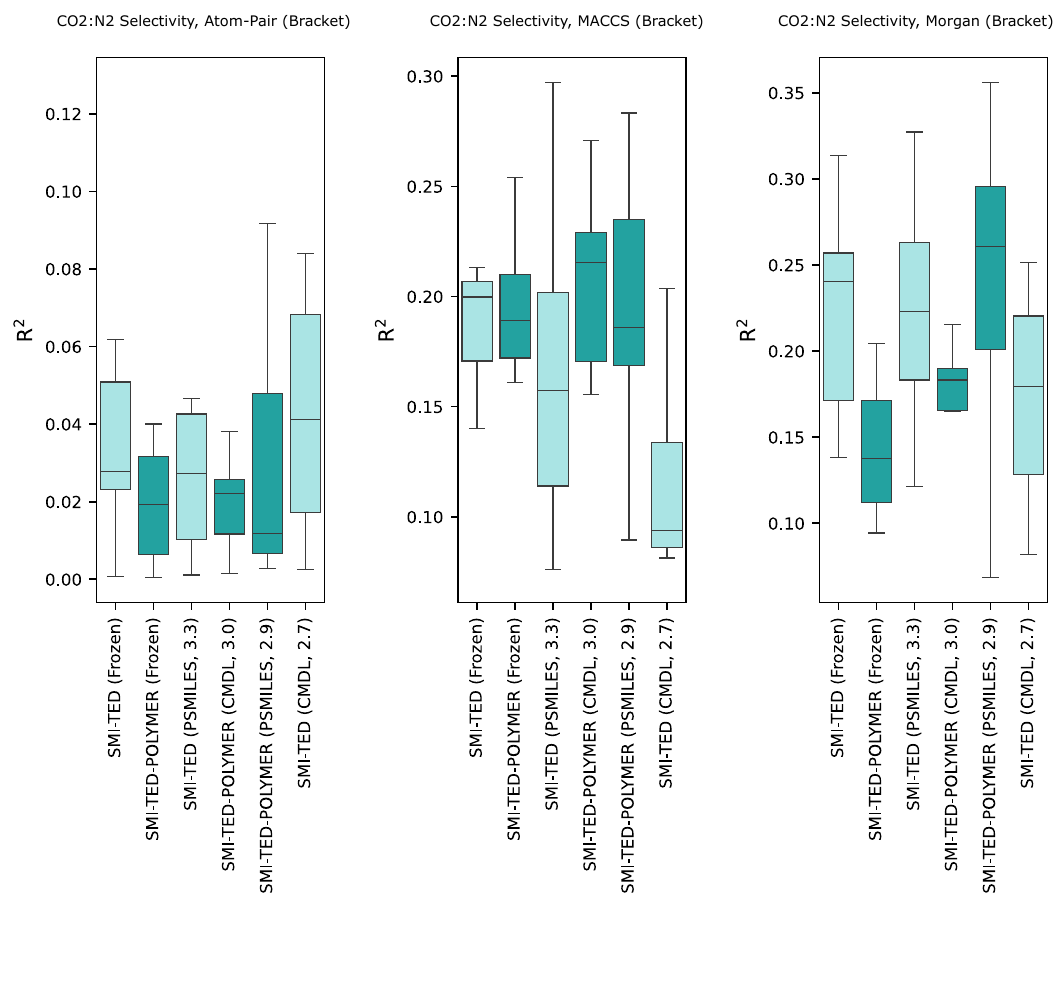}
\caption{Plots of fingerprint R\textsuperscript{2} value distributions for the CO\textsubscript{2}:N\textsubscript{2} selectivity benchmark dataset using the \textit{all} substitution strategy.}\label{netl_co2_n2_knn_fp_all}
\end{figure}

\begin{figure}[H]
\centering
\includegraphics[width=1\textwidth]{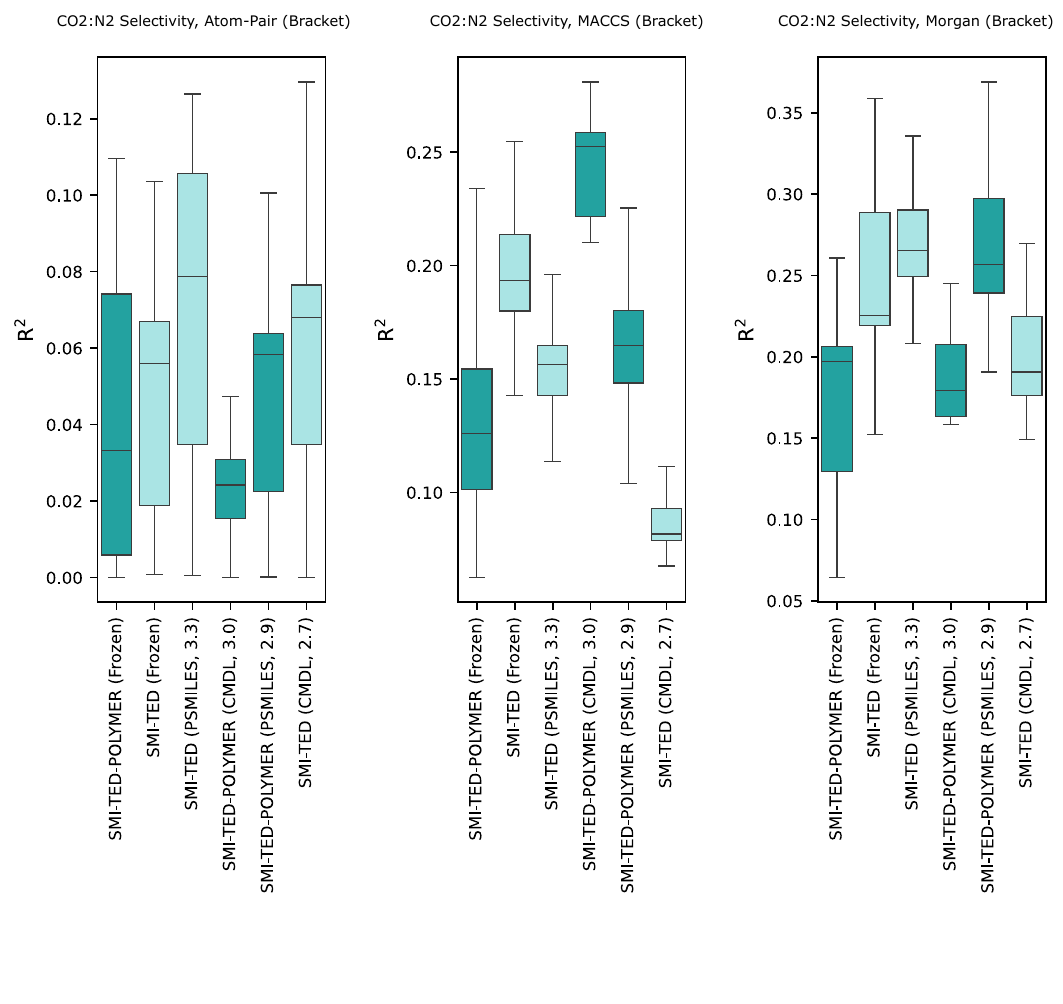}
\caption{Plots of fingerprint R\textsuperscript{2} value distributions for the CO\textsubscript{2}:N\textsubscript{2} selectivity benchmark dataset using the \textit{bracket} substitution strategy.}\label{netl_co2_n2_knn_fp_bracket}
\end{figure}

\subsection{Attention Figures}

\begin{figure}[H]
\centering
\includegraphics[width=1\textwidth]{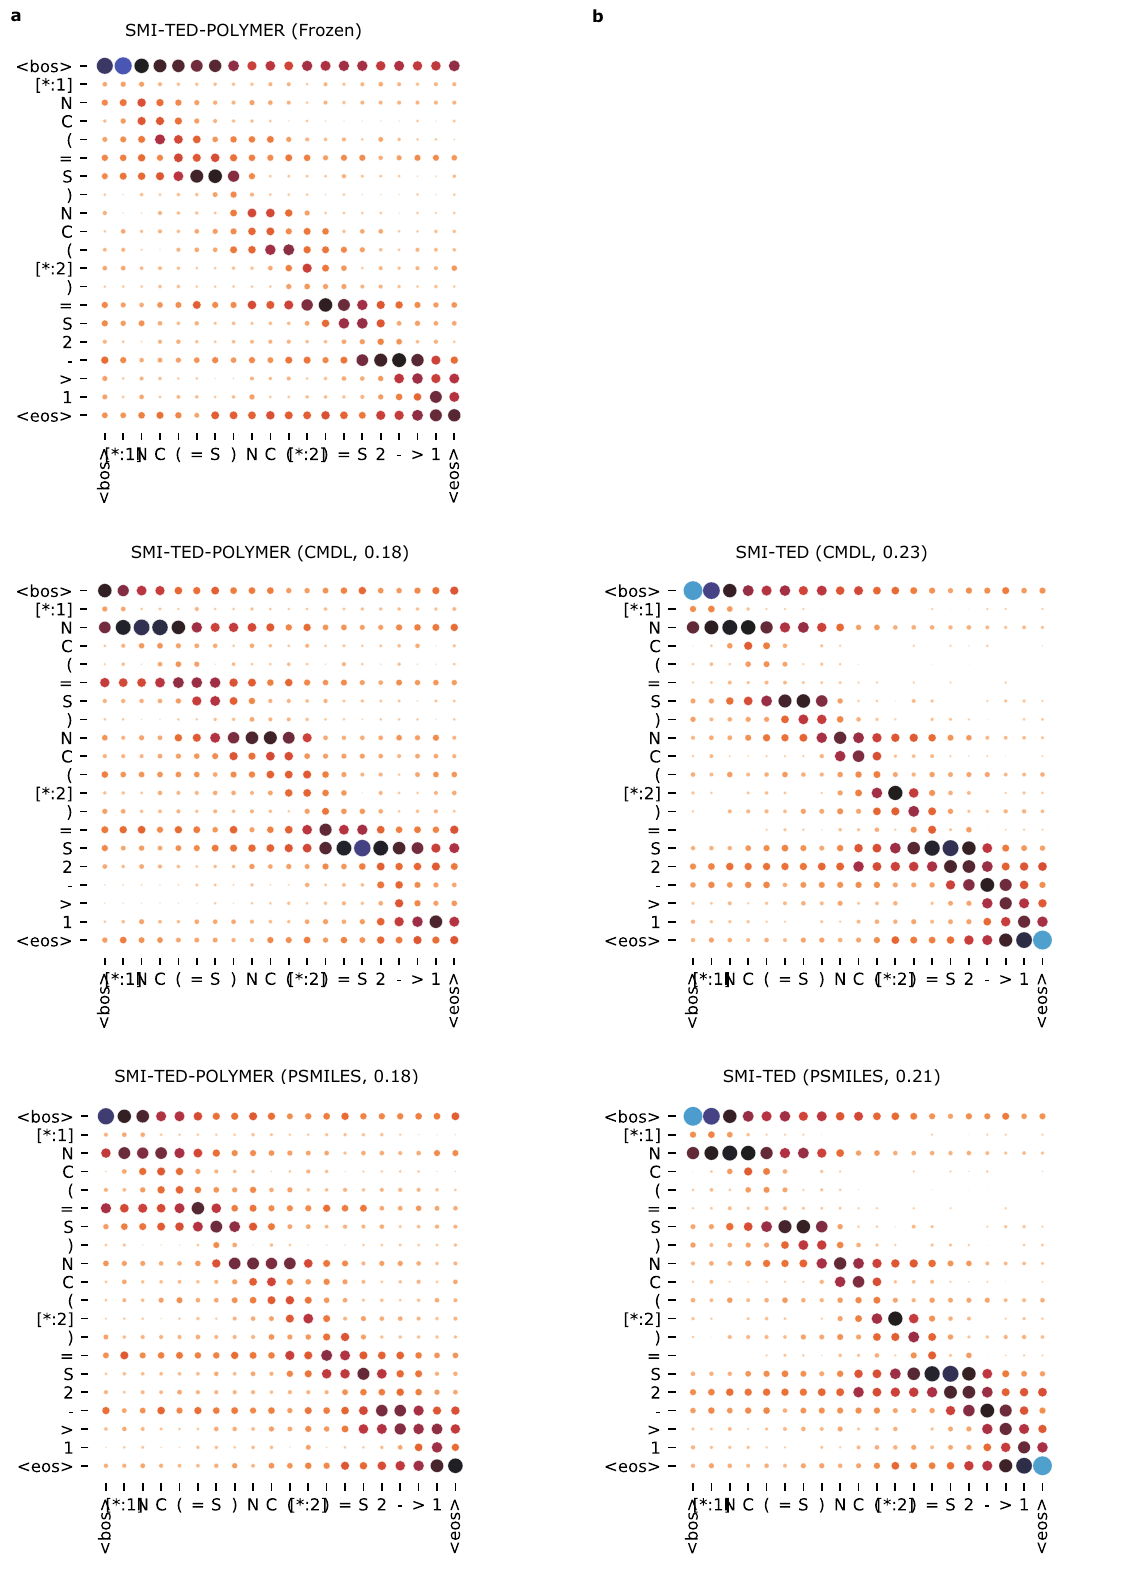}
\caption{Attention maps of CPG representations from the E\textsubscript{ea} dataset.}\label{eea_attn}
\end{figure}

%\begin{figure}[H]
%\centering
%\includegraphics[width=1\textwidth]{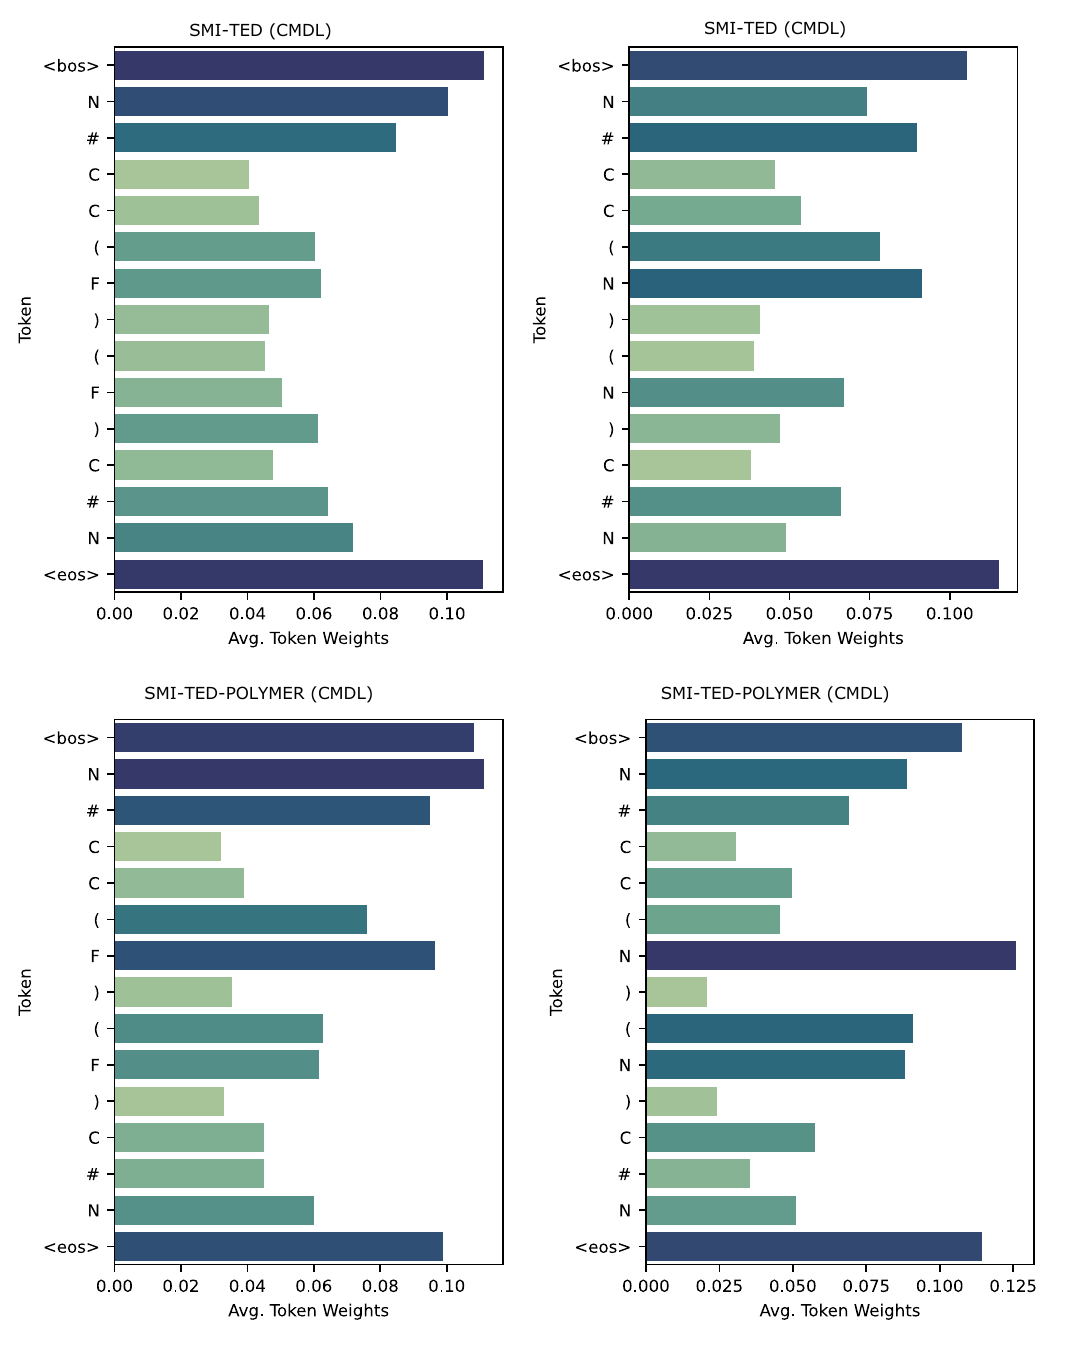}
%\caption{Comparison of average attention probabilities for each token}\label{attn_bar}
%\end{figure}

\begin{figure}[H]
\centering
\includegraphics[width=1\textwidth]{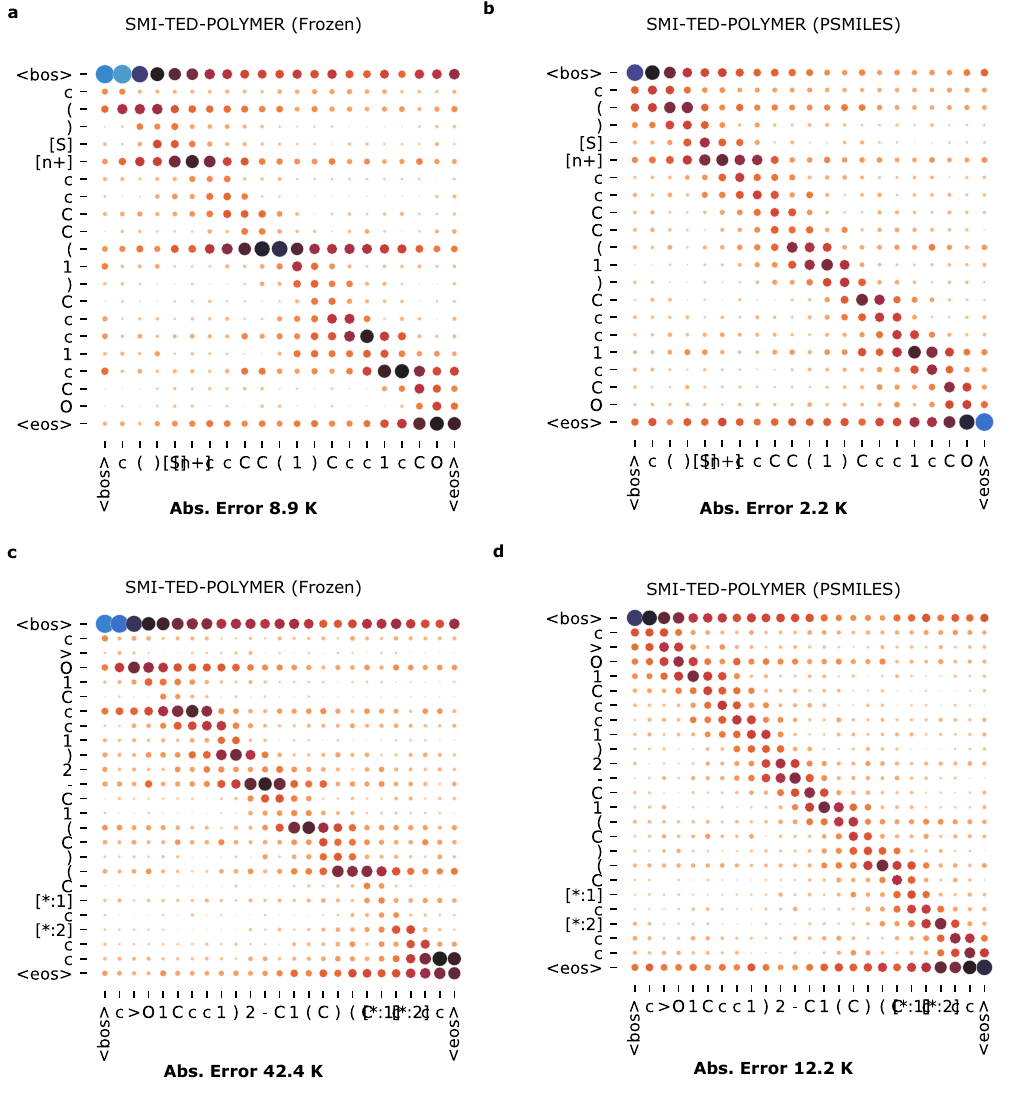}
\caption{Comparison of average attention probabilities for random representations}\label{rand_attn}
\end{figure}

\subsection{Historical Performance Comparisons}

\begin{figure}[H]
\centering
\includegraphics[width=1\textwidth]{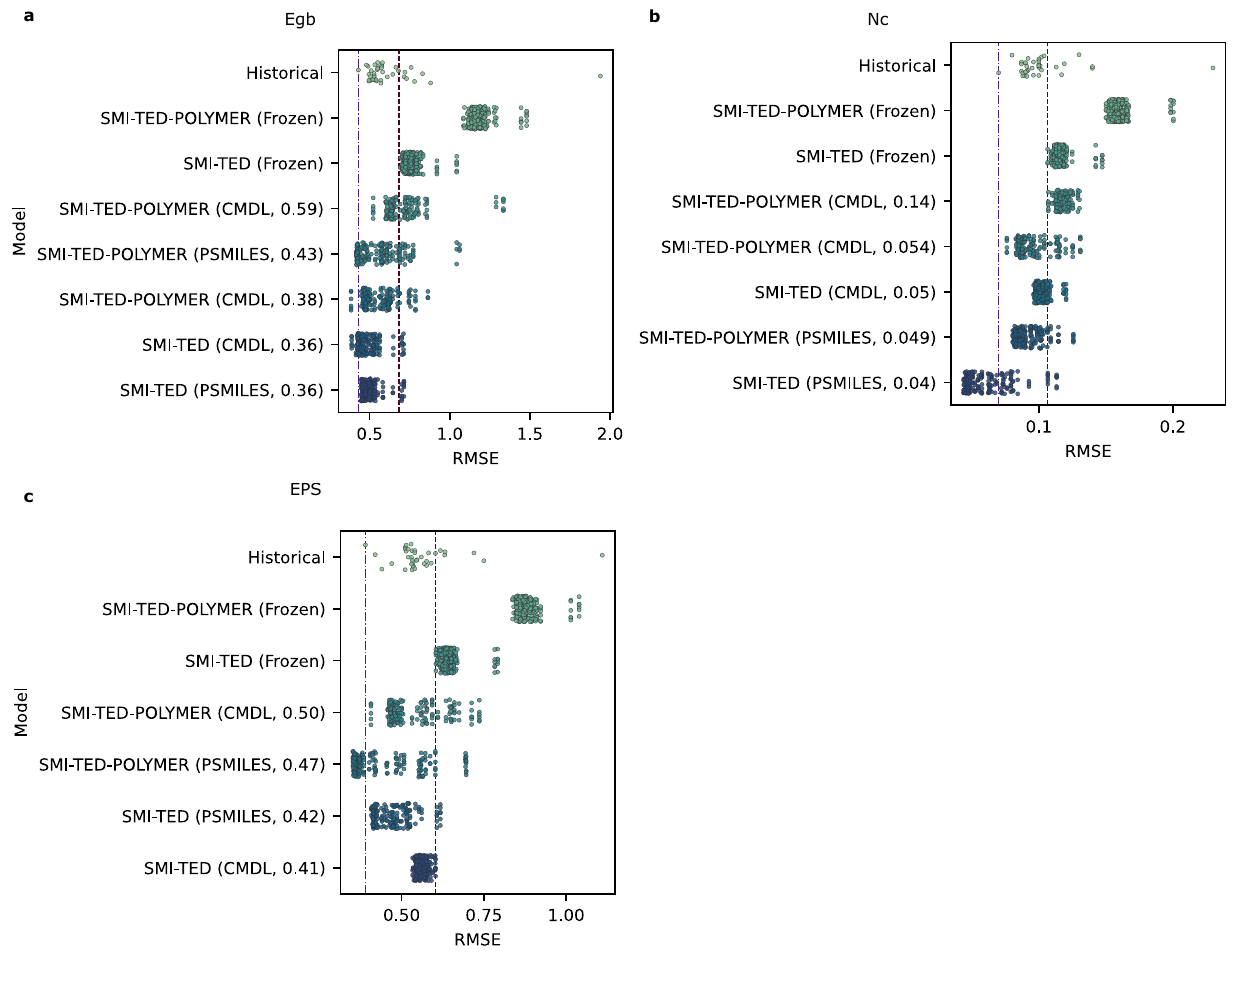}
\caption{Comparison of performance of SMI-TED models with reported historical values.}\label{hist_rmse}
\end{figure}

\subsection{Representation Evaluation Results}\label{rep_eval}

\paragraph{CV Score Box Plot Notes}As noted above not all atom substitutions resulted in valid SMILES strings which cannot be canonicalized. Likewise, not all atom-substitution strategies were used for each replacement atom token (see Supplementary Info~\ref{rep_exp_section}). Hence, no results are plotted in these instances. Special cases, such as the CPG representation, random token (RT), randomly shuffled CPG (RC), or randomly shuffled with random replacement token (RF) are included in all plots for reference. All box plots are plotted as facets of their respective substitution strategy (\textit{all} or \textit{bracket}) and whether or not the newly substituted representations were re-canonicalized (\textit{True} or \textit{False}).

\paragraph{Random Split Point Plot Notes}The point plots show the performance results of evaluation of the random 80:10:10 \textit{train}, \textit{valid}, and \textit{test} splits of the benchmark dataset for each representation and substitution strategy using the hyperparameter optimized XGBoost model. As with the \textit{CV Score Box Plots}, the point plots are plotted as facets, splitting the data by substitution strategy (\textit{all} or \textit{bracket}) and re-canonicalization (\textit{True} or \textit{False}). In all point plots the \textit{train}, \textit{valid}, and \textit{test} results are indicated with blue diamond, black circle, and red square markers, respectively.

\subsubsection{Polymer Chain Bandgap (E\textsubscript{gc}) CV Scores}\label{cvEgc}

\begin{figure}[H]
\centering
\includegraphics[width=1\textwidth]{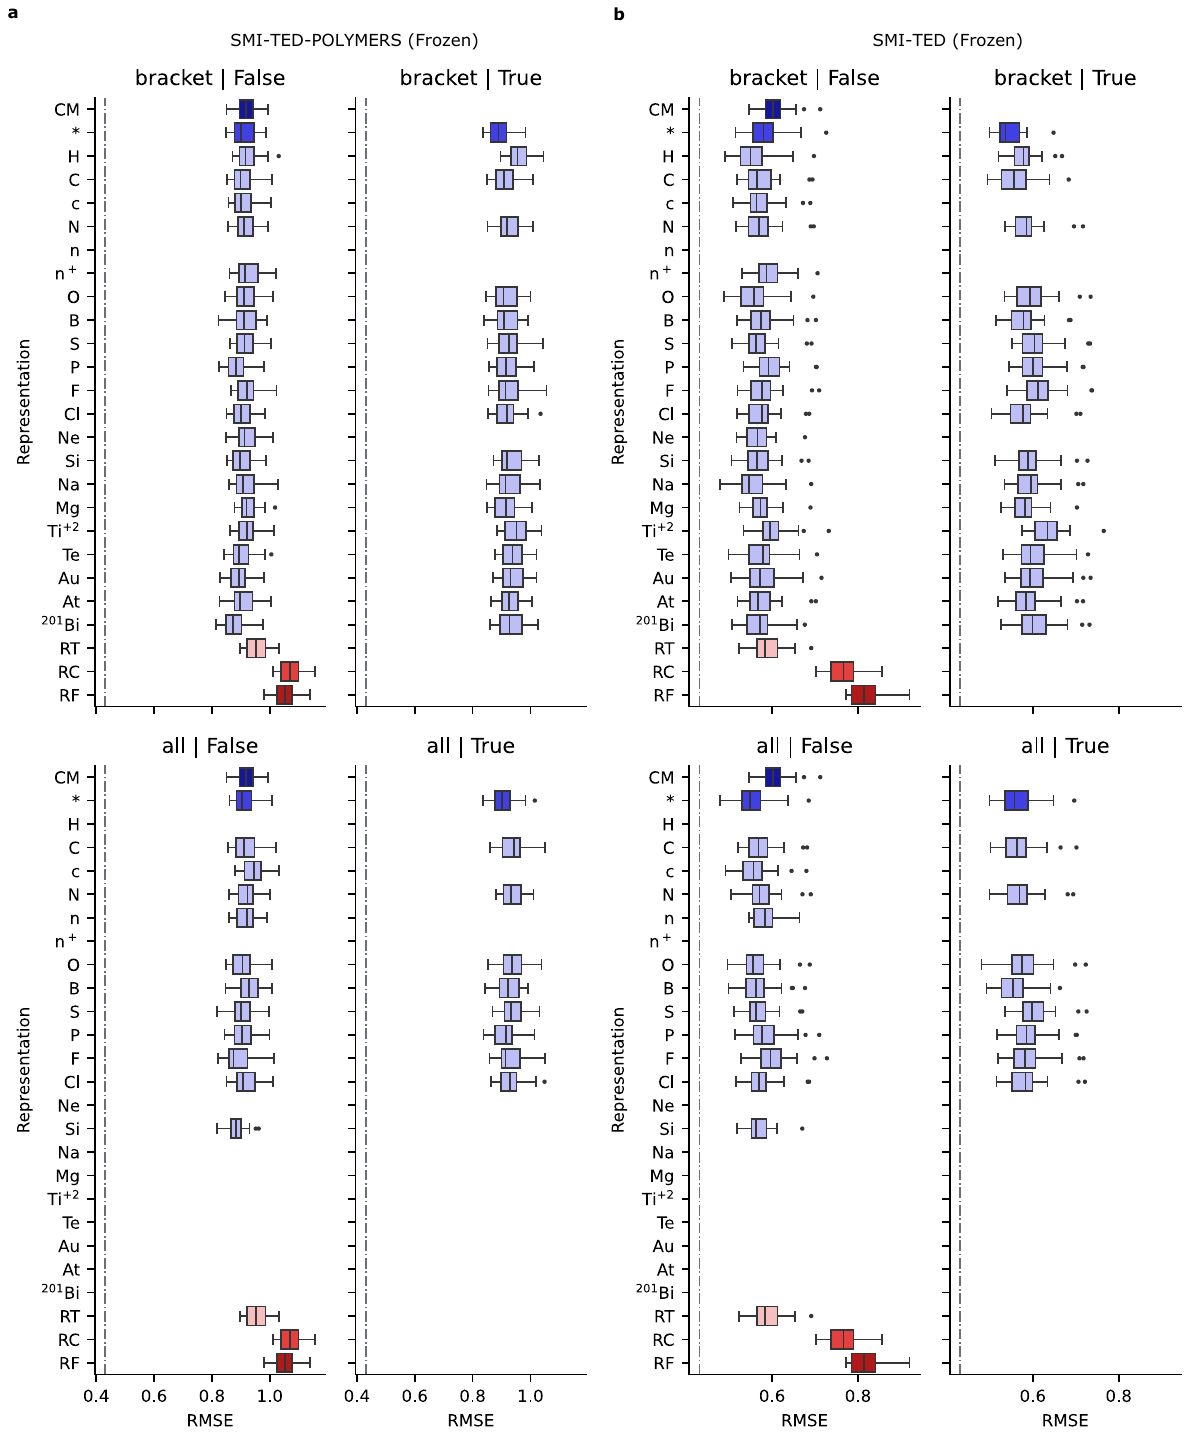}
\caption{Box plots for E\textsubscript{gc} repeated cross-validation experiments for SMI-TED-POLYMER (\textbf{a}) and SMI-TED (\textbf{b}) models with frozen weights.}\label{egc_token_box_frozen}
\end{figure}

\begin{figure}[H]
\centering
\includegraphics[width=1\textwidth]{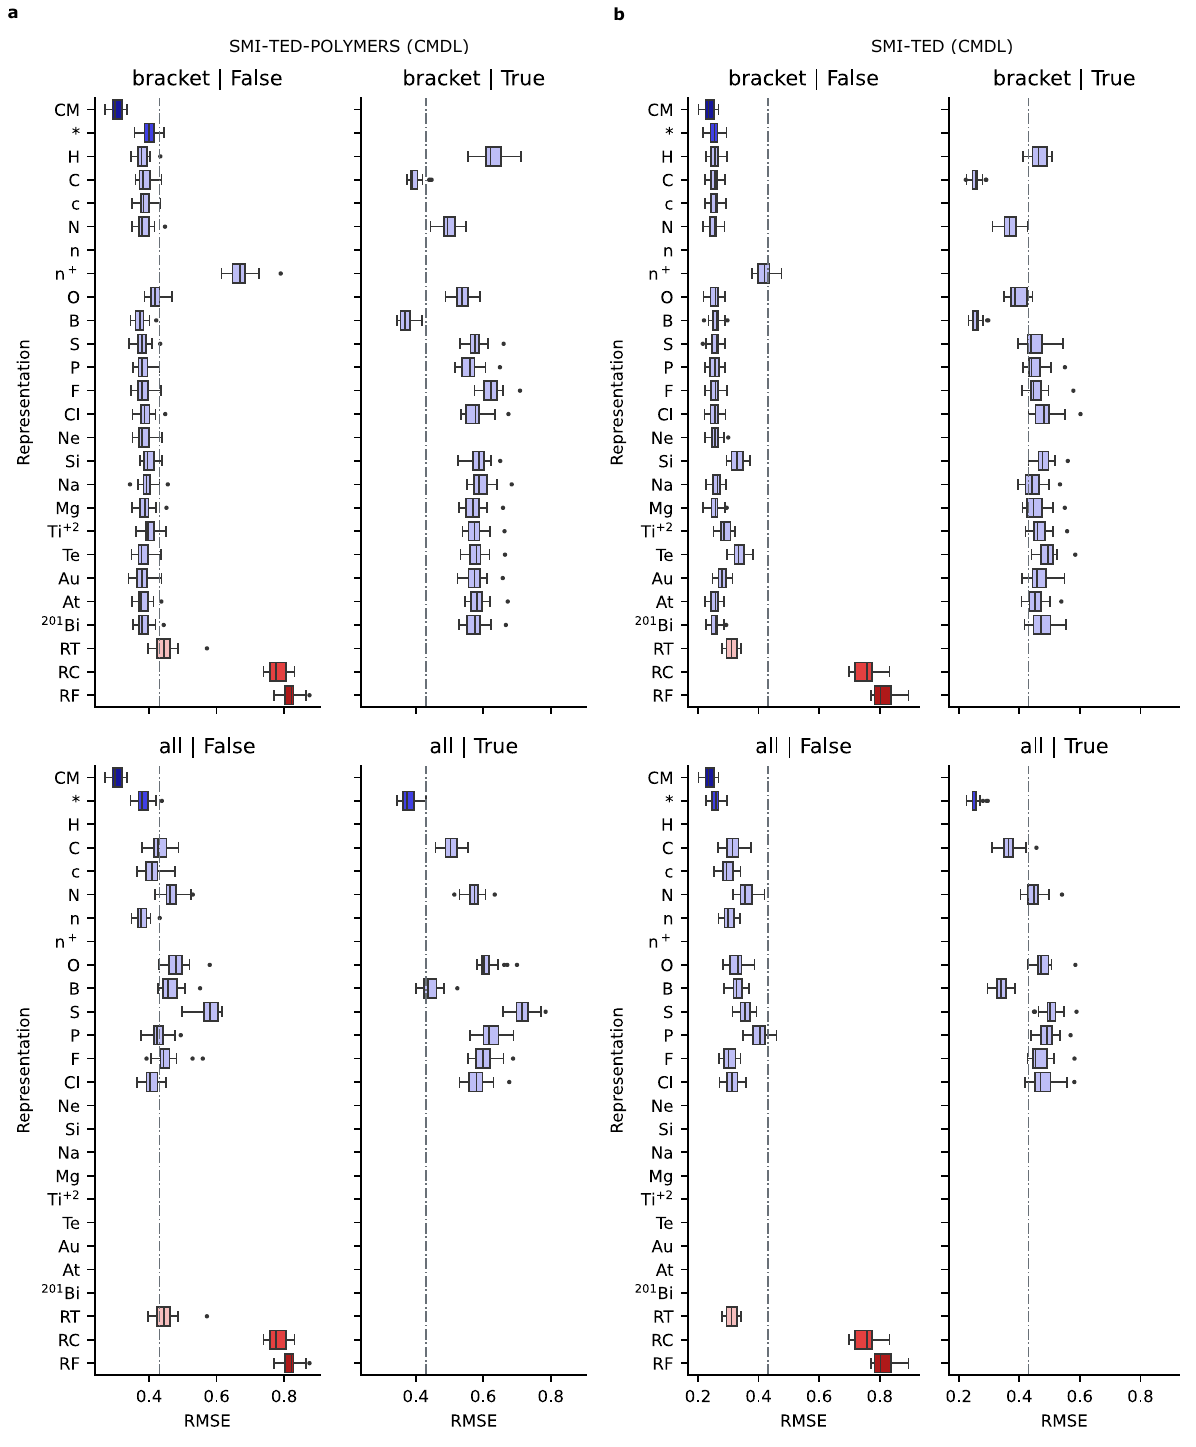}
\caption{Box plots for E\textsubscript{gc} repeated cross-validation experiments for SMI-TED-POLYMER (\textbf{a}) and SMI-TED (\textbf{b}) models fine-tuned with the CPG polymer graphs.}\label{egc_token_box_cmdl}
\end{figure}

\begin{figure}[H]
\centering
\includegraphics[width=1\textwidth]{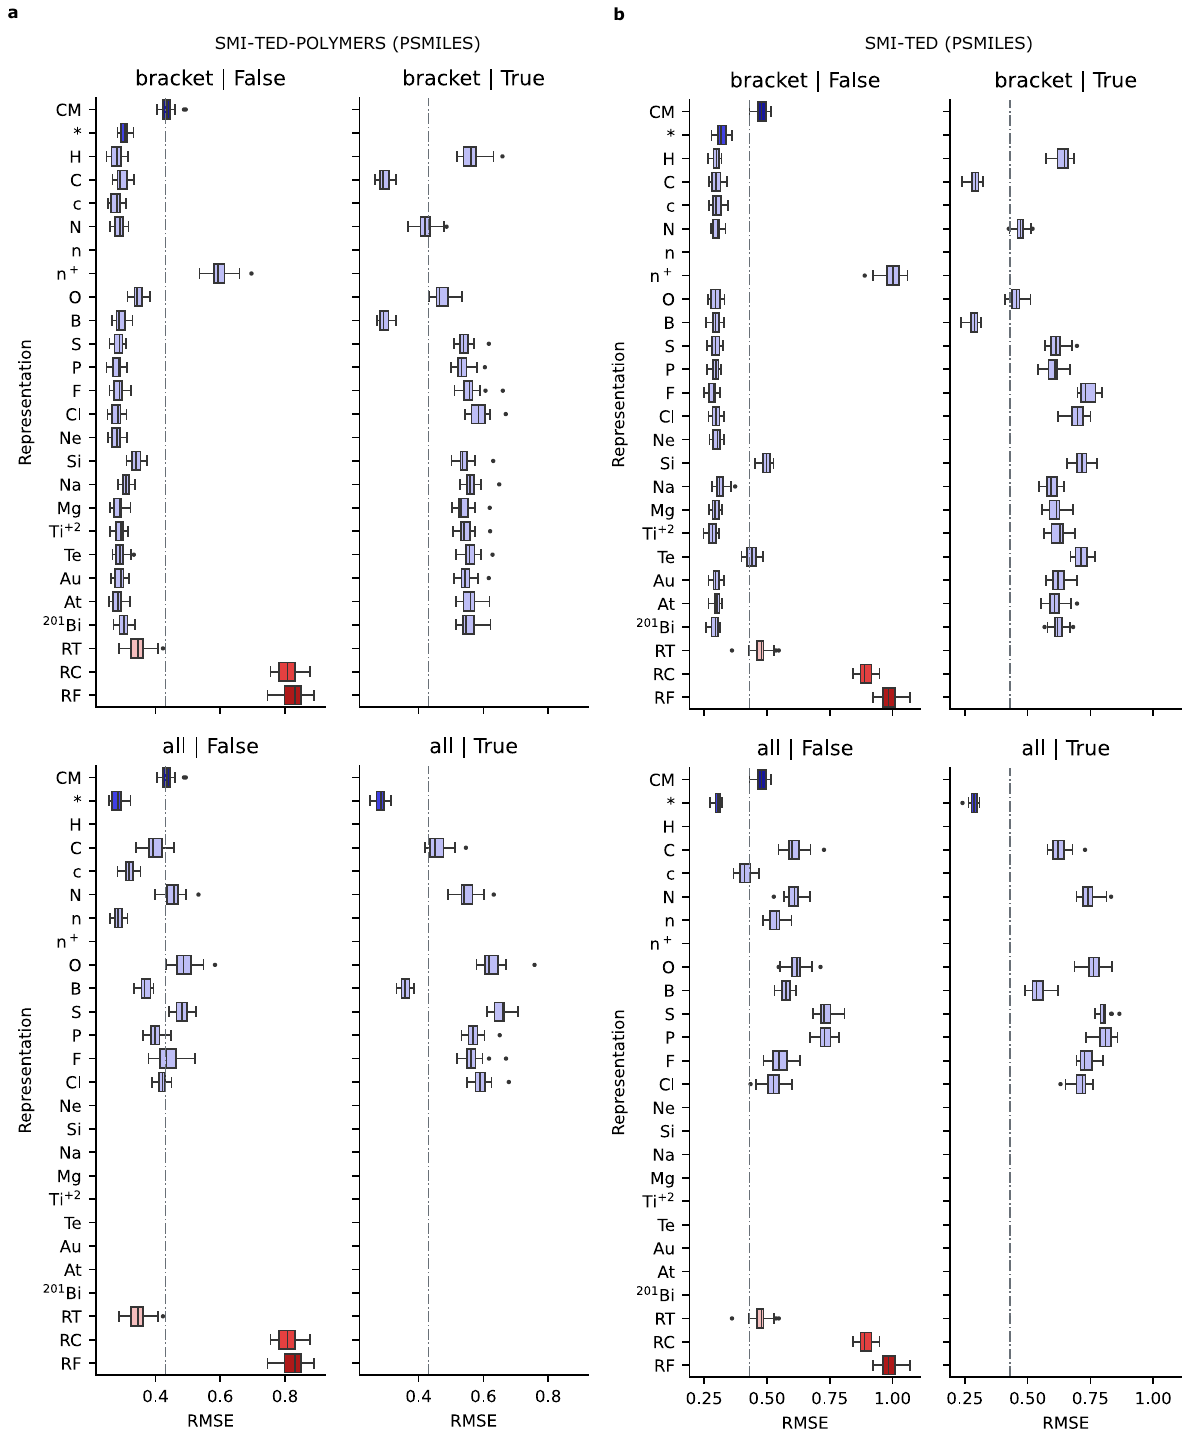}
\caption{Box plots for E\textsubscript{gc} repeated cross-validation experiments for SMI-TED-POLYMER (\textbf{a}) and SMI-TED (\textbf{b}) models fine-tuned with PSMILES.}\label{egc_token_box_psmiles}
\end{figure}

\subsubsection{Polymer Chain Bandgap (E\textsubscript{gc}) Random Split Scores}\label{rsEgc}

\begin{figure}[H]
\centering
\includegraphics[width=1\textwidth]{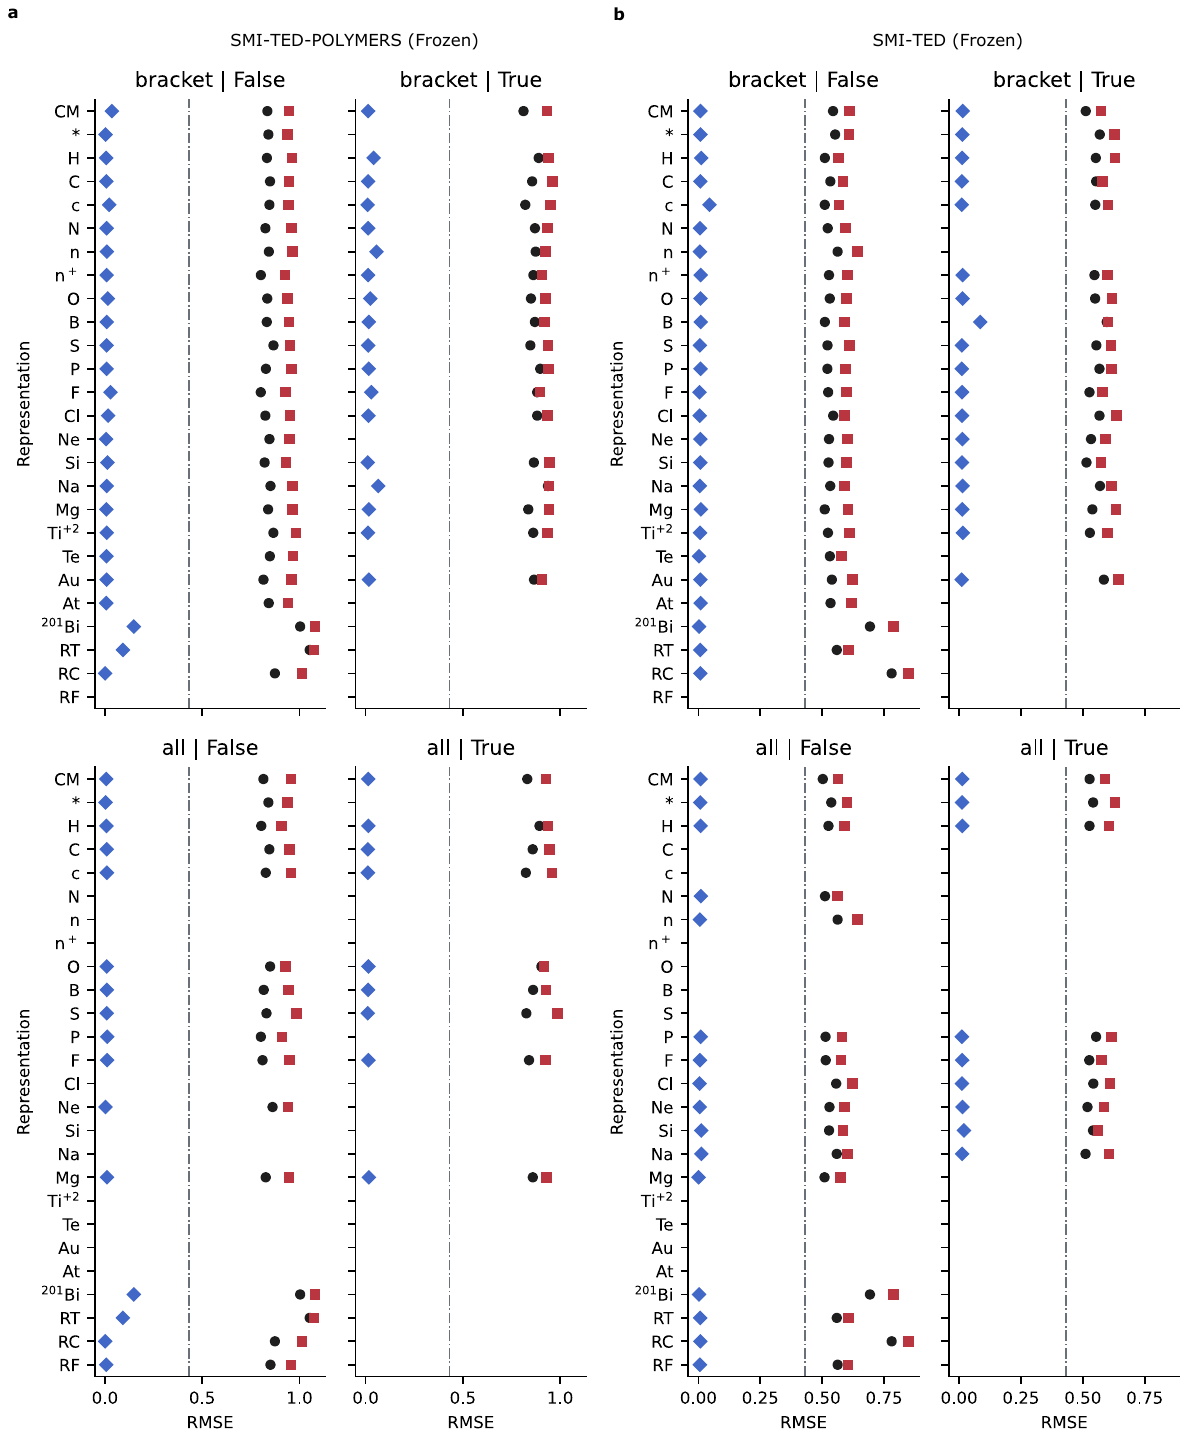}
\caption{Point plots for E\textsubscript{gc} benchmark experiments of RMSE using the base random train, valid, and test splits for SMI-TED-POLYMER (\textbf{a}) and SMI-TED (\textbf{b}) models with frozen weights.}\label{egc_token_point_frozen_rmse}
\end{figure}

\begin{figure}[H]
\centering
\includegraphics[width=1\textwidth]{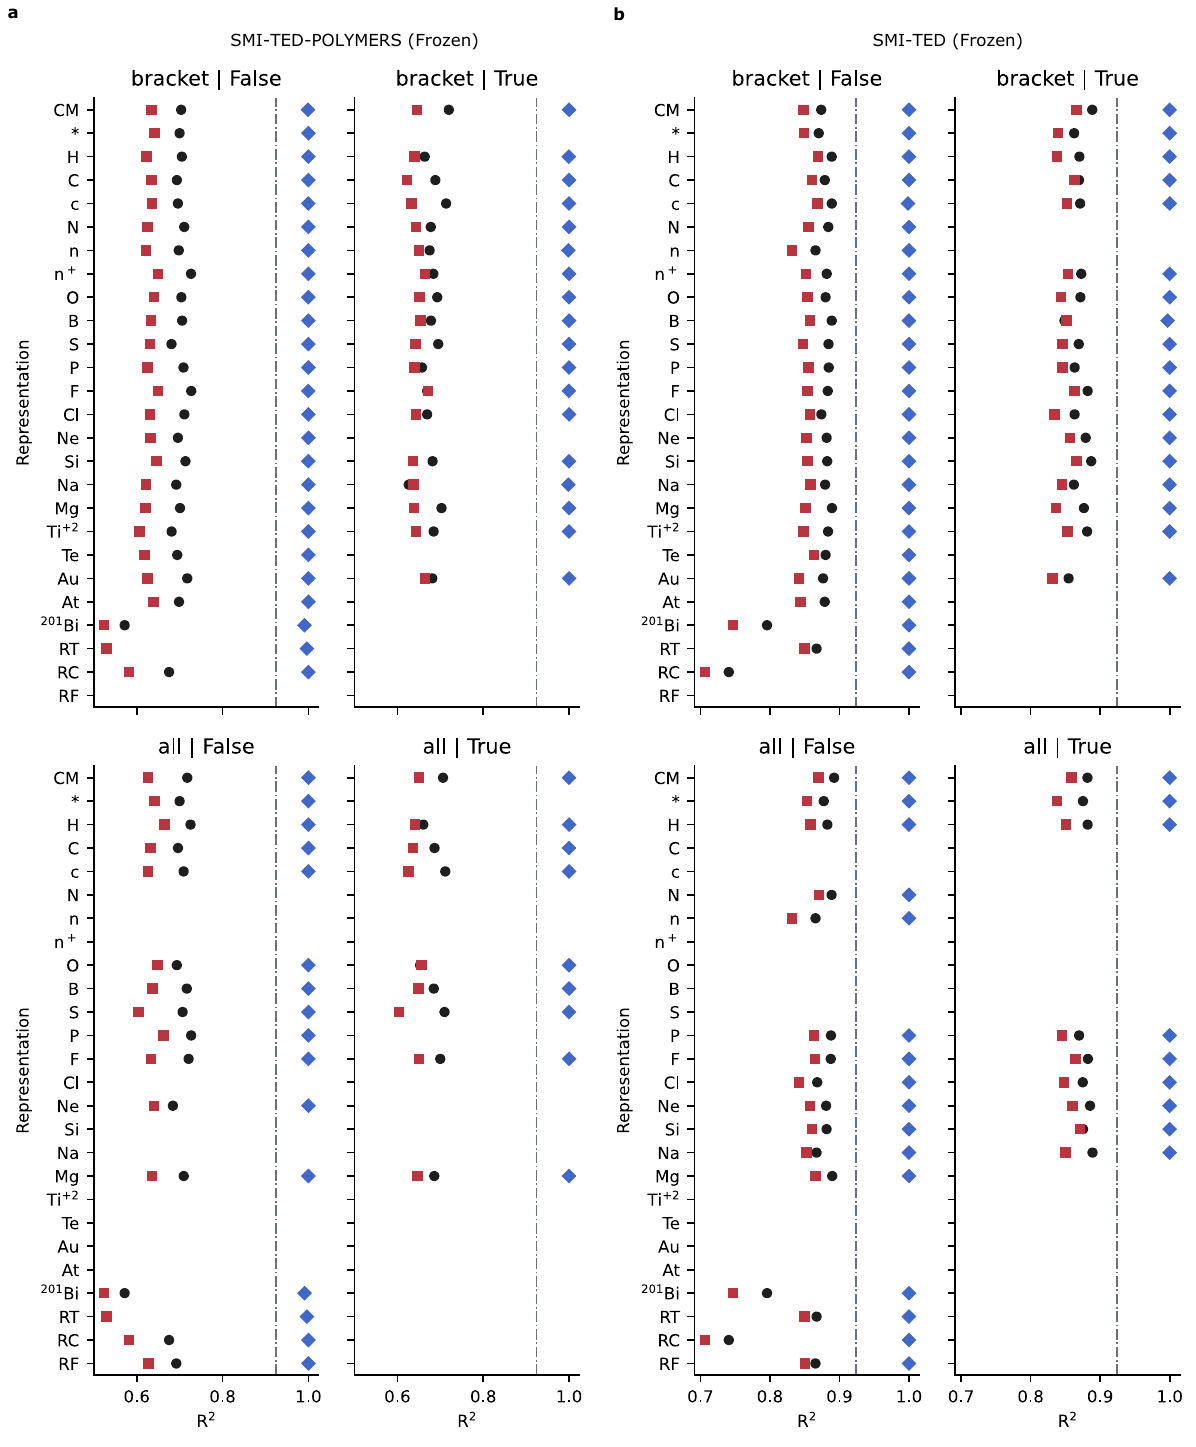}
\caption{Point plots for E\textsubscript{gc} benchmark experiments of R\textsuperscript{2} using the base random train, valid, and test splits for SMI-TED-POLYMER (\textbf{a}) and SMI-TED (\textbf{b}) models with frozen weights.}\label{egc_token_point_frozen_r2}
\end{figure}

\begin{figure}[H]
\centering
\includegraphics[width=1\textwidth]{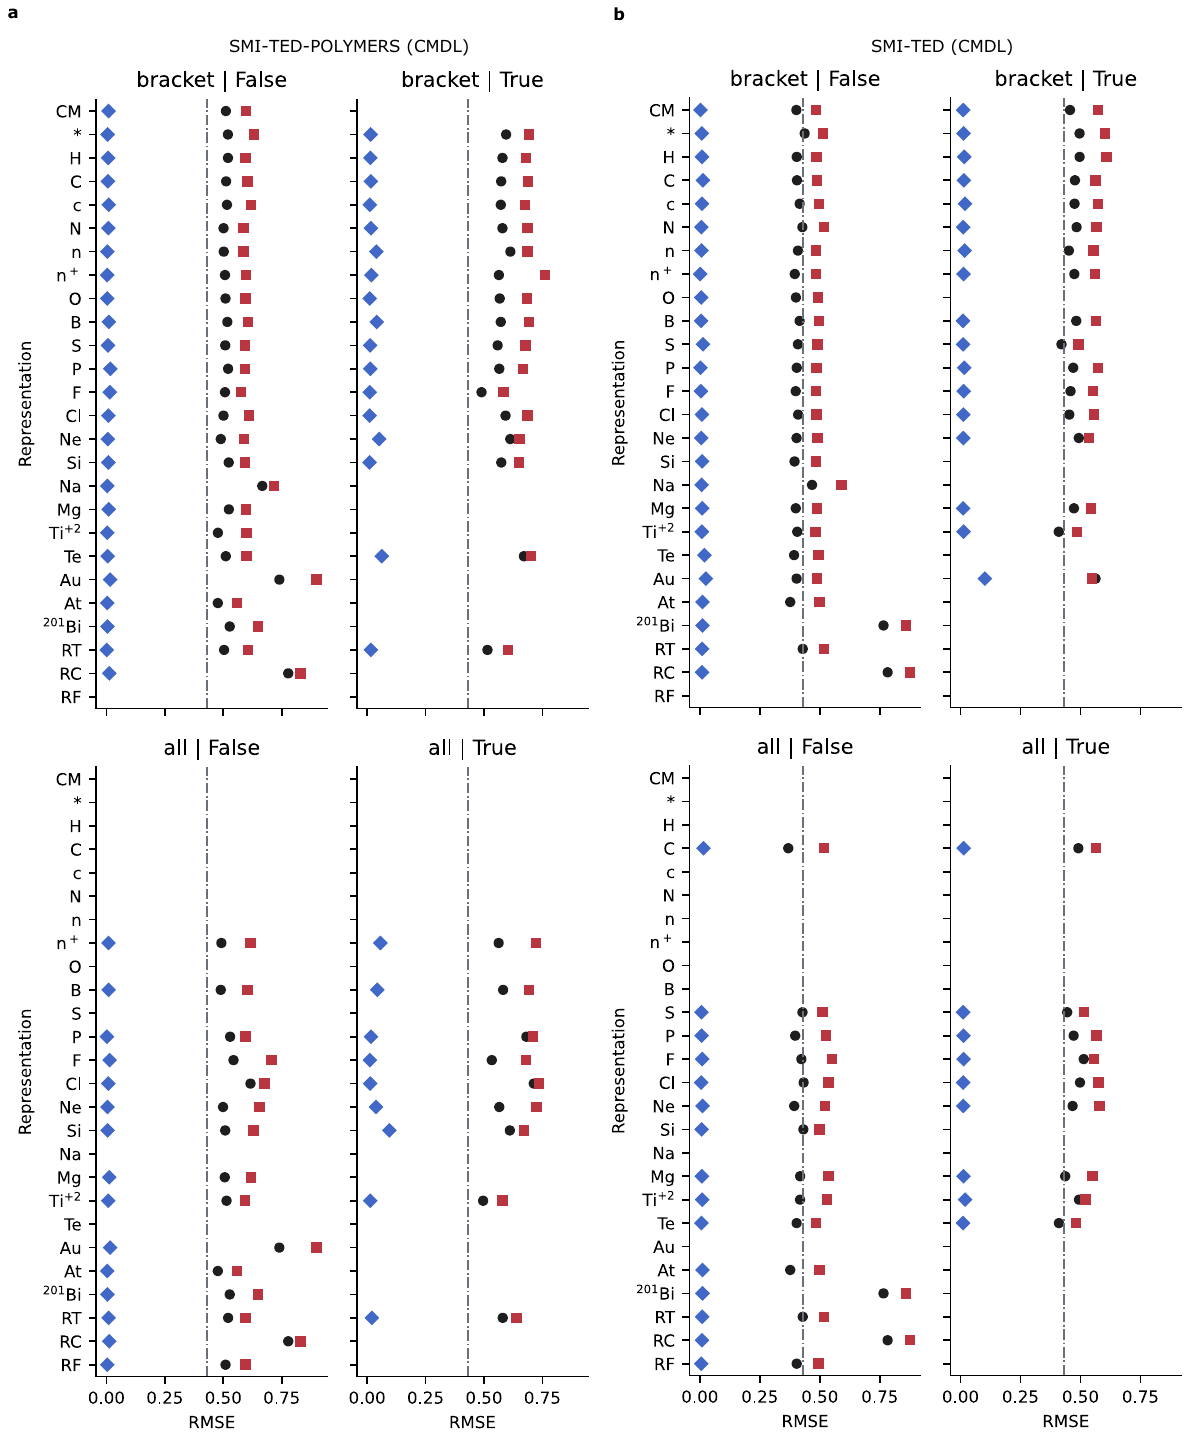}
\caption{Point plots for E\textsubscript{gc} benchmark experiments of RMSE using the base random train, valid, and test splits for SMI-TED-POLYMER (\textbf{a}) and SMI-TED (\textbf{b}) models fine-tuned using the CPG representation.}\label{egc_token_point_cmdl_rmse}
\end{figure}

\begin{figure}[H]
\centering
\includegraphics[width=1\textwidth]{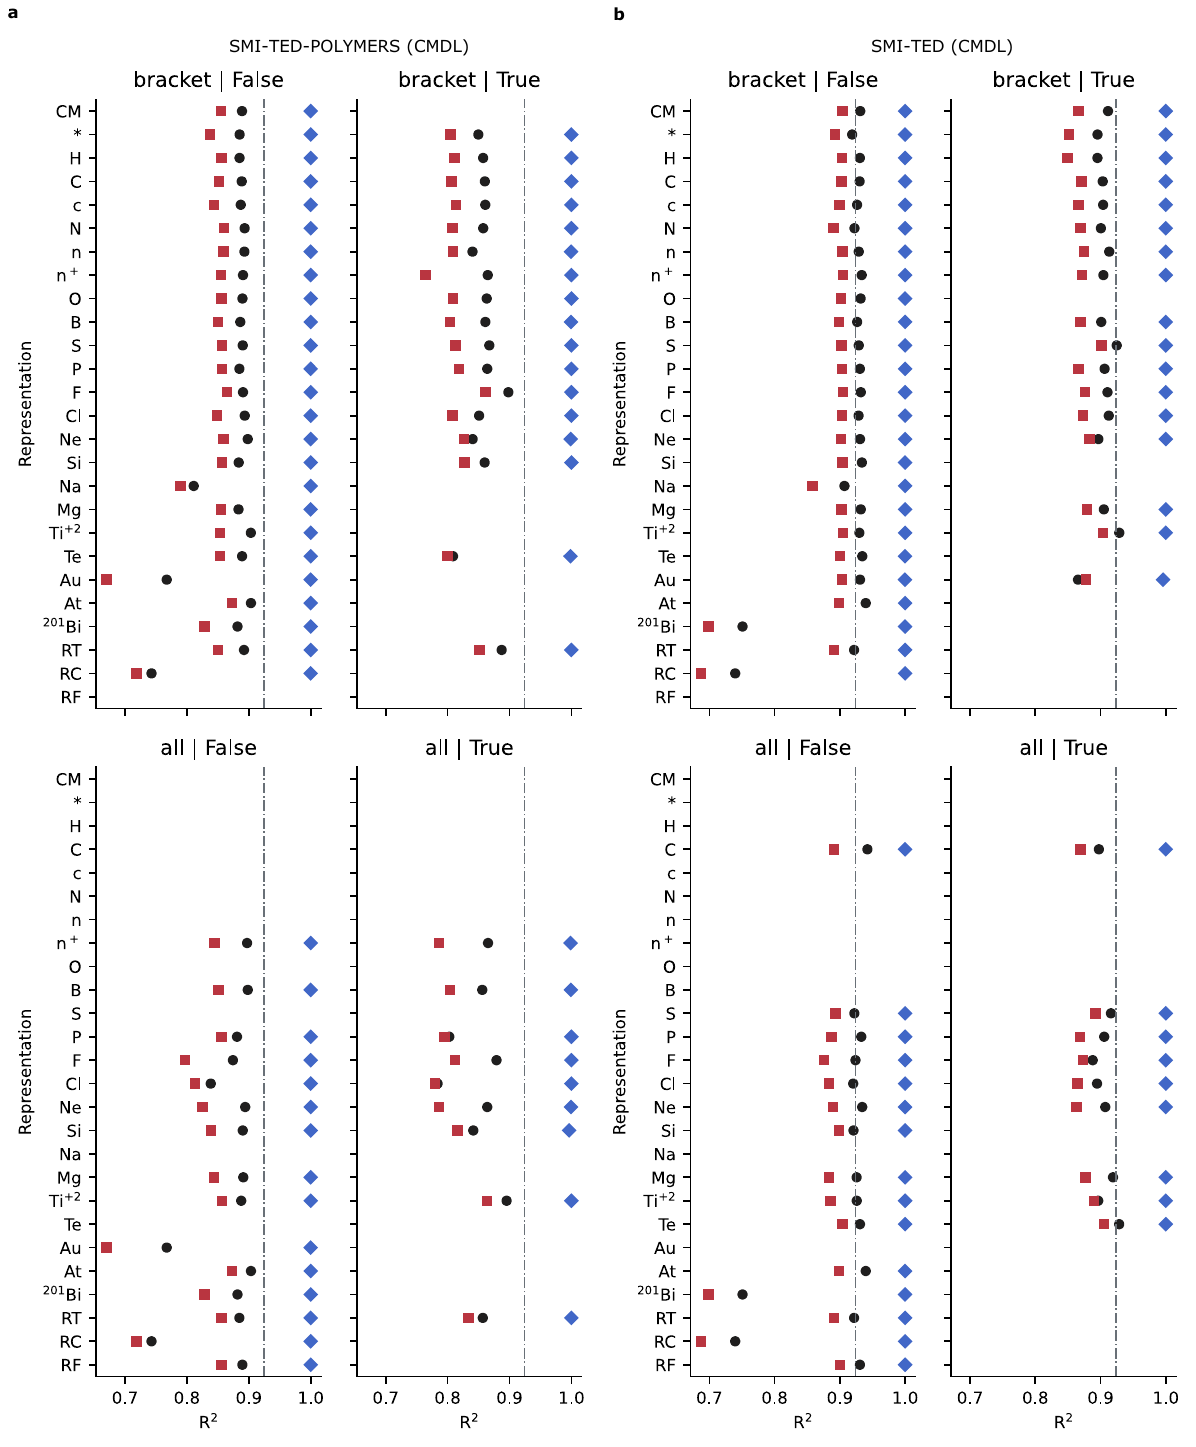}
\caption{Point plots for E\textsubscript{gc} benchmark experiments of R\textsuperscript{2} using the base random train, valid, and test splits for SMI-TED-POLYMER (\textbf{a}) and SMI-TED (\textbf{b}) models fine-tuned using the CPG representation.}\label{egc_token_point_cmdl_r2}
\end{figure}

\begin{figure}[H]
\centering
\includegraphics[width=1\textwidth]{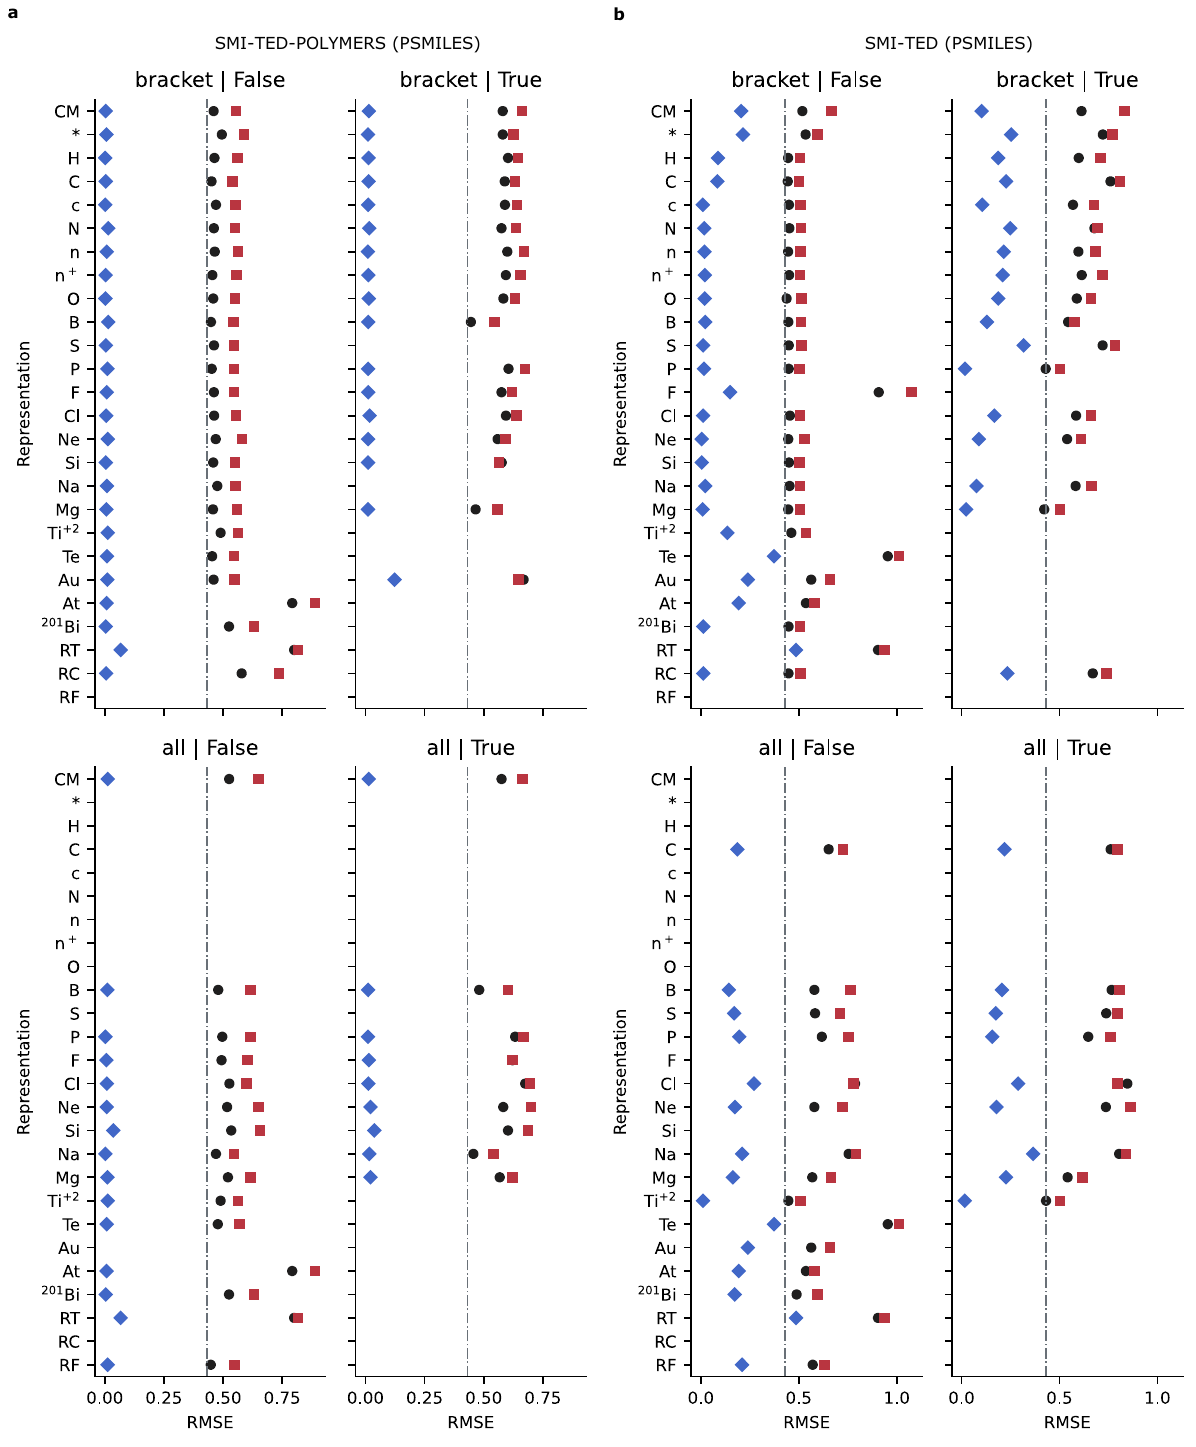}
\caption{Point plots for E\textsubscript{gc} benchmark experiments of RMSE using the base random train, valid, and test splits for SMI-TED-POLYMERS (\textbf{a}) and SMI-TED (\textbf{b}) models fine-tuned using PSMILES.}\label{egc_token_point_psmiles_rmse}
\end{figure}

\begin{figure}[H]
\centering
\includegraphics[width=1\textwidth]{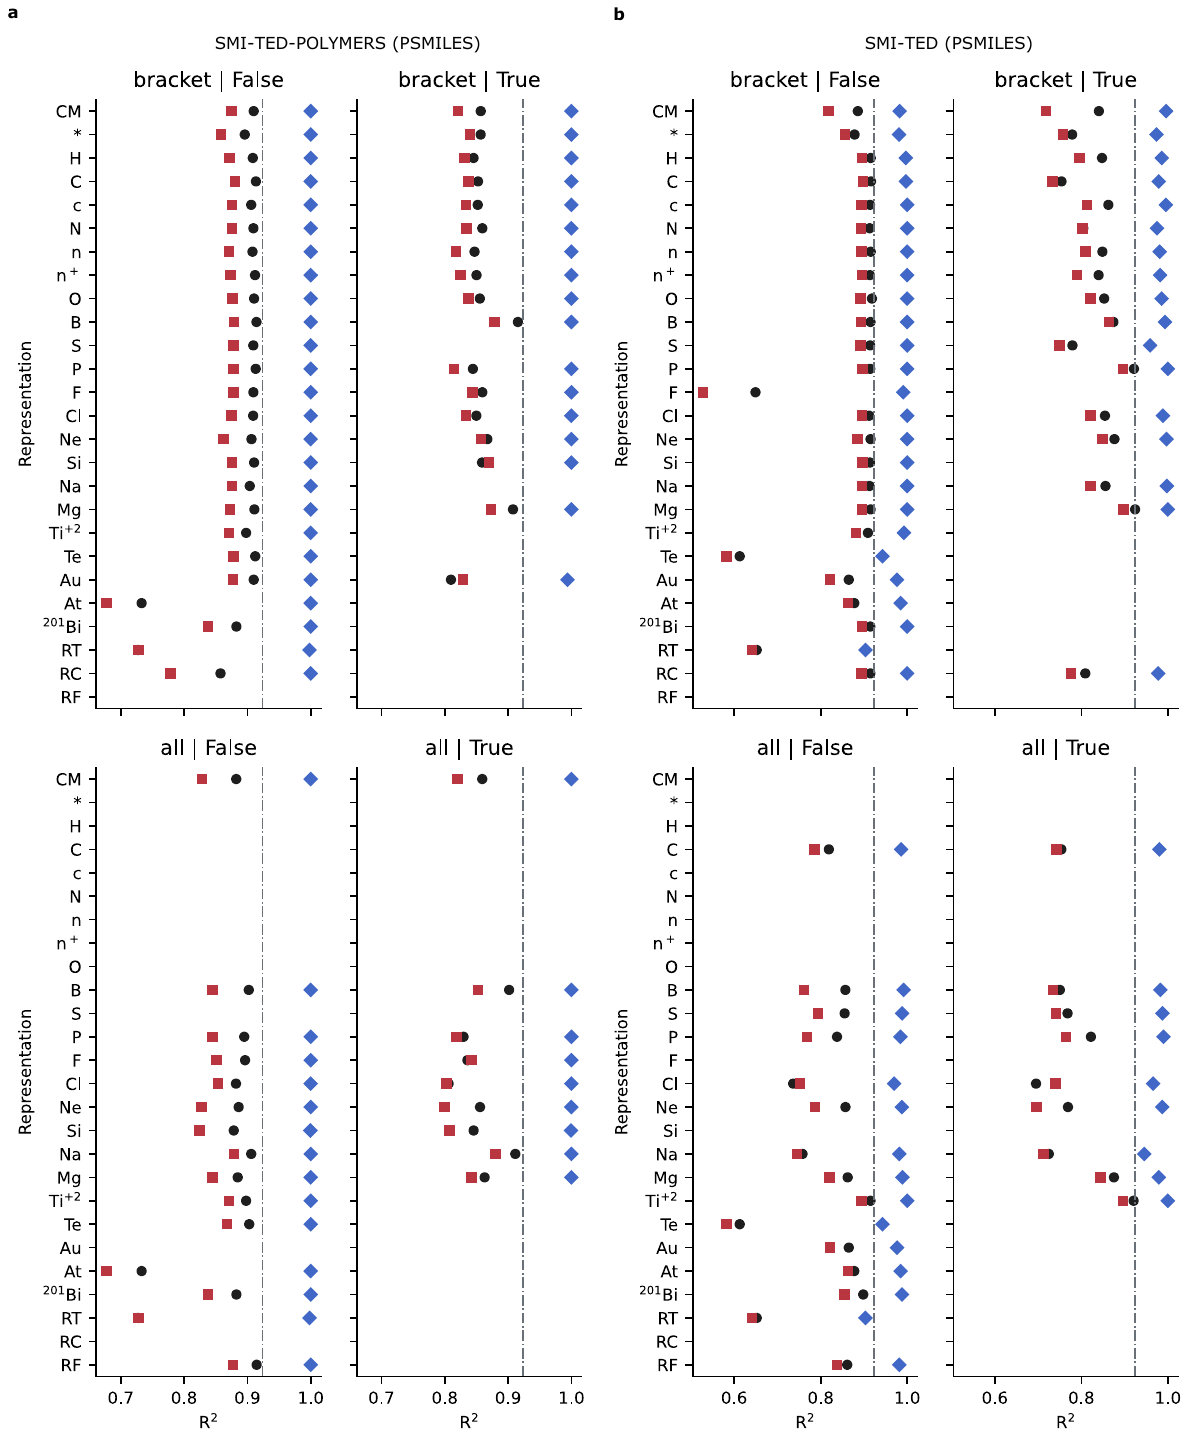}
\caption{Point plots for E\textsubscript{gc} benchmark experiments of R\textsuperscript{2} using the base random train, valid, and test splits for SMI-TED-POLYMERS (\textbf{a}) and SMI-TED (\textbf{b}) models fine-tuned using PSMILES.}\label{egc_token_point_psmiles_r2}
\end{figure}

\subsubsection{Polymer Bulk Bandgap (E\textsubscript{gb}) CV Scores}\label{cvEgb}

\begin{figure}[H]
\centering
\includegraphics[width=1\textwidth]{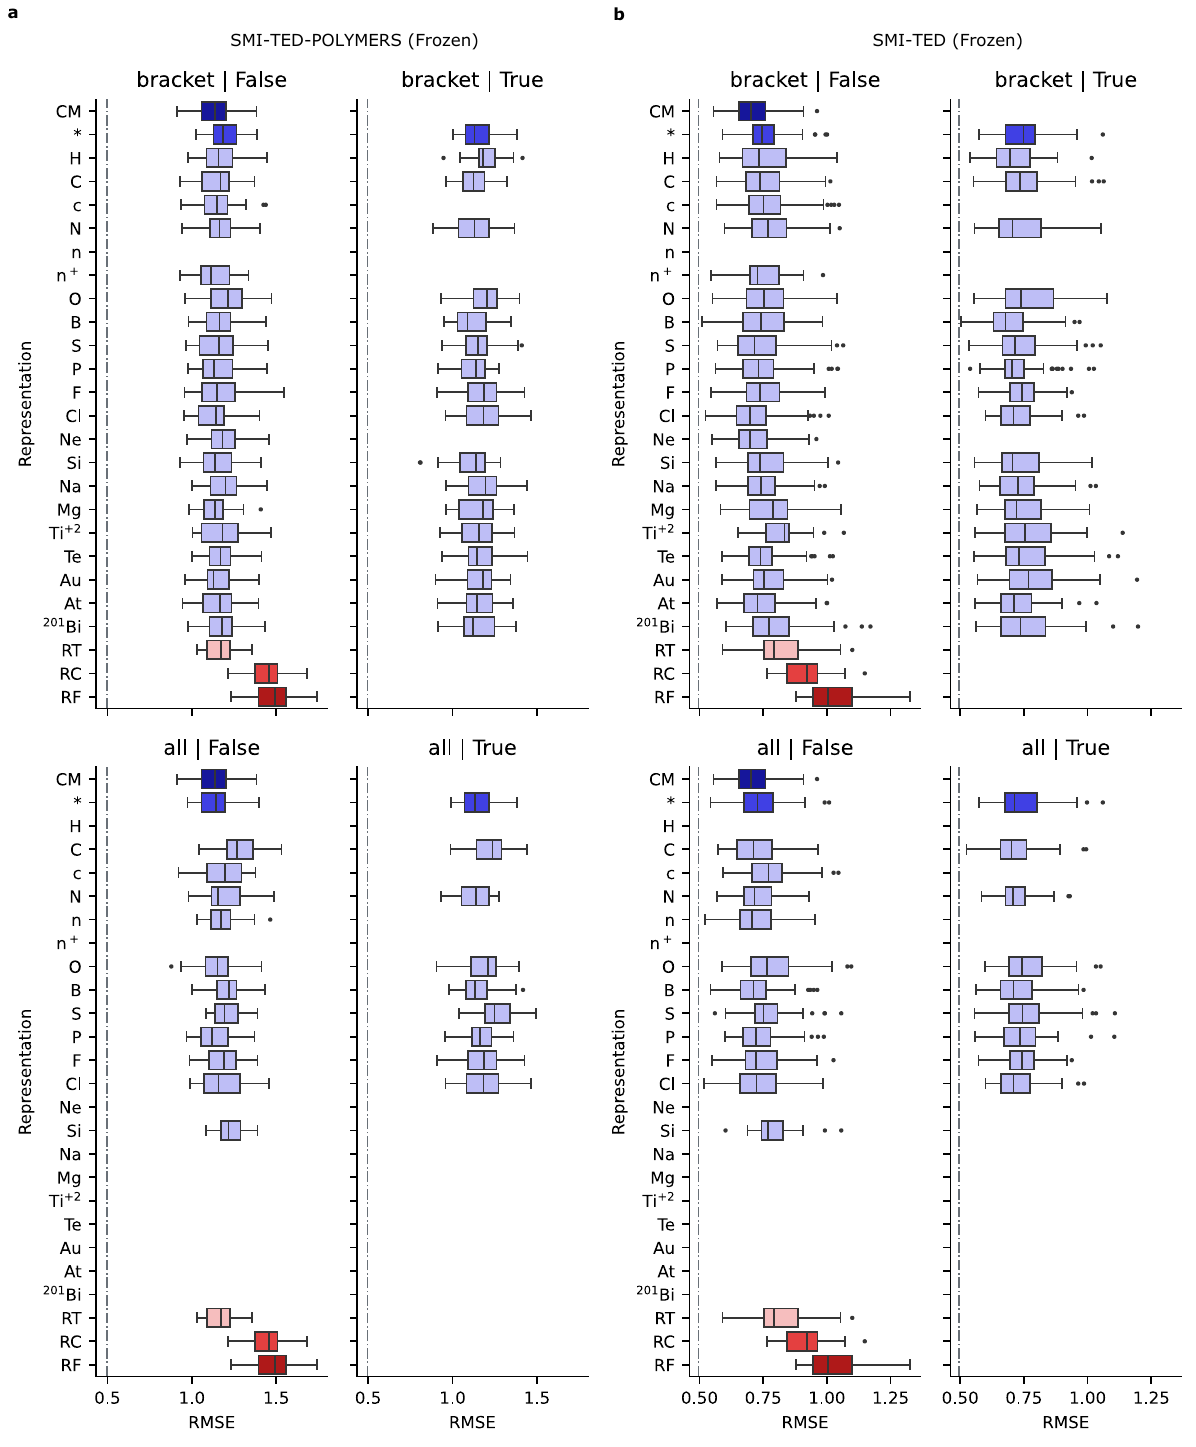}
\caption{Box plots for E\textsubscript{gb} repeated cross-validation experiments for SMI-TED-POLYMER (\textbf{a}) and SMI-TED (\textbf{b}) models with frozen weights.}\label{egb_token_box_frozen}
\end{figure}

\begin{figure}[H]
\centering
\includegraphics[width=1\textwidth]{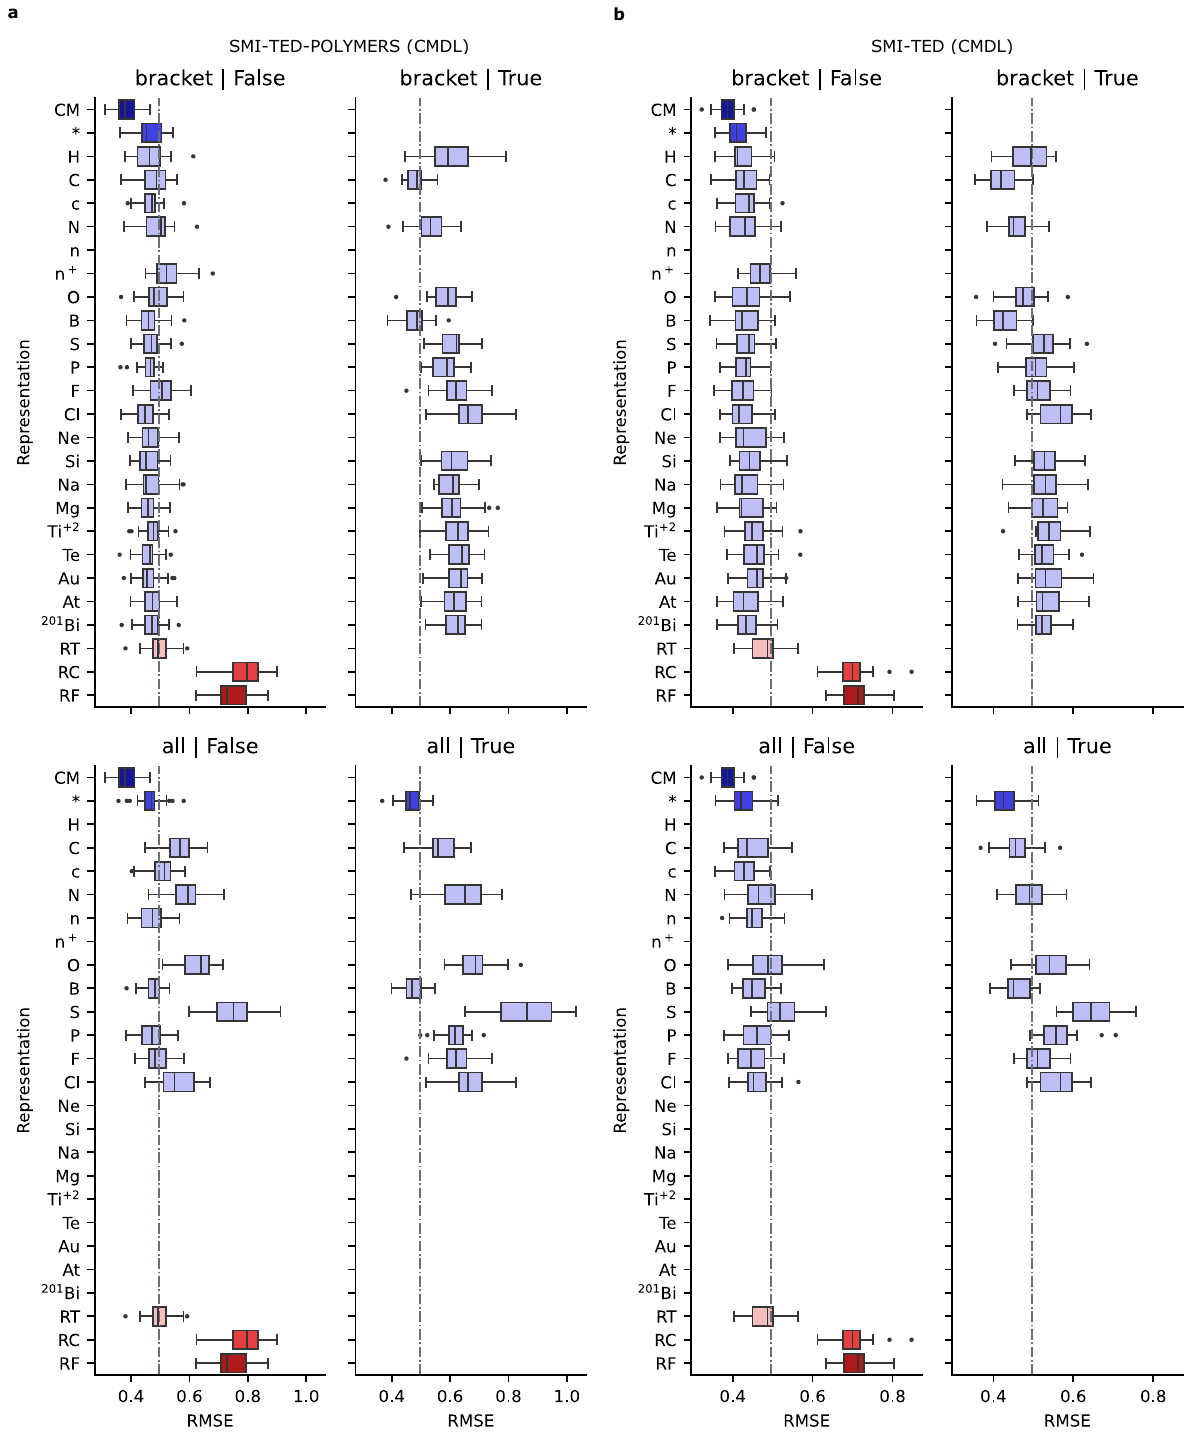}
\caption{Box plots for E\textsubscript{gb} repeated cross-validation experiments for SMI-TED-POLYMER (\textbf{a}) and SMI-TED (\textbf{b}) models fine-tuned with the CPG polymer graphs.}\label{egb_token_box_cmdl}
\end{figure}

\begin{figure}[H]
\centering
\includegraphics[width=1\textwidth]{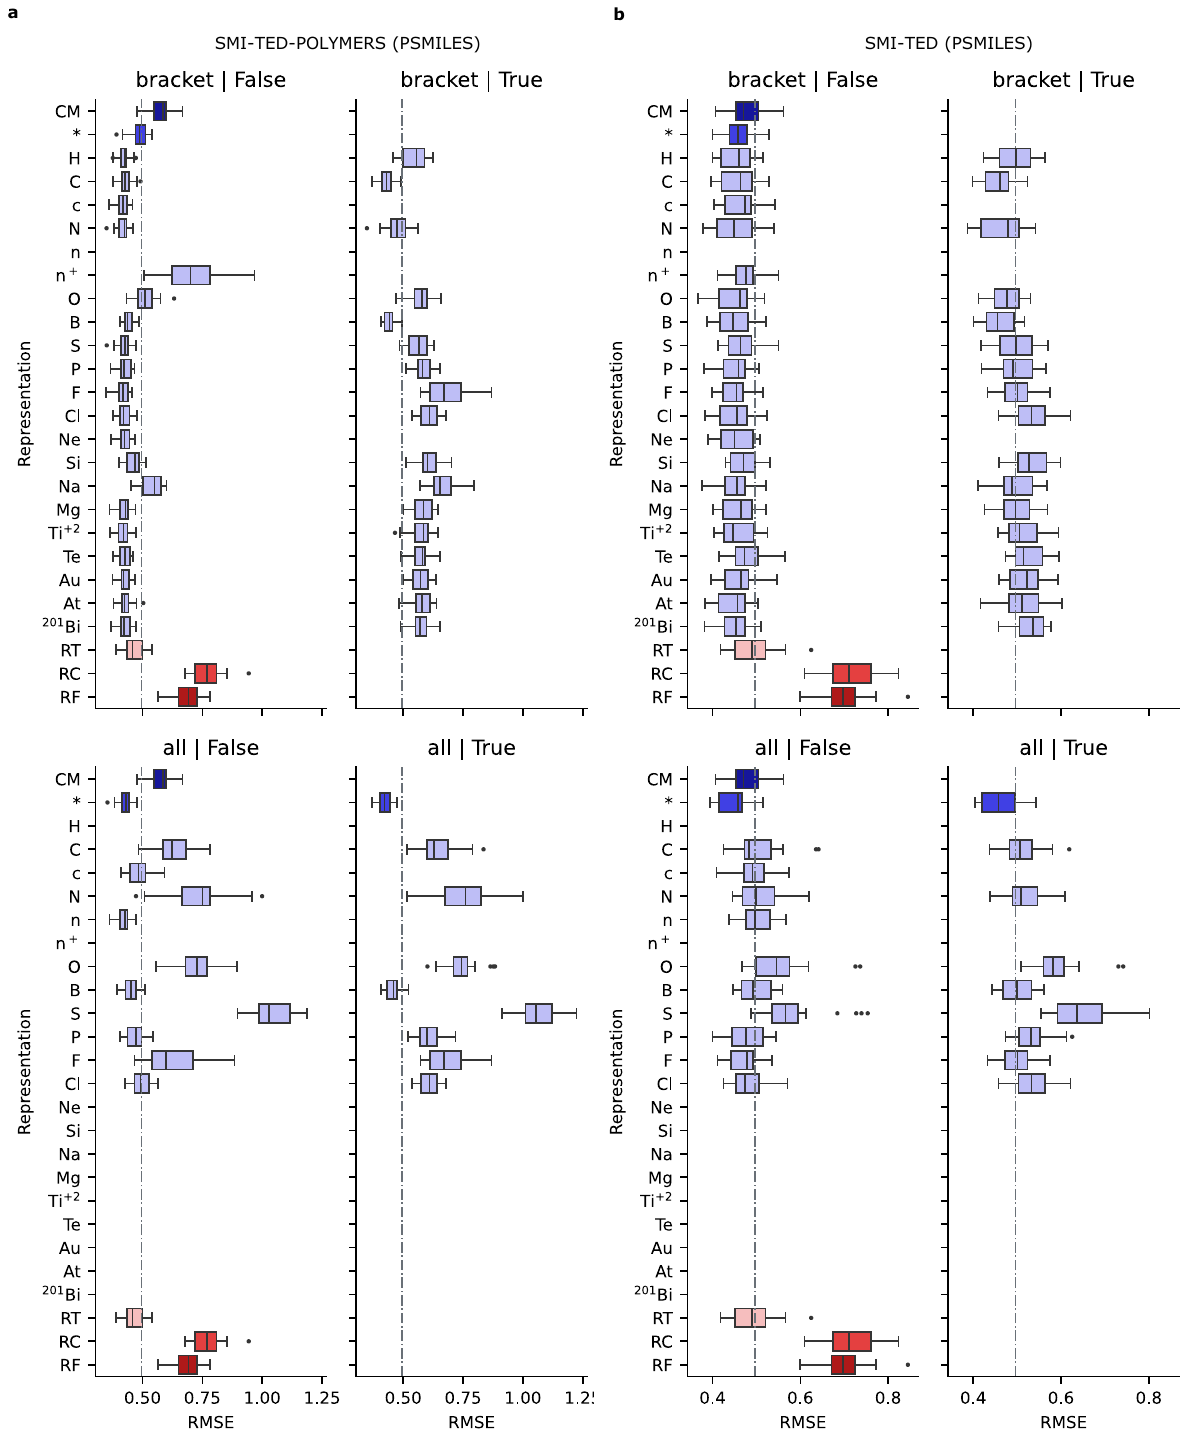}
\caption{Box plots for E\textsubscript{gb} repeated cross-validation experiments for SMI-TED-POLYMER (\textbf{a}) and SMI-TED (\textbf{b}) models fine-tuned with PSMILES.}\label{egb_token_box_psmiles}
\end{figure}

\subsubsection{Polymer Bulk Bandgap (E\textsubscript{gb}) Random Split Scores}\label{rsEgb}

\begin{figure}[H]
\centering
\includegraphics[width=1\textwidth]{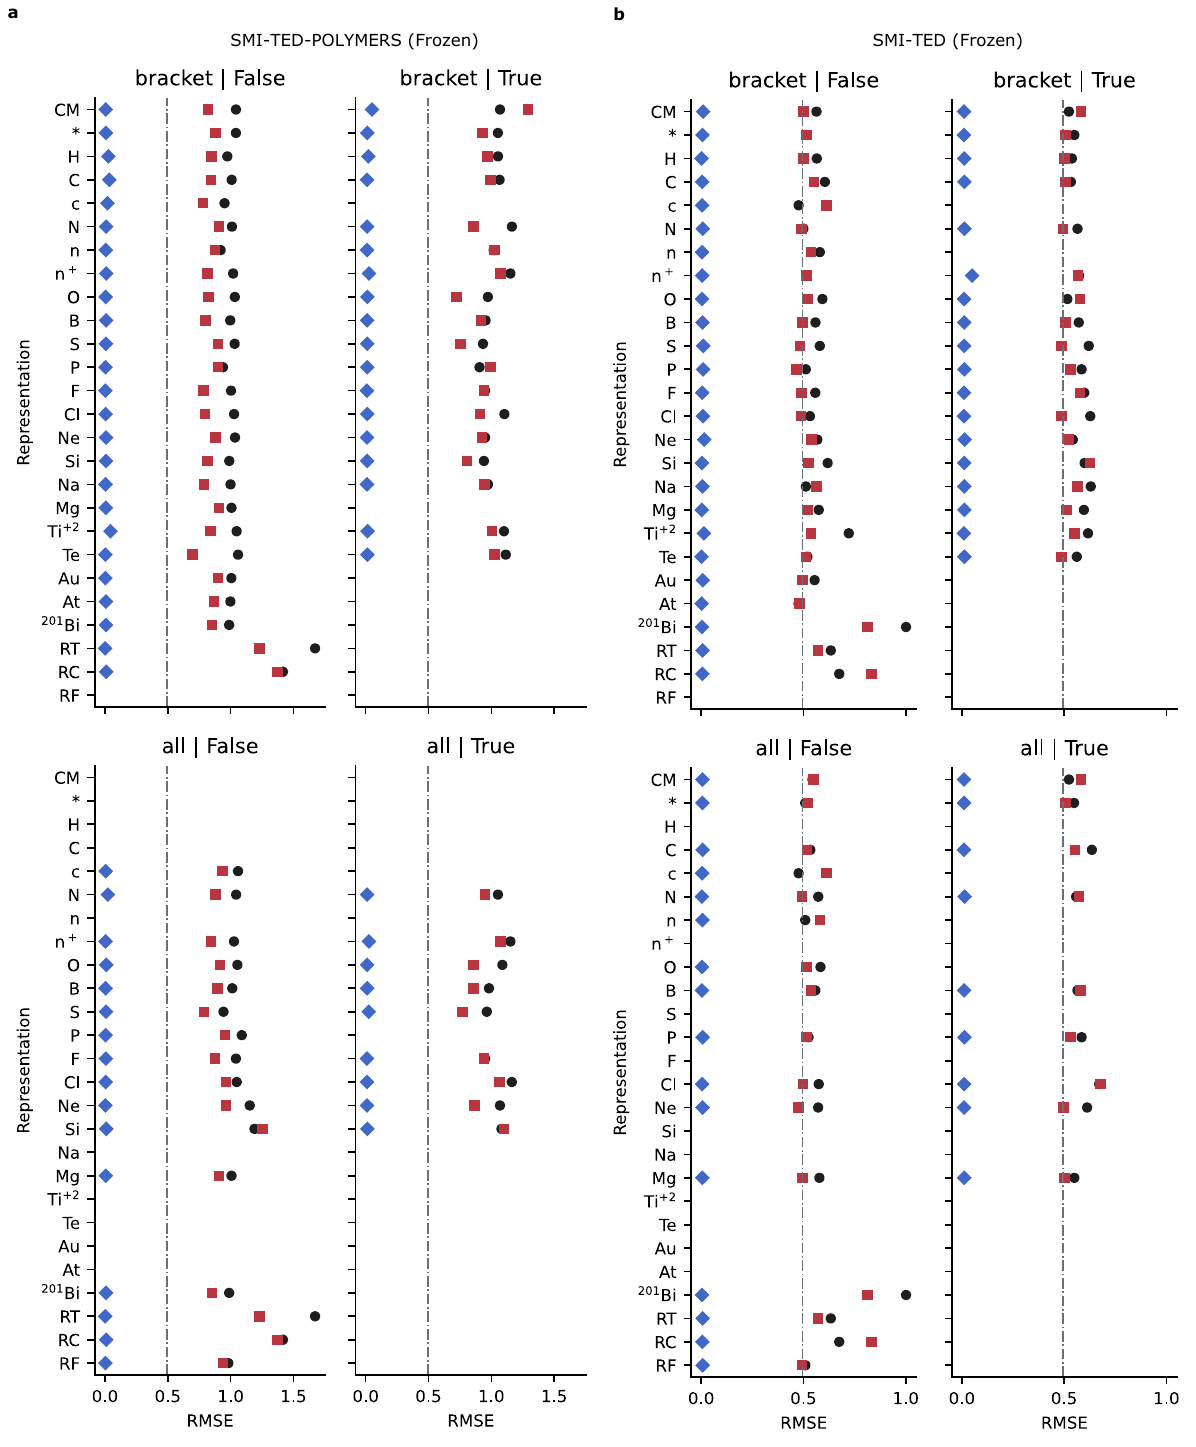}
\caption{Point plots for E\textsubscript{gb} benchmark experiments of RMSE using the base random train, valid, and test splits for SMI-TED-POLYMER (\textbf{a}) and SMI-TED (\textbf{b}) models with frozen weights.}\label{egb_token_point_frozen_rmse}
\end{figure}

\begin{figure}[H]
\centering
\includegraphics[width=1\textwidth]{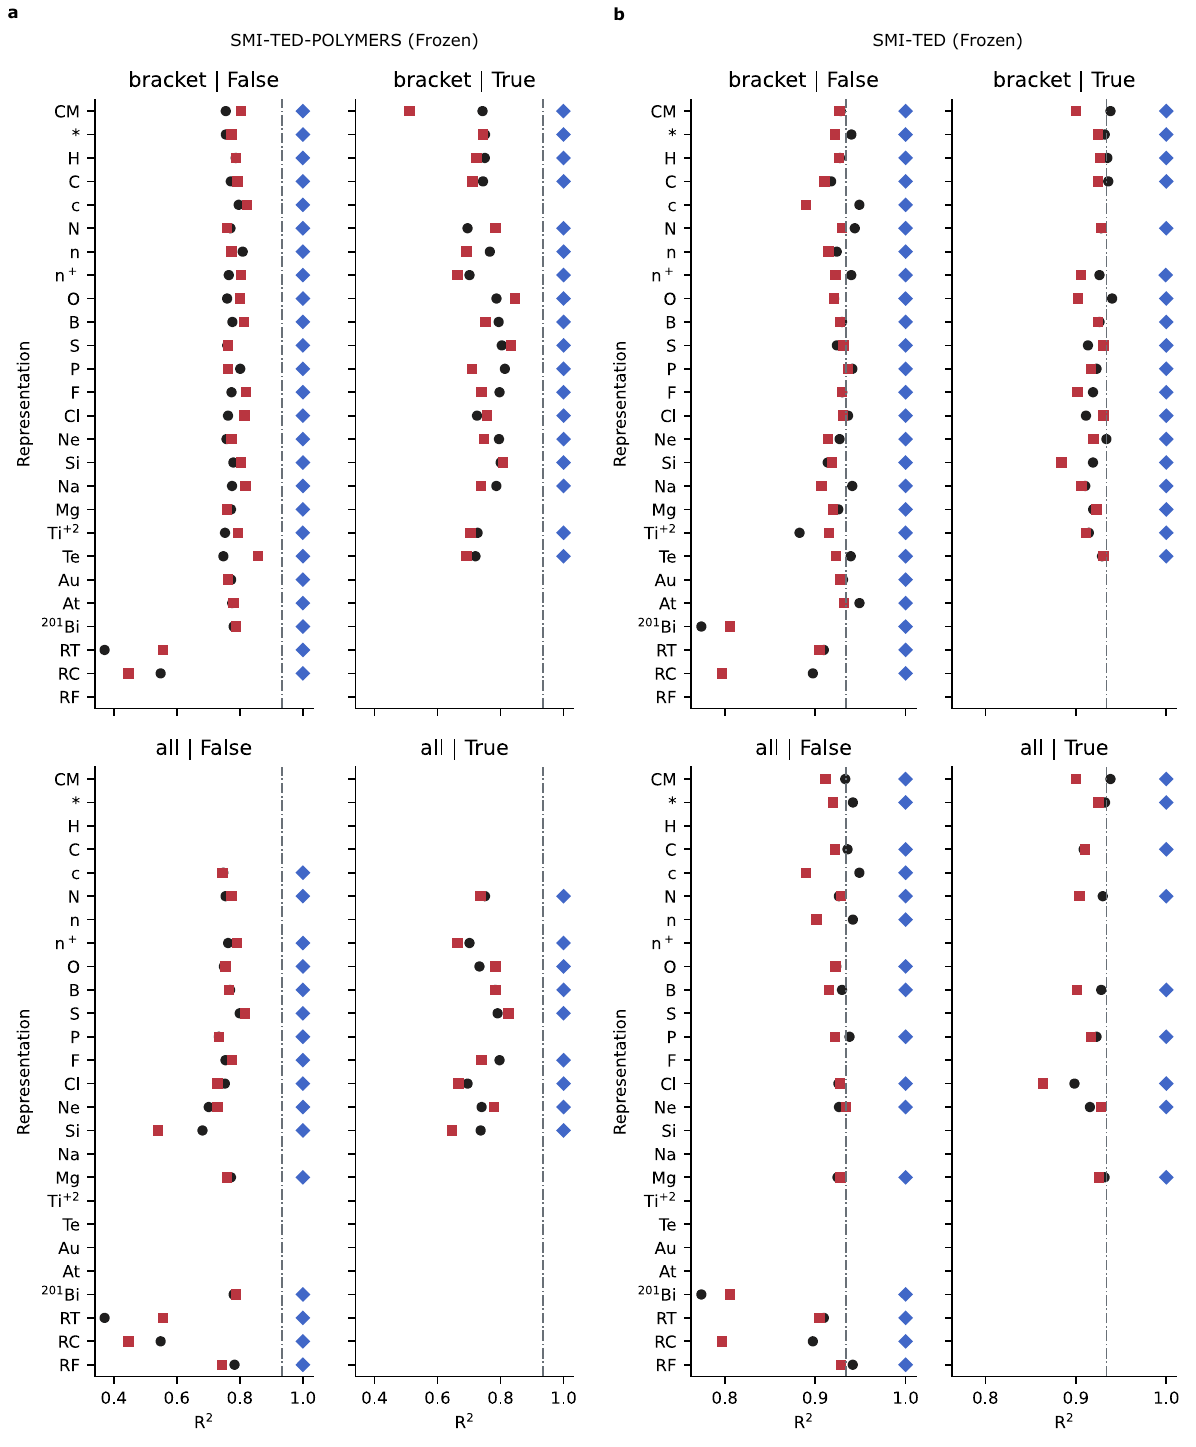}
\caption{Point plots for E\textsubscript{gb} benchmark experiments of R\textsuperscript{2} using the base random train, valid, and test splits for SMI-TED-POLYMER (\textbf{a}) and SMI-TED (\textbf{b}) models with frozen weights.}\label{egb_token_point_frozen_r2}
\end{figure}

\begin{figure}[H]
\centering
\includegraphics[width=1\textwidth]{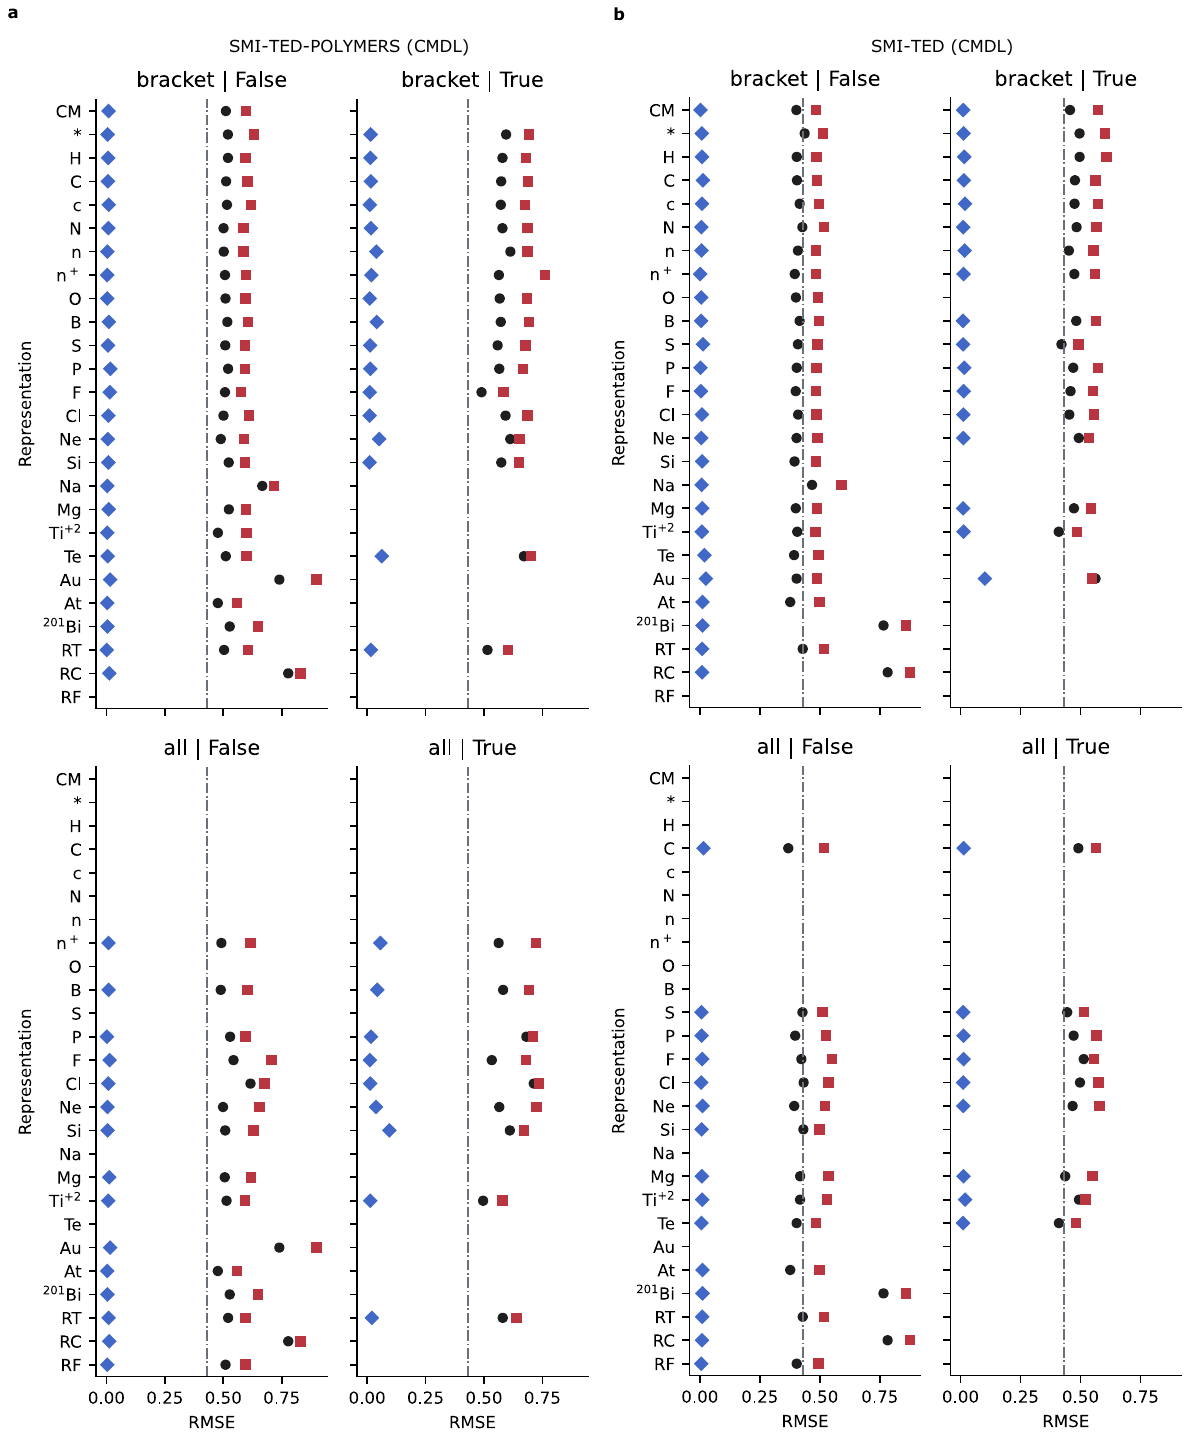}
\caption{Point plots for E\textsubscript{gb} benchmark experiments of RMSE using the base random train, valid, and test splits for SMI-TED-POLYMER (\textbf{a}) and SMI-TED (\textbf{b}) models fine-tuned using the CPG representation.}\label{egb_token_point_cmdl_rmse}
\end{figure}

\begin{figure}[H]
\centering
\includegraphics[width=1\textwidth]{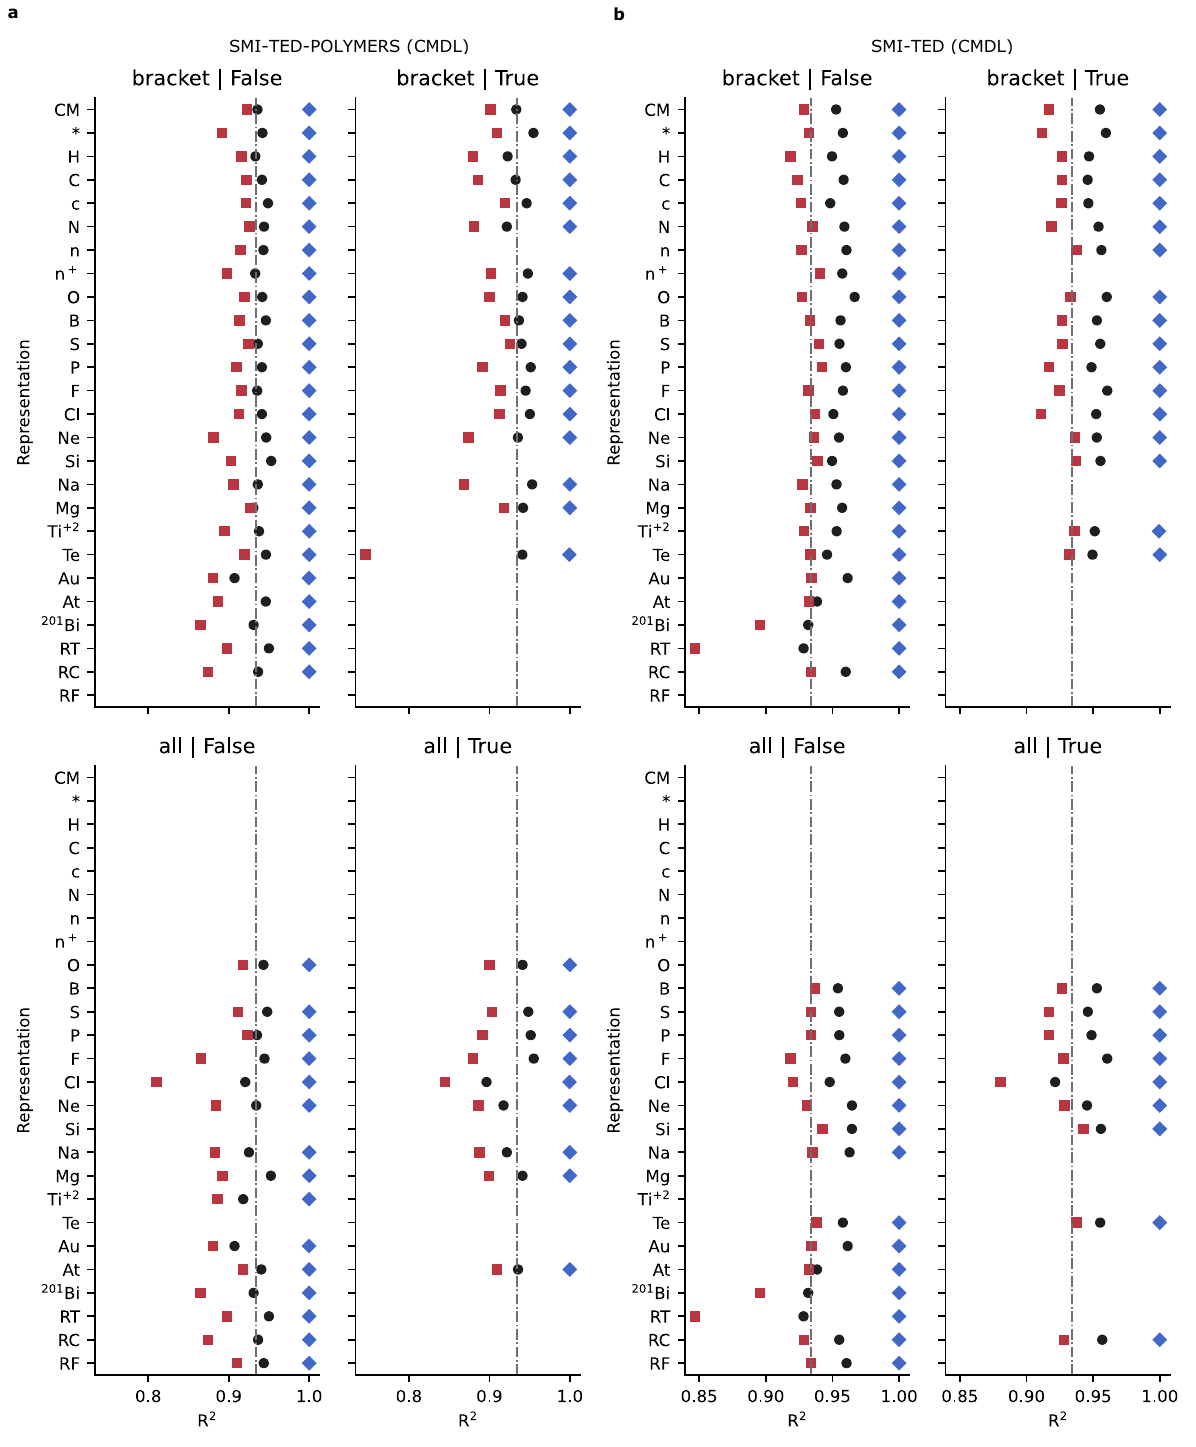}
\caption{Point plots for E\textsubscript{gb} benchmark experiments of R\textsuperscript{2} using the base random train, valid, and test splits for SMI-TED-POLYMER (\textbf{a}) and SMI-TED (\textbf{b}) models fine-tuned using the CPG representation.}\label{egb_token_point_cmdl_r2}
\end{figure}

\begin{figure}[H]
\centering
\includegraphics[width=1\textwidth]{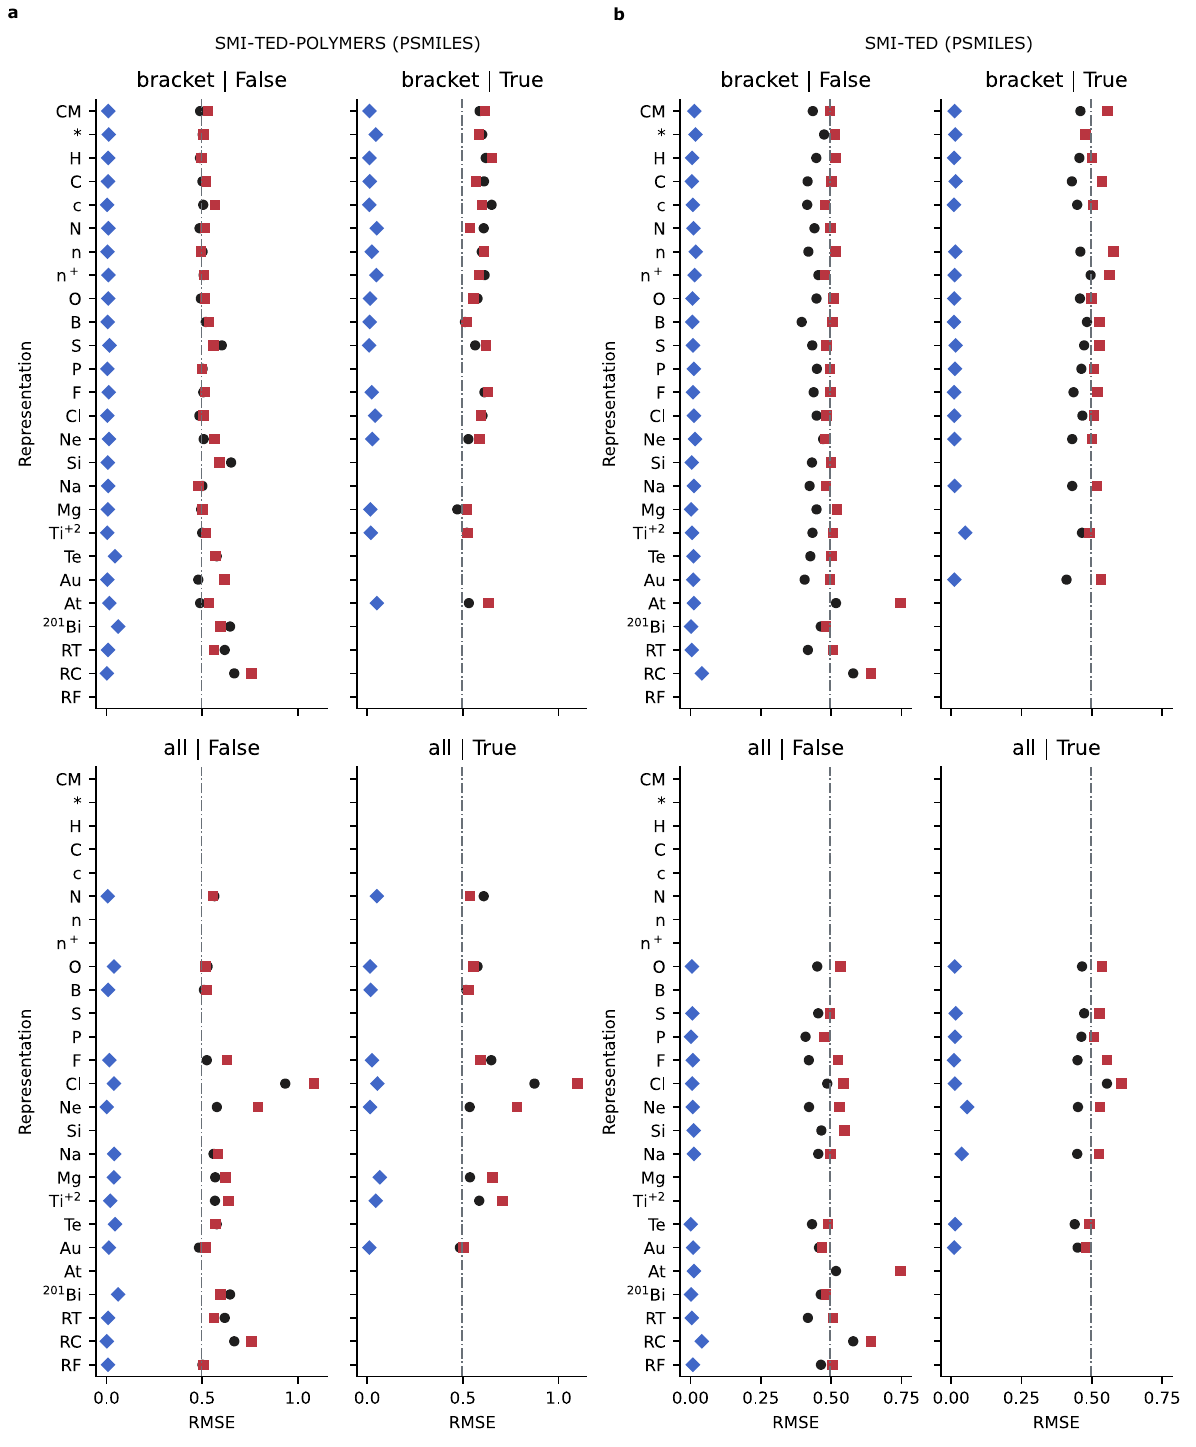}
\caption{Point plots for E\textsubscript{gb} benchmark experiments of RMSE using the base random train, valid, and test splits for SMI-TED-POLYMER (\textbf{a}) and SMI-TED (\textbf{b}) models fine-tuned using PSMILES.}\label{egb_token_point_psmiles_rmse}
\end{figure}

\begin{figure}[H]
\centering
\includegraphics[width=1\textwidth]{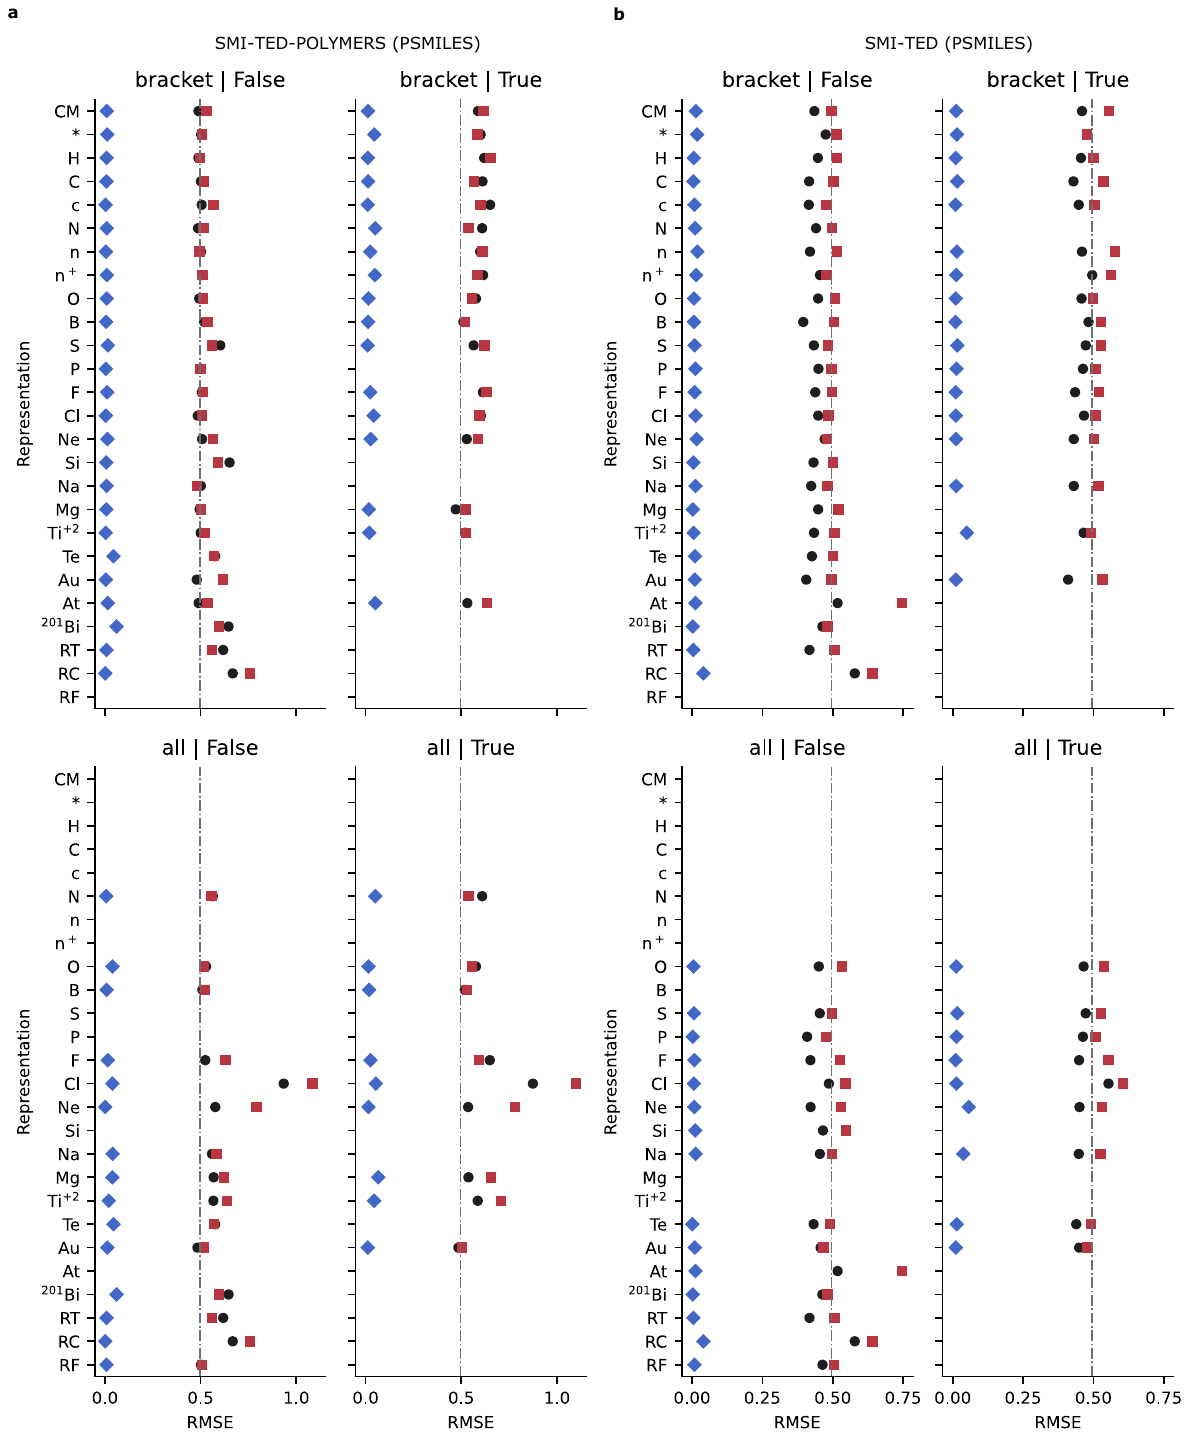}
\caption{Point plots for E\textsubscript{gb} benchmark experiments of R\textsuperscript{2} using the base random train, valid, and test splits for SMI-TED-POLYMER (\textbf{a}) and SMI-TED (\textbf{b}) models fine-tuned using PSMILES.}\label{egb_token_point_psmiles_r2}
\end{figure}

\subsubsection{Polymer Ionization Energy (E\textsubscript{i}) CV Scores}\label{cvEi}

\begin{figure}[H]
\centering
\includegraphics[width=1\textwidth]{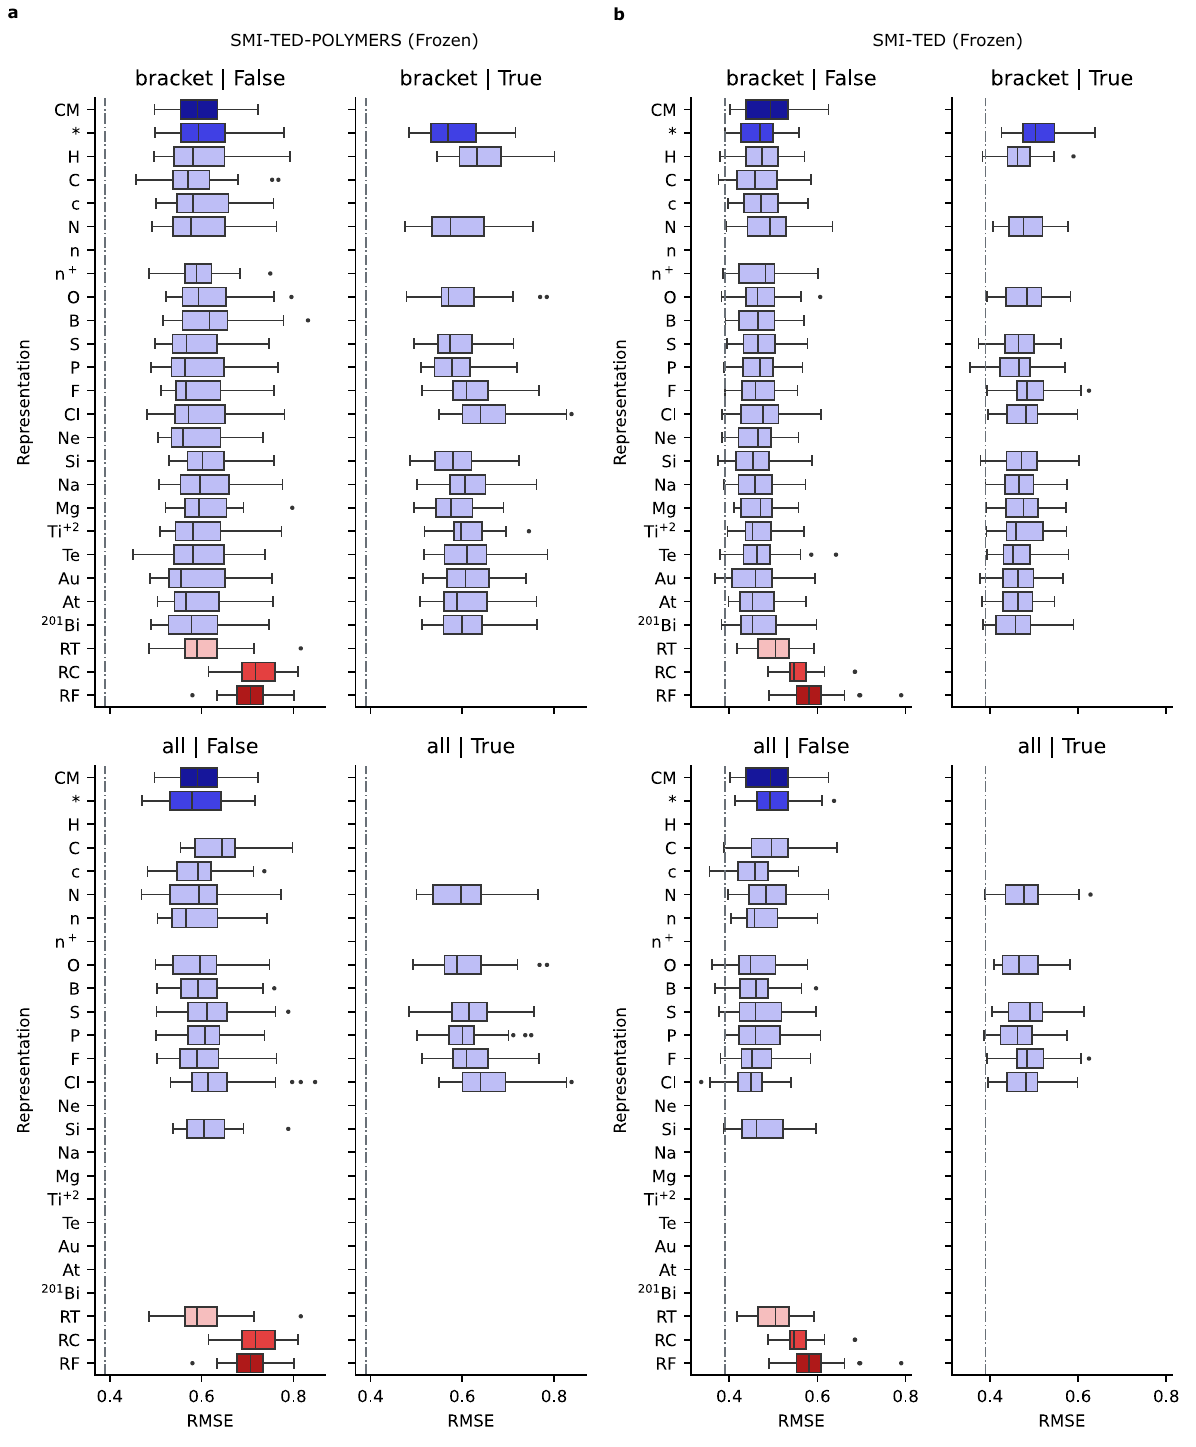}
\caption{Box plots for E\textsubscript{i} repeated cross-validation experiments for SMI-TED-POLYMER (\textbf{a}) and SMI-TED (\textbf{b}) models with frozen weights.}\label{ei_token_box_frozen}
\end{figure}

\begin{figure}[H]
\centering
\includegraphics[width=1\textwidth]{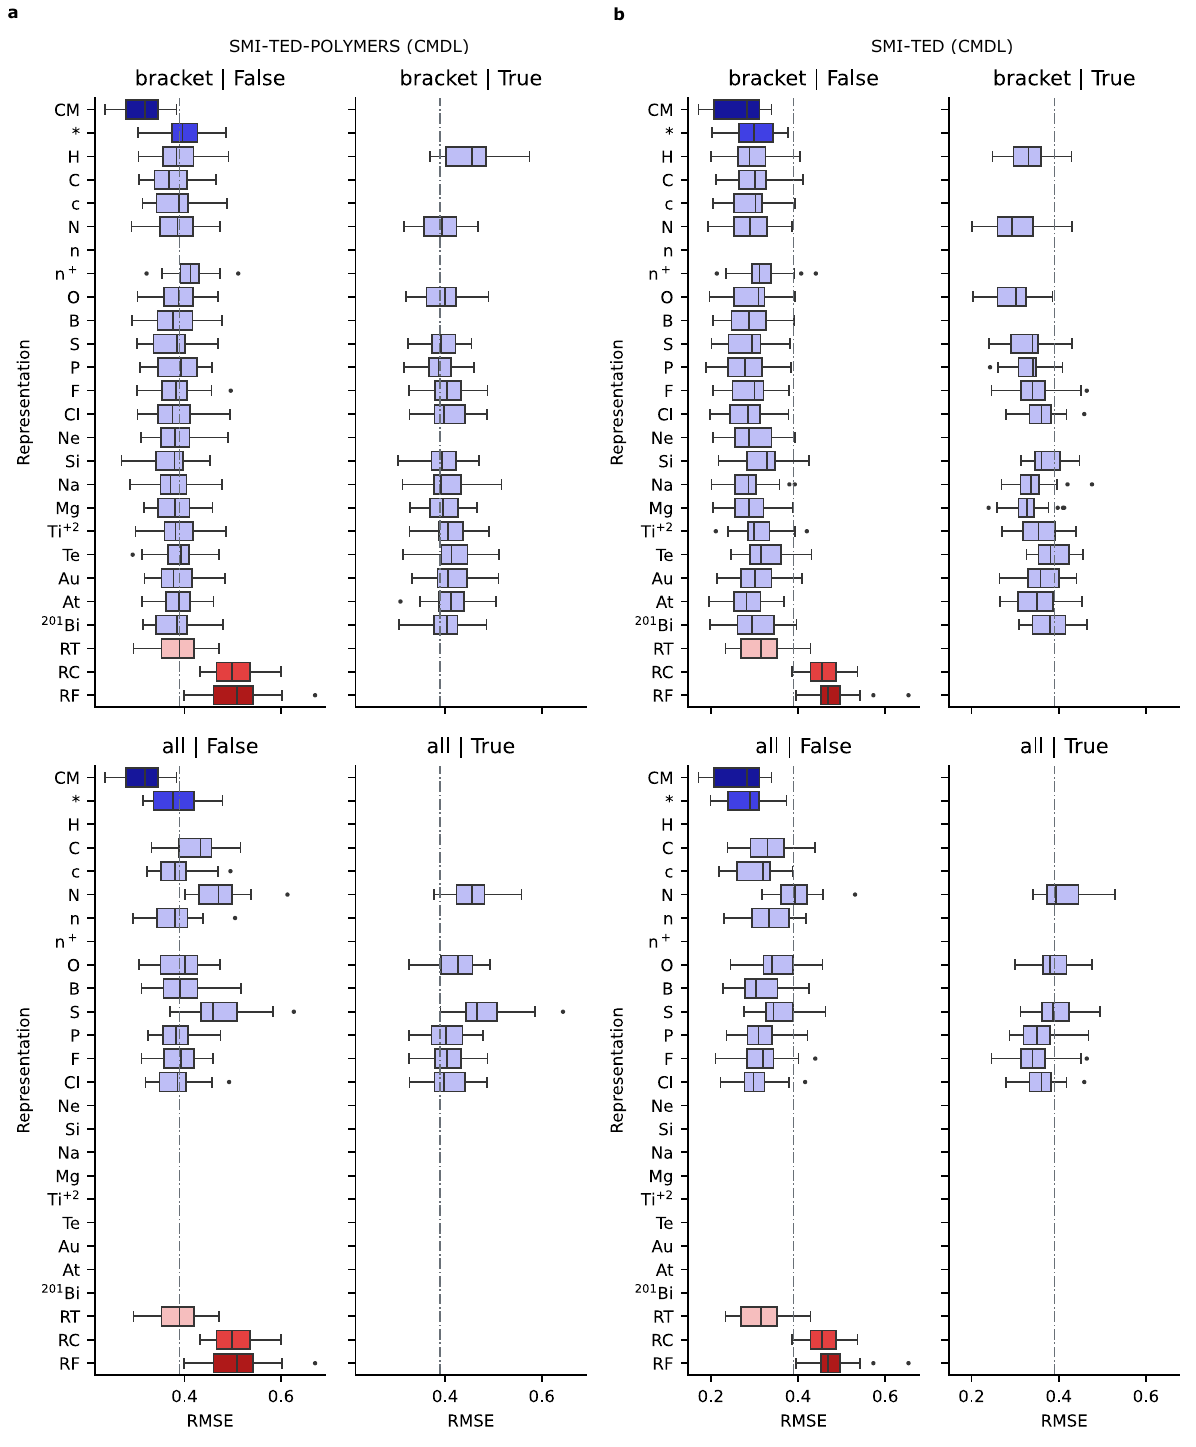}
\caption{Box plots for E\textsubscript{i} repeated cross-validation experiments for SMI-TED-POLYMER (\textbf{a}) and SMI-TED (\textbf{b}) models fine-tuned with the CPG polymer graphs.}\label{ei_token_box_cmdl}
\end{figure}

\begin{figure}[H]
\centering
\includegraphics[width=1\textwidth]{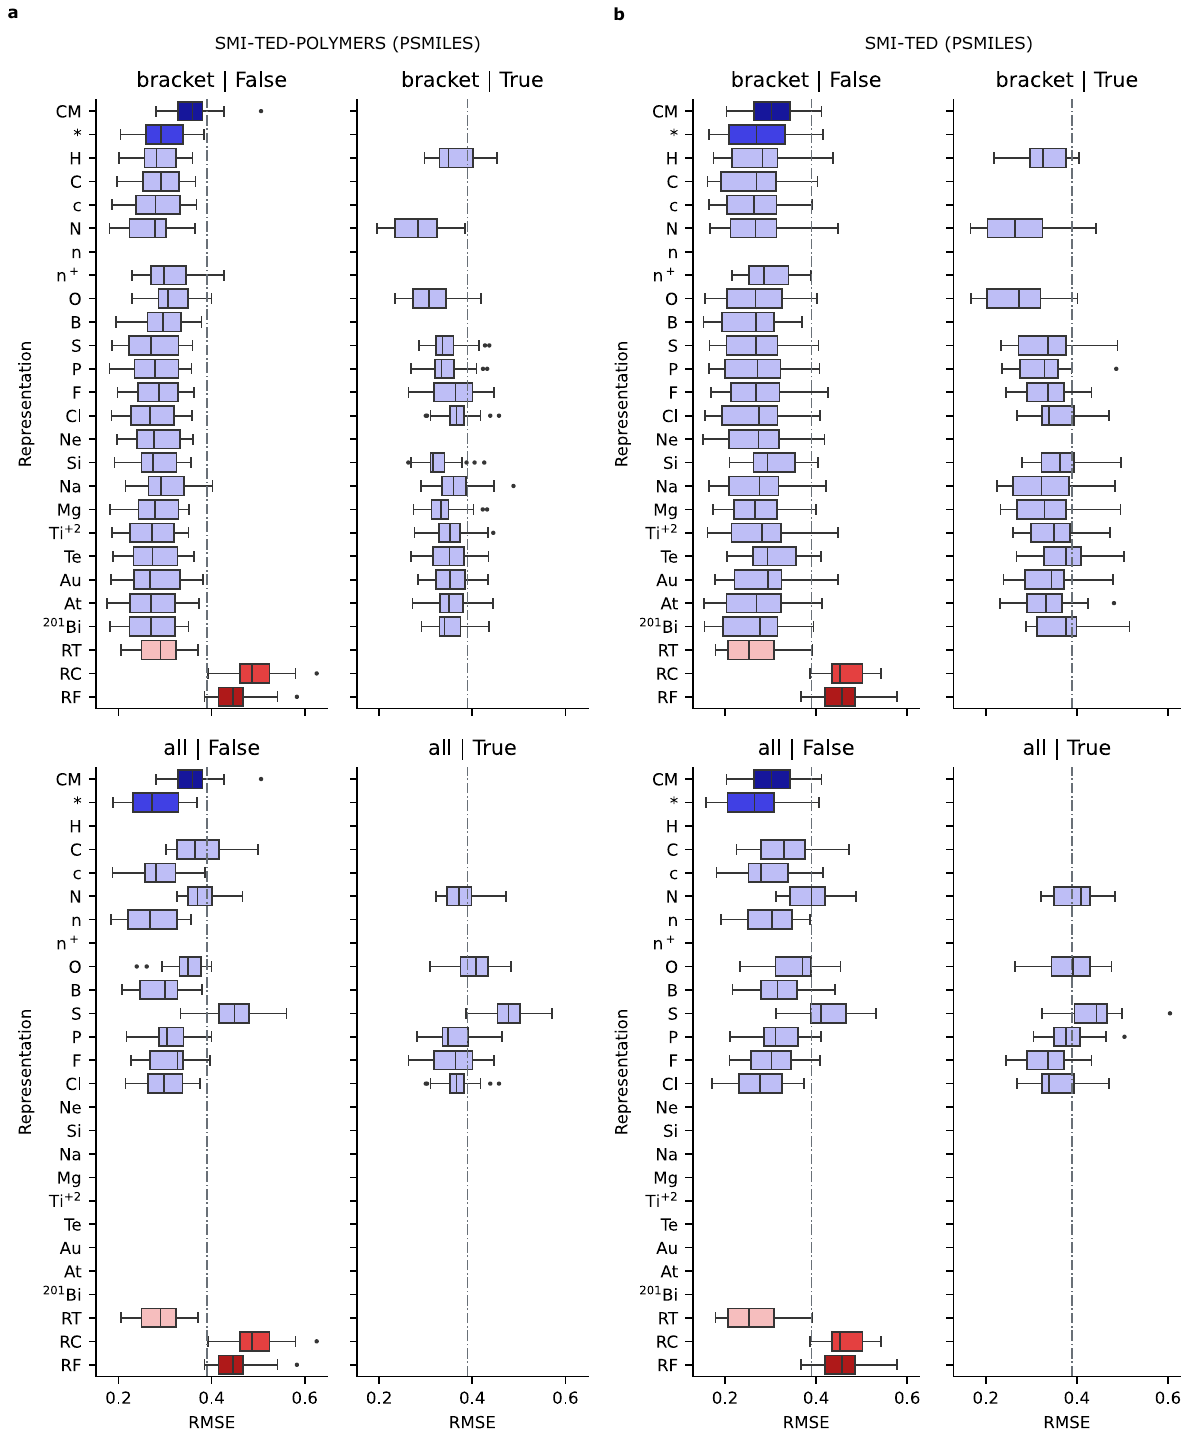}
\caption{Box plots for E\textsubscript{i} repeated cross-validation experiments for SMI-TED-POLYMER (\textbf{a}) and SMI-TED (\textbf{b}) models fine-tuned with PSMILES.}\label{ei_token_box_psmiles}
\end{figure}

\subsubsection{Polymer Ionization Energy (E\textsubscript{i}) Random Split Scores}\label{randEi}

\begin{figure}[H]
\centering
\includegraphics[width=1\textwidth]{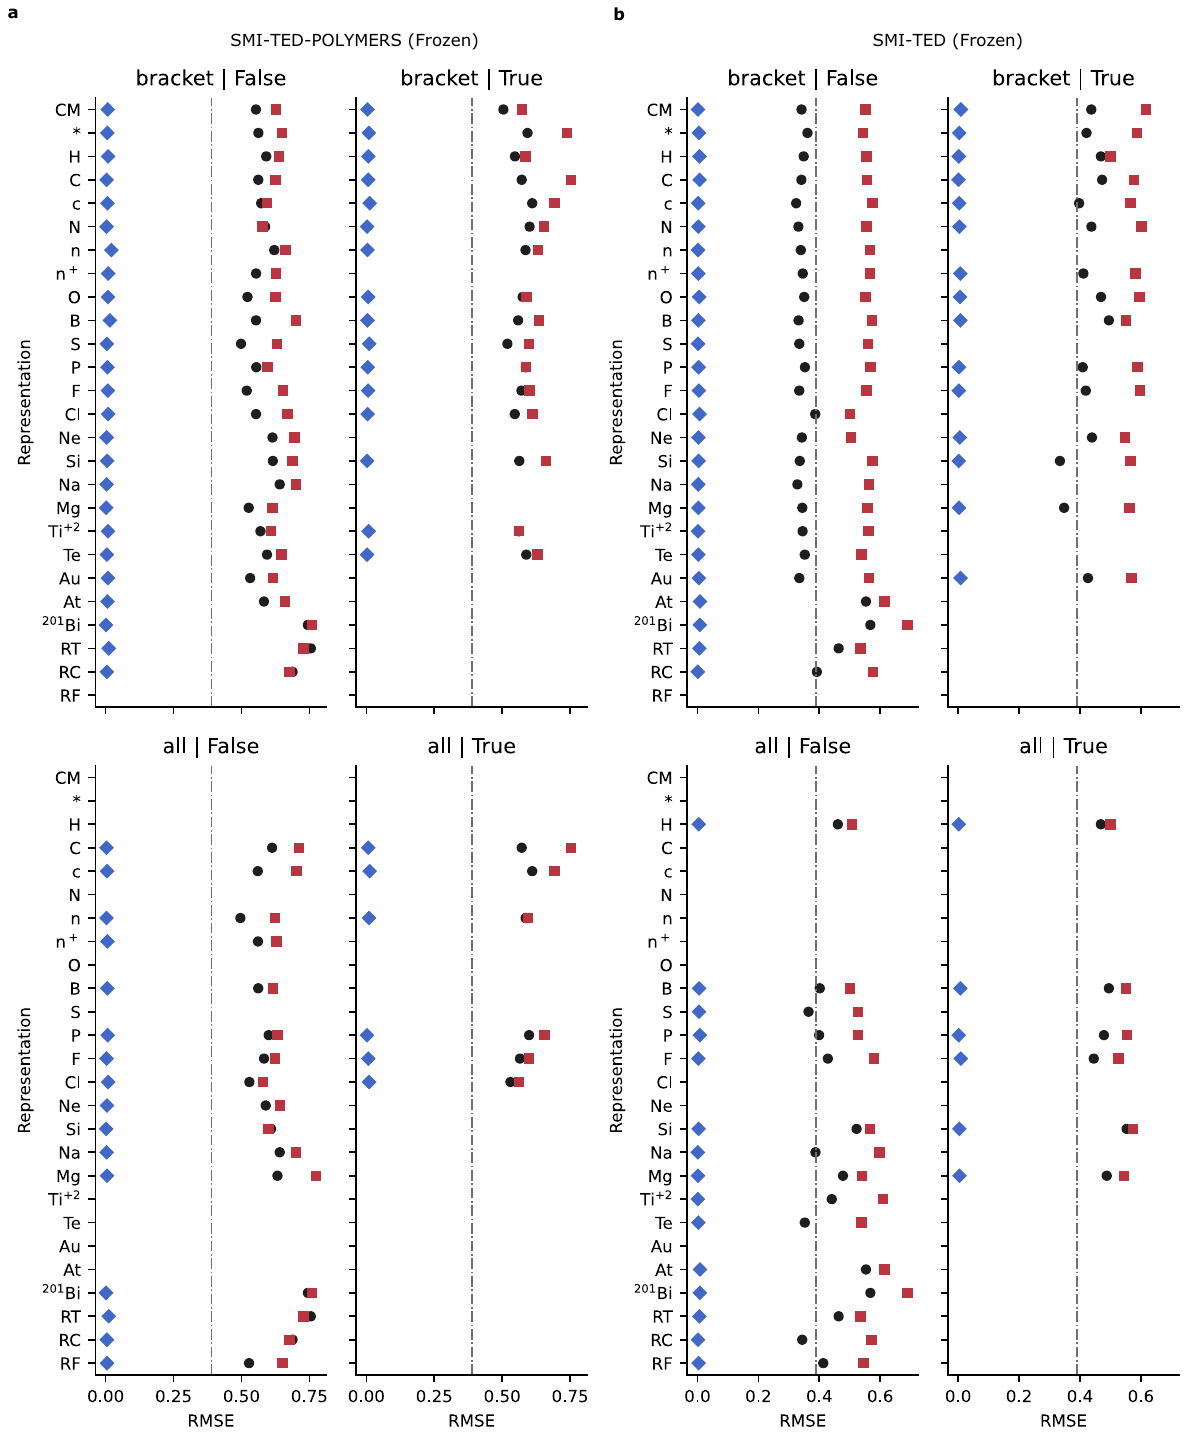}
\caption{Point plots for E\textsubscript{i} benchmark experiments of RMSE using the base random train, valid, and test splits for SMI-TED-POLYMER (\textbf{a}) and SMI-TED (\textbf{b}) models with frozen weights.}\label{ei_token_point_frozen_rmse}
\end{figure}

\begin{figure}[H]
\centering
\includegraphics[width=1\textwidth]{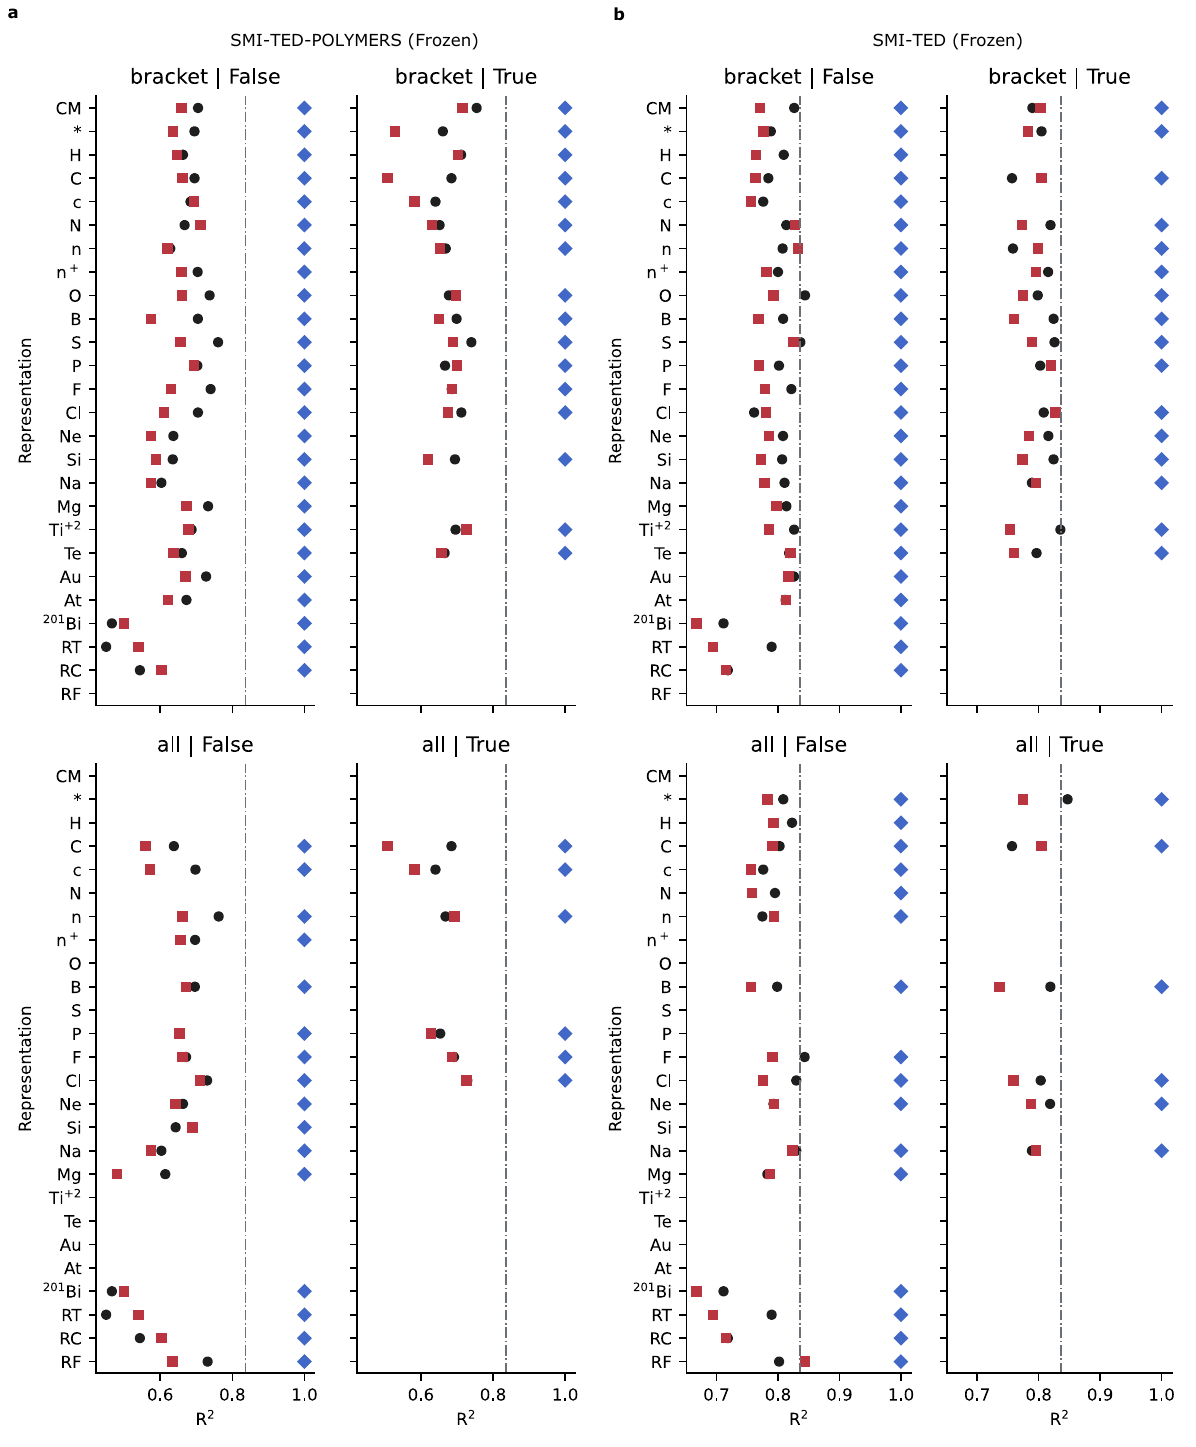}
\caption{Point plots for E\textsubscript{i} benchmark experiments of R\textsuperscript{2} using the base random train, valid, and test splits for SMI-TED-POLYMER (\textbf{a}) and SMI-TED (\textbf{b}) models with frozen weights.}\label{ei_token_point_frozen_r2}
\end{figure}

\begin{figure}[H]
\centering
\includegraphics[width=1\textwidth]{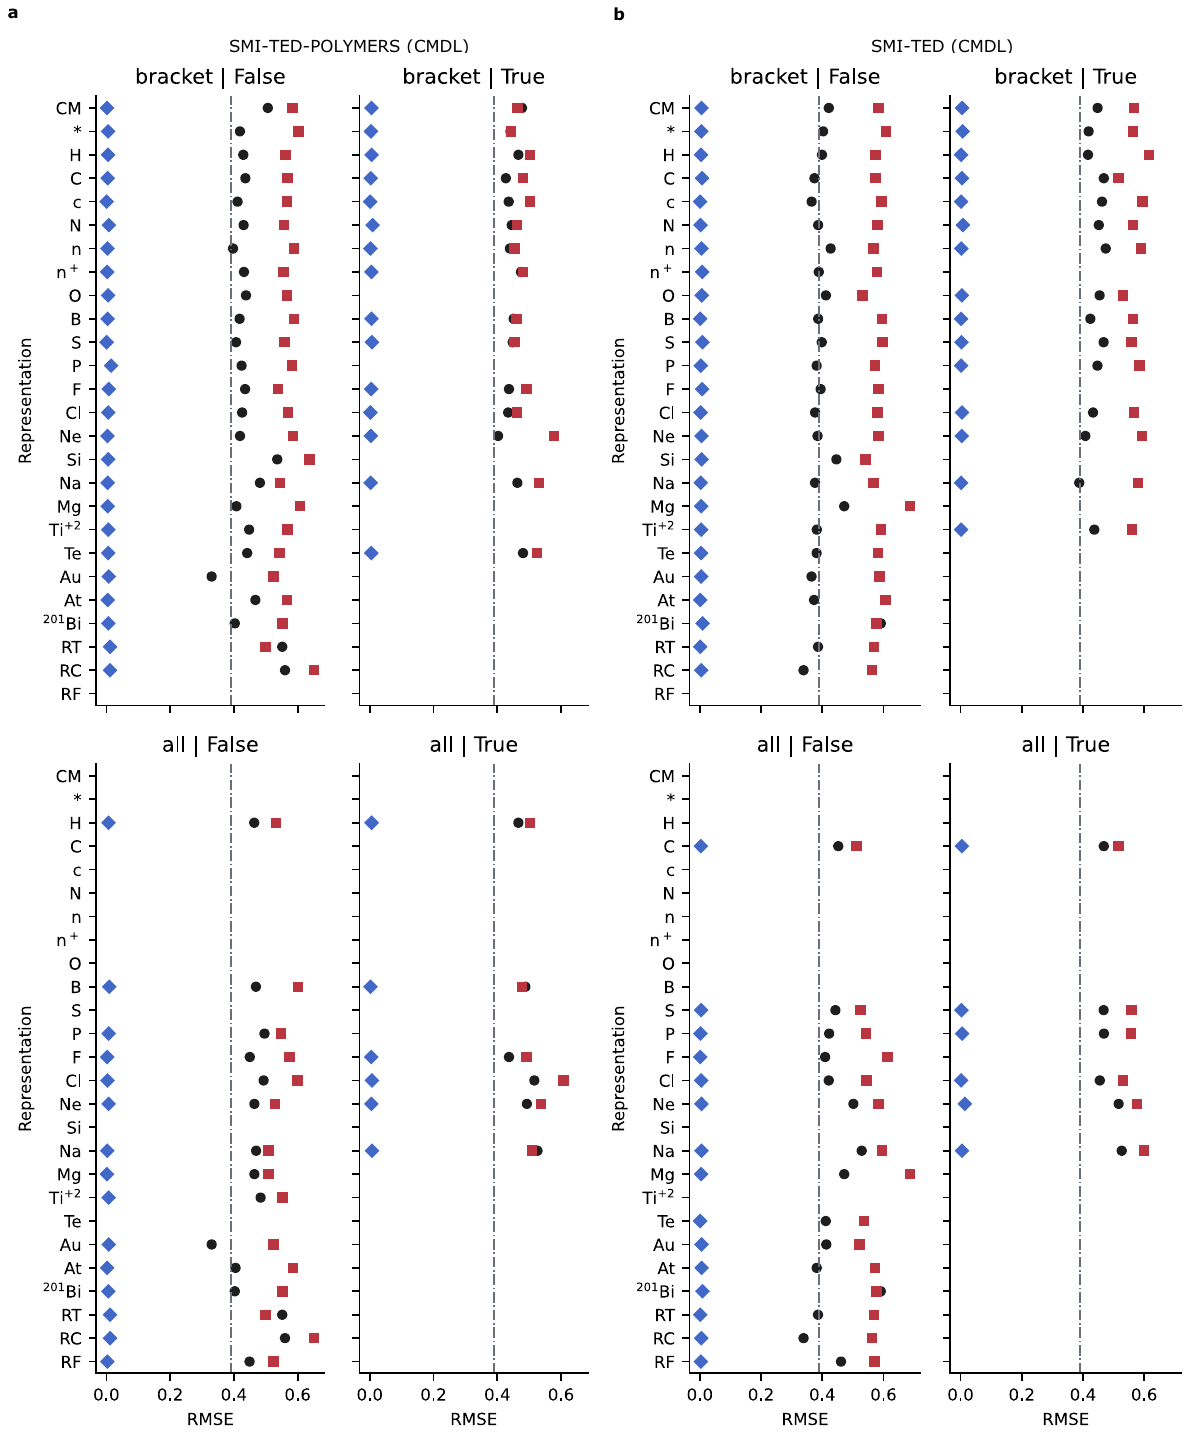}
\caption{Point plots for E\textsubscript{i} benchmark experiments of RMSE using the base random train, valid, and test splits for SMI-TED-POLYMER (\textbf{a}) and SMI-TED (\textbf{b}) models fine-tuned using the CPG representation.}\label{ei_token_point_cmdl_rmse}
\end{figure}

\begin{figure}
\centering
\includegraphics[width=1\textwidth]{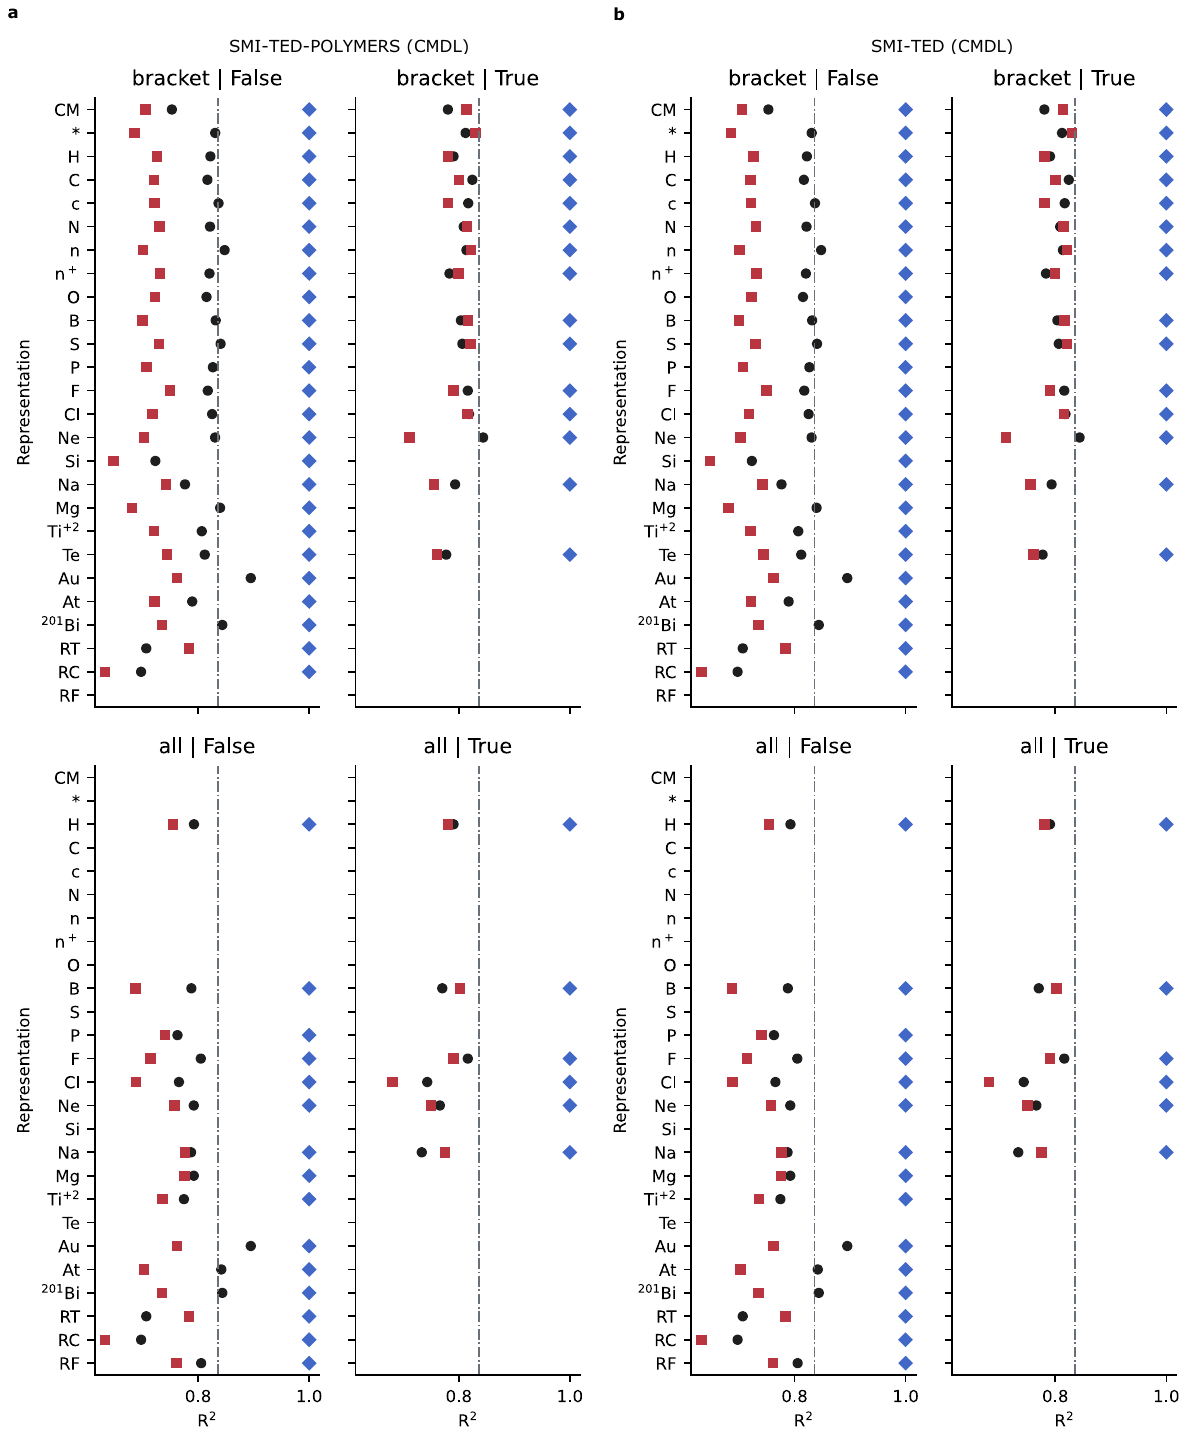}
\caption{Point plots for E\textsubscript{i} benchmark experiments of R\textsuperscript{2} using the base random train, valid, and test splits for SMI-TED-POLYMER (\textbf{a}) and SMI-TED (\textbf{b}) models fine-tuned using the CPG representation.}\label{ei_token_point_cmdl_r2}
\end{figure}

\begin{figure}[H]
\centering
\includegraphics[width=1\textwidth]{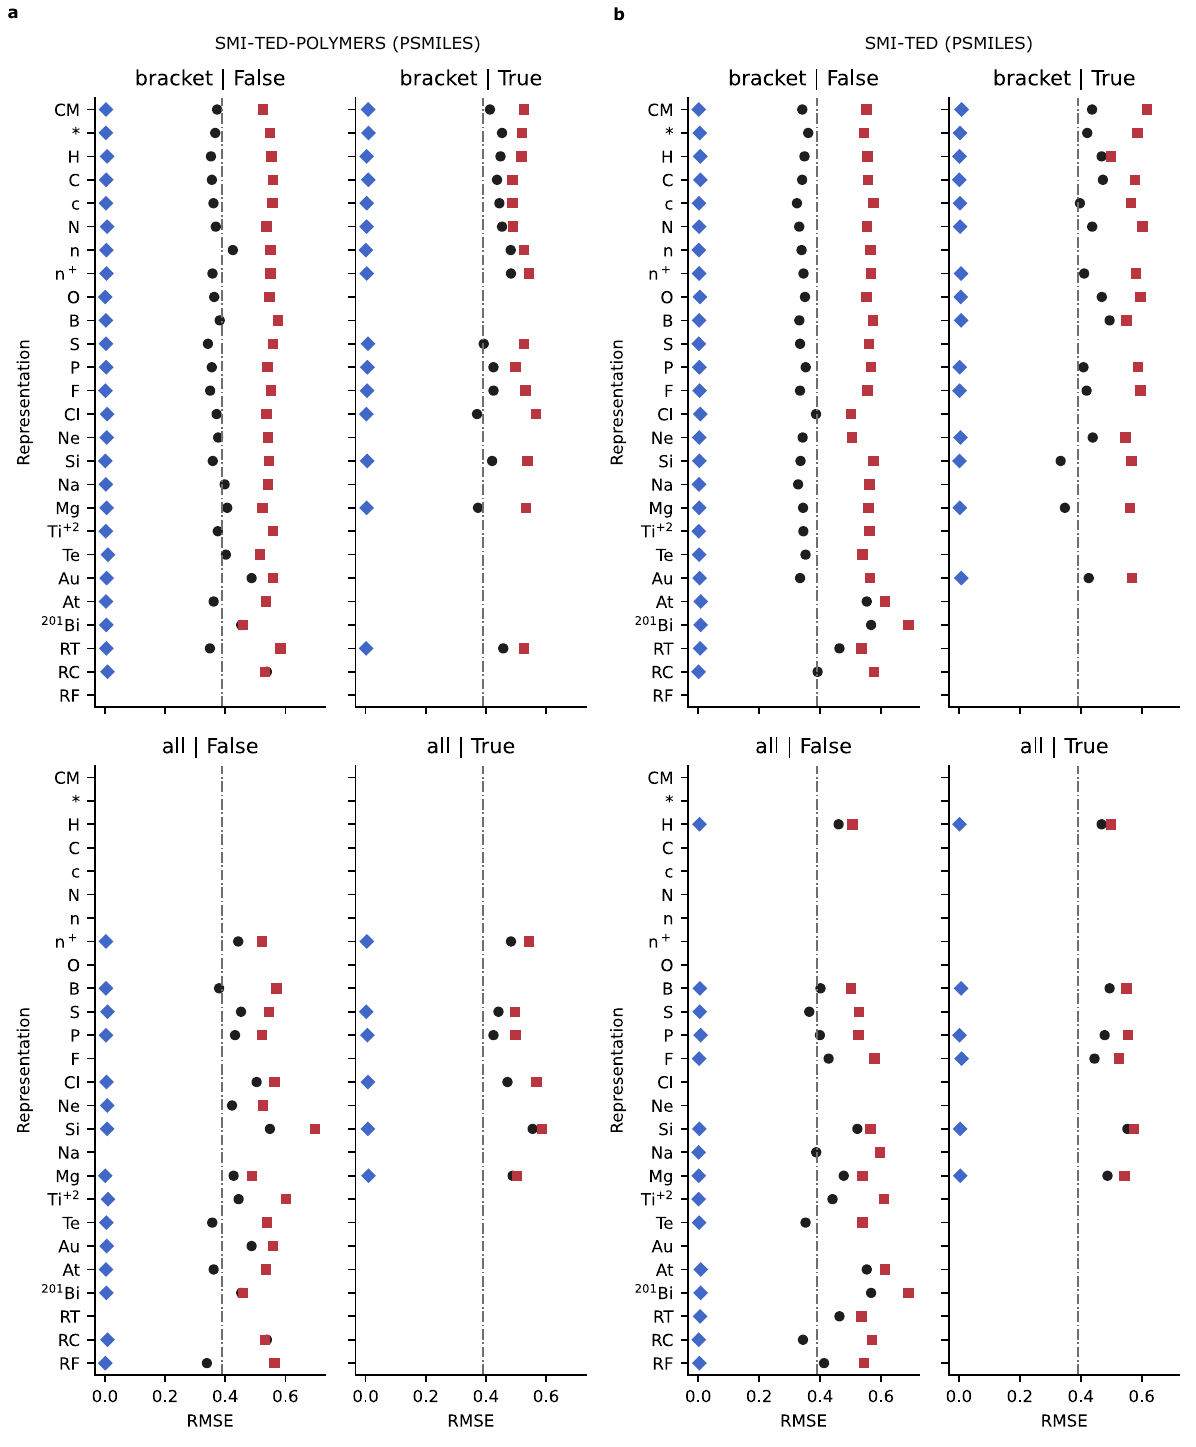}
\caption{Point plots for E\textsubscript{i} benchmark experiments of RMSE using the base random train, valid, and test splits for SMI-TED-POLYMER (\textbf{a}) and SMI-TED (\textbf{b}) models fine-tuned using PSMILES.}\label{ei_token_point_psmiles_rmse}
\end{figure}

\begin{figure}[H]
\centering
\includegraphics[width=1\textwidth]{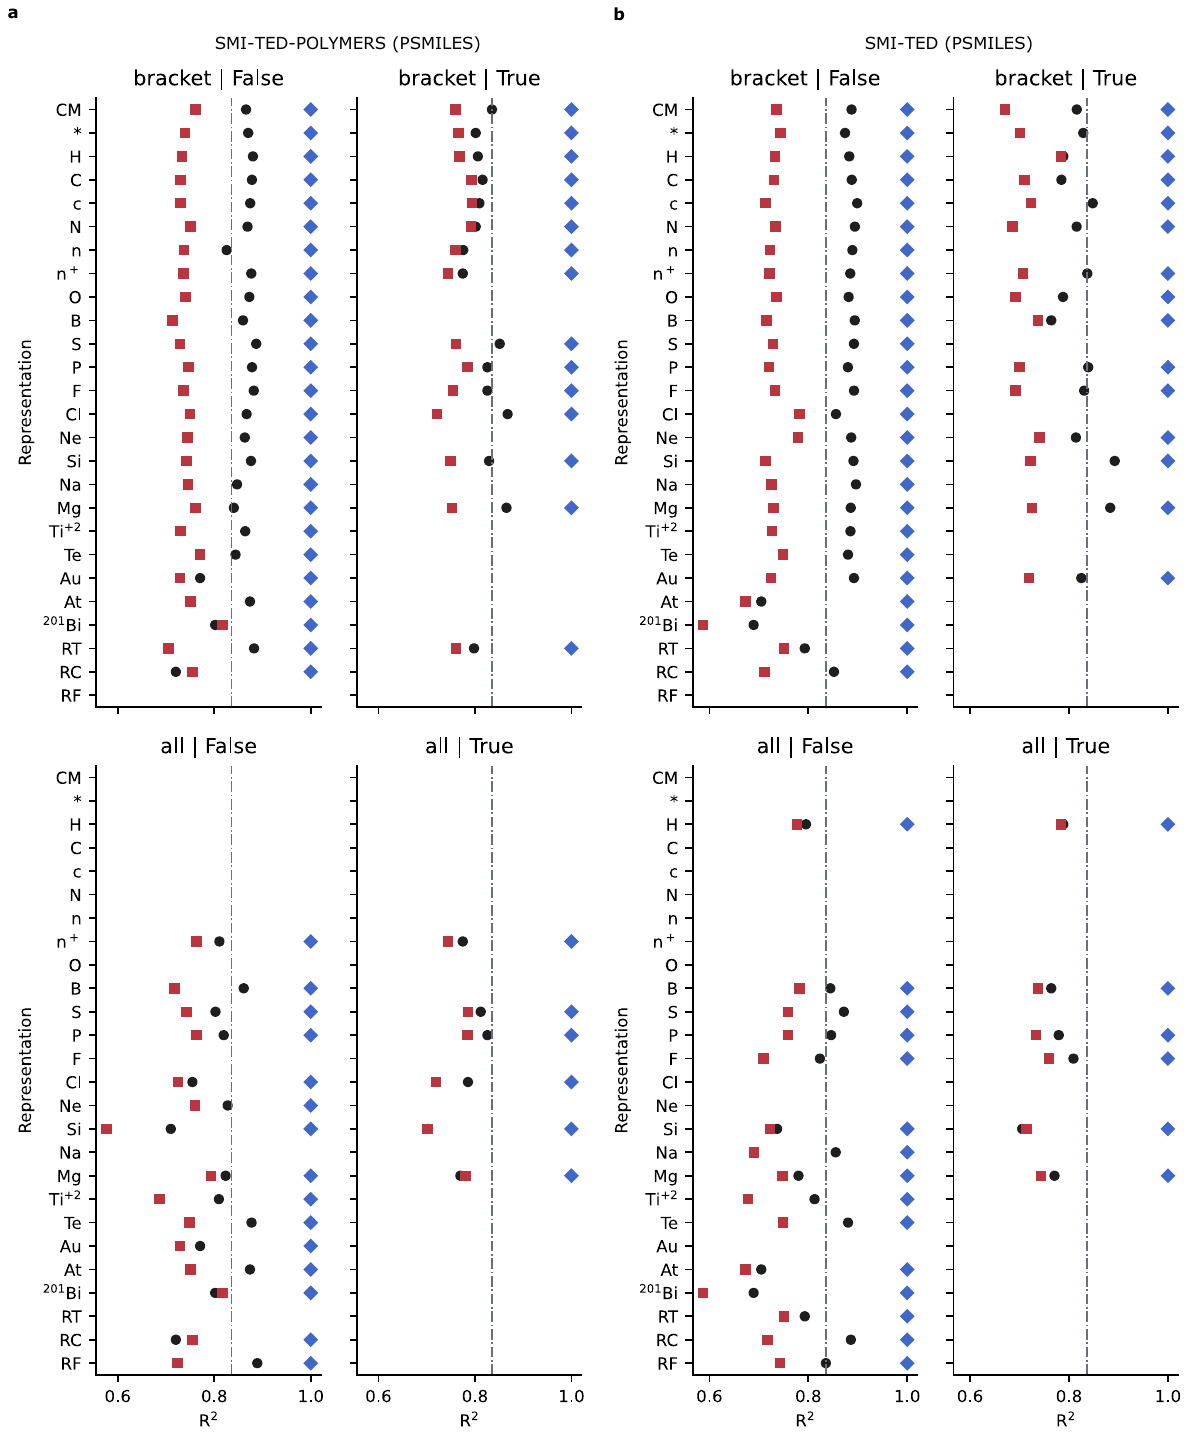}
\caption{Point plots for E\textsubscript{i} benchmark experiments of R\textsuperscript{2} using the base random train, valid, and test splits for SMI-TED-POLYMER (\textbf{a}) and SMI-TED (\textbf{b}) models fine-tuned using PSMILES.}\label{ei_token_point_psmiles_r2}
\end{figure}

\subsubsection{Polymer Dielectric Constant (EPS) CV Scores}\label{cvEPS}

\begin{figure}[H]
\centering
\includegraphics[width=1\textwidth]{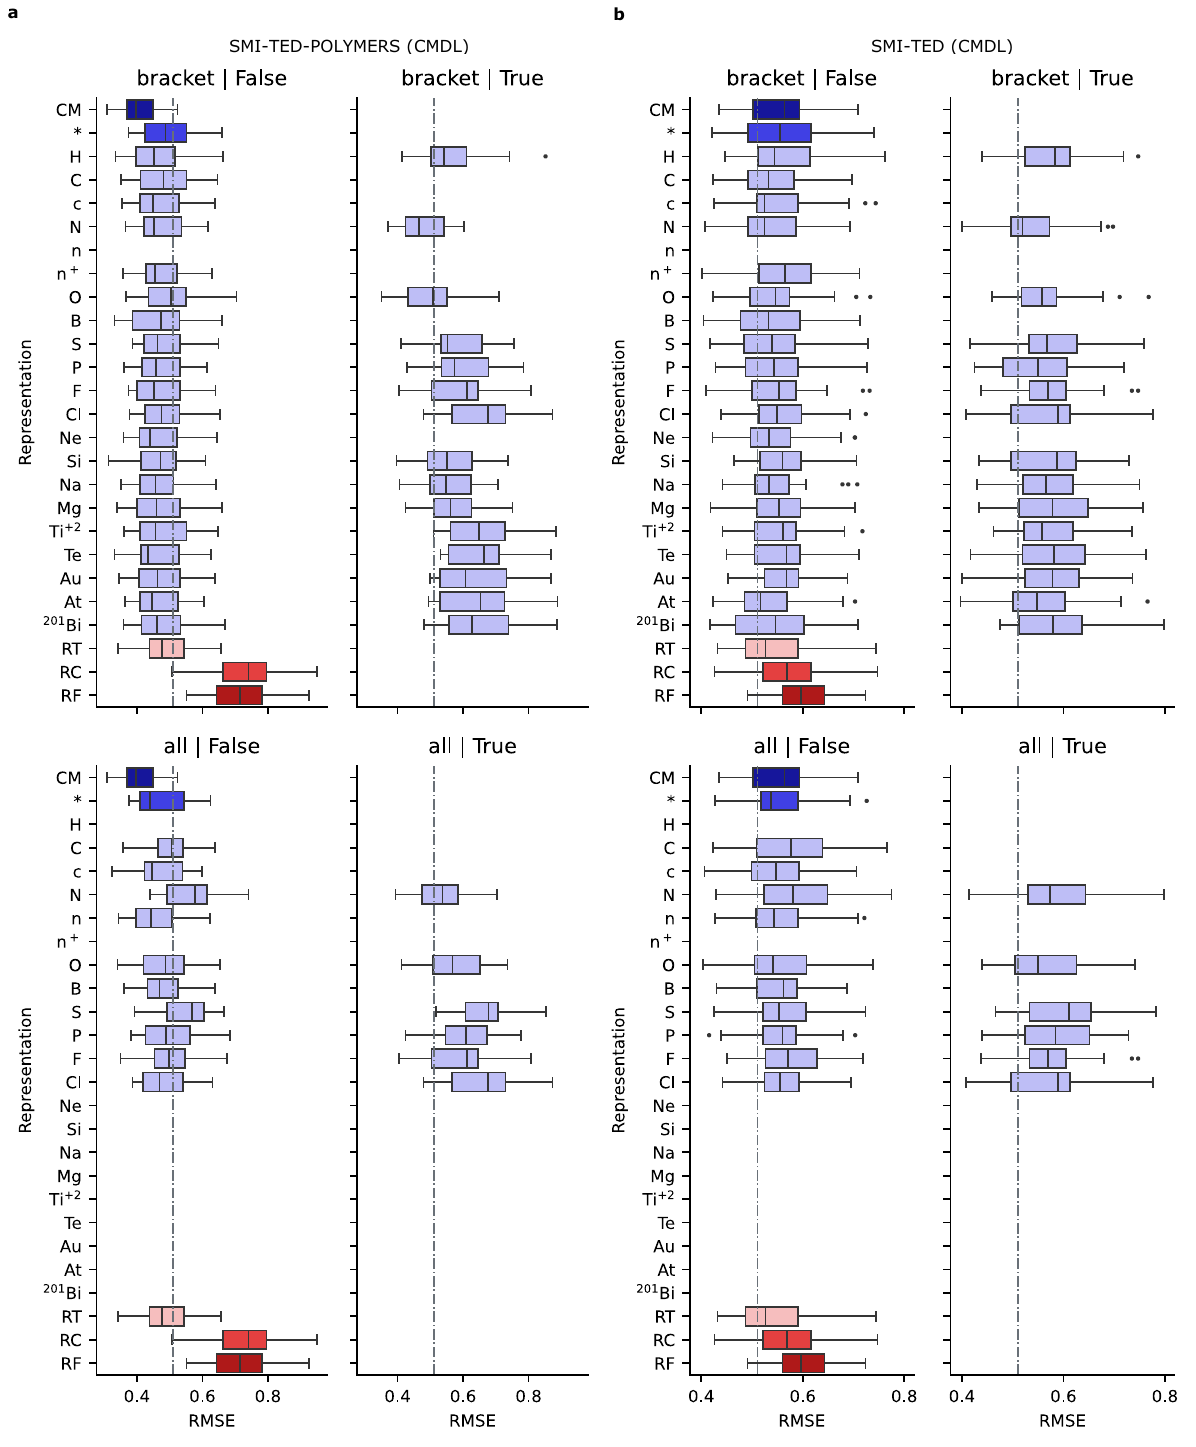}
\caption{Box plots for EPS repeated cross-validation experiments for SMI-TED-POLYMER (\textbf{a}) and SMI-TED (\textbf{b}) models fine-tuned with the CPG polymer graphs.}\label{eps_token_box_cmdl}
\end{figure}

\begin{figure}[H]
\centering
\includegraphics[width=1\textwidth]{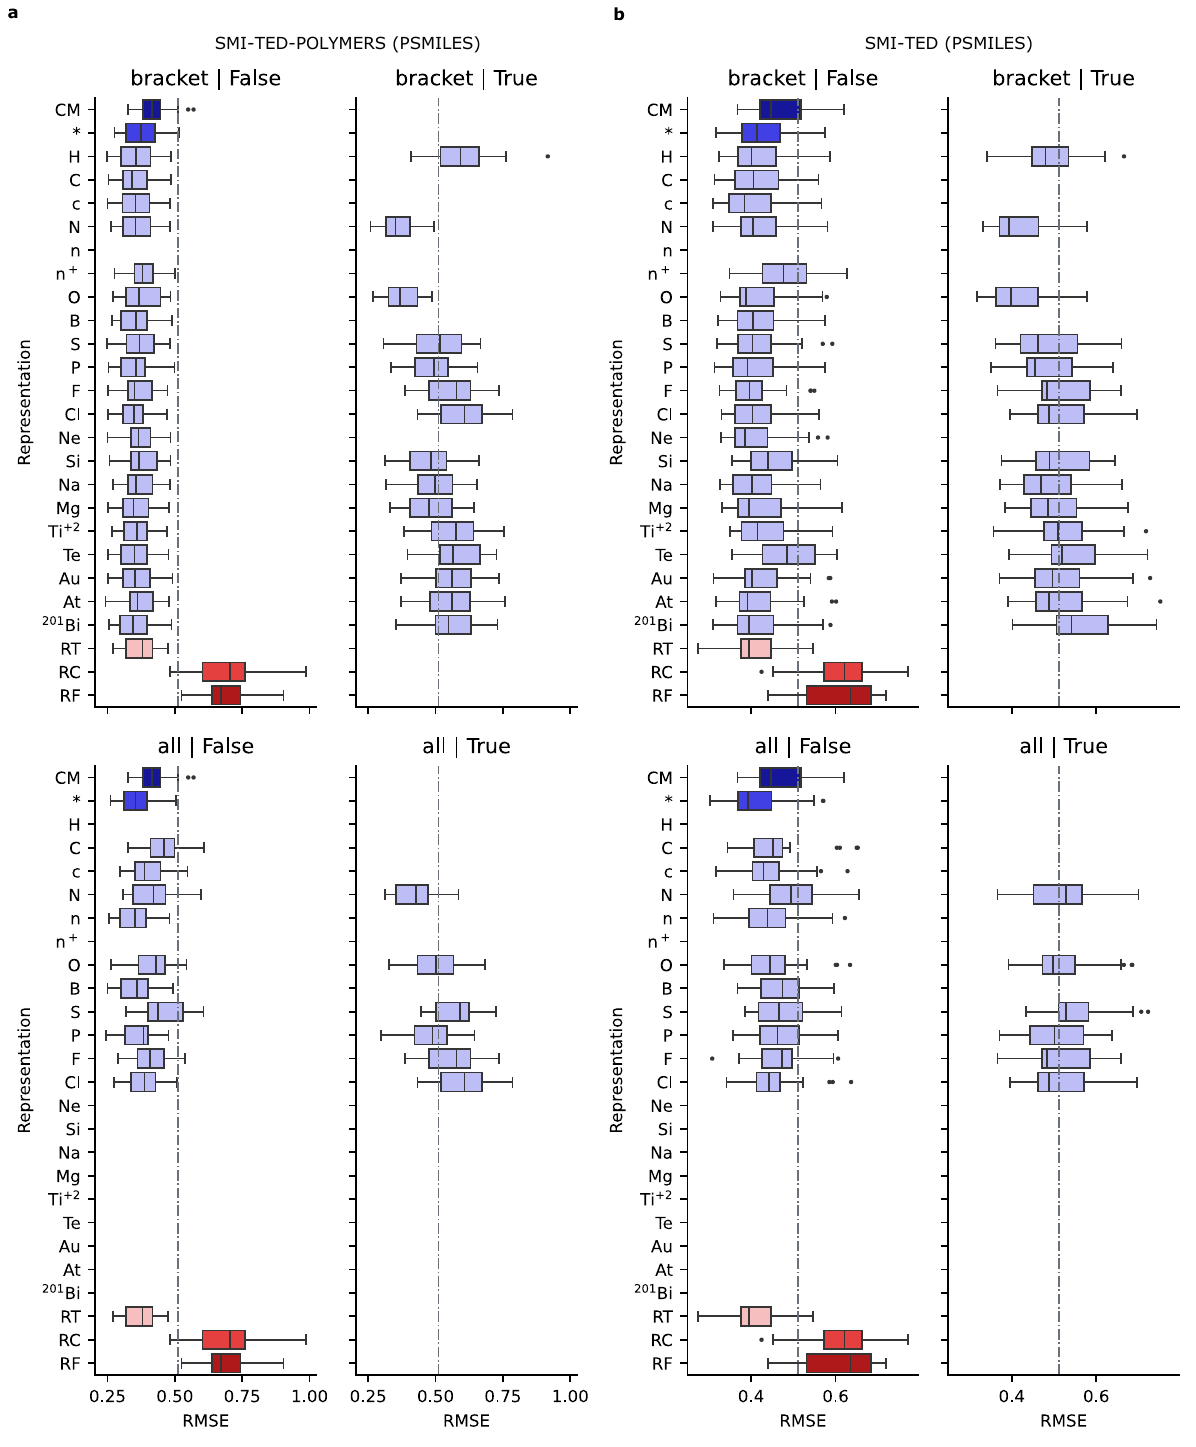}
\caption{Box plots for EPS repeated cross-validation experiments for SMI-TED-POLYMER (\textbf{a}) and SMI-TED (\textbf{b}) models fine-tuned with PSMILES.}\label{eps_token_box_psmiles}
\end{figure}

\begin{figure}[H]
\centering
\includegraphics[width=1\textwidth]{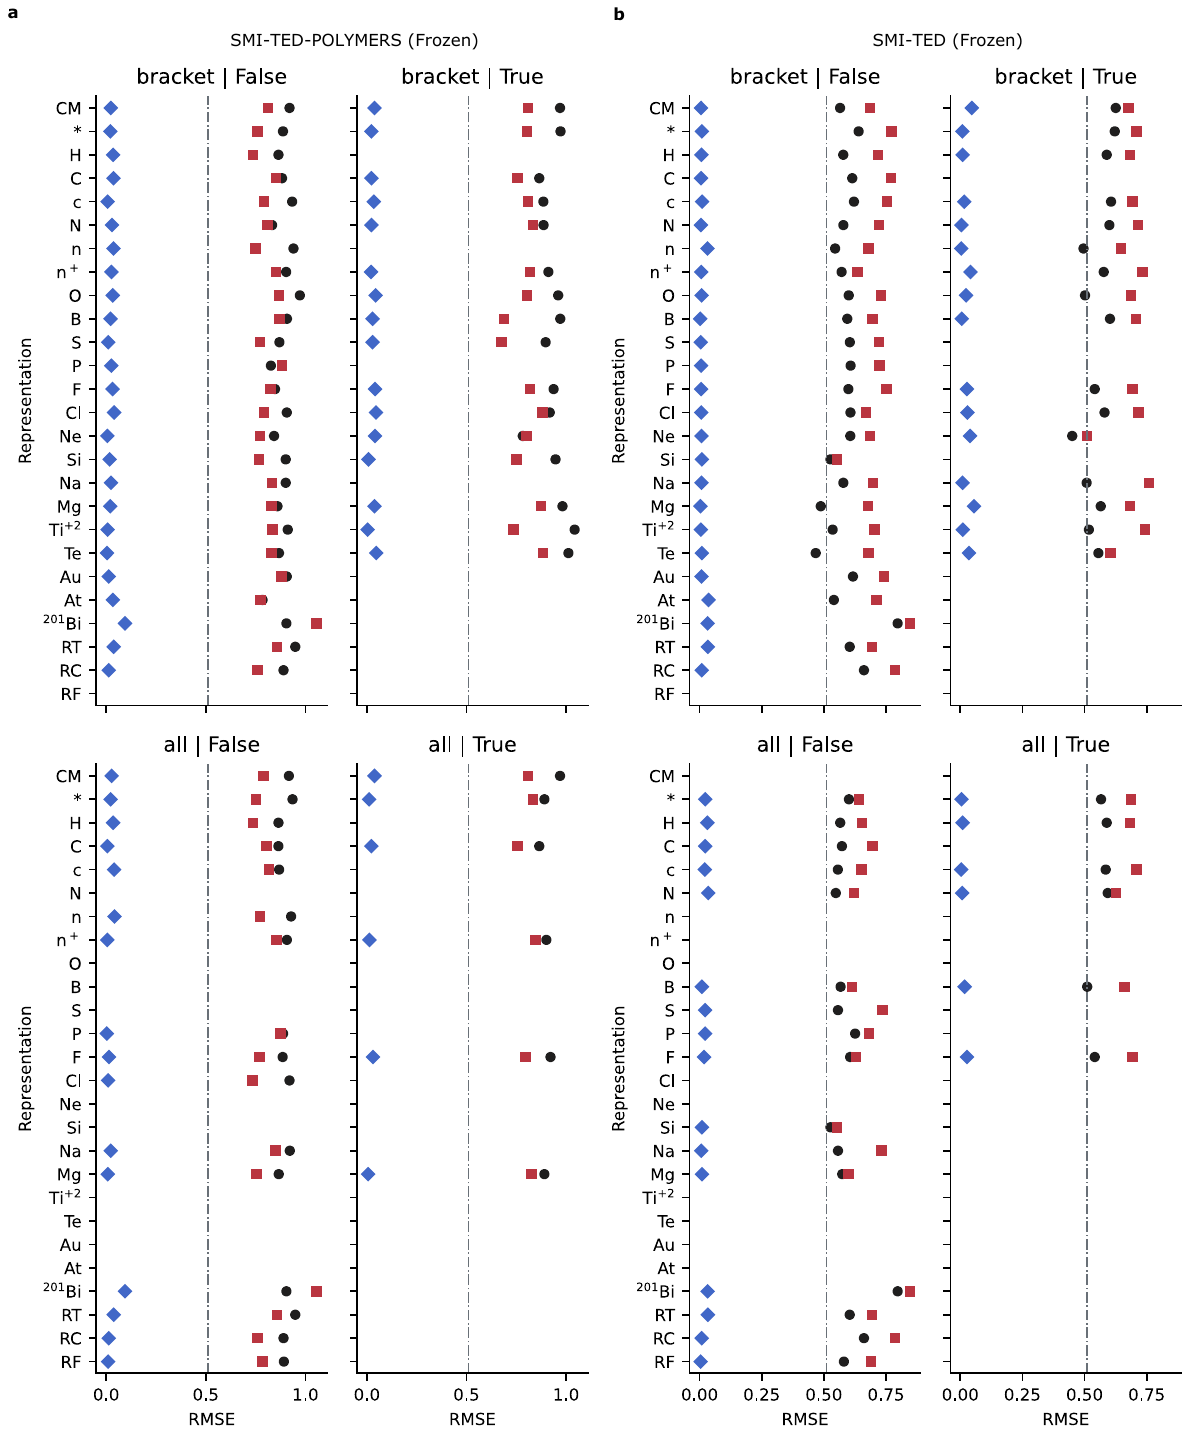}
\caption{Point plots for EPS benchmark experiments of RMSE using the base random train, valid, and test splits for SMI-TED-POLYMER (\textbf{a}) and SMI-TED (\textbf{b}) models with frozen weights.}\label{eps_token_point_frozen_rmse}
\end{figure}

\subsubsection{Polymer Dielectric Constant (EPS) Random Split Scores}\label{randEPS}

\begin{figure}[H]
\centering
\includegraphics[width=1\textwidth]{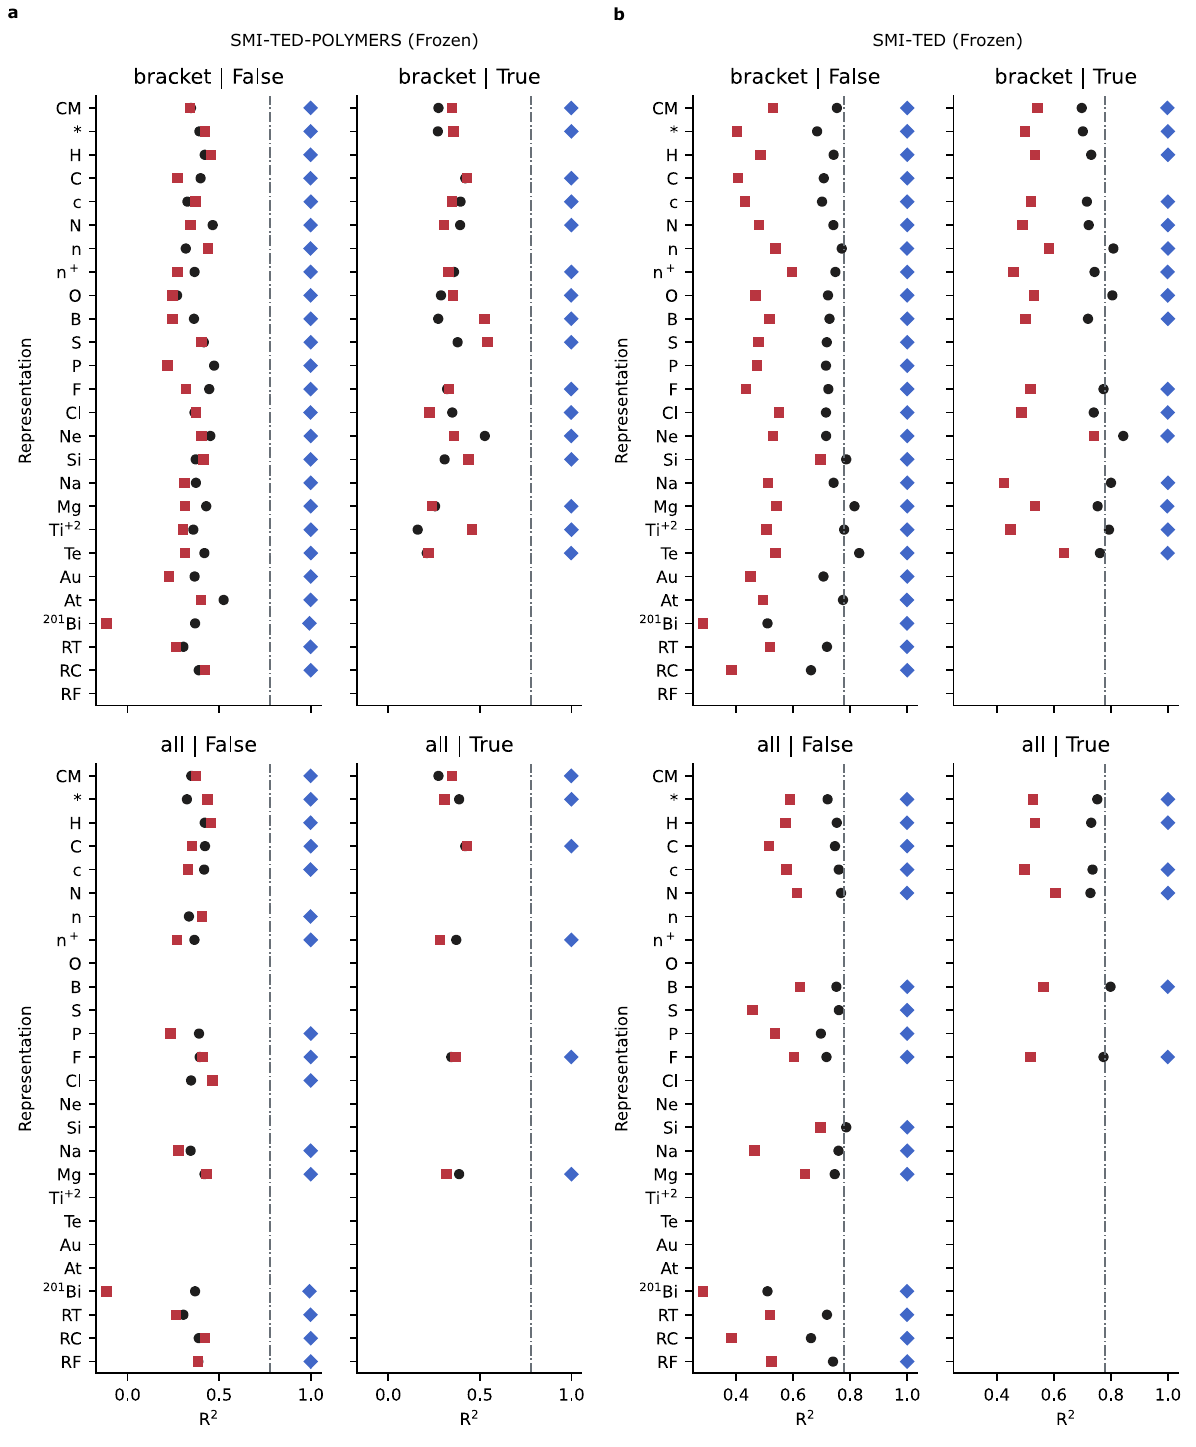}
\caption{Point plots for EPS benchmark experiments of R\textsuperscript{2} using the base random train, valid, and test splits for SMI-TED-POLYMER (\textbf{a}) and SMI-TED (\textbf{b}) models with frozen weights.}\label{eps_token_point_frozen_r2}
\end{figure}

\begin{figure}[H]
\centering
\includegraphics[width=1\textwidth]{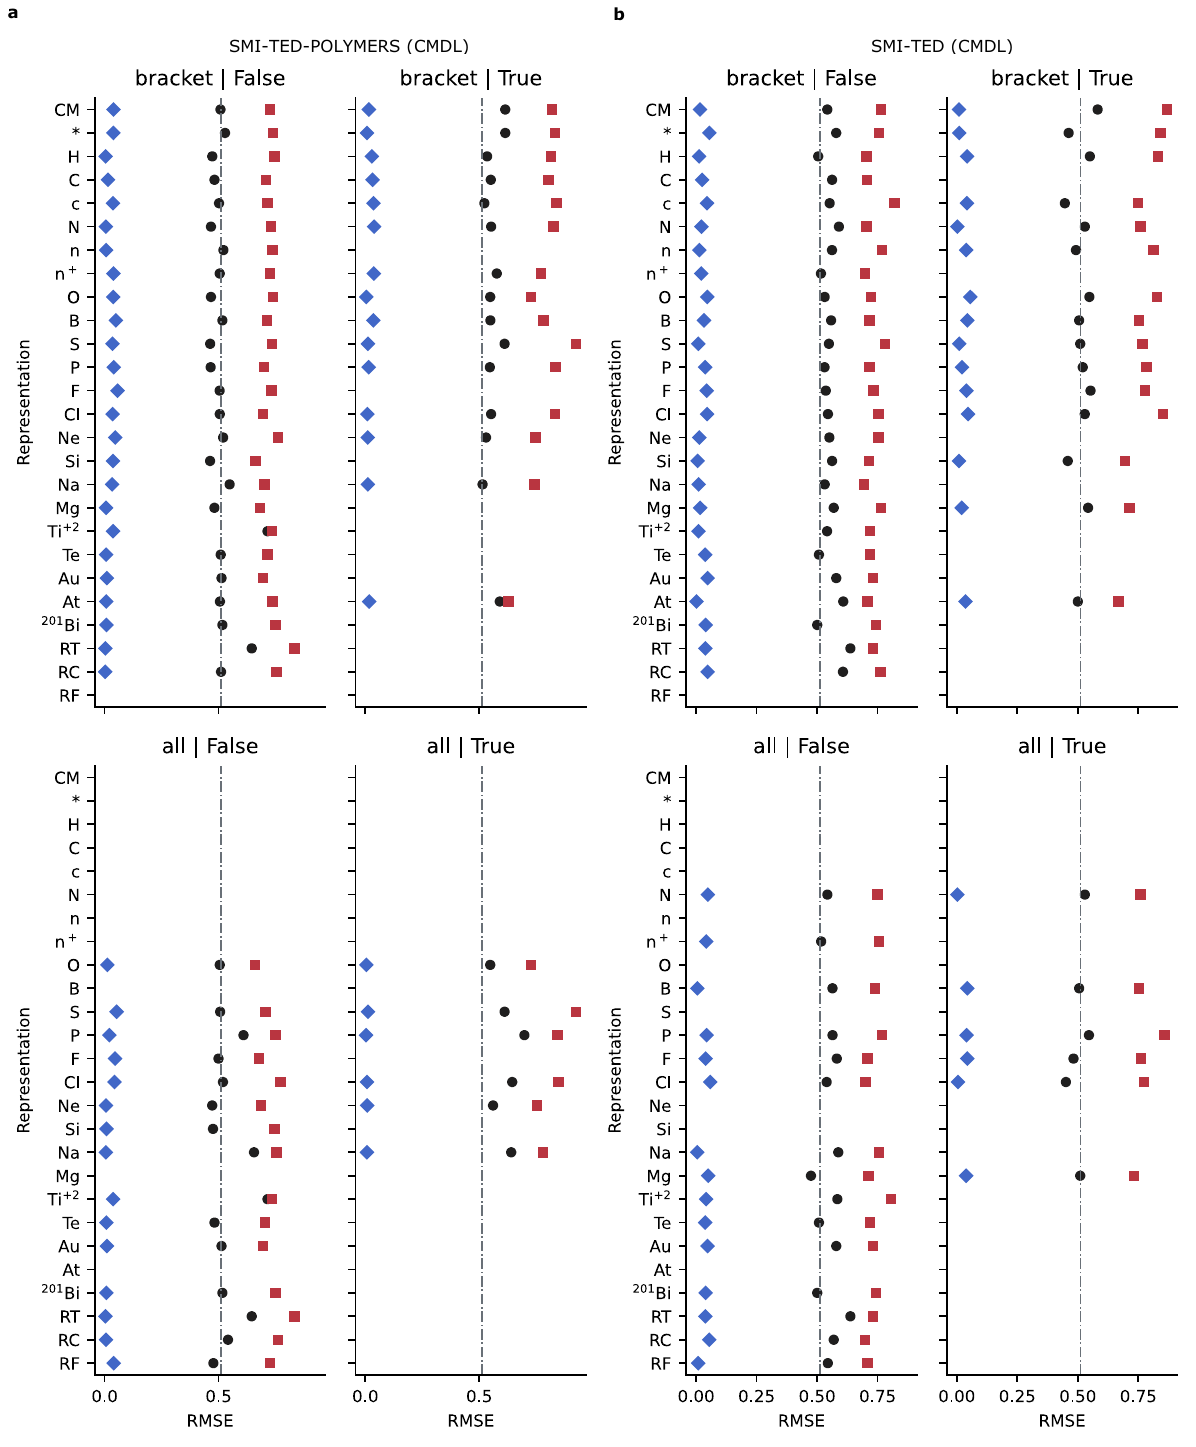}
\caption{Point plots for EPS benchmark experiments of RMSE using the base random train, valid, and test splits for SMI-TED-POLYMER (\textbf{a}) and SMI-TED (\textbf{b}) models fine-tuned using the CPG representation.}\label{eps_token_point_cmdl_rmse}
\end{figure}

\begin{figure}[H]
\centering
\includegraphics[width=1\textwidth]{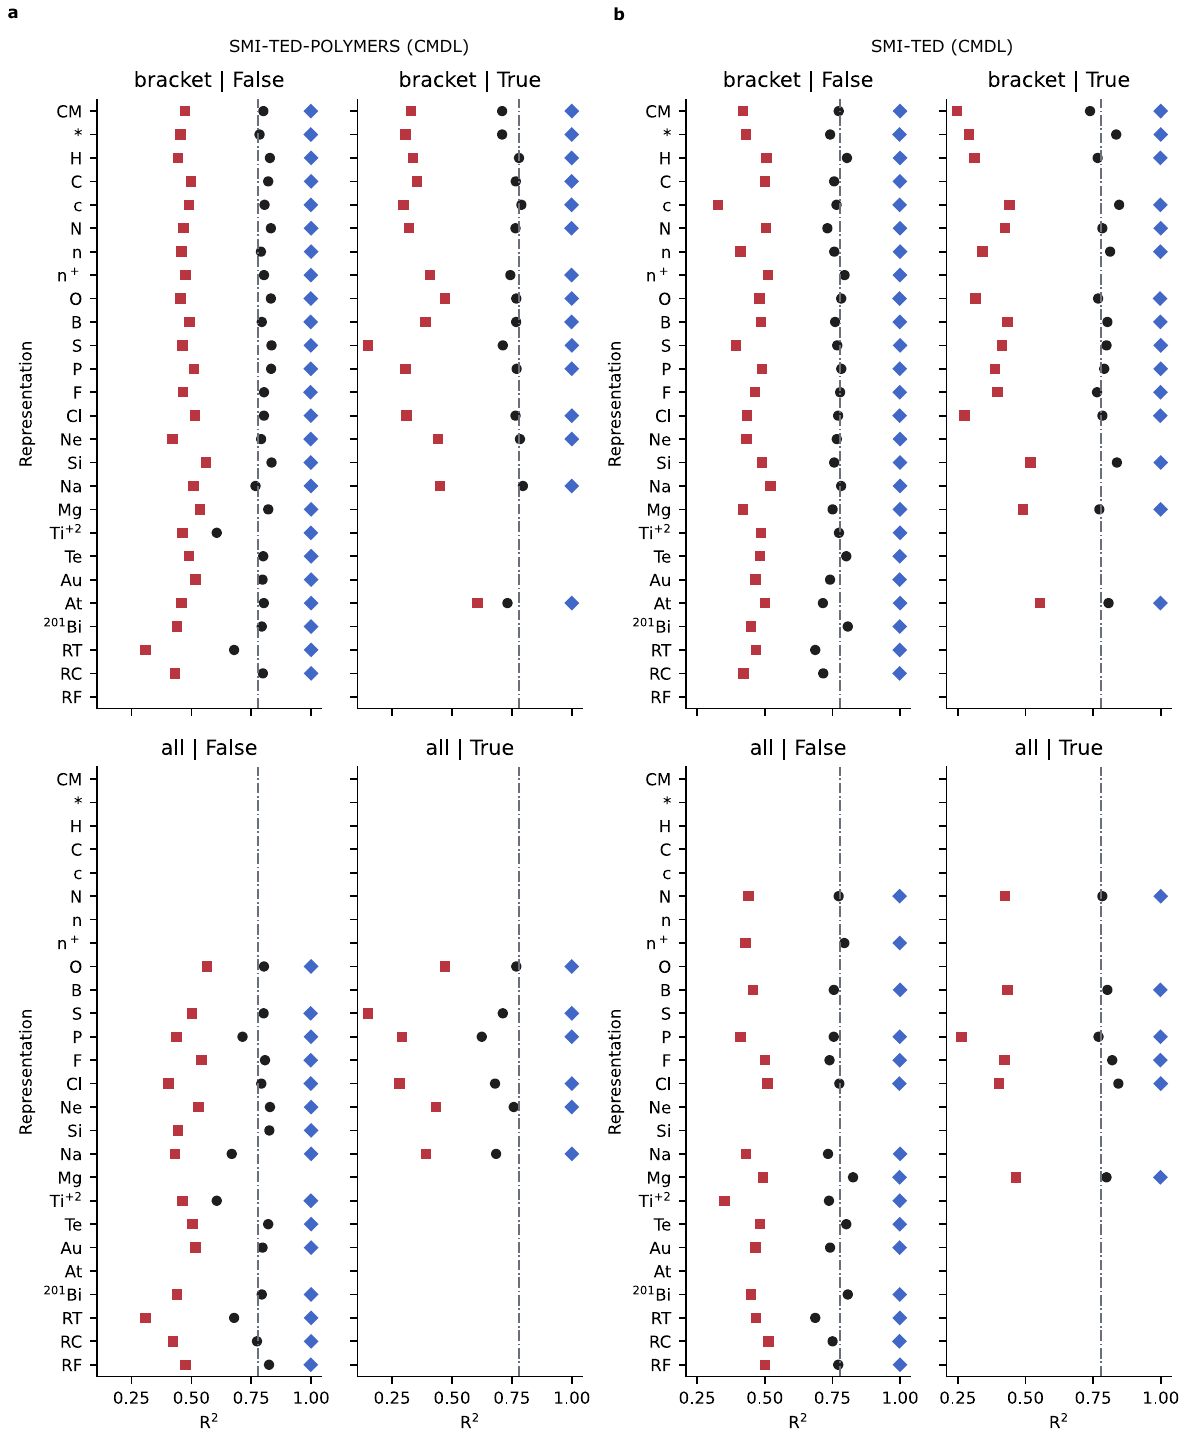}
\caption{Point plots for EPS benchmark experiments of R\textsuperscript{2} using the base random train, valid, and test splits for SMI-TED-POLYMER (\textbf{a}) and SMI-TED (\textbf{b}) models fine-tuned using the CPG representation.}\label{eps_token_point_cmdl_r2}
\end{figure}

\begin{figure}[H]
\centering
\includegraphics[width=1\textwidth]{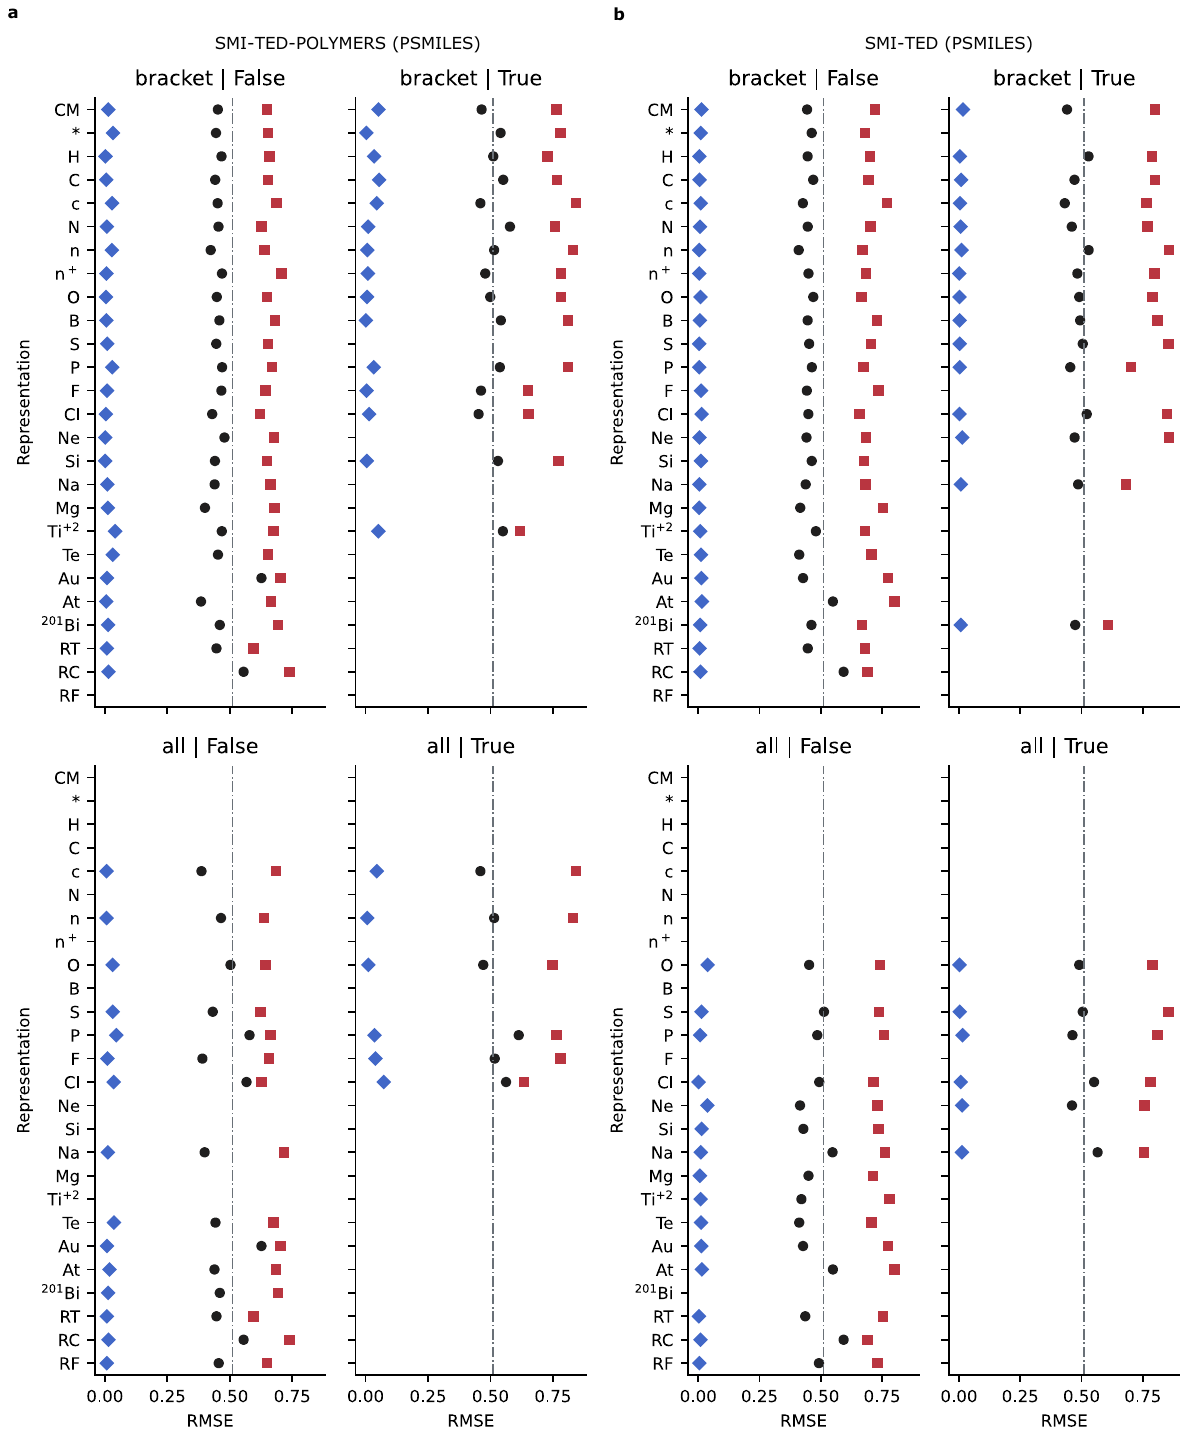}
\caption{Point plots for EPS benchmark experiments of RMSE using the base random train, valid, and test splits for SMI-TED-POLYMER (\textbf{a}) and SMI-TED (\textbf{b}) models fine-tuned using PSMILES.}\label{eps_token_point_psmiles_rmse}
\end{figure}

\begin{figure}[H]
\centering
\includegraphics[width=1\textwidth]{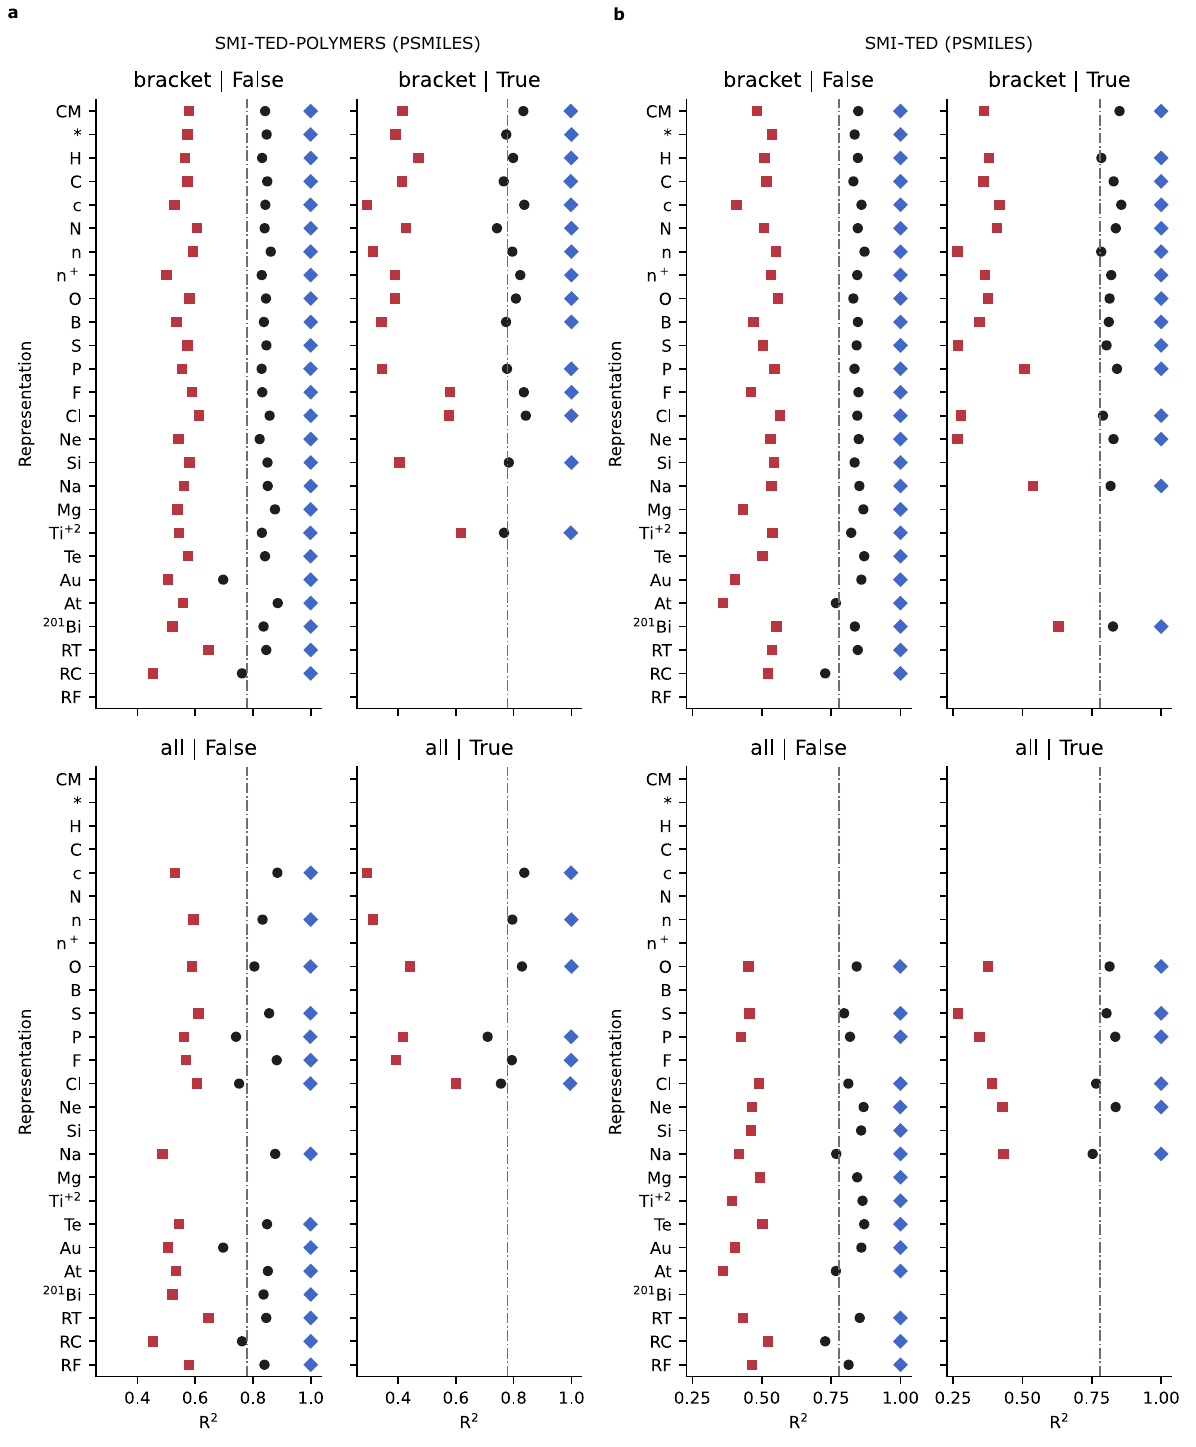}
\caption{Point plots for EPS benchmark experiments of R\textsuperscript{2} using the base random train, valid, and test splits for SMI-TED-POLYMER (\textbf{a}) and SMI-TED (\textbf{b}) models fine-tuned using PSMILES.}\label{eps_token_point_psmiles_r2}
\end{figure}

\subsubsection{Polymer Electron Affinity (E\textsubscript{ea}) CV Scores}\label{cvEea}

\begin{figure}[H]
\centering
\includegraphics[width=1\textwidth]{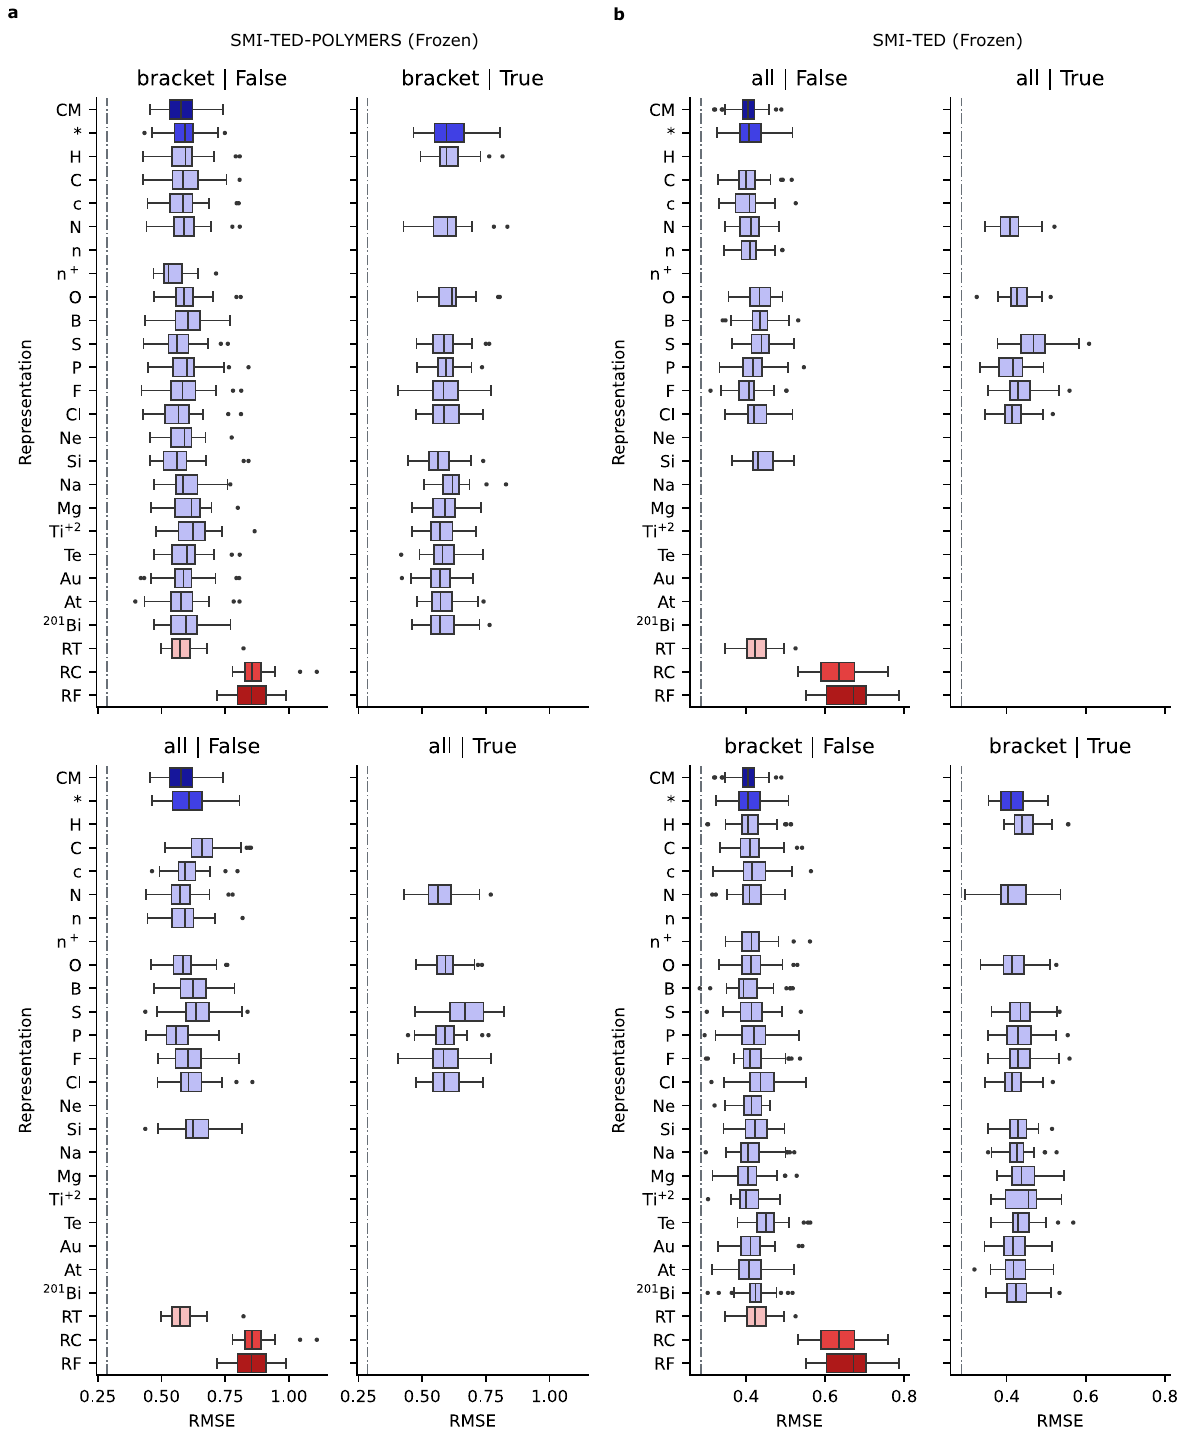}
\caption{Box plots for E\textsubscript{ea} repeated cross-validation experiments for SMI-TED-POLYMER (\textbf{a}) and SMI-TED (\textbf{b}) models with frozen weights.}\label{eea_token_box_frozen}
\end{figure}

\begin{figure}[H]
\centering
\includegraphics[width=1\textwidth]{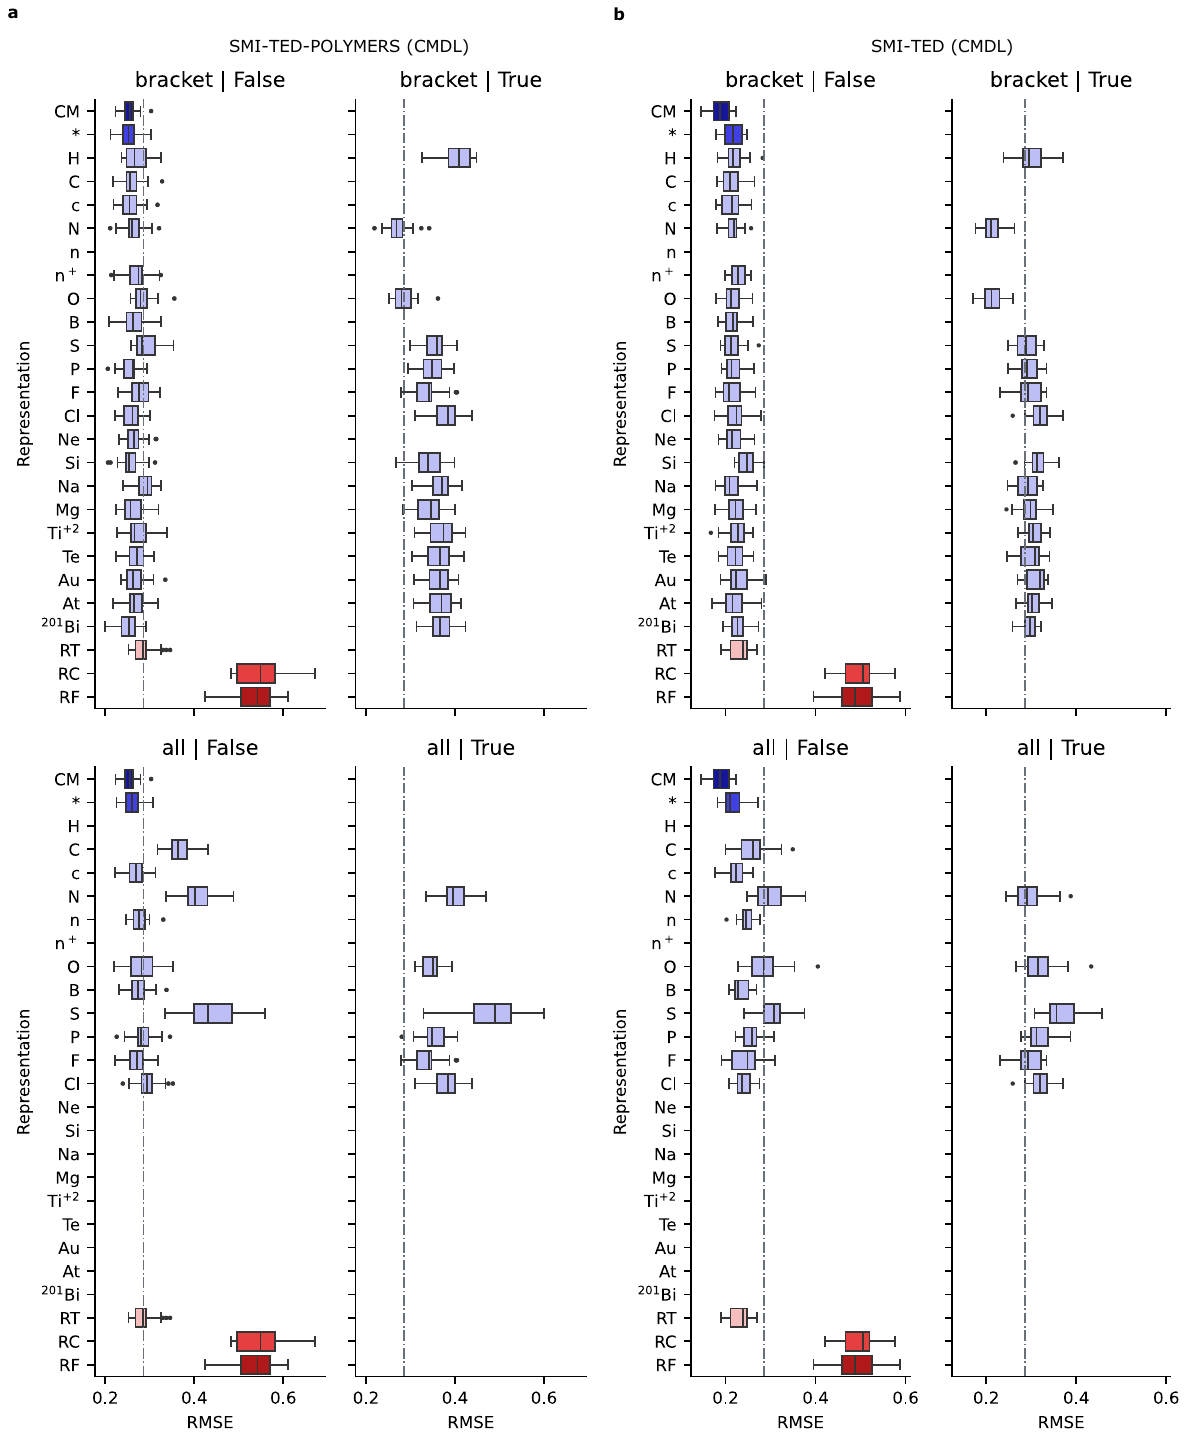}
\caption{Box plots for E\textsubscript{ea} repeated cross-validation experiments for SMI-TED-POLYMER (\textbf{a}) and SMI-TED (\textbf{b}) models fine-tuned with the CPG polymer graphs.}\label{eea_token_box_cmdl}
\end{figure}

\begin{figure}[H]
\centering
\includegraphics[width=1\textwidth]{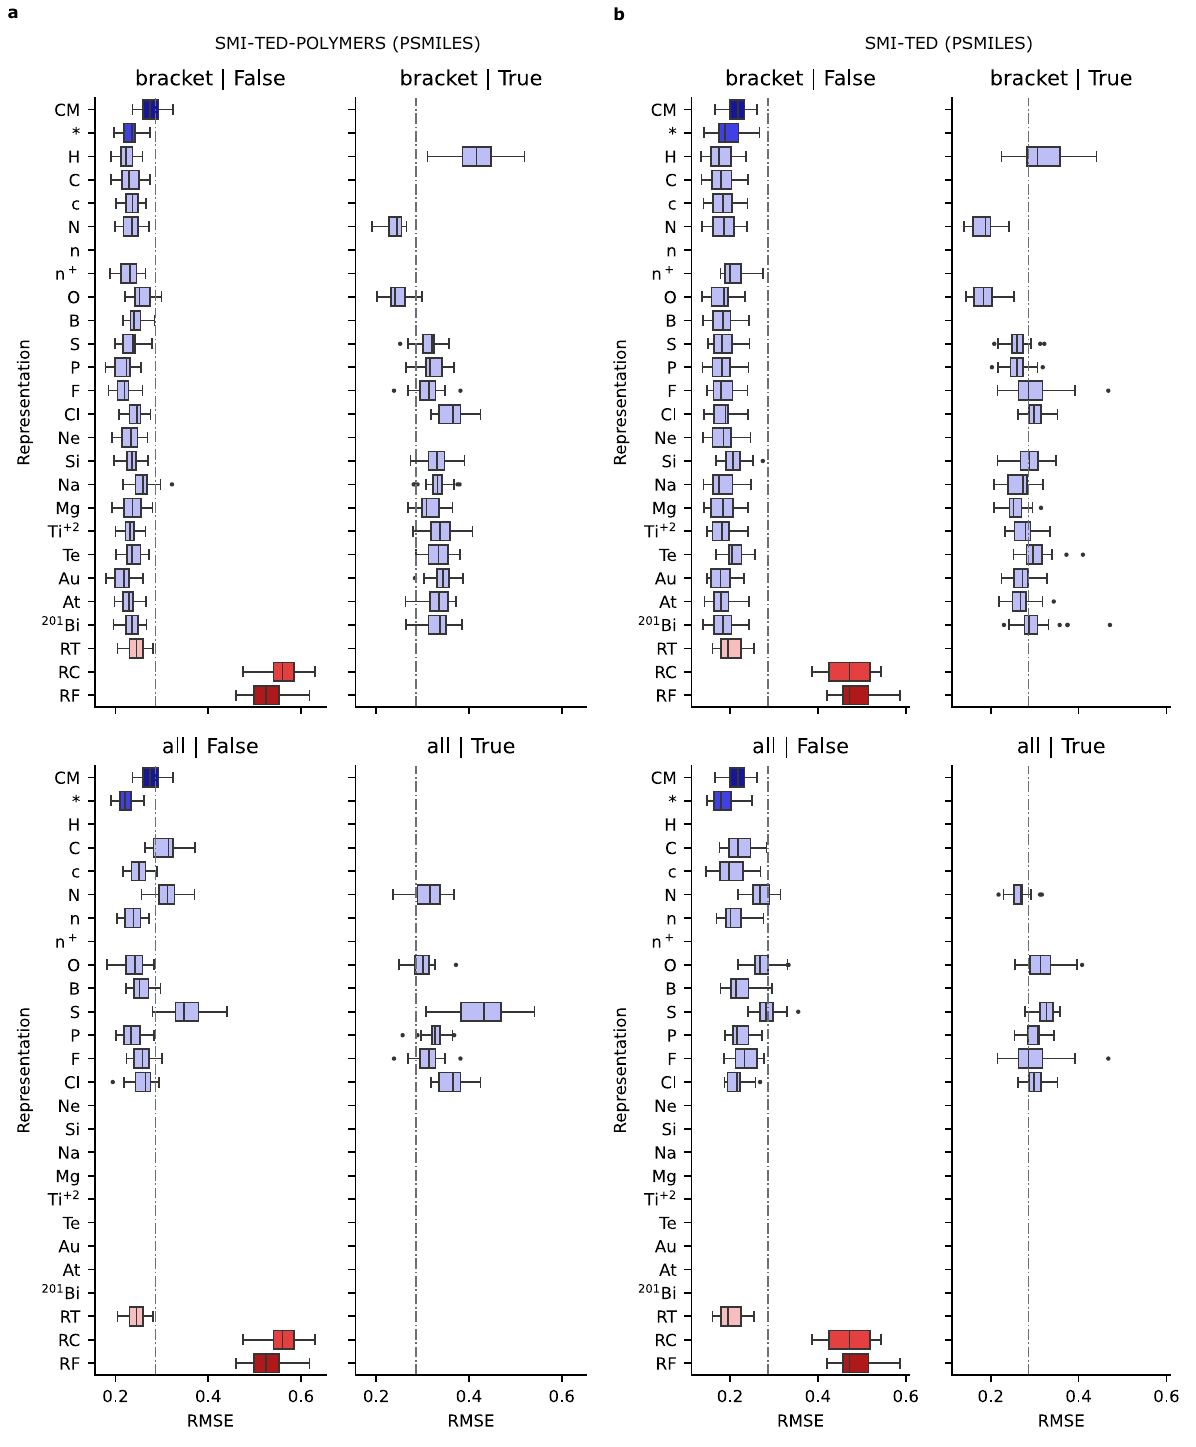}
\caption{Box plots for E\textsubscript{ea} repeated cross-validation experiments for SMI-TED-POLYMER (\textbf{a}) and SMI-TED (\textbf{b}) models fine-tuned with PSMILES.}\label{eea_token_box_psmiles}
\end{figure}

\subsubsection{Polymer Electron Affinity (E\textsubscript{ea}) Random Split Scores}\label{randEea}

\begin{figure}[H]
\centering
\includegraphics[width=1\textwidth]{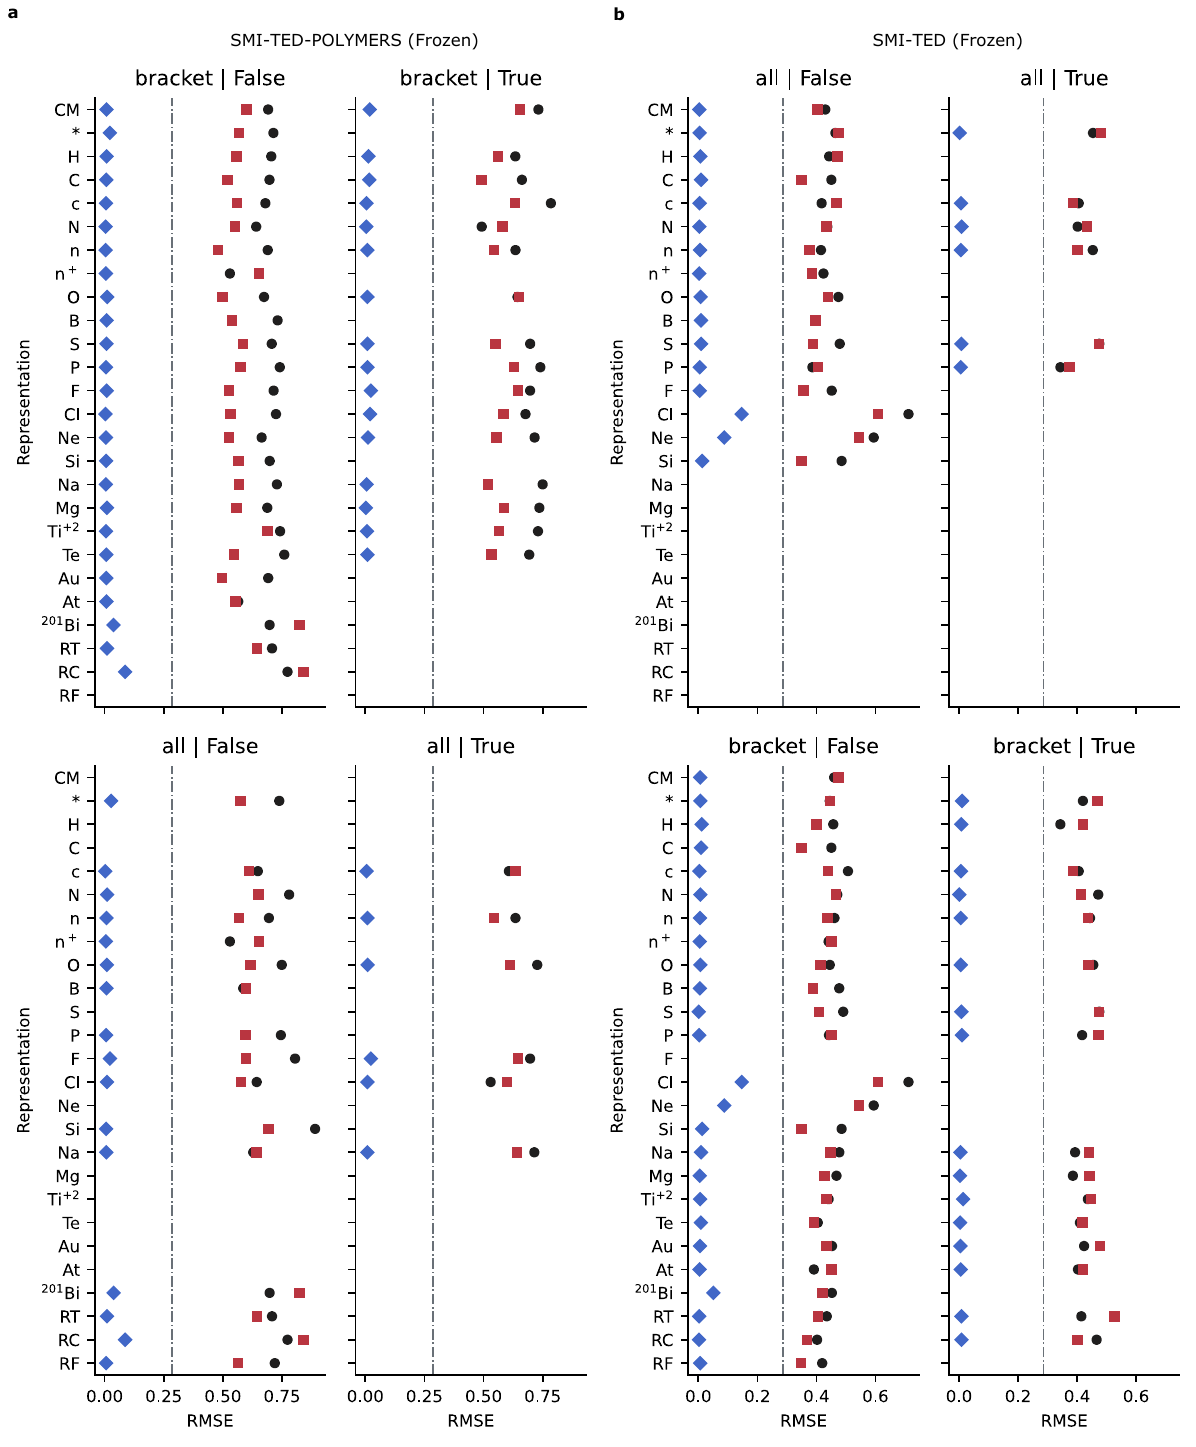}
\caption{Point plots for E\textsubscript{ea} benchmark experiments of RMSE using the base random train, valid, and test splits for SMI-TED-POLYMER (\textbf{a}) and SMI-TED (\textbf{b}) models with frozen weights.}\label{eea_token_point_frozen_rmse}
\end{figure}

\begin{figure}[H]
\centering
\includegraphics[width=1\textwidth]{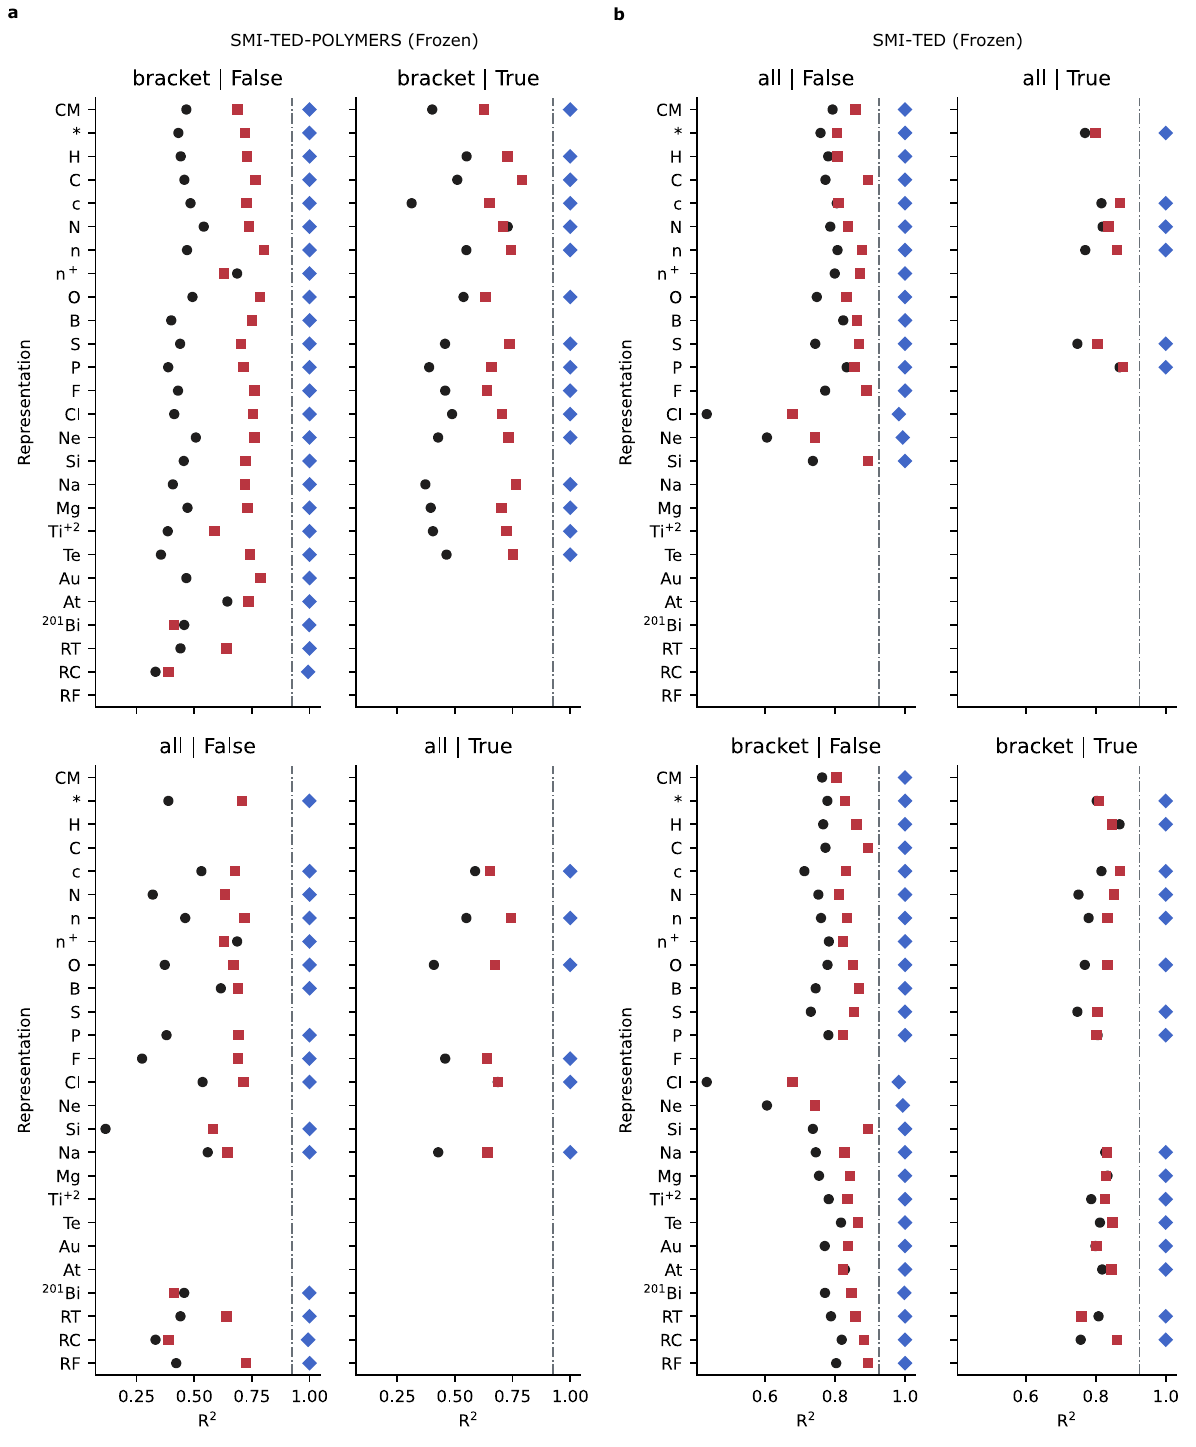}
\caption{Point plots for E\textsubscript{ea} benchmark experiments of R\textsuperscript{2} using the base random train, valid, and test splits for SMI-TED-POLYMER (\textbf{a}) and SMI-TED (\textbf{b}) models with frozen weights.}\label{eea_token_point_frozen_r2}
\end{figure}

\begin{figure}[H]
\centering
\includegraphics[width=1\textwidth]{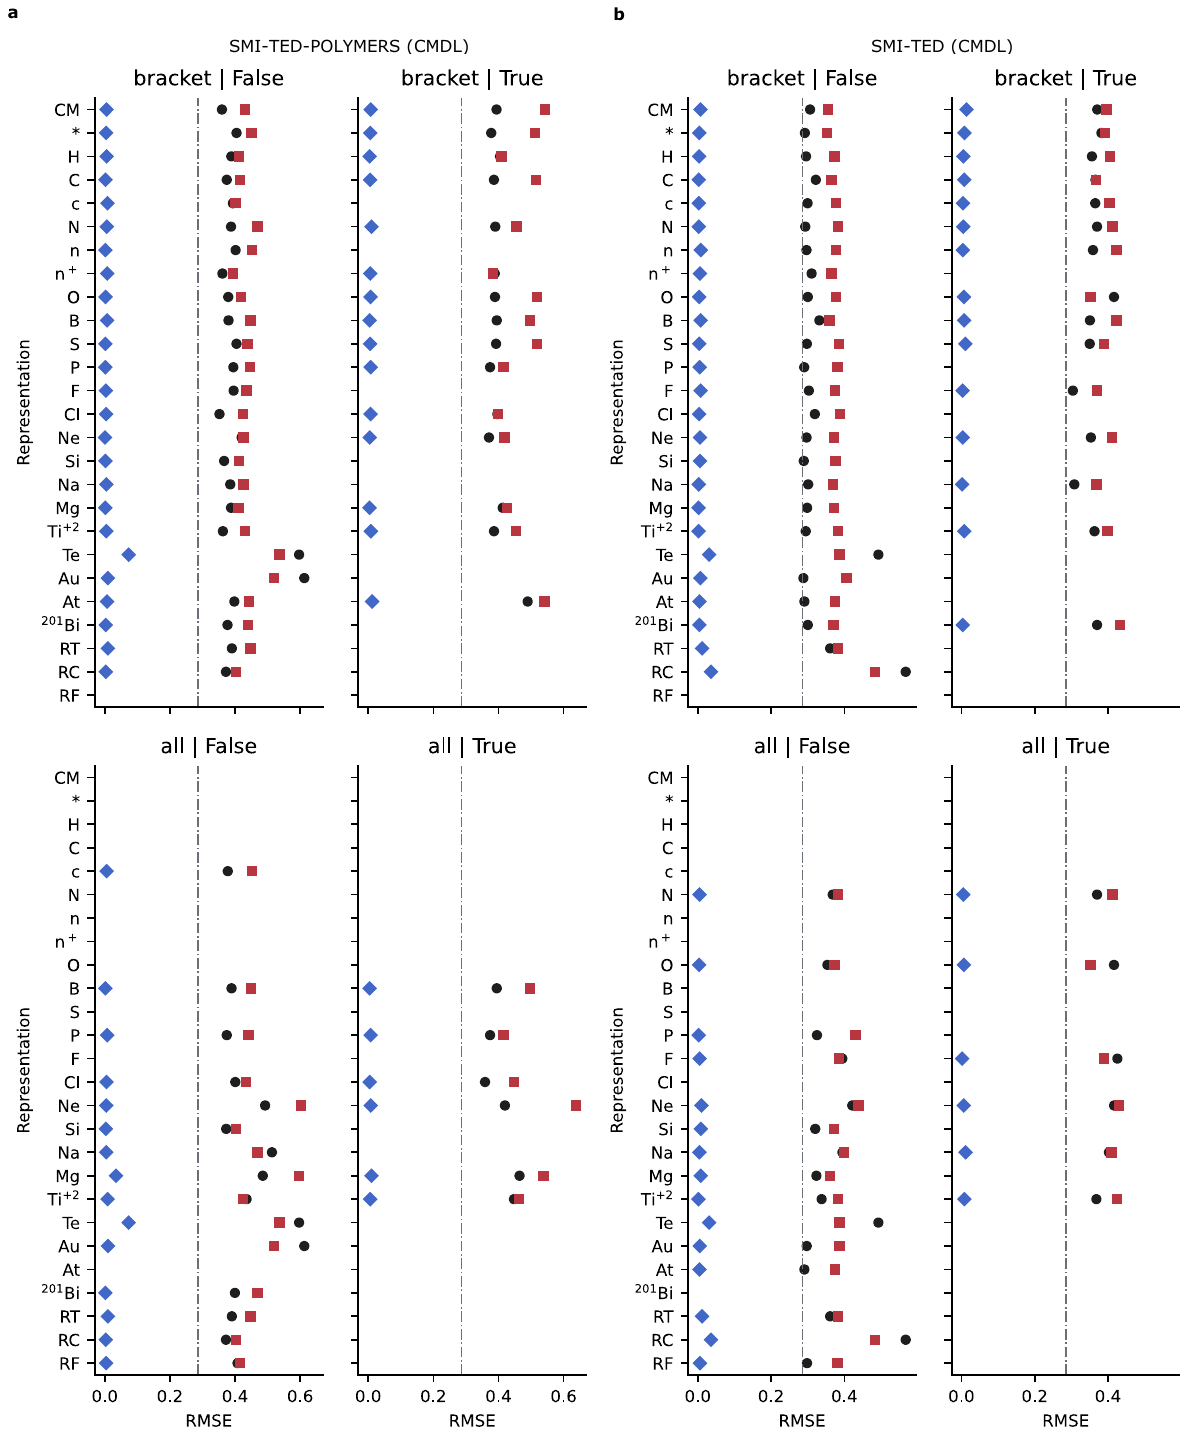}
\caption{Point plots for E\textsubscript{ea} benchmark experiments of RMSE using the base random train, valid, and test splits for SMI-TED-POLYMER (\textbf{a}) and SMI-TED (\textbf{b}) models fine-tuned using the CPG representation.}\label{eea_token_point_cmdl_rmse}
\end{figure}

\begin{figure}[H]
\centering
\includegraphics[width=1\textwidth]{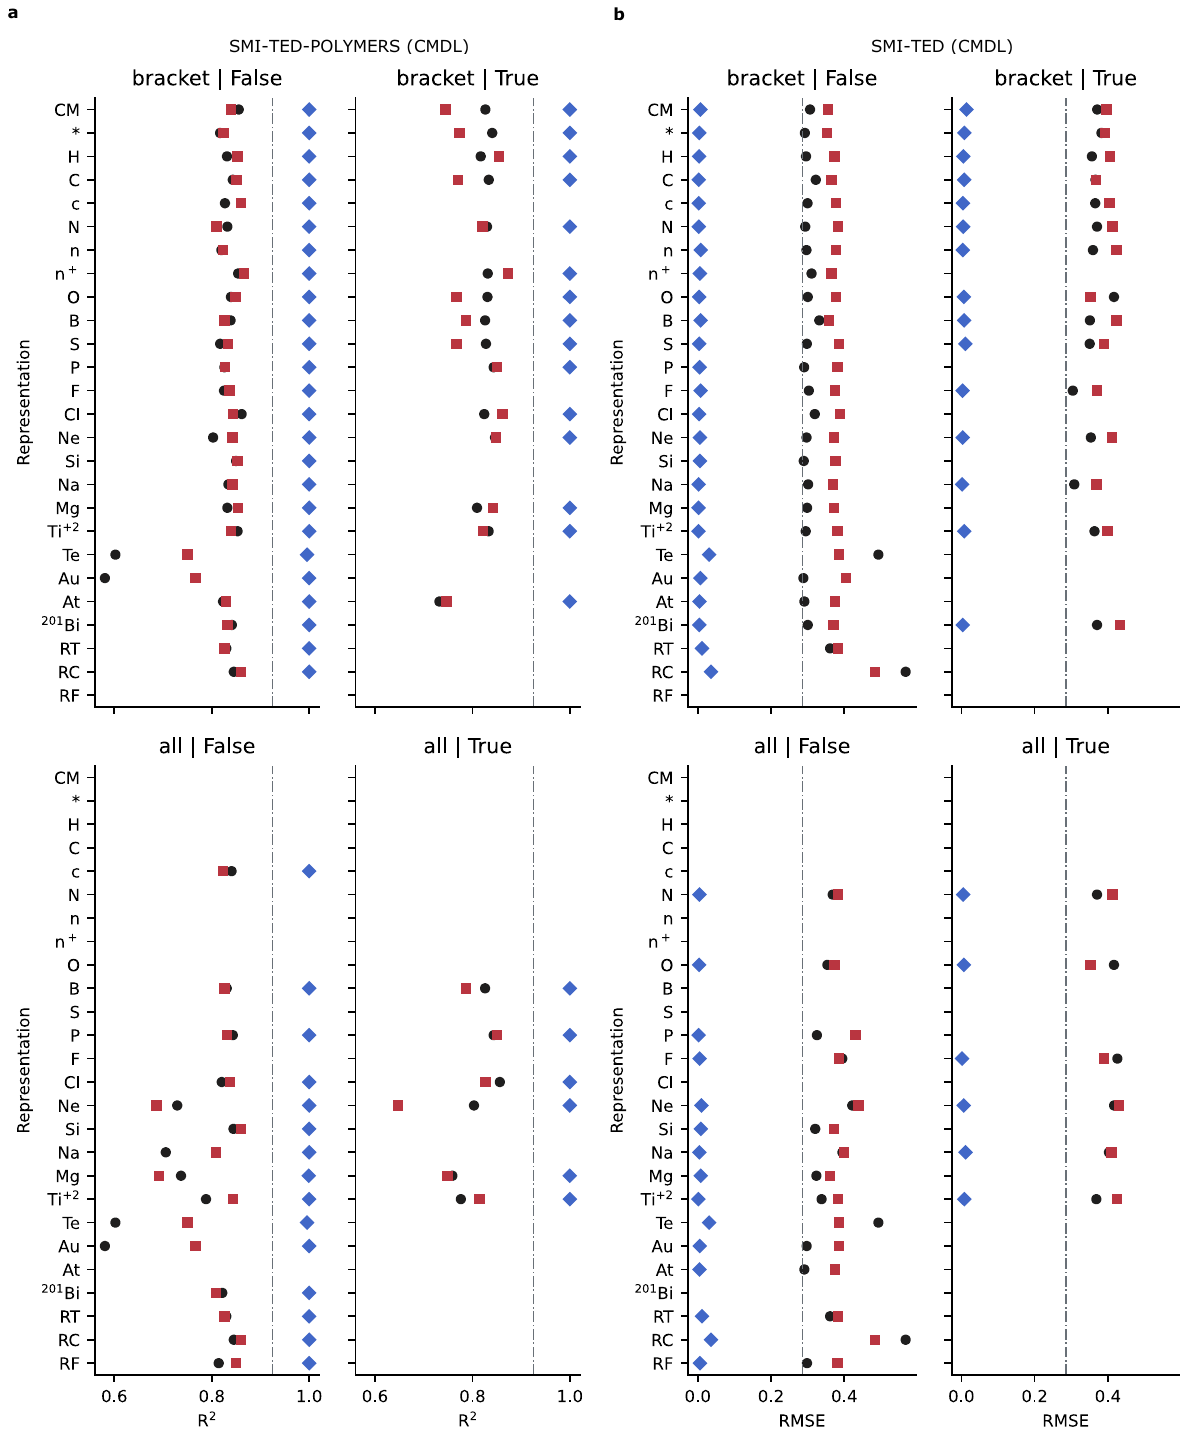}
\caption{Point plots for E\textsubscript{ea} benchmark experiments of R\textsuperscript{2} using the base random train, valid, and test splits for SMI-TED-POLYMER (\textbf{a}) and SMI-TED (\textbf{b}) models fine-tuned using the CPG representation.}\label{eea_token_point_cmdl_r2}
\end{figure}

\begin{figure}[H]
\centering
\includegraphics[width=1\textwidth]{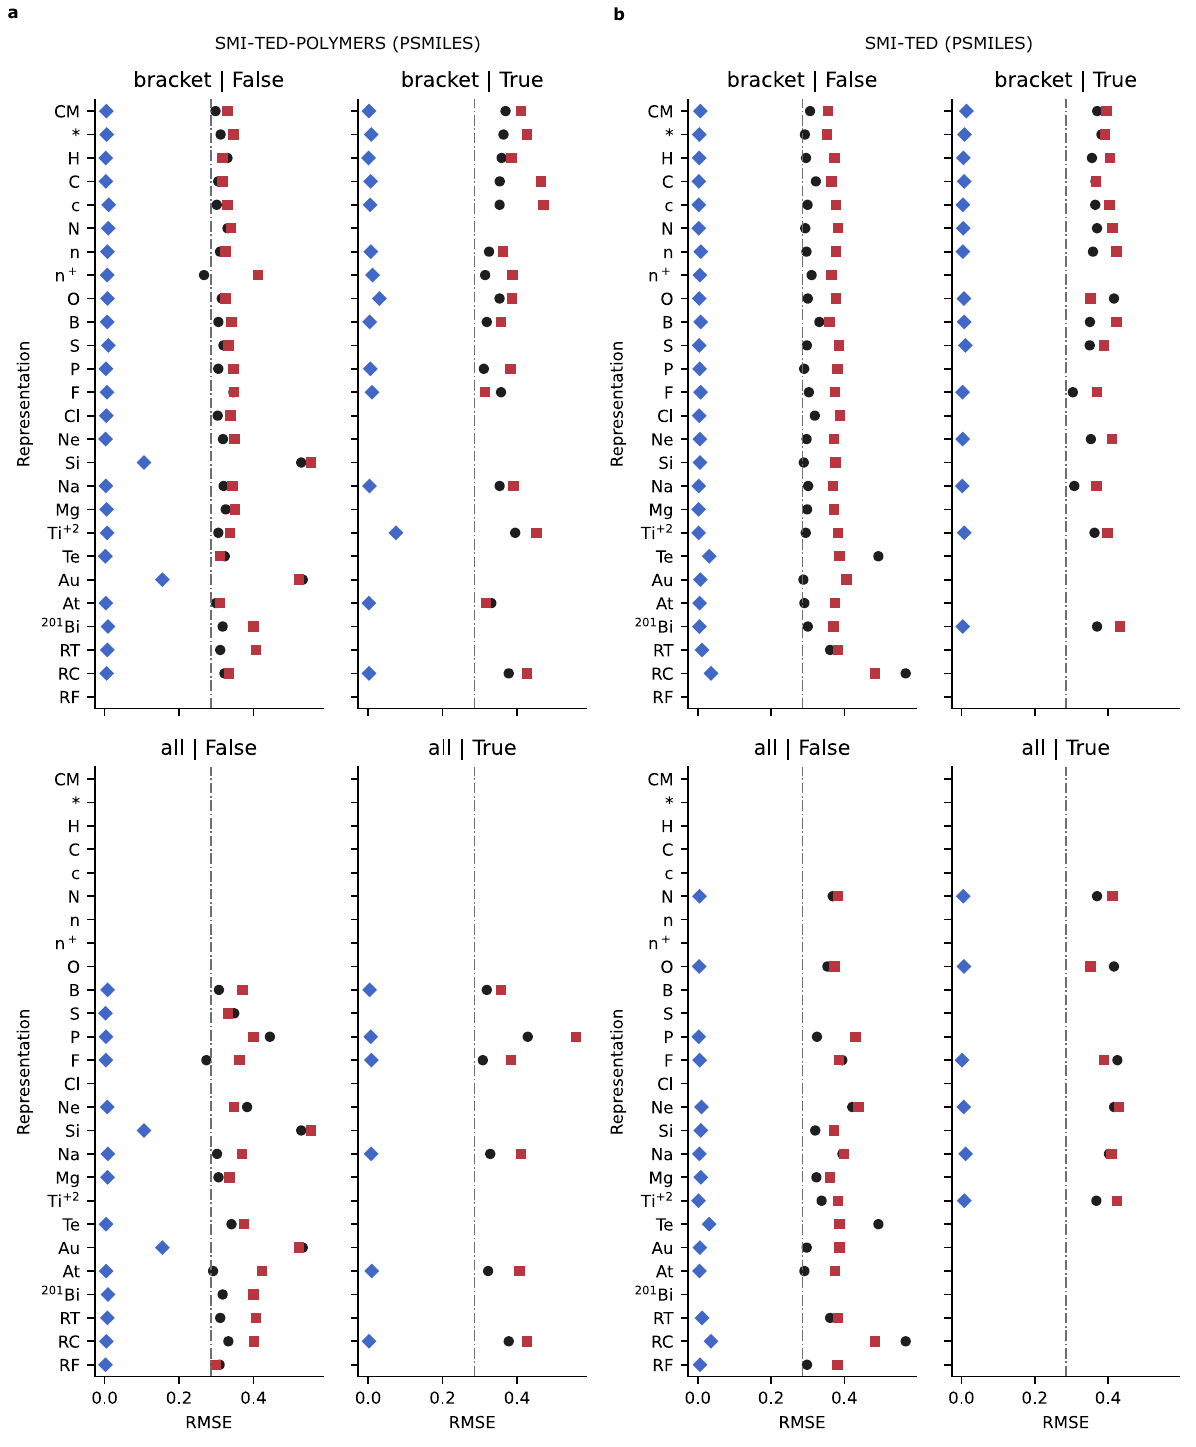}
\caption{Point plots for E\textsubscript{ea} benchmark experiments of RMSE using the base random train, valid, and test splits for SMI-TED-POLYMER (\textbf{a}) and SMI-TED (\textbf{b}) models fine-tuned using PSMILES.}\label{eea_token_point_psmiles_rmse}
\end{figure}

\begin{figure}
\centering
\includegraphics[width=1\textwidth]{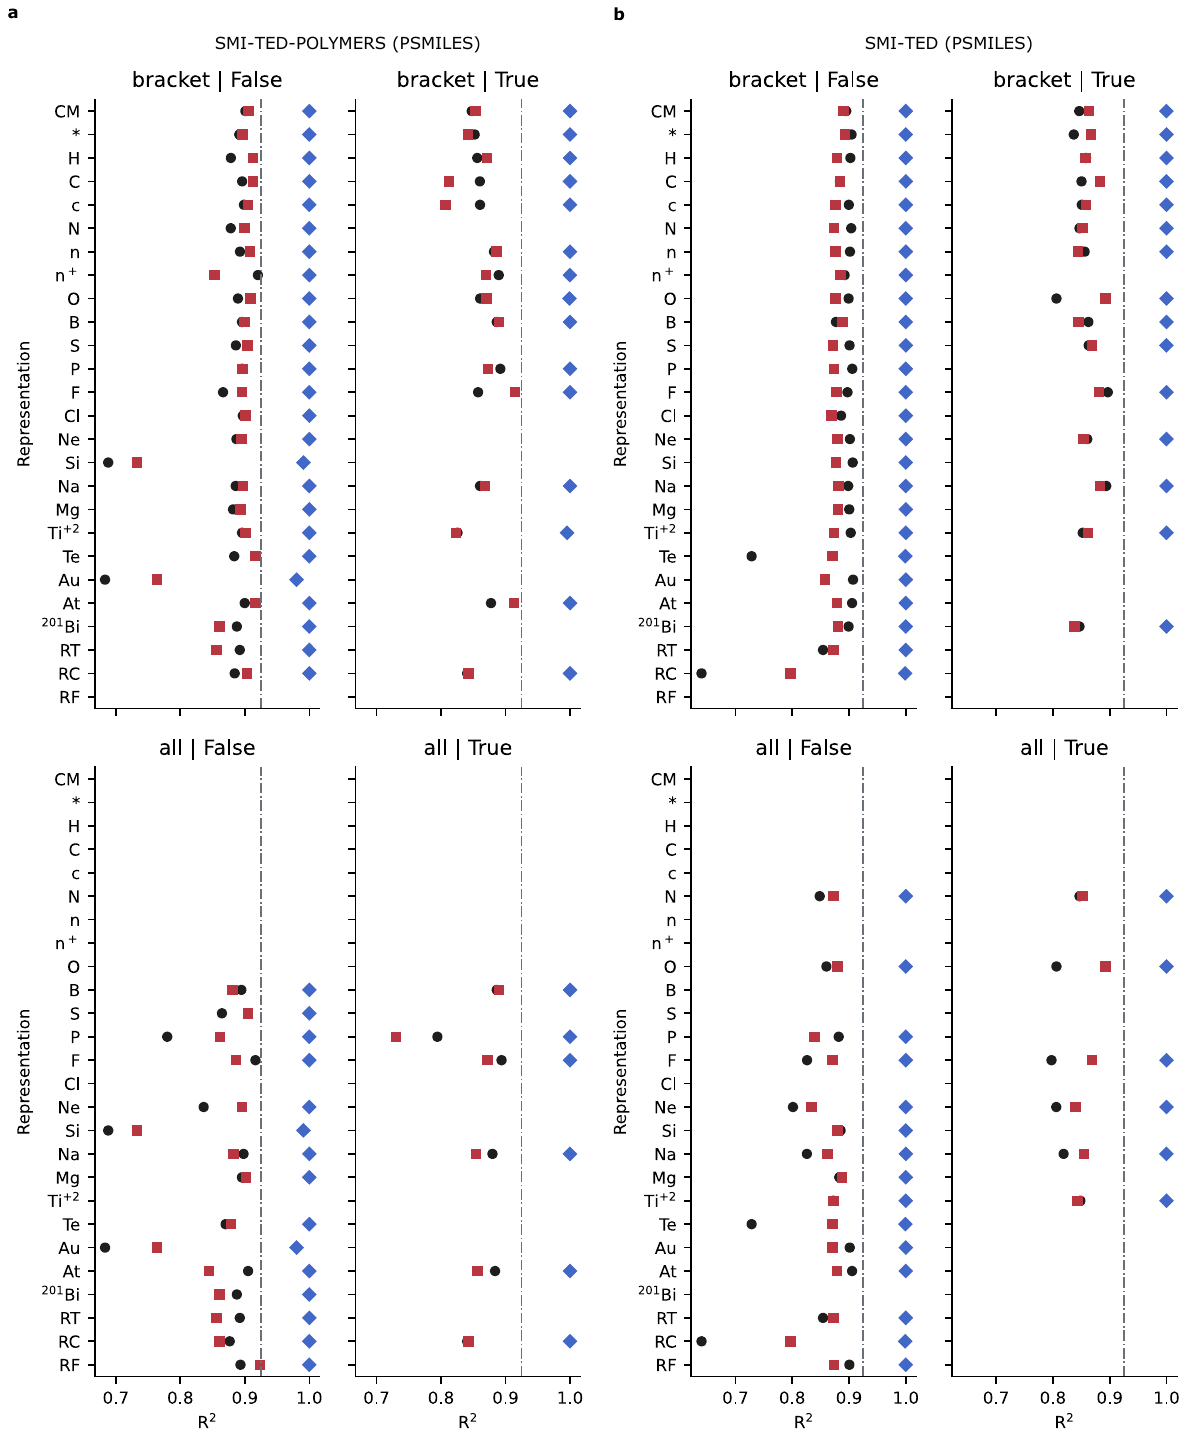}
\caption{Point plots for E\textsubscript{ea} benchmark experiments of R\textsuperscript{2} using the base random train, valid, and test splits for SMI-TED-POLYMER (\textbf{a}) and SMI-TED (\textbf{b}) models fine-tuned using PSMILES.}\label{eea_token_point_psmiles_r2}
\end{figure}

\subsubsection{Polymer Atomization Energy (E\textsubscript{at}) CV Scores}\label{cvEat}

\begin{figure}[H]
\centering
\includegraphics[width=1\textwidth]{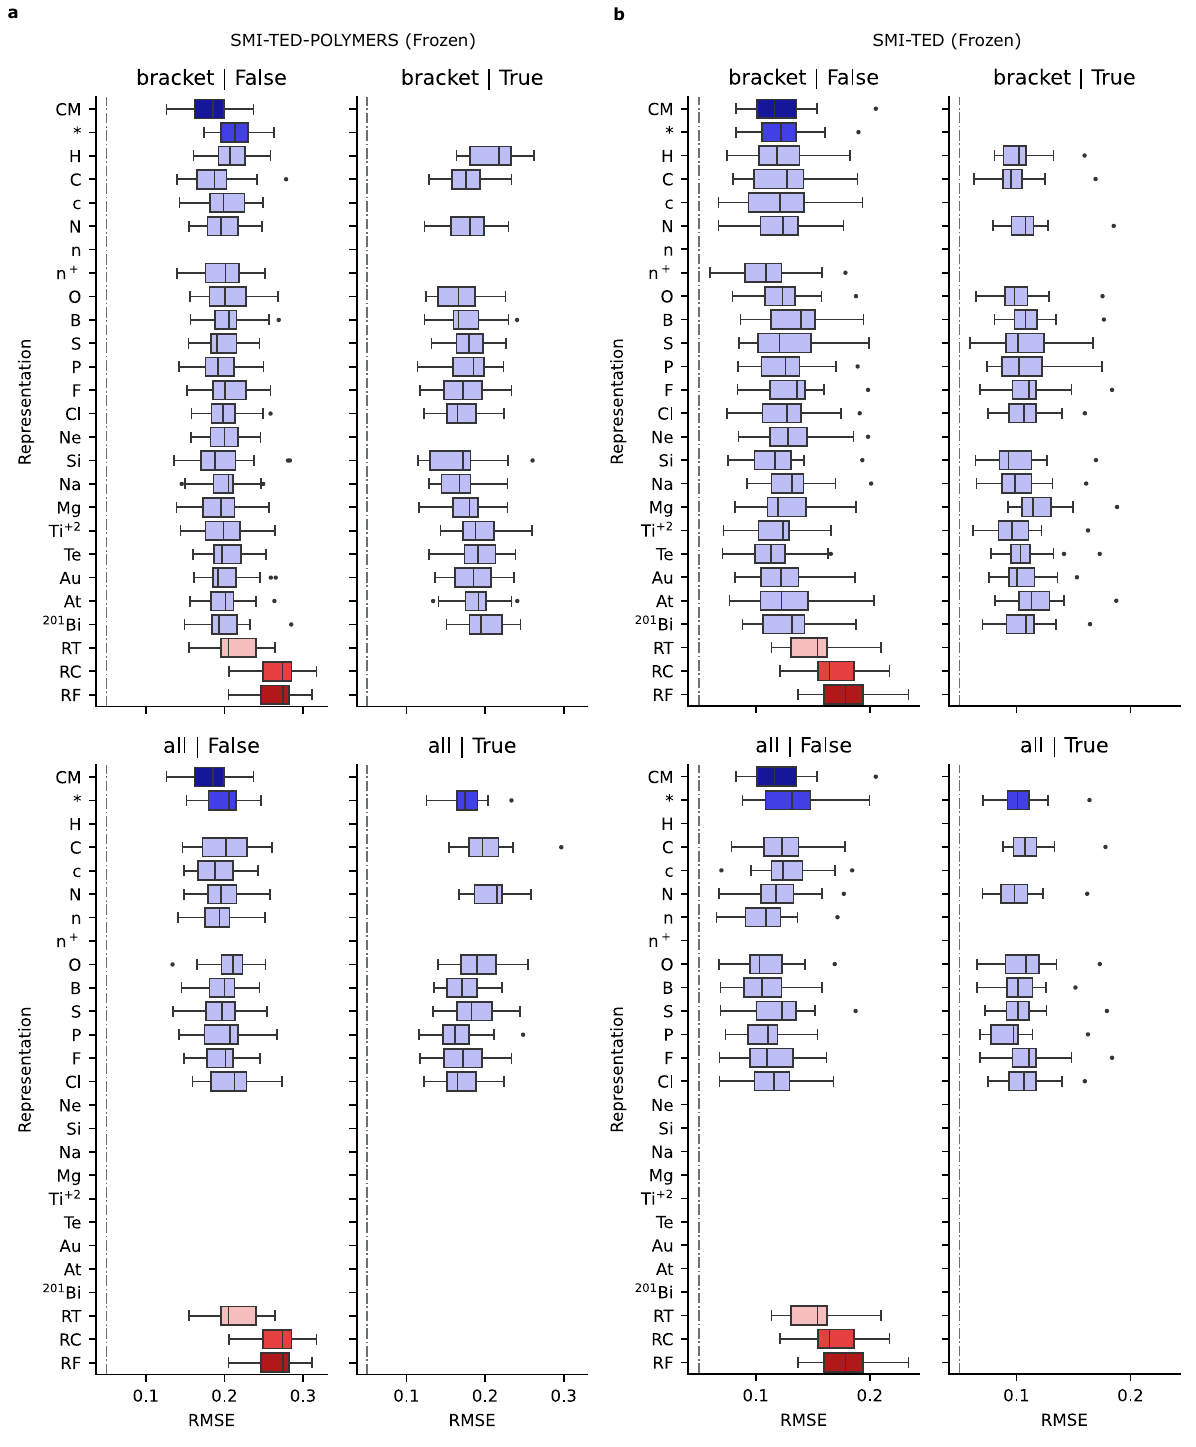}
\caption{Box plots for E\textsubscript{at} repeated cross-validation experiments for SMI-TED-POLYMER (\textbf{a}) and SMI-TED (\textbf{b}) models with frozen weights.}\label{eat_token_box_frozen}
\end{figure}

\begin{figure}[H]
\centering
\includegraphics[width=1\textwidth]{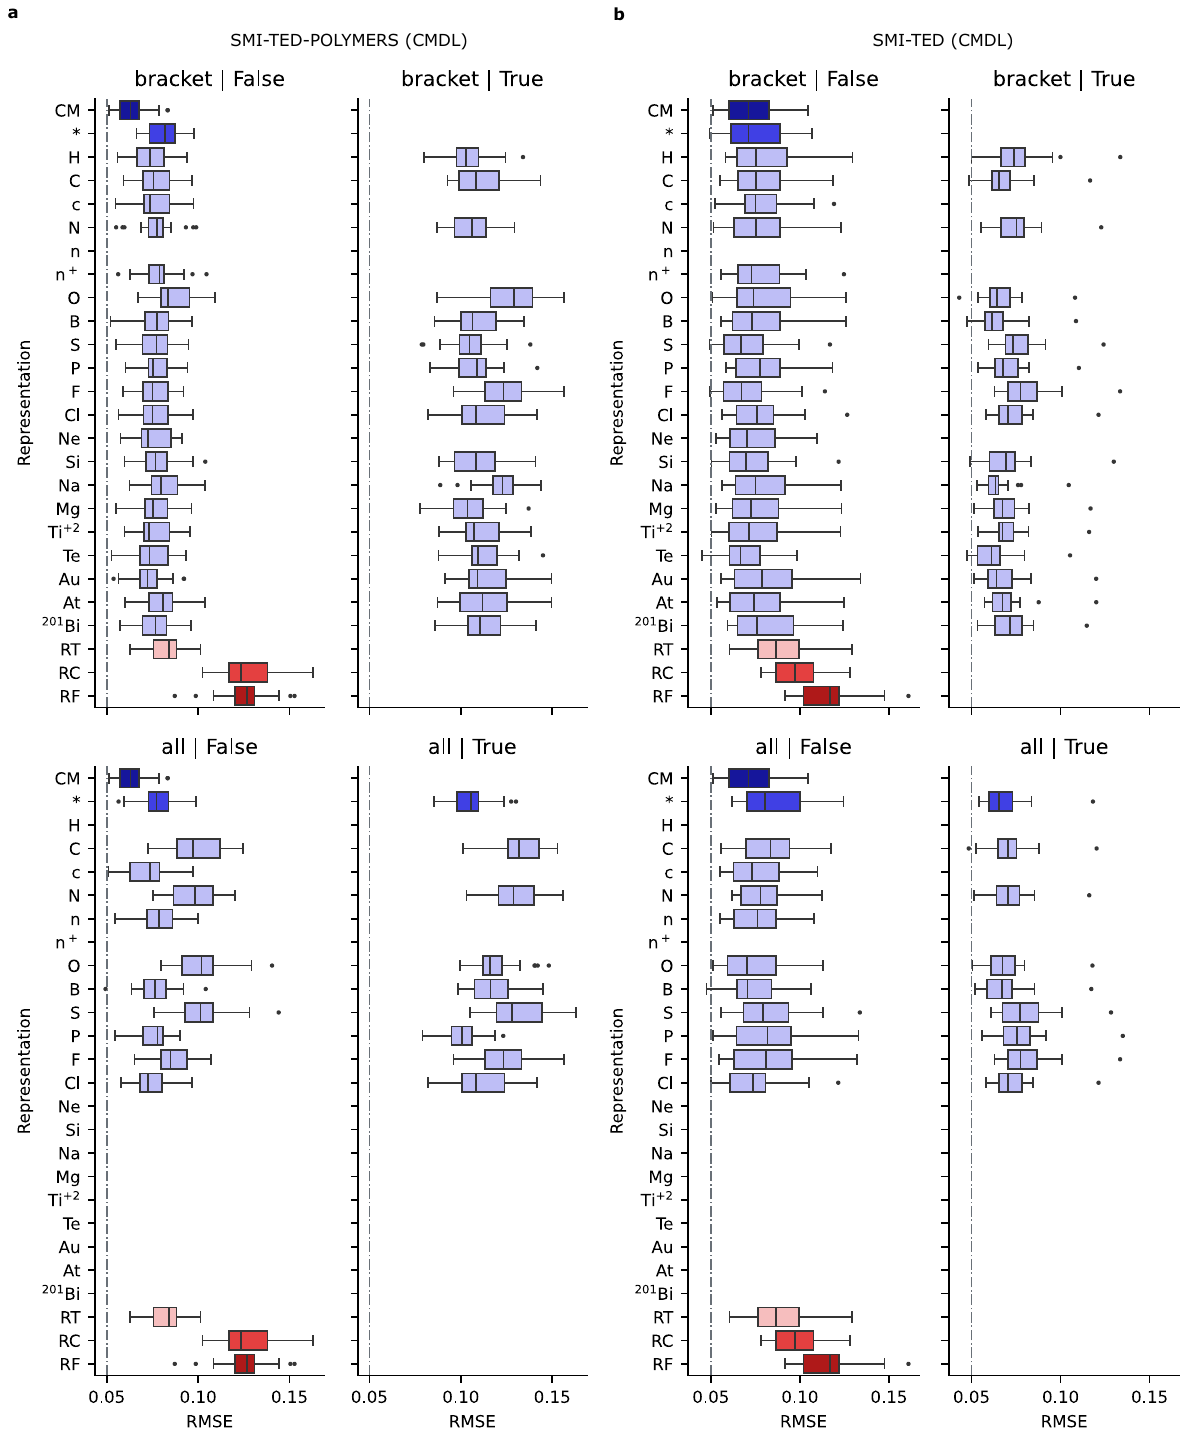}
\caption{Box plots for E\textsubscript{at} repeated cross-validation experiments for SMI-TED-POLYMER (\textbf{a}) and SMI-TED (\textbf{b}) models fine-tuned with the CPG polymer graphs.}\label{eat_token_box_cmdl}
\end{figure}

\begin{figure}[H]
\centering
\includegraphics[width=1\textwidth]{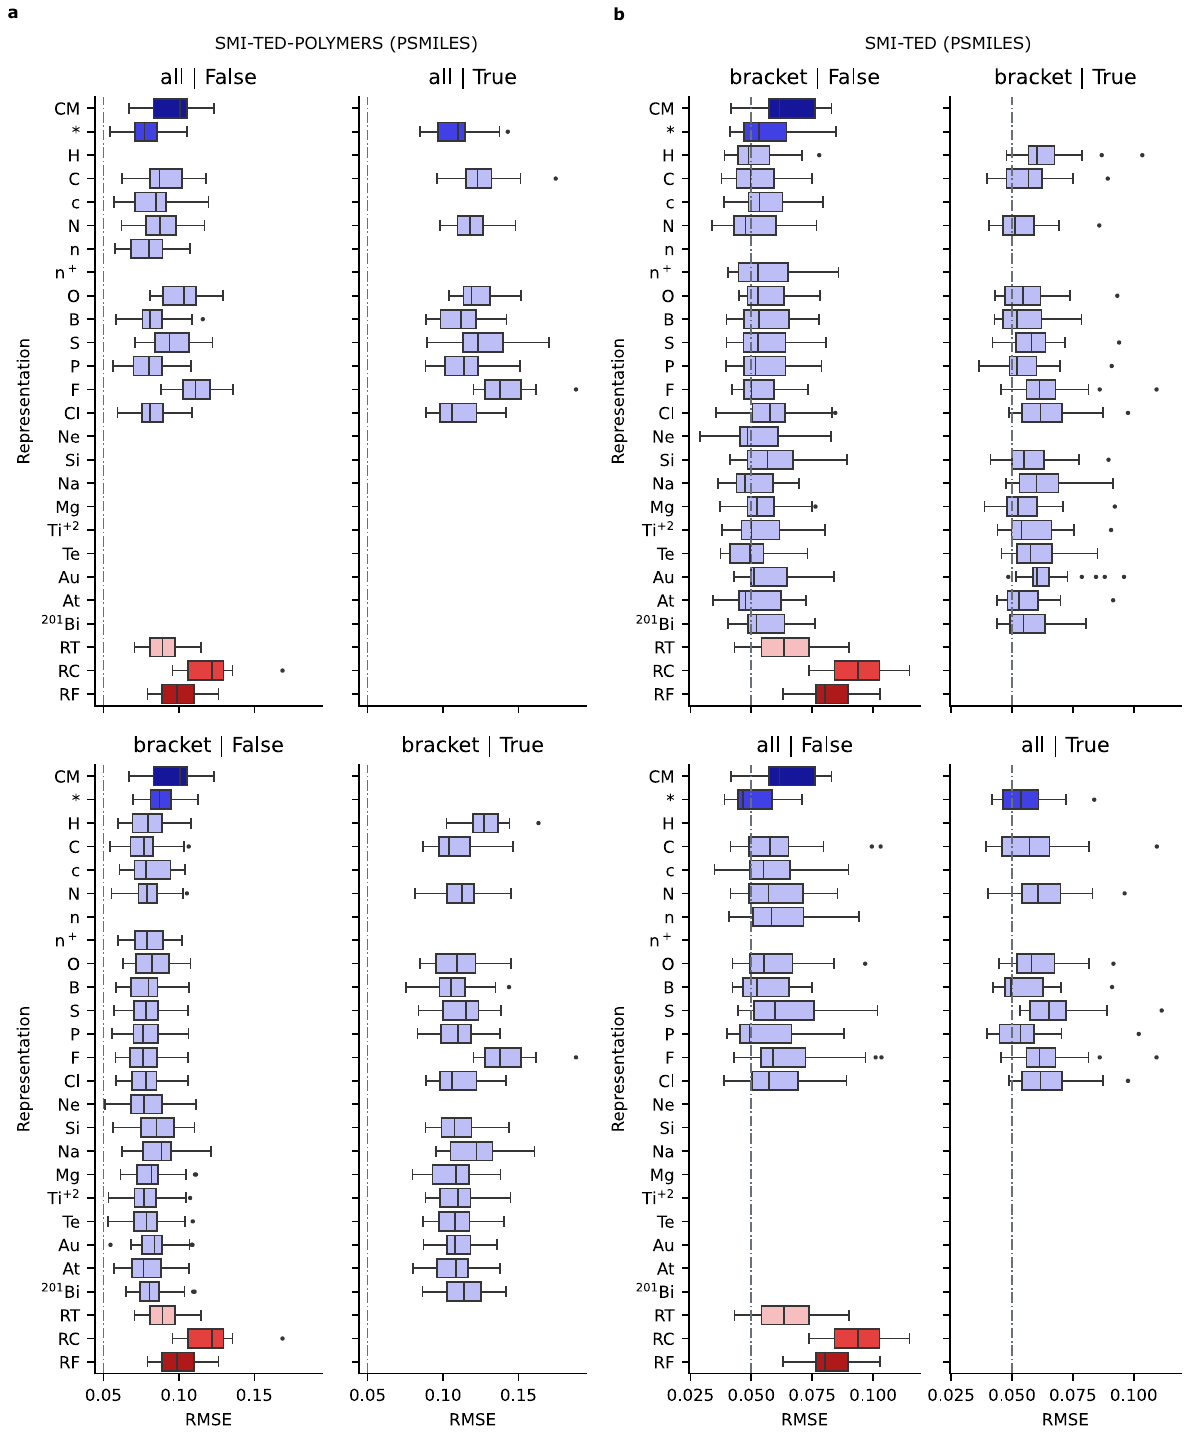}
\caption{Box plots for E\textsubscript{at} repeated cross-validation experiments for SMI-TED-POLYMER (\textbf{a}) and SMI-TED (\textbf{b}) models fine-tuned with PSMILES.}\label{eat_token_box_psmiles}
\end{figure}

\subsubsection{Polymer Atomization Energy (E\textsubscript{at}) Random Split Scores}\label{randEat}

\begin{figure}[H]
\centering
\includegraphics[width=1\textwidth]{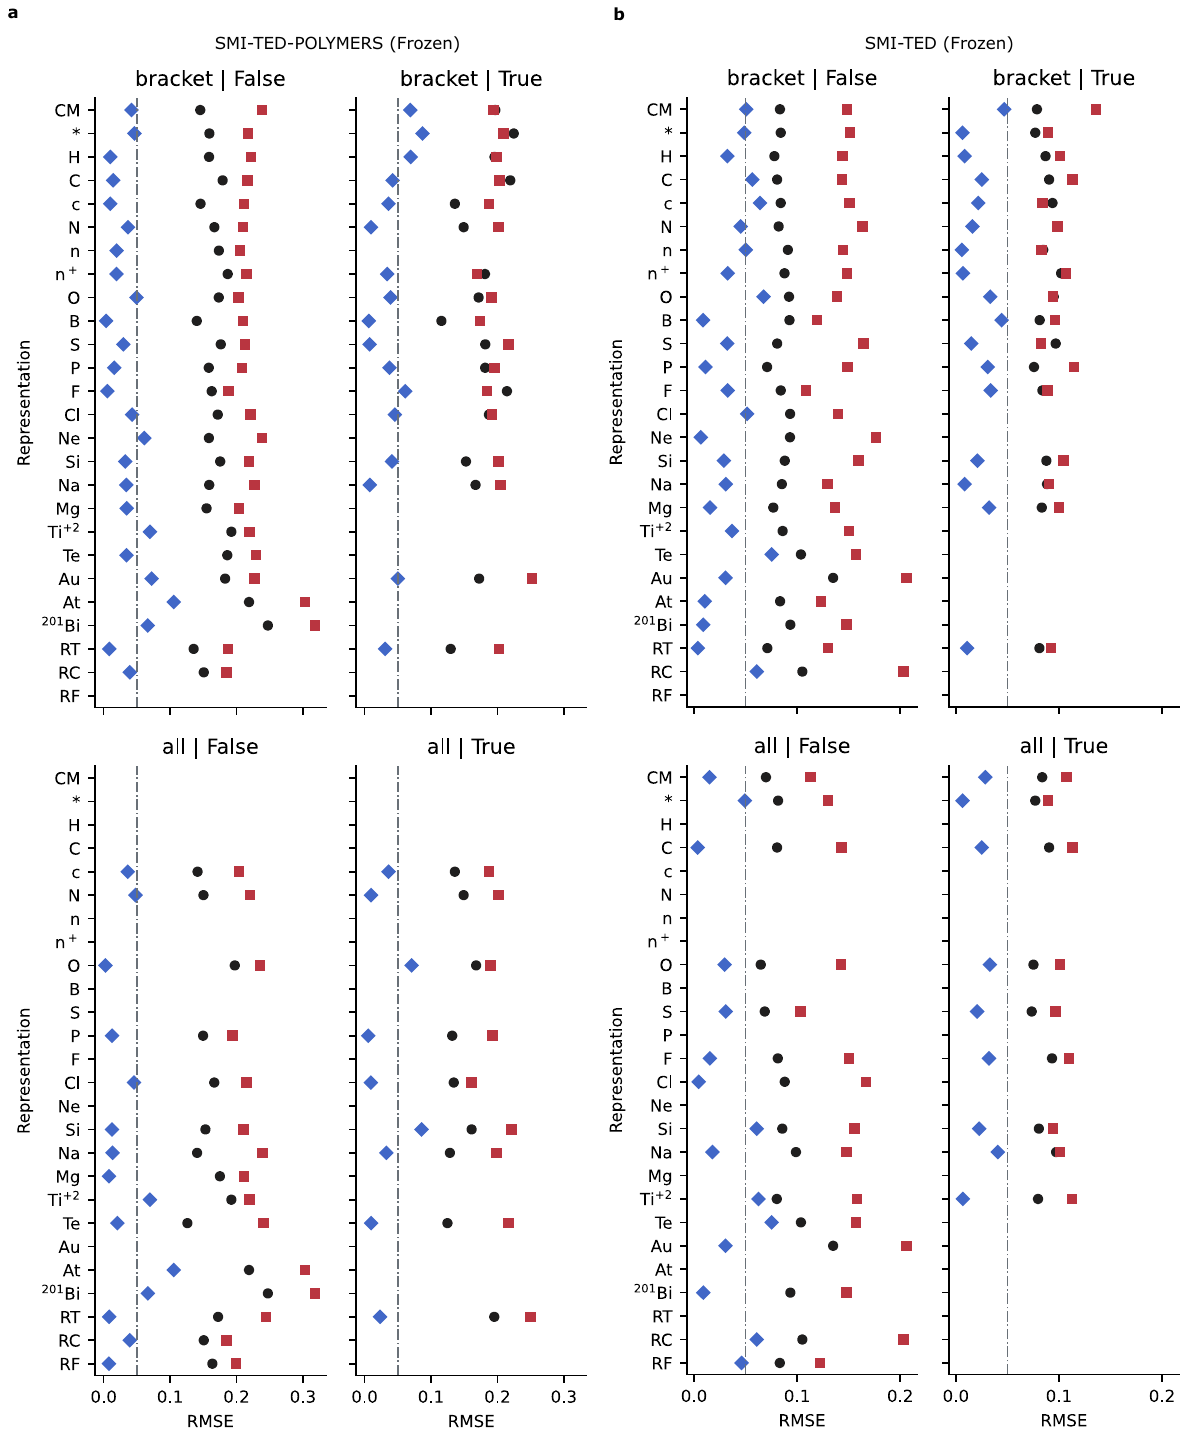}
\caption{Point plots for E\textsubscript{at} benchmark experiments of RMSE using the base random train, valid, and test splits for SMI-TED-POLYMER (\textbf{a}) and SMI-TED (\textbf{b}) models with frozen weights.}\label{eat_token_point_frozen_rmse}
\end{figure}

\begin{figure}[H]
\centering
\includegraphics[width=1\textwidth]{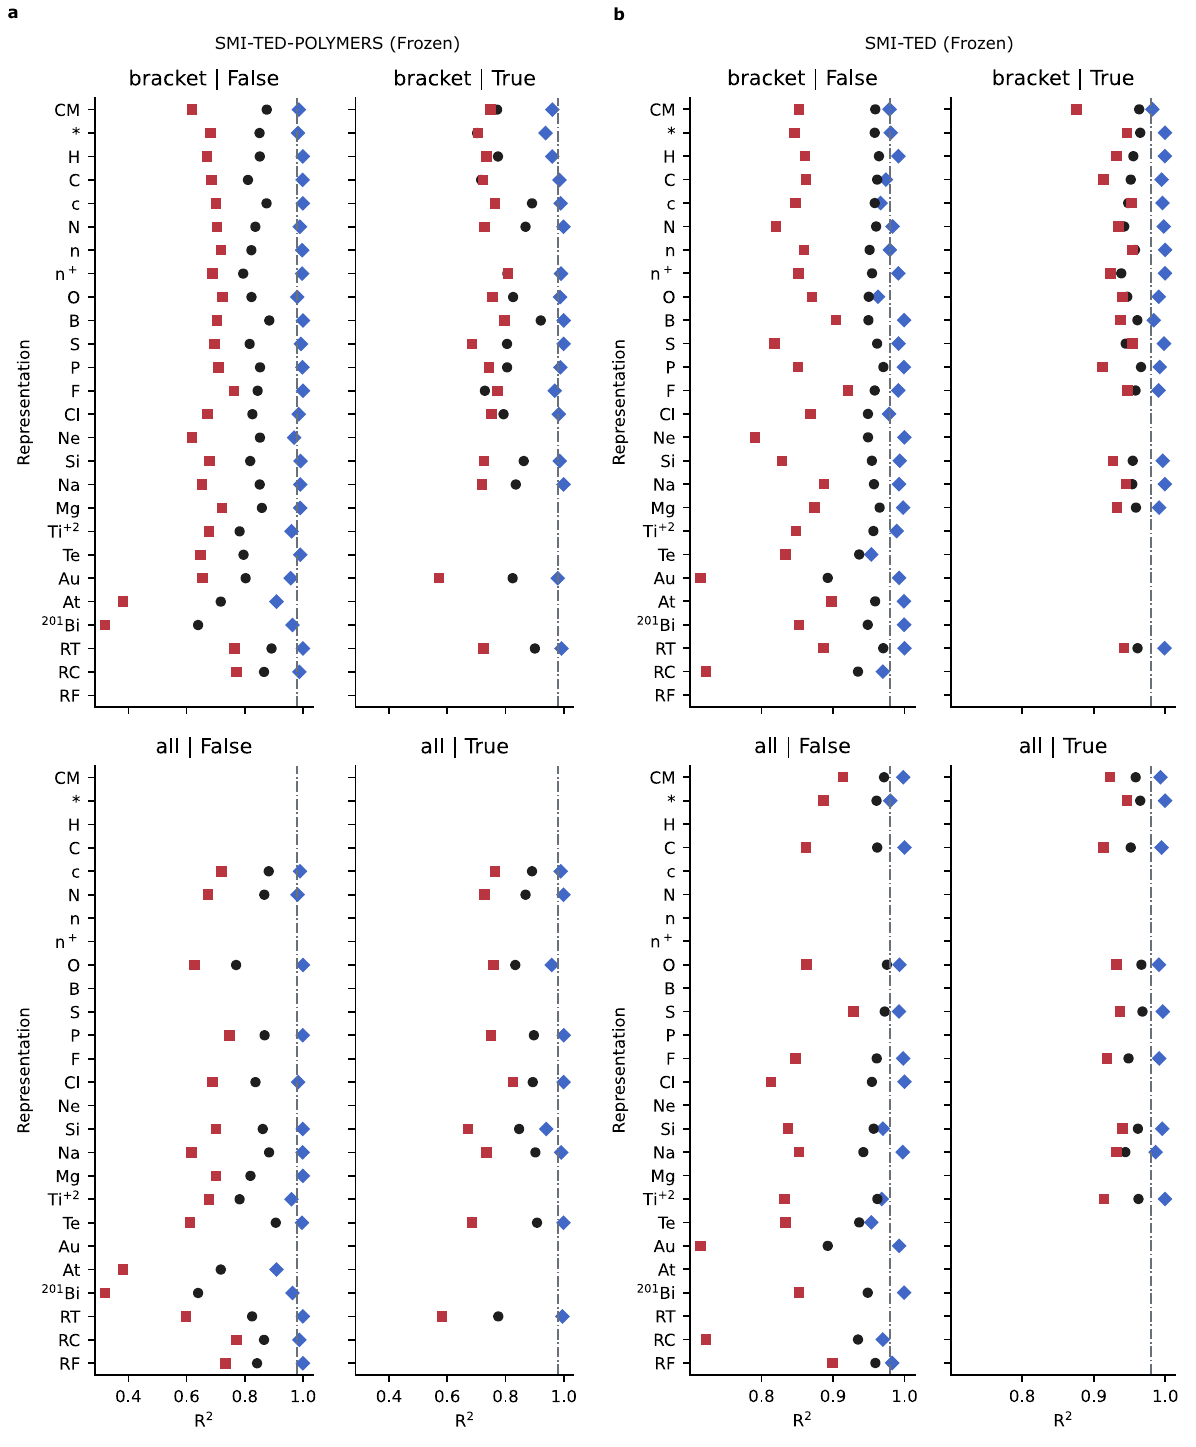}
\caption{Point plots for E\textsubscript{at} benchmark experiments of R\textsuperscript{2} using the base random train, valid, and test splits for SMI-TED-POLYMER (\textbf{a}) and SMI-TED (\textbf{b}) models with frozen weights.}\label{eat_token_point_frozen_r2}
\end{figure}

\begin{figure}[H]
\centering
\includegraphics[width=1\textwidth]{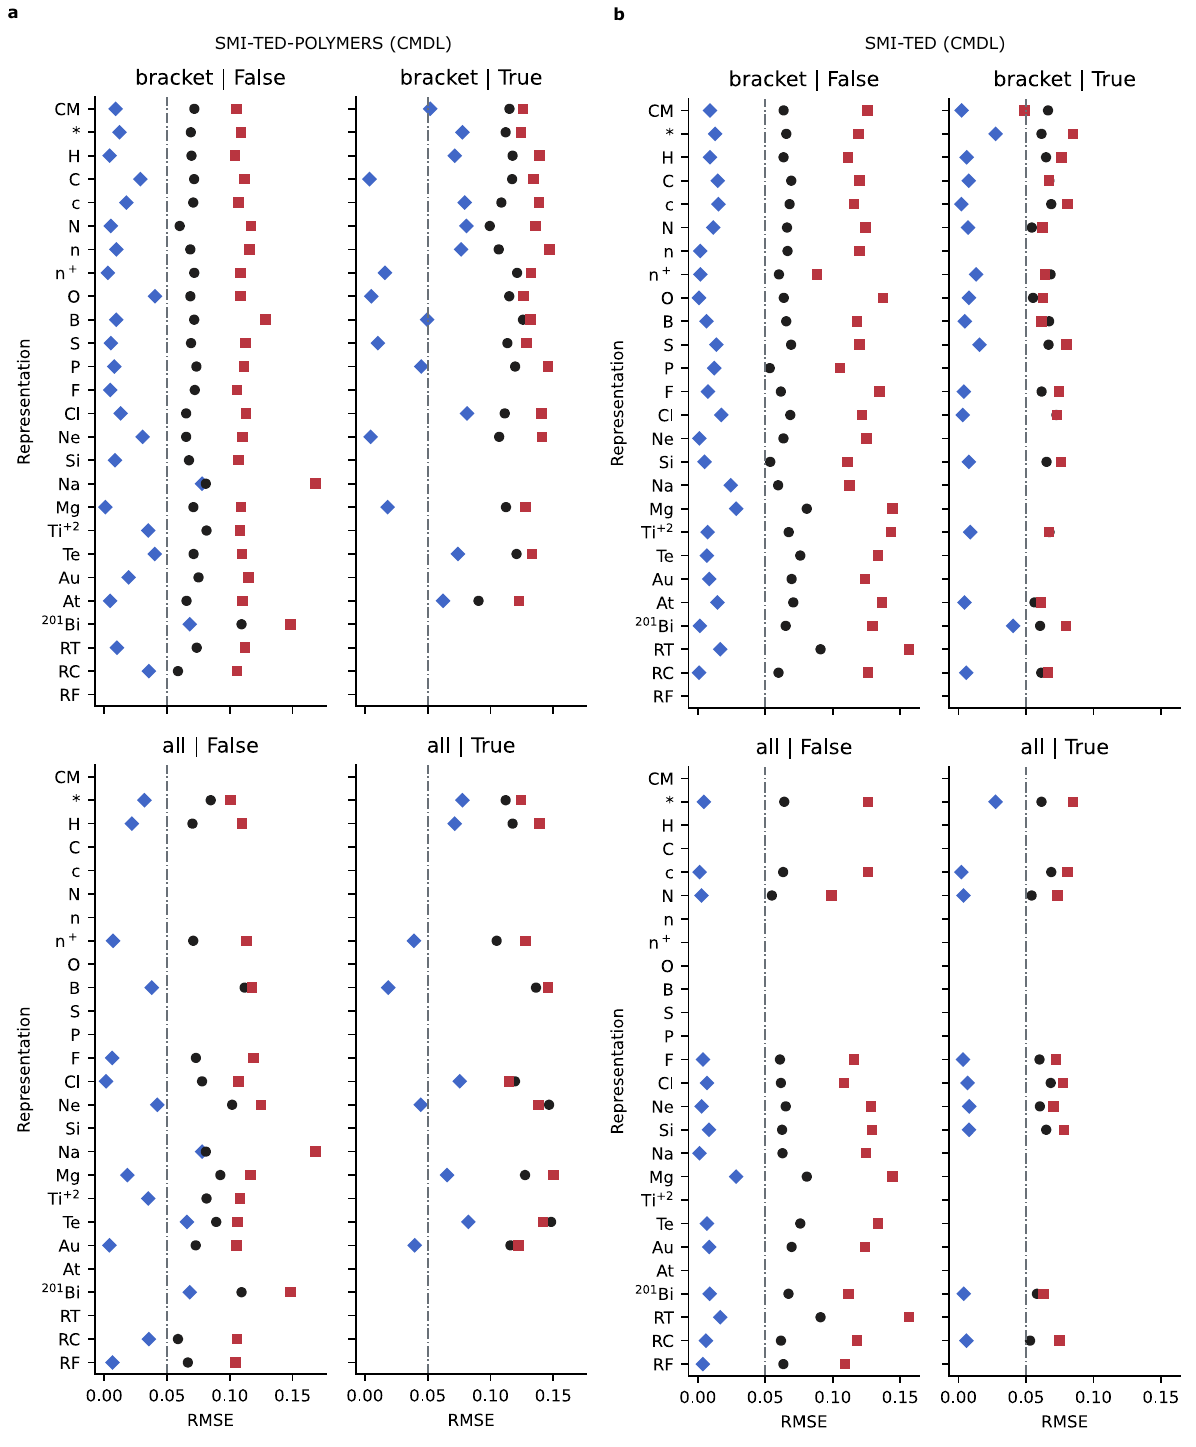}
\caption{Point plots for E\textsubscript{at} benchmark experiments of RMSE using the base random train, valid, and test splits for SMI-TED-POLYMER (\textbf{a}) and SMI-TED (\textbf{b}) models fine-tuned using the CPG representation.}\label{eat_token_point_cmdl_rmse}
\end{figure}

\begin{figure}
\centering
\includegraphics[width=1\textwidth]{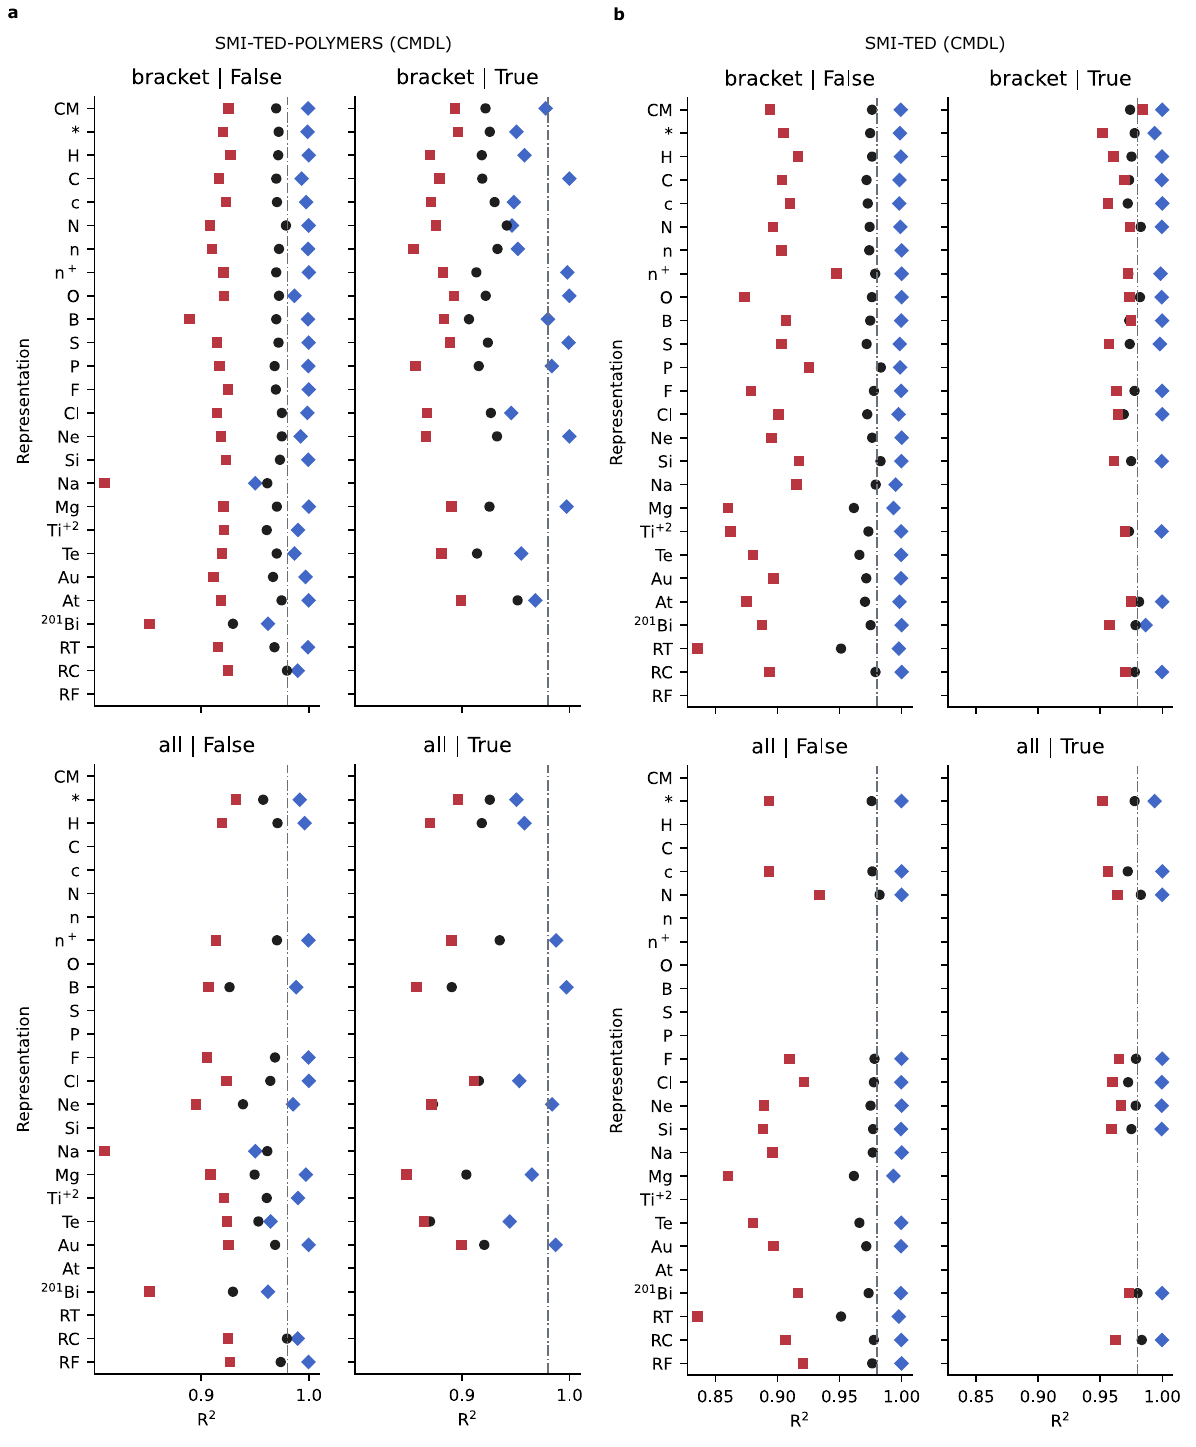}
\caption{Point plots for E\textsubscript{at} benchmark experiments of R\textsuperscript{2} using the base random train, valid, and test splits for SMI-TED-POLYMER (\textbf{a}) and SMI-TED (\textbf{b}) models fine-tuned using the CPG representation.}\label{eat_token_point_cmdl_r2}
\end{figure}

\begin{figure}[H]
\centering
\includegraphics[width=1\textwidth]{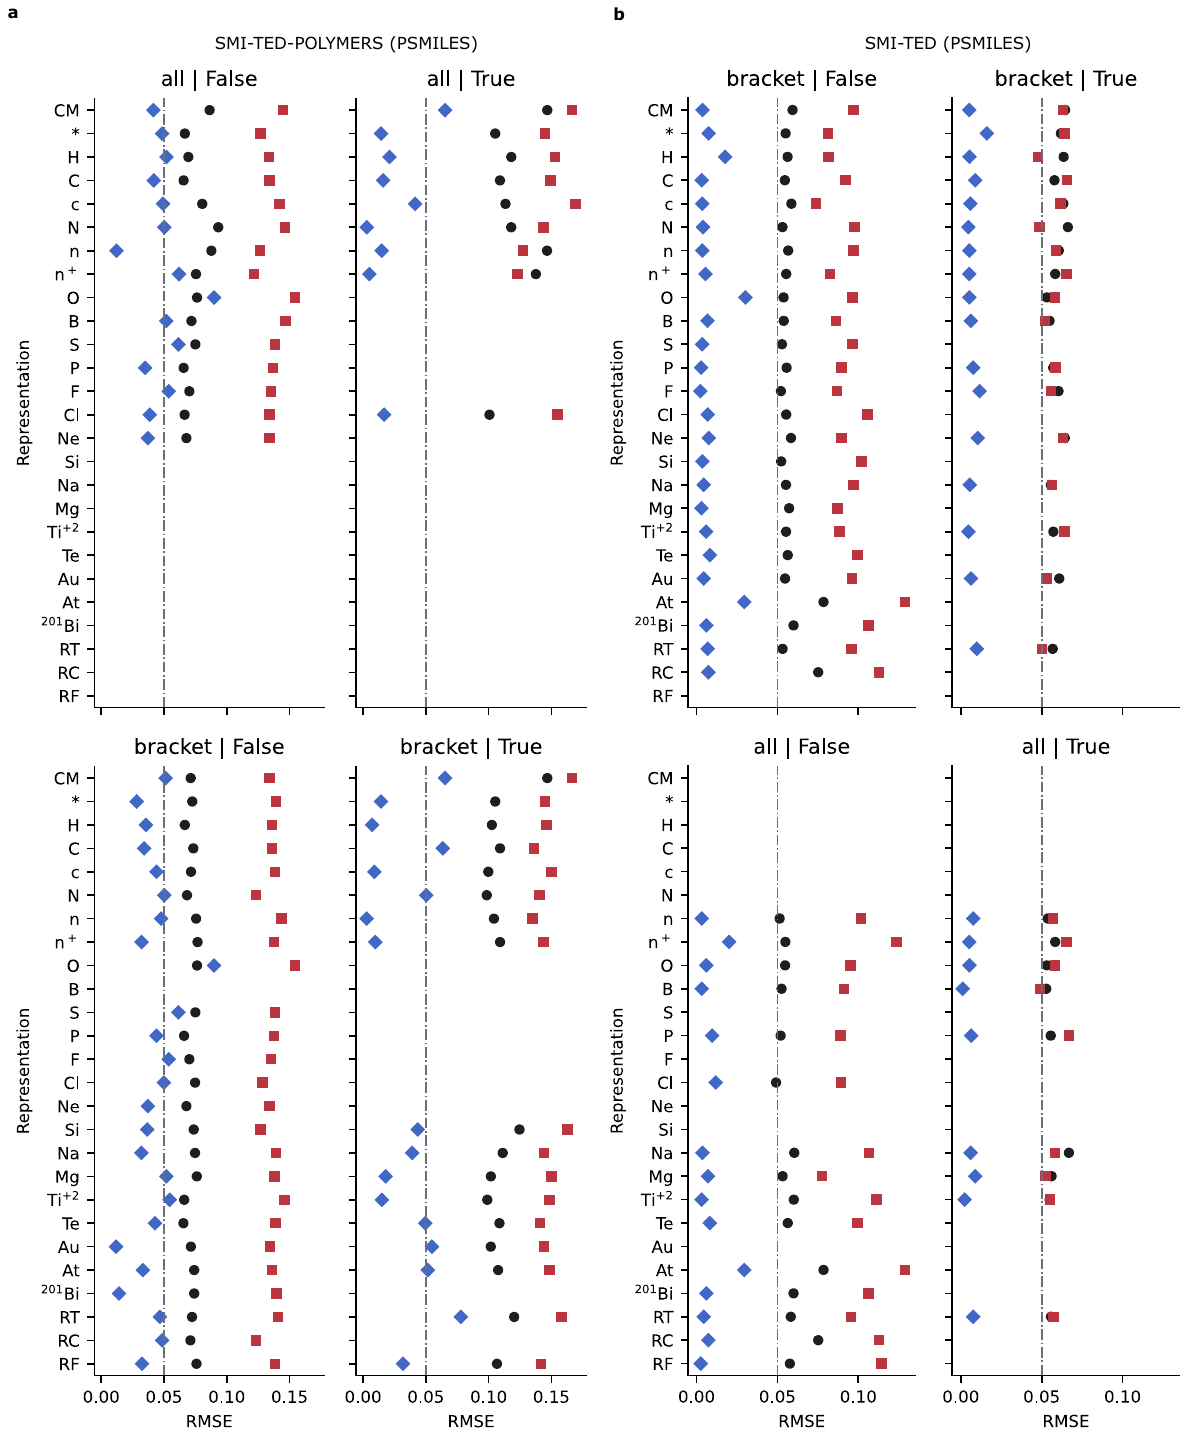}
\caption{Point plots for E\textsubscript{at} benchmark experiments of RMSE using the base random train, valid, and test splits for SMI-TED-POLYMER (\textbf{a}) and SMI-TED (\textbf{b}) models fine-tuned using PSMILES.}\label{eat_token_point_psmiles_rmse}
\end{figure}

\begin{figure}[H]
\centering
\includegraphics[width=1\textwidth]{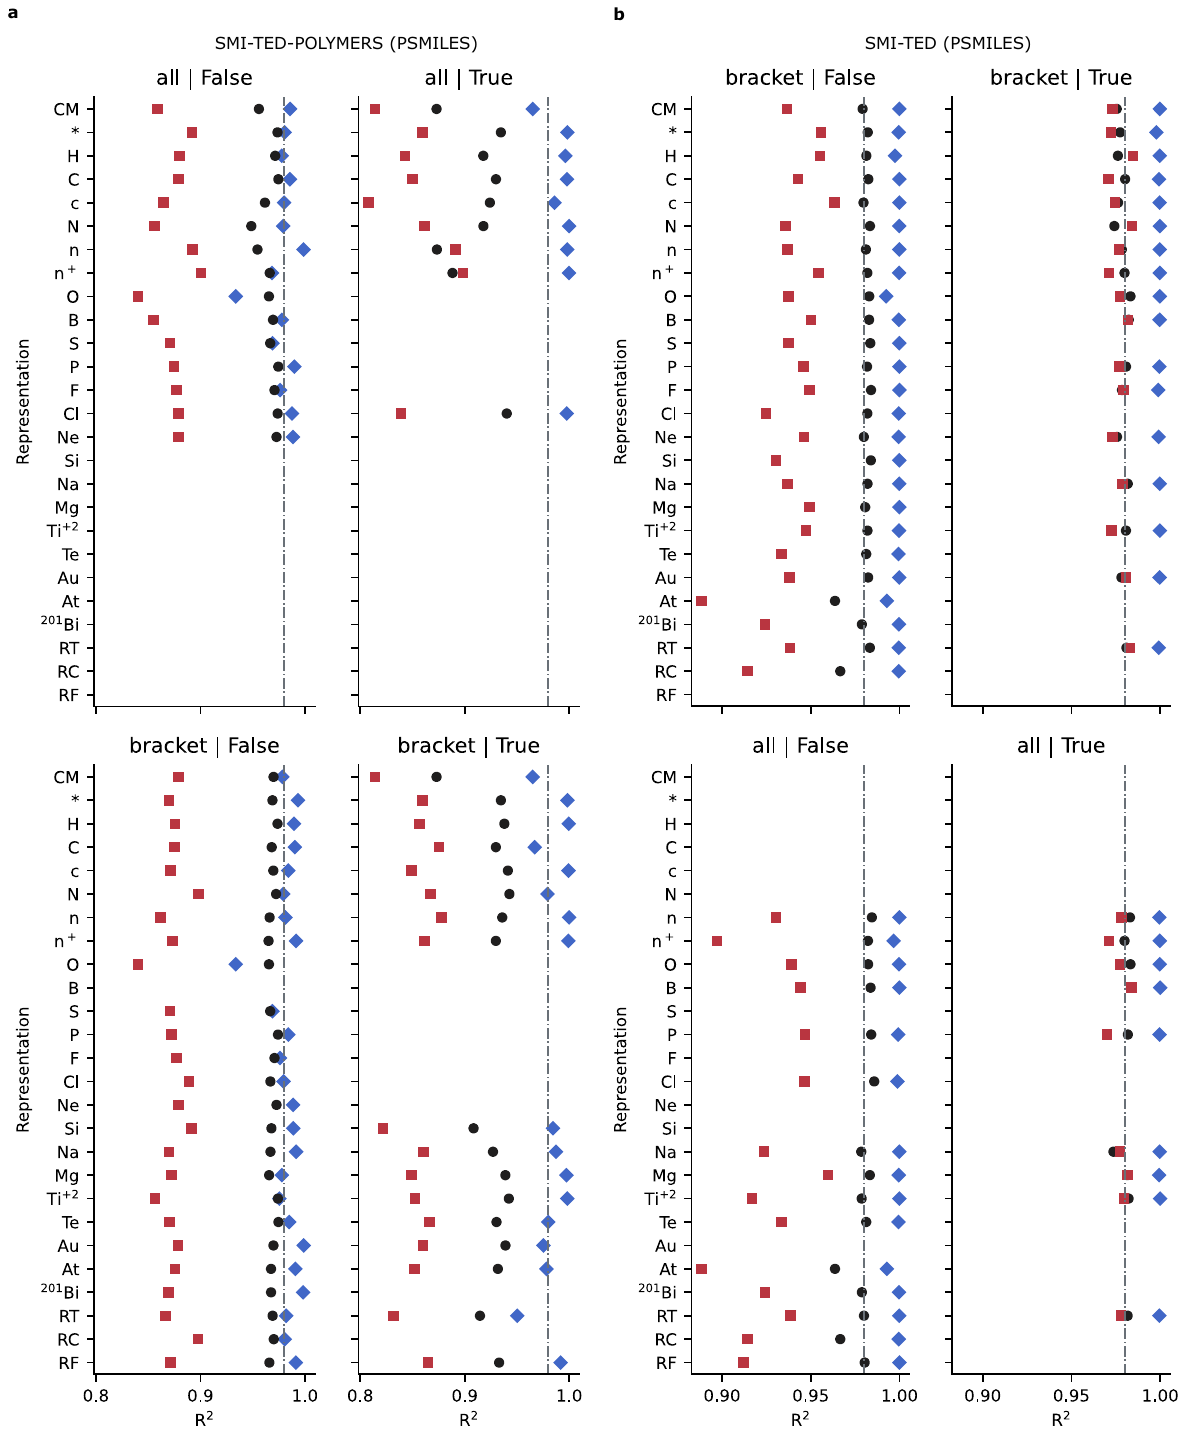}
\caption{Point plots for E\textsubscript{i} benchmark experiments of R\textsuperscript{2} using the base random train, valid, and test splits for SMI-TED-POLYMER (\textbf{a}) and SMI-TED (\textbf{b}) models fine-tuned using PSMILES.}\label{eat_token_point_psmiles_r2}
\end{figure}

\subsubsection{Refractivity Index (N\textsubscript{c}) CV Scores}\label{cvNc}

\begin{figure}[H]
\centering
\includegraphics[width=1\textwidth]{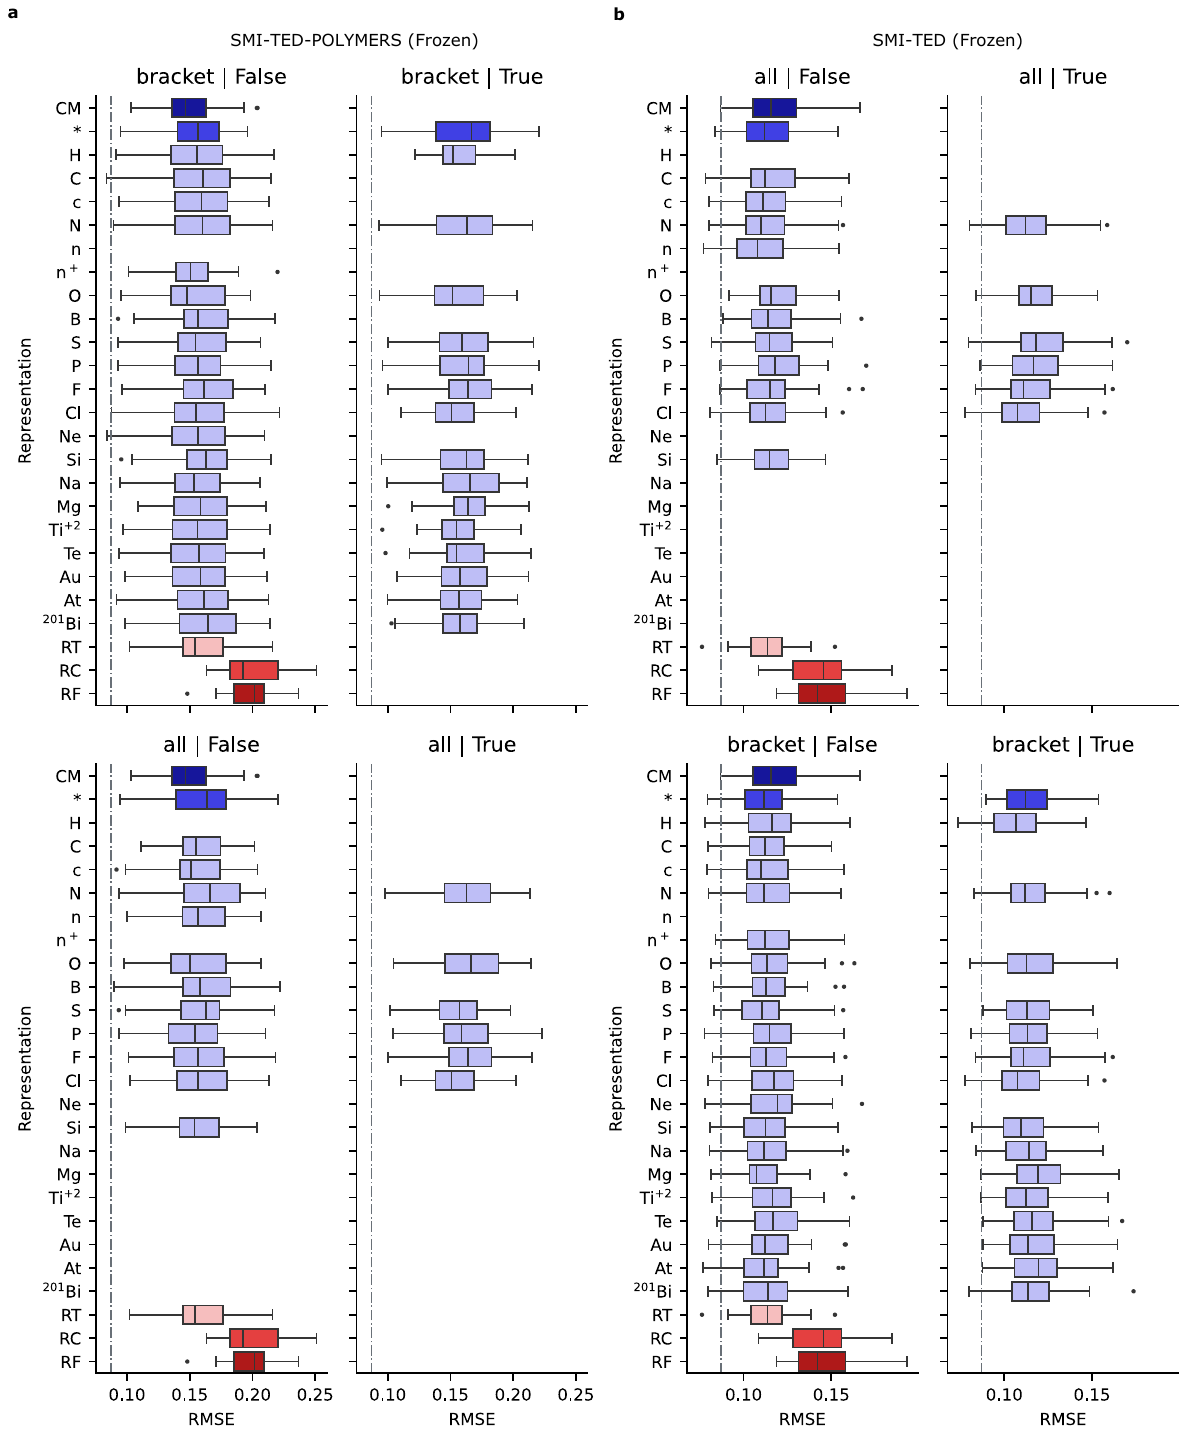}
\caption{Box plots for N\textsubscript{c} repeated cross-validation experiments for SMI-TED-POLYMER (\textbf{a}) and SMI-TED (\textbf{b}) models with frozen weights.}\label{nc_token_box_frozen}
\end{figure}

\begin{figure}[H]
\centering
\includegraphics[width=1\textwidth]{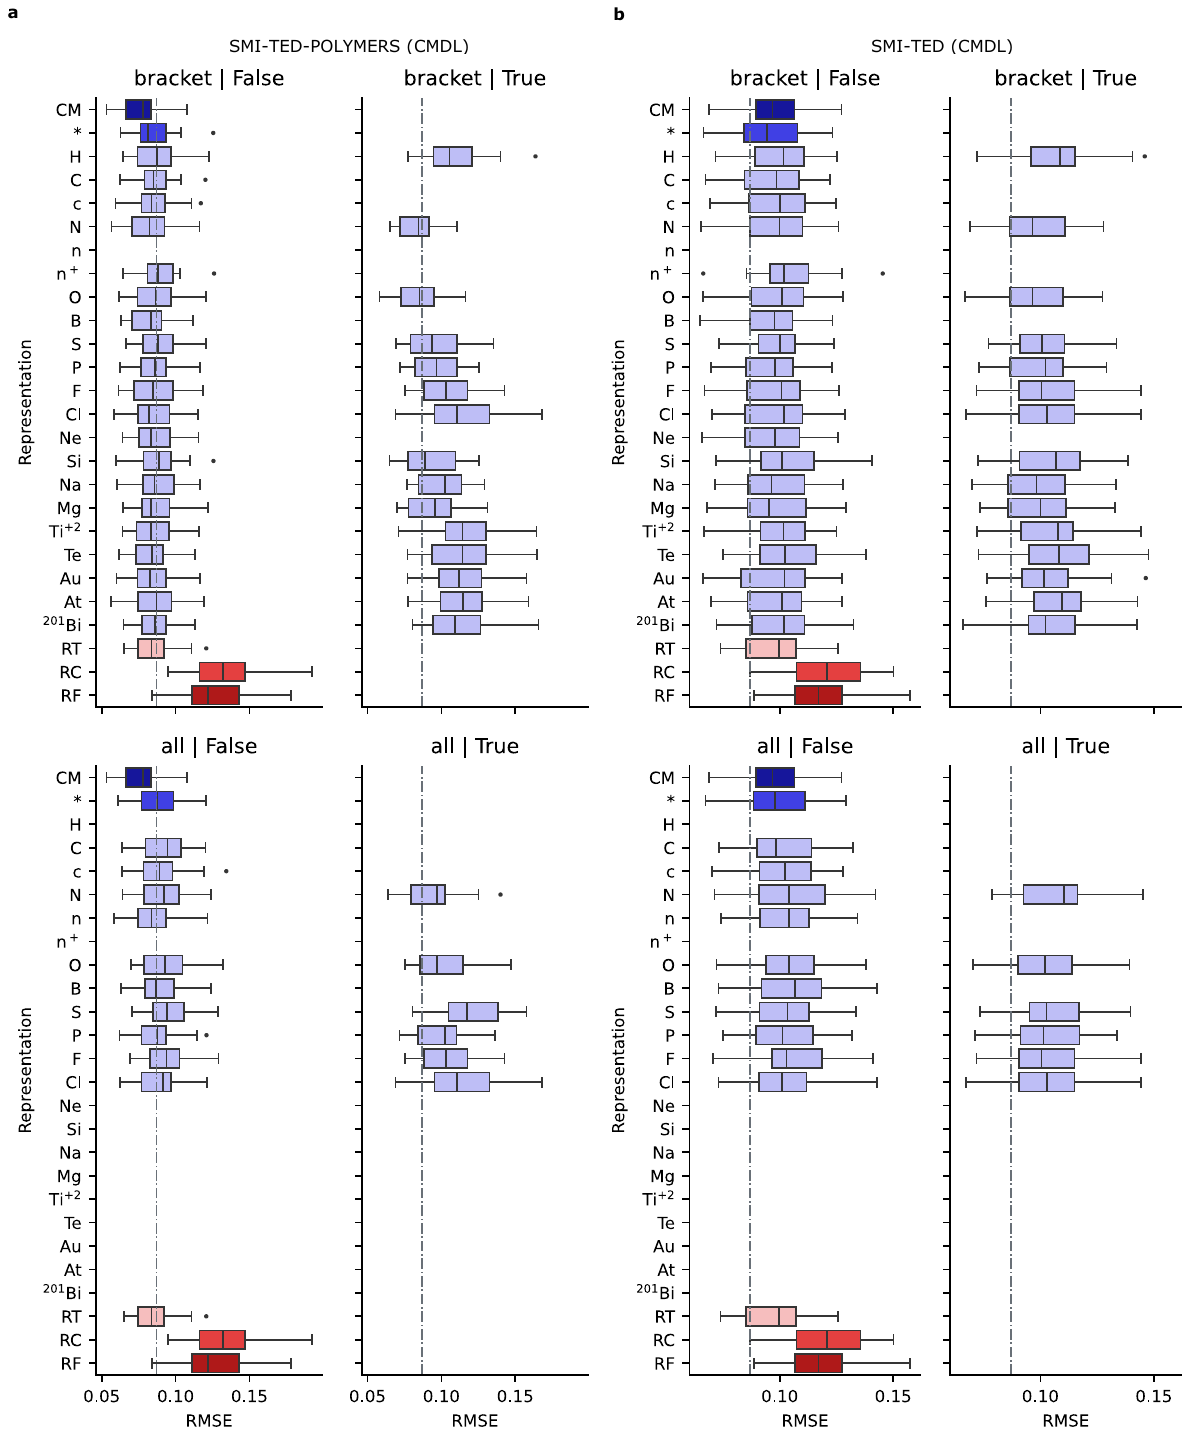}
\caption{Box plots for N\textsubscript{c} repeated cross-validation experiments for SMI-TED-POLYMER (\textbf{a}) and SMI-TED (\textbf{b}) models fine-tuned with the CPG polymer graphs.}\label{nc_token_box_cmdl}
\end{figure}

\begin{figure}[H]
\centering
\includegraphics[width=1\textwidth]{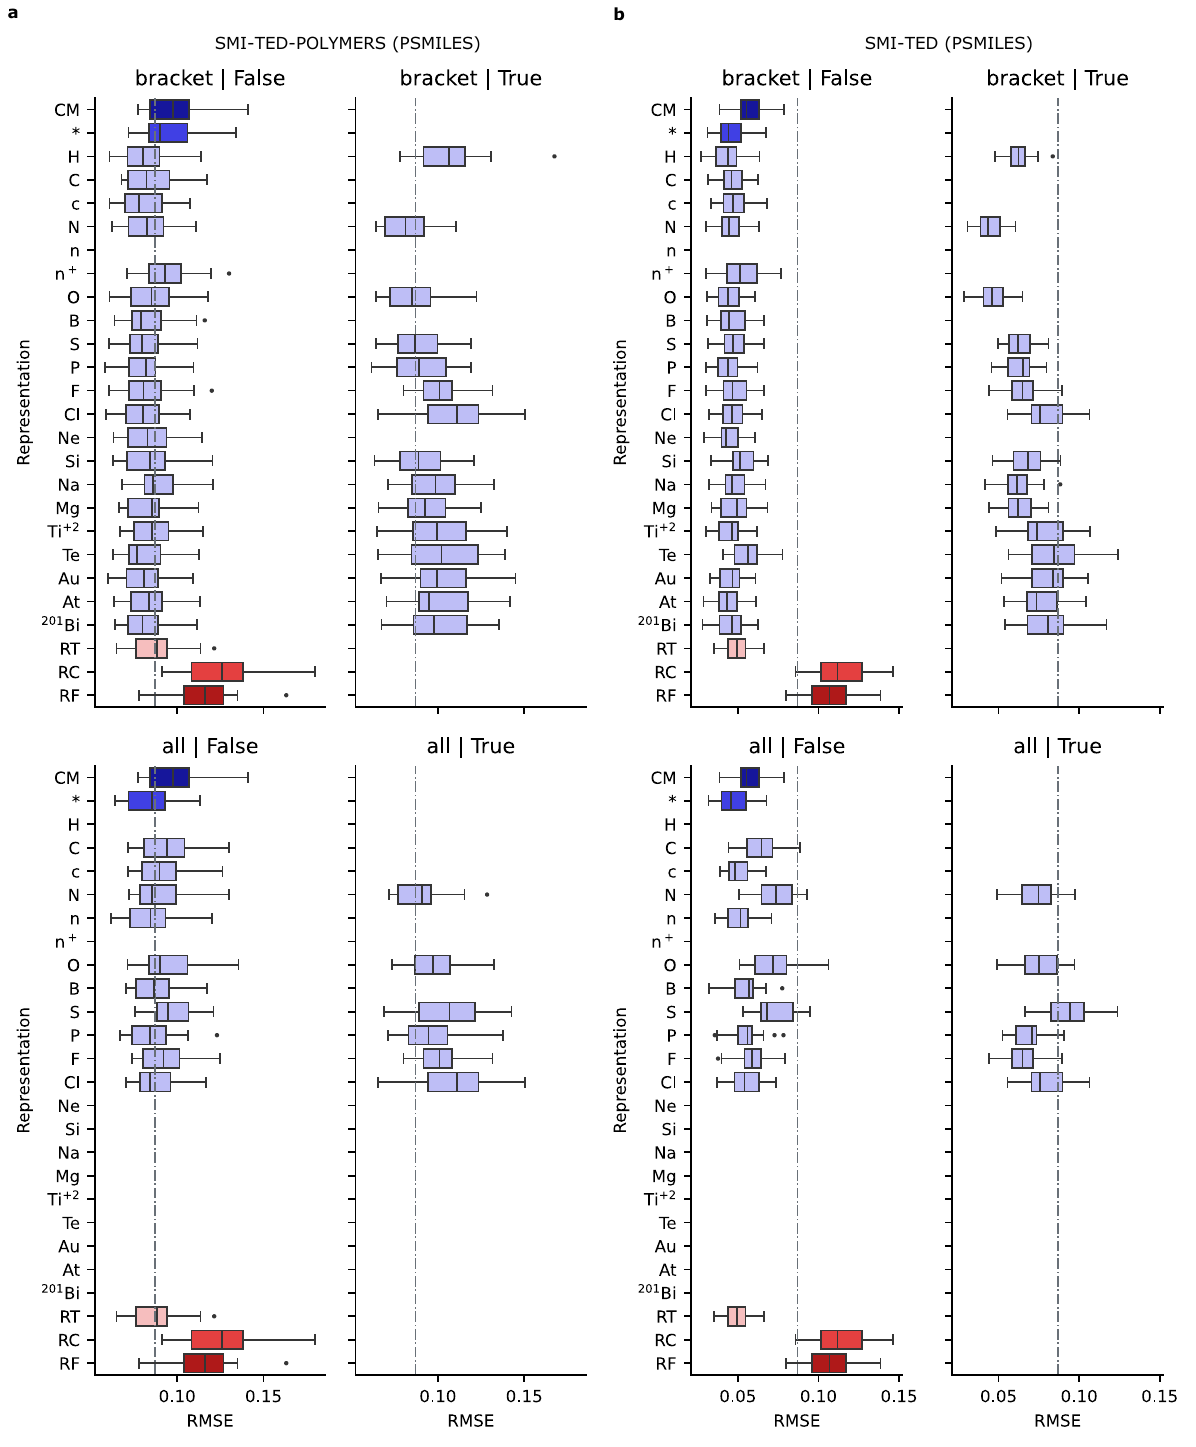}
\caption{Box plots for N\textsubscript{c} repeated cross-validation experiments for SMI-TED-POLYMER (\textbf{a}) and SMI-TED (\textbf{b}) models fine-tuned with PSMILES.}\label{nc_token_box_psmiles}
\end{figure}

\subsubsection{Refractivity Index (N\textsubscript{c}) Random Split Scores}\label{randNc}

\begin{figure}[H]
\centering
\includegraphics[width=1\textwidth]{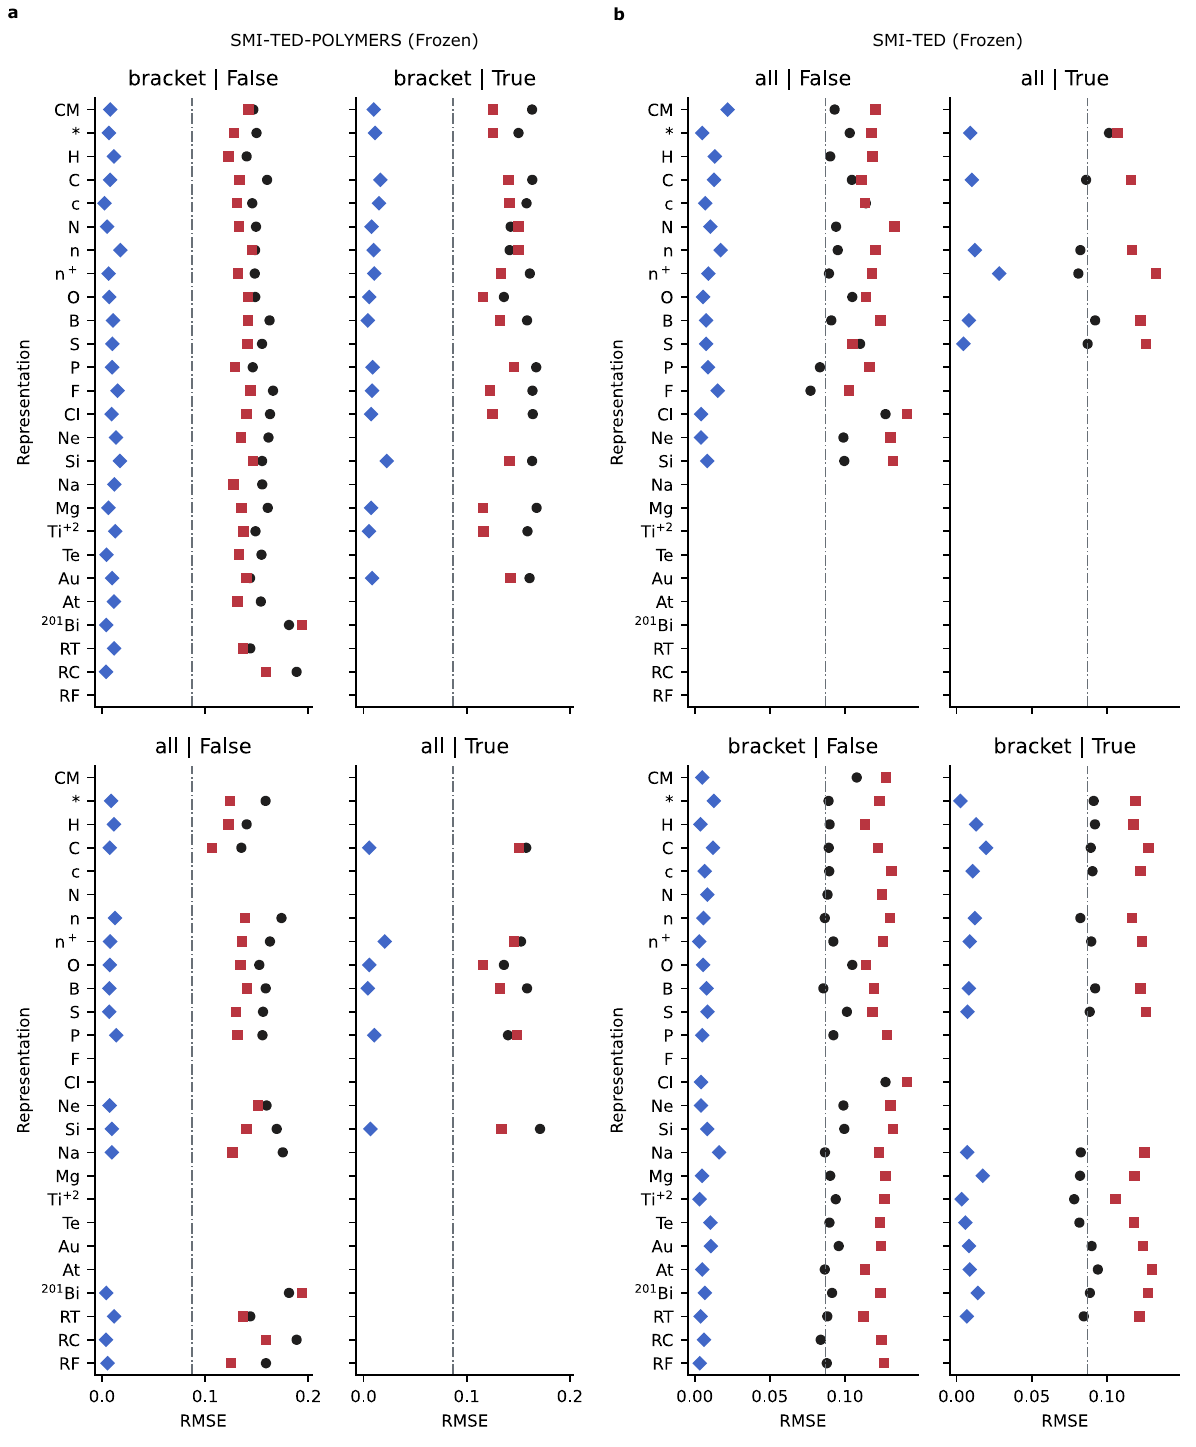}
\caption{Point plots for N\textsubscript{c} benchmark experiments of RMSE using the base random train, valid, and test splits for SMI-TED-POLYMER (\textbf{a}) and SMI-TED (\textbf{b}) models with frozen weights.}\label{nc_token_point_frozen_rmse}
\end{figure}

\begin{figure}[H]
\centering
\includegraphics[width=1\textwidth]{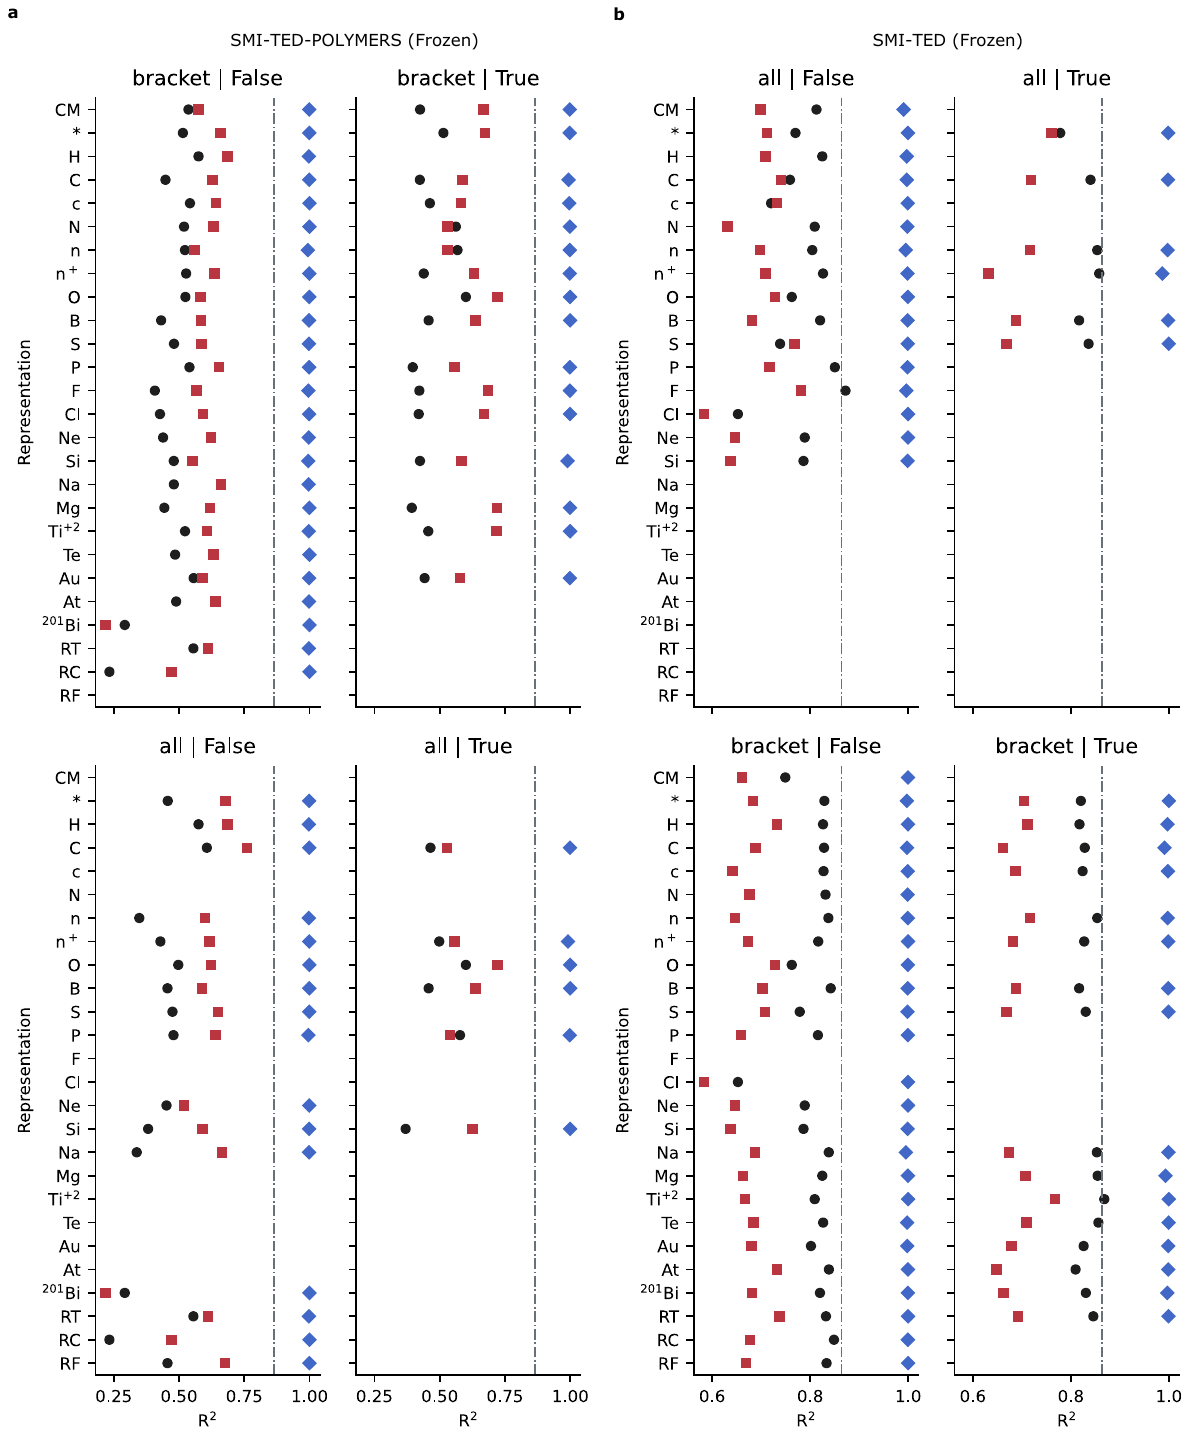}
\caption{Point plots for N\textsubscript{c} benchmark experiments of R\textsuperscript{2} using the base random train, valid, and test splits for SMI-TED-POLYMER (\textbf{a}) and SMI-TED (\textbf{b}) models with frozen weights.}\label{nc_token_point_frozen_r2}
\end{figure}

\begin{figure}[H]
\centering
\includegraphics[width=1\textwidth]{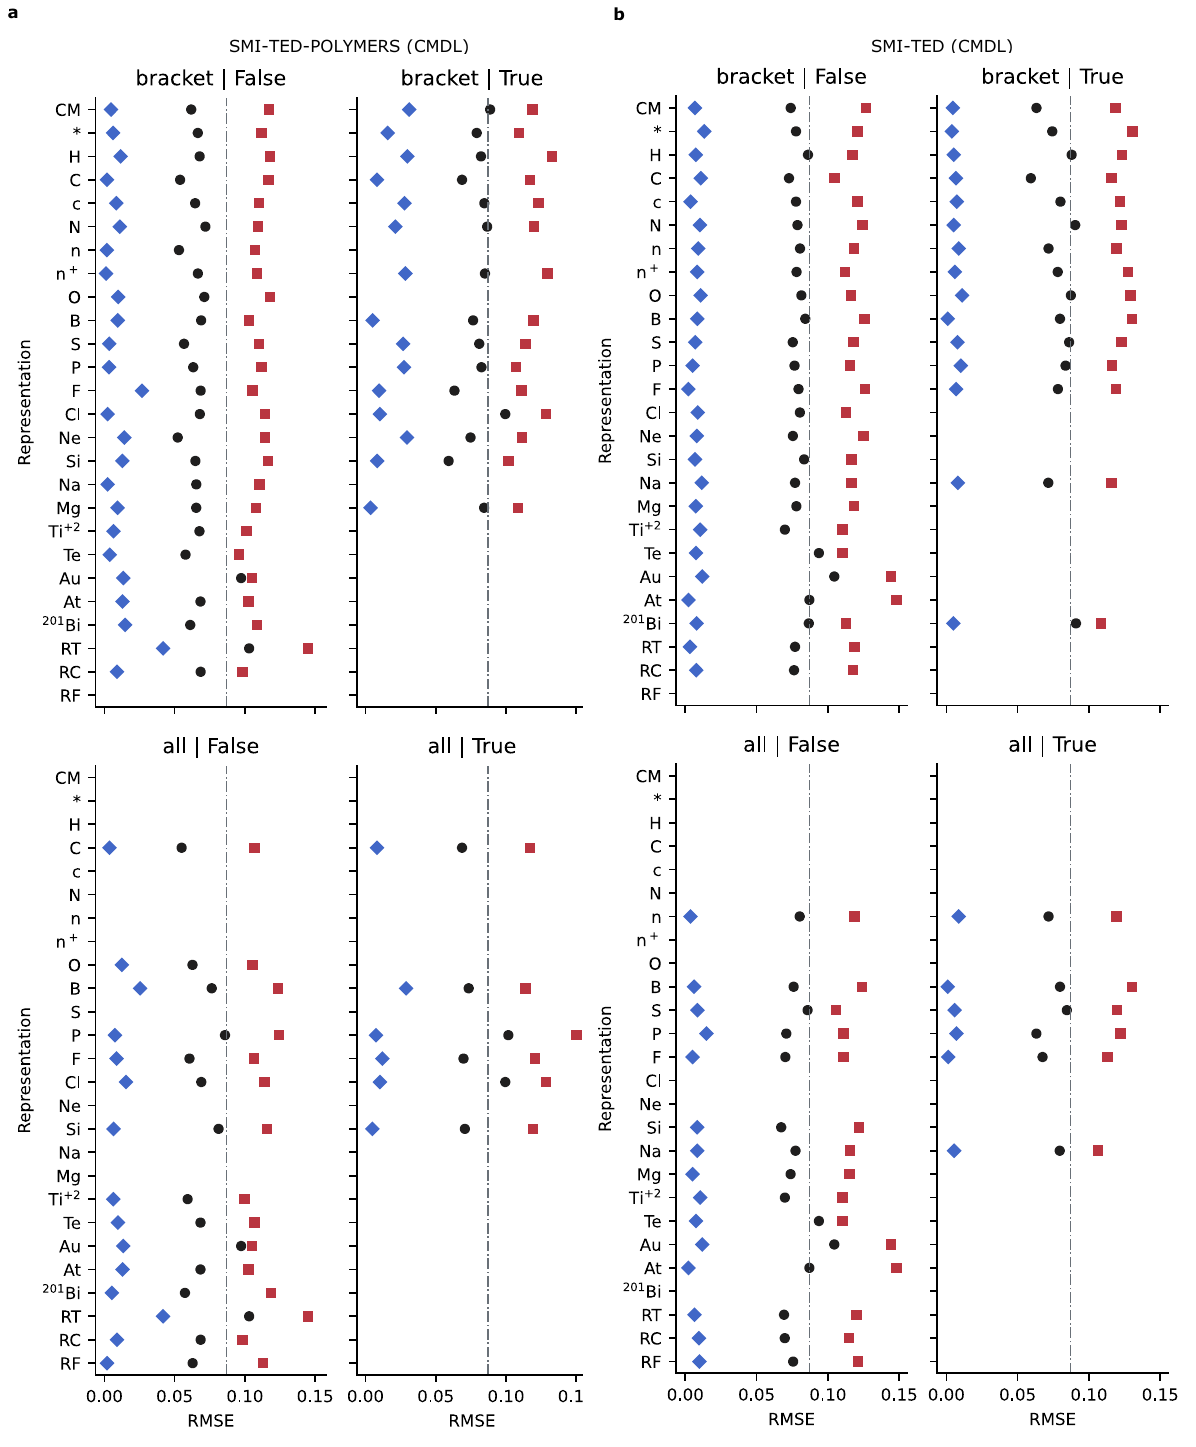}
\caption{Point plots for N\textsubscript{c} benchmark experiments of RMSE using the base random train, valid, and test splits for SMI-TED-POLYMER (\textbf{a}) and SMI-TED (\textbf{b}) models fine-tuned with CPG.}\label{nc_token_point_cmdl_rmse}
\end{figure}

\begin{figure}[H]
\centering
\includegraphics[width=1\textwidth]{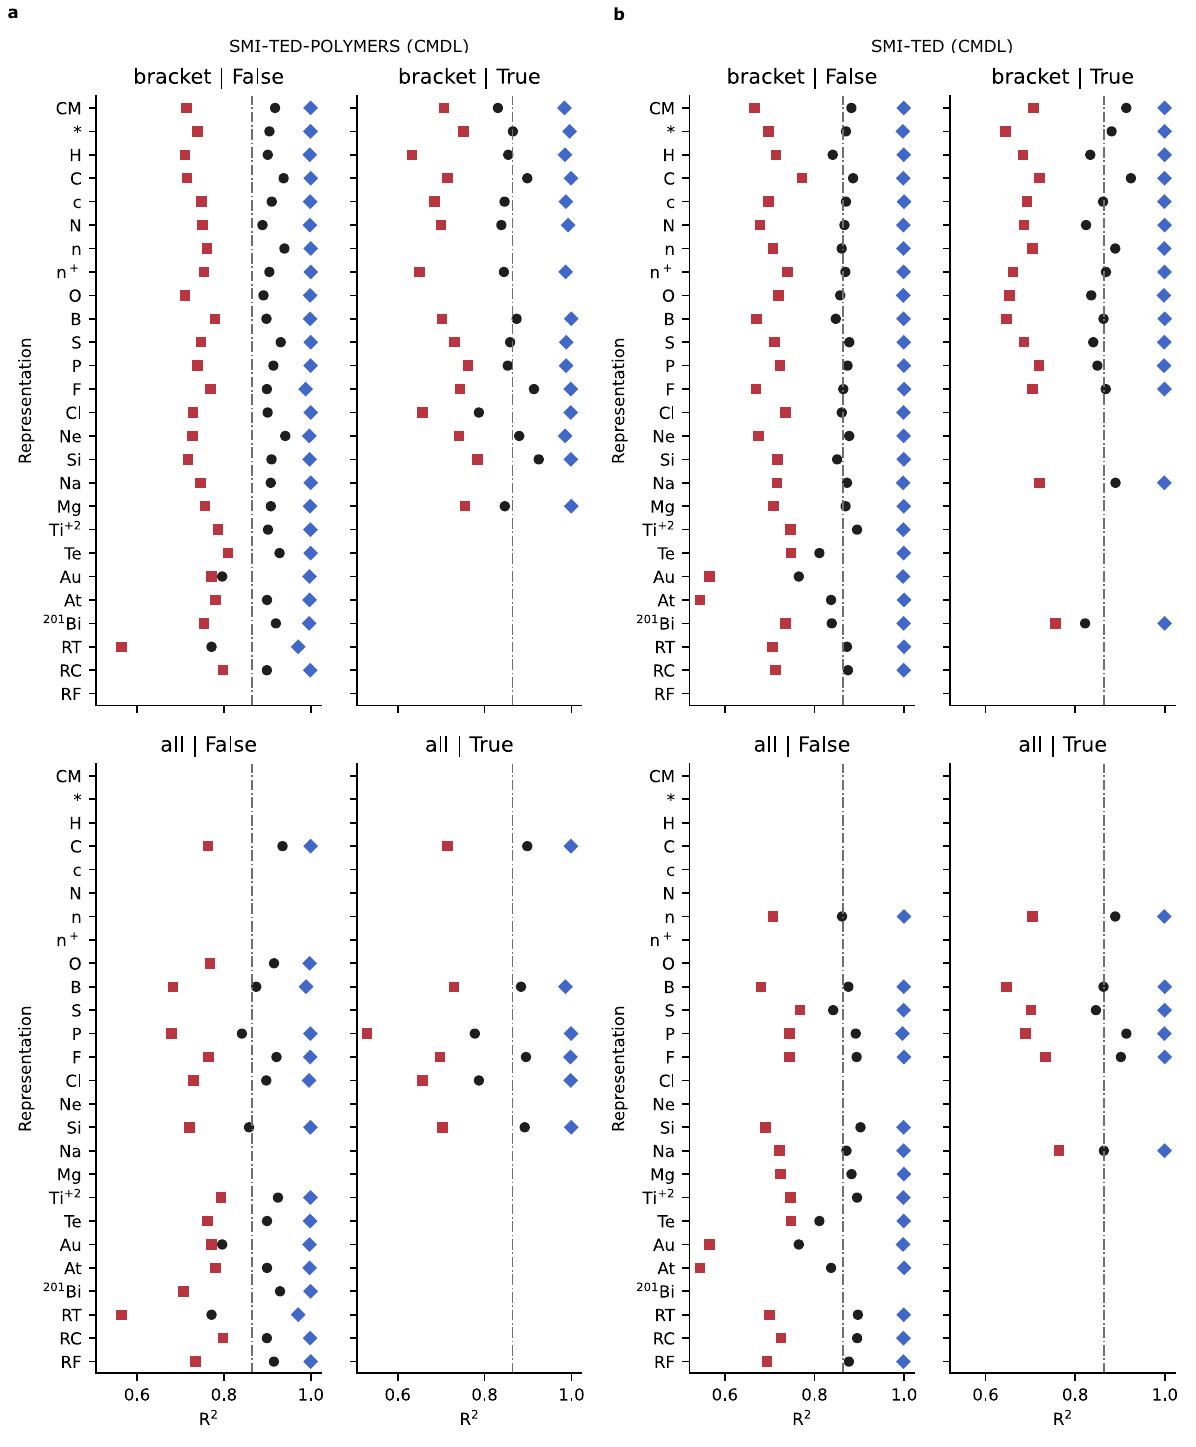}
\caption{Point plots for N\textsubscript{c} benchmark experiments of R\textsuperscript{2} using the base random train, valid, and test splits for SMI-TED-POLYMER (\textbf{a}) and SMI-TED (\textbf{b}) models fine-tuned with CPG.}\label{nc_token_point_cmdl_r2}
\end{figure}

\begin{figure}[H]
\centering
\includegraphics[width=1\textwidth]{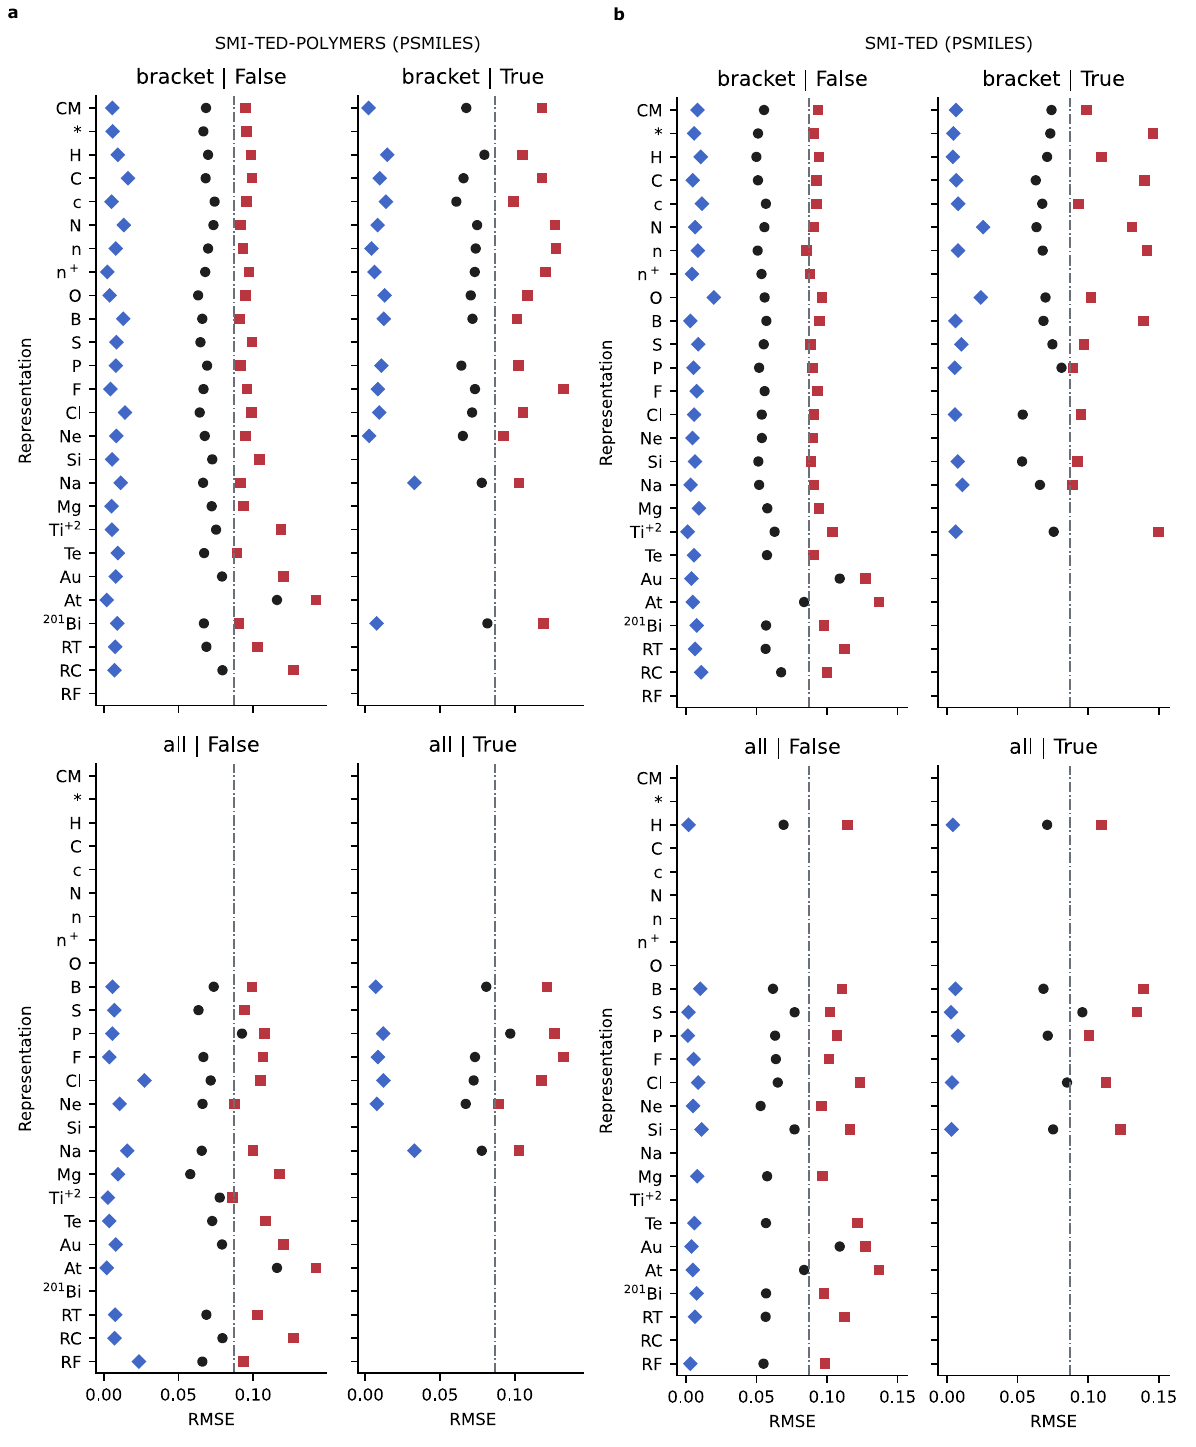}
\caption{Point plots for N\textsubscript{c} benchmark experiments of RMSE using the base random train, valid, and test splits for SMI-TED-POLYMER (\textbf{a}) and SMI-TED (\textbf{b}) models fine-tuned with PSMILES.}\label{nc_token_point_psmiles_rmse}
\end{figure}

\begin{figure}[H]
\centering
\includegraphics[width=1\textwidth]{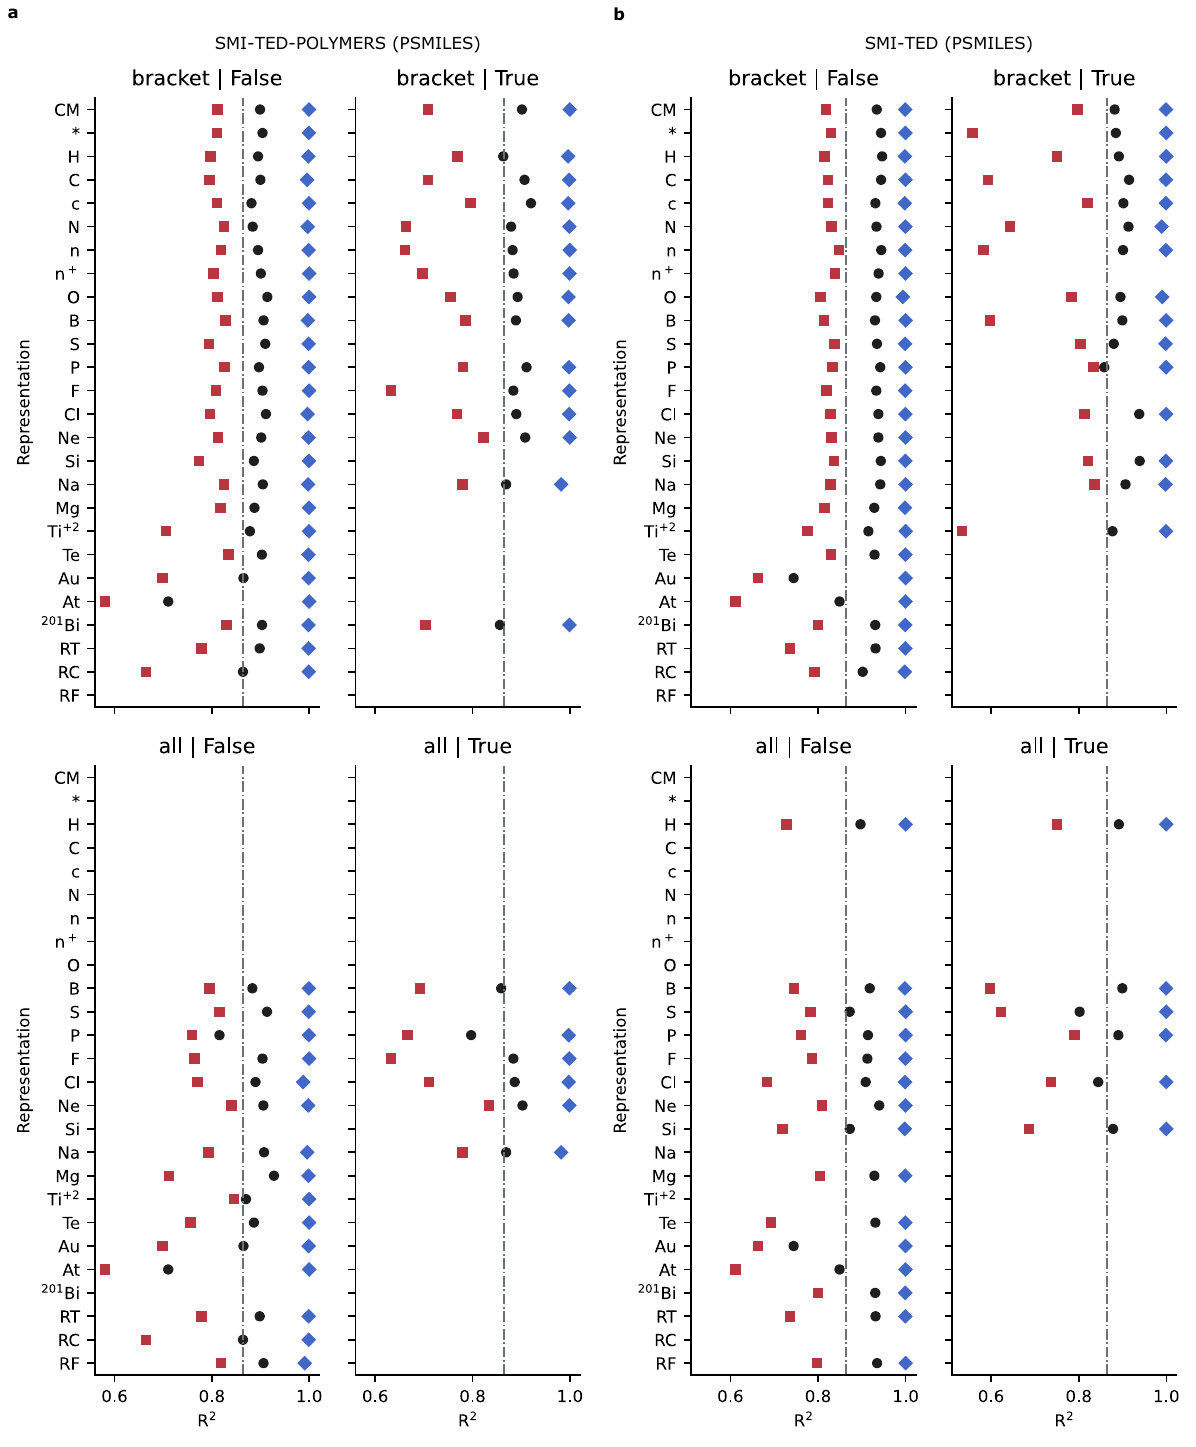}
\caption{Point plots for N\textsubscript{c} benchmark experiments of R\textsuperscript{2} using the base random train, valid, and test splits for SMI-TED-POLYMER (\textbf{a}) and SMI-TED (\textbf{b}) models fine-tuned with PSMILES.}\label{nc_token_point_psmiles_r2}
\end{figure}

\subsubsection{Crystallization Tendency (X\textsubscript{c}) CV Scores}\label{cvXc}

\begin{figure}[H]
\centering
\includegraphics[width=1\textwidth]{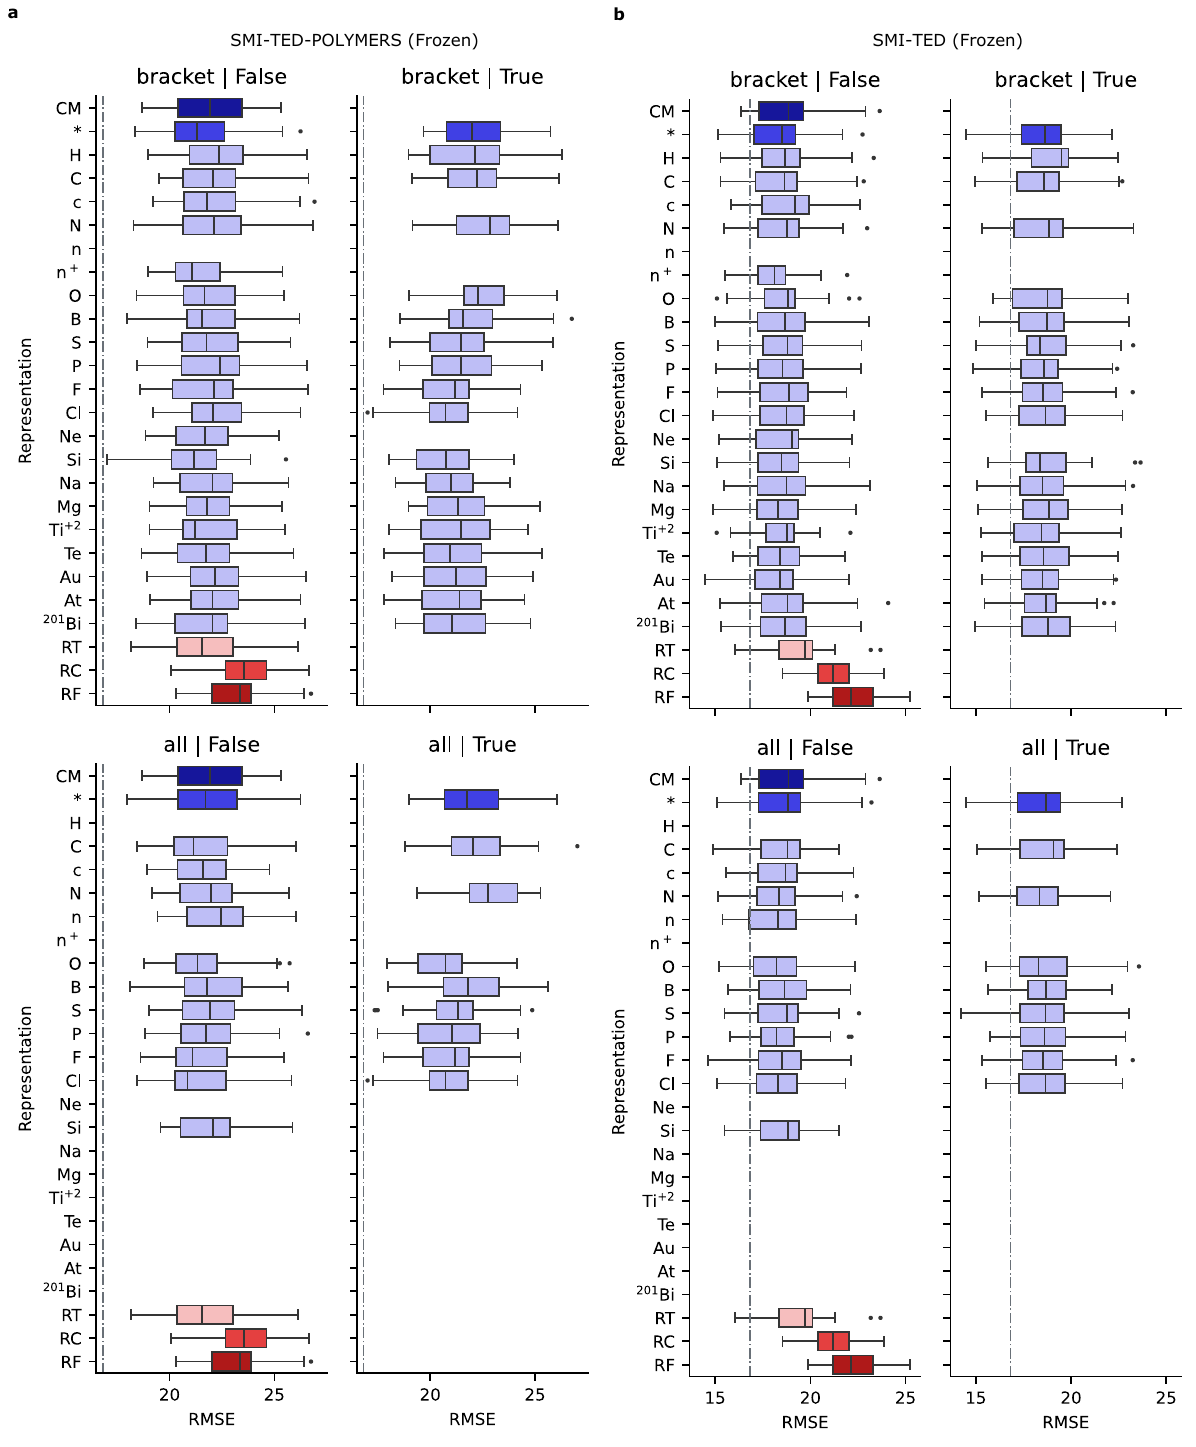}
\caption{Box plots for X\textsubscript{c} repeated cross-validation experiments for SMI-TED-POLYMER (\textbf{a}) and SMI-TED (\textbf{b}) models with frozen weights.}\label{xc_token_box_frozen}
\end{figure}

\begin{figure}[H]
\centering
\includegraphics[width=1\textwidth]{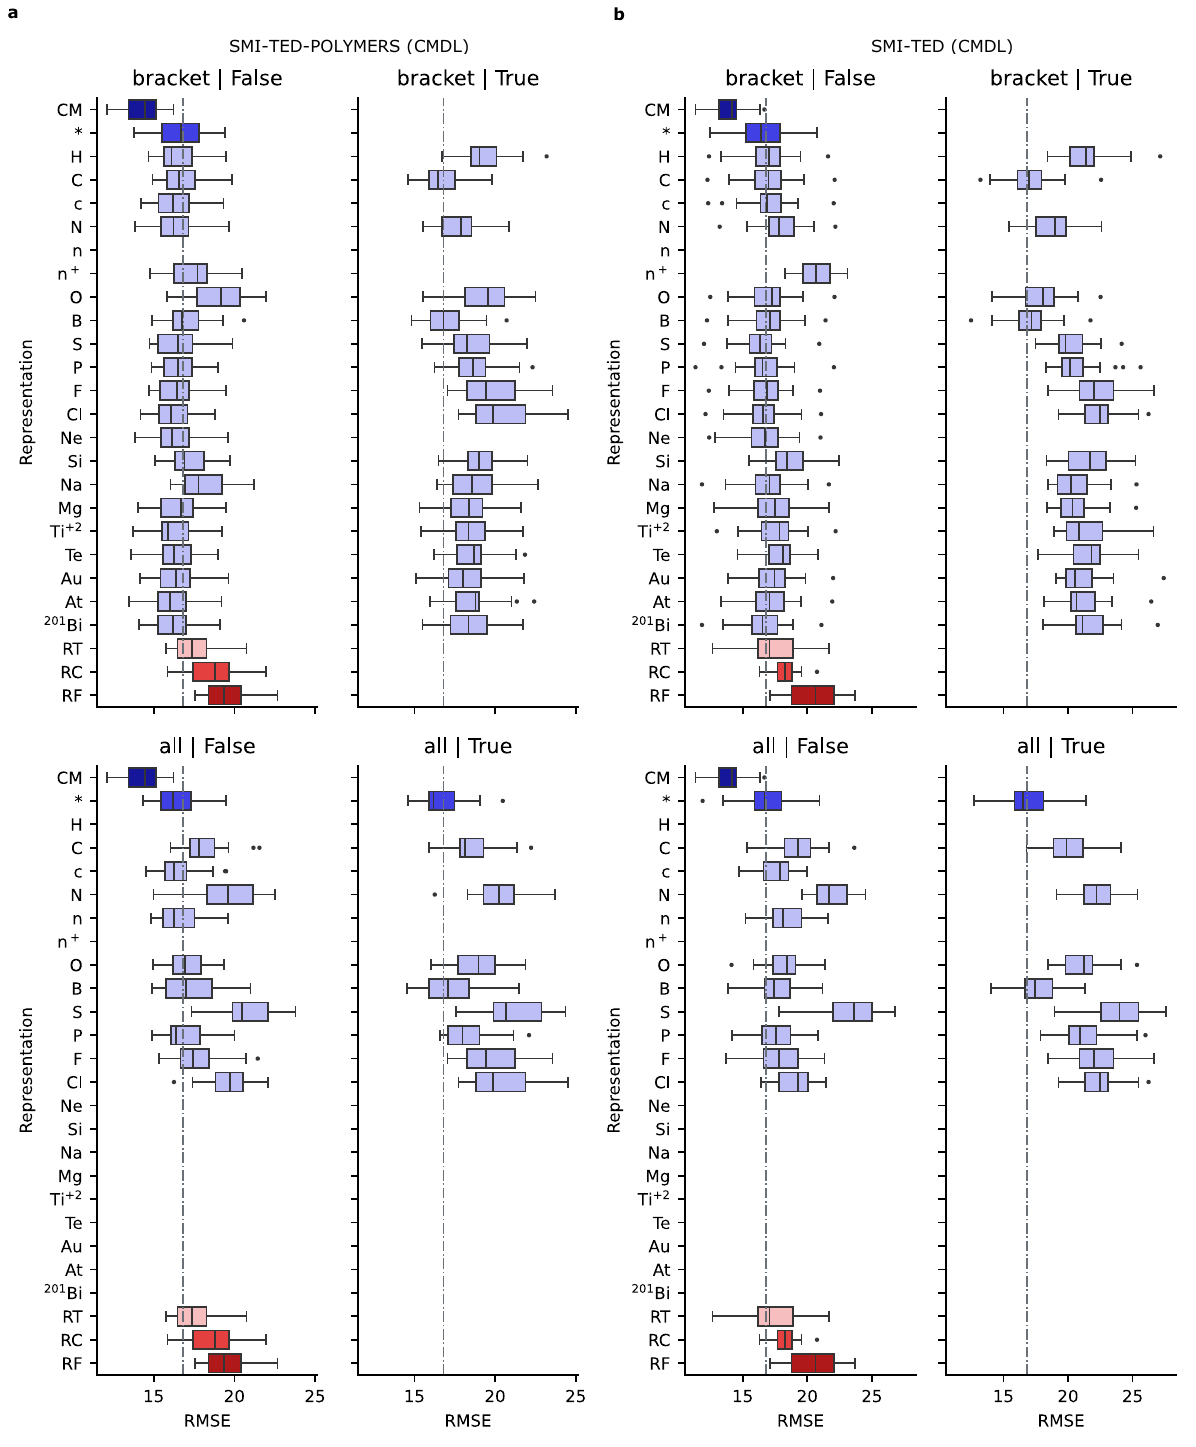}
\caption{Box plots for X\textsubscript{c} repeated cross-validation experiments for SMI-TED-POLYMER (\textbf{a}) and SMI-TED (\textbf{b}) models fine-tuned with the CPG polymer graphs.}\label{xc_token_box_cmdl}
\end{figure}

\begin{figure}[H]
\centering
\includegraphics[width=1\textwidth]{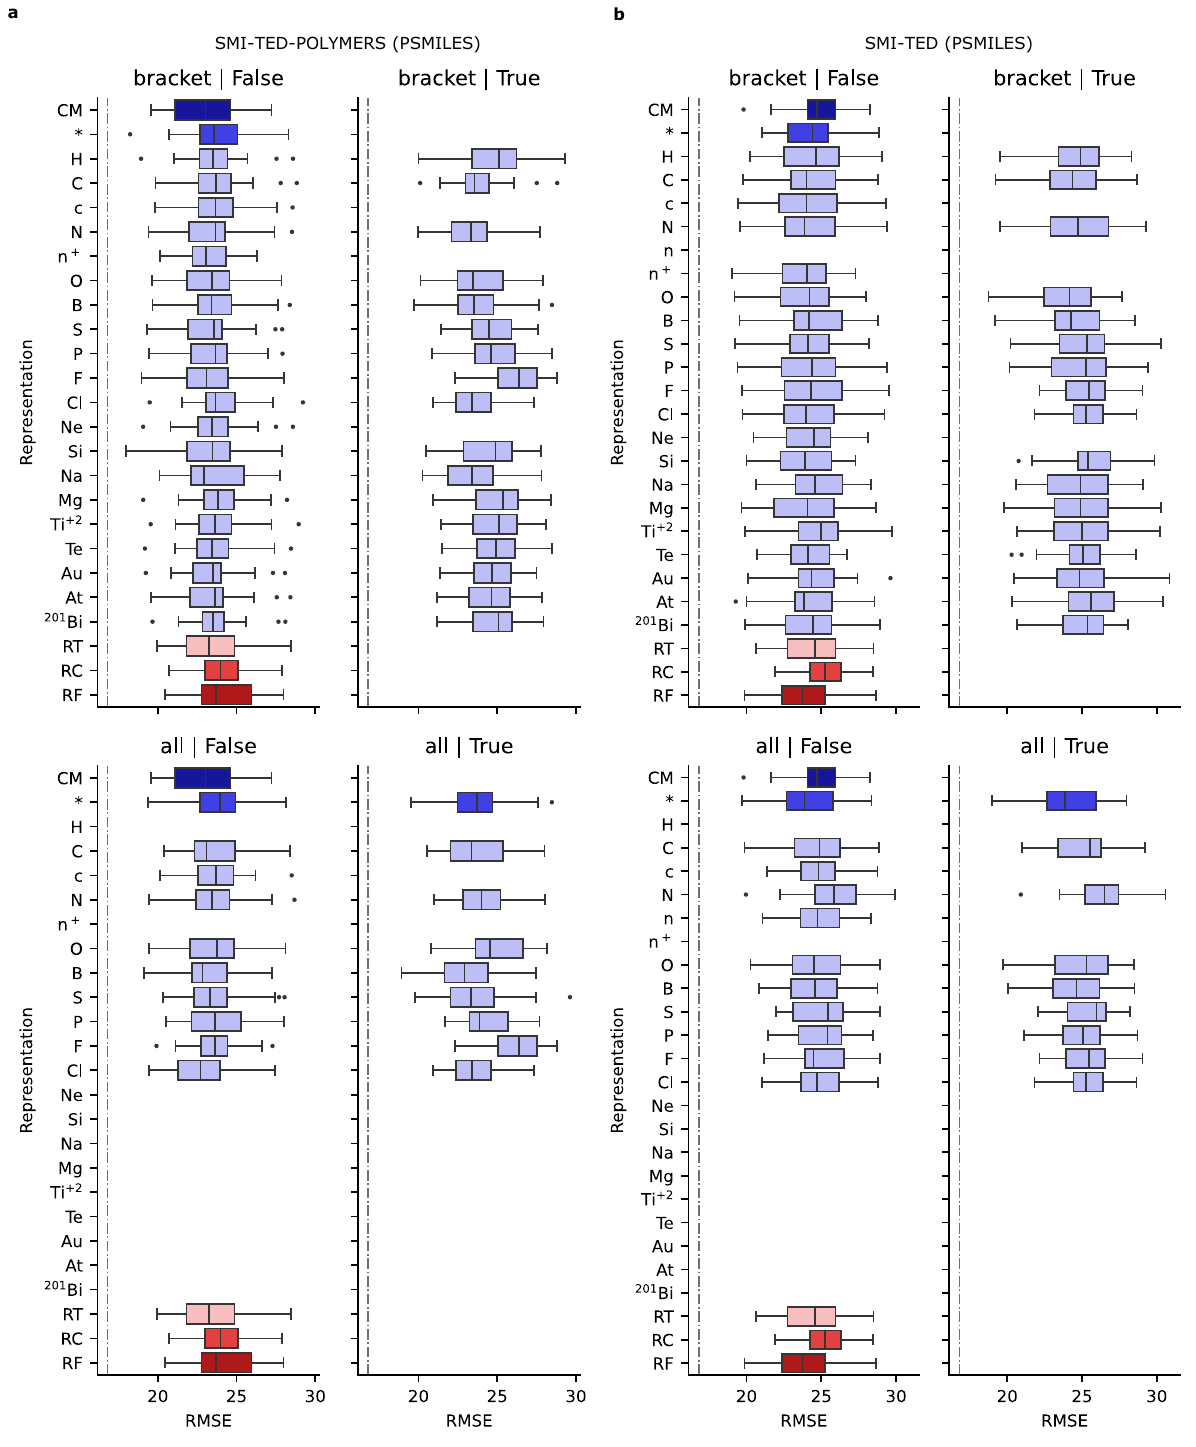}
\caption{Box plots for X\textsubscript{c} repeated cross-validation experiments for SMI-TED-POLYMER (\textbf{a}) and SMI-TED (\textbf{b}) models fine-tuned with PSMILES.}\label{xc_token_box_psmiles}
\end{figure}

\subsubsection{Crystallization Tendency (X\textsubscript{c}) Random Split Scores}\label{randXc}

\begin{figure}[H]
\centering
\includegraphics[width=1\textwidth]{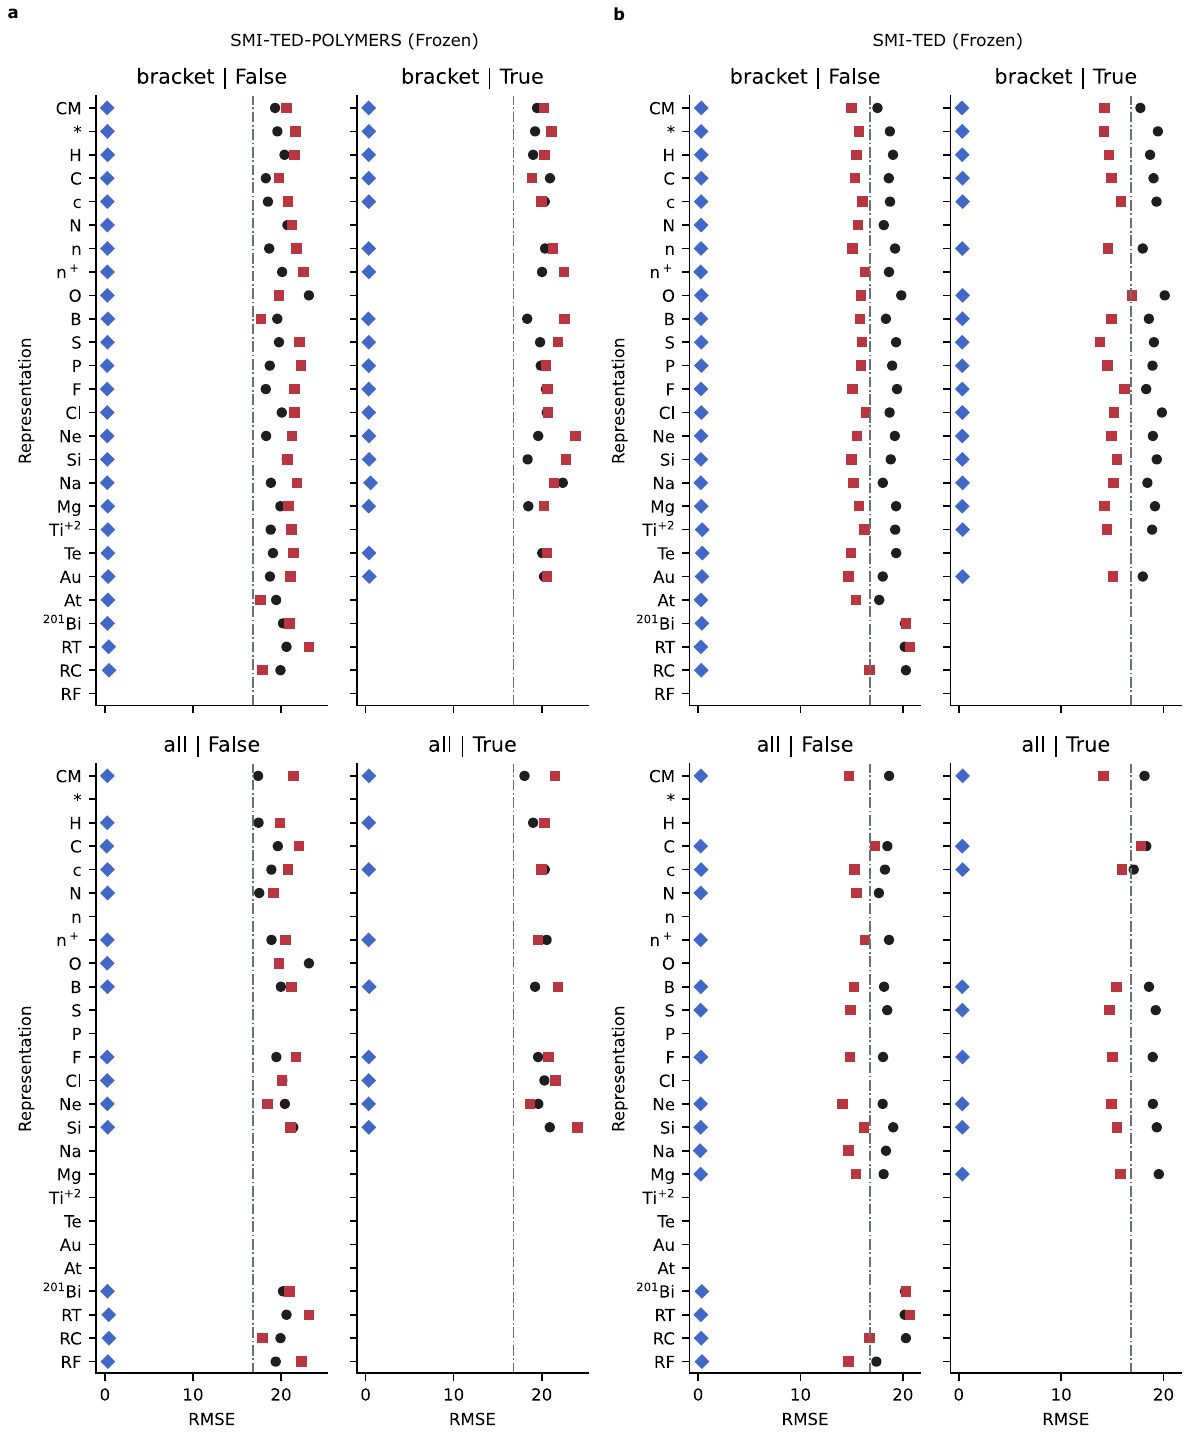}
\caption{Point plots for X\textsubscript{c} benchmark experiments of RMSE using the base random train, valid, and test splits for SMI-TED-POLYMER (\textbf{a}) and SMI-TED (\textbf{b}) models with frozen weights.}\label{xc_token_point_frozen_rmse}
\end{figure}

\begin{figure}[H]
\centering
\includegraphics[width=1\textwidth]{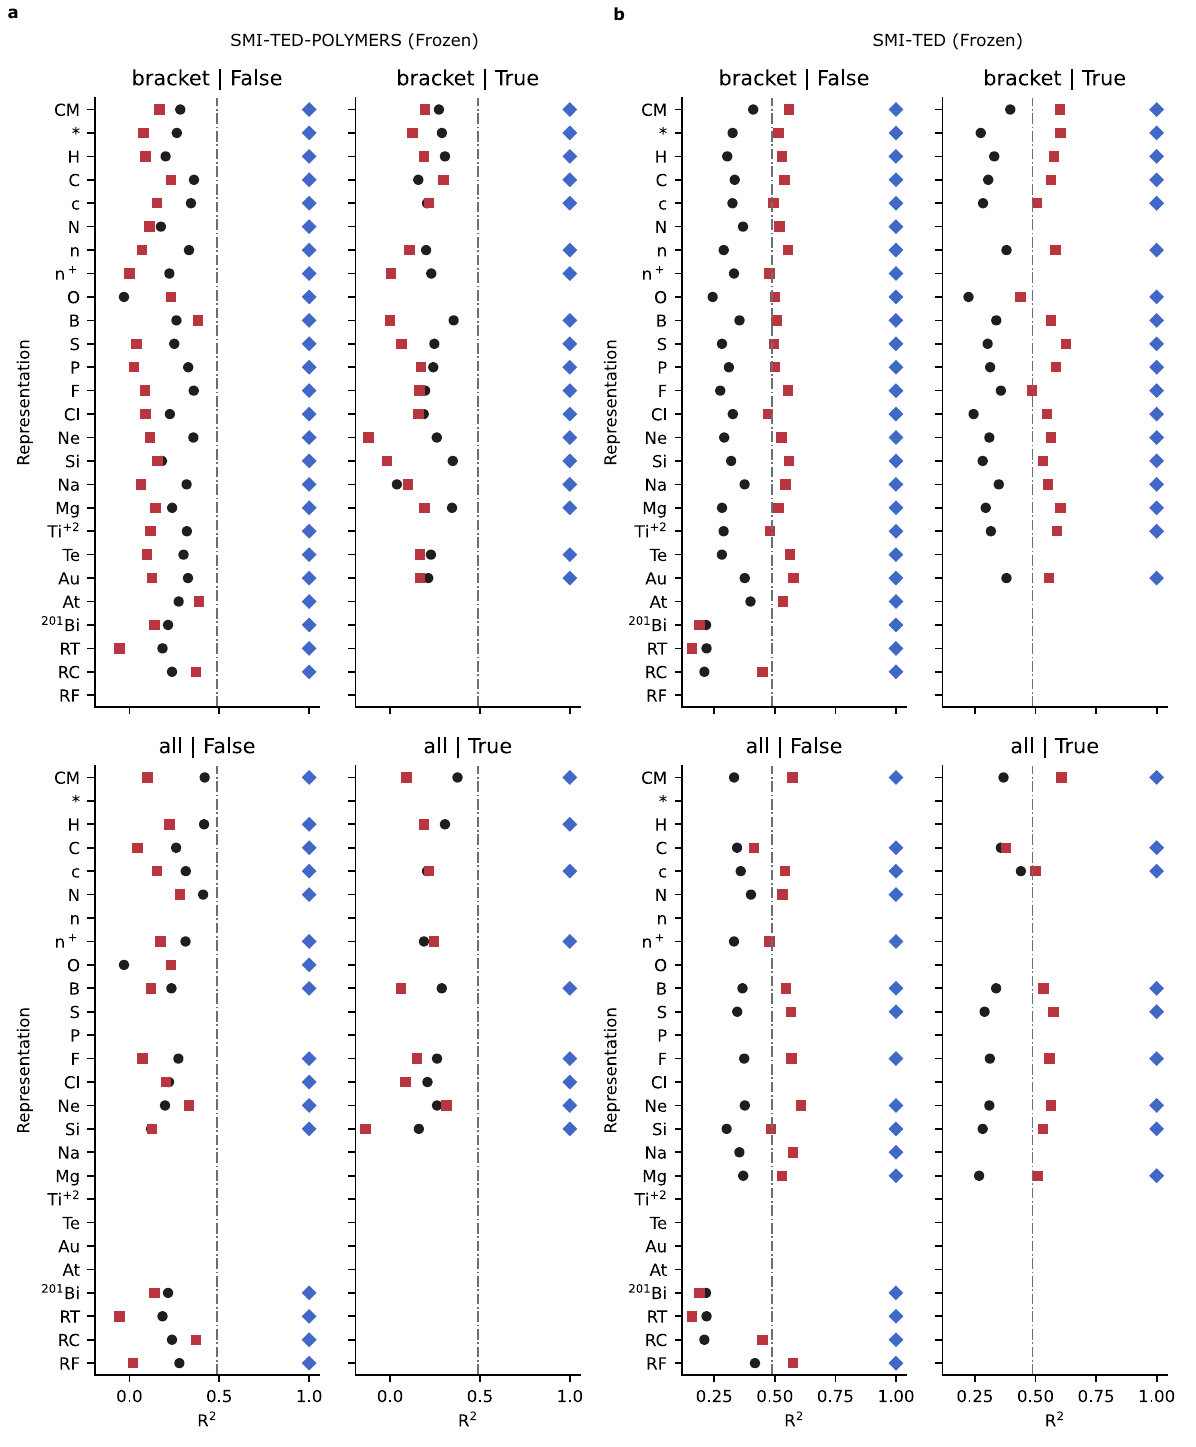}
\caption{Point plots for X\textsubscript{c} benchmark experiments of R\textsuperscript{2} using the base random train, valid, and test splits for SMI-TED-POLYMER (\textbf{a}) and SMI-TED (\textbf{b}) models with frozen weights.}\label{xc_token_point_frozen_r2}
\end{figure}

\begin{figure}[H]
\centering
\includegraphics[width=1\textwidth]{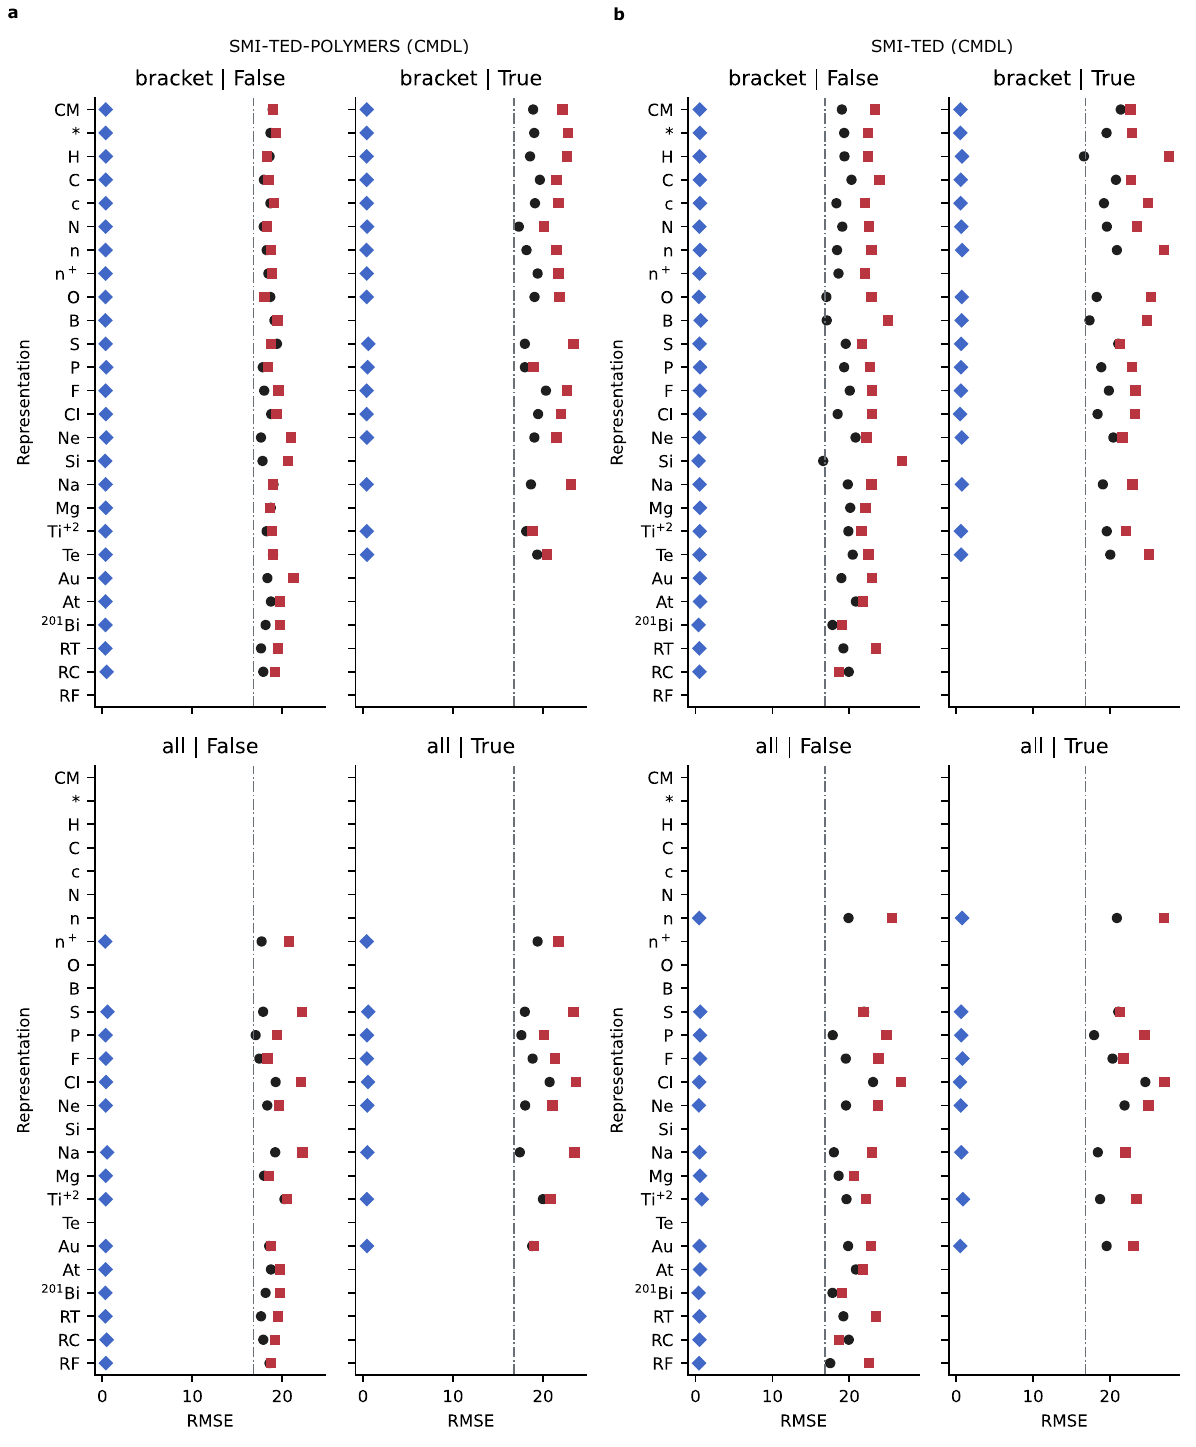}
\caption{Point plots for X\textsubscript{c} benchmark experiments of RMSE using the base random train, valid, and test splits for SMI-TED-POLYMER (\textbf{a}) and SMI-TED (\textbf{b}) models fine-tuned with CPG.}\label{xc_token_point_cmdl_rmse}
\end{figure}

\begin{figure}[H]
\centering
\includegraphics[width=1\textwidth]{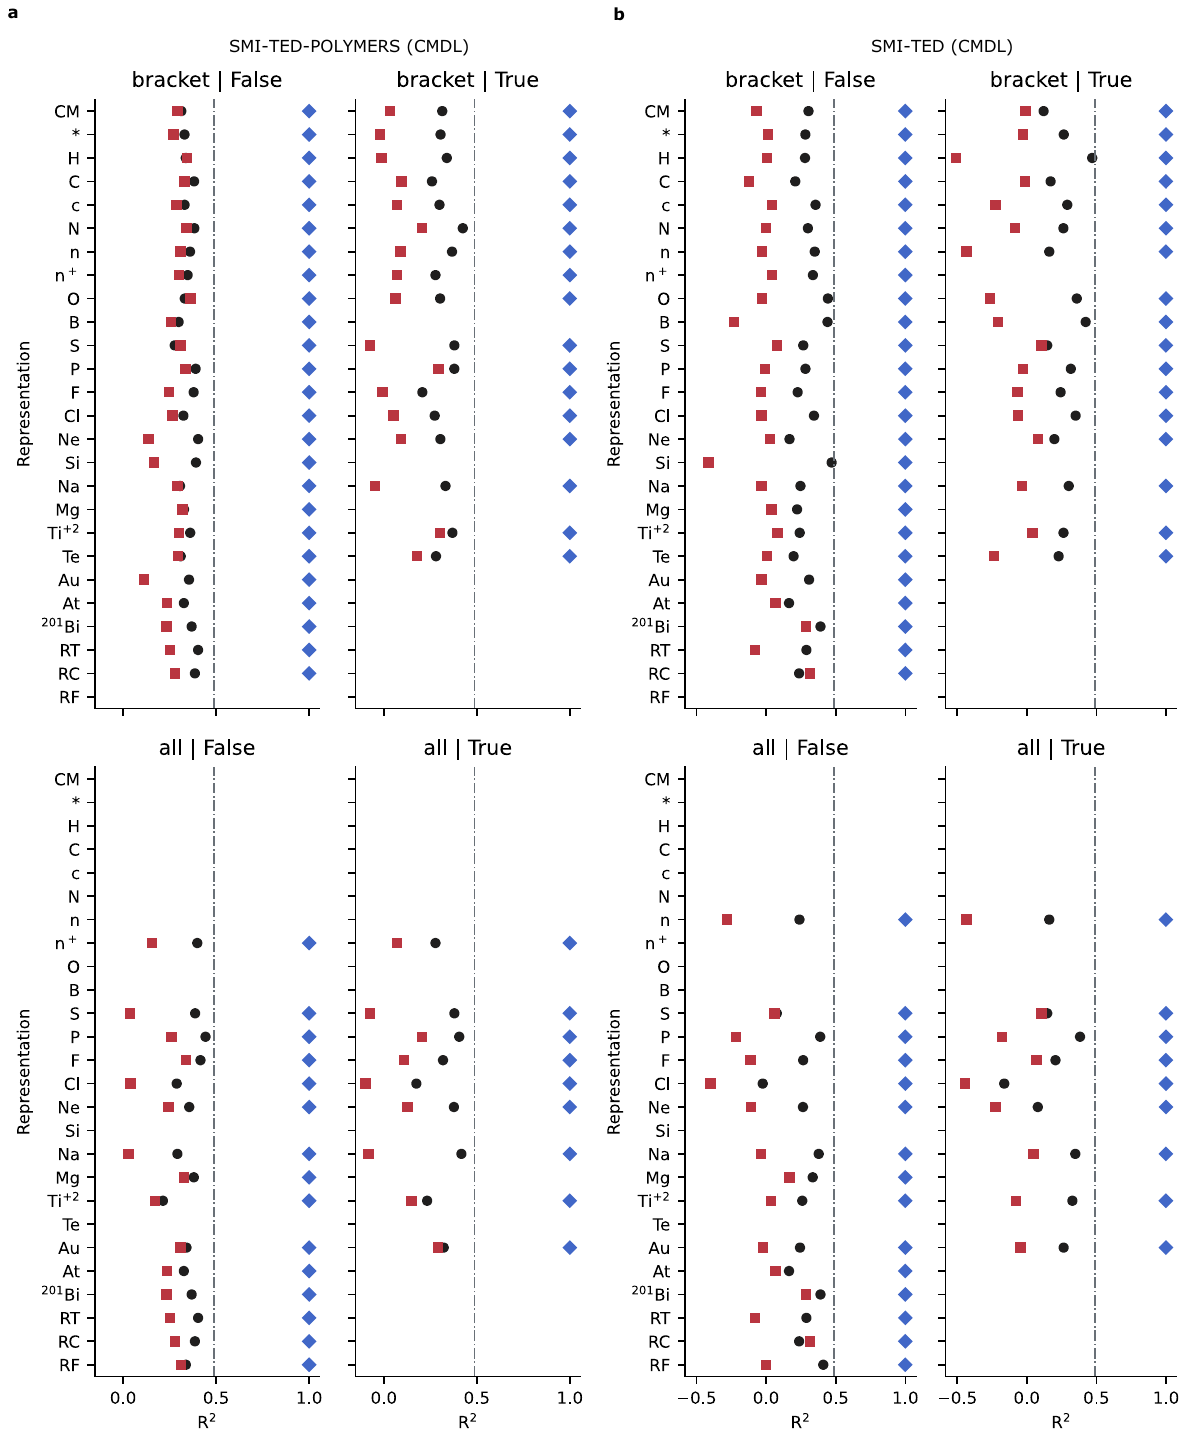}
\caption{Point plots for X\textsubscript{c} benchmark experiments of R\textsuperscript{2} using the base random train, valid, and test splits for SMI-TED-POLYMER (\textbf{a}) and SMI-TED (\textbf{b}) models fine-tuned with CPG.}\label{xc_token_point_cmdl_r2}
\end{figure}

\begin{figure}[H]
\centering
\includegraphics[width=1\textwidth]{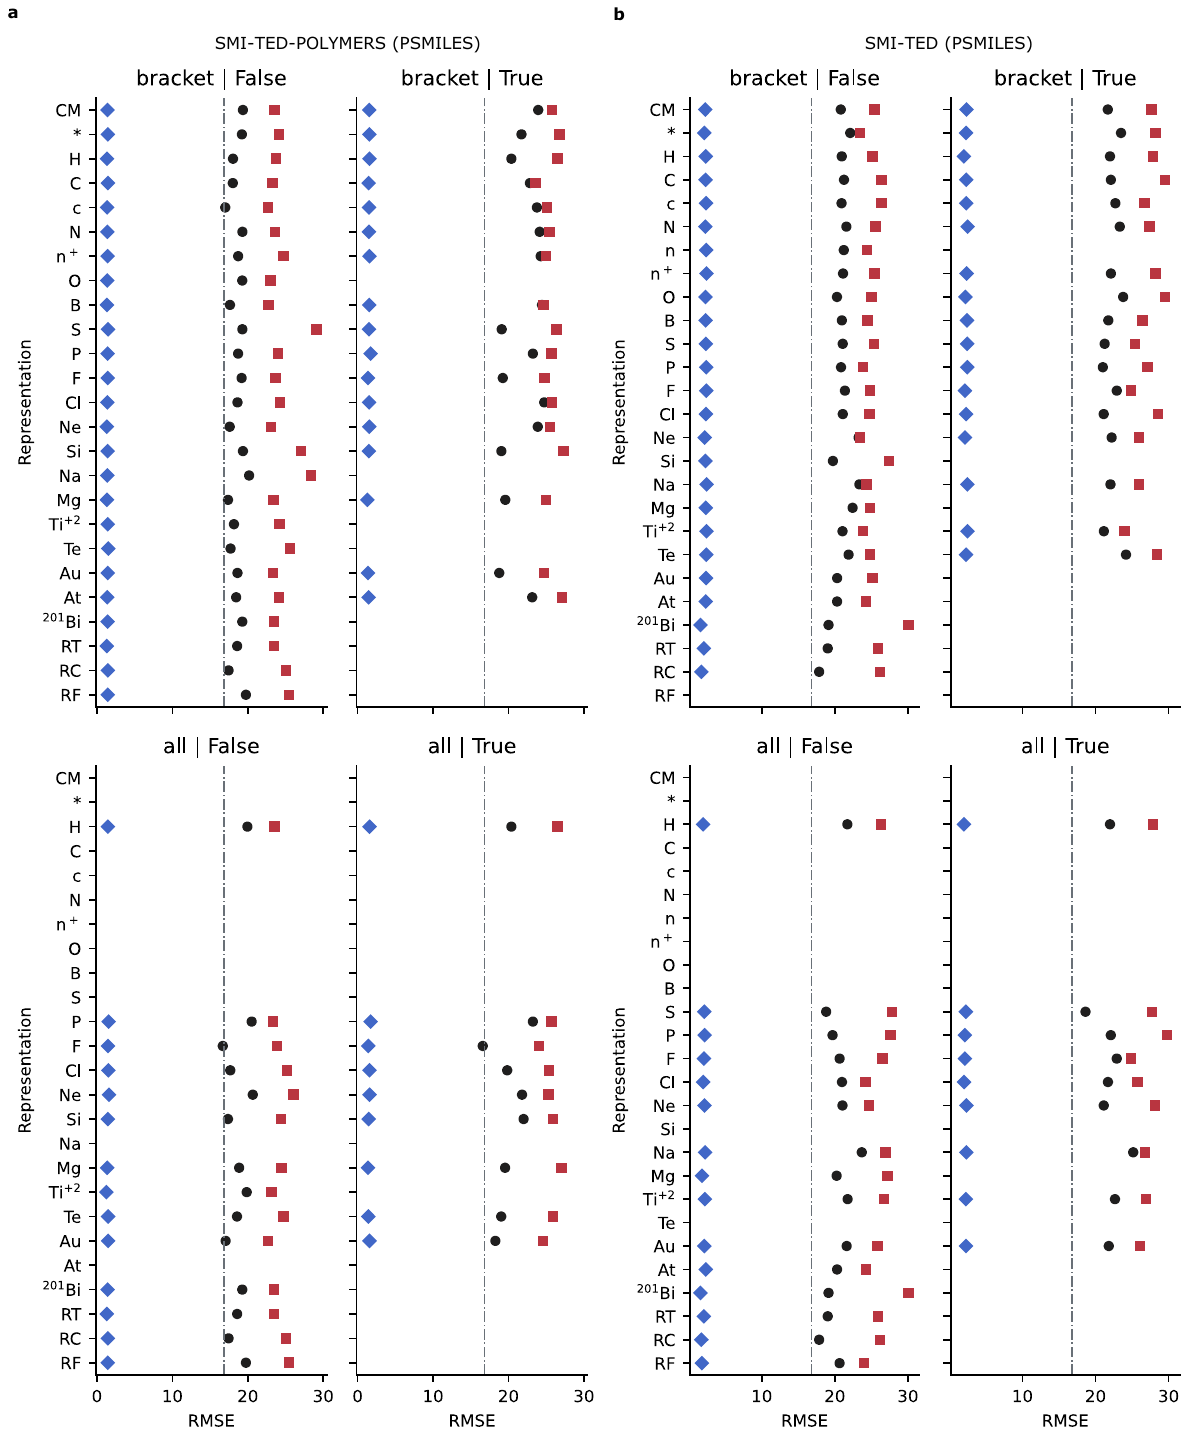}
\caption{Point plots for X\textsubscript{c} benchmark experiments of RMSE using the base random train, valid, and test splits for SMI-TED-POLYMER (\textbf{a}) and SMI-TED (\textbf{b}) models fine-tuned with PSMILES.}\label{xc_token_point_psmiles_rmse}
\end{figure}

\begin{figure}[H]
\centering
\includegraphics[width=1\textwidth]{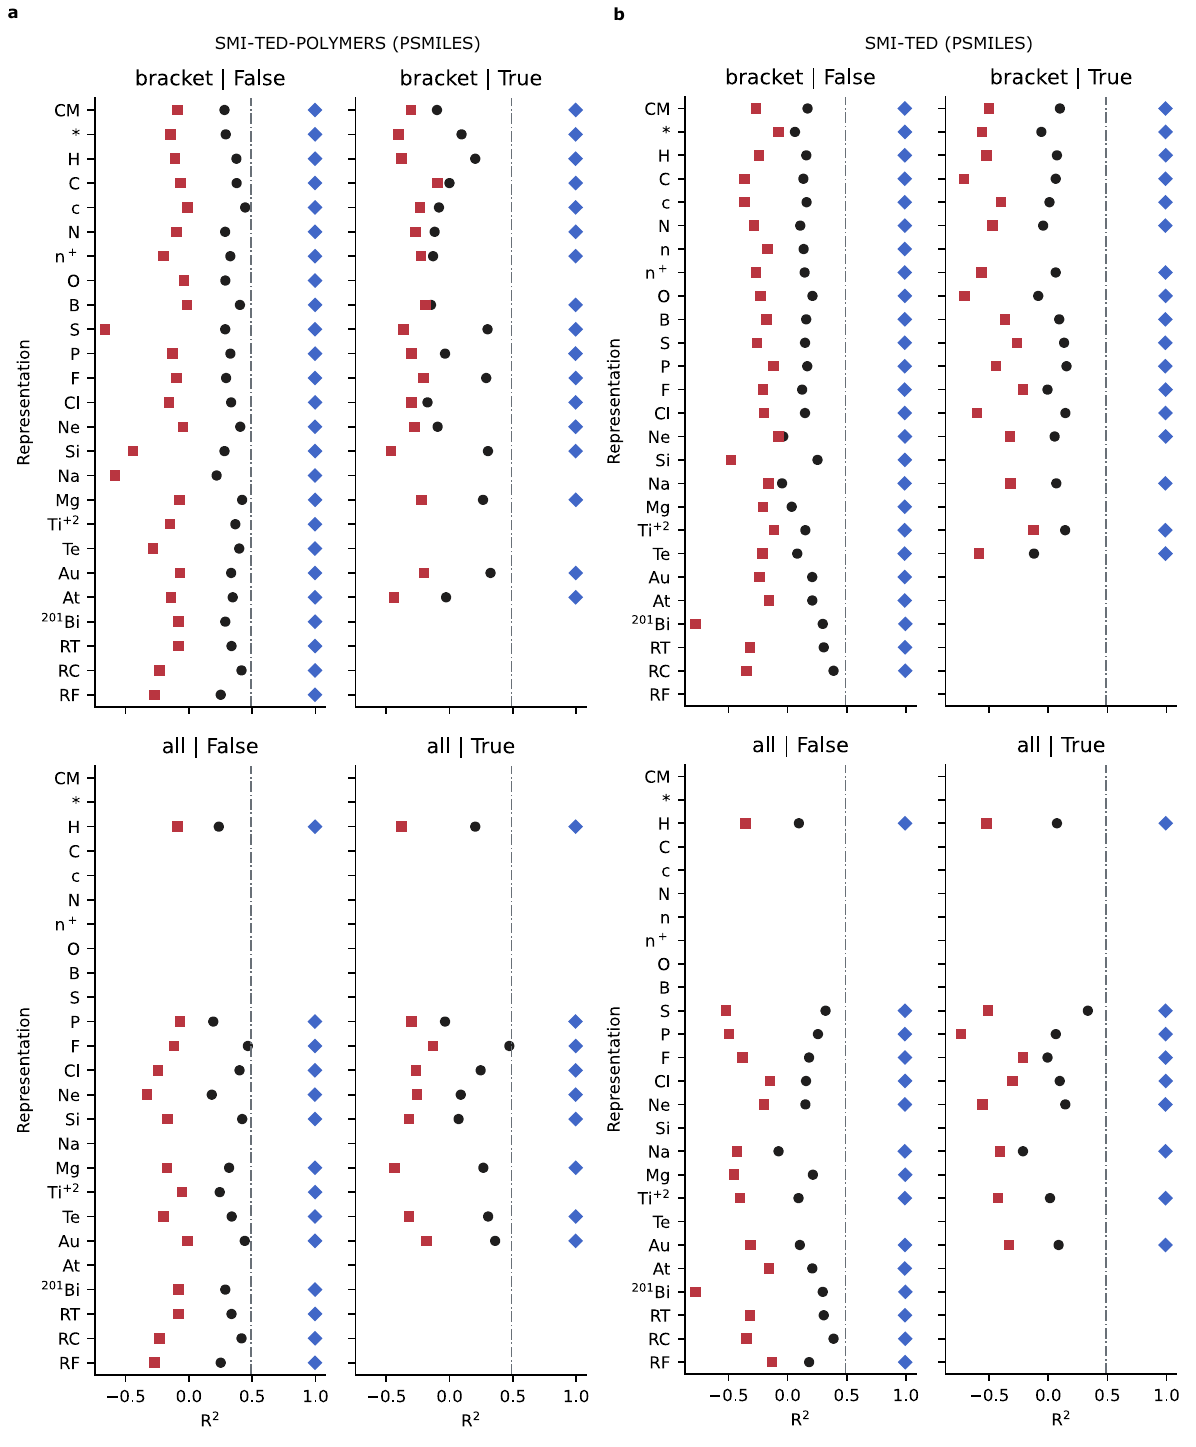}
\caption{Point plots for X\textsubscript{c} benchmark experiments of R\textsuperscript{2} using the base random train, valid, and test splits for SMI-TED-POLYMER (\textbf{a}) and SMI-TED (\textbf{b}) models fine-tuned with PSMILES.}\label{xc_token_point_psmiles_r2}
\end{figure}

\subsubsection{Glass Transition Temperature (T\textsubscript{g}-II) CV Scores}\label{cvAcsTg}

\begin{figure}[H]
\centering
\includegraphics[width=1\textwidth]{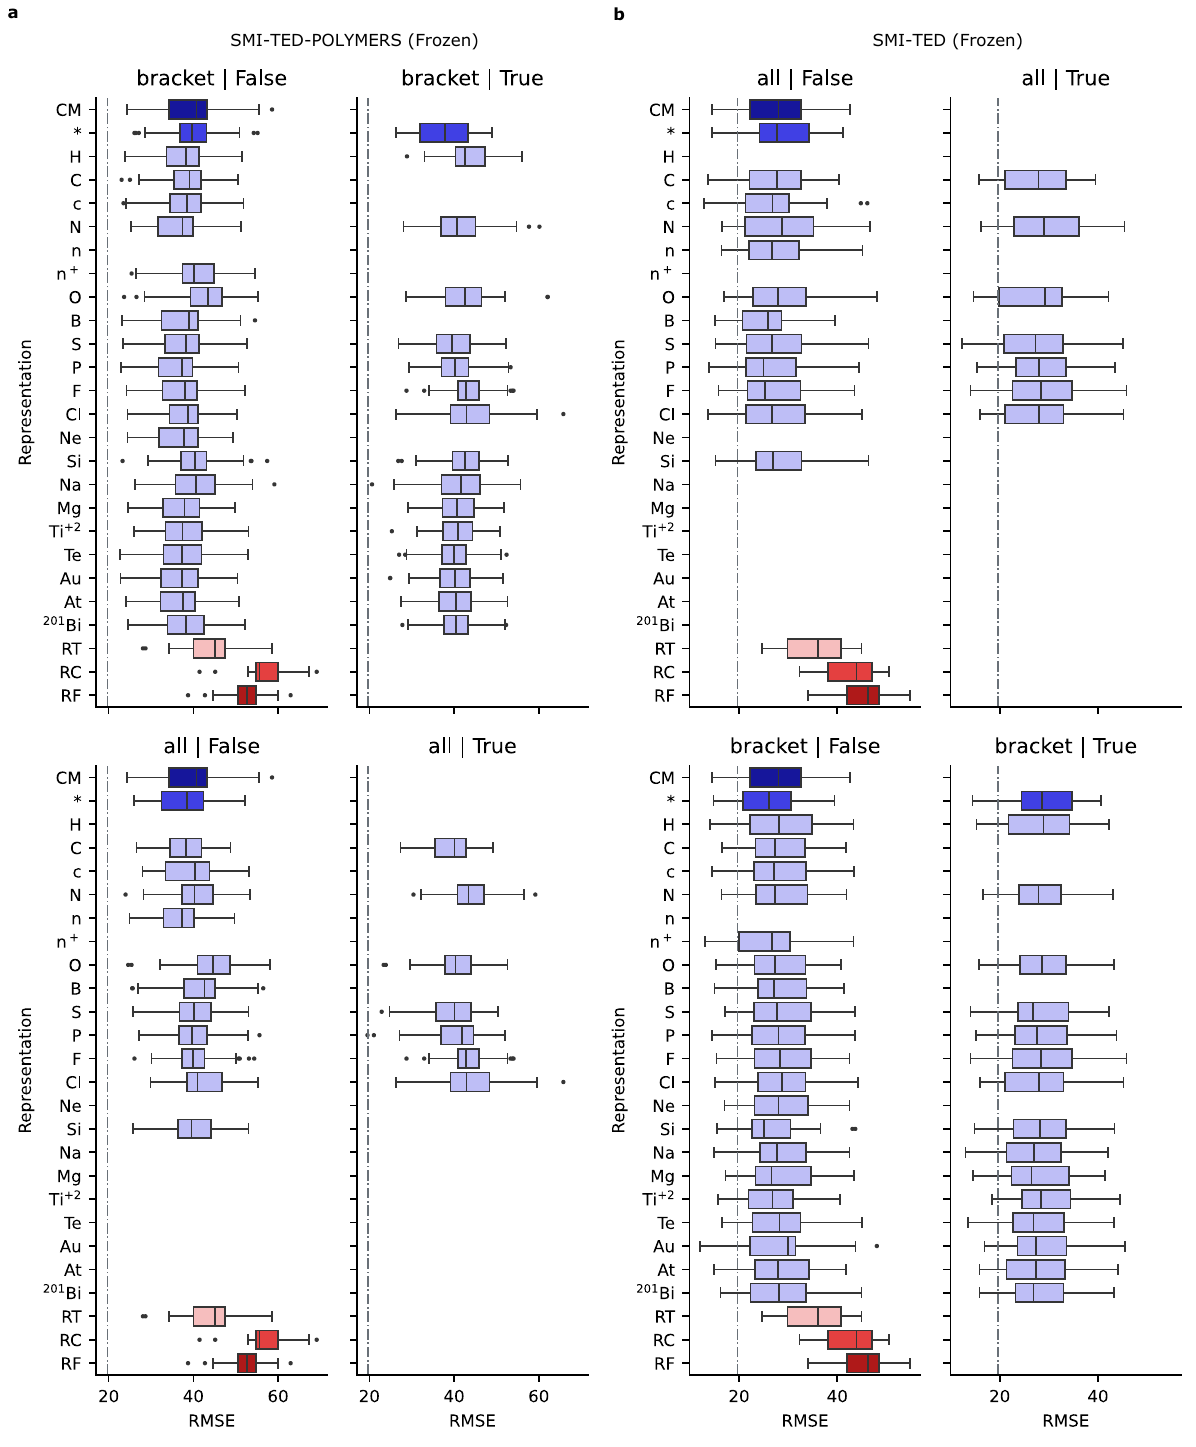}
\caption{Box plots for T\textsubscript{g}-II repeated cross-validation experiments for SMI-TED-POLYMER (\textbf{a}) and SMI-TED (\textbf{b}) models with frozen weights.}\label{acs_ami_tg_token_box_frozen}
\end{figure}

\begin{figure}[H]
\centering
\includegraphics[width=1\textwidth]{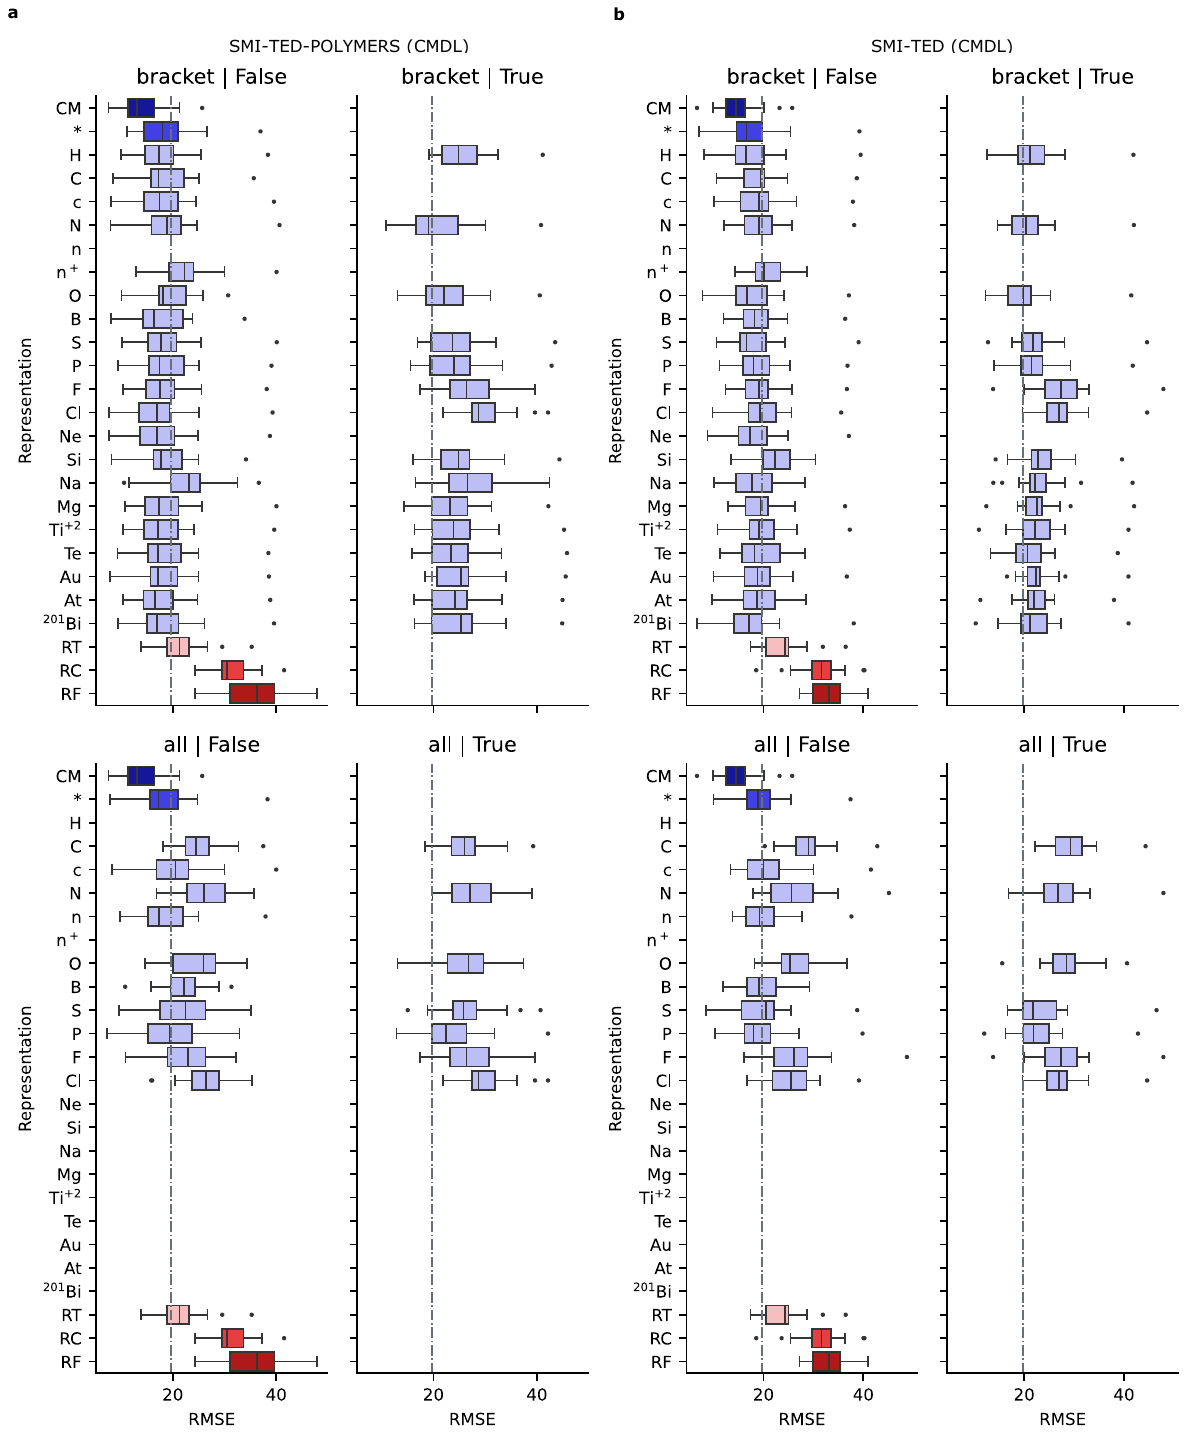}
\caption{Box plots for T\textsubscript{g}-II repeated cross-validation experiments for SMI-TED-POLYMER (\textbf{a}) and SMI-TED (\textbf{b}) models fine-tuned with the CPG polymer graphs.}\label{acs_ami_tg_token_box_cmdl}
\end{figure}

\begin{figure}[H]
\centering
\includegraphics[width=1\textwidth]{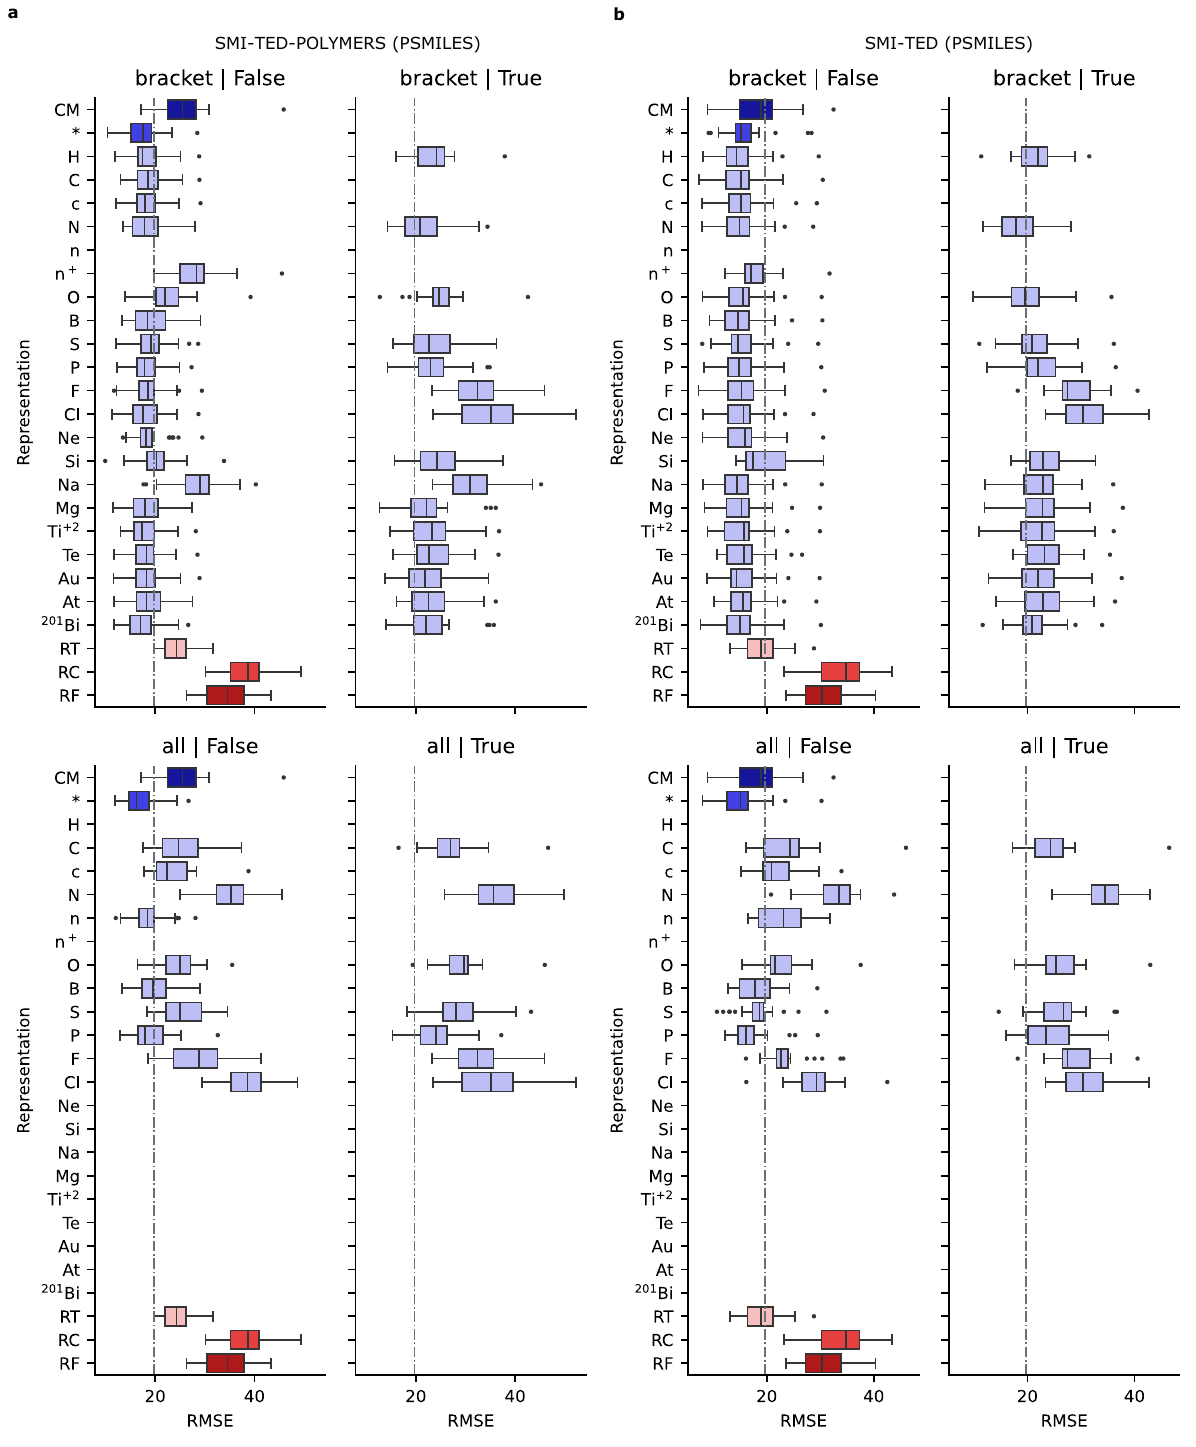}
\caption{Box plots for T\textsubscript{g}-II repeated cross-validation experiments for SMI-TED-POLYMER (\textbf{a}) and SMI-TED (\textbf{b}) models fine-tuned with PSMILES.}\label{acs_ami_tg_token_box_psmiles}
\end{figure}

\subsubsection{Glass Transition Temperature (T\textsubscript{g}-II) Random Split Scores}\label{randAcsTg}

\begin{figure}[H]
\centering
\includegraphics[width=1\textwidth]{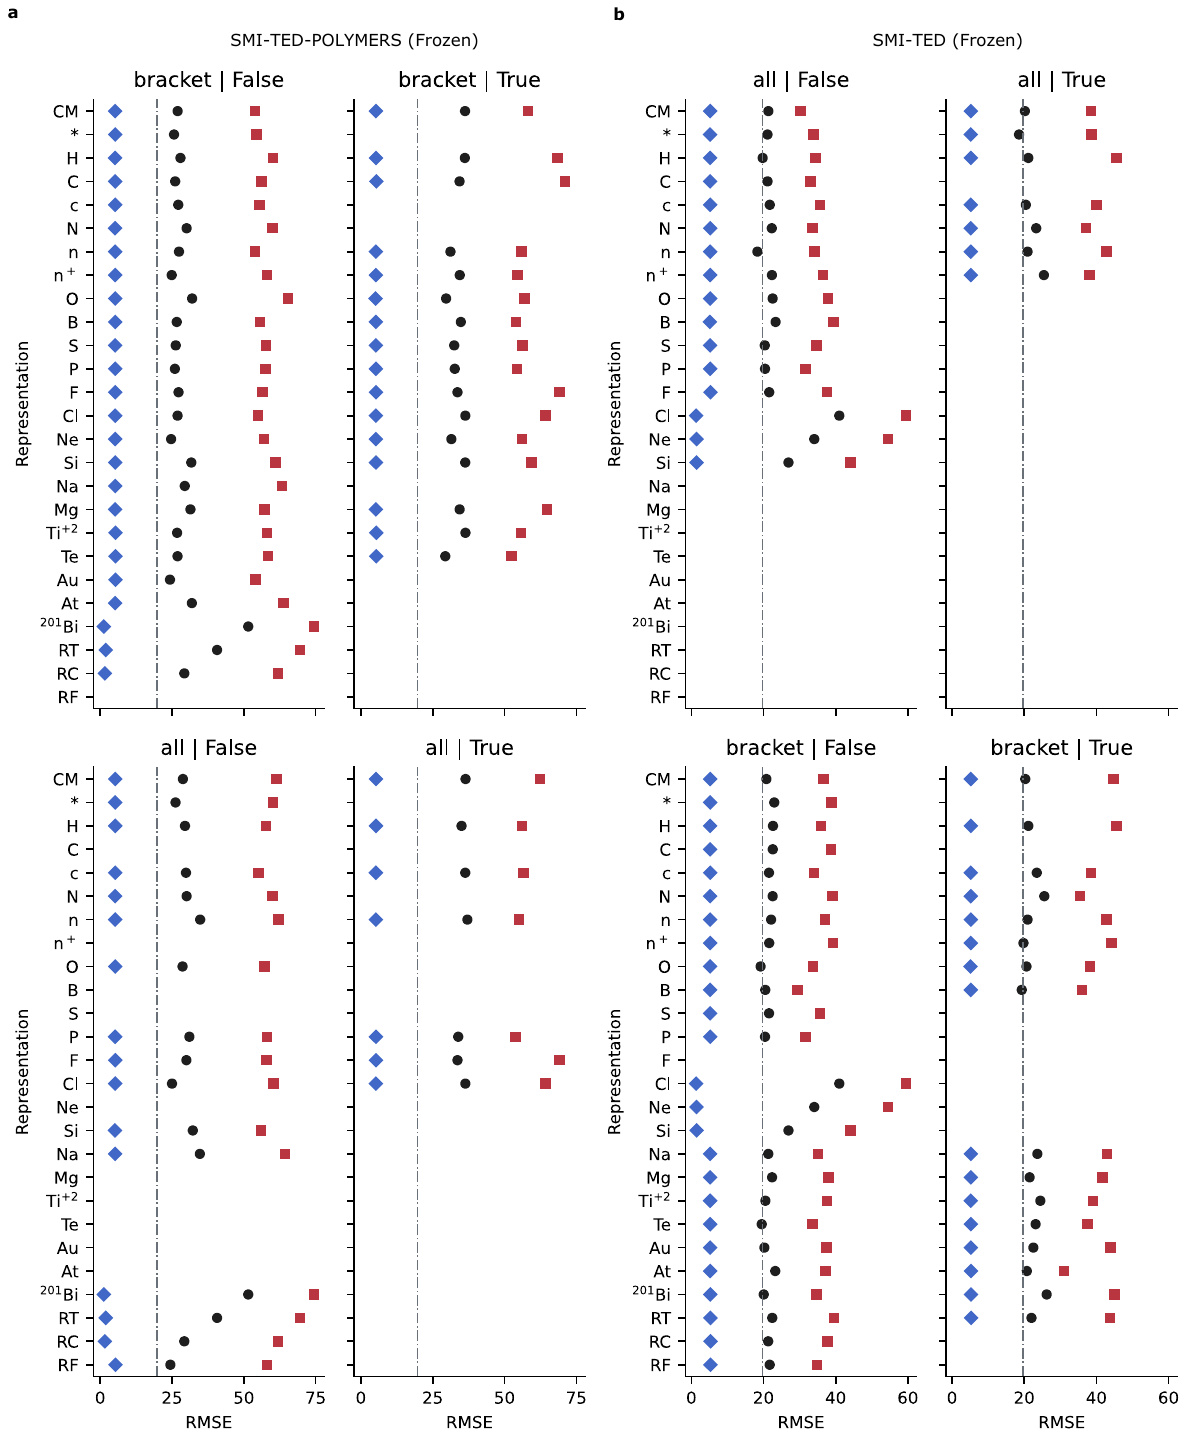}
\caption{Point plots for T\textsubscript{g}-II benchmark experiments of RMSE using the base random train, valid, and test splits for SMI-TED-POLYMER (\textbf{a}) and SMI-TED (\textbf{b}) models with frozen weights.}\label{acs_ami_tg_token_point_frozen_rmse}
\end{figure}

\begin{figure}[H]
\centering
\includegraphics[width=1\textwidth]{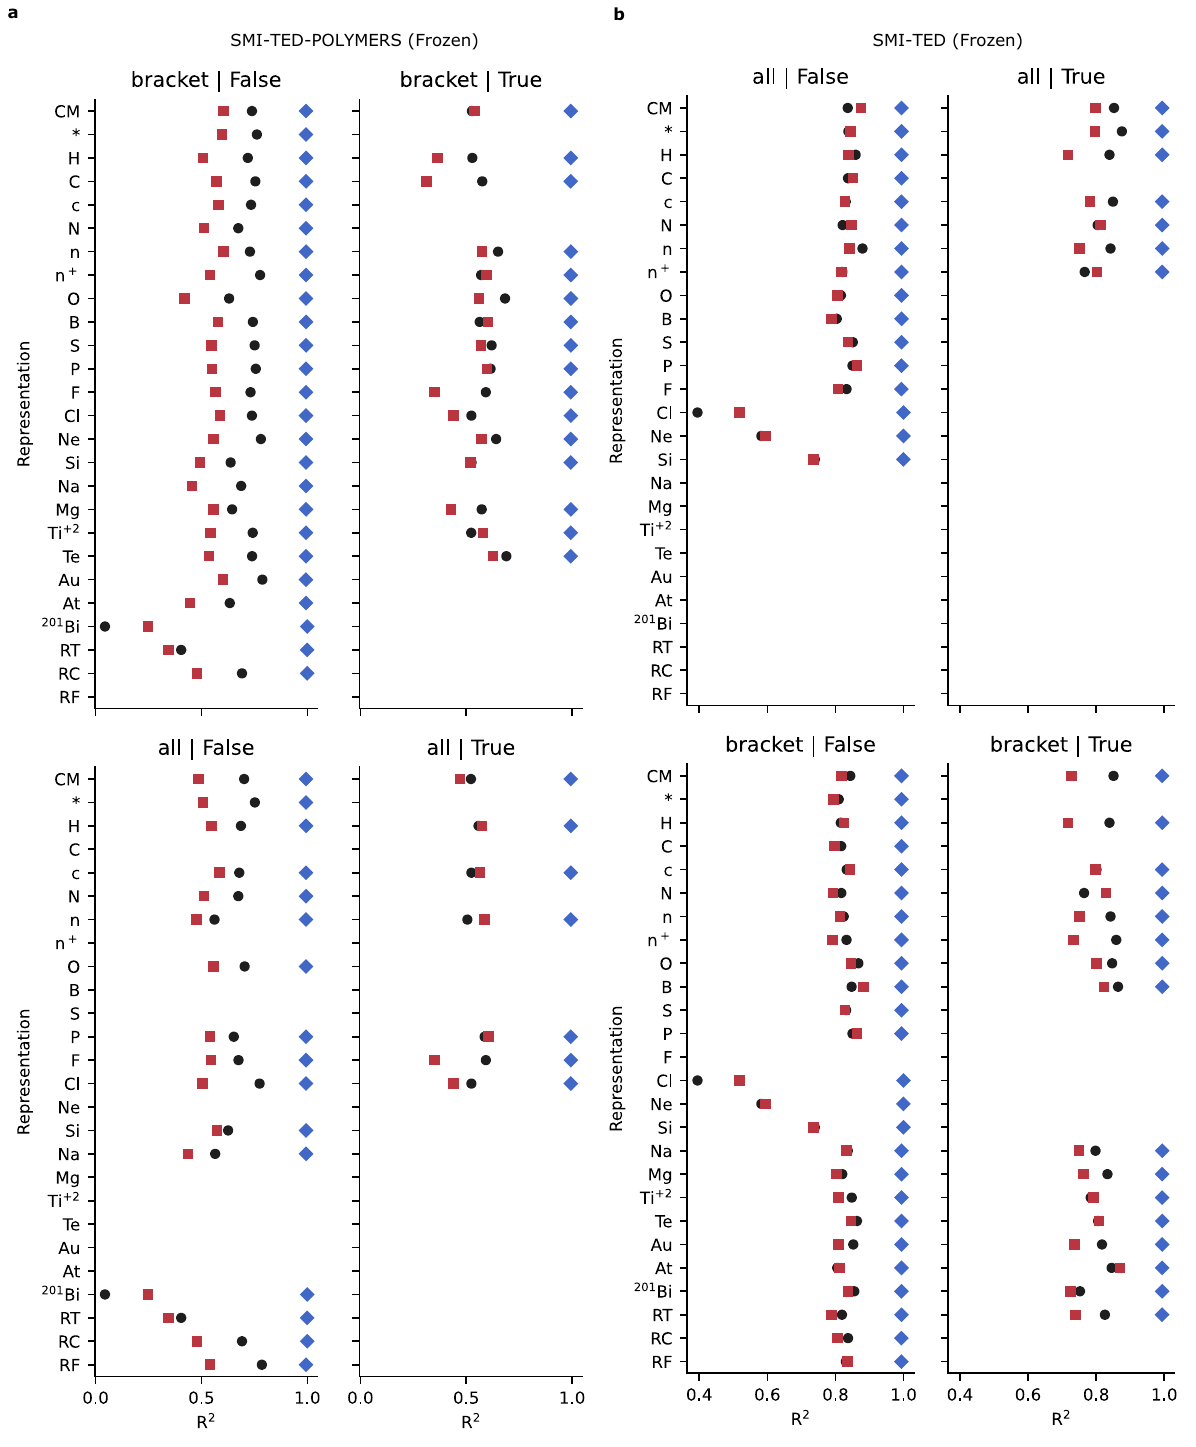}
\caption{Point plots for T\textsubscript{g}-II benchmark experiments of R\textsuperscript{2} using the base random train, valid, and test splits for SMI-TED-POLYMER (\textbf{a}) and SMI-TED (\textbf{b}) models with frozen weights.}\label{acs_ami_tg_token_point_frozen_r2}
\end{figure}

\begin{figure}[H]
\centering
\includegraphics[width=1\textwidth]{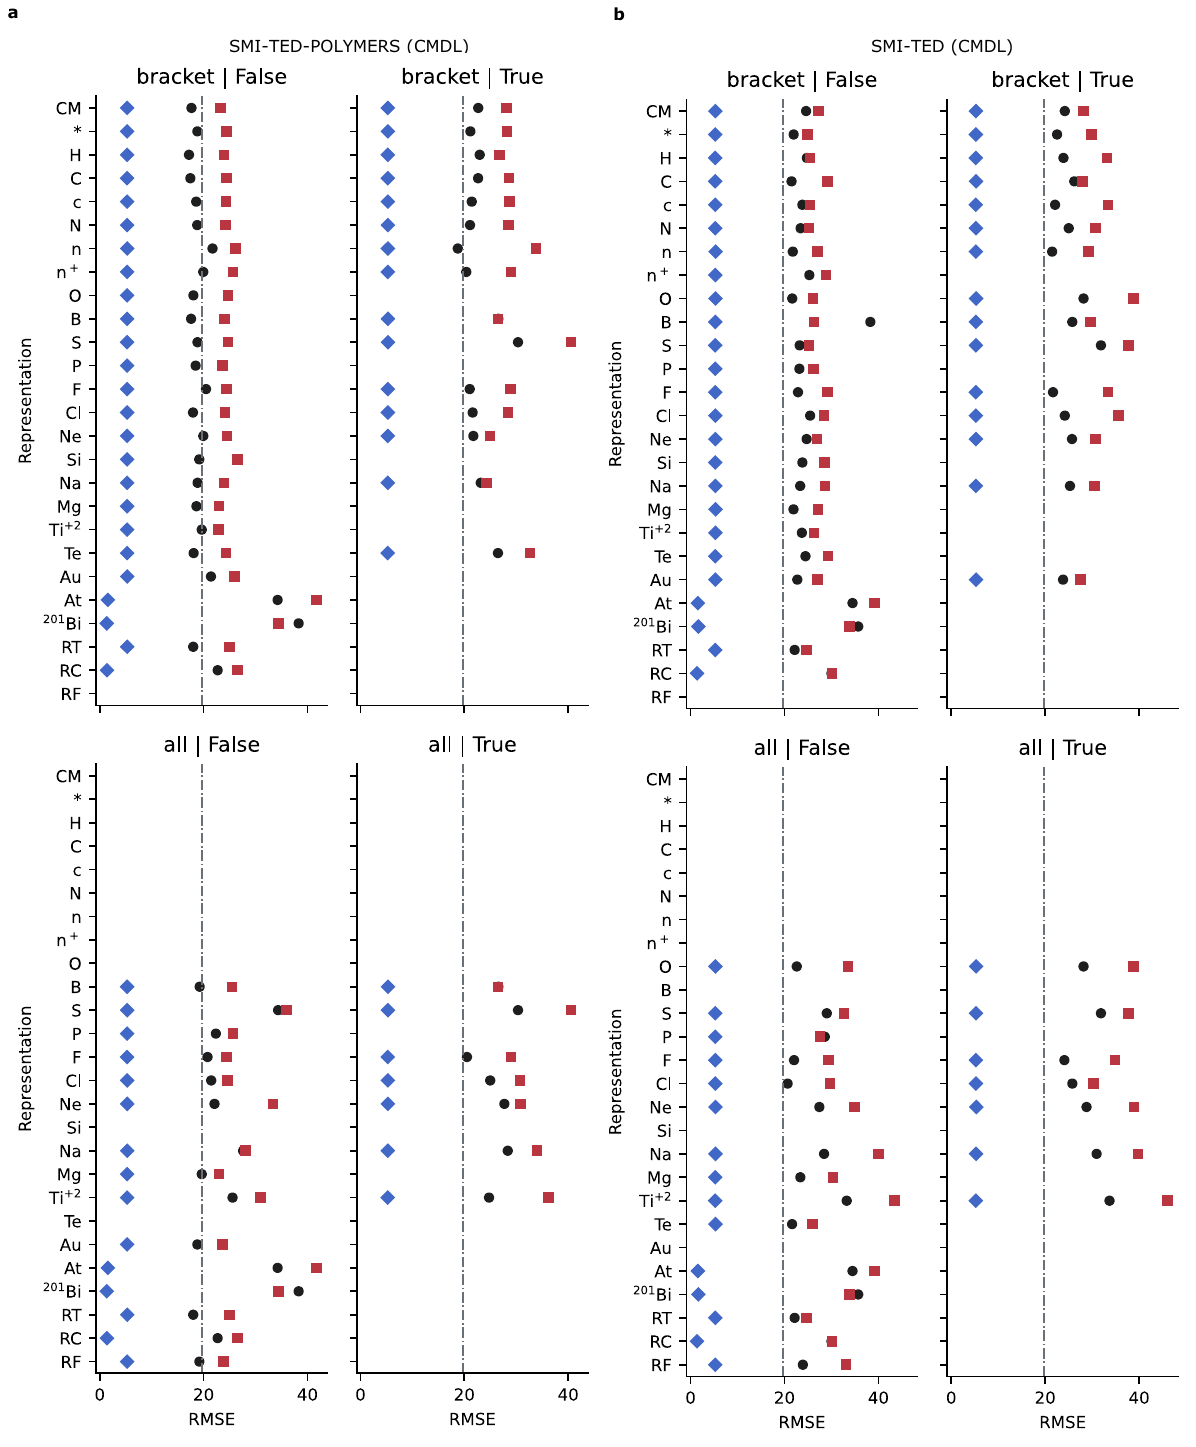}
\caption{Point plots for T\textsubscript{g}-II benchmark experiments of RMSE using the base random train, valid, and test splits for SMI-TED-POLYMER (\textbf{a}) and SMI-TED (\textbf{b}) models fine-tuned with CPG.}\label{acs_ami_tg_token_point_cmdl_rmse}
\end{figure}

\begin{figure}[H]
\centering
\includegraphics[width=1\textwidth]{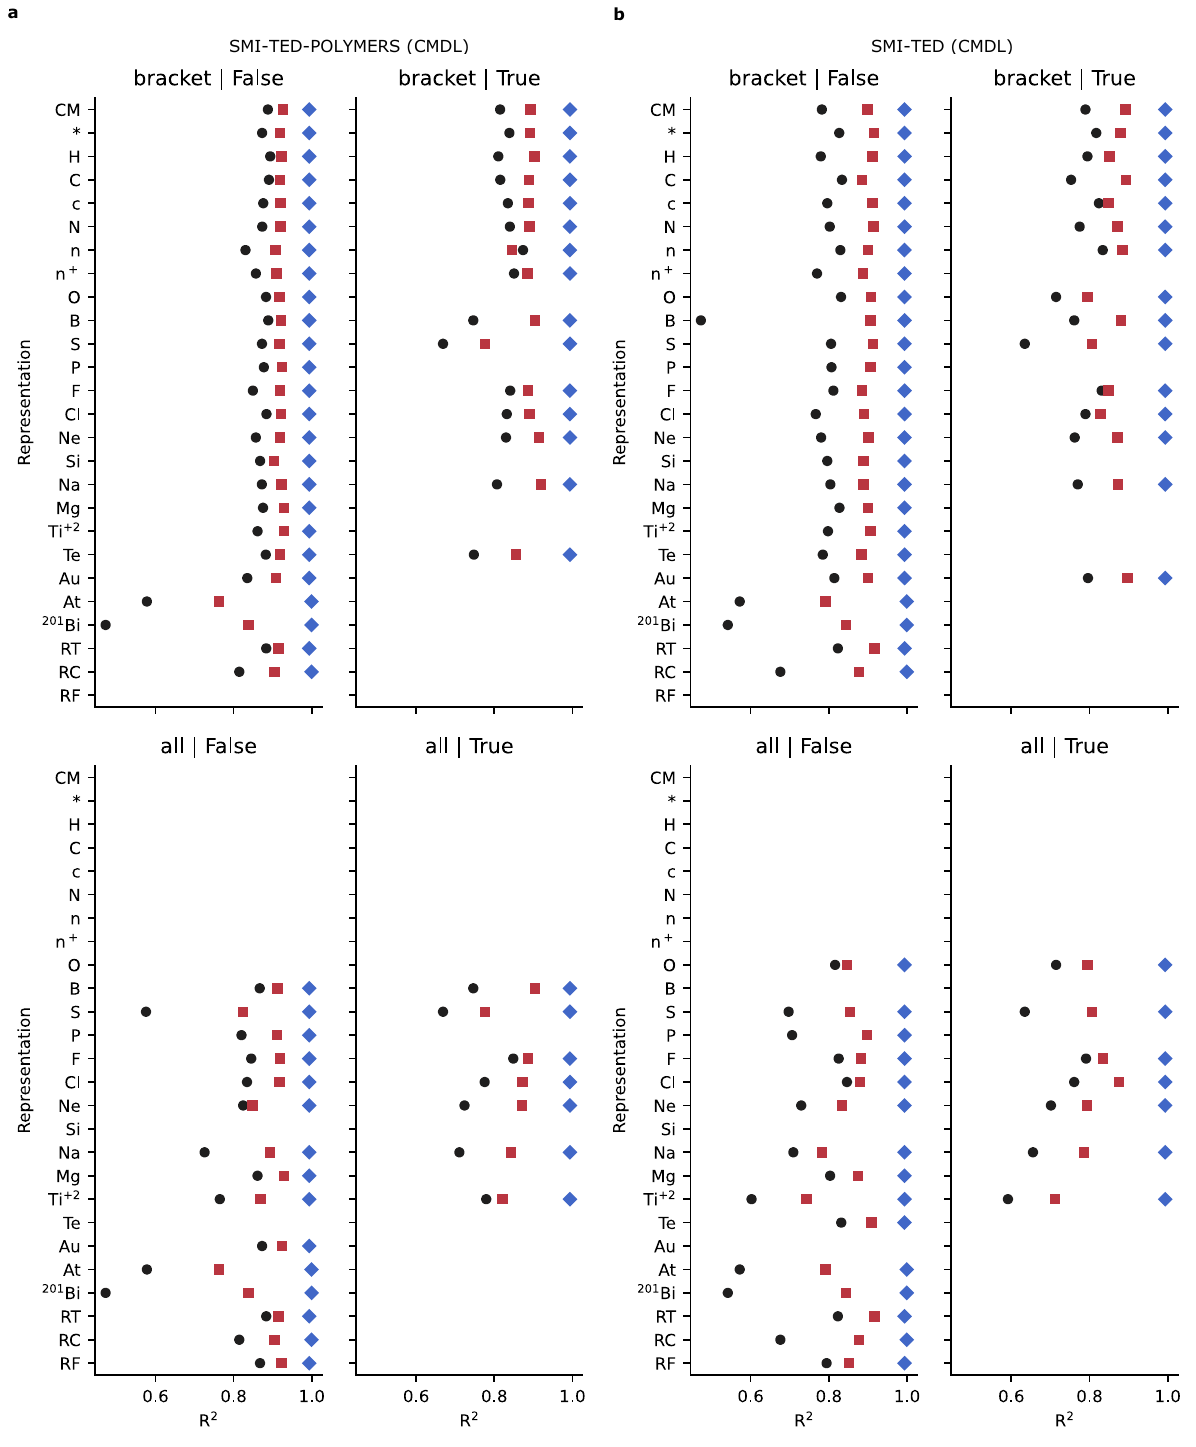}
\caption{Point plots for T\textsubscript{g}-II benchmark experiments of R\textsuperscript{2} using the base random train, valid, and test splits for SMI-TED-POLYMER (\textbf{a}) and SMI-TED (\textbf{b}) models fine-tuned with CPG.}\label{acs_ami_tg_token_point_cmdl_r2}
\end{figure}

\begin{figure}[H]
\centering
\includegraphics[width=1\textwidth]{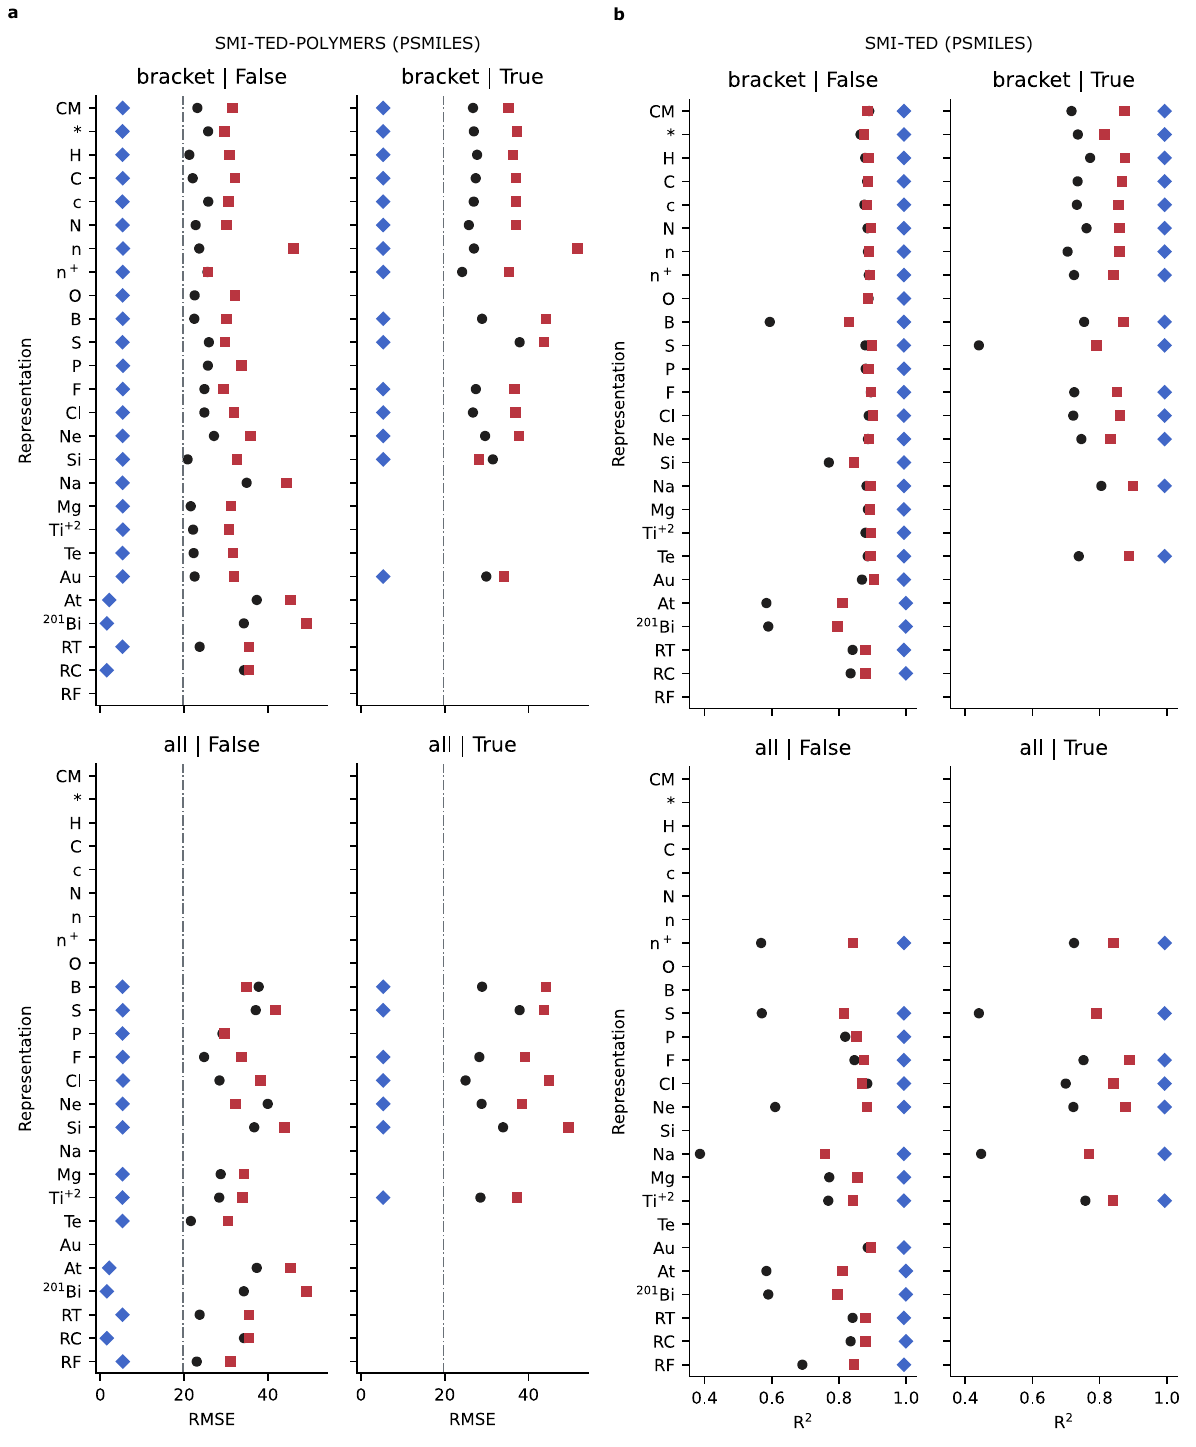}
\caption{Point plots for T\textsubscript{g}-II benchmark experiments of RMSE using the base random train, valid, and test splits for SMI-TED-POLYMER (\textbf{a}) and SMI-TED (\textbf{b}) models fine-tuned with PSMILES.}\label{acs_ami_tg_token_point_psmiles_rmse}
\end{figure}

\begin{figure}[H]
\centering
\includegraphics[width=1\textwidth]{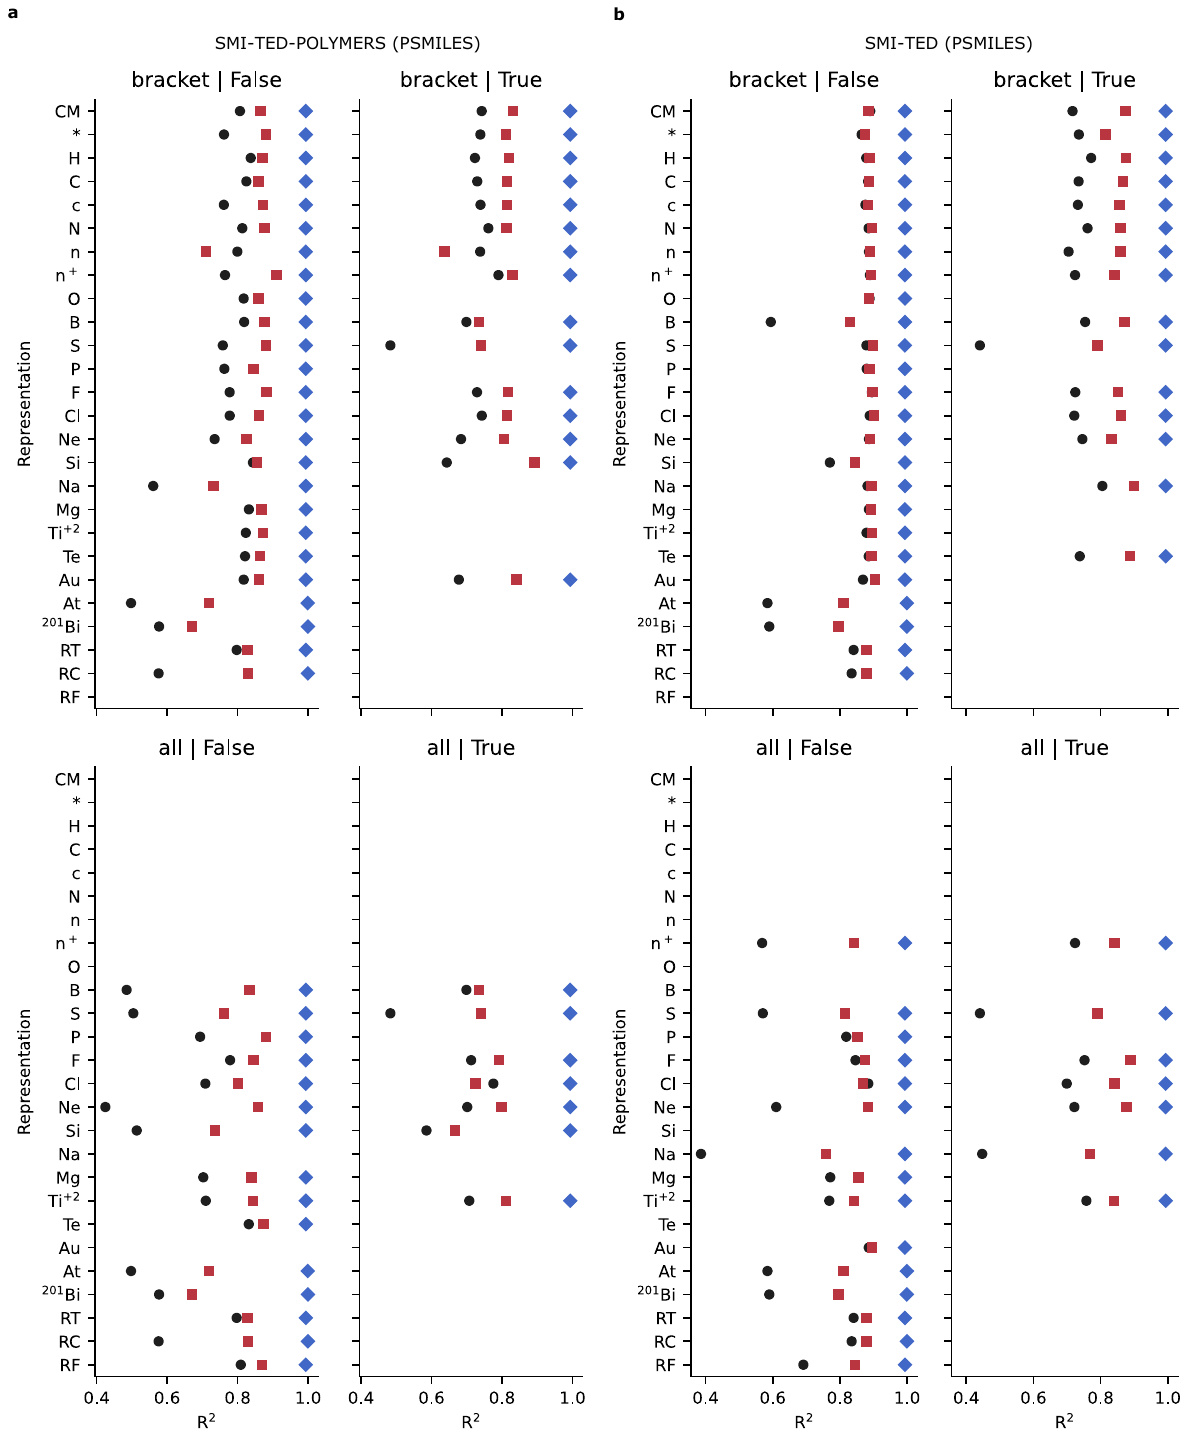}
\caption{Point plots for T\textsubscript{g}-II benchmark experiments of R\textsuperscript{2} using the base random train, valid, and test splits for SMI-TED-POLYMER (\textbf{a}) and SMI-TED (\textbf{b}) models fine-tuned with PSMILES.}\label{acs_ami_tg_token_point_psmiles_r2}
\end{figure}

\subsubsection{CO\textsubscript{2} Gas Permeability CV Scores}\label{cv_netl_co2}

\begin{figure}[H]
\centering
\includegraphics[width=1\textwidth]{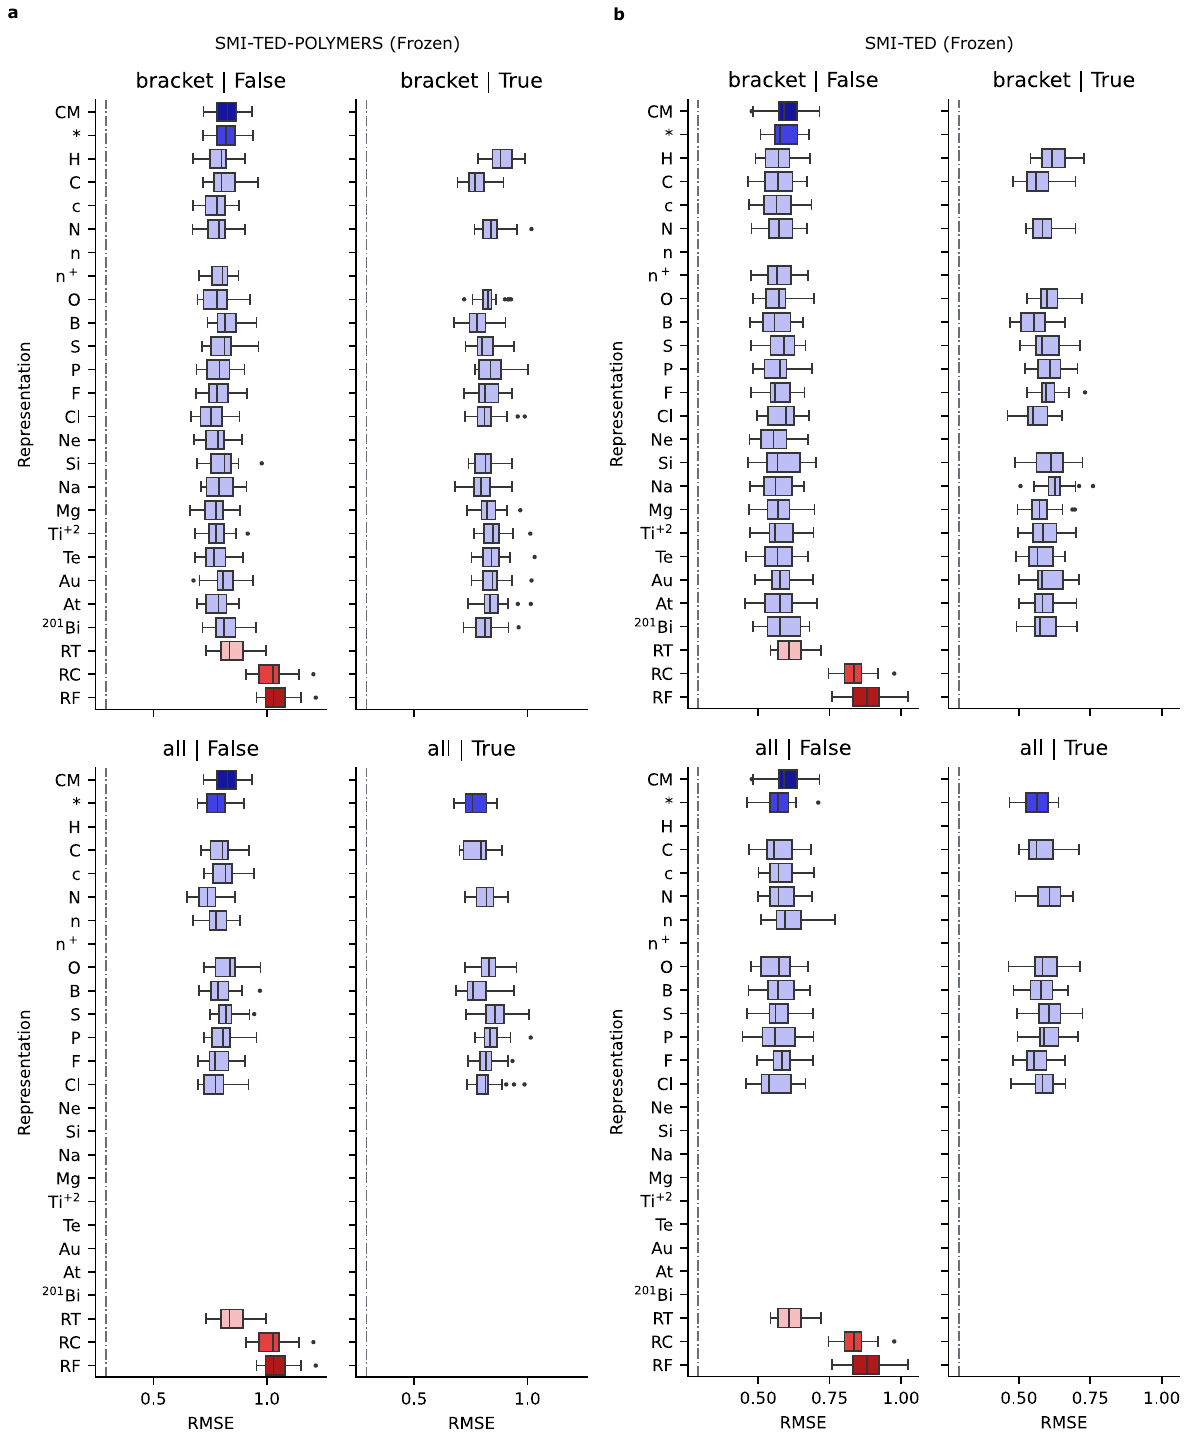}
\caption{Box plots for CO\textsubscript{2} gas permeability repeated cross-validation experiments for SMI-TED-POLYMER (\textbf{a}) and SMI-TED (\textbf{b}) models with frozen weights.}\label{netl_co2_token_box_frozen}
\end{figure}

\begin{figure}[H]
\centering
\includegraphics[width=1\textwidth]{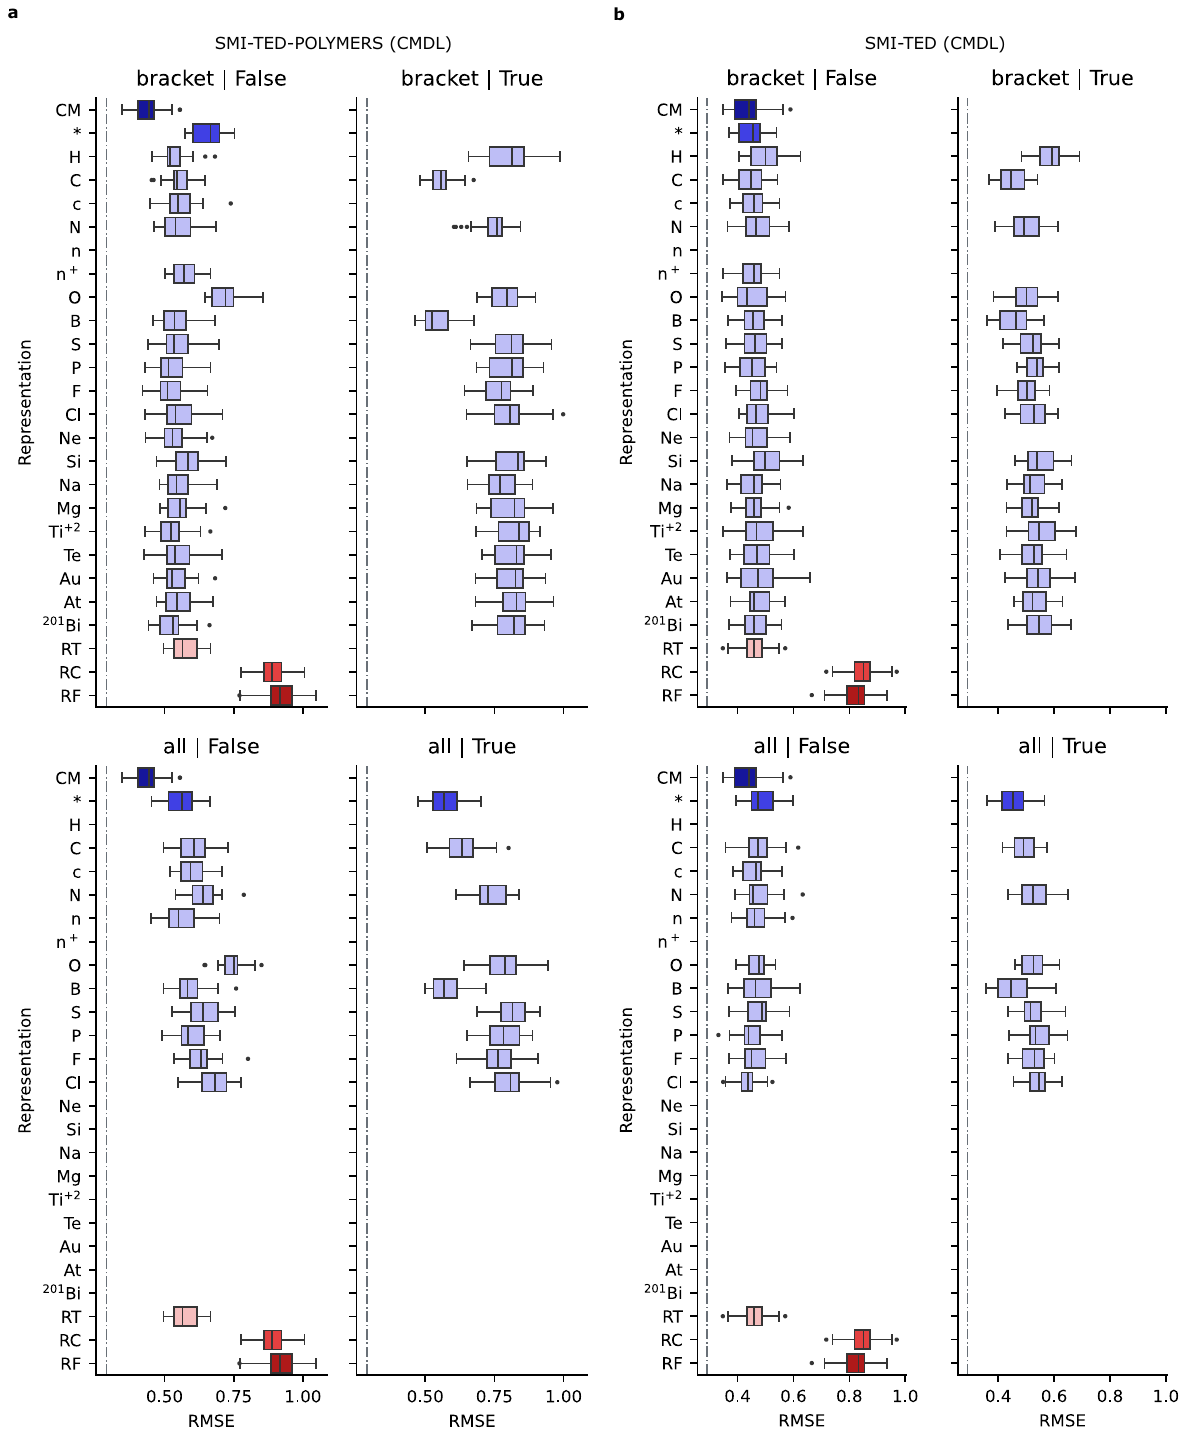}
\caption{Box plots for CO\textsubscript{2} gas permeability repeated cross-validation experiments for SMI-TED-POLYMER (\textbf{a}) and SMI-TED (\textbf{b}) models fine-tuned with the CPG polymer graphs.}\label{netl_co2_token_box_cmdl}
\end{figure}

\begin{figure}[H]
\centering
\includegraphics[width=1\textwidth]{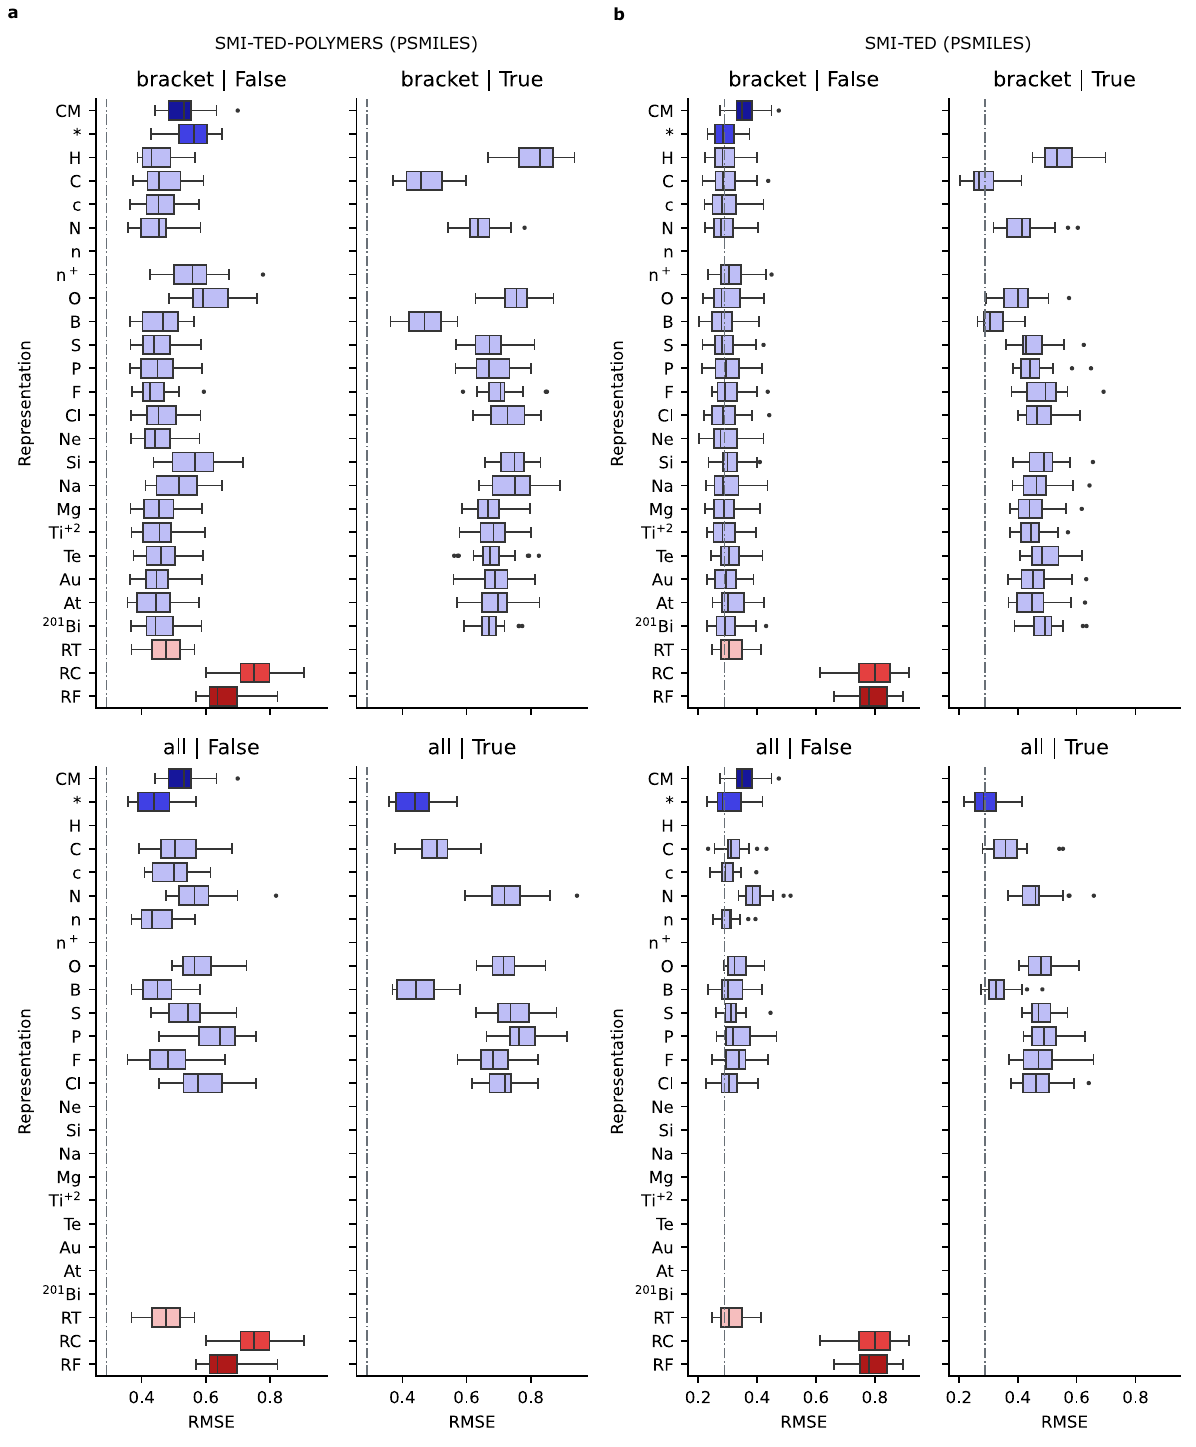}
\caption{Box plots for CO\textsubscript{2} gas permeability repeated cross-validation experiments for SMI-TED-POLYMER (\textbf{a}) and SMI-TED (\textbf{b}) models fine-tuned with PSMILES.}\label{netl_co2_token_box_psmiles}
\end{figure}

\subsubsection{CO\textsubscript{2} Gas Permeability Random Split Scores}\label{rand_netl_co2}

\begin{figure}[H]
\centering
\includegraphics[width=1\textwidth]{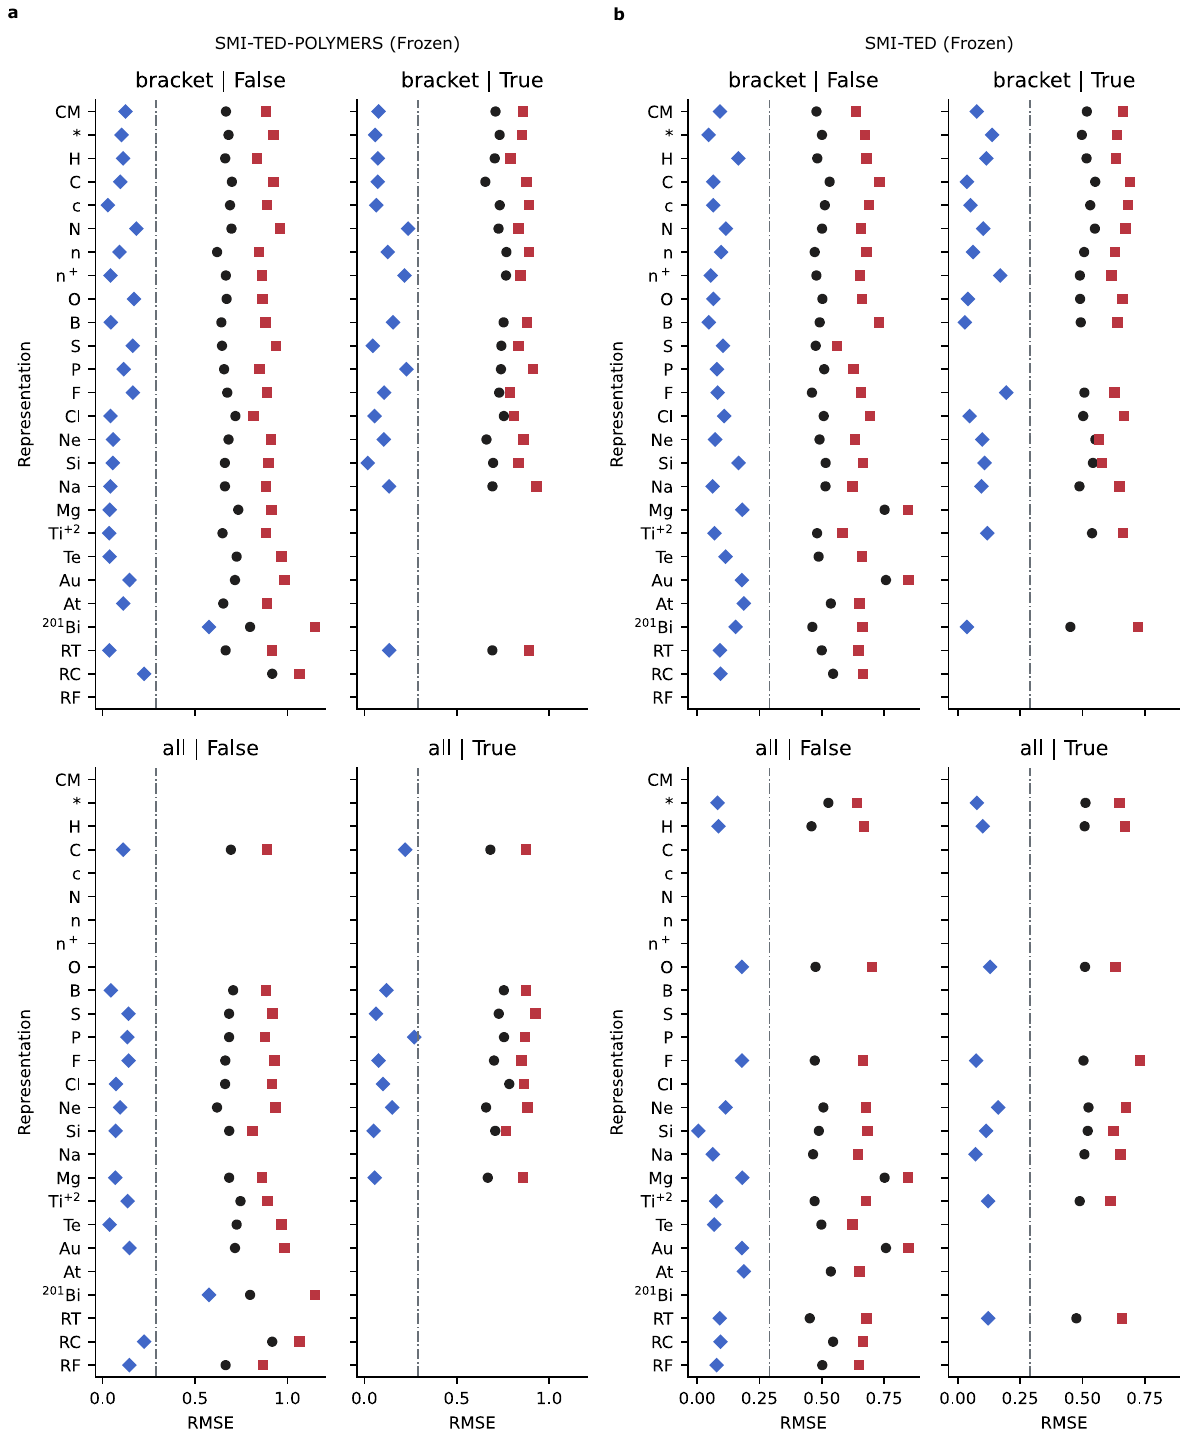}
\caption{Point plots for CO\textsubscript{2} gas permeability benchmark experiments of RMSE using the base random train, valid, and test splits for SMI-TED-POLYMER (\textbf{a}) and SMI-TED (\textbf{b}) models with frozen weights.}\label{netl_co2_token_point_frozen_rmse}
\end{figure}

\begin{figure}[H]
\centering
\includegraphics[width=1\textwidth]{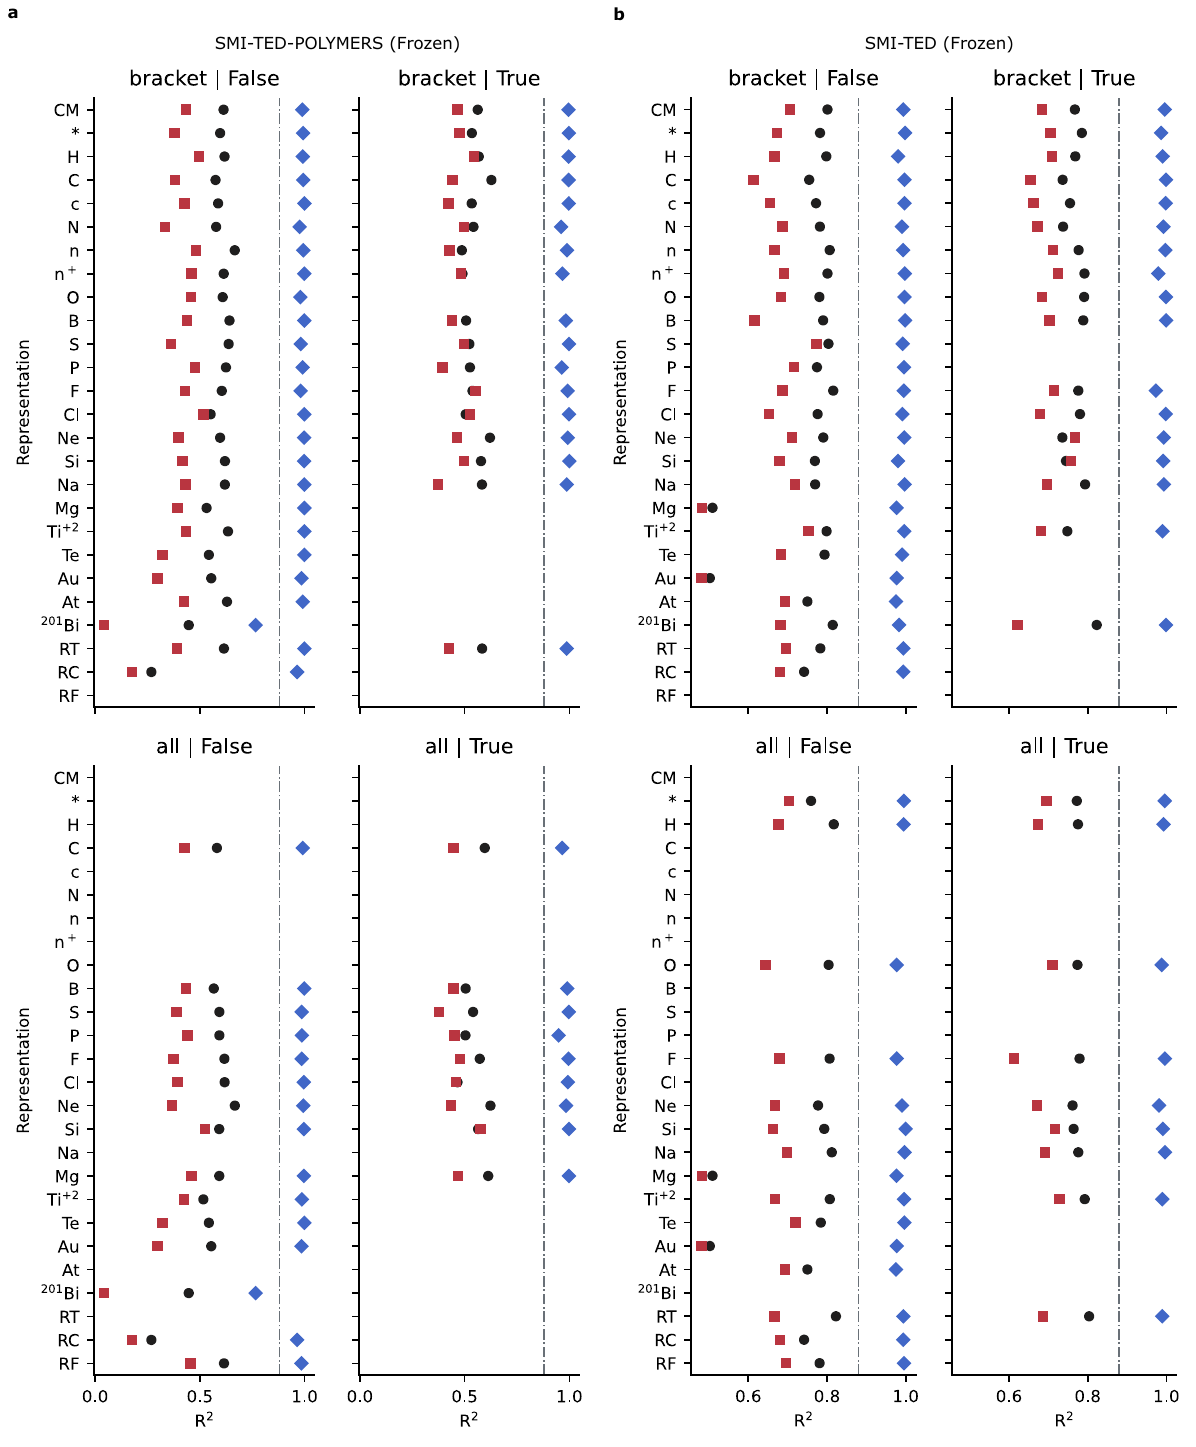}
\caption{Point plots for CO\textsubscript{2} gas permeability benchmark experiments of R\textsuperscript{2} using the base random train, valid, and test splits for SMI-TED-POLYMER (\textbf{a}) and SMI-TED (\textbf{b}) models with frozen weights.}\label{netl_co2_token_point_frozen_r2}
\end{figure}

\begin{figure}[H]
\centering
\includegraphics[width=1\textwidth]{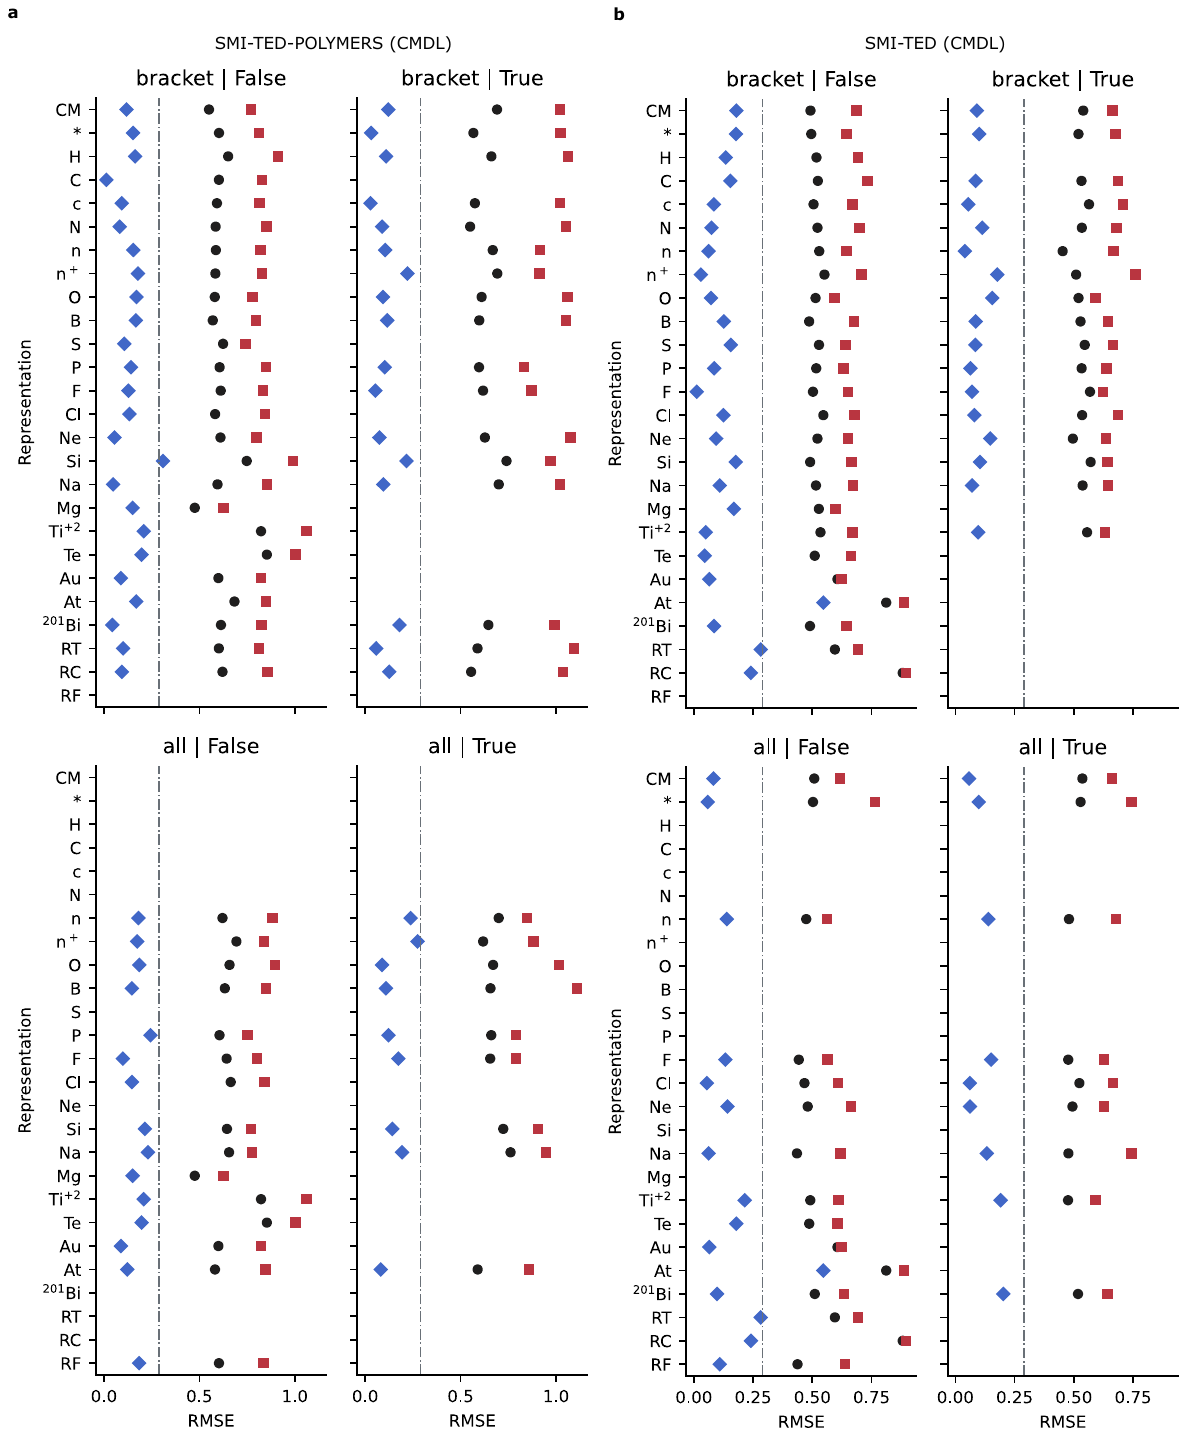}
\caption{Point plots for CO\textsubscript{2} gas permeability benchmark experiments of RMSE using the base random train, valid, and test splits for SMI-TED-POLYMER (\textbf{a}) and SMI-TED (\textbf{b}) models fine-tuned using the CPG representation.}\label{netl_co2_token_point_cmdl_rmse}
\end{figure}

\begin{figure}
\centering
\includegraphics[width=1\textwidth]{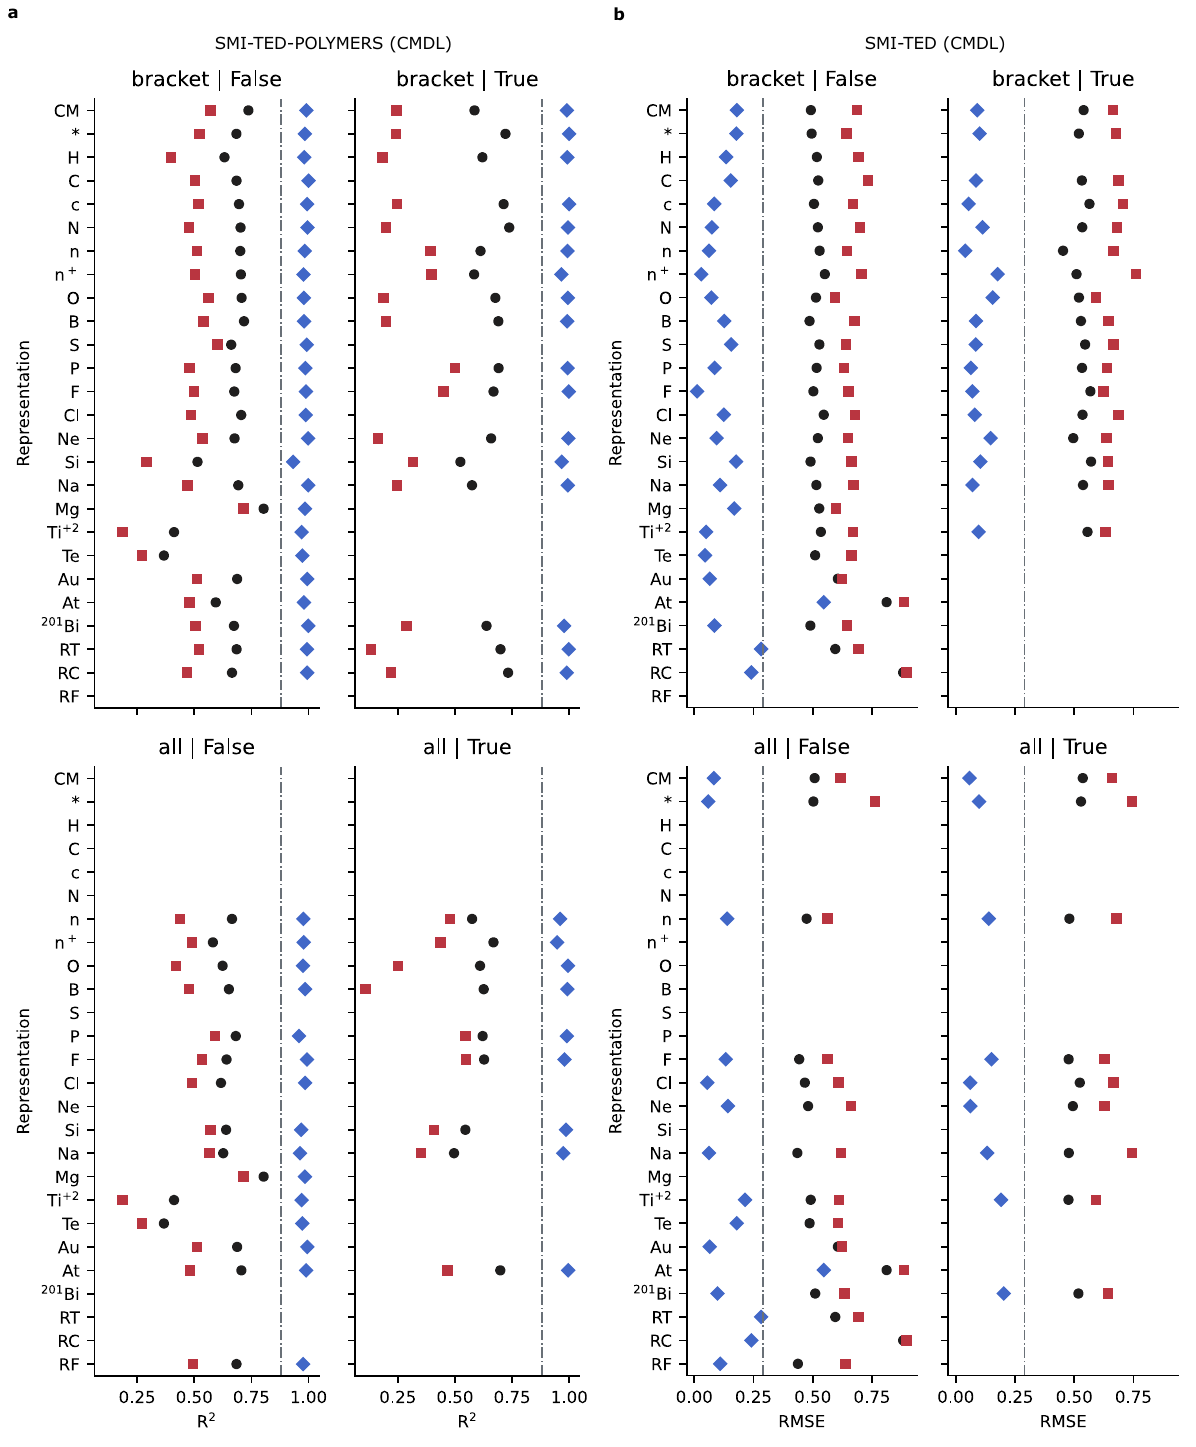}
\caption{Point plots for CO\textsubscript{2} gas permeability benchmark experiments of R\textsuperscript{2} using the base random train, valid, and test splits for SMI-TED-POLYMER (\textbf{a}) and SMI-TED (\textbf{b}) models fine-tuned using the CPG representation.}\label{netl_co2_token_point_cmdl_r2}
\end{figure}

\begin{figure}[H]
\centering
\includegraphics[width=1\textwidth]{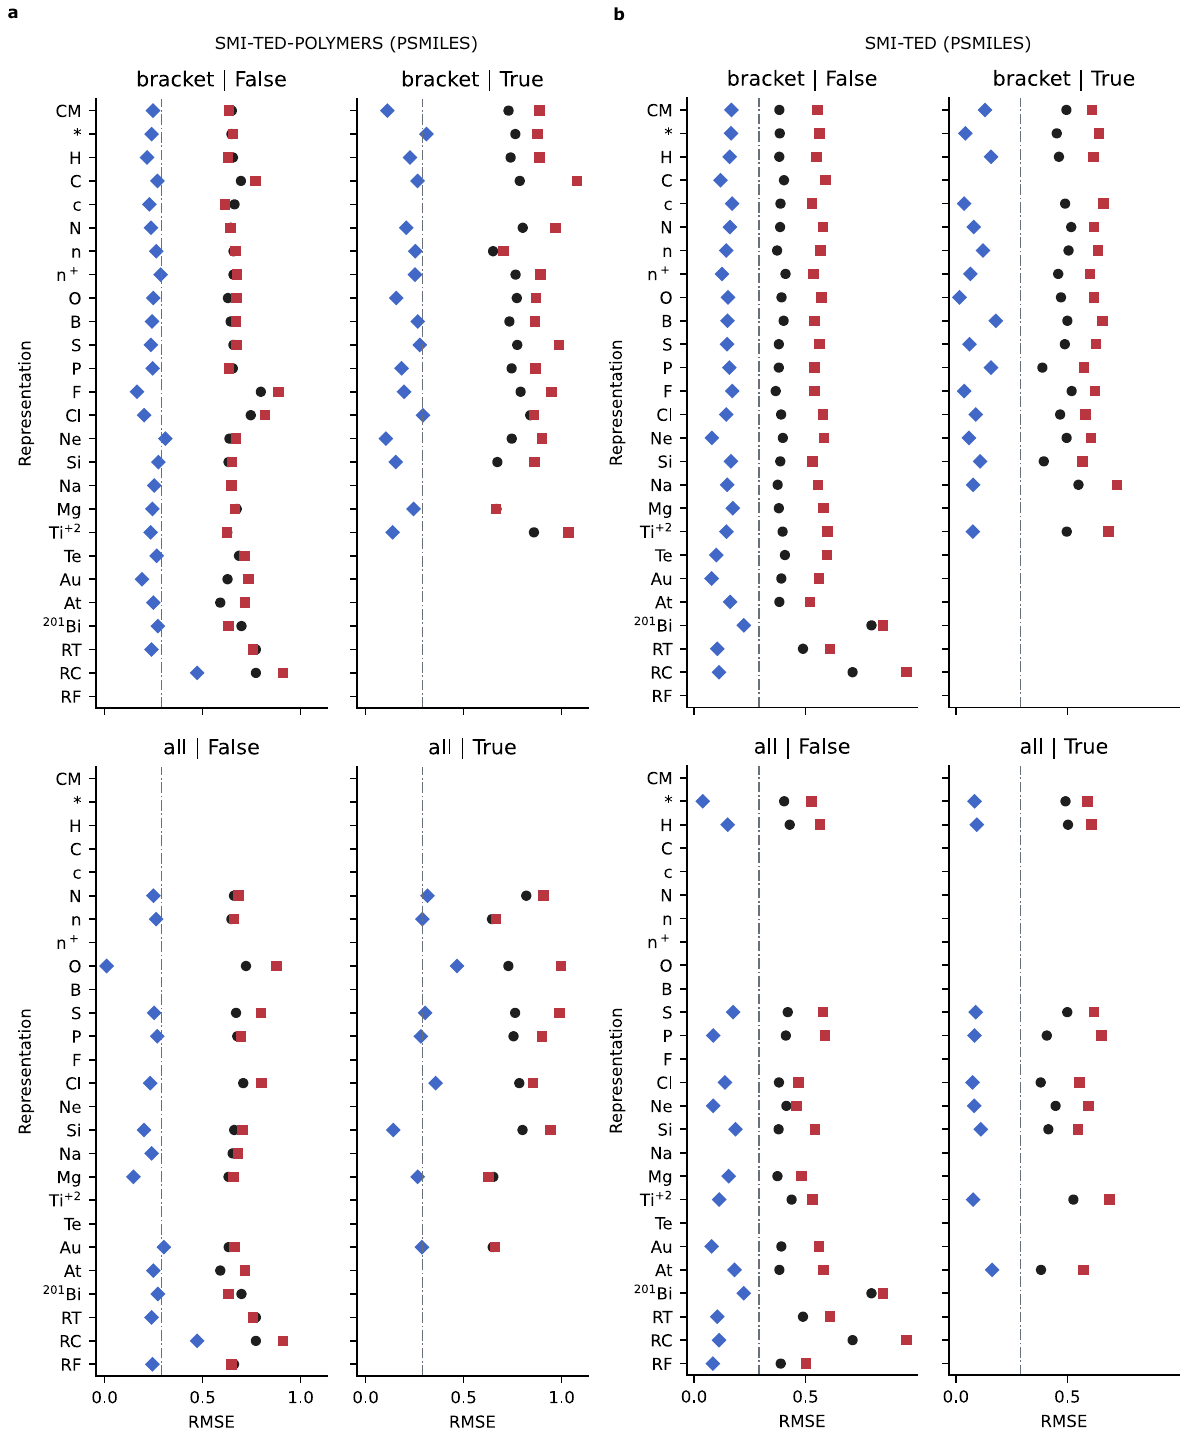}
\caption{Point plots for CO\textsubscript{2} gas permeability benchmark experiments of RMSE using the base random train, valid, and test splits for SMI-TED-POLYMER (\textbf{a}) and SMI-TED (\textbf{b}) models fine-tuned using PSMILES.}\label{netl_co2_token_point_psmiles_rmse}
\end{figure}

\begin{figure}[H]
\centering
\includegraphics[width=1\textwidth]{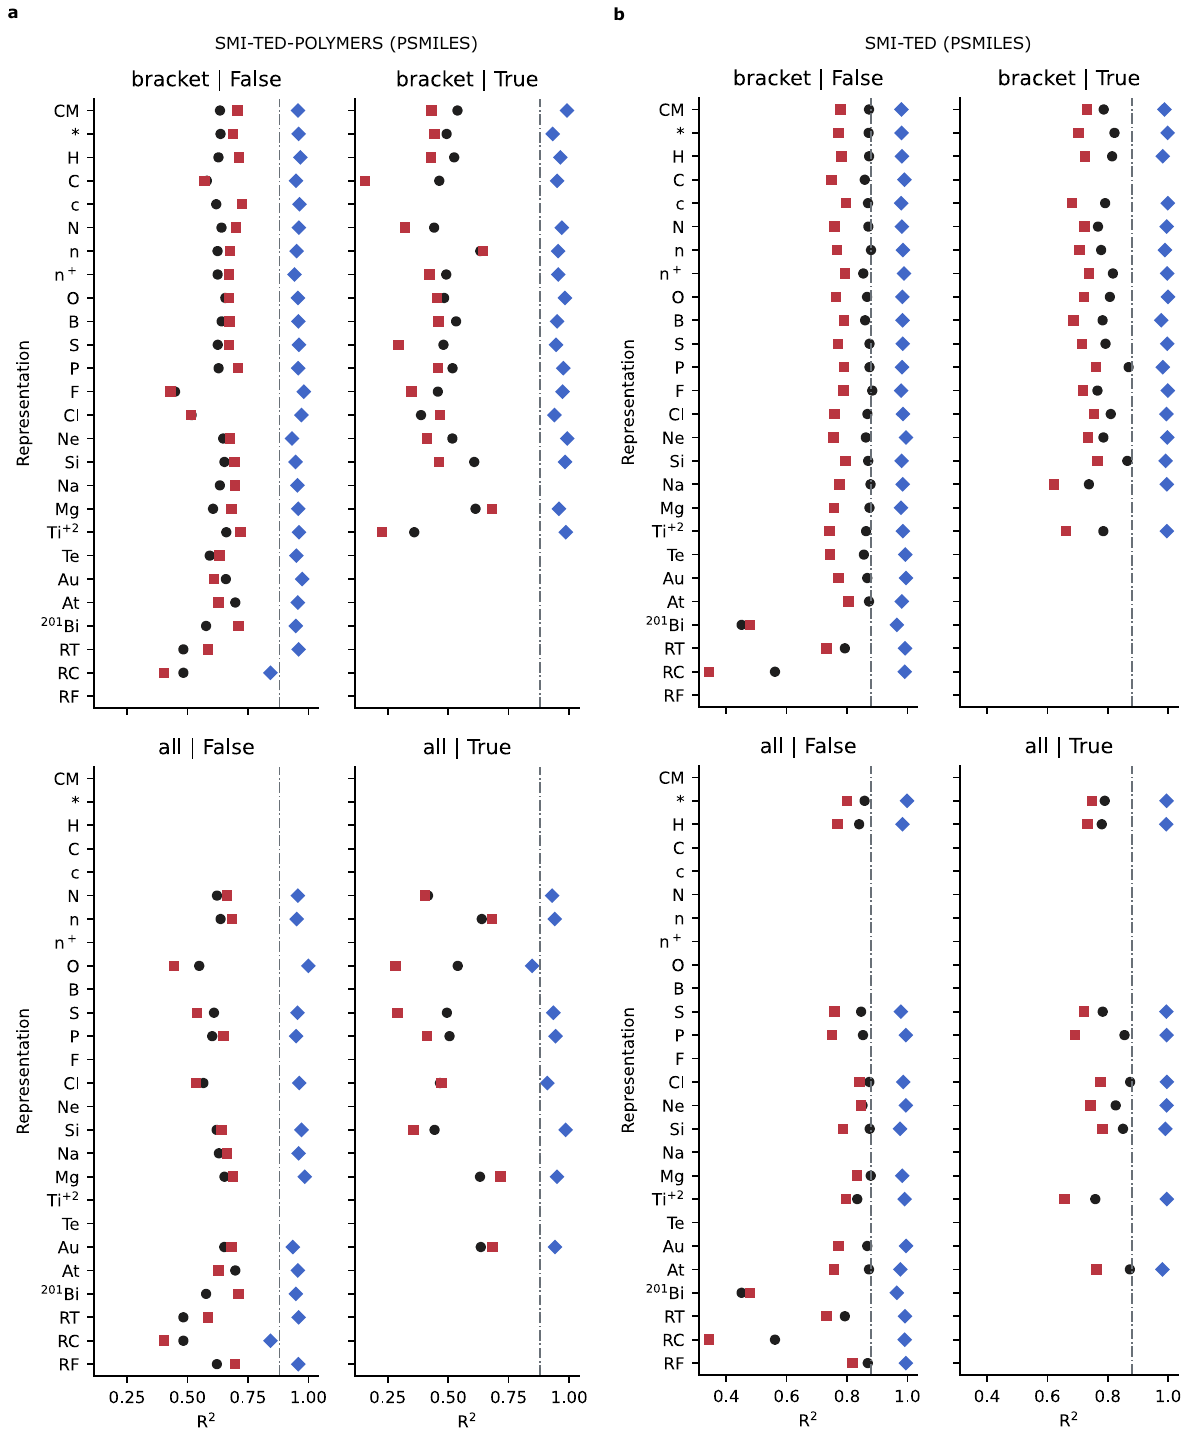}
\caption{Point plots for CO\textsubscript{2} gas permeability benchmark experiments of R\textsuperscript{2} using the base random train, valid, and test splits for SMI-TED-POLYMER (\textbf{a}) and SMI-TED (\textbf{b}) models fine-tuned using PSMILES.}\label{netl_co2_token_point_psmiles_r2}
\end{figure}

\subsubsection{N\textsubscript{2} Gas Permeability CV Scores}\label{cv_netl_n2}

\begin{figure}[H]
\centering
\includegraphics[width=1\textwidth]{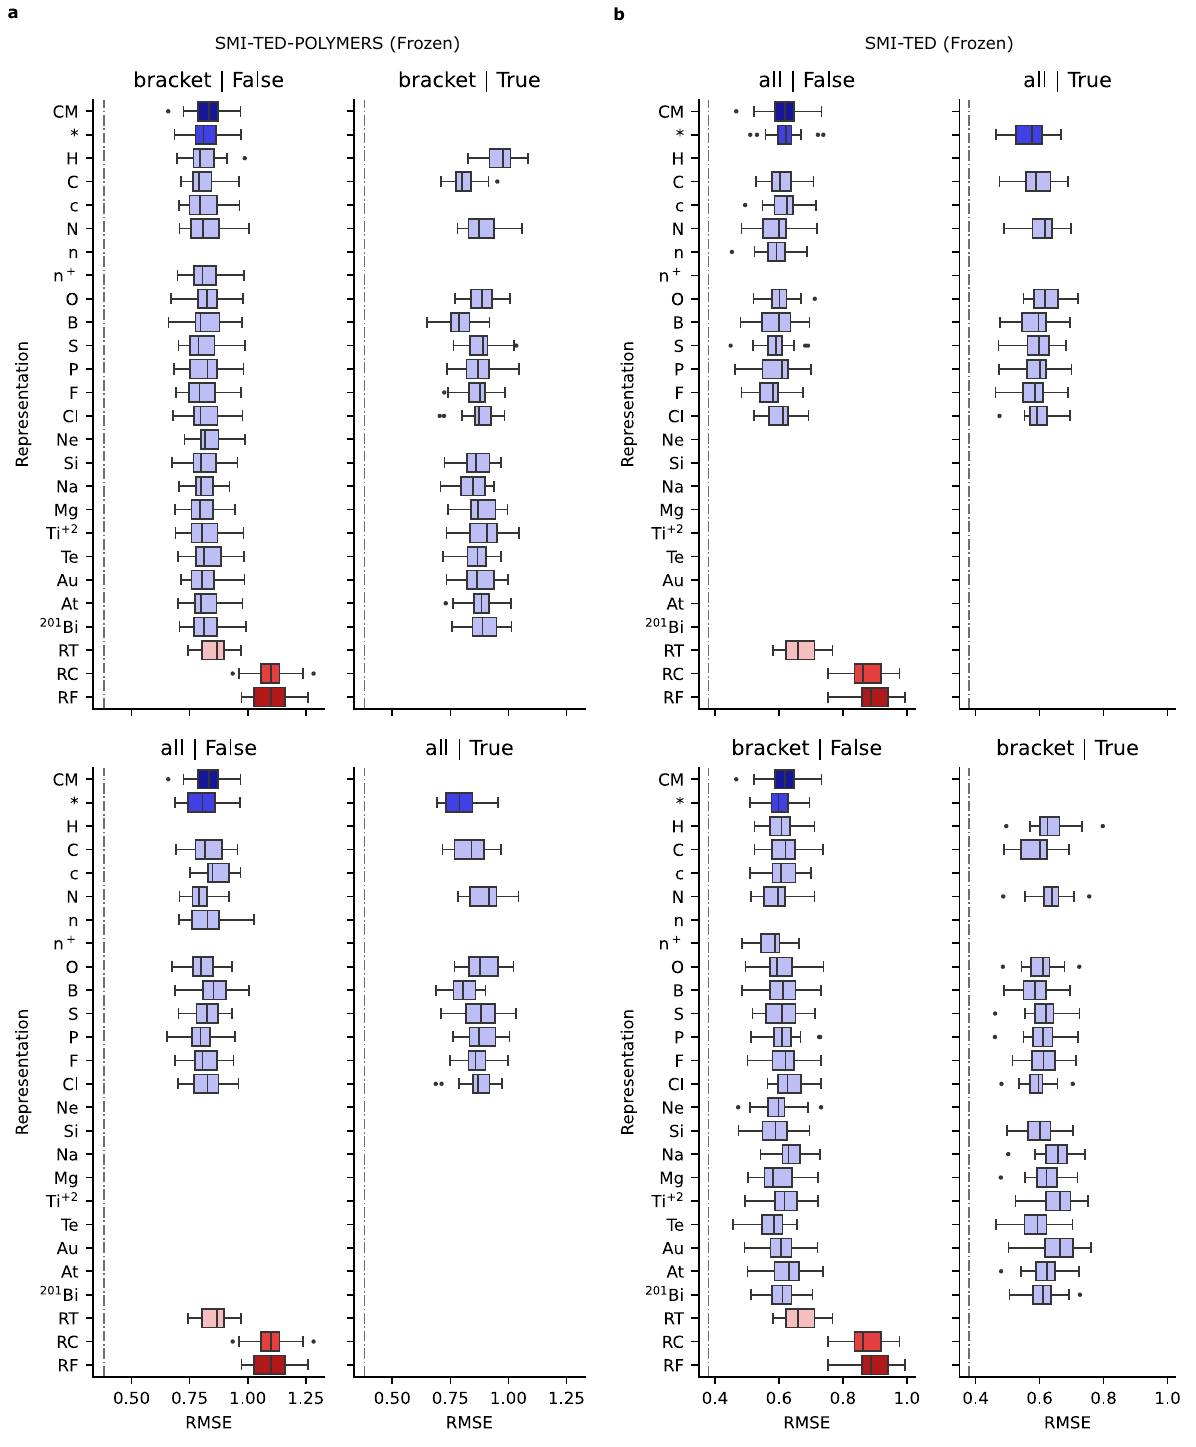}
\caption{Box plots for N\textsubscript{2} gas permeability repeated cross-validation experiments for SMI-TED-POLYMER (\textbf{a}) and SMI-TED (\textbf{b}) models with frozen weights.}\label{netl_n2_token_box_frozen}
\end{figure}

\begin{figure}[H]
\centering
\includegraphics[width=1\textwidth]{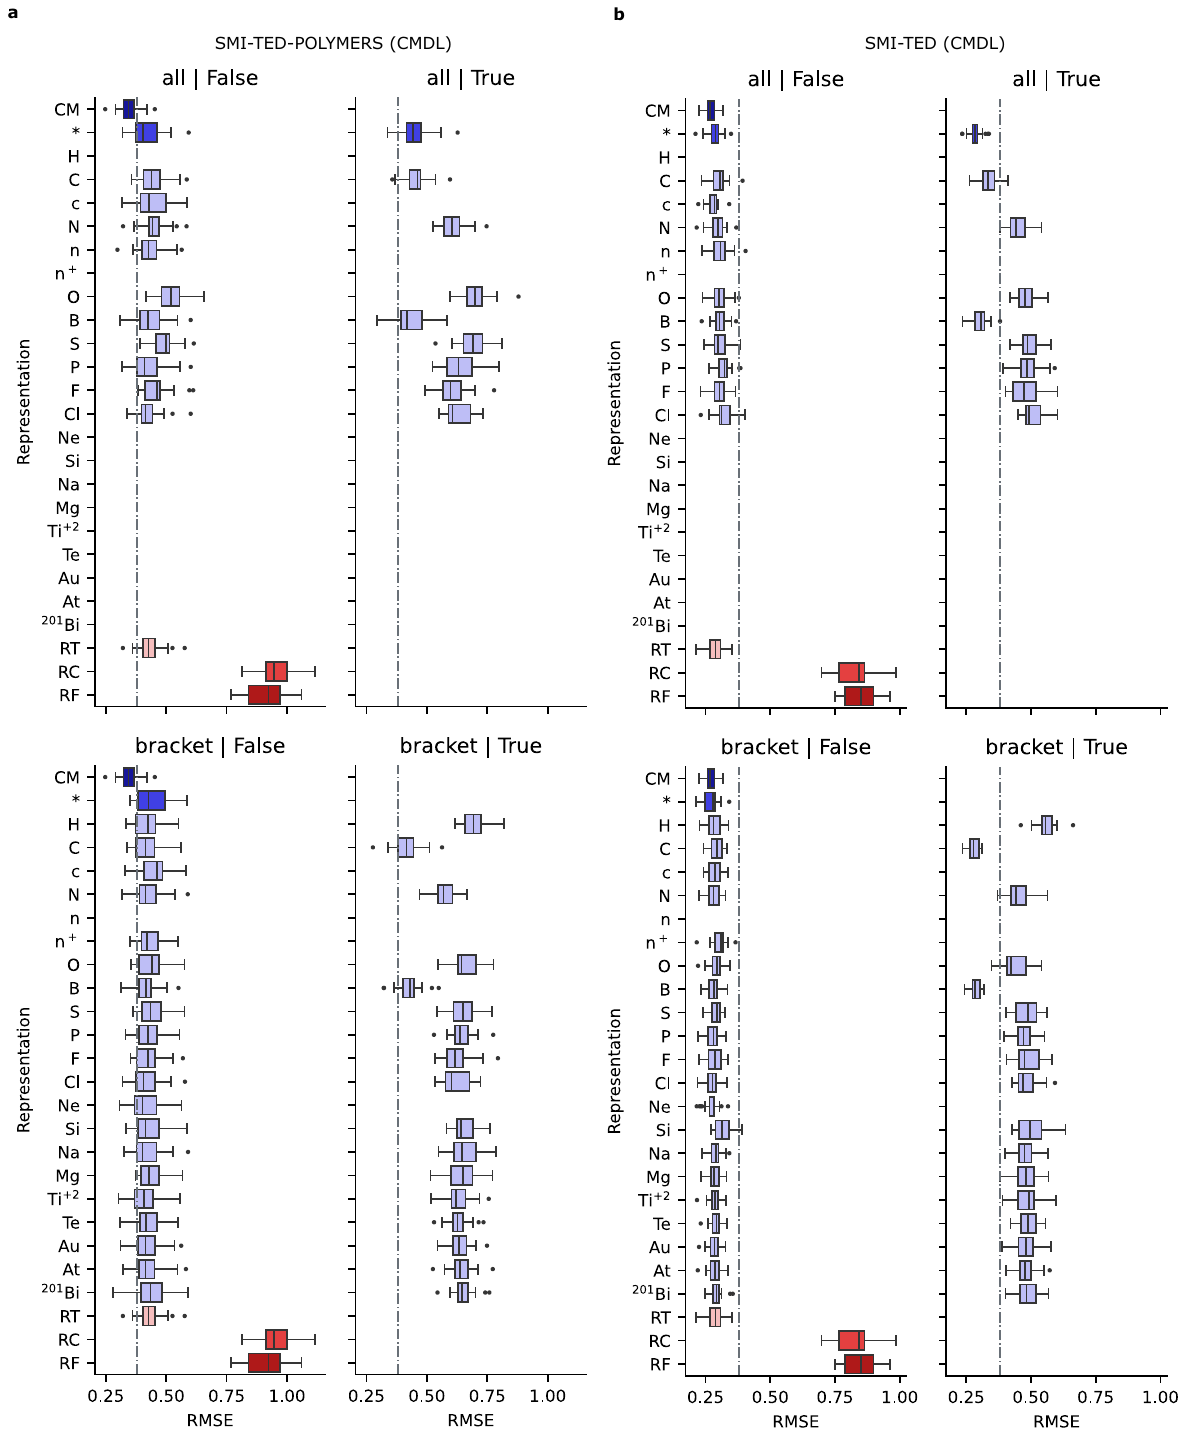}
\caption{Box plots for N\textsubscript{2} gas permeability repeated cross-validation experiments for SMI-TED-POLYMER (\textbf{a}) and SMI-TED (\textbf{b}) models fine-tuned with the CPG polymer graphs.}\label{netl_n2_token_box_cmdl}
\end{figure}

\begin{figure}[H]
\centering
\includegraphics[width=1\textwidth]{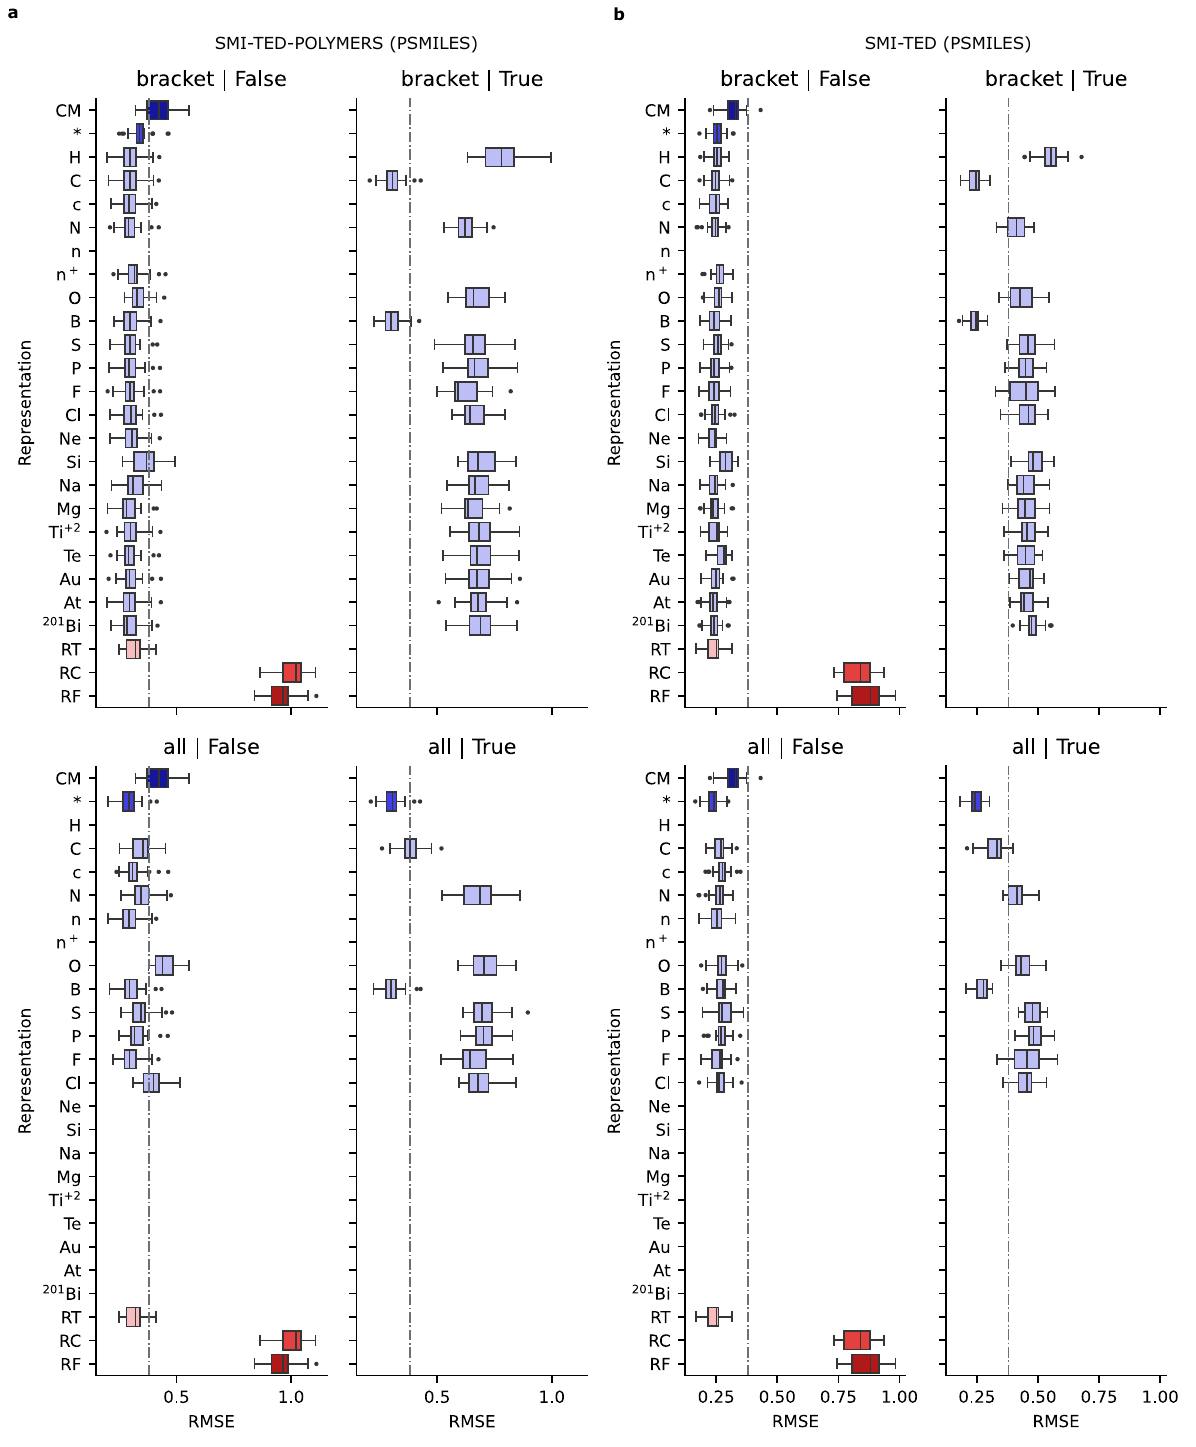}
\caption{Box plots for N\textsubscript{2} gas permeability repeated cross-validation experiments for SMI-TED-POLYMER (\textbf{a}) and SMI-TED (\textbf{b}) models fine-tuned with PSMILES.}\label{netl_n2_token_box_psmiles}
\end{figure}

\subsubsection{N\textsubscript{2} Gas Permeability Random Split Scores}\label{rand_netl_n2}

\begin{figure}[H]
\centering
\includegraphics[width=1\textwidth]{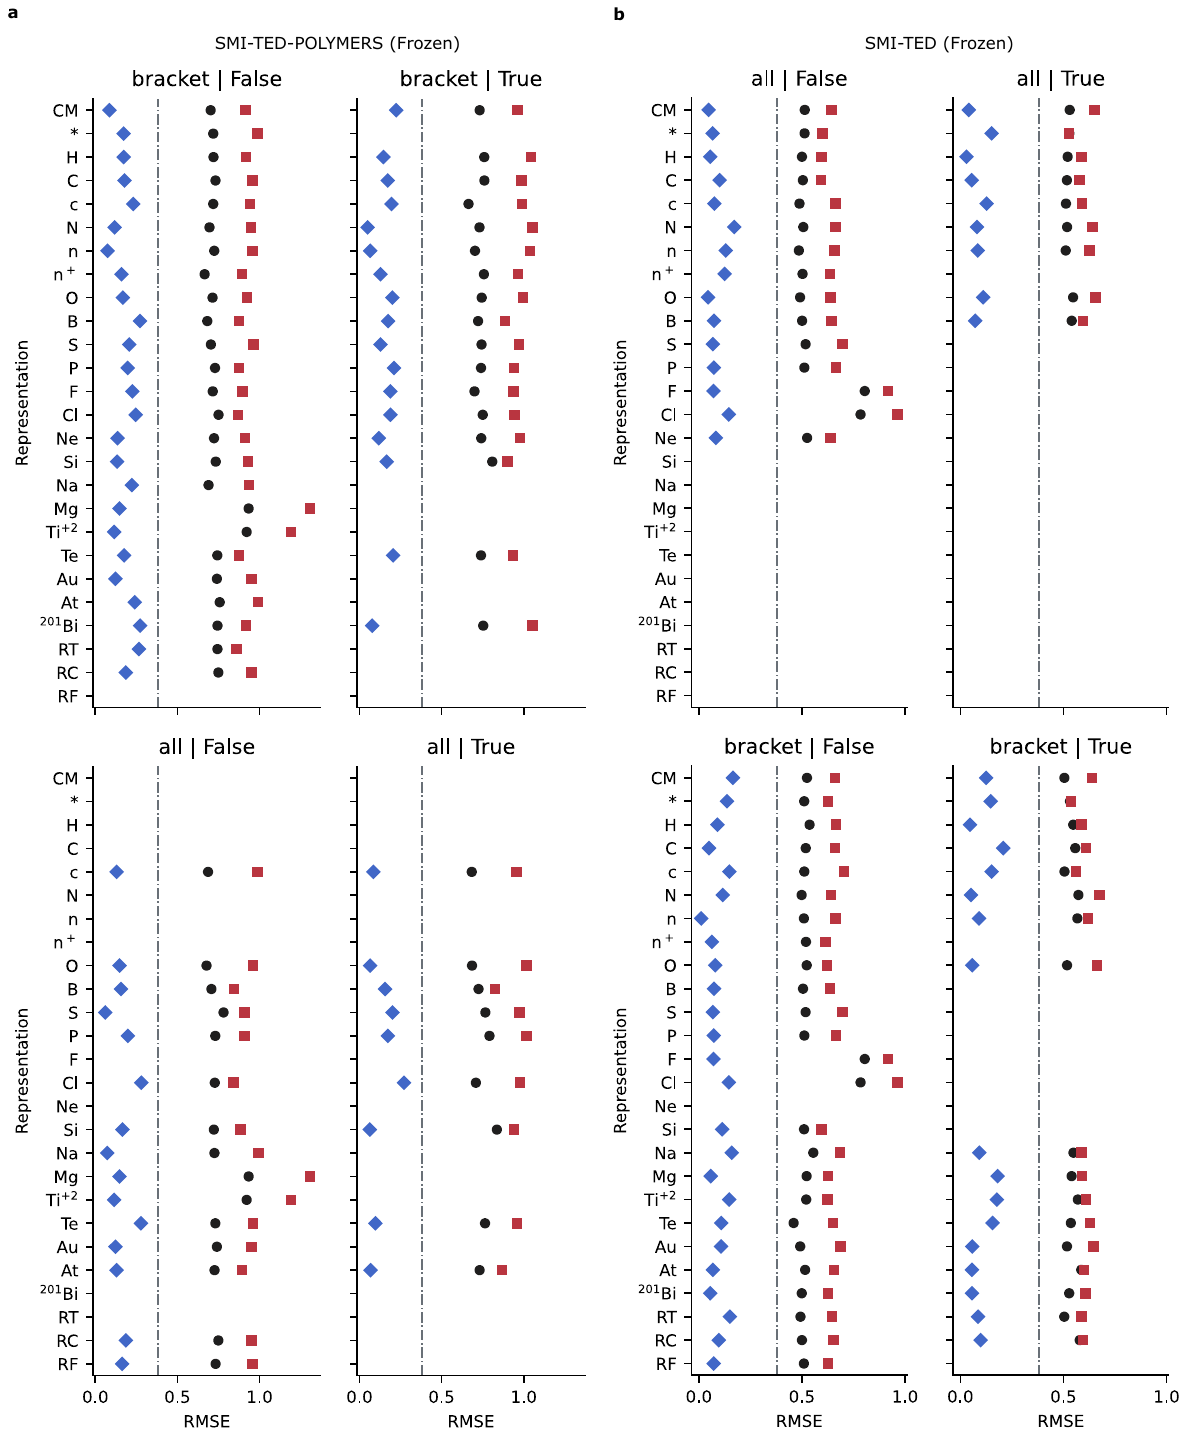}
\caption{Point plots for N\textsubscript{2} gas permeability benchmark experiments of RMSE using the base random train, valid, and test splits for SMI-TED-POLYMER (\textbf{a}) and SMI-TED (\textbf{b}) models with frozen weights.}\label{netl_n2_token_point_frozen_rmse}
\end{figure}

\begin{figure}[H]
\centering
\includegraphics[width=1\textwidth]{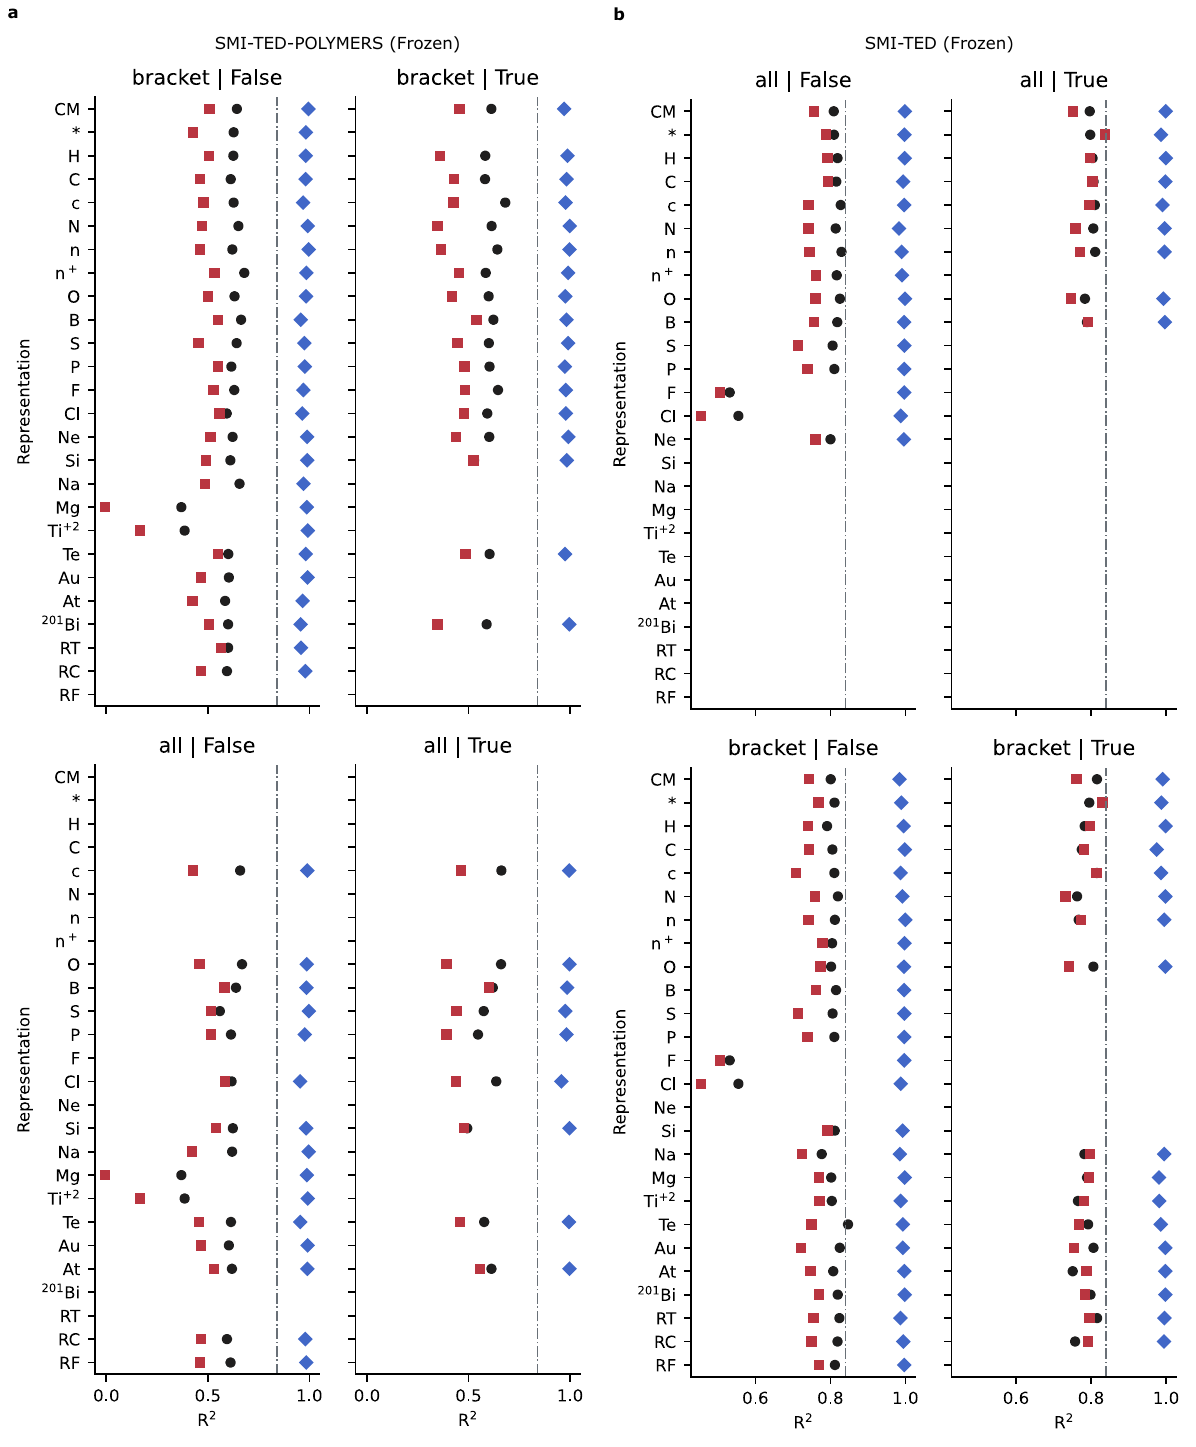}
\caption{Point plots for N\textsubscript{2} gas permeability benchmark experiments of R\textsuperscript{2} using the base random train, valid, and test splits for SMI-TED-POLYMER (\textbf{a}) and SMI-TED (\textbf{b}) models with frozen weights.}\label{netl_n2_token_point_frozen_r2}
\end{figure}

\begin{figure}[H]
\centering
\includegraphics[width=1\textwidth]{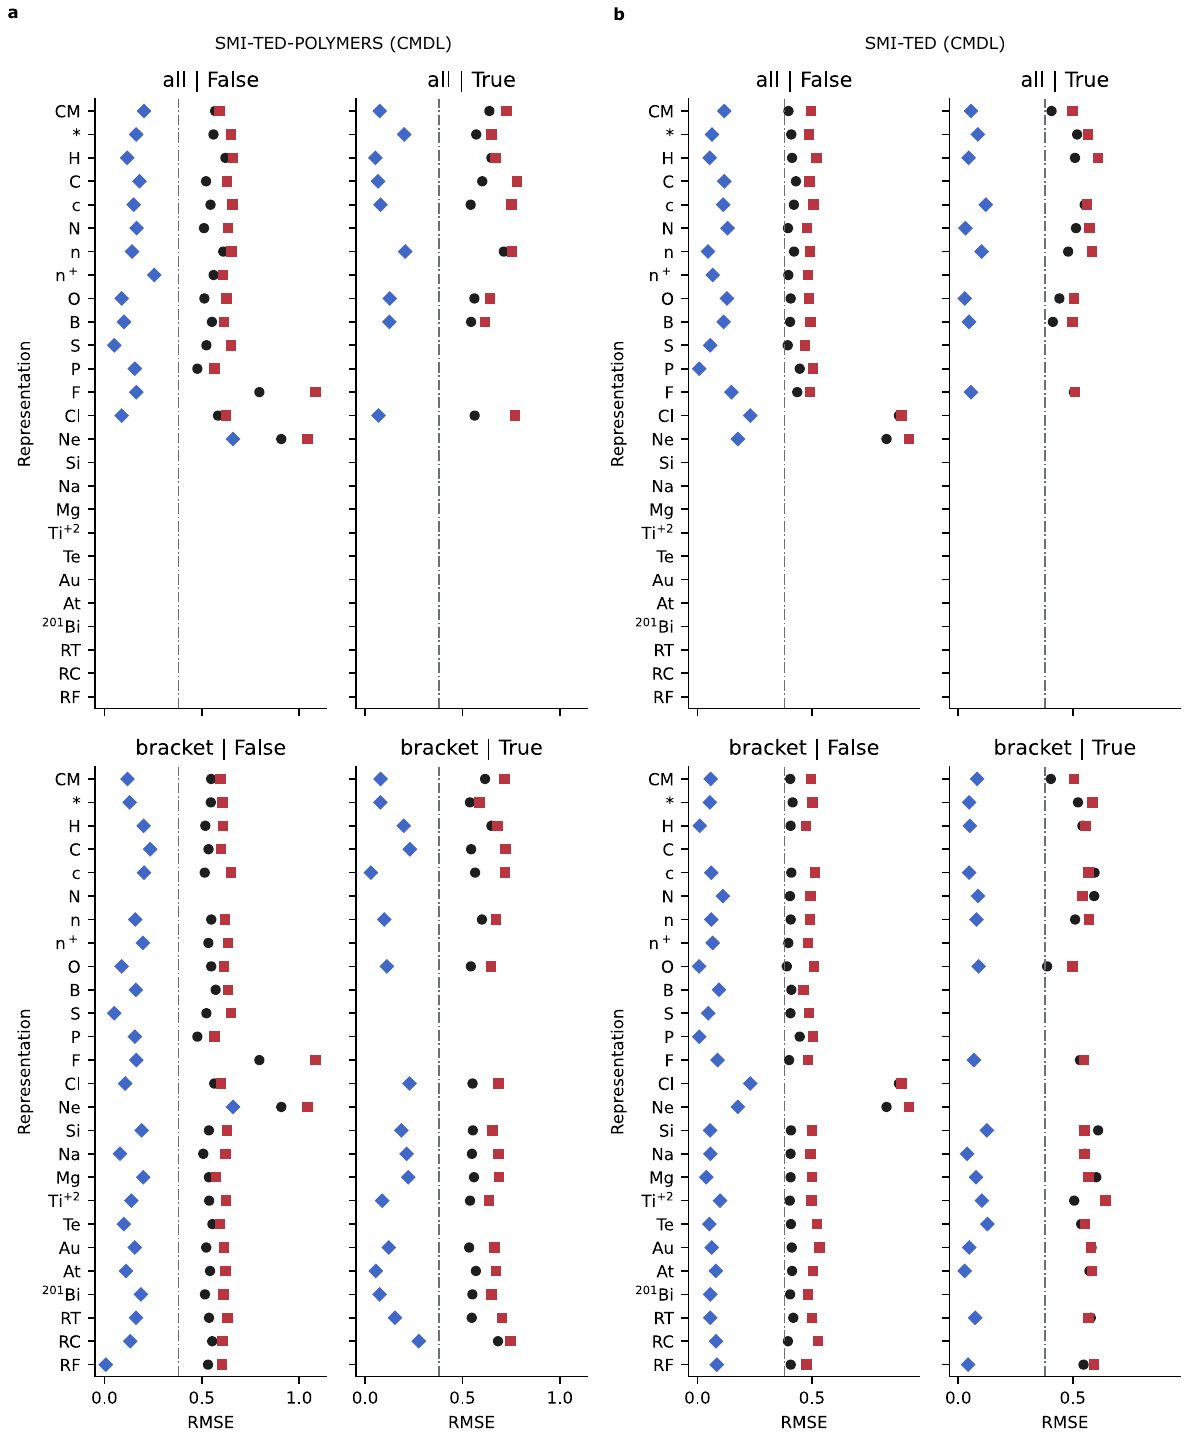}
\caption{Point plots for N\textsubscript{2} gas permeability benchmark experiments of RMSE using the base random train, valid, and test splits for SMI-TED-POLYMER (\textbf{a}) and SMI-TED (\textbf{b}) models fine-tuned using the CPG representation.}\label{netl_n2_token_point_cmdl_rmse}
\end{figure}

\begin{figure}
\centering
\includegraphics[width=1\textwidth]{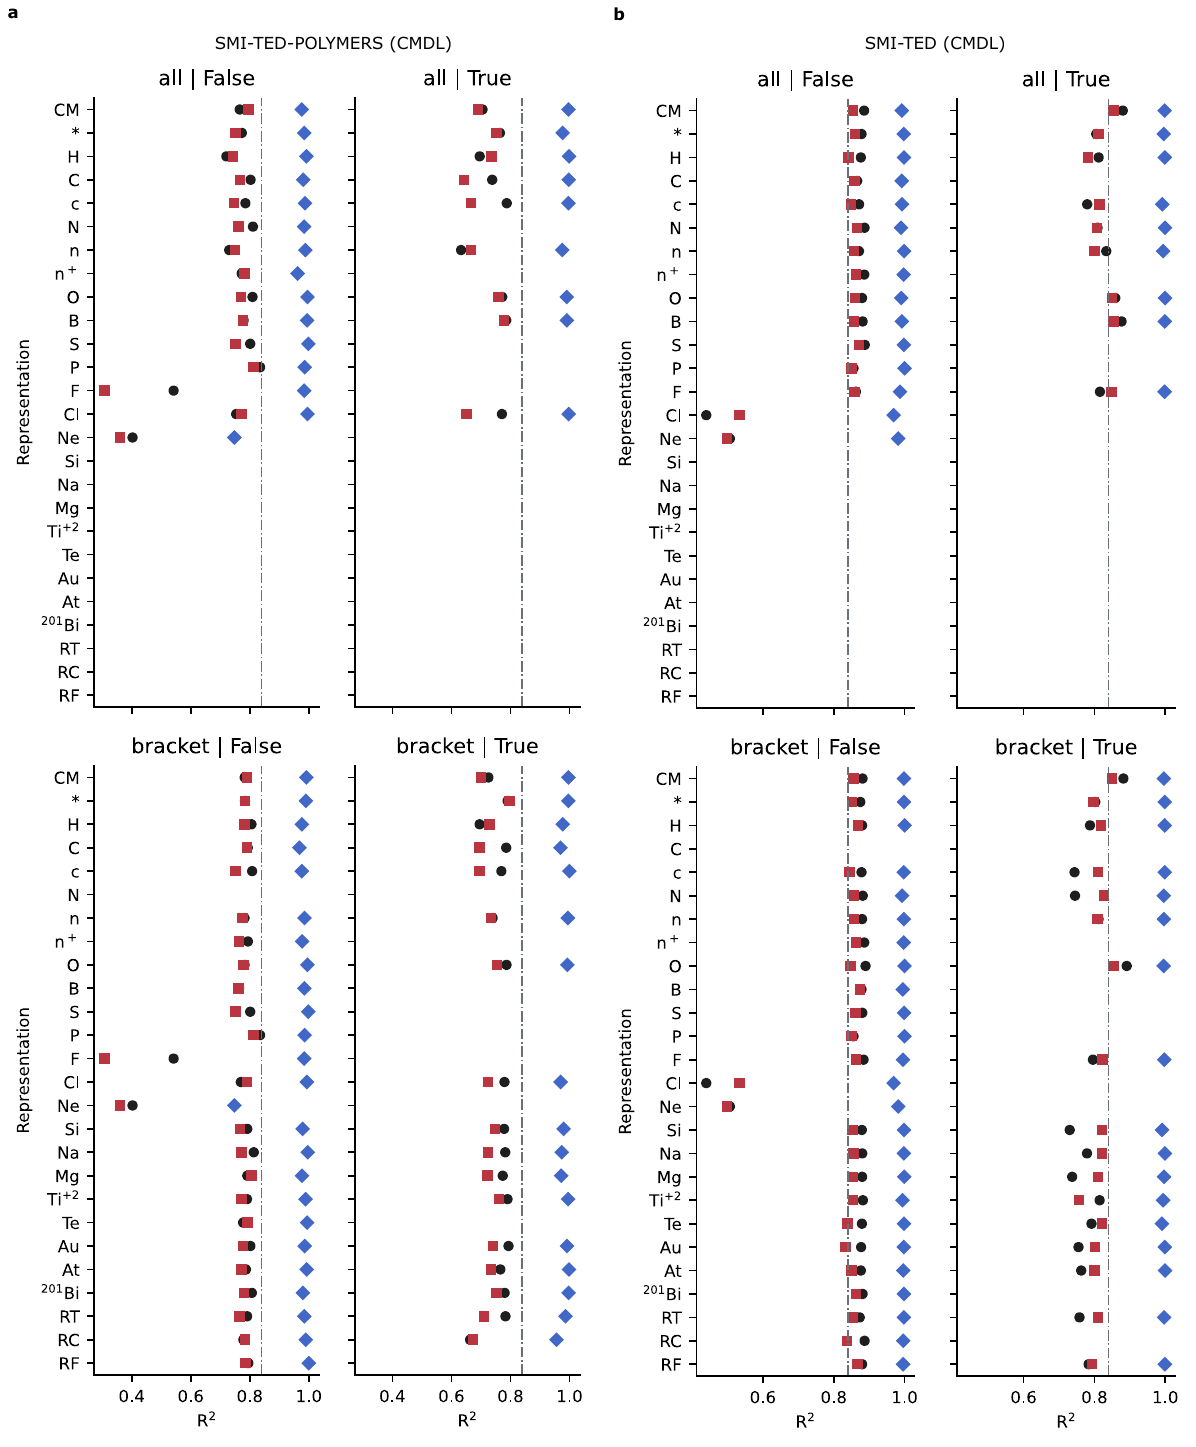}
\caption{Point plots for N\textsubscript{2} gas permeability benchmark experiments of R\textsuperscript{2} using the base random train, valid, and test splits for SMI-TED-POLYMER (\textbf{a}) and SMI-TED (\textbf{b}) models fine-tuned using the CPG representation.}\label{netl_n2_token_point_cmdl_r2}
\end{figure}

\begin{figure}[H]
\centering
\includegraphics[width=1\textwidth]{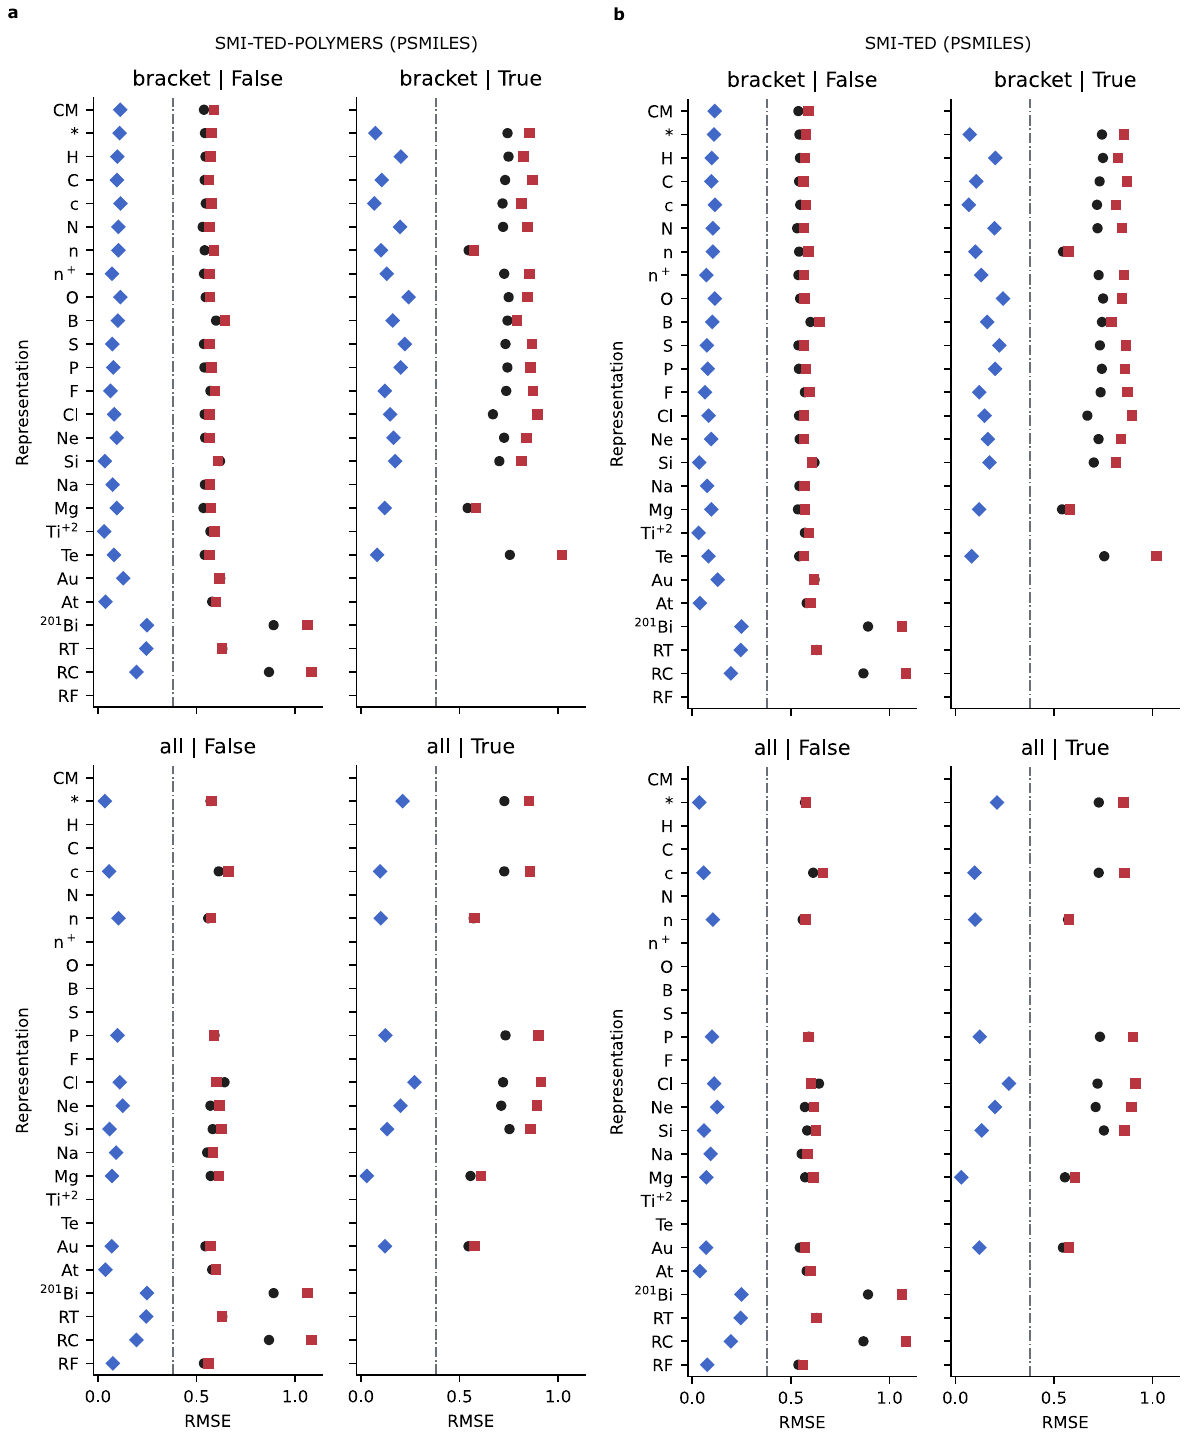}
\caption{Point plots for N\textsubscript{2} gas permeability benchmark experiments of RMSE using the base random train, valid, and test splits for SMI-TED-POLYMER (\textbf{a}) and SMI-TED (\textbf{b}) models fine-tuned using PSMILES.}\label{netl_n2_token_point_psmiles_rmse}
\end{figure}

\subsubsection{CH\textsubscript{4} Gas Permeability CV Scores}\label{cv_netl_ch4}

\begin{figure}[H]
\centering
\includegraphics[width=1\textwidth]{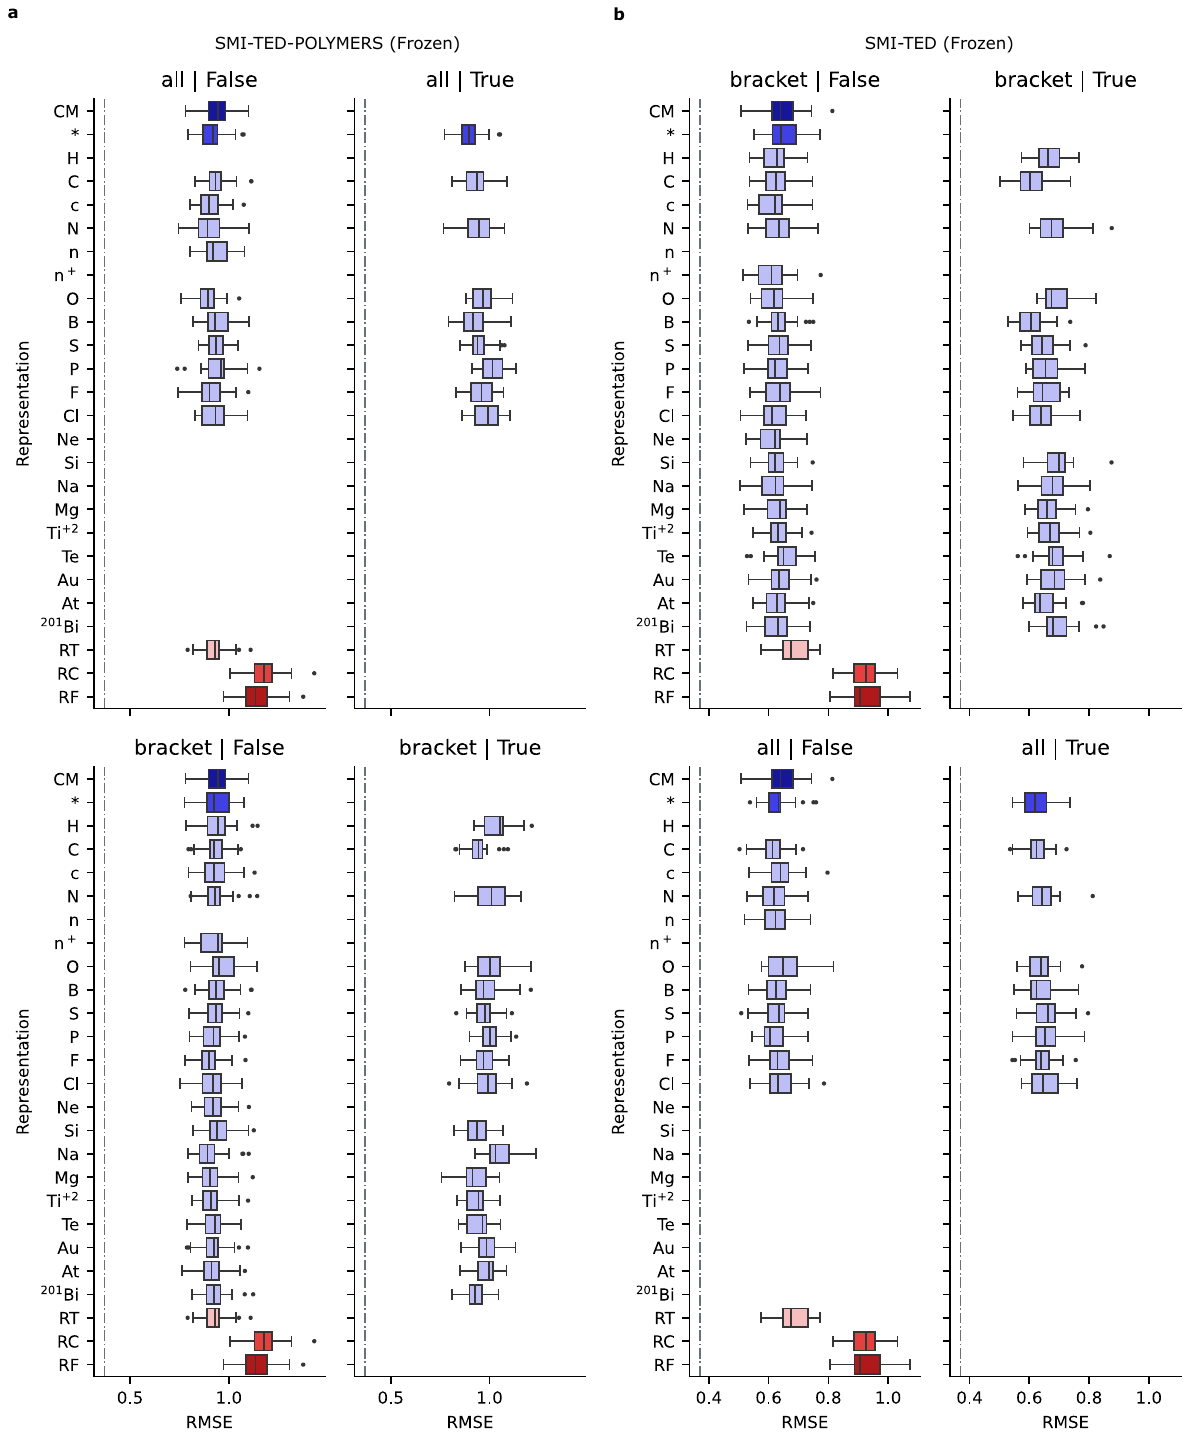}
\caption{Box plots for CH\textsubscript{4} gas permeability repeated cross-validation experiments for SMI-TED-POLYMER (\textbf{a}) and SMI-TED (\textbf{b}) models with frozen weights.}\label{netl_ch4_token_box_frozen}
\end{figure}

\begin{figure}[H]
\centering
\includegraphics[width=1\textwidth]{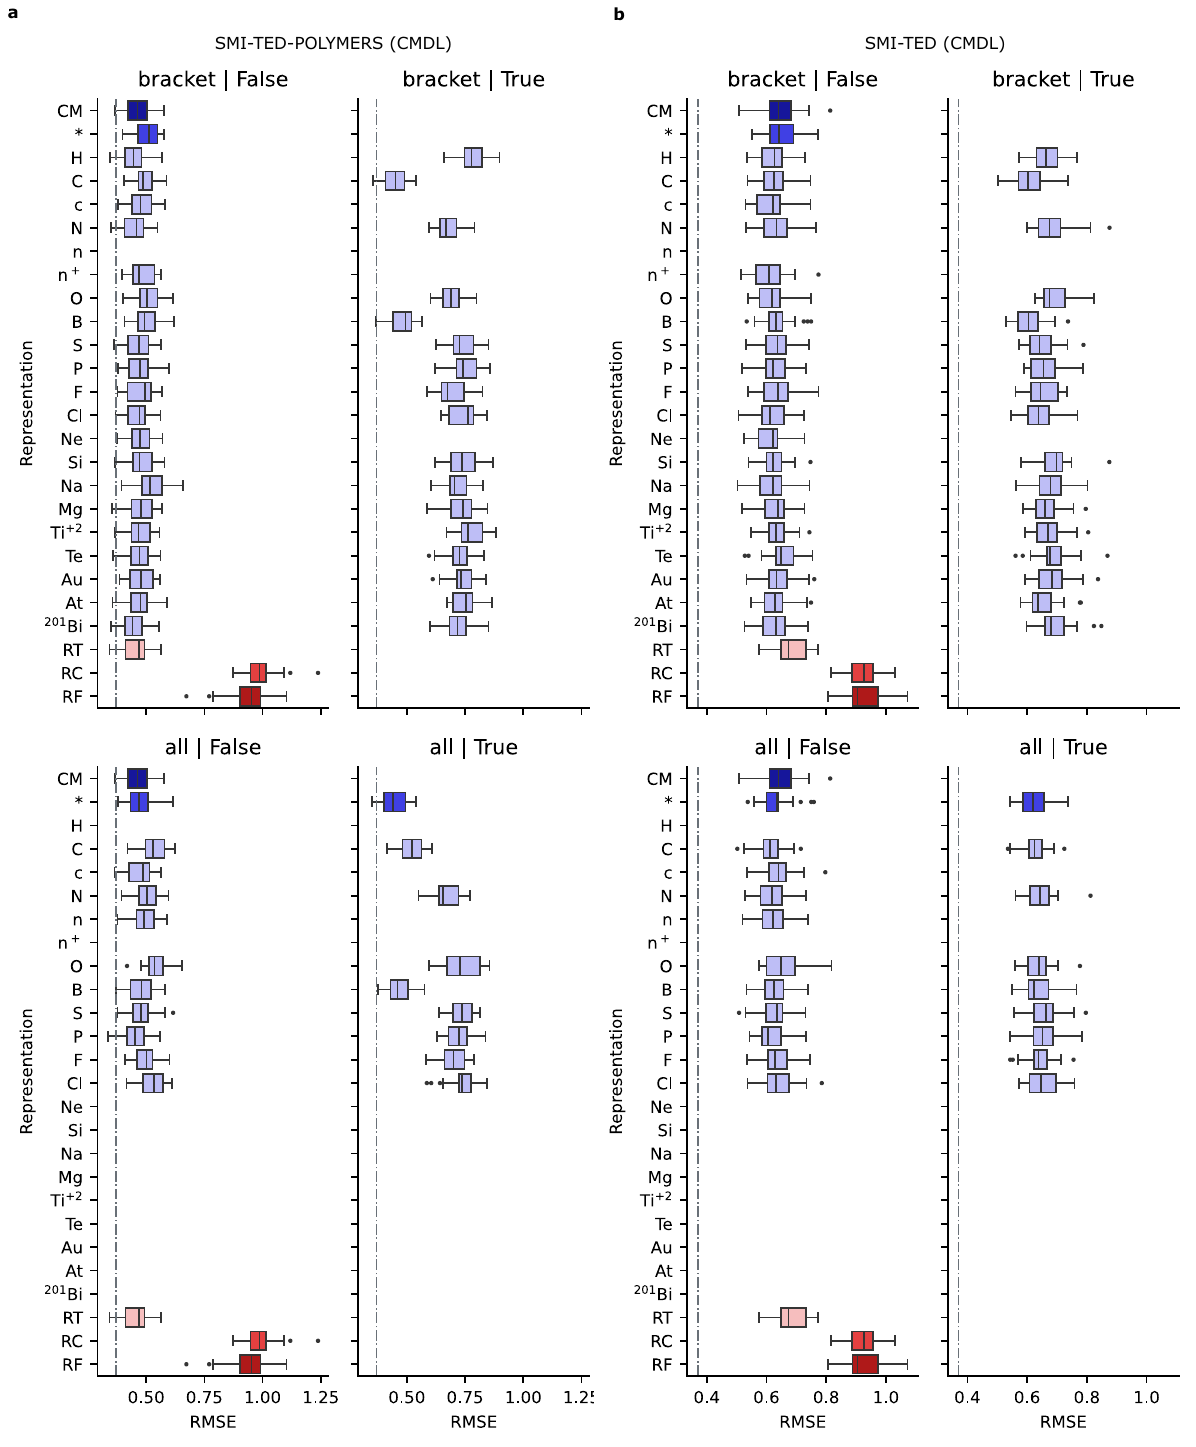}
\caption{Box plots for CH\textsubscript{4} gas permeability repeated cross-validation experiments for SMI-TED-POLYMER (\textbf{a}) and SMI-TED (\textbf{b}) models fine-tuned with the CPG polymer graphs.}\label{netl_ch4_token_box_cmdl}
\end{figure}

\begin{figure}[H]
\centering
\includegraphics[width=1\textwidth]{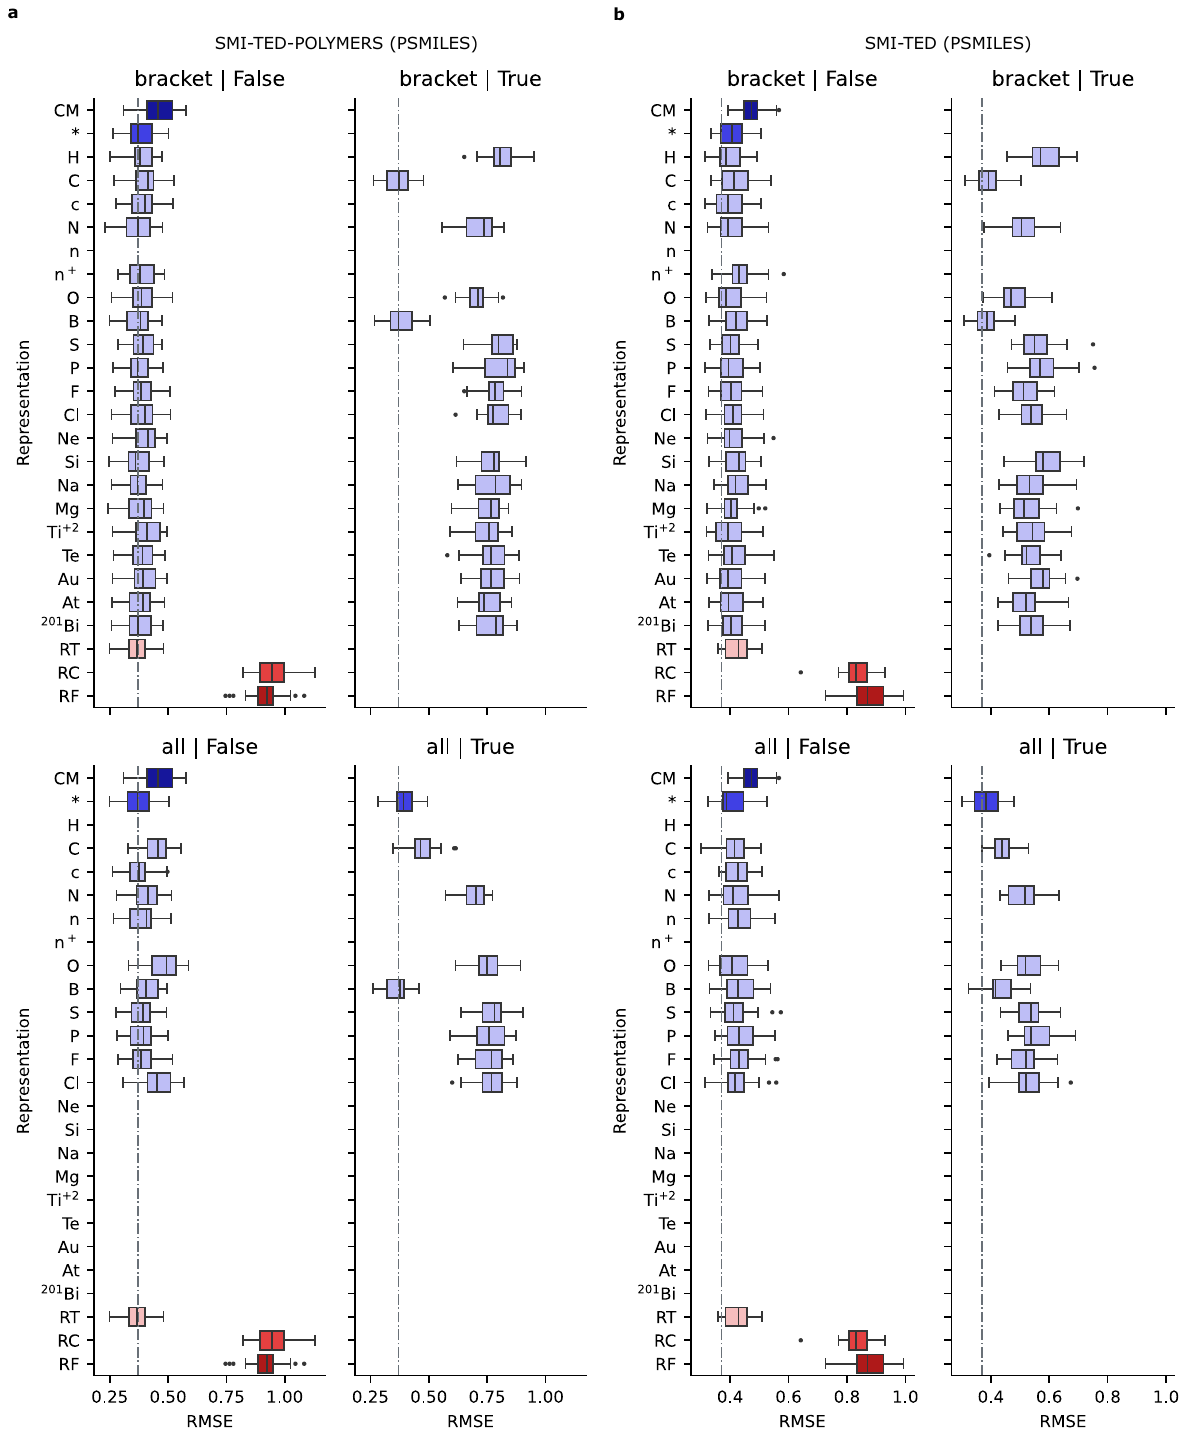}
\caption{Box plots for CH\textsubscript{4} gas permeability repeated cross-validation experiments for SMI-TED-POLYMER (\textbf{a}) and SMI-TED (\textbf{b}) models fine-tuned with PSMILES.}\label{netl_ch4_token_box_psmiles}
\end{figure}

\subsubsection{CH\textsubscript{4} Gas Permeability Random Split Scores}\label{rand_netl_ch4}

\begin{figure}[H]
\centering
\includegraphics[width=1\textwidth]{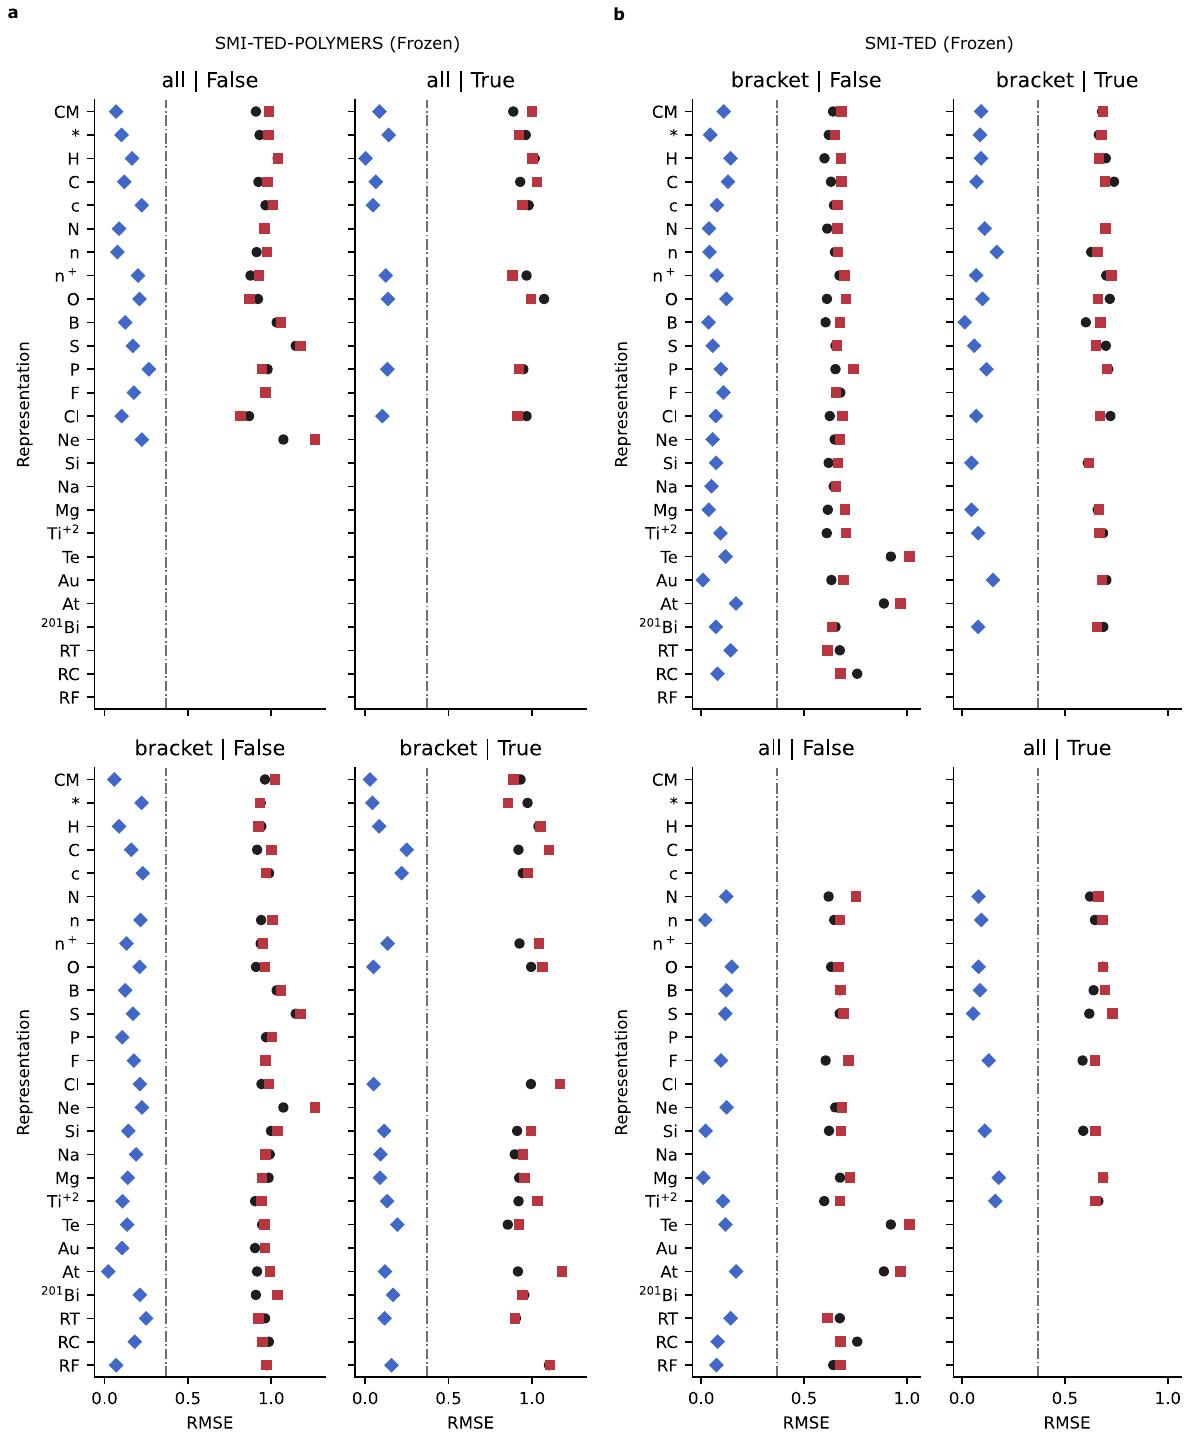}
\caption{Point plots for CH\textsubscript{4} gas permeability benchmark experiments of RMSE using the base random train, valid, and test splits for SMI-TED-POLYMER (\textbf{a}) and SMI-TED (\textbf{b}) models with frozen weights.}\label{netl_ch4_token_point_frozen_rmse}
\end{figure}

\begin{figure}[H]
\centering
\includegraphics[width=1\textwidth]{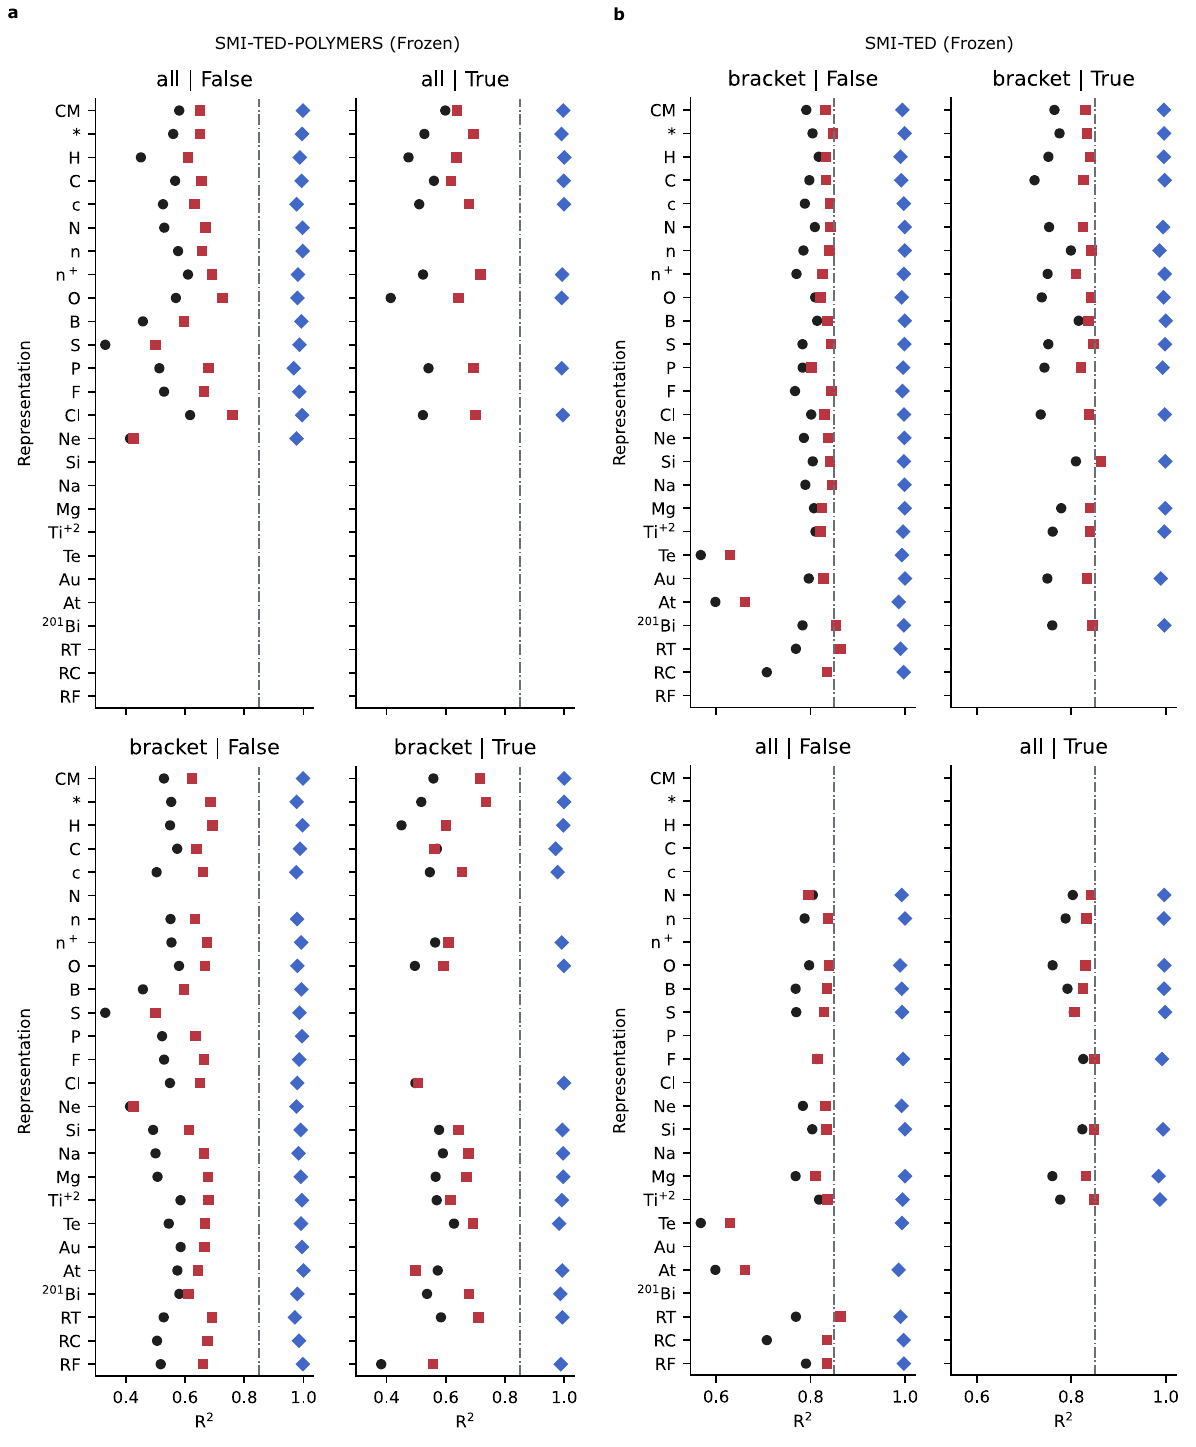}
\caption{Point plots for CH\textsubscript{4} gas permeability benchmark experiments of R\textsuperscript{2} using the base random train, valid, and test splits for SMI-TED-POLYMER (\textbf{a}) and SMI-TED (\textbf{b}) models with frozen weights.}\label{netl_ch4_token_point_frozen_r2}
\end{figure}

\begin{figure}[H]
\centering
\includegraphics[width=1\textwidth]{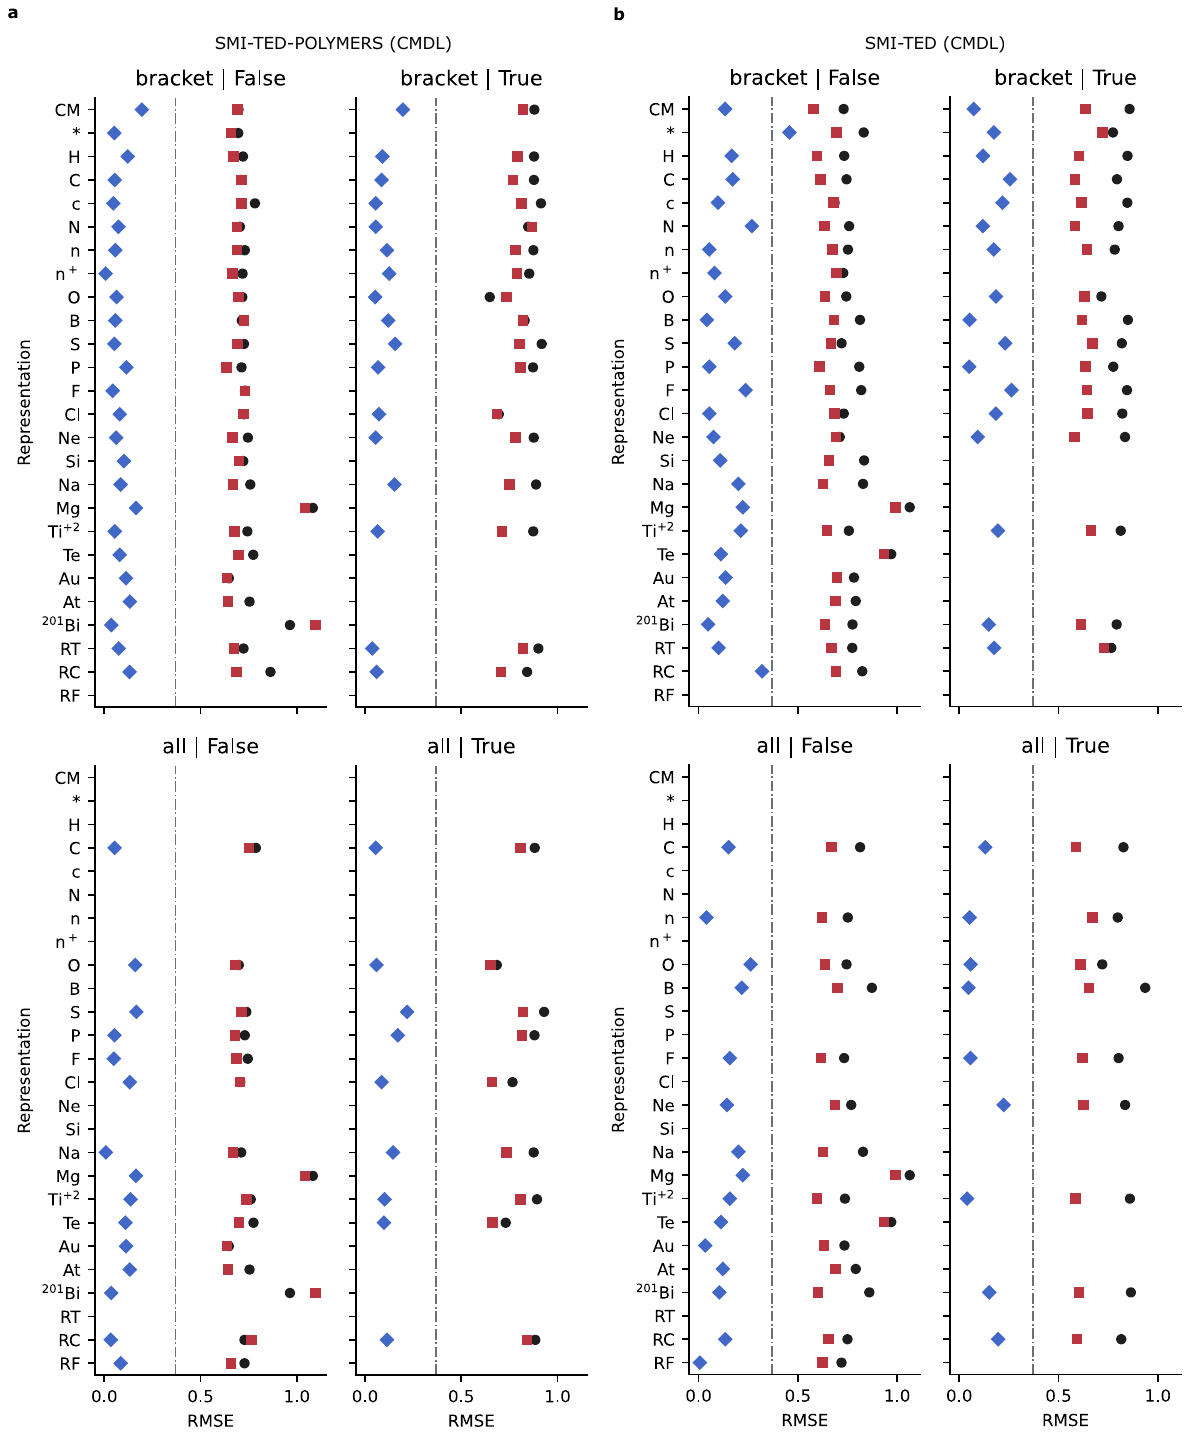}
\caption{Point plots for CH\textsubscript{4} gas permeability benchmark experiments of RMSE using the base random train, valid, and test splits for SMI-TED-POLYMER (\textbf{a}) and SMI-TED (\textbf{b}) models fine-tuned using the CPG representation.}\label{netl_ch4_token_point_cmdl_rmse}
\end{figure}

\begin{figure}
\centering
\includegraphics[width=1\textwidth]{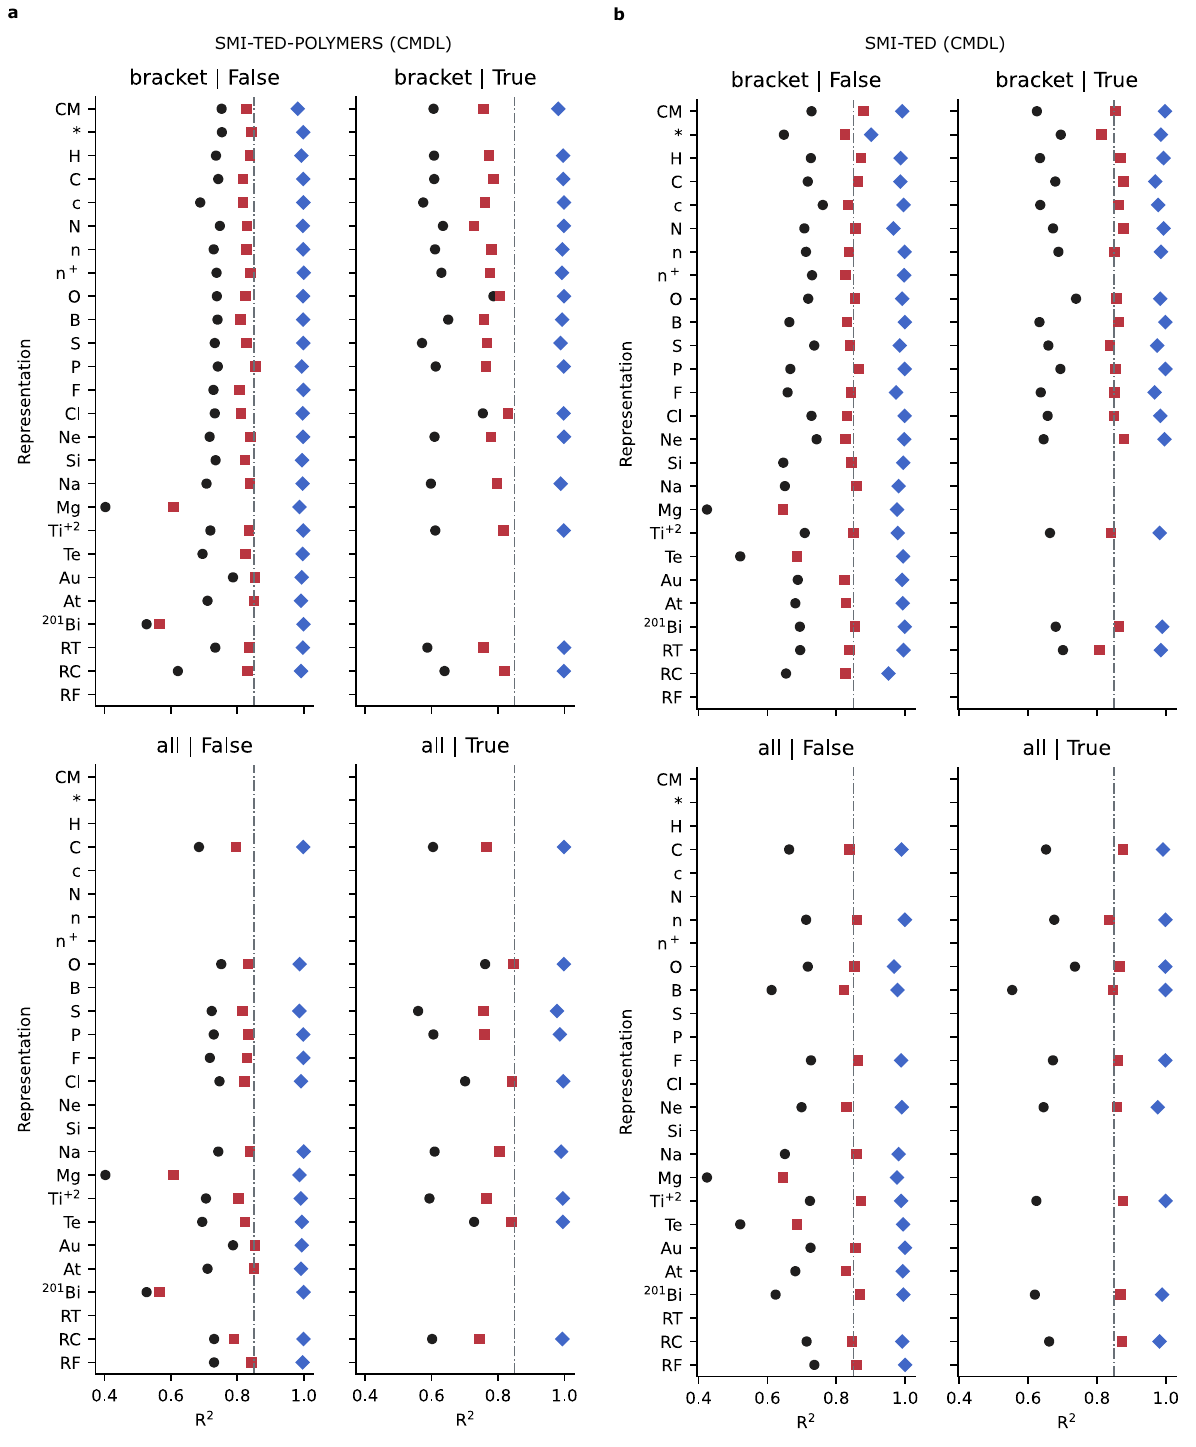}
\caption{Point plots for CH\textsubscript{4} gas permeability benchmark experiments of R\textsuperscript{2} using the base random train, valid, and test splits for SMI-TED-POLYMER (\textbf{a}) and SMI-TED (\textbf{b}) models fine-tuned using the CPG representation.}\label{netl_ch4_token_point_cmdl_r2}
\end{figure}

\begin{figure}[H]
\centering
\includegraphics[width=1\textwidth]{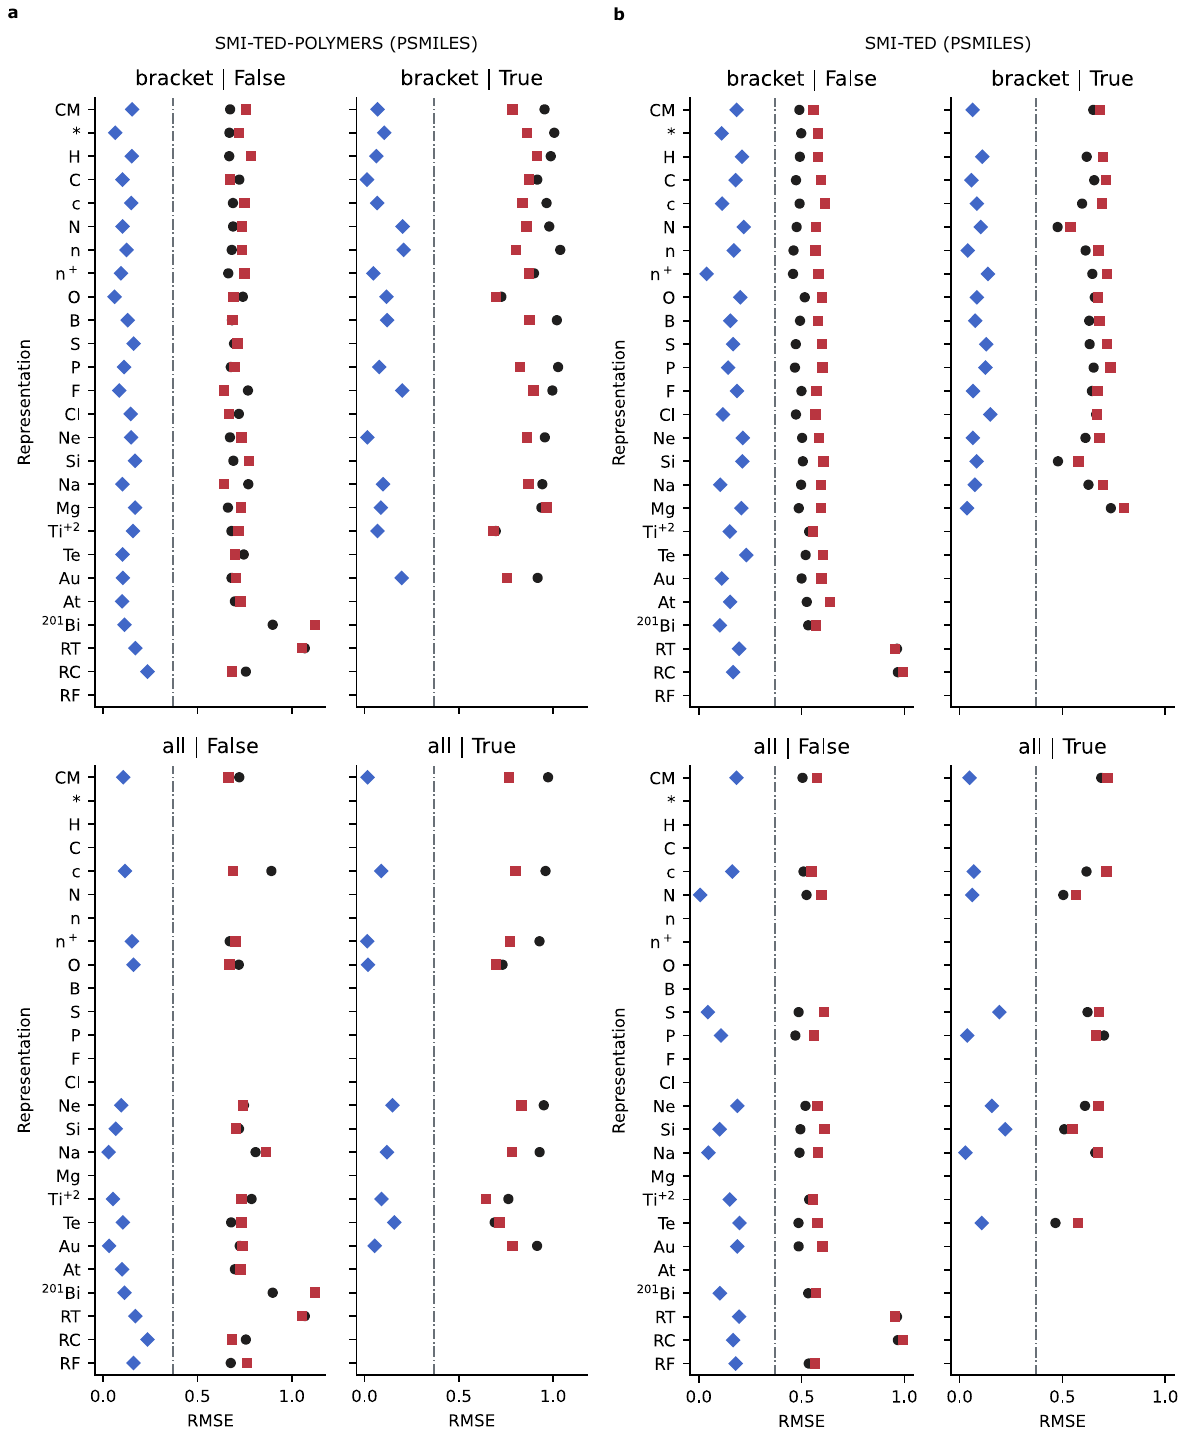}
\caption{Point plots for CH\textsubscript{4} gas permeability benchmark experiments of RMSE using the base random train, valid, and test splits for SMI-TED-POLYMER (\textbf{a}) and SMI-TED (\textbf{b}) models fine-tuned using PSMILES.}\label{netl_ch4_token_point_psmiles_rmse}
\end{figure}

\subsubsection{CO\textsubscript{2}:CH\textsubscript{4} Gas Selectivity CV Scores}\label{cv_netl_co2_ch4}

\begin{figure}[H]
\centering
\includegraphics[width=1\textwidth]{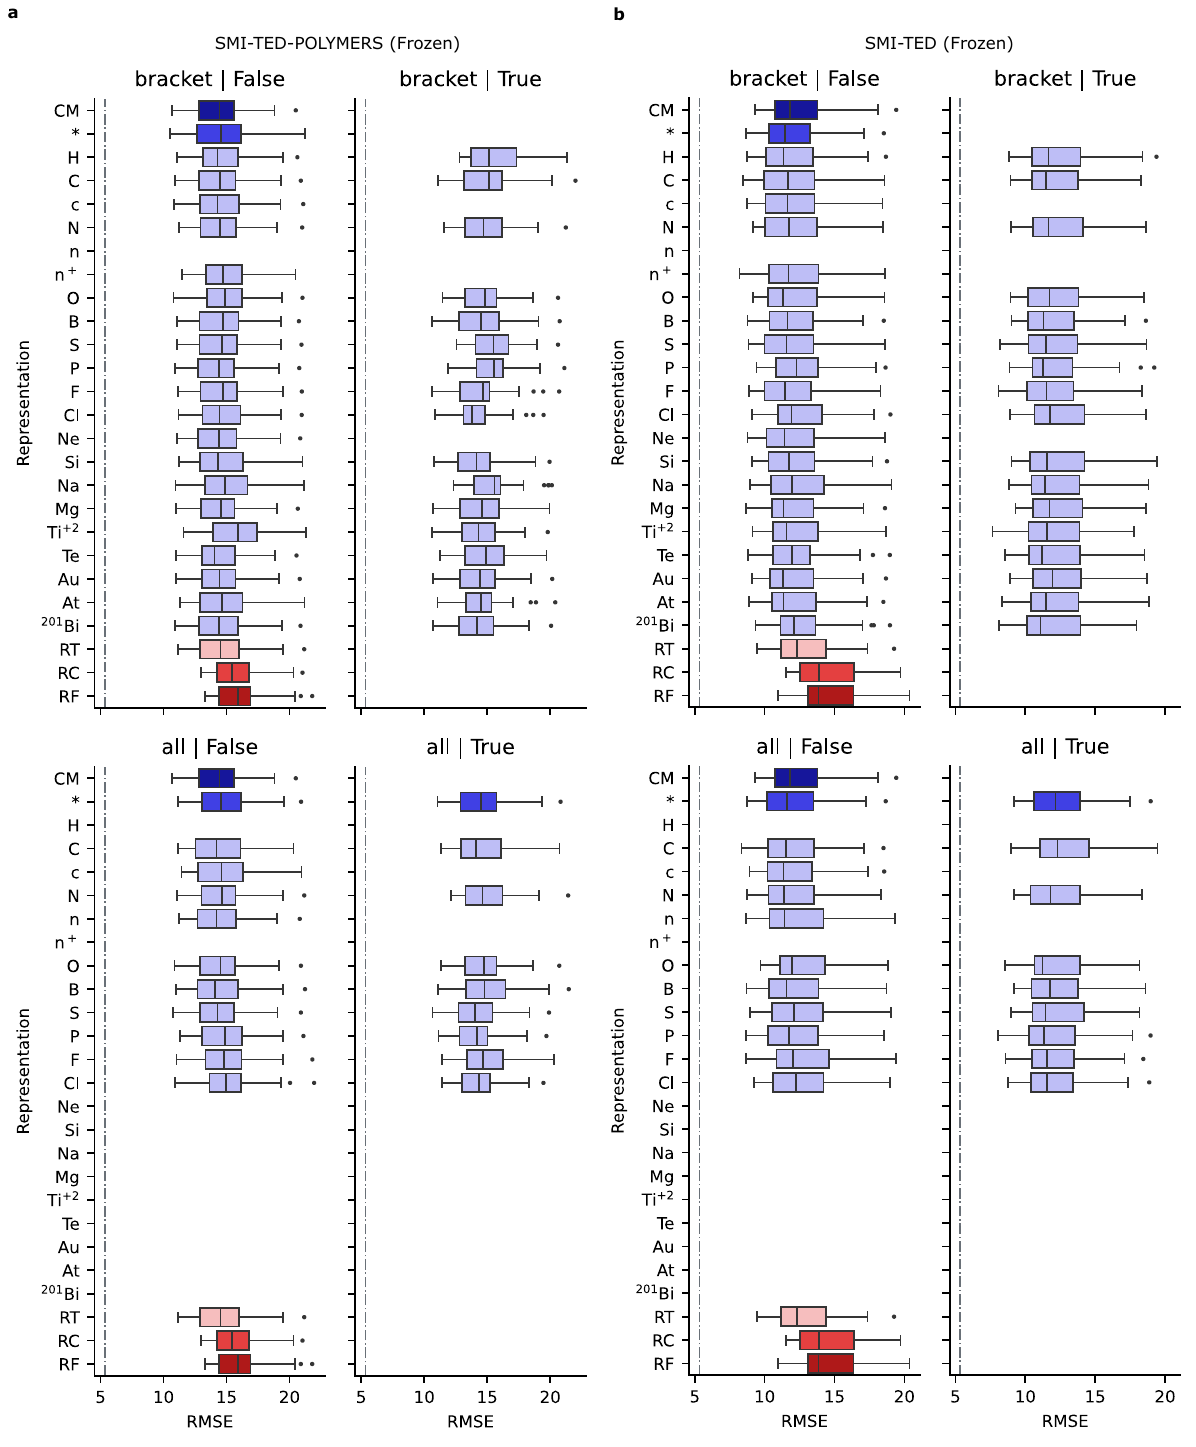}
\caption{Box plots for CO\textsubscript{2}:CH\textsubscript{4} gas selectivity repeated cross-validation experiments for SMI-TED-POLYMER (\textbf{a}) and SMI-TED (\textbf{b}) models with frozen weights.}\label{netl_co2_ch4_token_box_frozen}
\end{figure}

\begin{figure}[H]
\centering
\includegraphics[width=1\textwidth]{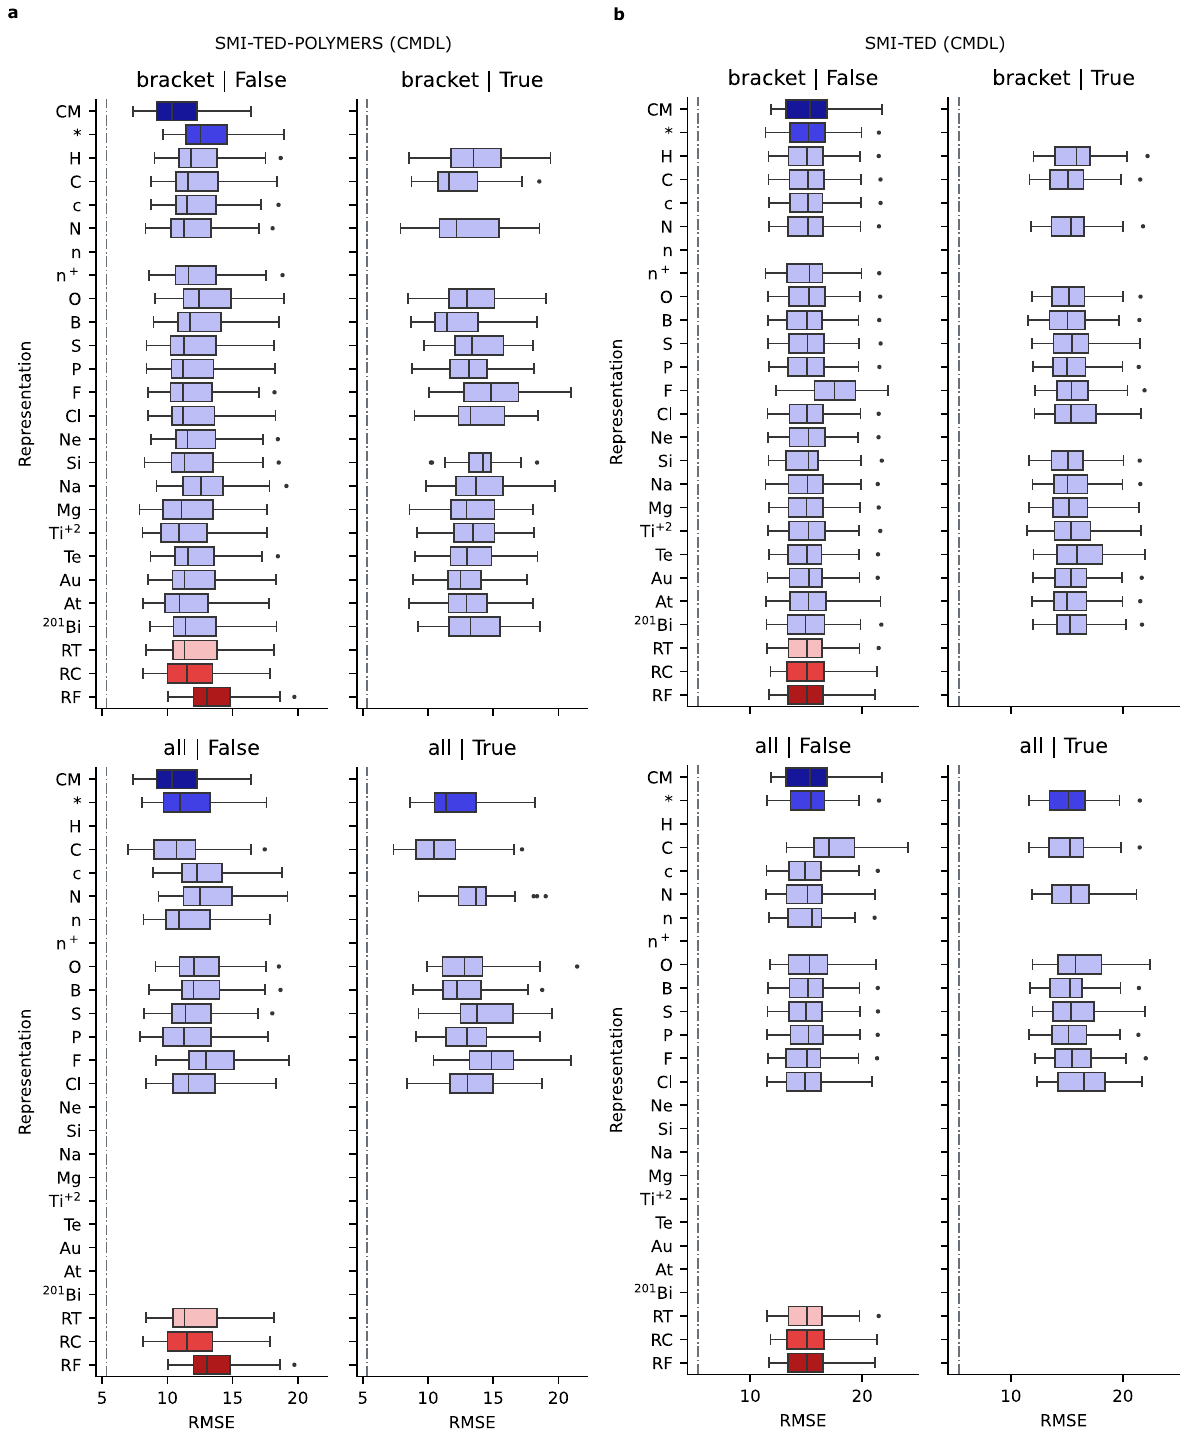}
\caption{Box plots for CO\textsubscript{2}:CH\textsubscript{4} gas selectivity repeated cross-validation experiments for SMI-TED-POLYMER (\textbf{a}) and SMI-TED (\textbf{b}) models fine-tuned with the CPG polymer graphs.}\label{netl_co2_ch4_token_box_cmdl}
\end{figure}

\begin{figure}[H]
\centering
\includegraphics[width=1\textwidth]{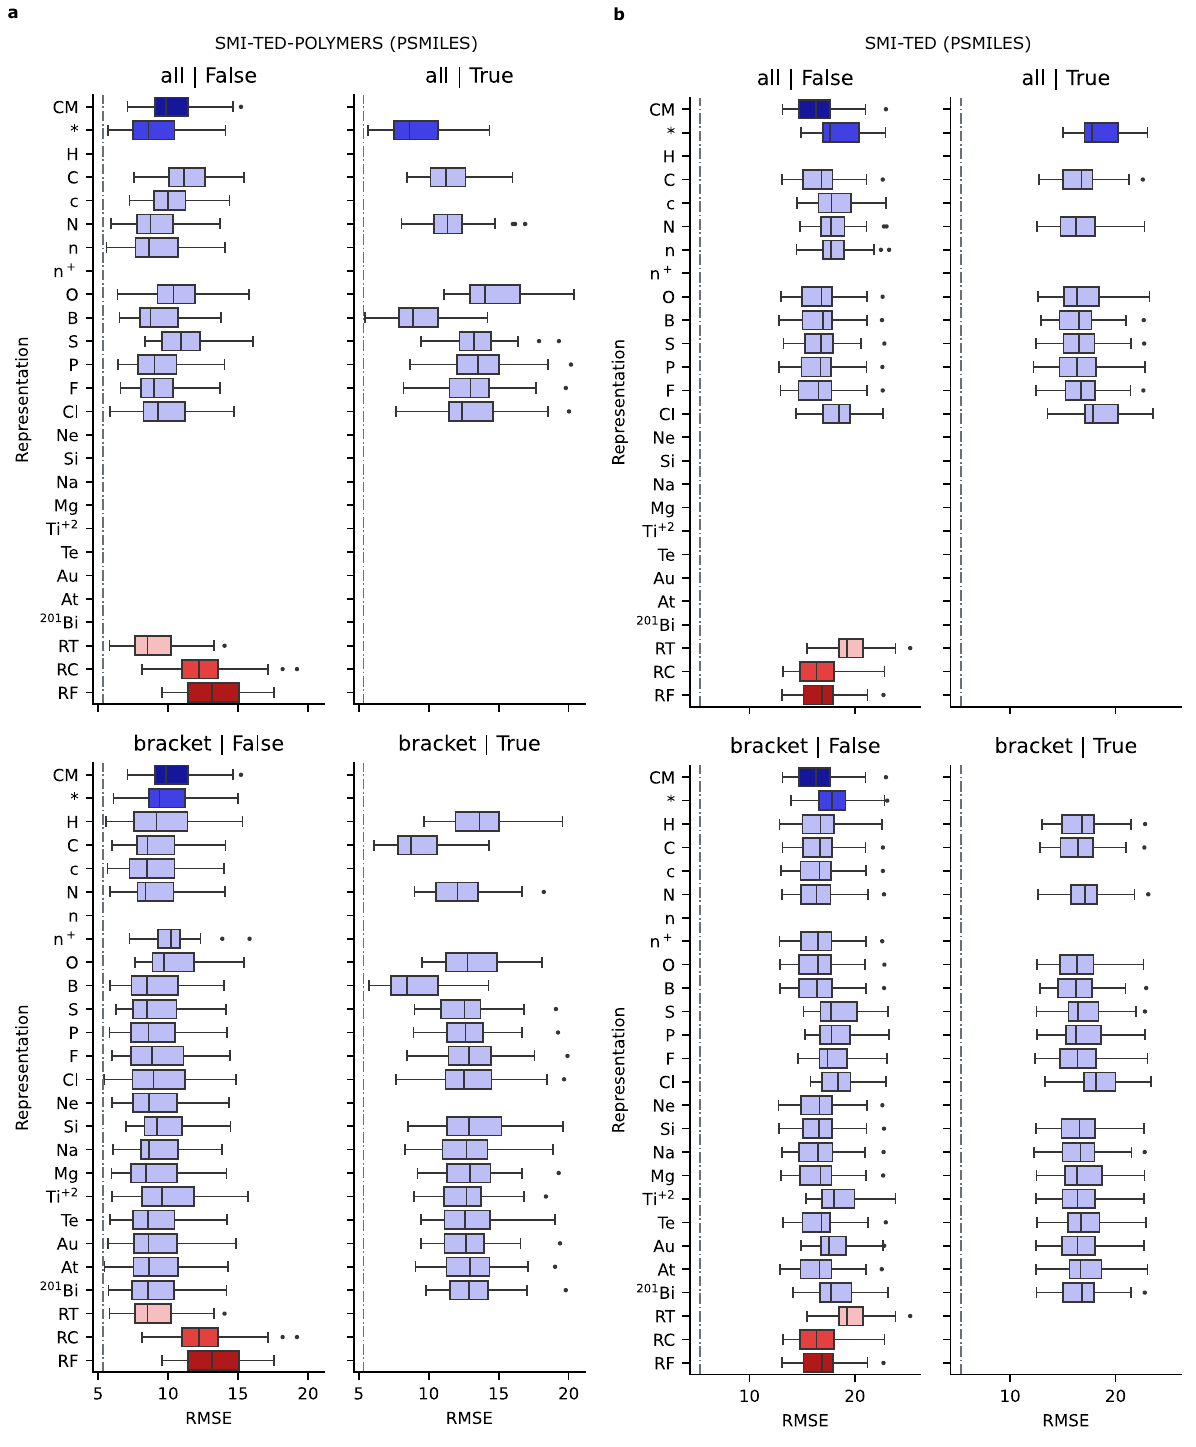}
\caption{Box plots for CO\textsubscript{2}:CH\textsubscript{4} gas selectivity repeated cross-validation experiments for SMI-TED-POLYMER (\textbf{a}) and SMI-TED (\textbf{b}) models fine-tuned with PSMILES.}\label{netl_co2_ch4_token_box_psmiles}
\end{figure}

\subsubsection{CO\textsubscript{2}:CH\textsubscript{4} Gas Selectivity Random Split Scores}\label{rand_netl_co2_ch4}

\begin{figure}[H]
\centering
\includegraphics[width=1\textwidth]{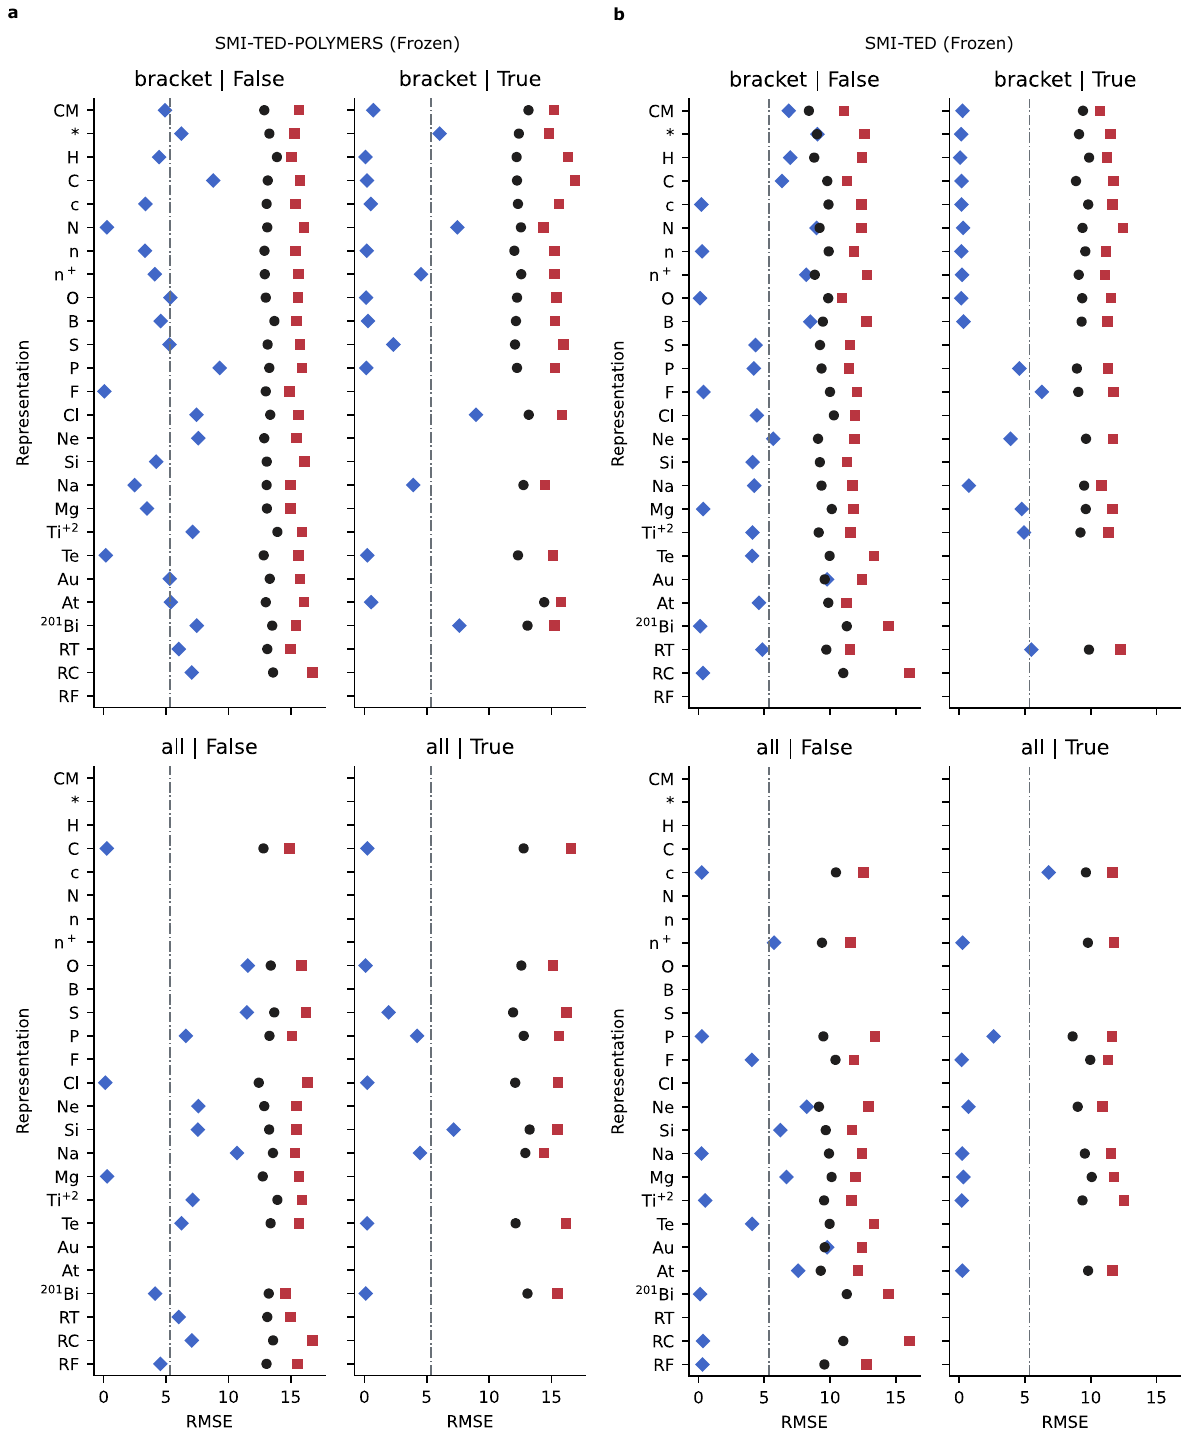}
\caption{Point plots for CO\textsubscript{2}:CH\textsubscript{4} gas selectivity benchmark experiments of RMSE using the base random train, valid, and test splits for SMI-TED-POLYMER (\textbf{a}) and SMI-TED (\textbf{b}) models with frozen weights.}\label{netl_co2_ch4_token_point_frozen_rmse}
\end{figure}

\begin{figure}[H]
\centering
\includegraphics[width=1\textwidth]{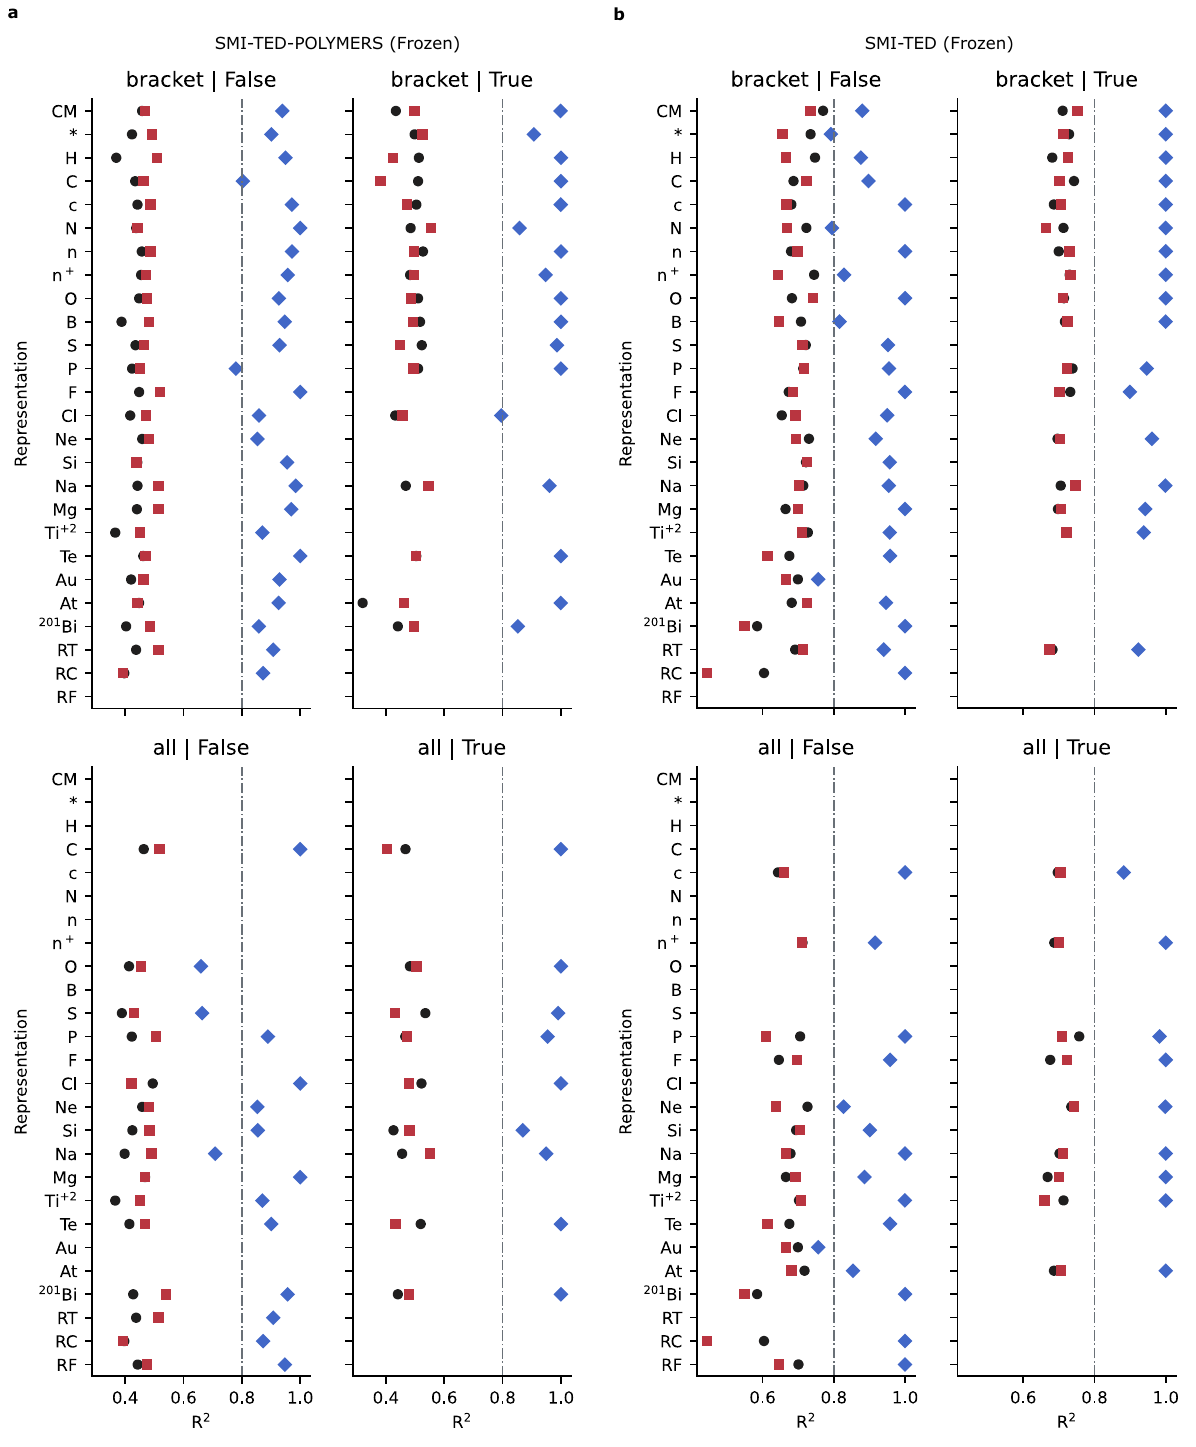}
\caption{Point plots for CO\textsubscript{2}:CH\textsubscript{4} gas selectivity benchmark experiments of R\textsuperscript{2} using the base random train, valid, and test splits for SMI-TED-POLYMER (\textbf{a}) and SMI-TED (\textbf{b}) models with frozen weights.}\label{netl_co2_ch4_token_point_frozen_r2}
\end{figure}

\begin{figure}[H]
\centering
\includegraphics[width=1\textwidth]{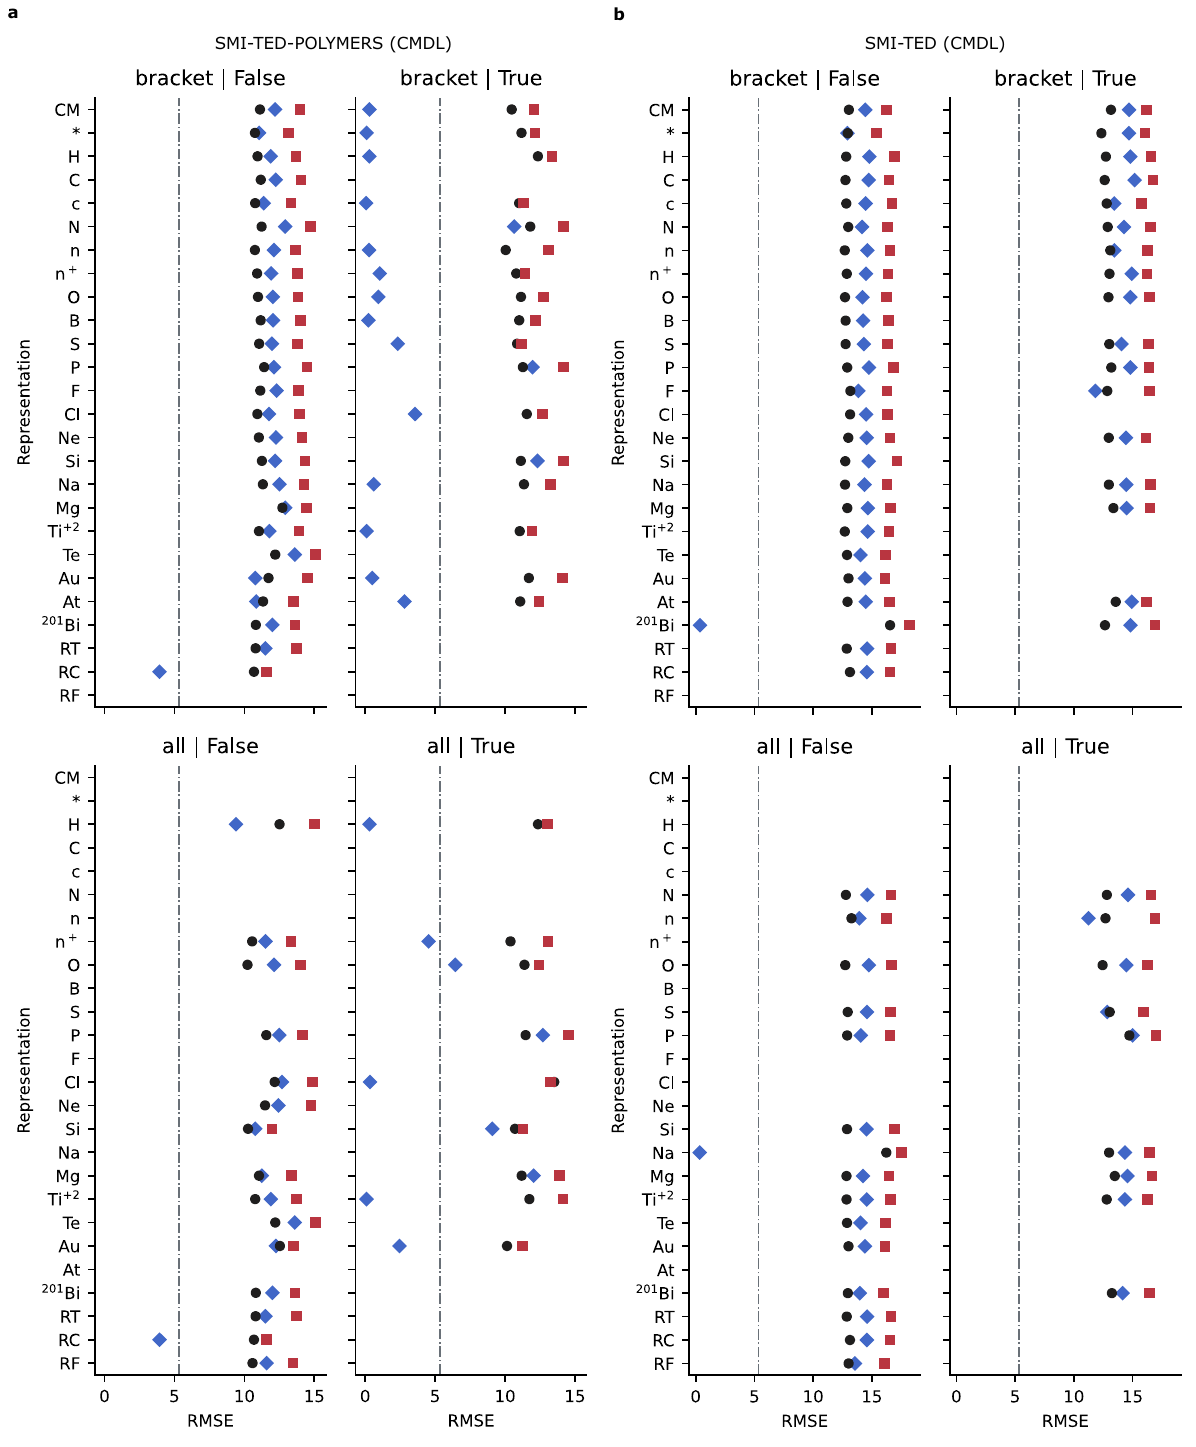}
\caption{Point plots for CO\textsubscript{2}:CH\textsubscript{4} gas selectivity benchmark experiments of RMSE using the base random train, valid, and test splits for SMI-TED-POLYMER (\textbf{a}) and SMI-TED (\textbf{b}) models fine-tuned using the CPG representation.}\label{netl_co2_ch4_token_point_cmdl_rmse}
\end{figure}

\begin{figure}
\centering
\includegraphics[width=1\textwidth]{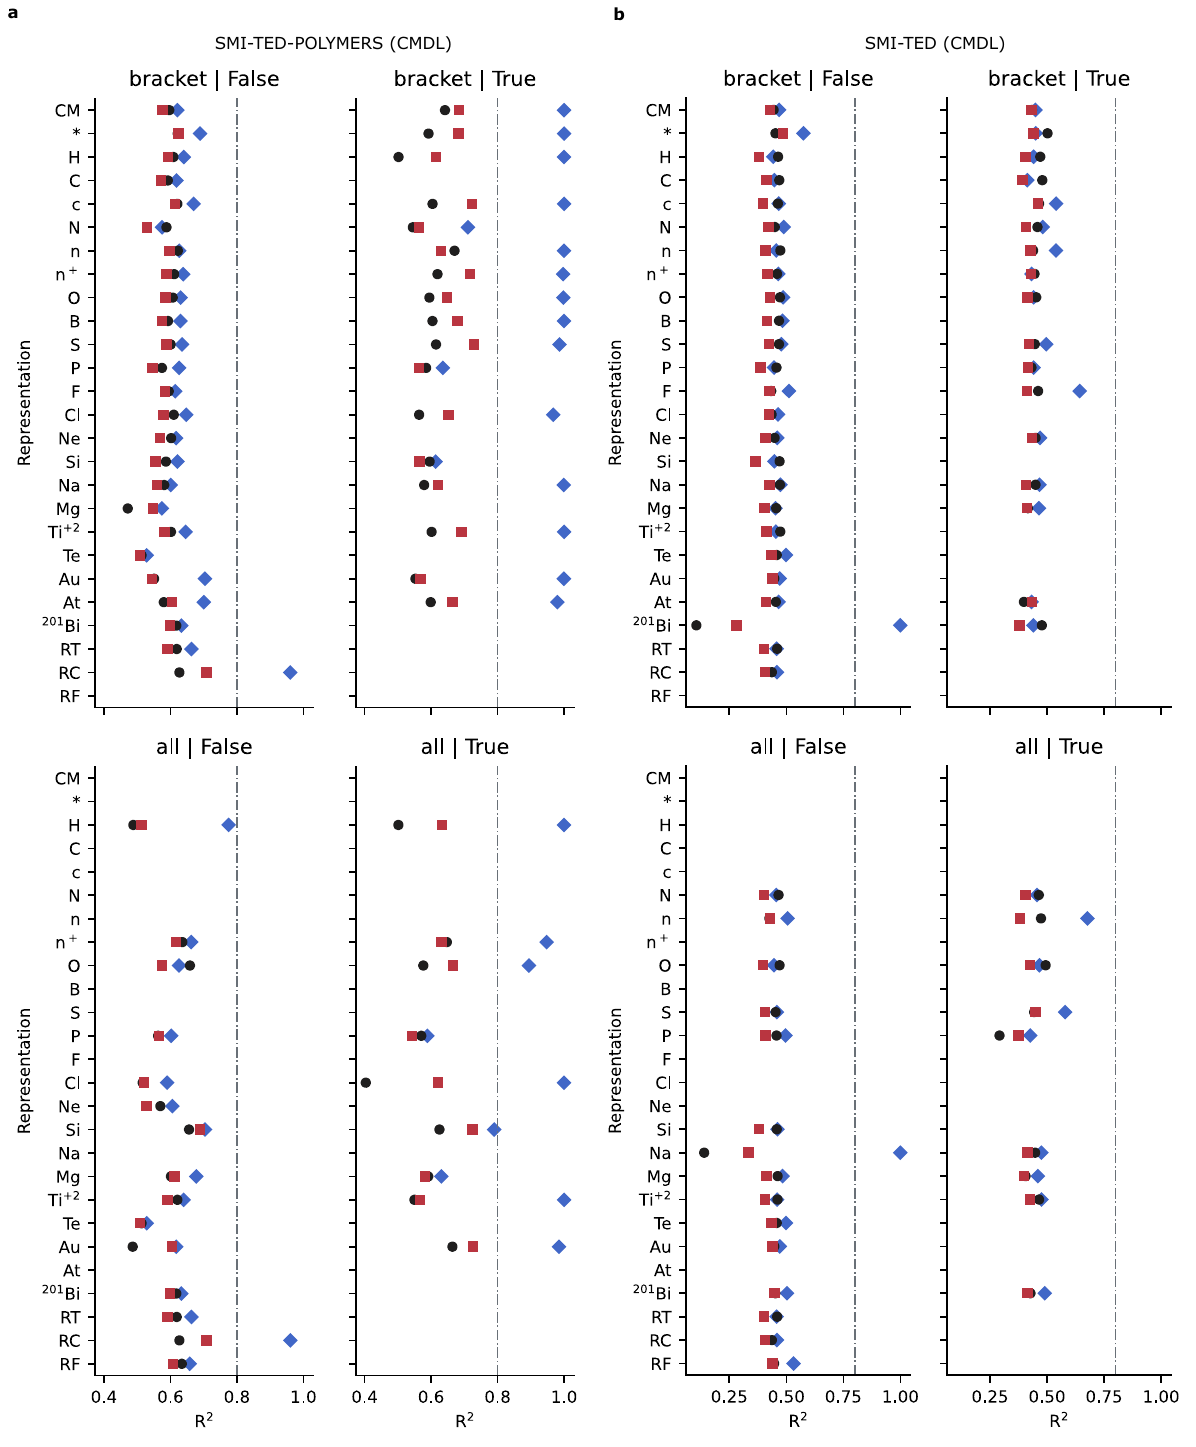}
\caption{Point plots for CO\textsubscript{2}:CH\textsubscript{4} gas selectivity benchmark experiments of R\textsuperscript{2} using the base random train, valid, and test splits for SMI-TED-POLYMER (\textbf{a}) and SMI-TED (\textbf{b}) models fine-tuned using the CPG representation.}\label{netl_co2_ch4_token_point_cmdl_r2}
\end{figure}

\begin{figure}[H]
\centering
\includegraphics[width=1\textwidth]{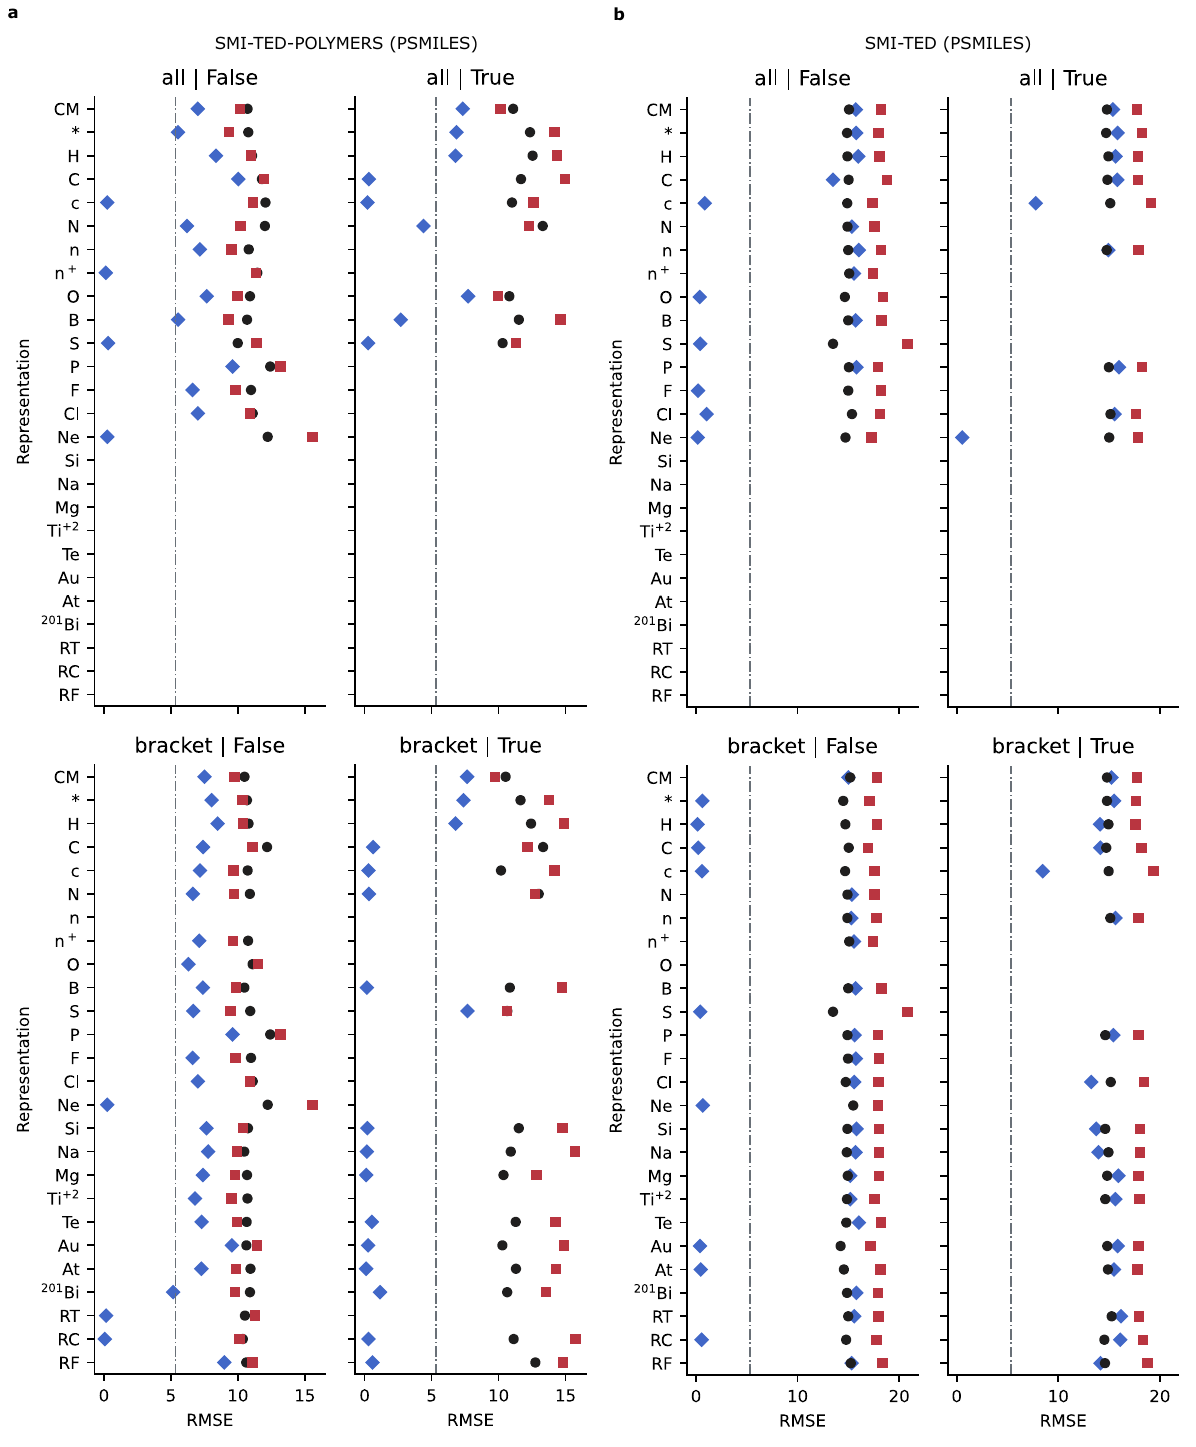}
\caption{Point plots for CO\textsubscript{2}:CH\textsubscript{4} gas selectivity benchmark experiments of RMSE using the base random train, valid, and test splits for SMI-TED-POLYMER (\textbf{a}) and SMI-TED (\textbf{b}) models fine-tuned using PSMILES.}\label{netl_co2_ch4_token_point_psmiles_rmse}
\end{figure}

\subsubsection{CO\textsubscript{2}:N\textsubscript{2} Gas Selectivity CV Scores}\label{cv_netl_co2_n2}

\begin{figure}[H]
\centering
\includegraphics[width=1\textwidth]{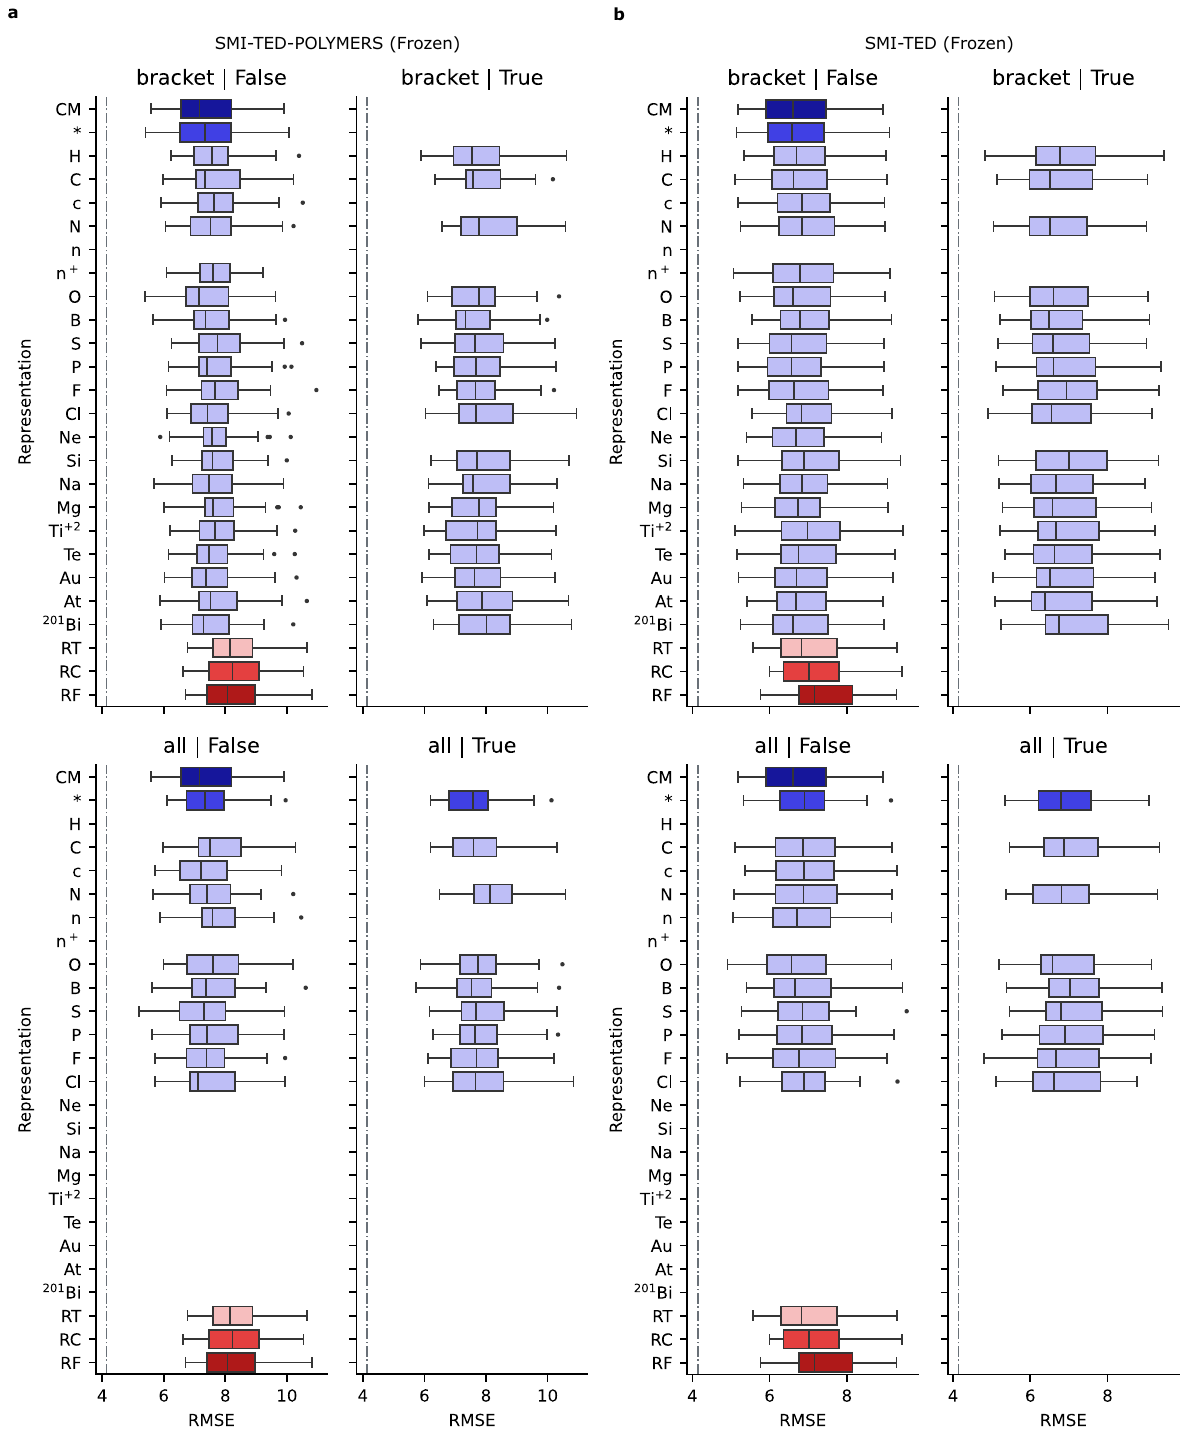}
\caption{Box plots for CO\textsubscript{2}:N\textsubscript{2} gas selectivity repeated cross-validation experiments for SMI-TED-POLYMER (\textbf{a}) and SMI-TED (\textbf{b}) models with frozen weights.}\label{netl_co2_n2_token_box_frozen}
\end{figure}

\begin{figure}[H]
\centering
\includegraphics[width=1\textwidth]{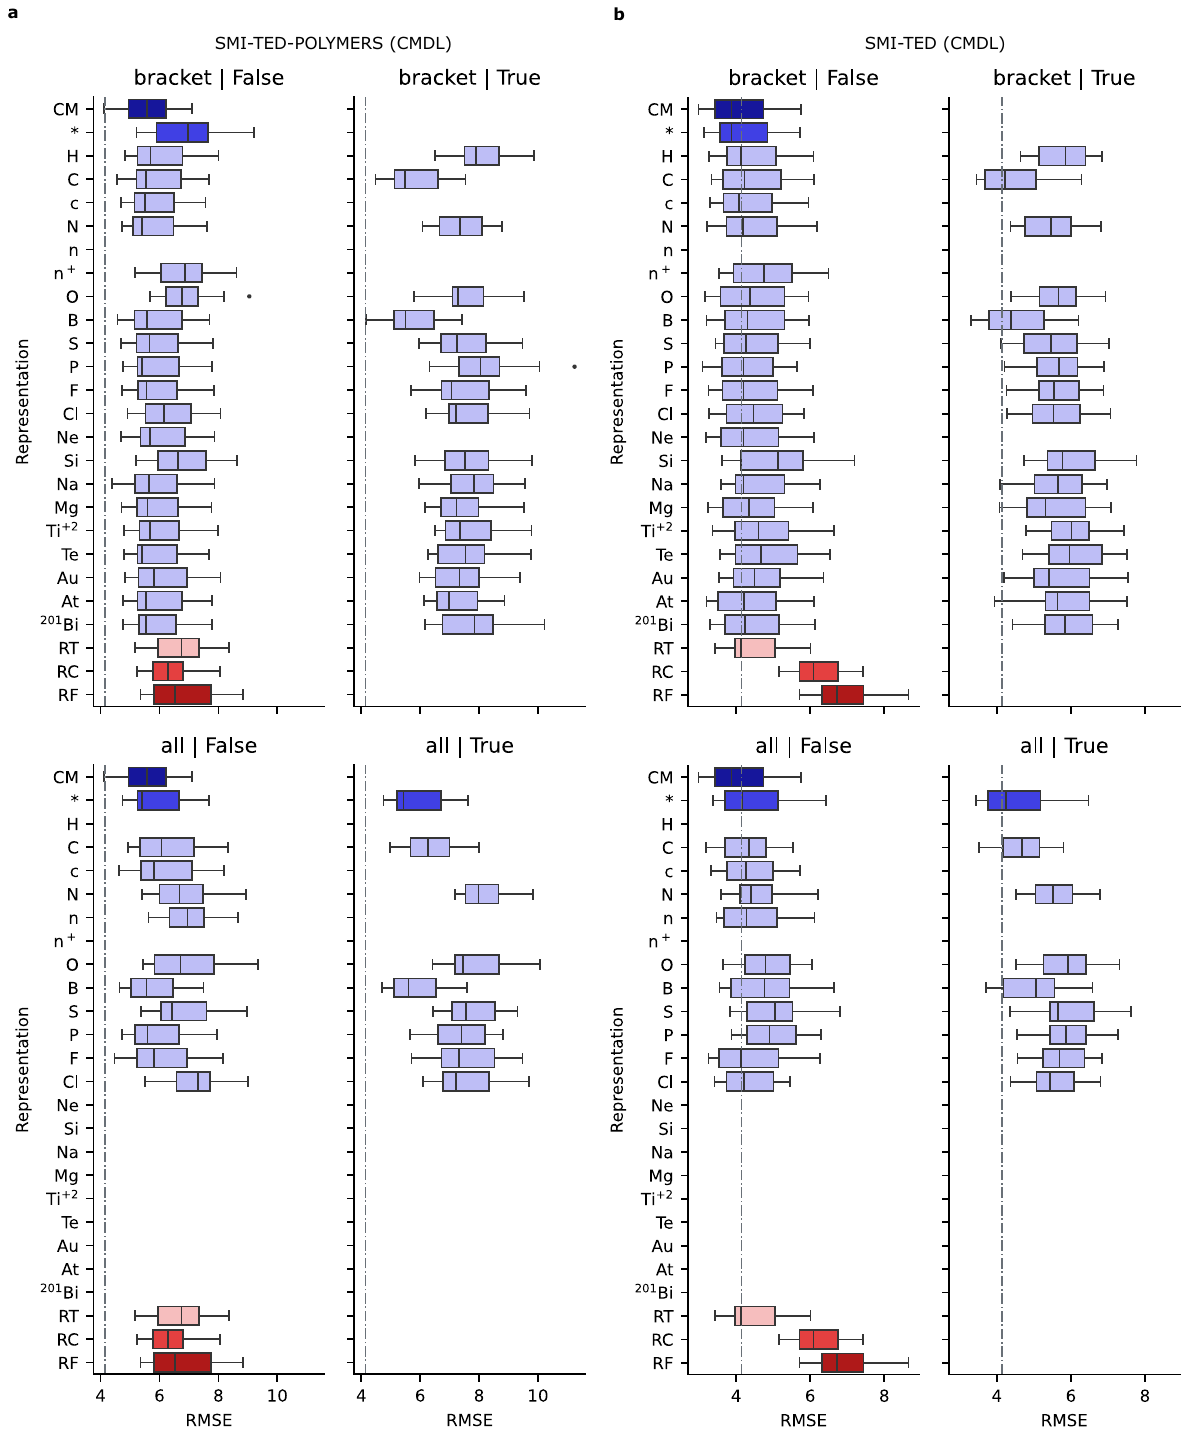}
\caption{Box plots for CO\textsubscript{2}:N\textsubscript{2} gas selectivity repeated cross-validation experiments for SMI-TED-POLYMER (\textbf{a}) and SMI-TED (\textbf{b}) models fine-tuned with the CPG polymer graphs.}\label{netl_co2_n2_token_box_cmdl}
\end{figure}

\begin{figure}[H]
\centering
\includegraphics[width=1\textwidth]{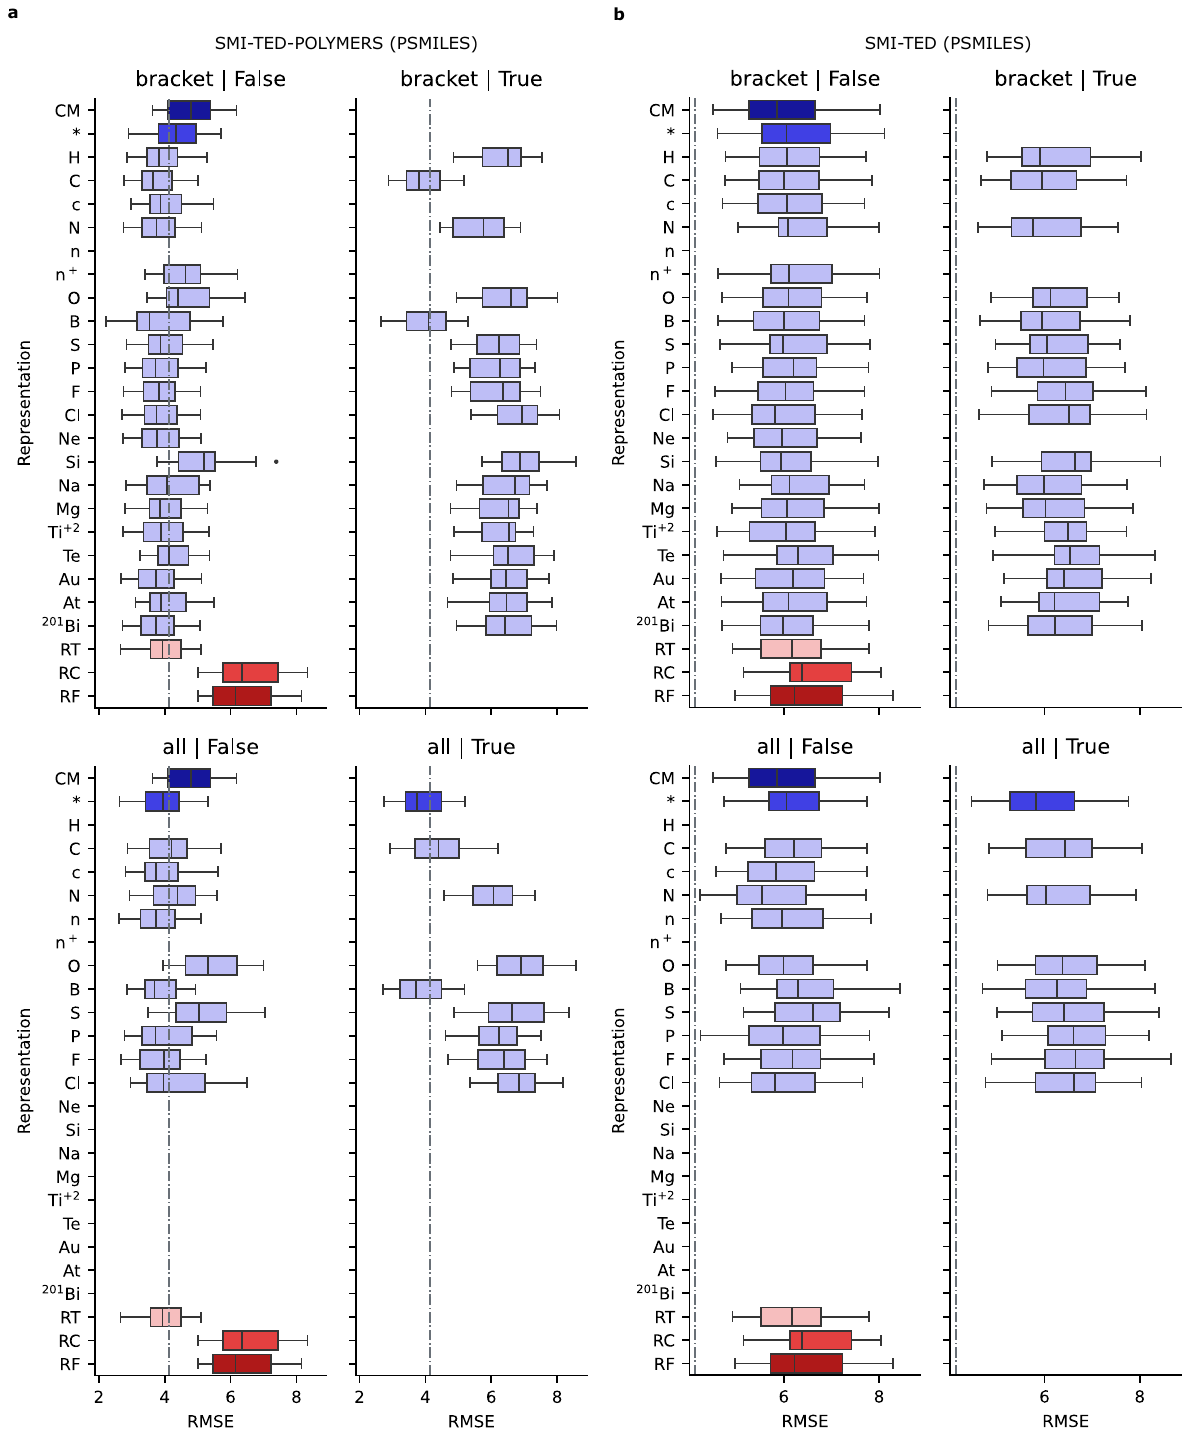}
\caption{Box plots for CO\textsubscript{2}:N\textsubscript{2} gas selectivity repeated cross-validation experiments for SMI-TED-POLYMER (\textbf{a}) and SMI-TED (\textbf{b}) models fine-tuned with PSMILES.}\label{netl_co2_n2_token_box_psmiles}
\end{figure}

\subsubsection{CO\textsubscript{2}:N\textsubscript{2} Gas Selectivity Random Split Scores}\label{rand_netl_co2_n2}

\begin{figure}[H]
\centering
\includegraphics[width=1\textwidth]{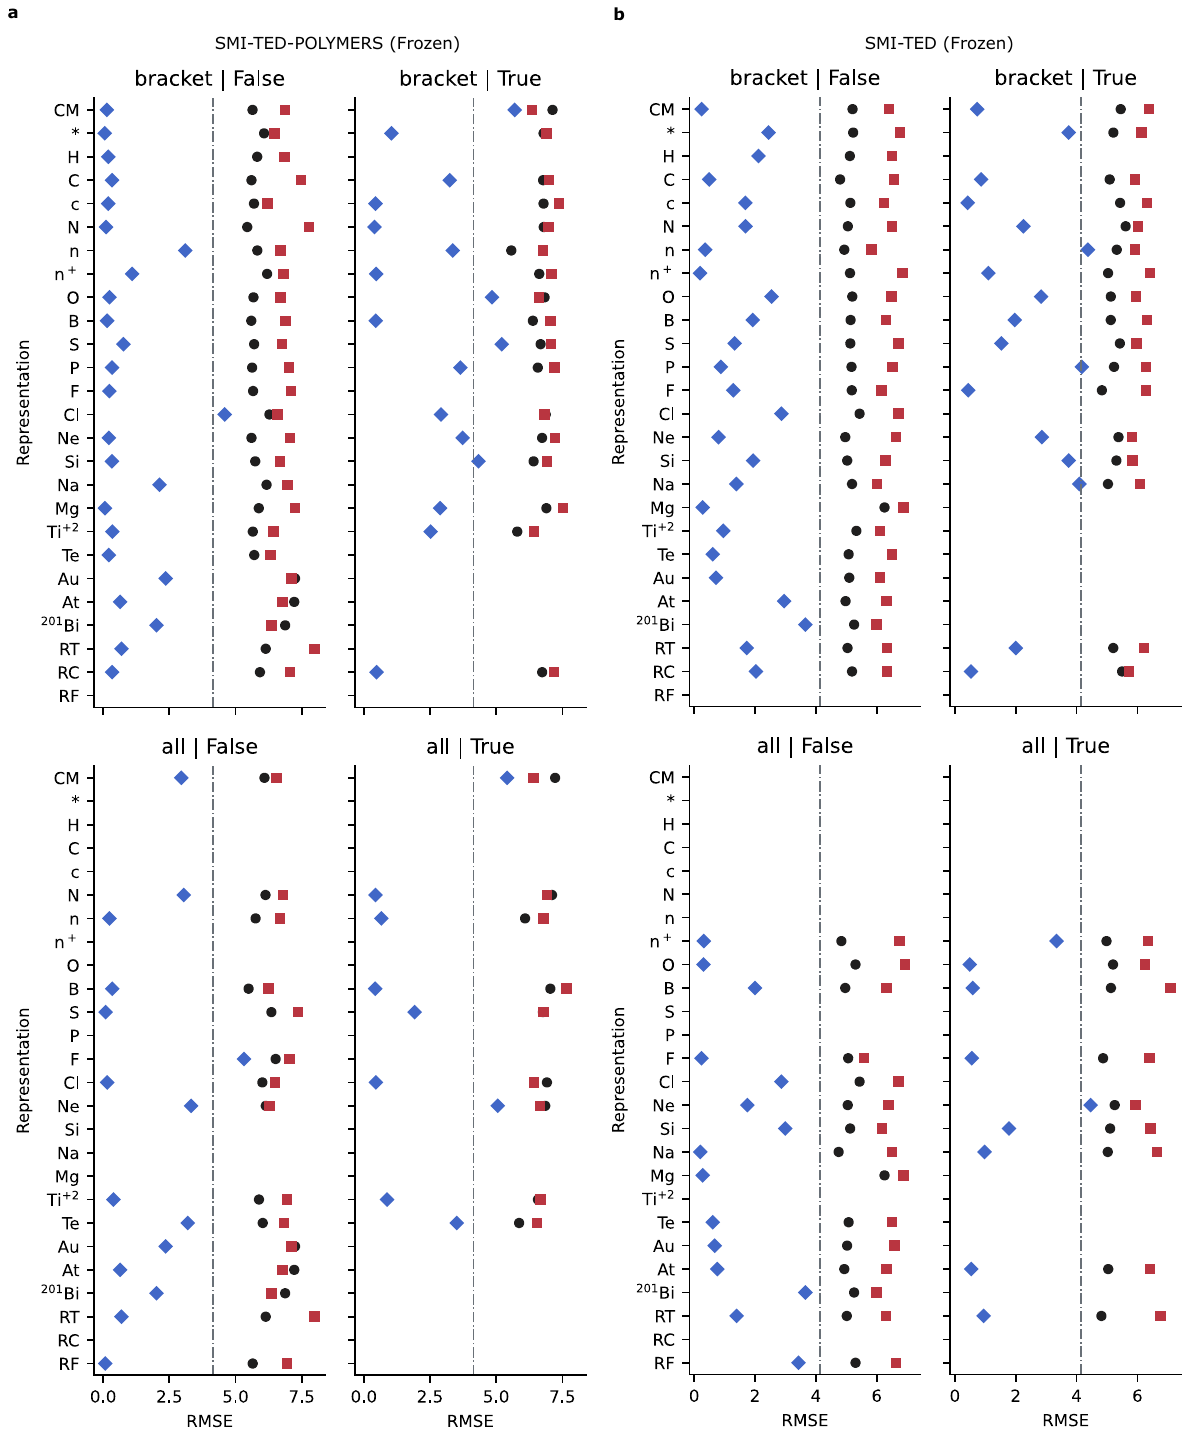}
\caption{Point plots for CO\textsubscript{2}:N\textsubscript{2} gas selectivity benchmark experiments of RMSE using the base random train, valid, and test splits for SMI-TED-POLYMER (\textbf{a}) and SMI-TED (\textbf{b}) models with frozen weights.}\label{netl_co2_n2_token_point_frozen_rmse}
\end{figure}

\begin{figure}[H]
\centering
\includegraphics[width=1\textwidth]{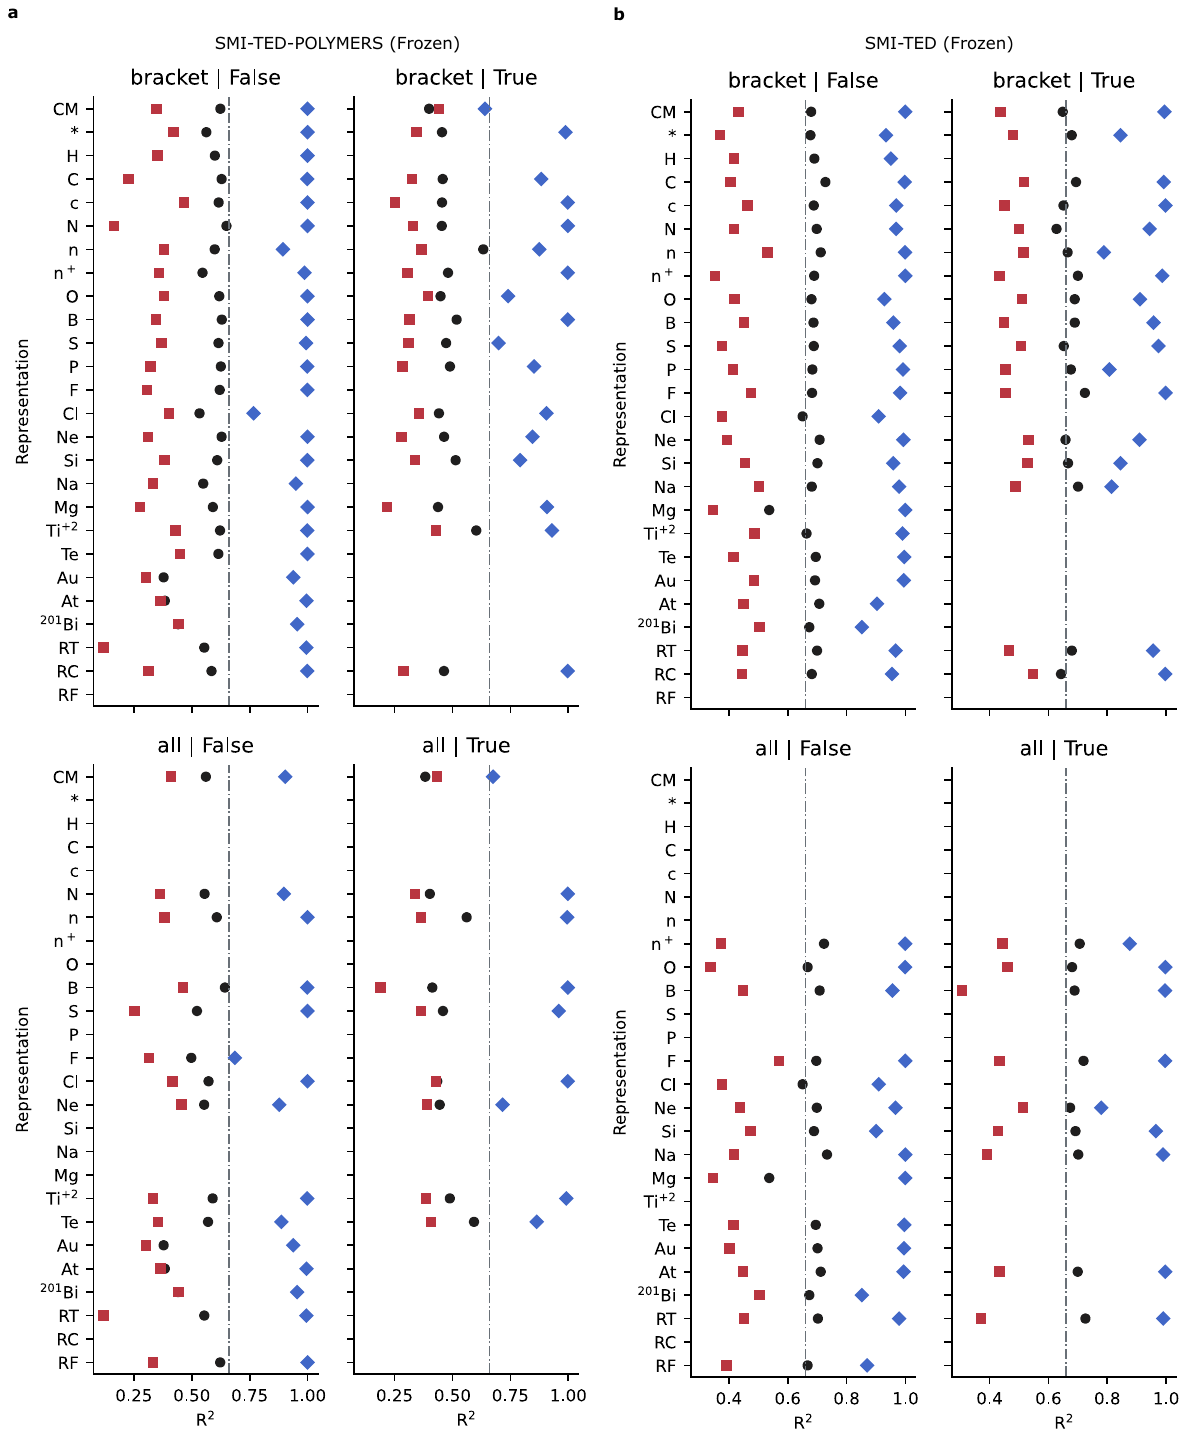}
\caption{Point plots for CO\textsubscript{2}:N\textsubscript{2} gas selectivity benchmark experiments of R\textsuperscript{2} using the base random train, valid, and test splits for SMI-TED-POLYMER (\textbf{a}) and SMI-TED (\textbf{b}) models with frozen weights.}\label{netl_co2_n2_token_point_frozen_r2}
\end{figure}

\begin{figure}[H]
\centering
\includegraphics[width=1\textwidth]{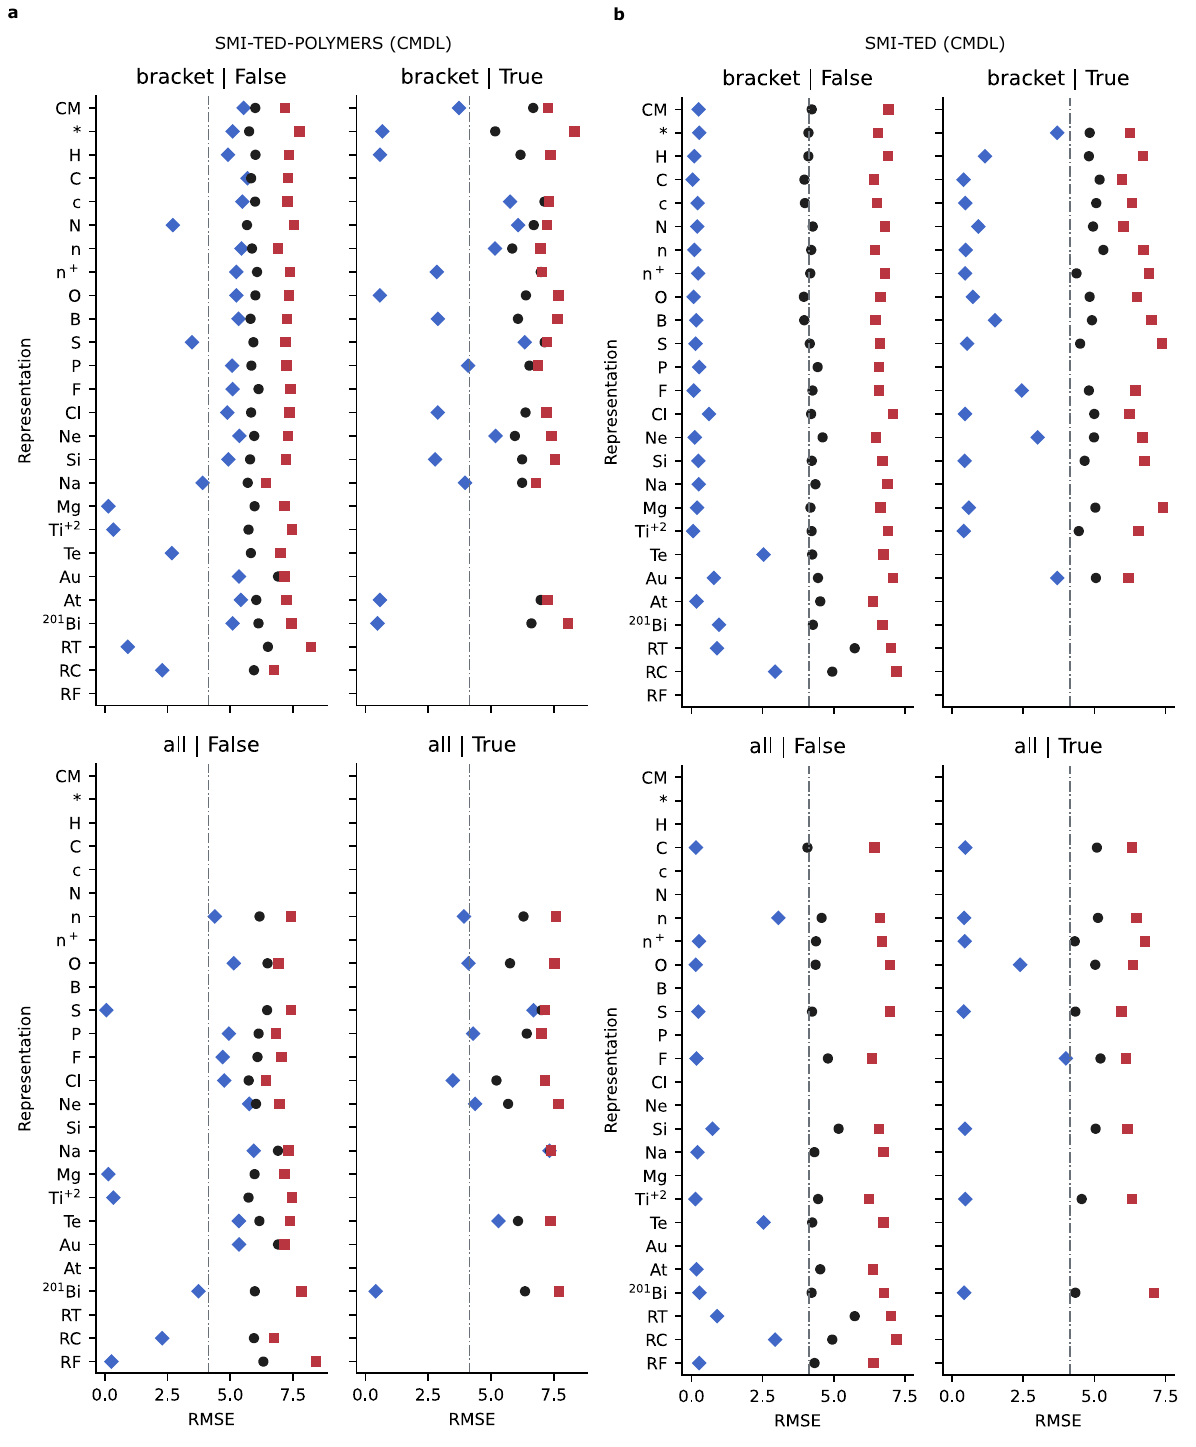}
\caption{Point plots for CO\textsubscript{2}:N\textsubscript{2} gas selectivity benchmark experiments of RMSE using the base random train, valid, and test splits for SMI-TED-POLYMER (\textbf{a}) and SMI-TED (\textbf{b}) models fine-tuned using the CPG representation.}\label{netl_co2_n2_token_point_cmdl_rmse}
\end{figure}

\begin{figure}
\centering
\includegraphics[width=1\textwidth]{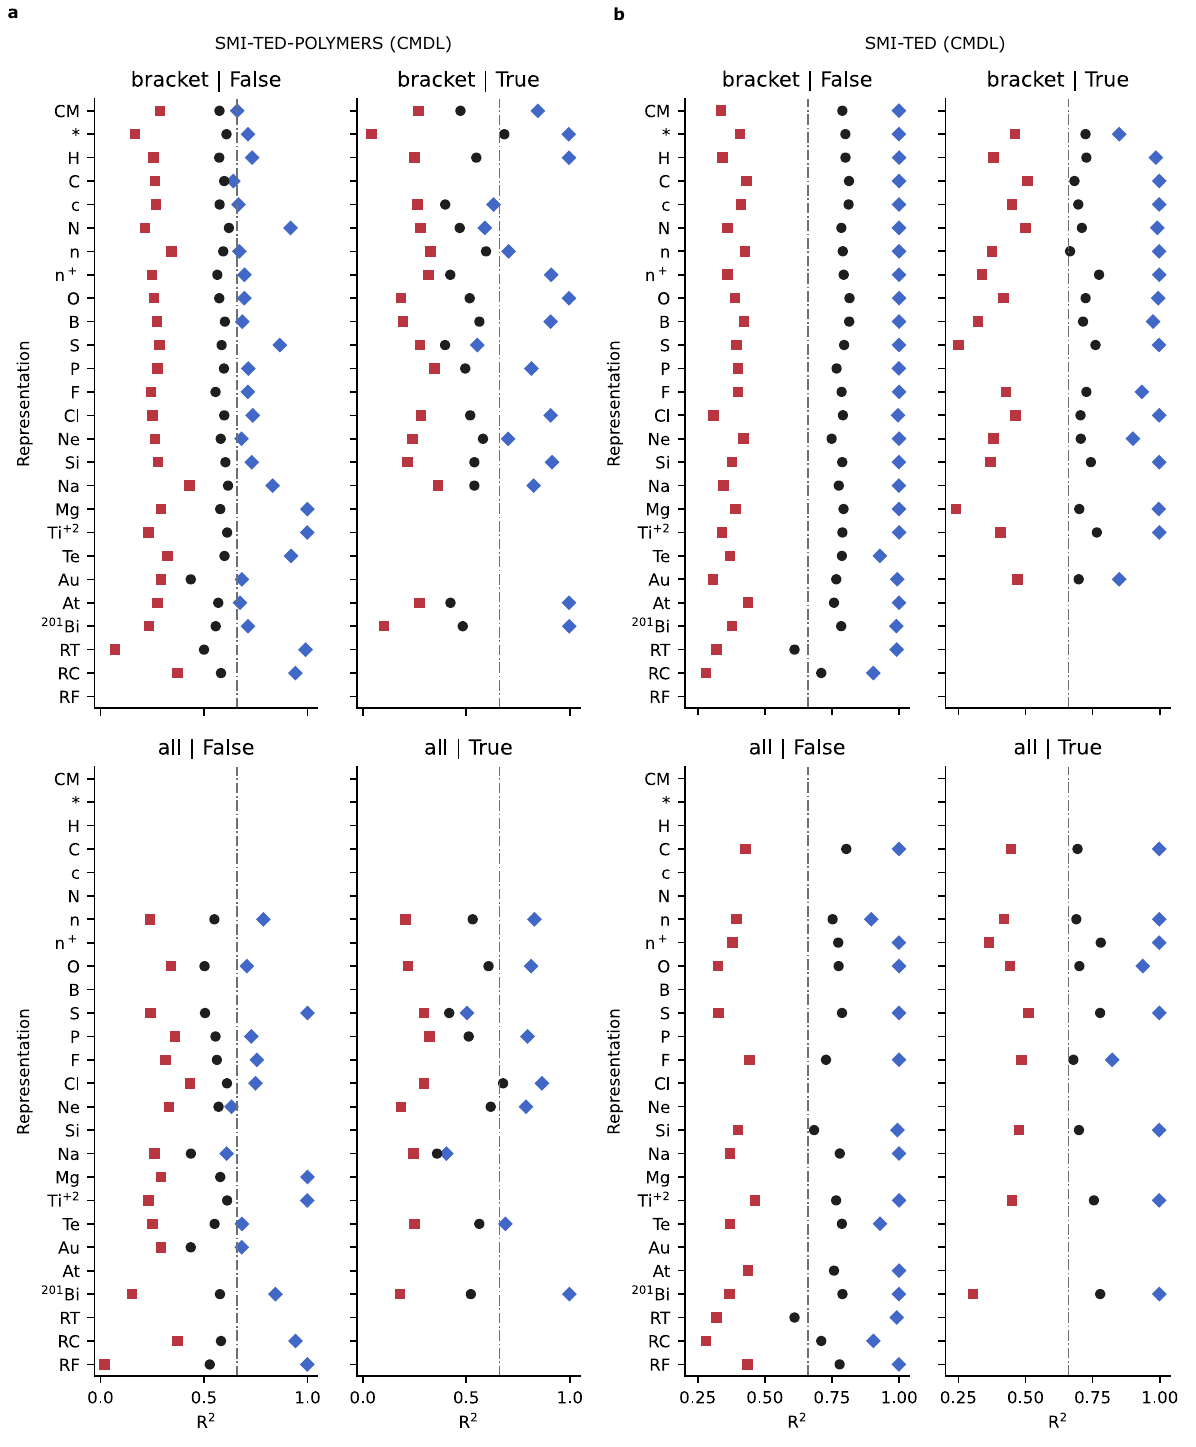}
\caption{Point plots for CO\textsubscript{2}:N\textsubscript{2} gas selectivity benchmark experiments of R\textsuperscript{2} using the base random train, valid, and test splits for SMI-TED-POLYMER (\textbf{a}) and SMI-TED (\textbf{b}) models fine-tuned using the CPG representation.}\label{netl_co2_n2_token_point_cmdl_r2}
\end{figure}

\begin{figure}[H]
\centering
\includegraphics[width=1\textwidth]{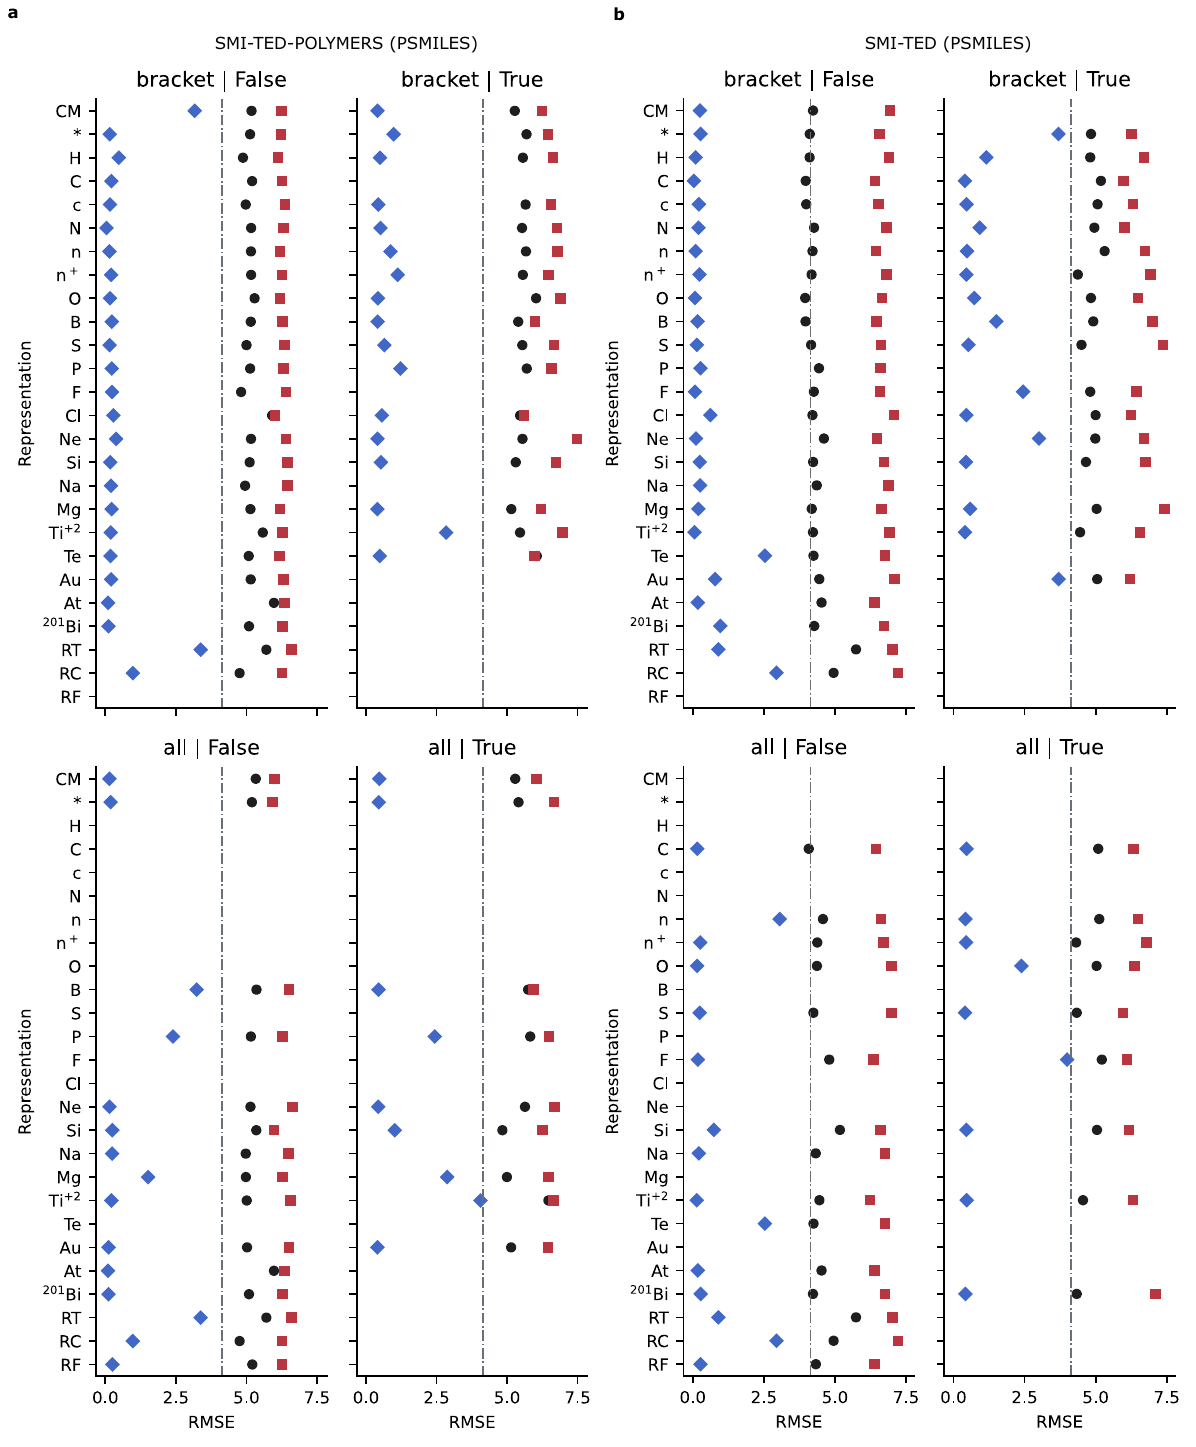}
\caption{Point plots for CO\textsubscript{2}:N\textsubscript{2} gas selectivity benchmark experiments of RMSE using the base random train, valid, and test splits for SMI-TED-POLYMER (\textbf{a}) and SMI-TED (\textbf{b}) models fine-tuned using PSMILES.}\label{netl_co2_n2_token_point_psmiles_rmse}
\end{figure}

\end{document}
