# Supplementary material for: Understanding Structural Representation in Foundation Models for Polymers
Source: arXiv:2512.11881 source file (2026-09-18)
Supplement: Supplementary file 10 [file netl_ch4.tex]

\subsubsection{CH\textsubscript{4} Gas Permeability CV Scores}\label{cv_netl_ch4}

\begin{figure}[H]
\centering
\includegraphics[width=1\textwidth]{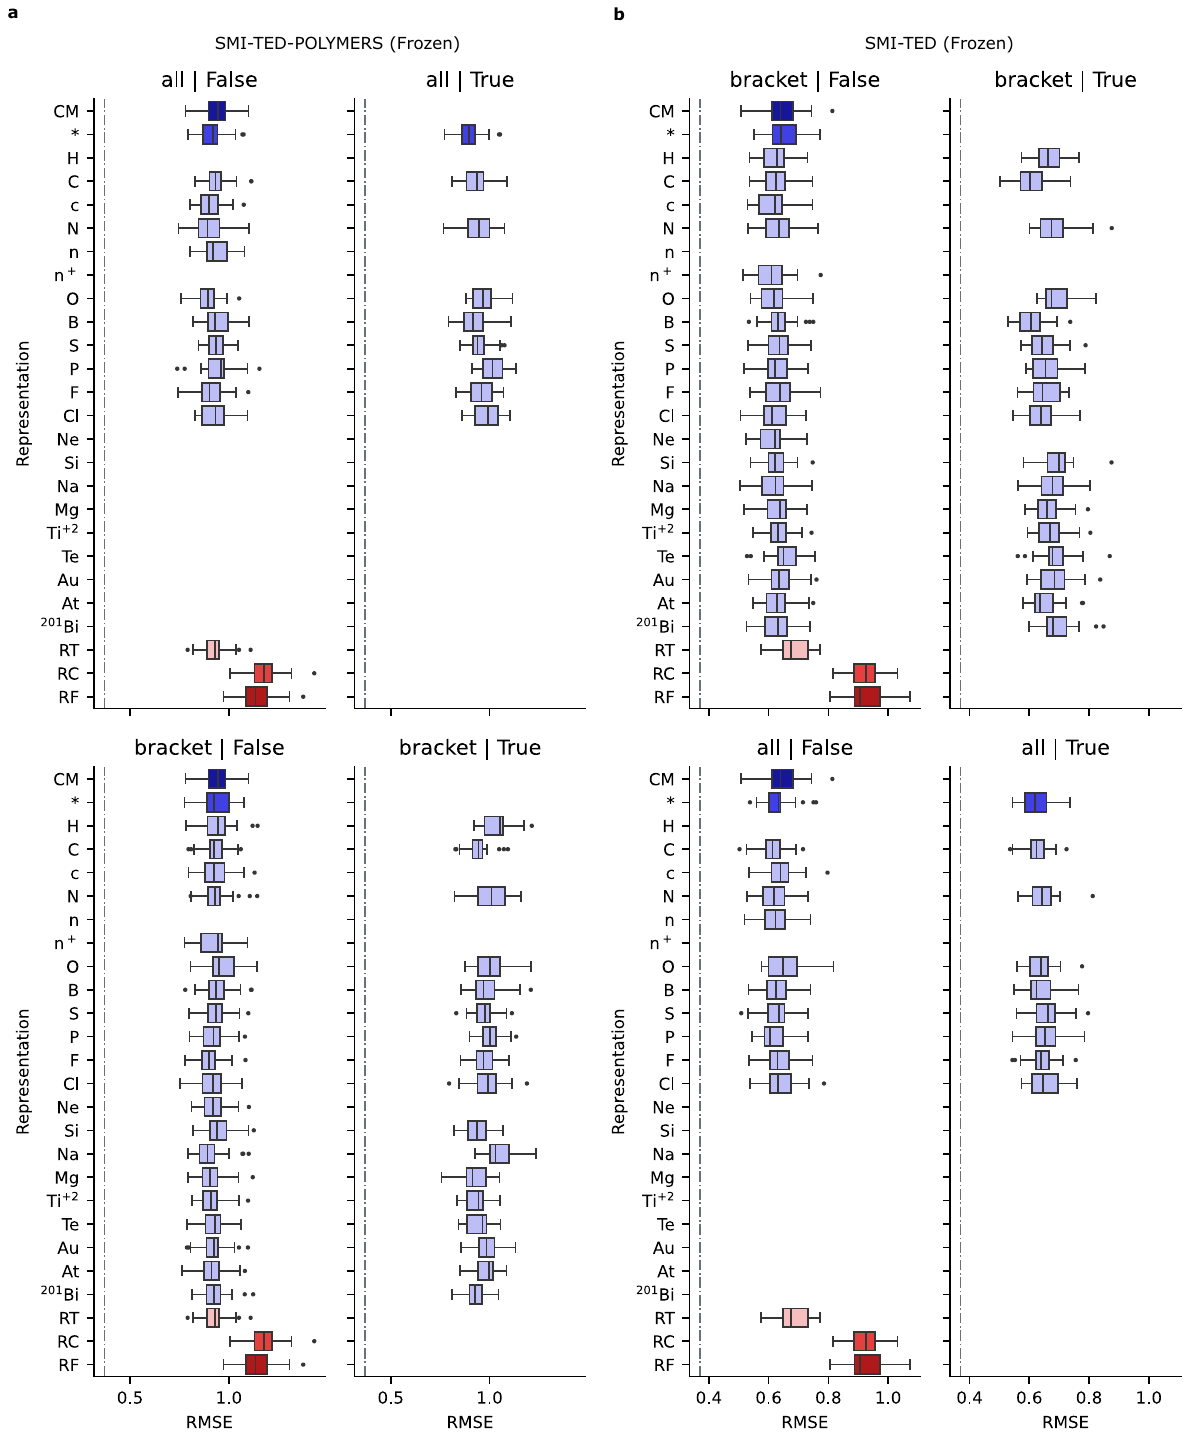}
\caption{Box plots for CH\textsubscript{4} gas permeability repeated cross-validation experiments for SMI-TED-POLYMER (\textbf{a}) and SMI-TED (\textbf{b}) models with frozen weights.}\label{netl_ch4_token_box_frozen}
\end{figure}

\begin{figure}[H]
\centering
\includegraphics[width=1\textwidth]{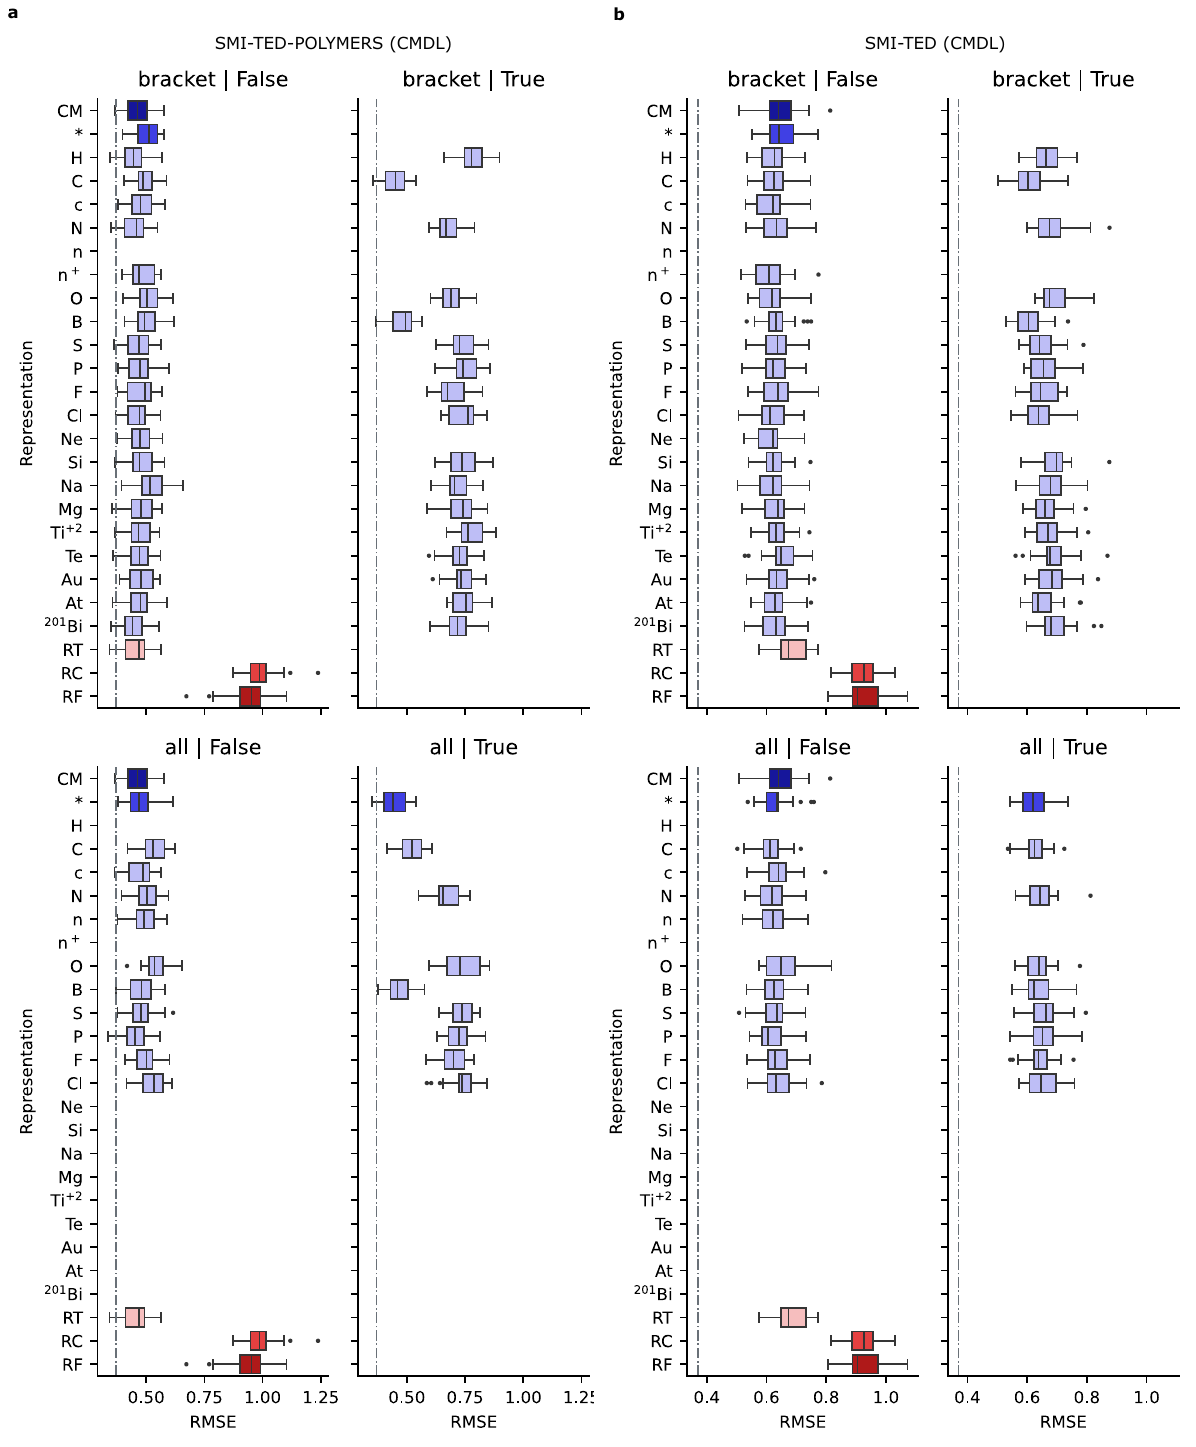}
\caption{Box plots for CH\textsubscript{4} gas permeability repeated cross-validation experiments for SMI-TED-POLYMER (\textbf{a}) and SMI-TED (\textbf{b}) models fine-tuned with the CPG polymer graphs.}\label{netl_ch4_token_box_cmdl}
\end{figure}

\begin{figure}[H]
\centering
\includegraphics[width=1\textwidth]{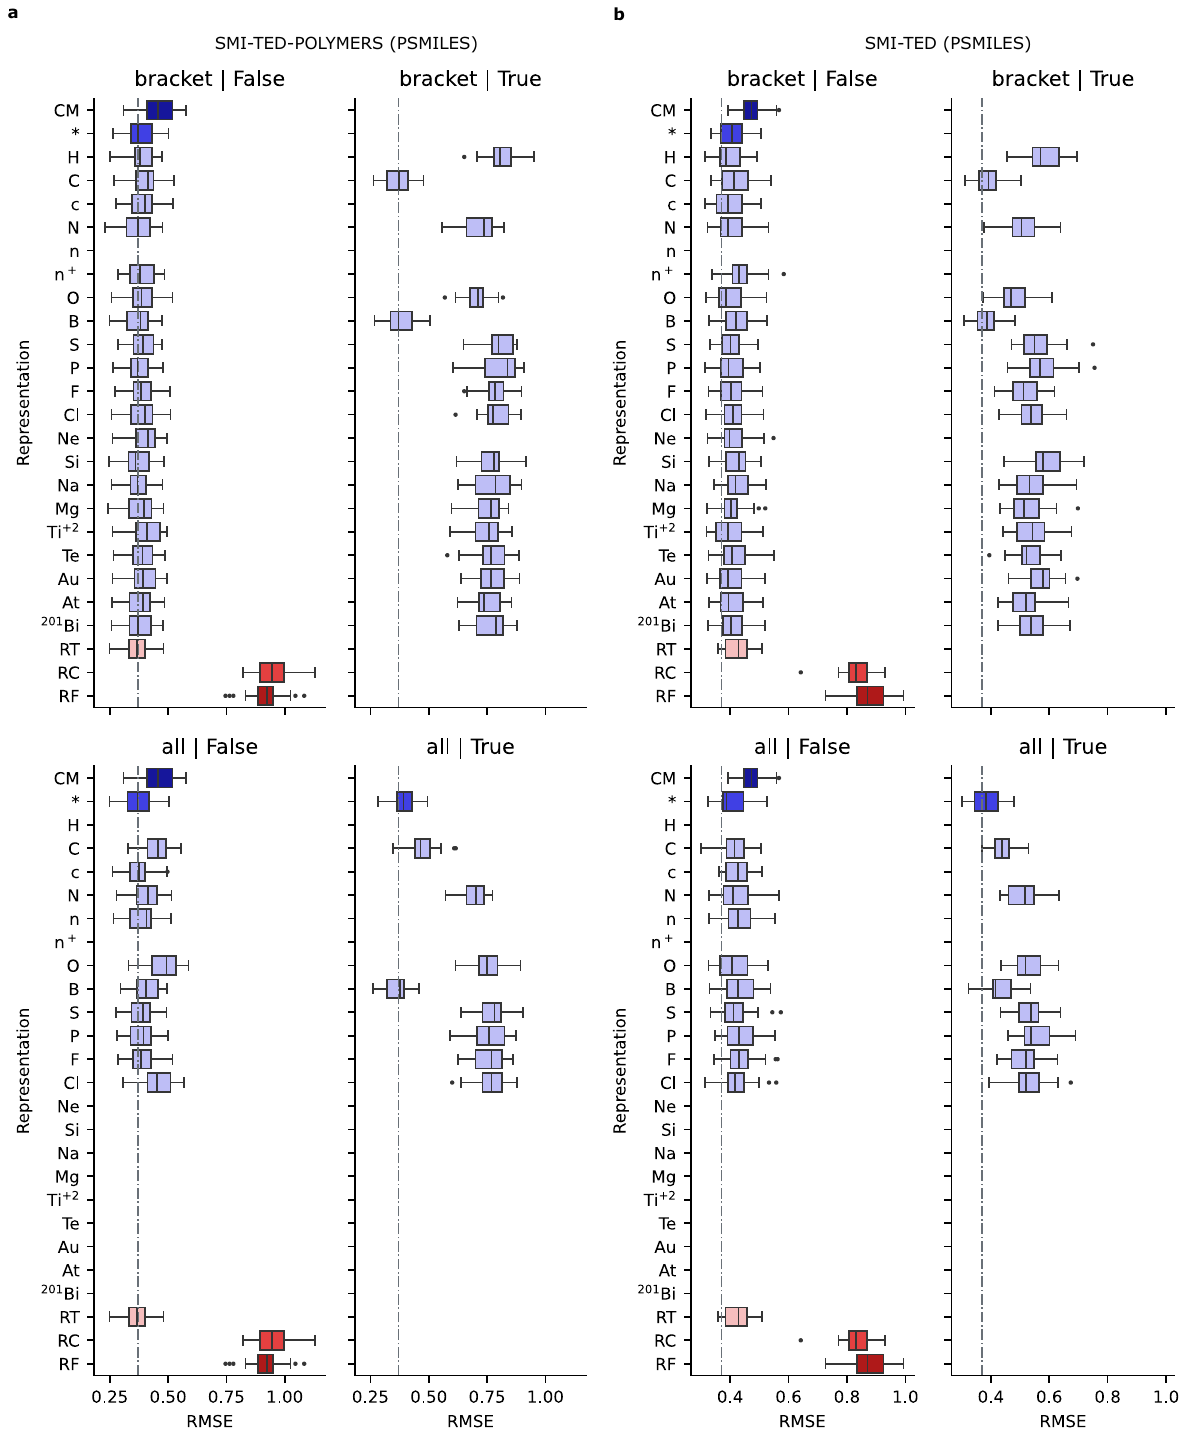}
\caption{Box plots for CH\textsubscript{4} gas permeability repeated cross-validation experiments for SMI-TED-POLYMER (\textbf{a}) and SMI-TED (\textbf{b}) models fine-tuned with PSMILES.}\label{netl_ch4_token_box_psmiles}
\end{figure}

\subsubsection{CH\textsubscript{4} Gas Permeability Random Split Scores}\label{rand_netl_ch4}

\begin{figure}[H]
\centering
\includegraphics[width=1\textwidth]{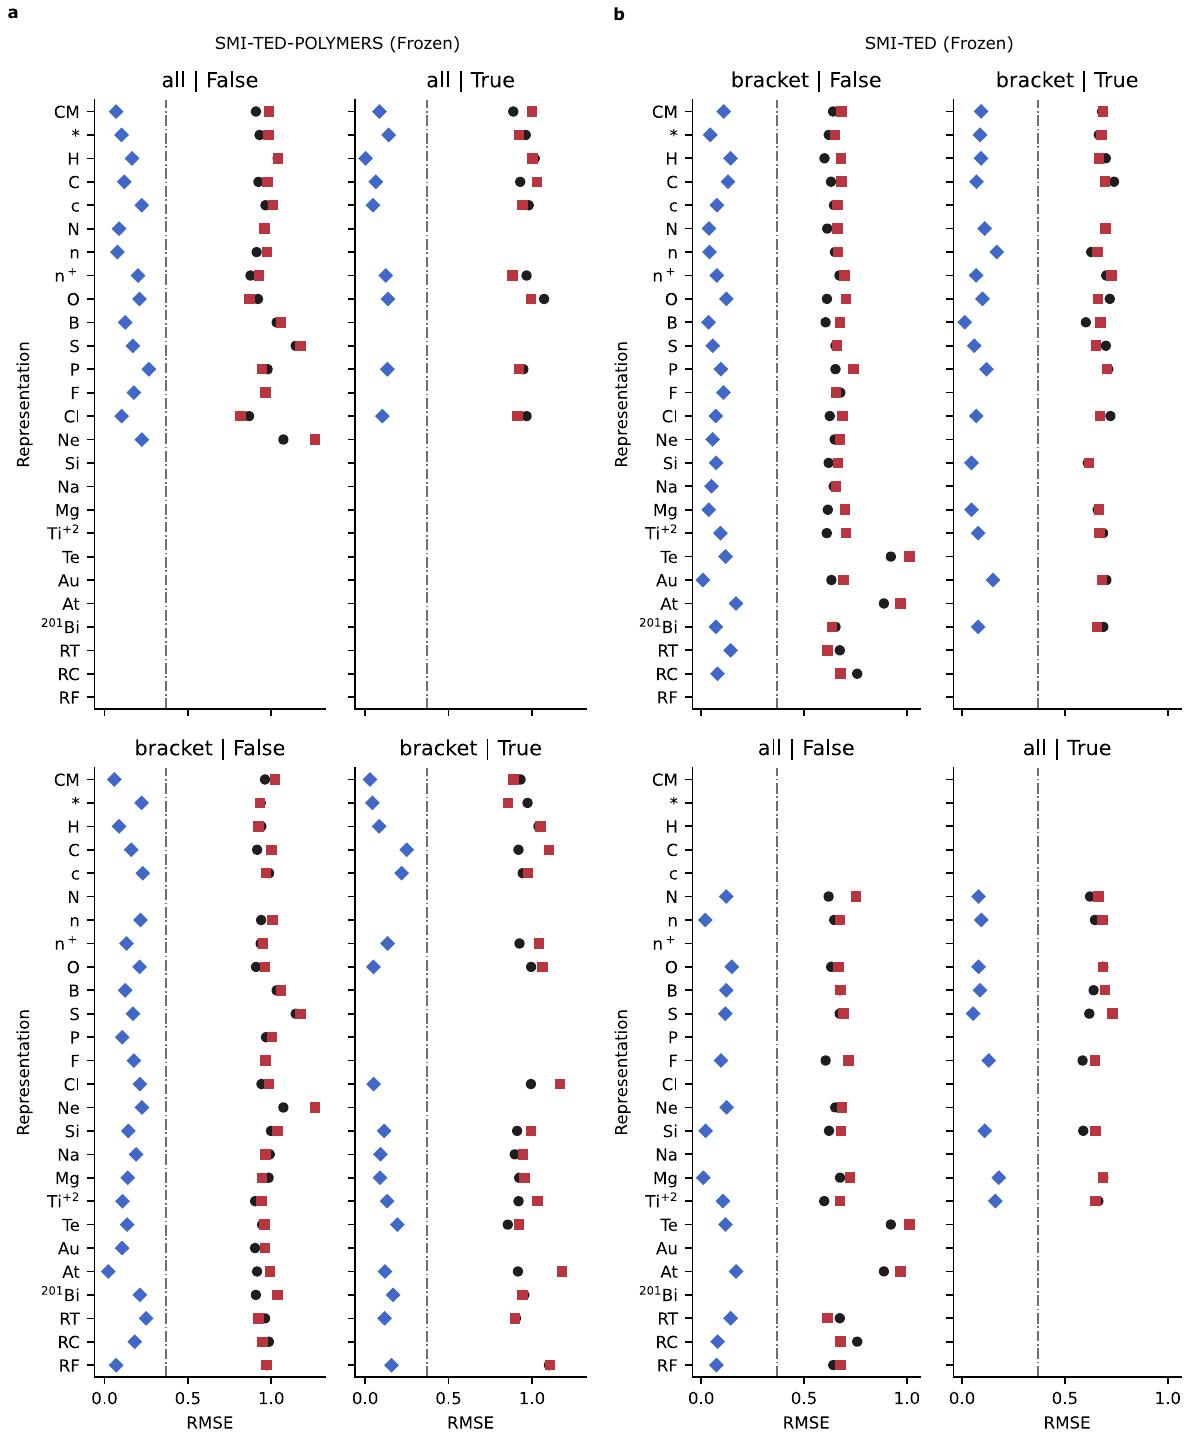}
\caption{Point plots for CH\textsubscript{4} gas permeability benchmark experiments of RMSE using the base random train, valid, and test splits for SMI-TED-POLYMER (\textbf{a}) and SMI-TED (\textbf{b}) models with frozen weights.}\label{netl_ch4_token_point_frozen_rmse}
\end{figure}

\begin{figure}[H]
\centering
\includegraphics[width=1\textwidth]{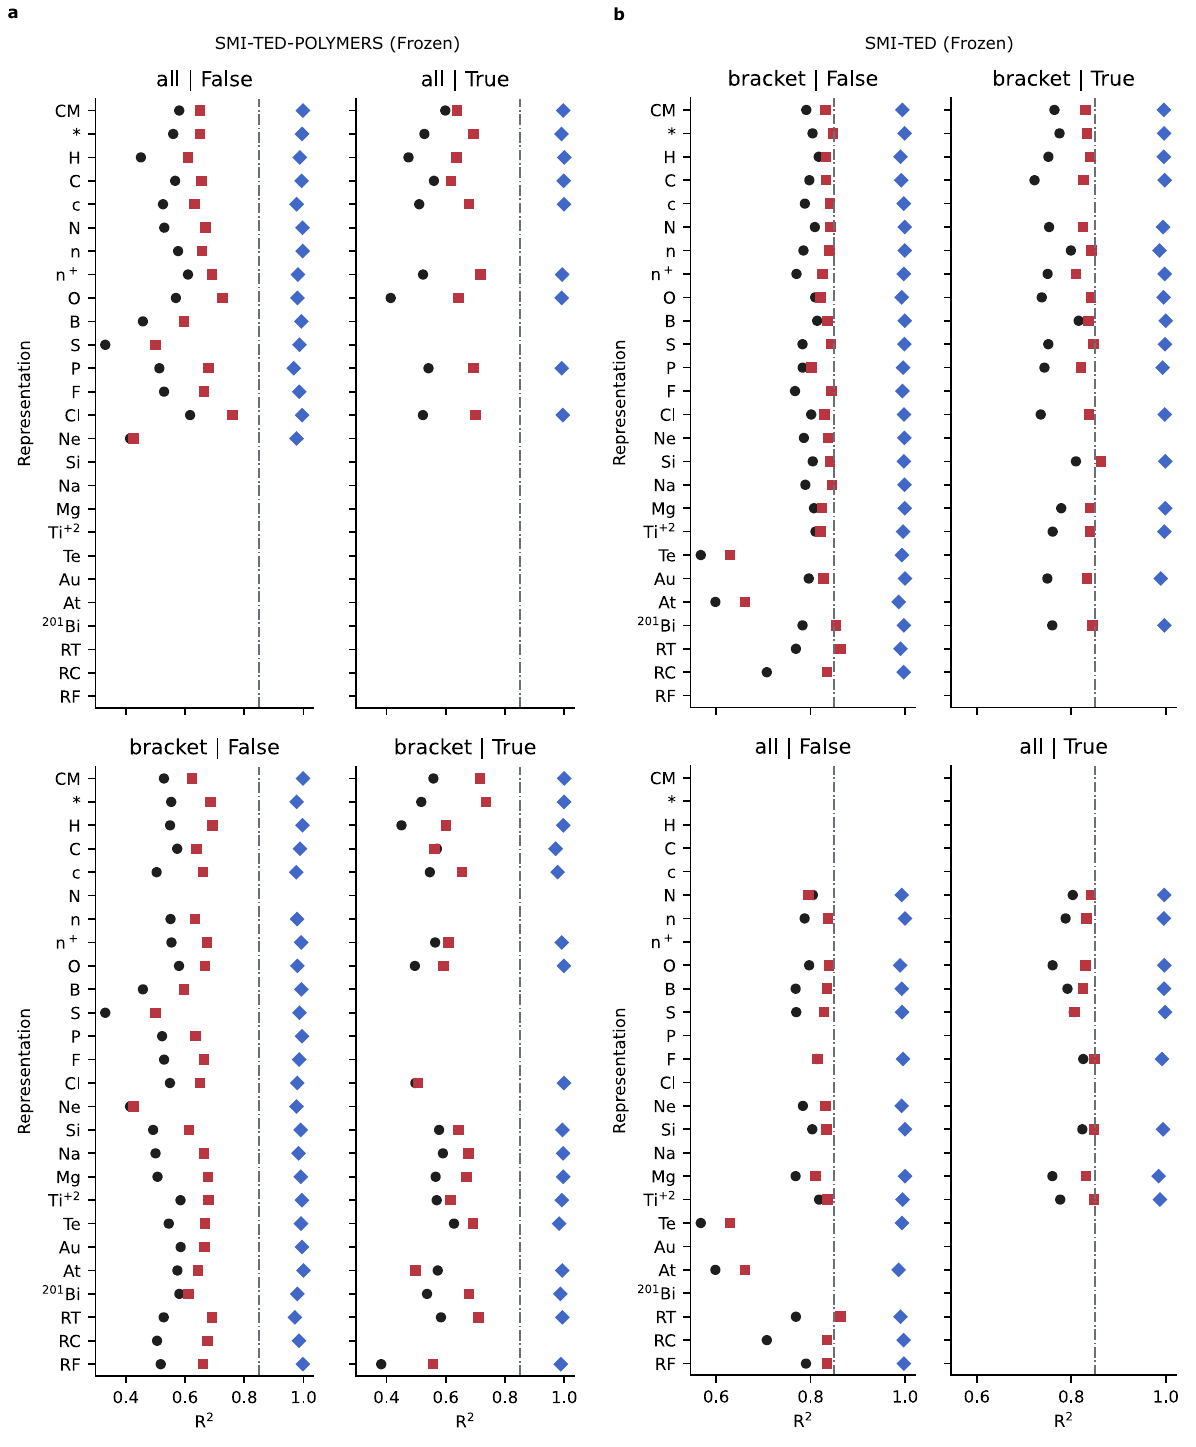}
\caption{Point plots for CH\textsubscript{4} gas permeability benchmark experiments of R\textsuperscript{2} using the base random train, valid, and test splits for SMI-TED-POLYMER (\textbf{a}) and SMI-TED (\textbf{b}) models with frozen weights.}\label{netl_ch4_token_point_frozen_r2}
\end{figure}

\begin{figure}[H]
\centering
\includegraphics[width=1\textwidth]{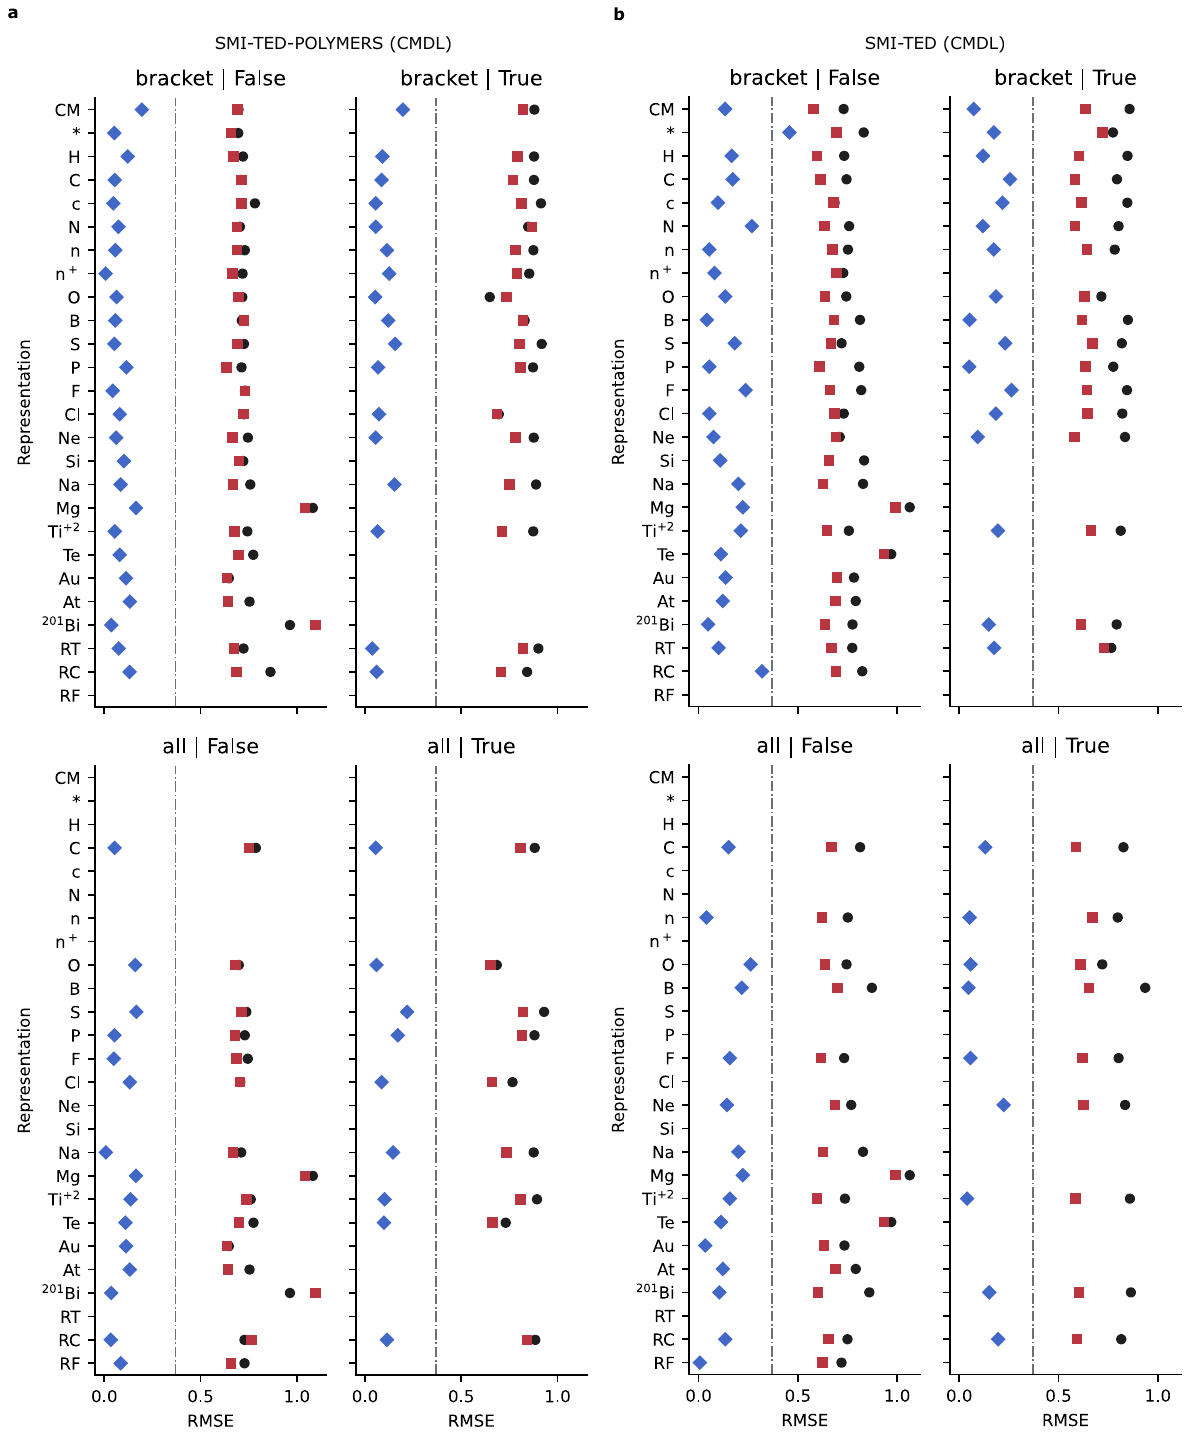}
\caption{Point plots for CH\textsubscript{4} gas permeability benchmark experiments of RMSE using the base random train, valid, and test splits for SMI-TED-POLYMER (\textbf{a}) and SMI-TED (\textbf{b}) models fine-tuned using the CPG representation.}\label{netl_ch4_token_point_cmdl_rmse}
\end{figure}

\begin{figure}
\centering
\includegraphics[width=1\textwidth]{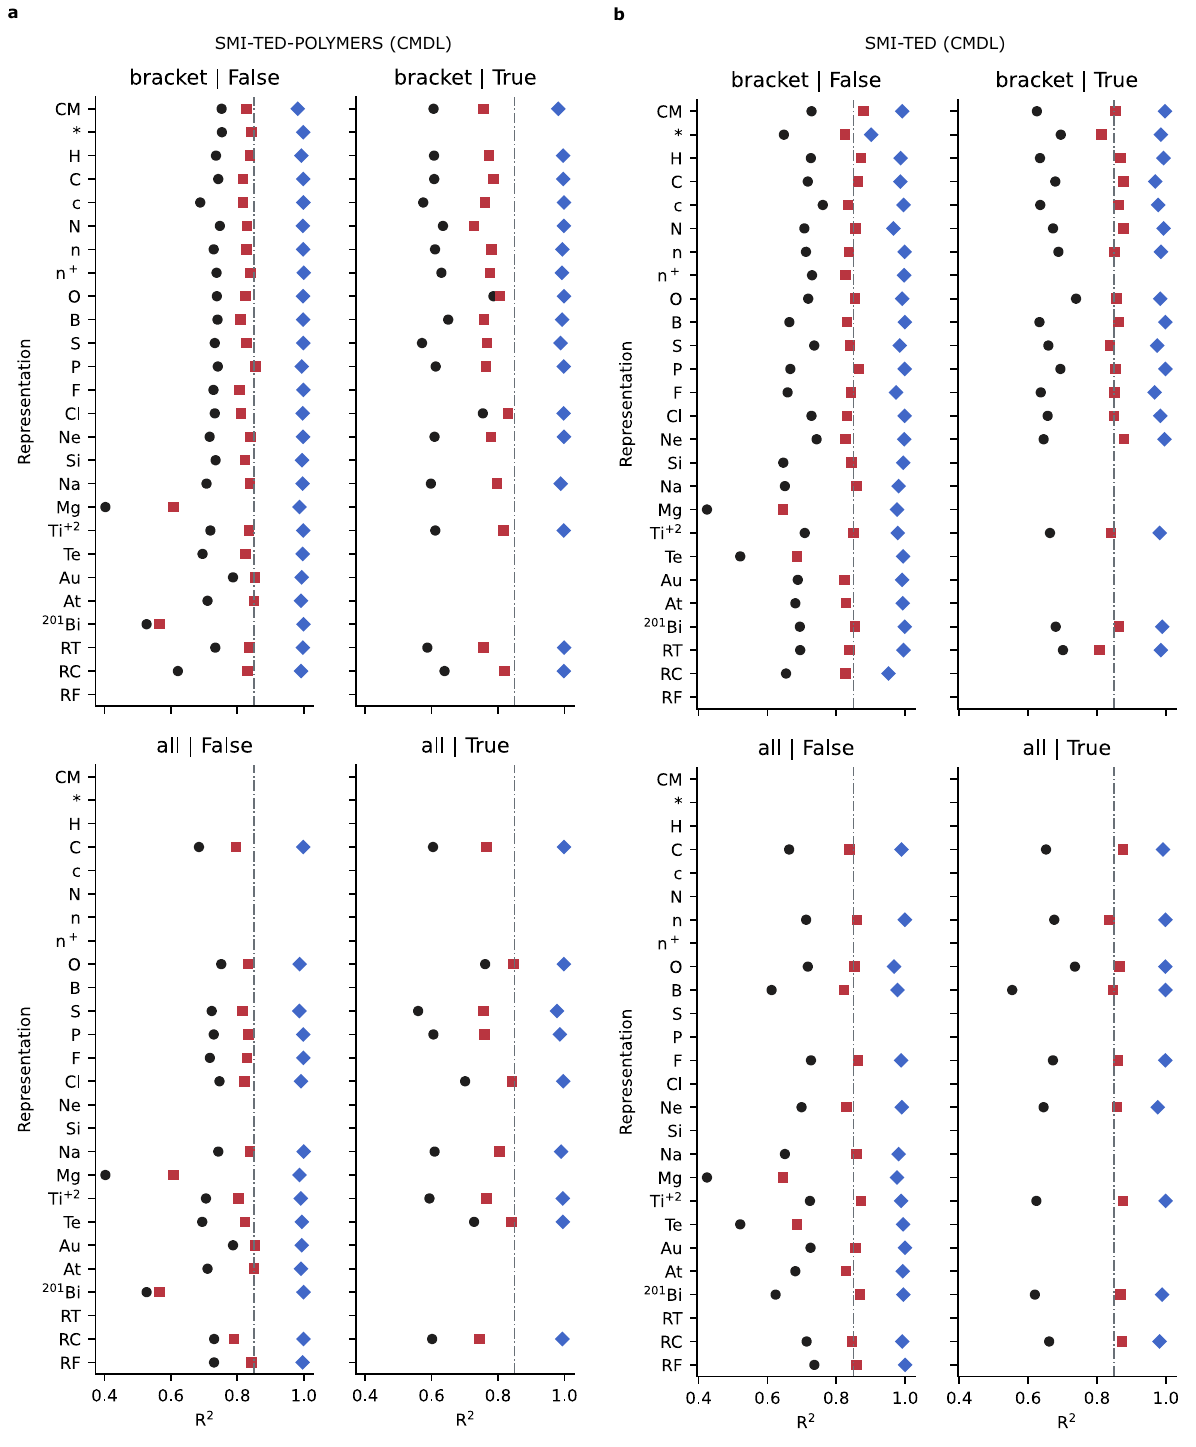}
\caption{Point plots for CH\textsubscript{4} gas permeability benchmark experiments of R\textsuperscript{2} using the base random train, valid, and test splits for SMI-TED-POLYMER (\textbf{a}) and SMI-TED (\textbf{b}) models fine-tuned using the CPG representation.}\label{netl_ch4_token_point_cmdl_r2}
\end{figure}

\begin{figure}[H]
\centering
\includegraphics[width=1\textwidth]{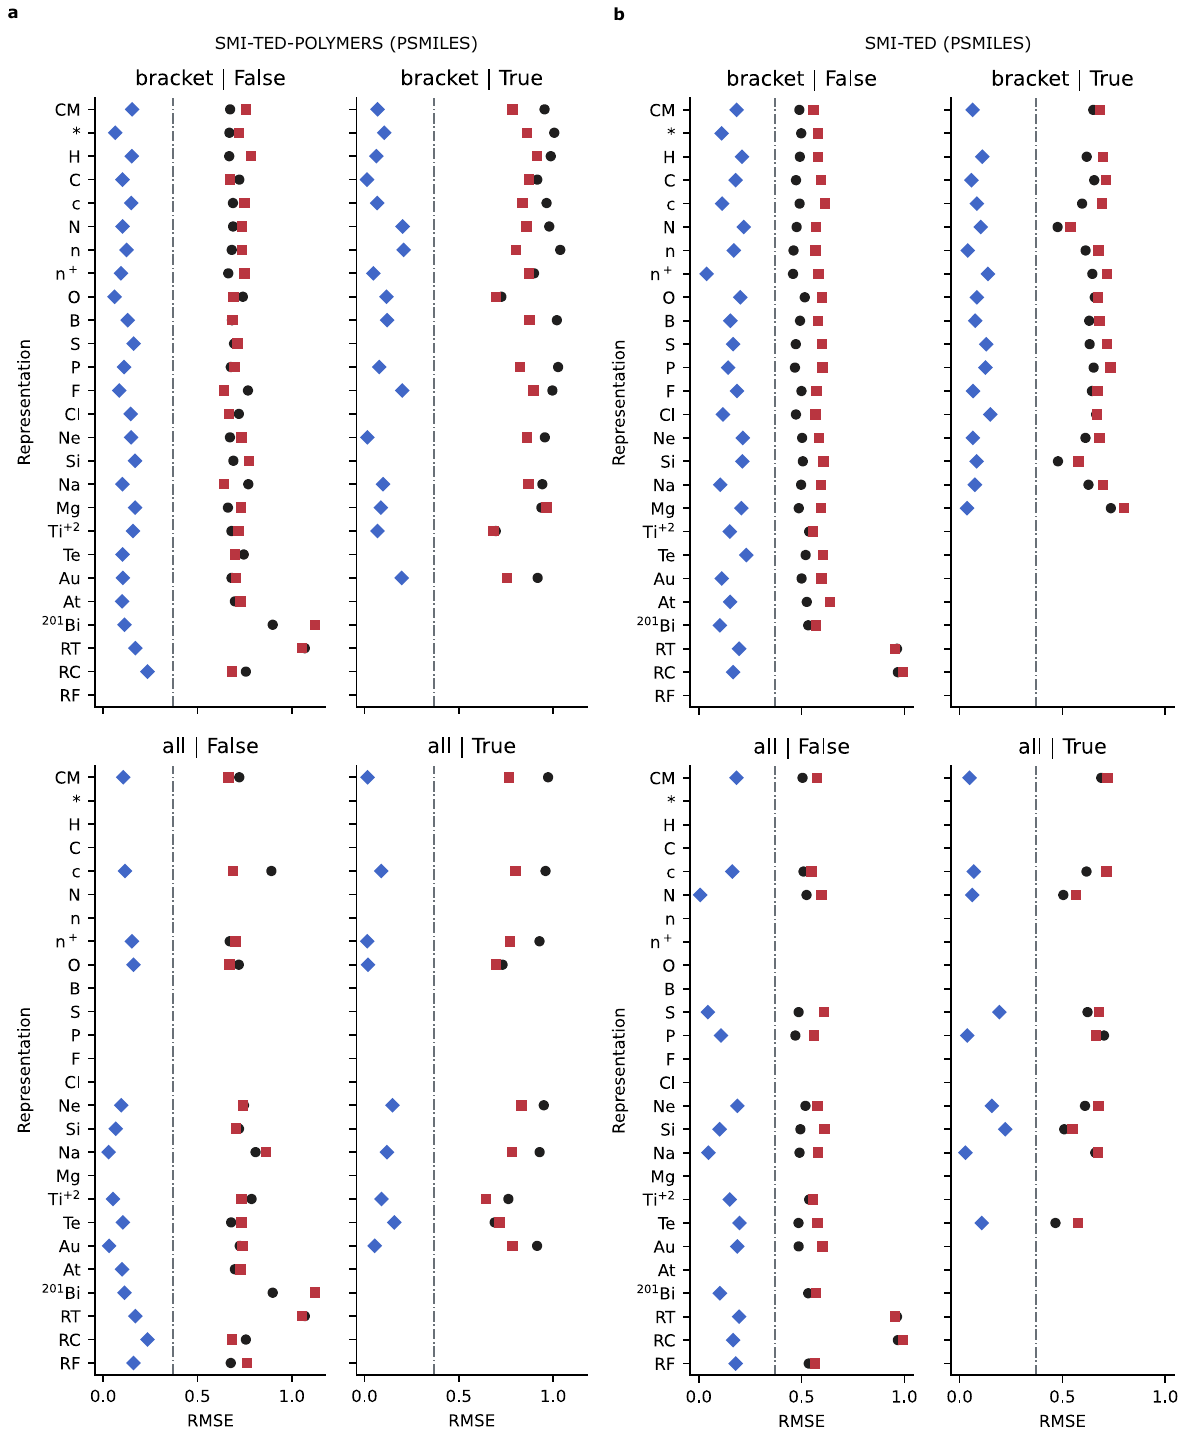}
\caption{Point plots for CH\textsubscript{4} gas permeability benchmark experiments of RMSE using the base random train, valid, and test splits for SMI-TED-POLYMER (\textbf{a}) and SMI-TED (\textbf{b}) models fine-tuned using PSMILES.}\label{netl_ch4_token_point_psmiles_rmse}
\end{figure}
