# Supplementary material for: Understanding Structural Representation in Foundation Models for Polymers
Source: arXiv:2512.11881 source file (2026-09-18)
Supplement: Supplementary file 15 [file xc_si.tex]

\subsubsection{Crystallization Tendency (X\textsubscript{c}) CV Scores}\label{cvXc}

\begin{figure}[H]
\centering
\includegraphics[width=1\textwidth]{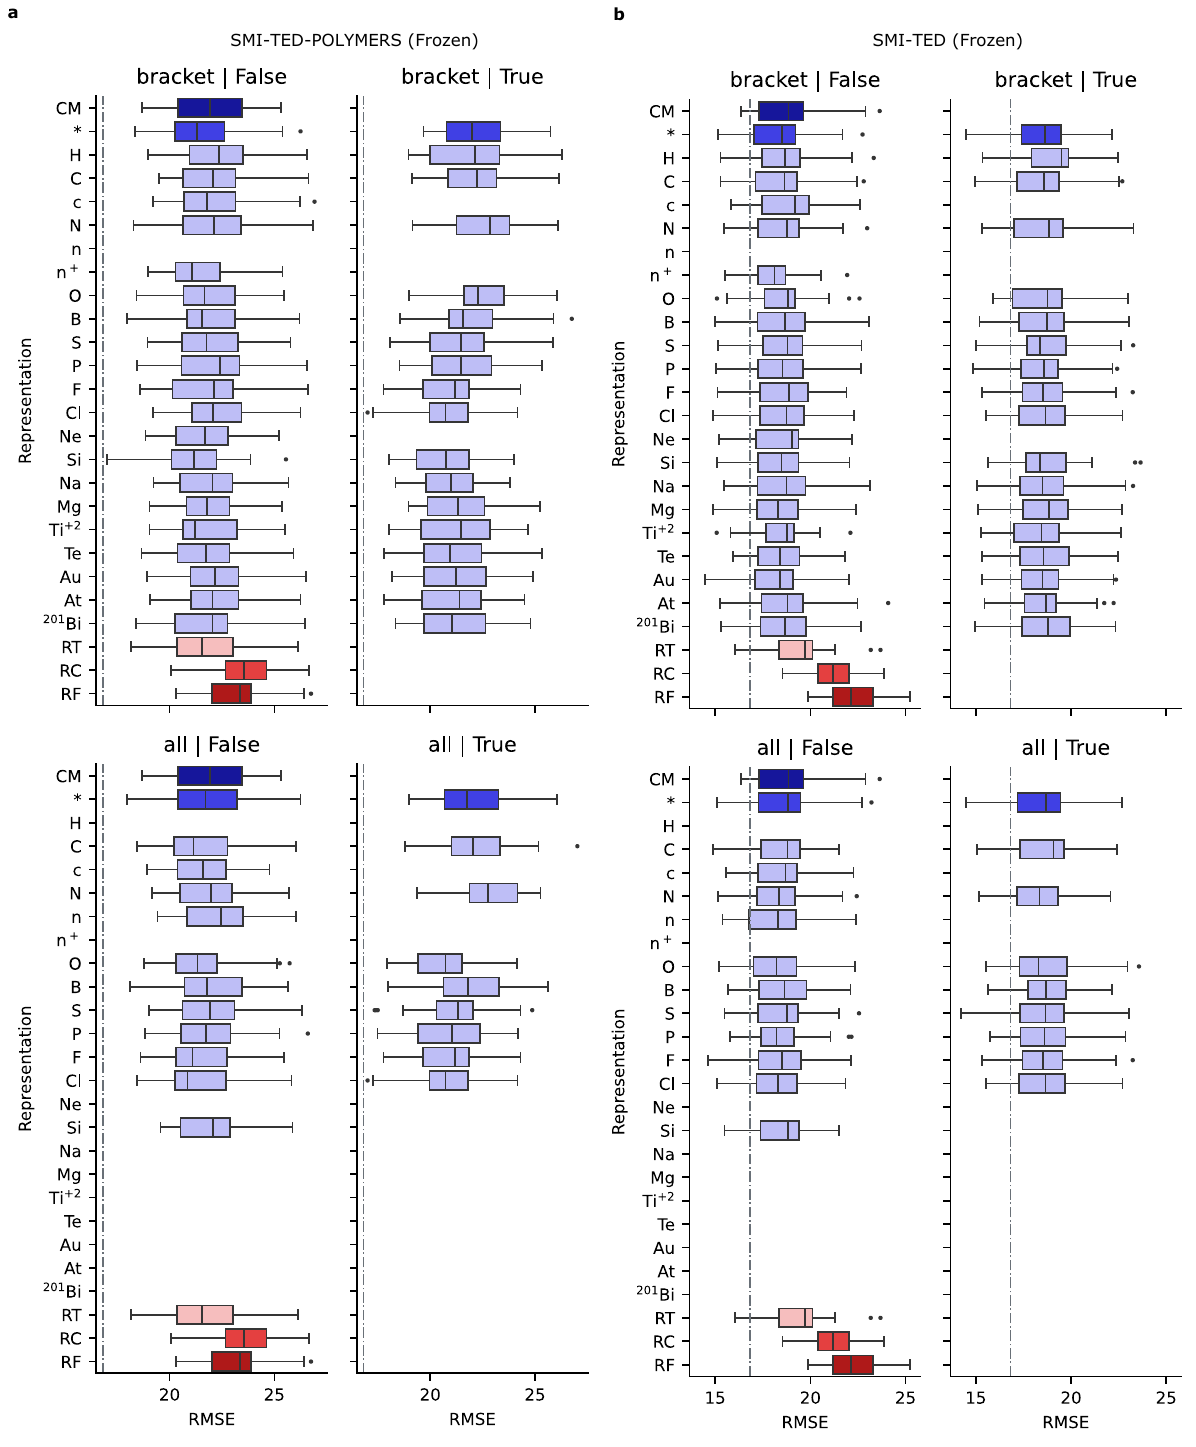}
\caption{Box plots for X\textsubscript{c} repeated cross-validation experiments for SMI-TED-POLYMER (\textbf{a}) and SMI-TED (\textbf{b}) models with frozen weights.}\label{xc_token_box_frozen}
\end{figure}

\begin{figure}[H]
\centering
\includegraphics[width=1\textwidth]{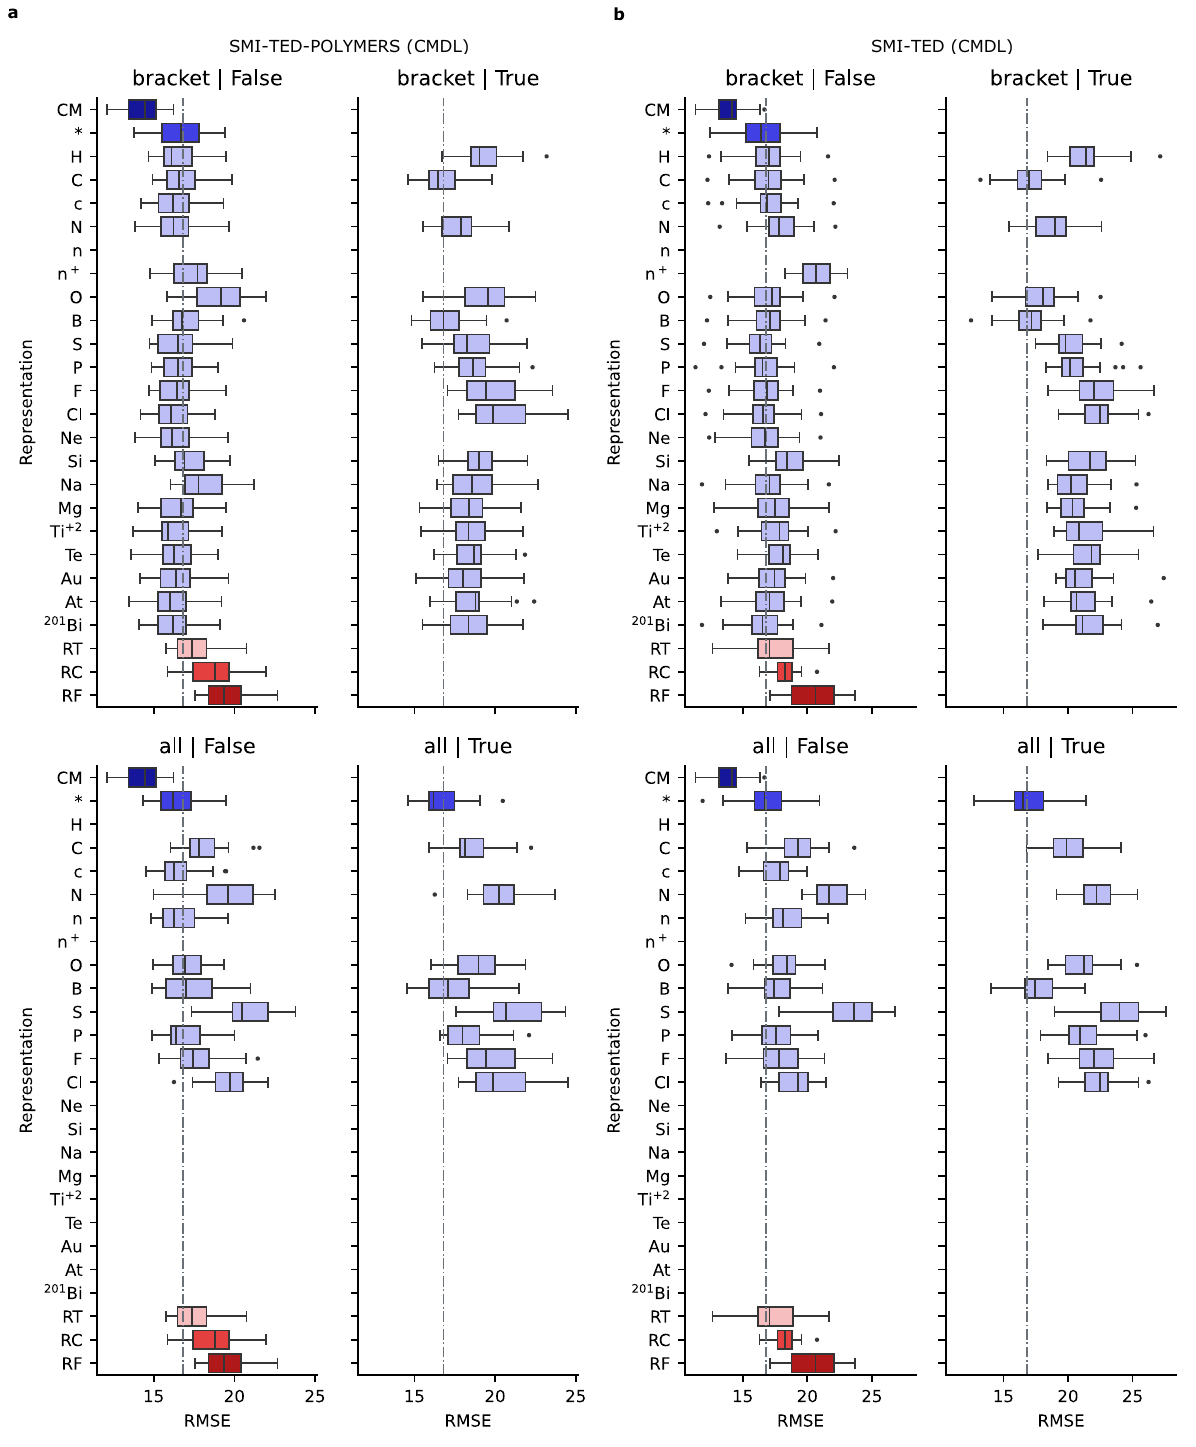}
\caption{Box plots for X\textsubscript{c} repeated cross-validation experiments for SMI-TED-POLYMER (\textbf{a}) and SMI-TED (\textbf{b}) models fine-tuned with the CPG polymer graphs.}\label{xc_token_box_cmdl}
\end{figure}

\begin{figure}[H]
\centering
\includegraphics[width=1\textwidth]{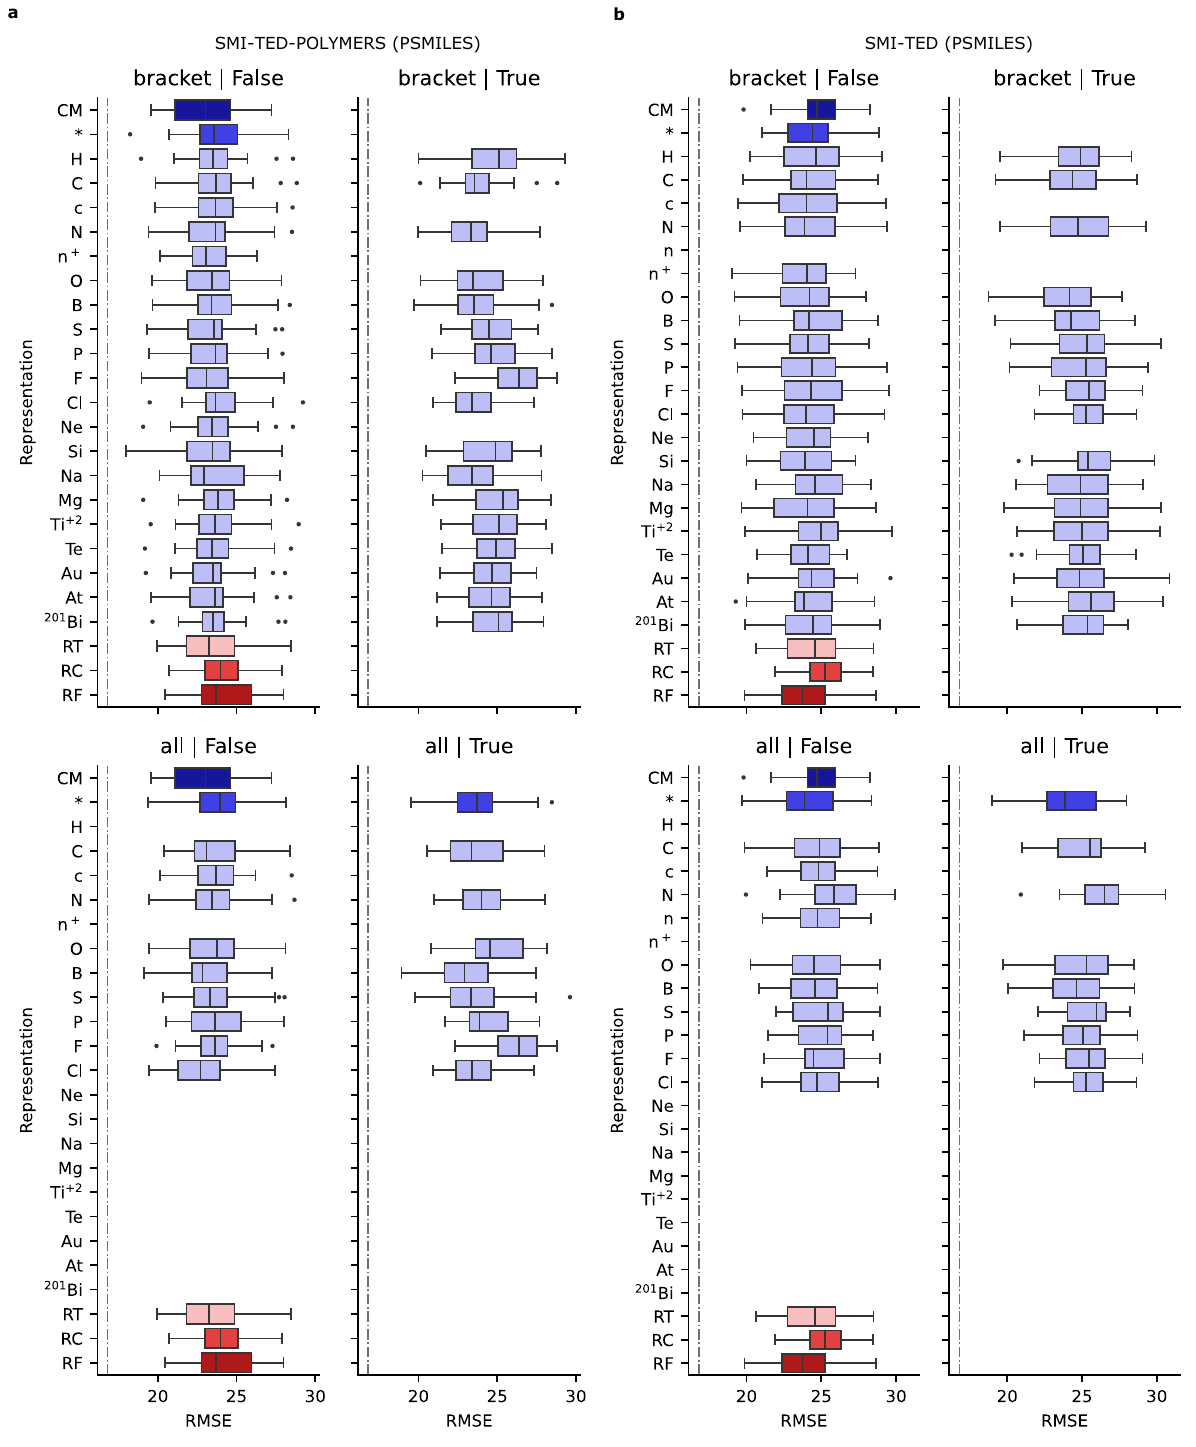}
\caption{Box plots for X\textsubscript{c} repeated cross-validation experiments for SMI-TED-POLYMER (\textbf{a}) and SMI-TED (\textbf{b}) models fine-tuned with PSMILES.}\label{xc_token_box_psmiles}
\end{figure}

\subsubsection{Crystallization Tendency (X\textsubscript{c}) Random Split Scores}\label{randXc}

\begin{figure}[H]
\centering
\includegraphics[width=1\textwidth]{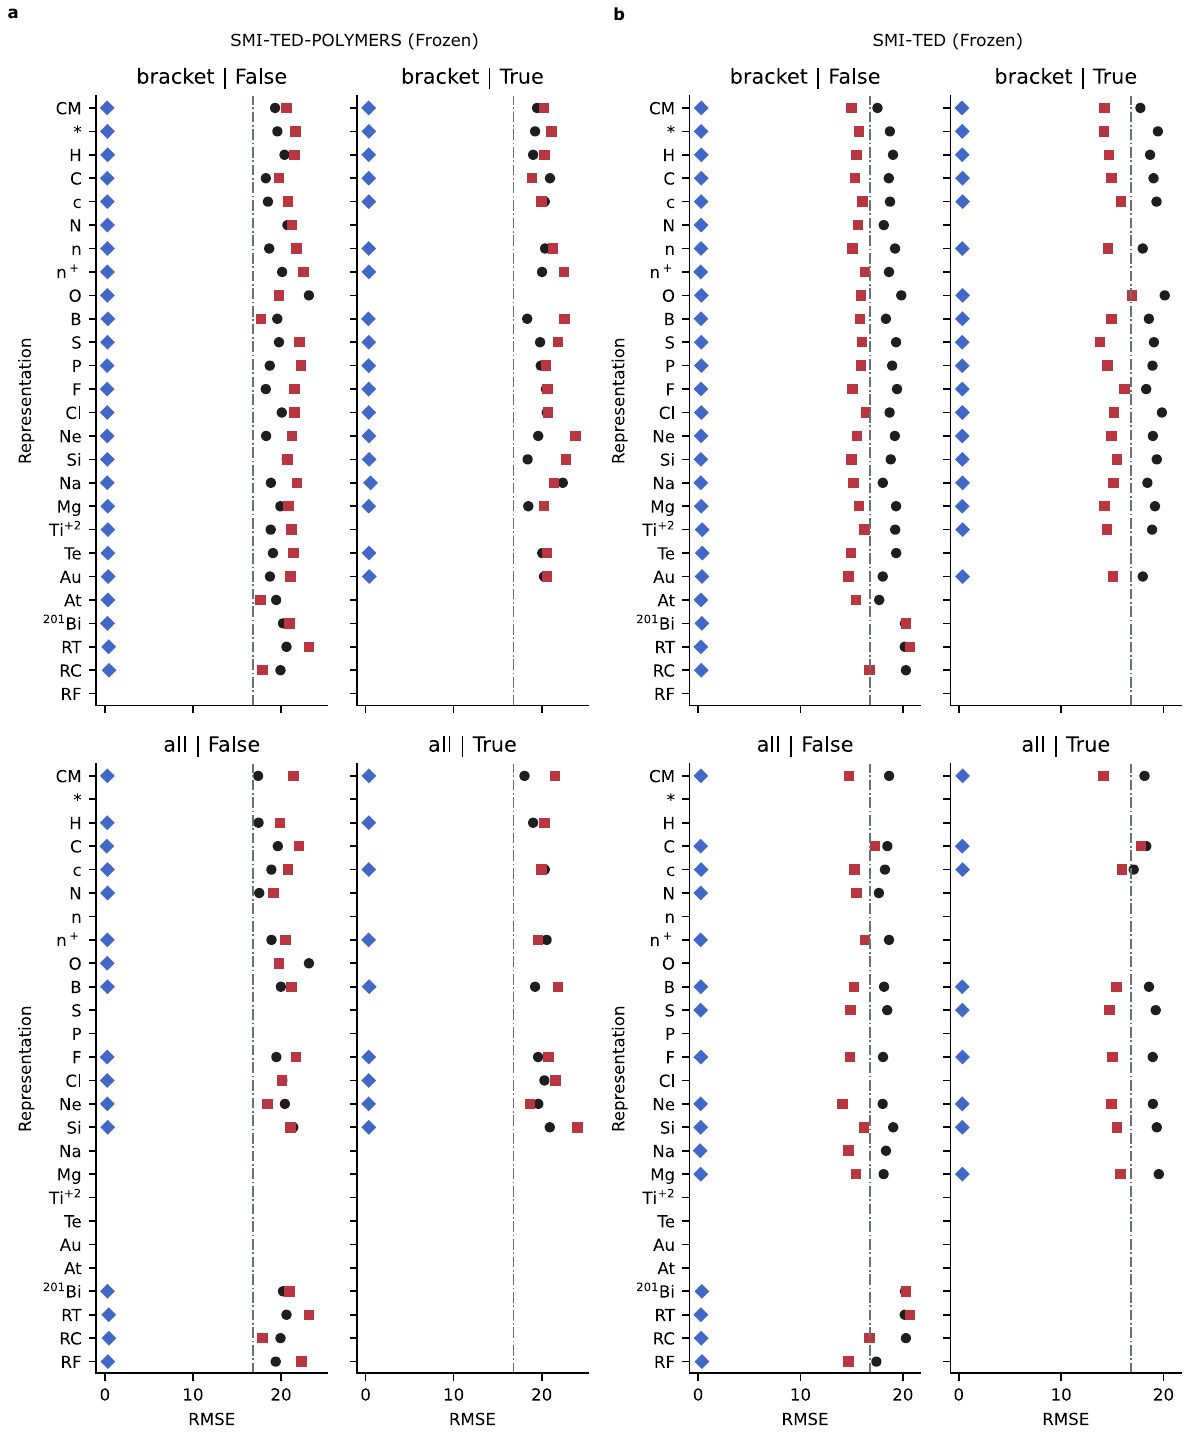}
\caption{Point plots for X\textsubscript{c} benchmark experiments of RMSE using the base random train, valid, and test splits for SMI-TED-POLYMER (\textbf{a}) and SMI-TED (\textbf{b}) models with frozen weights.}\label{xc_token_point_frozen_rmse}
\end{figure}

\begin{figure}[H]
\centering
\includegraphics[width=1\textwidth]{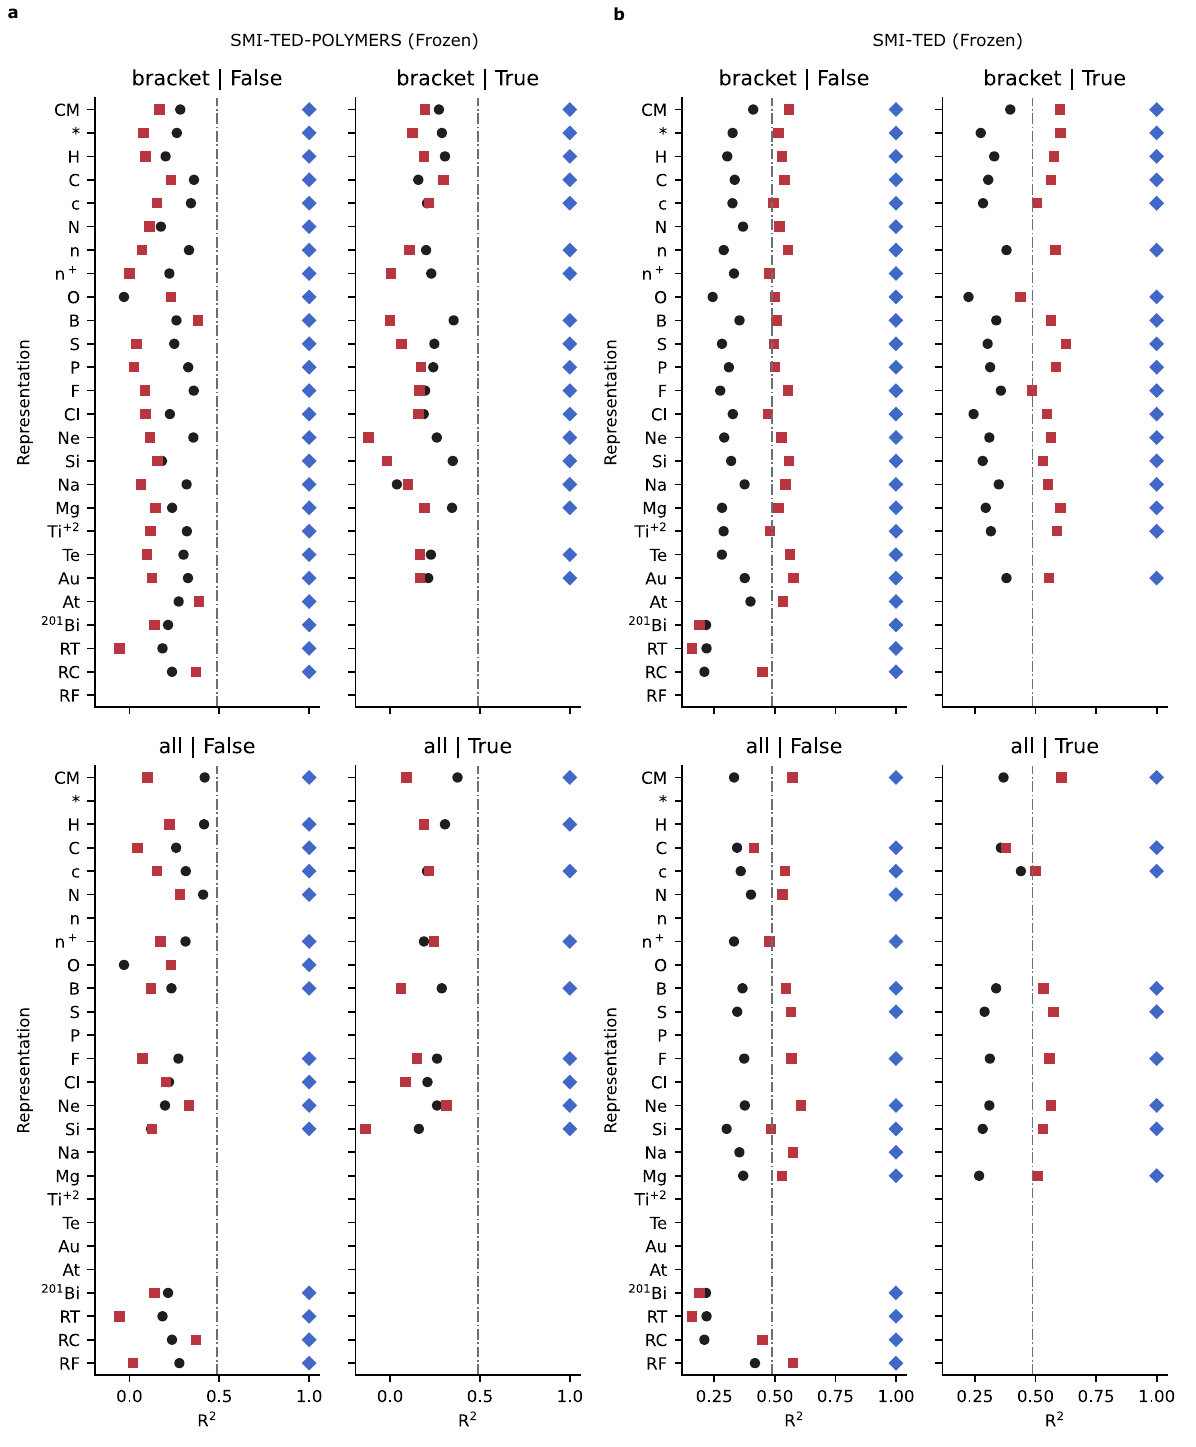}
\caption{Point plots for X\textsubscript{c} benchmark experiments of R\textsuperscript{2} using the base random train, valid, and test splits for SMI-TED-POLYMER (\textbf{a}) and SMI-TED (\textbf{b}) models with frozen weights.}\label{xc_token_point_frozen_r2}
\end{figure}

\begin{figure}[H]
\centering
\includegraphics[width=1\textwidth]{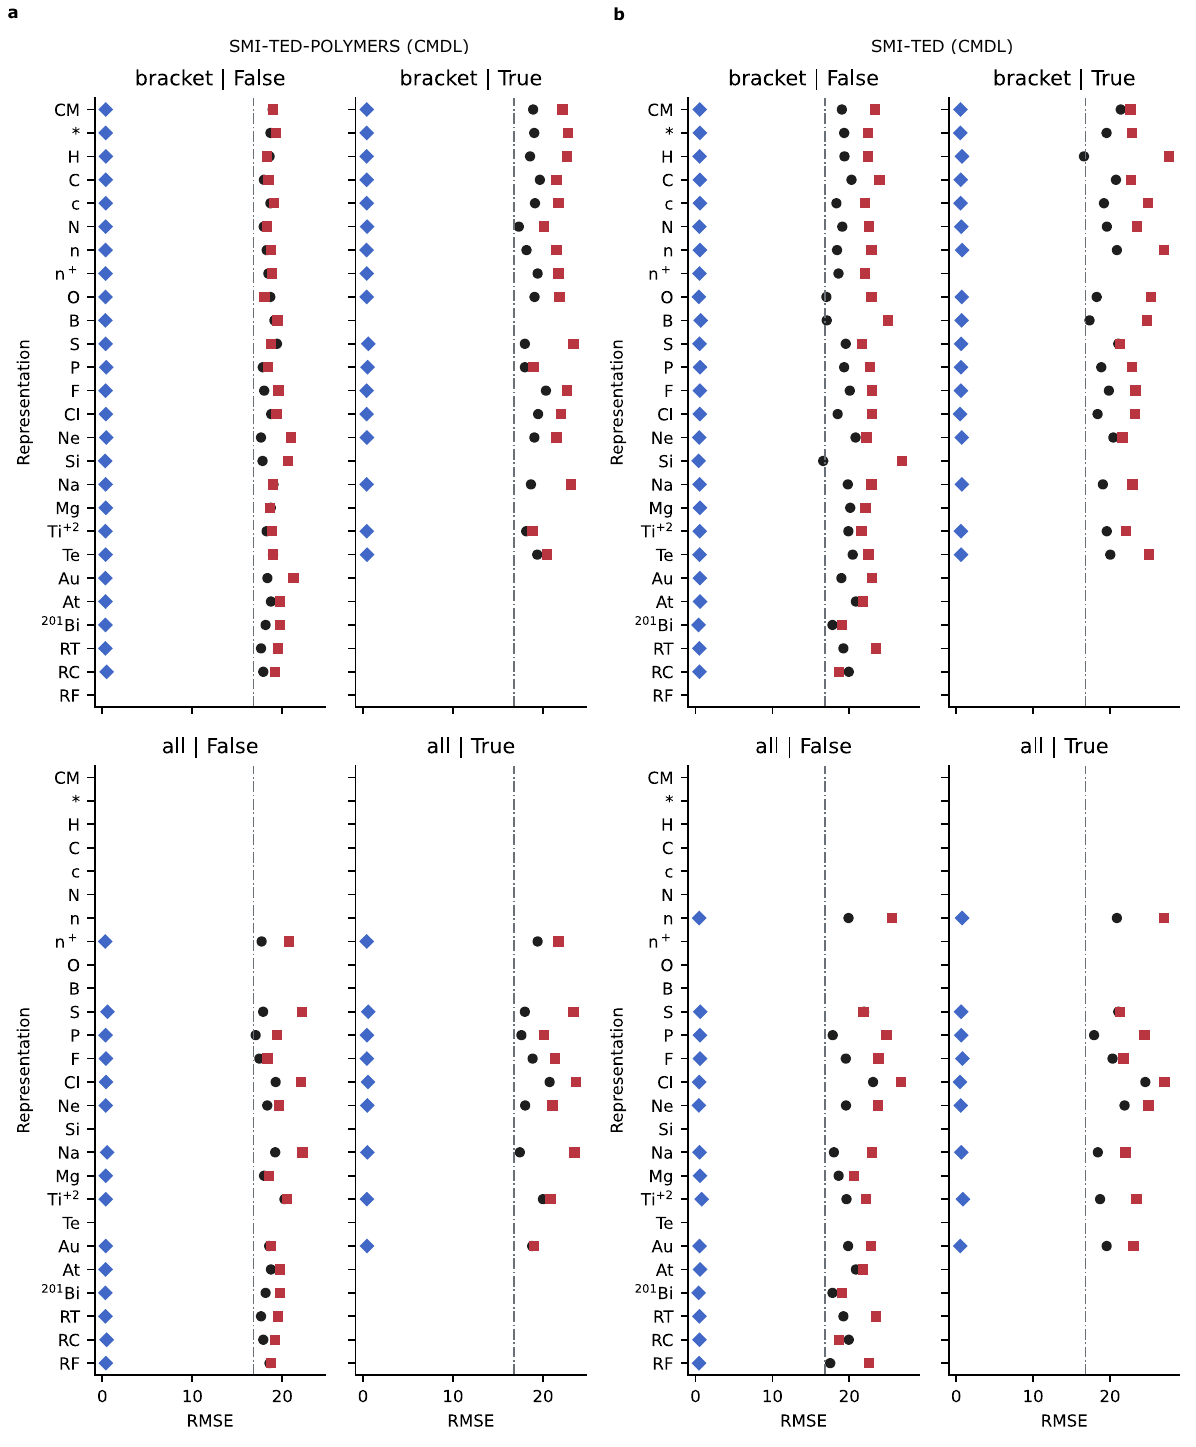}
\caption{Point plots for X\textsubscript{c} benchmark experiments of RMSE using the base random train, valid, and test splits for SMI-TED-POLYMER (\textbf{a}) and SMI-TED (\textbf{b}) models fine-tuned with CPG.}\label{xc_token_point_cmdl_rmse}
\end{figure}

\begin{figure}[H]
\centering
\includegraphics[width=1\textwidth]{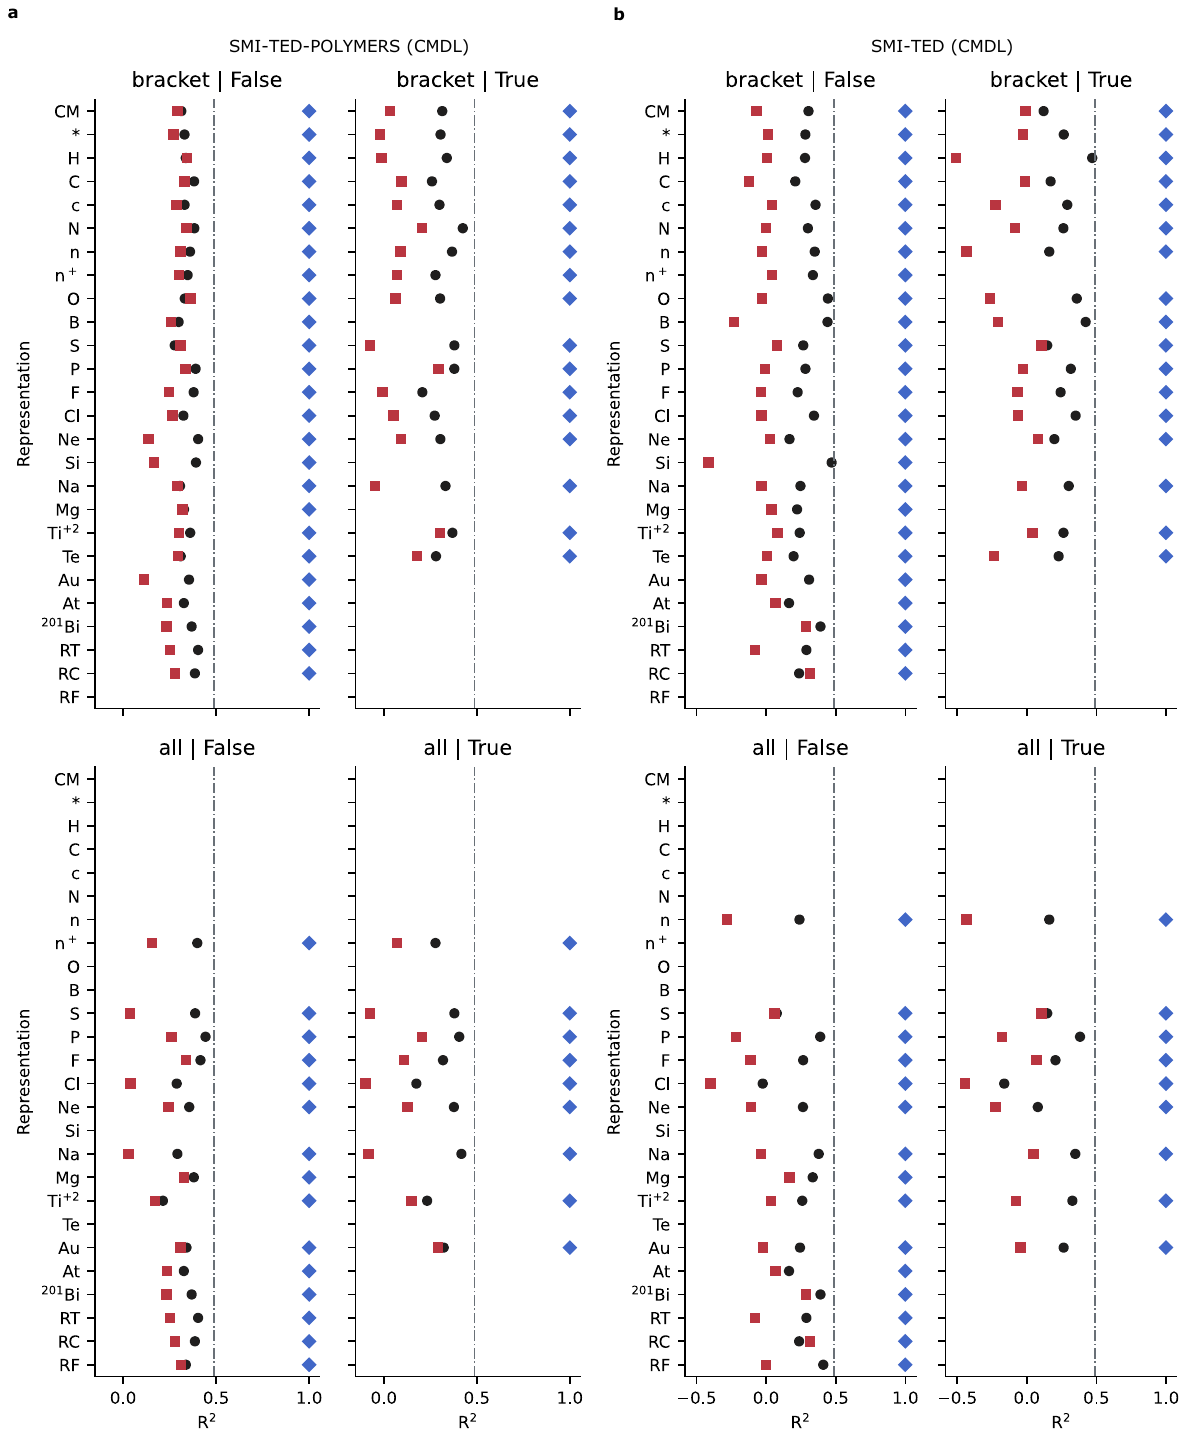}
\caption{Point plots for X\textsubscript{c} benchmark experiments of R\textsuperscript{2} using the base random train, valid, and test splits for SMI-TED-POLYMER (\textbf{a}) and SMI-TED (\textbf{b}) models fine-tuned with CPG.}\label{xc_token_point_cmdl_r2}
\end{figure}

\begin{figure}[H]
\centering
\includegraphics[width=1\textwidth]{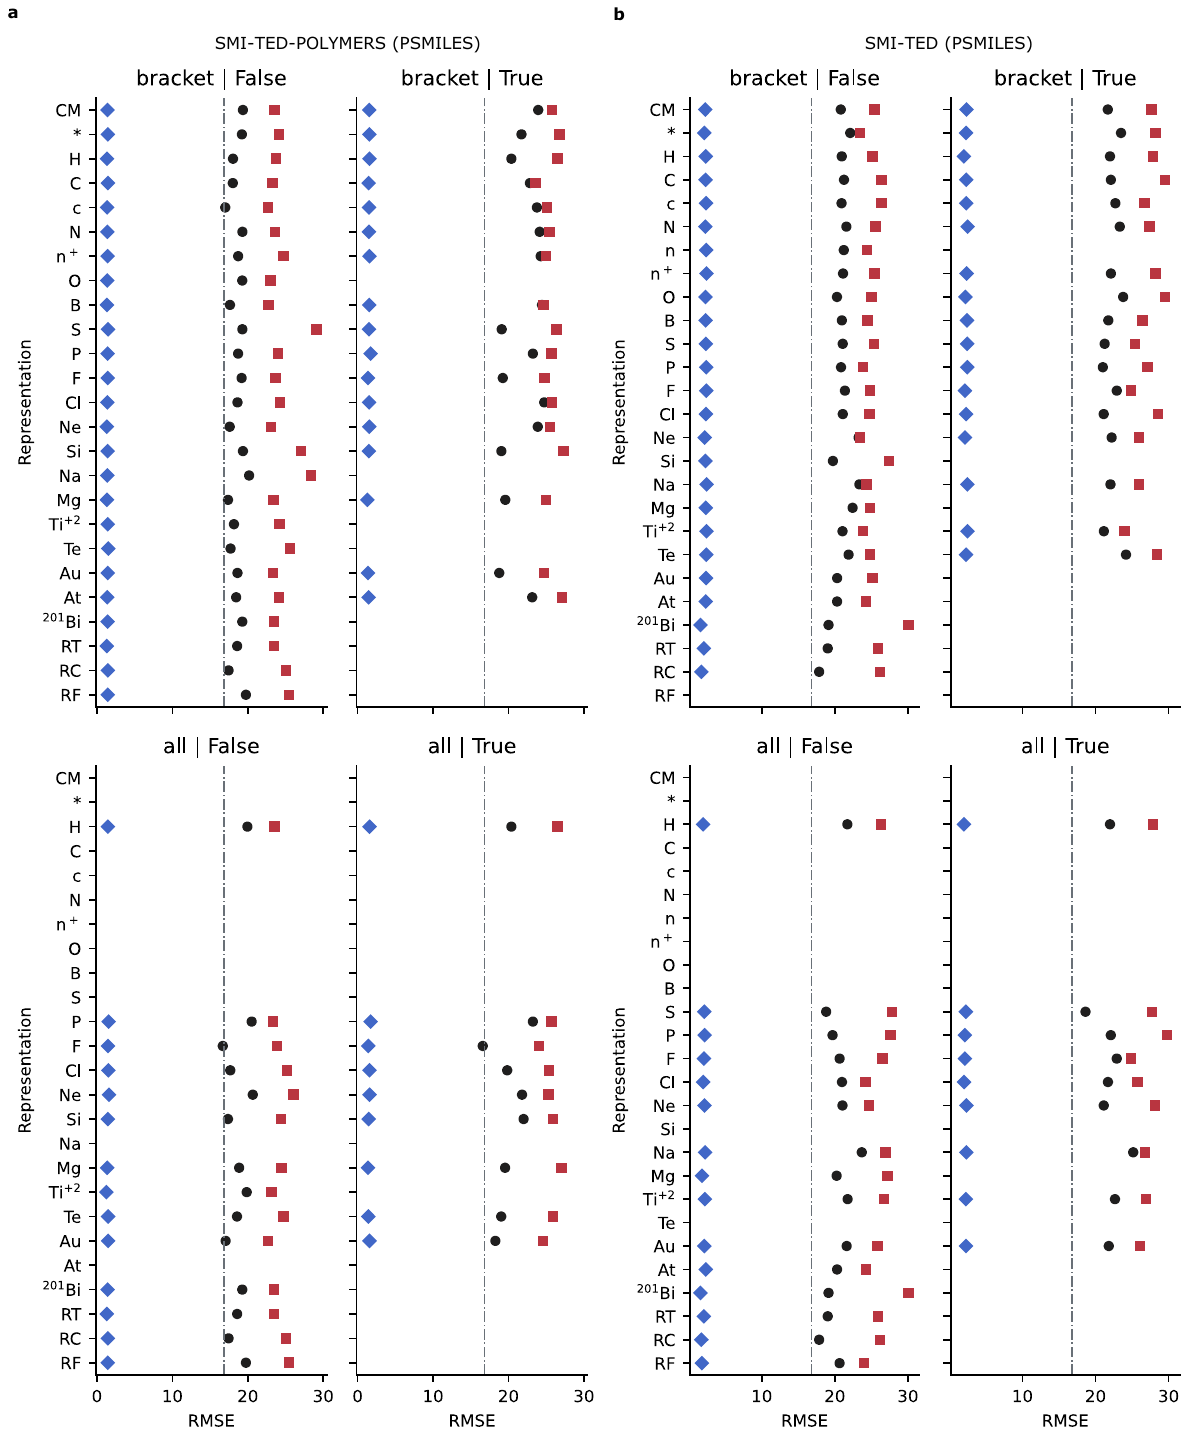}
\caption{Point plots for X\textsubscript{c} benchmark experiments of RMSE using the base random train, valid, and test splits for SMI-TED-POLYMER (\textbf{a}) and SMI-TED (\textbf{b}) models fine-tuned with PSMILES.}\label{xc_token_point_psmiles_rmse}
\end{figure}

\begin{figure}[H]
\centering
\includegraphics[width=1\textwidth]{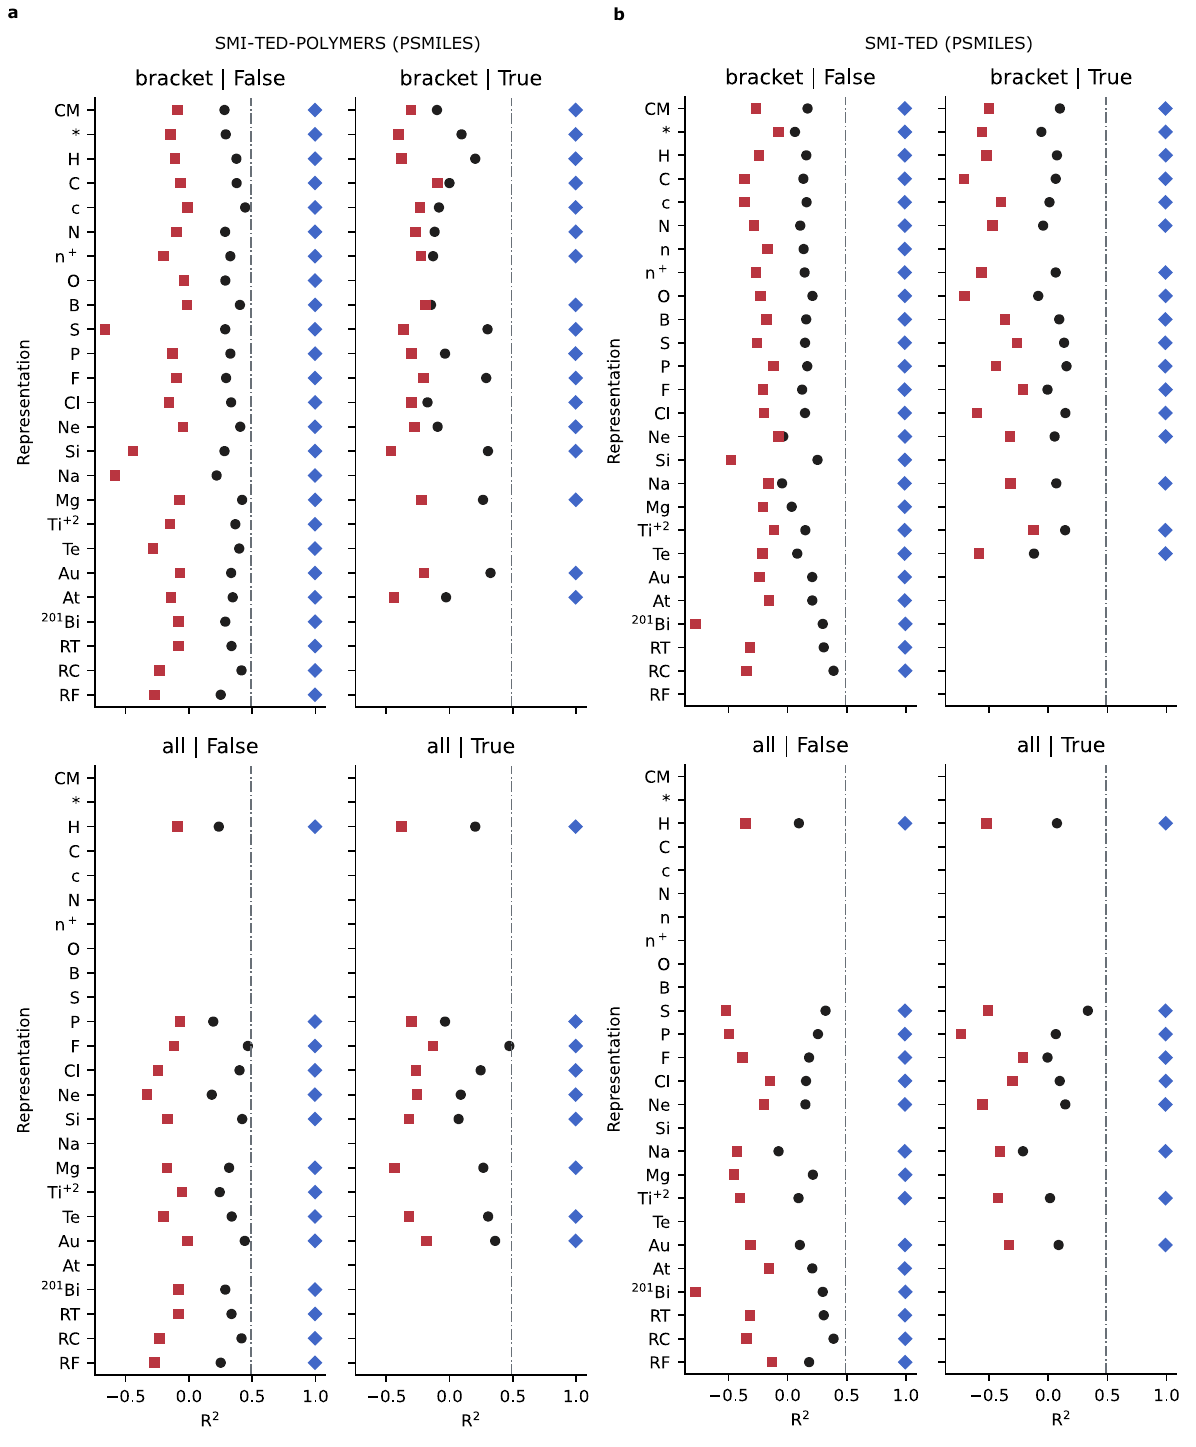}
\caption{Point plots for X\textsubscript{c} benchmark experiments of R\textsuperscript{2} using the base random train, valid, and test splits for SMI-TED-POLYMER (\textbf{a}) and SMI-TED (\textbf{b}) models fine-tuned with PSMILES.}\label{xc_token_point_psmiles_r2}
\end{figure}
